# Supplementary material for: Likelihood-based meta-analysis with few studies: Empirical and simulation studies
Source: arXiv:1807.09037 source file (2018-10-30)
Supplement: Supplementary file 1 [file Supplement-1.pdf]

RR  
( $n_i=25, \pi_0=0.1$ )

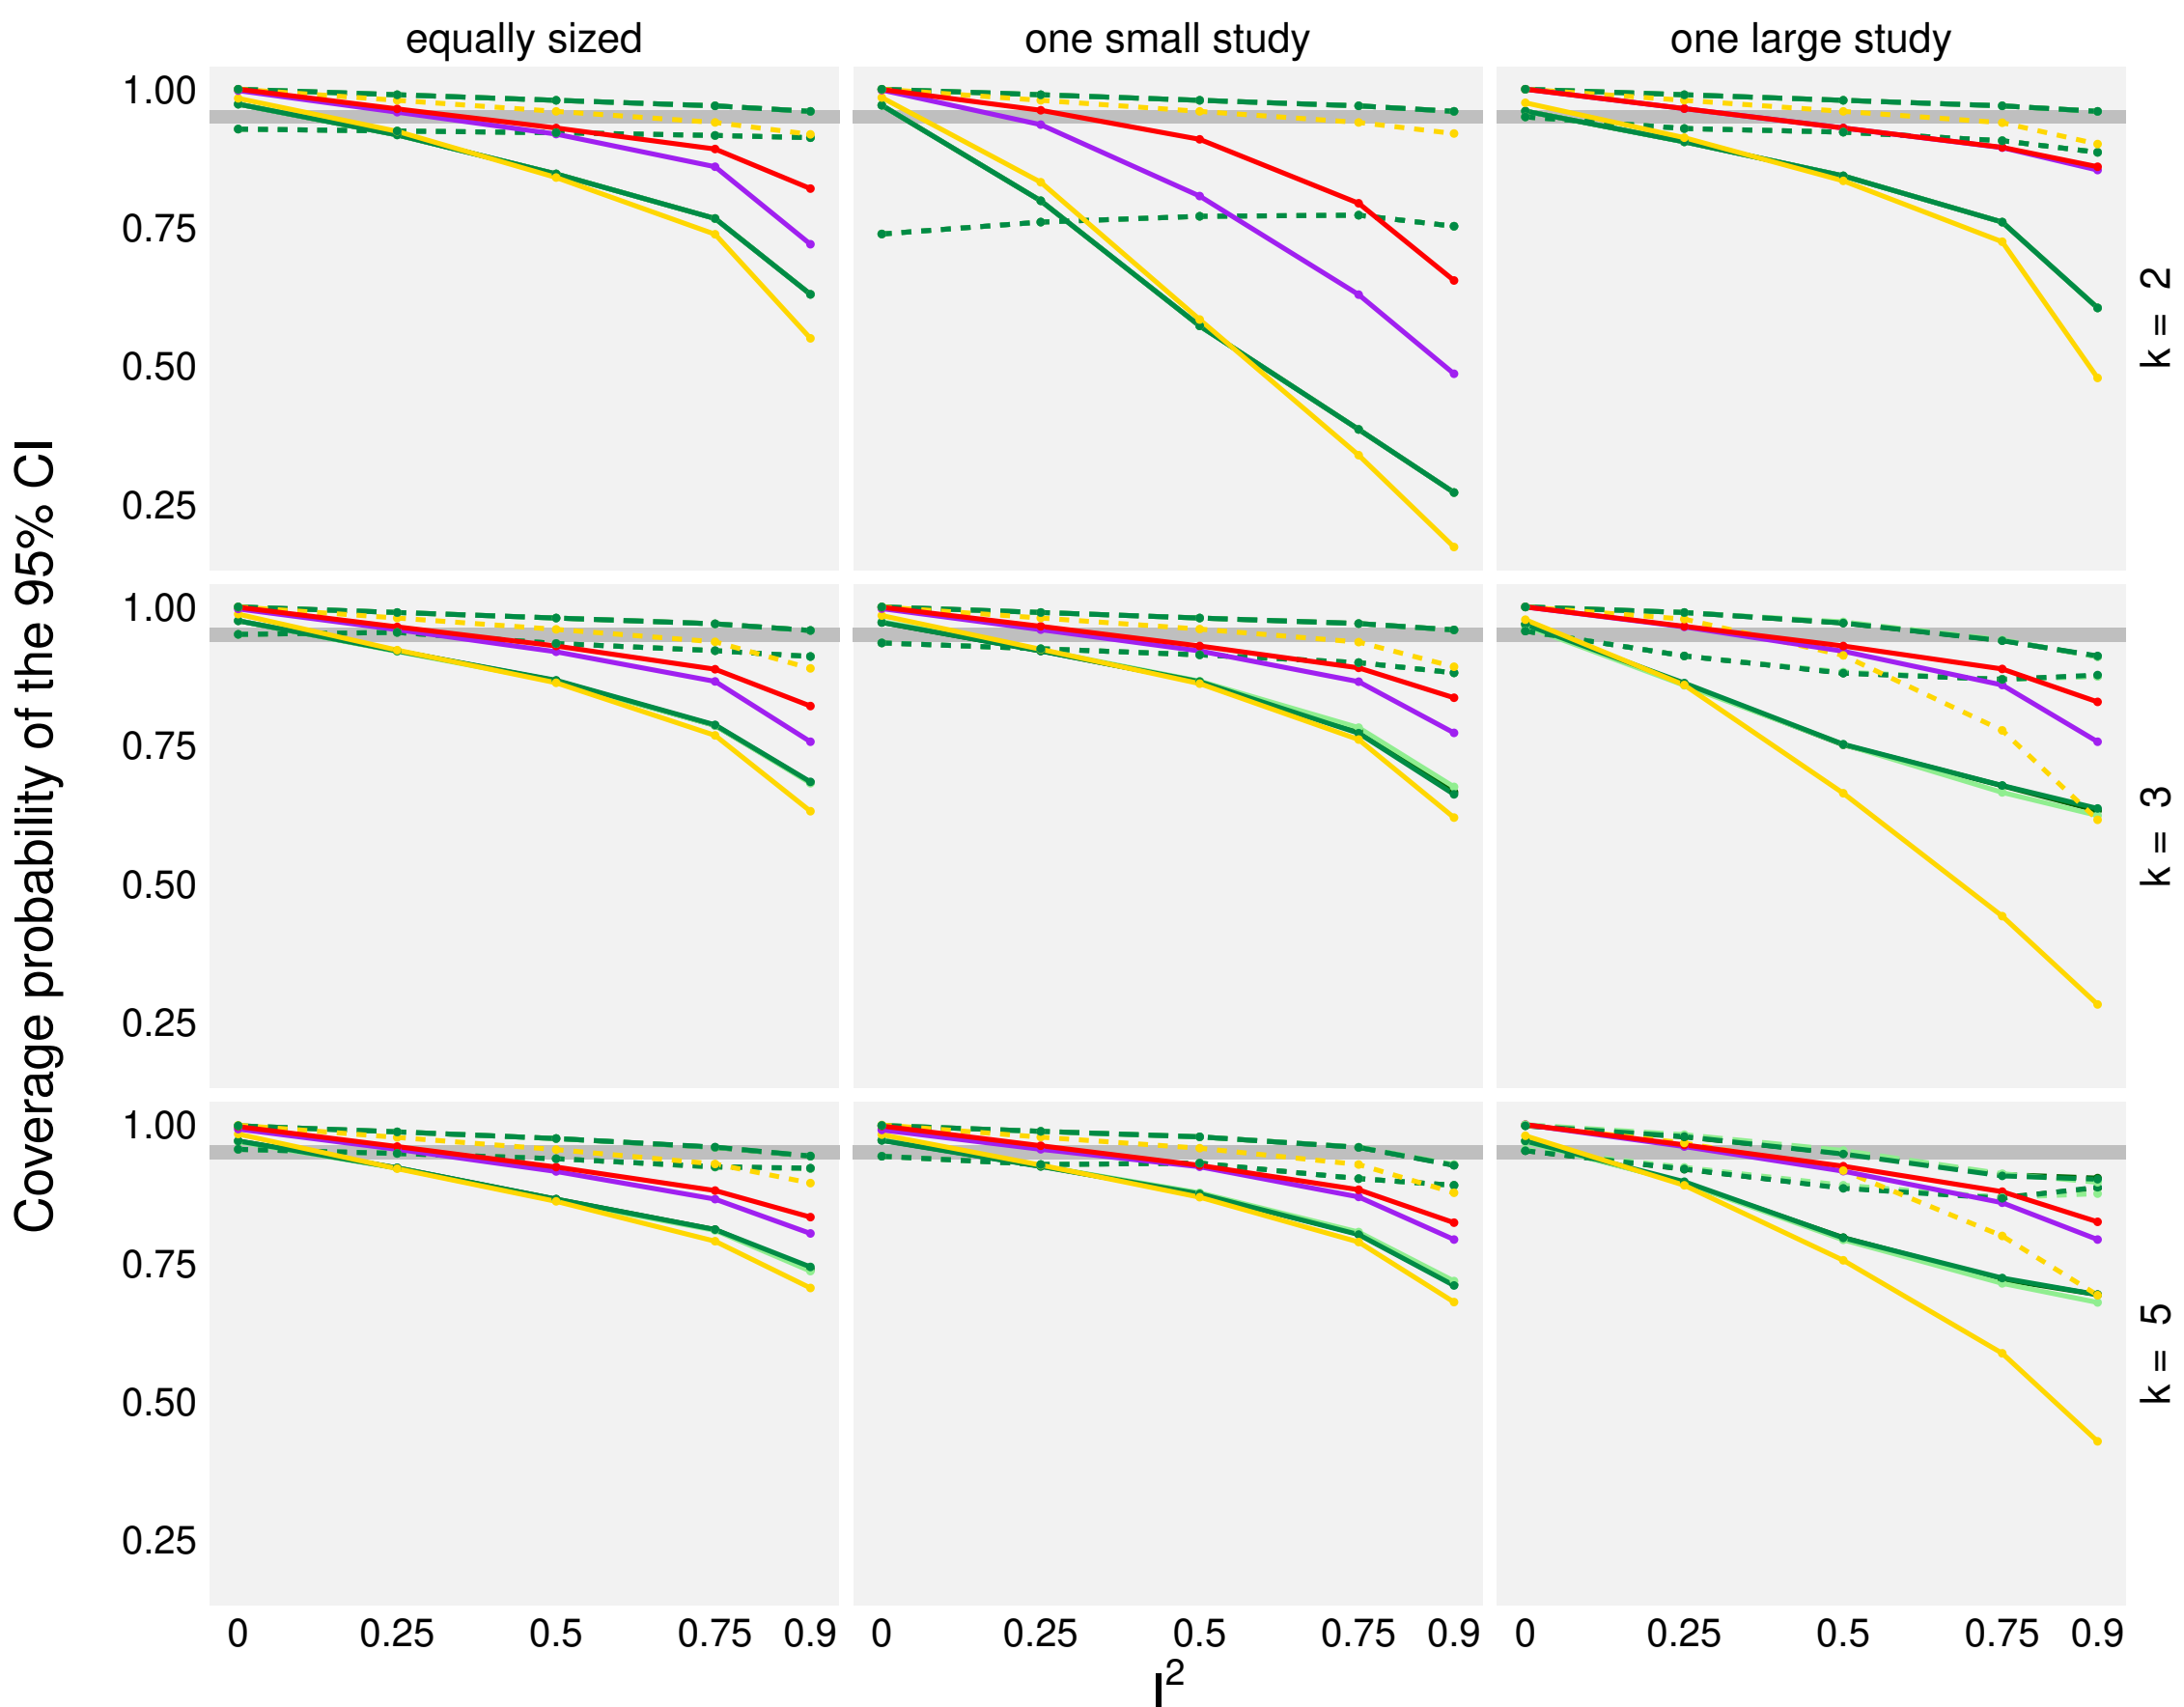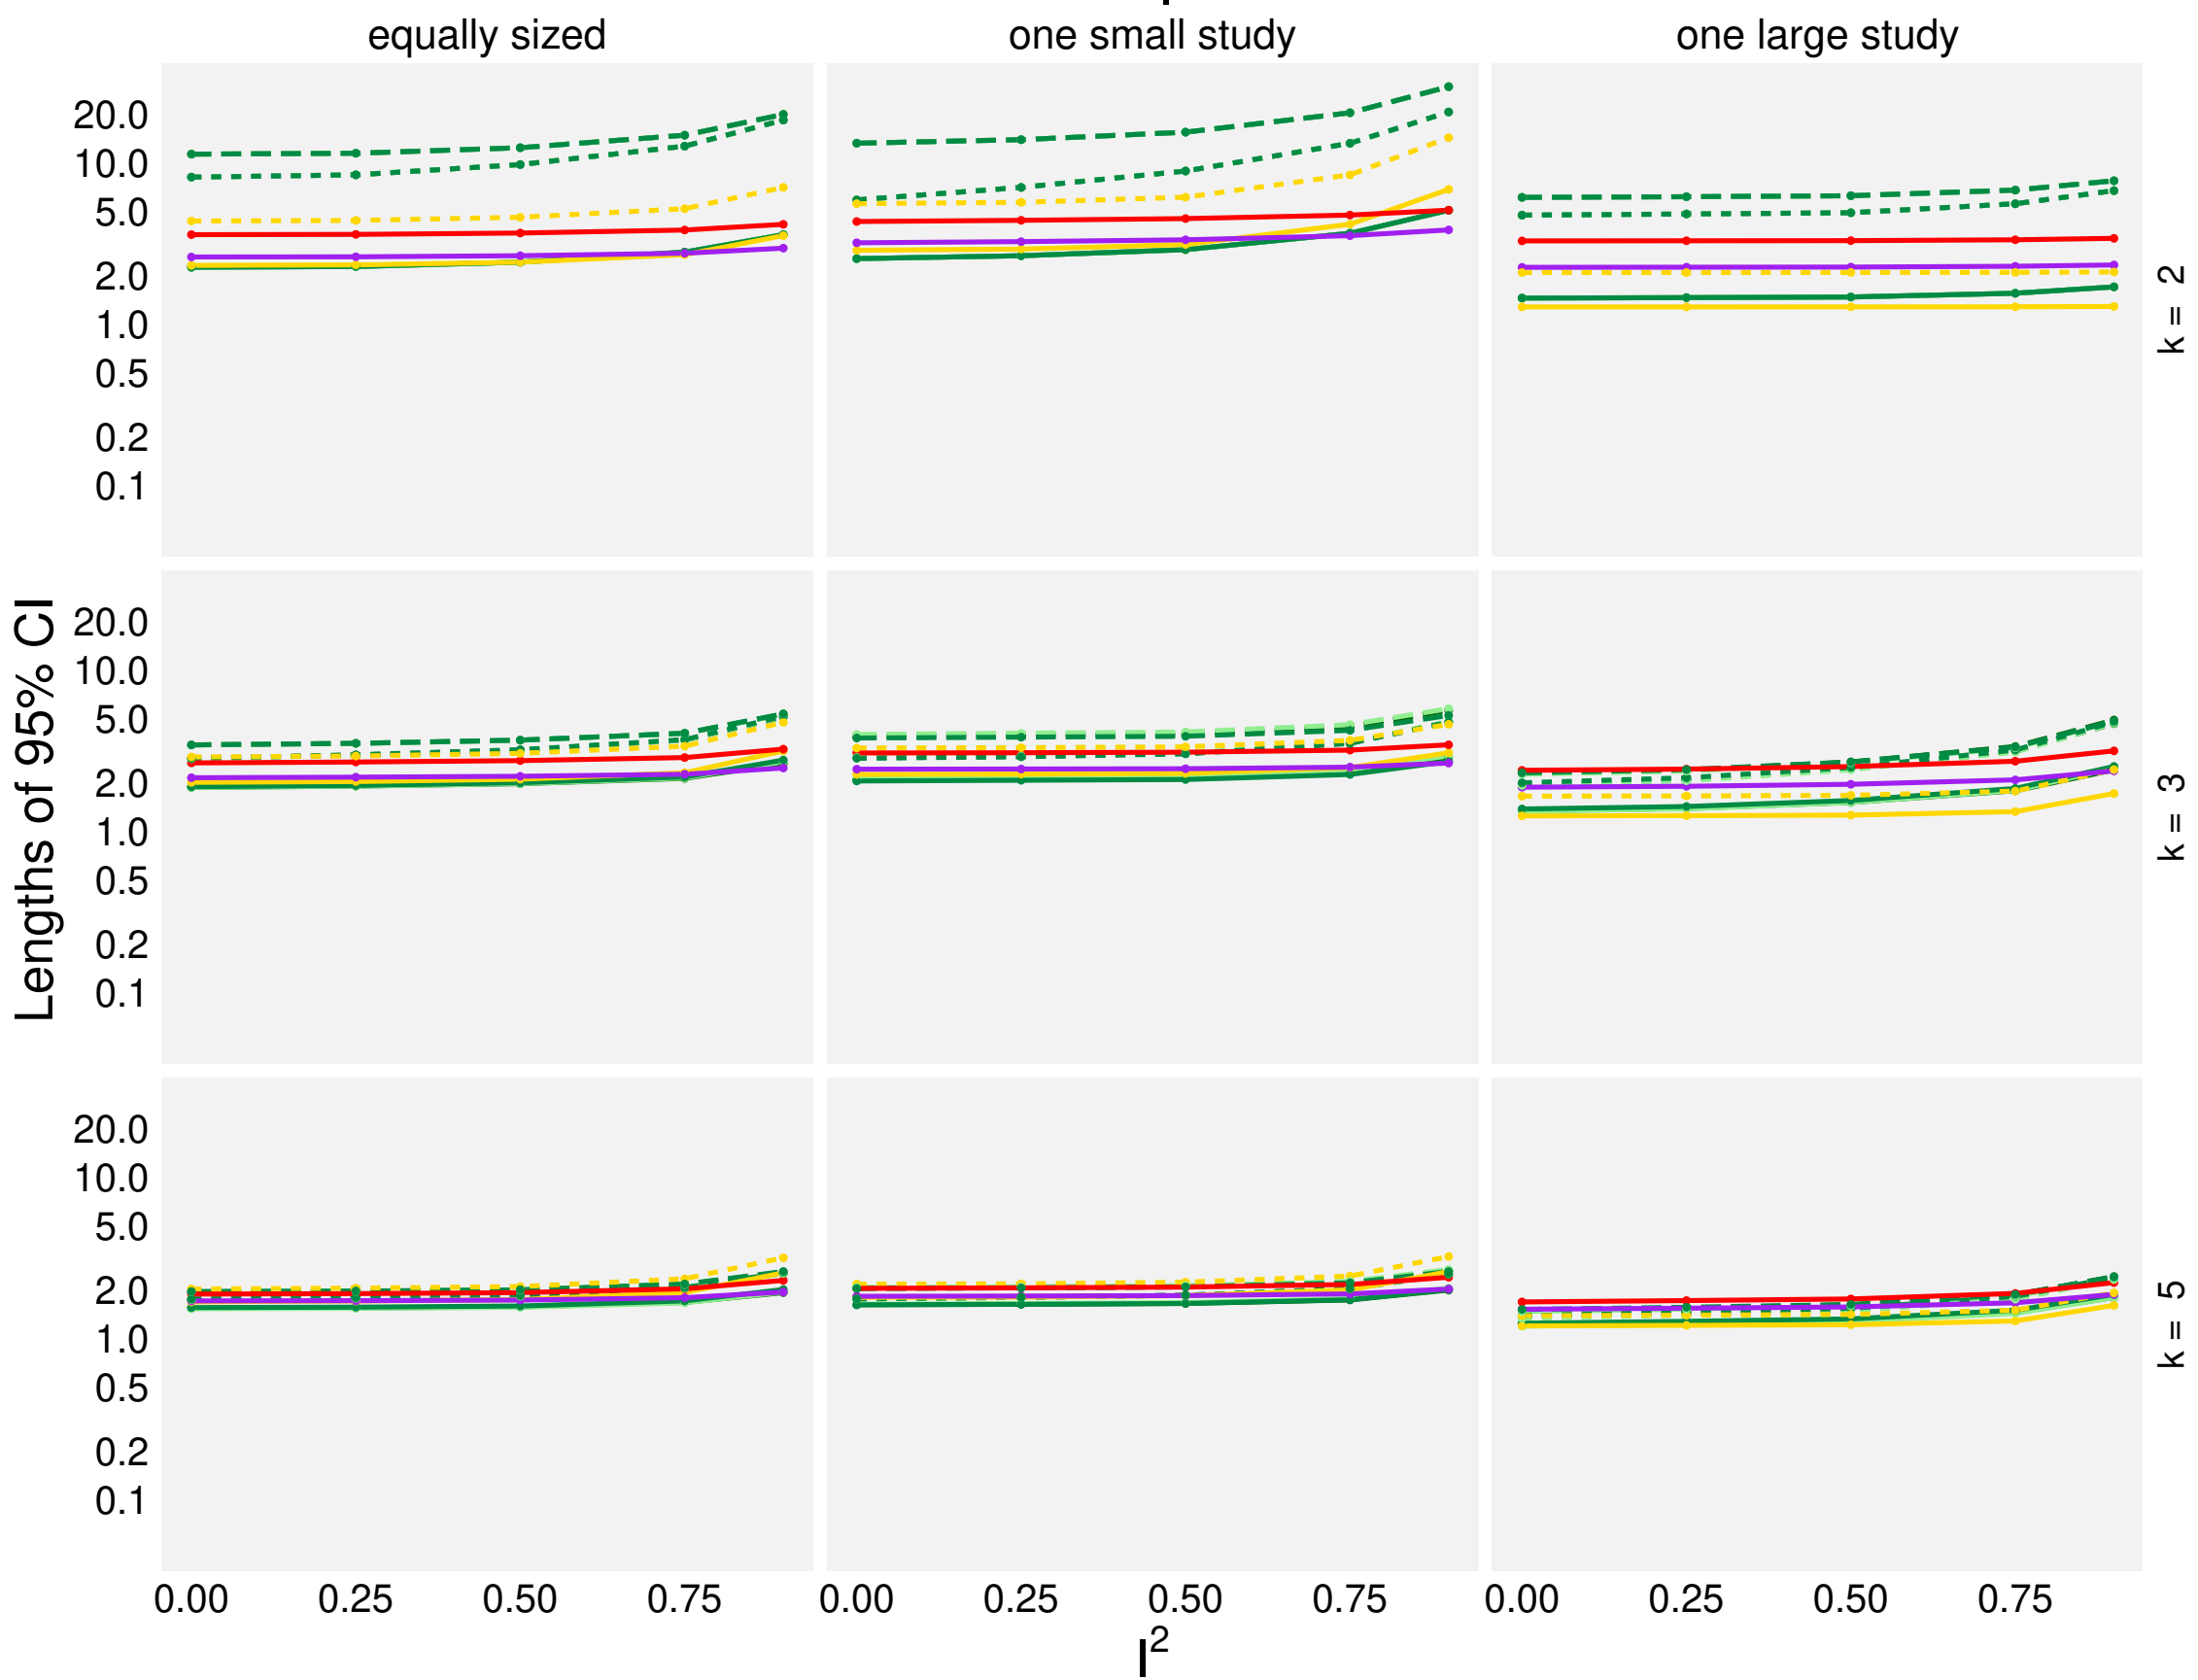

— NN — DL      — PN — PL      — normal quantiles  
 — NN — REML      — NN — Bayes HN(0.5)      - - HKSJ or Student's t  
 — NN — EB      — NN — Bayes HN(1)      - - mHKSJ

RR  
( $n_i=25, \pi_0=0.3$ )

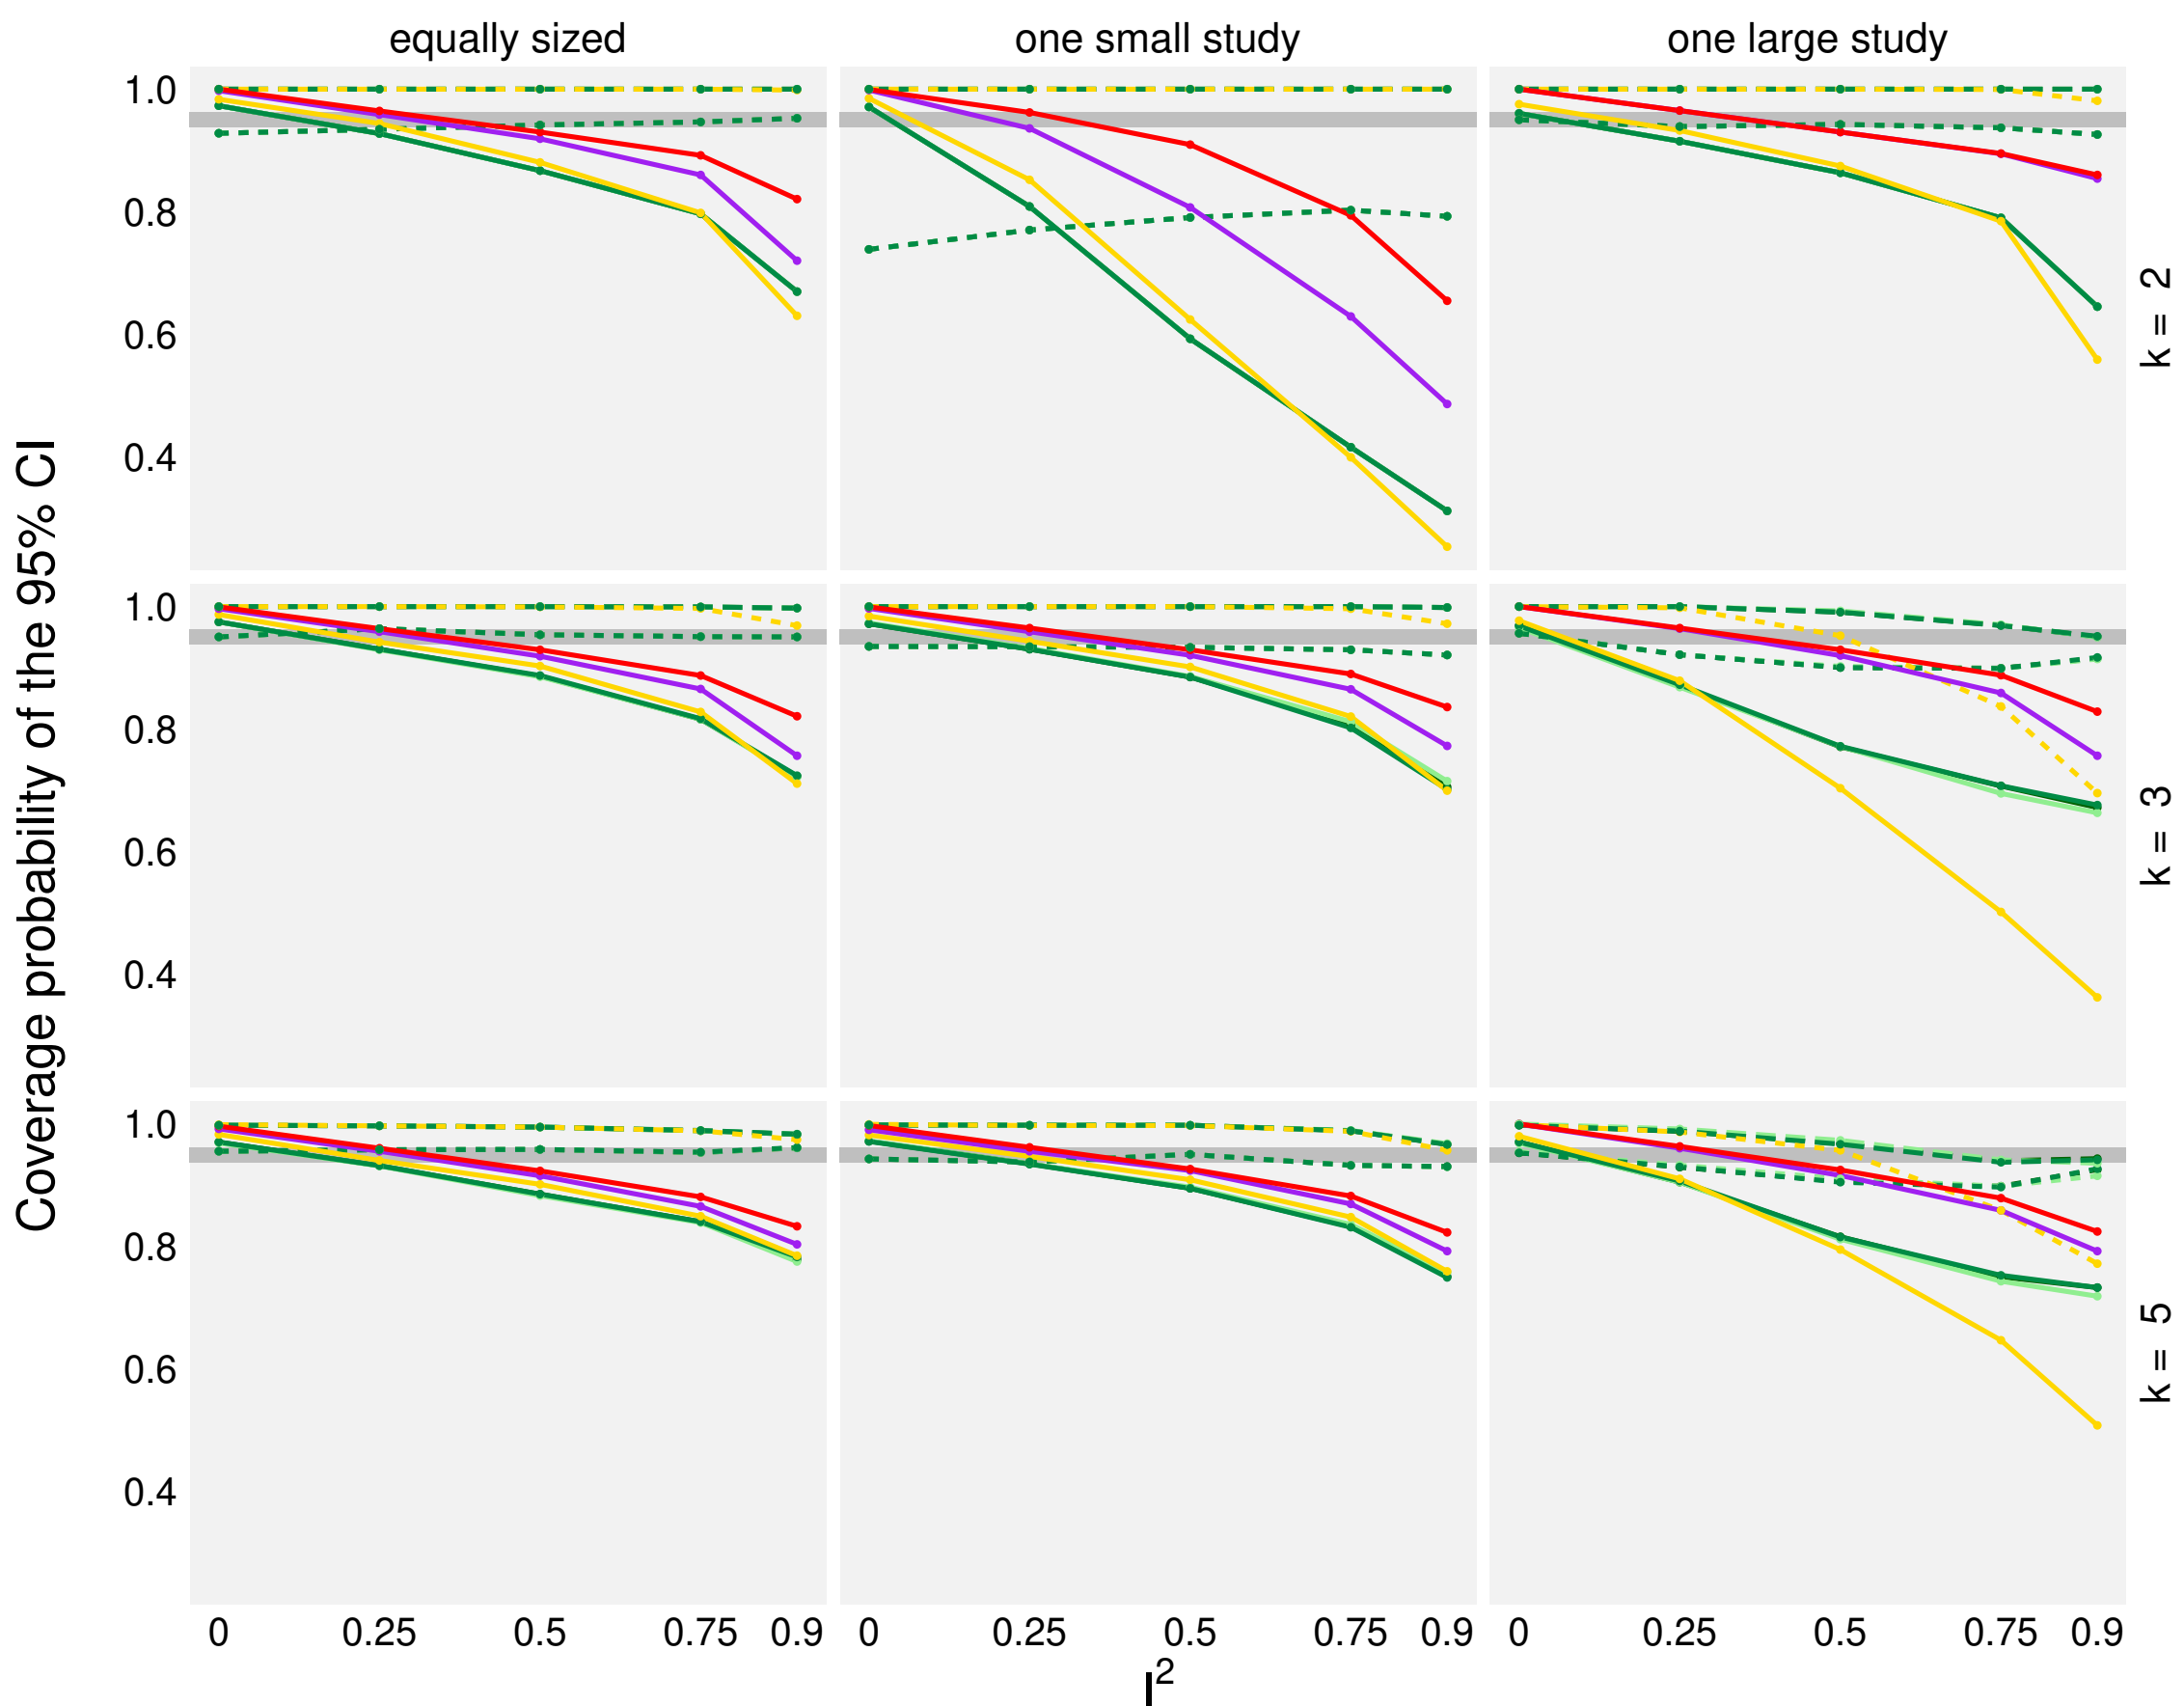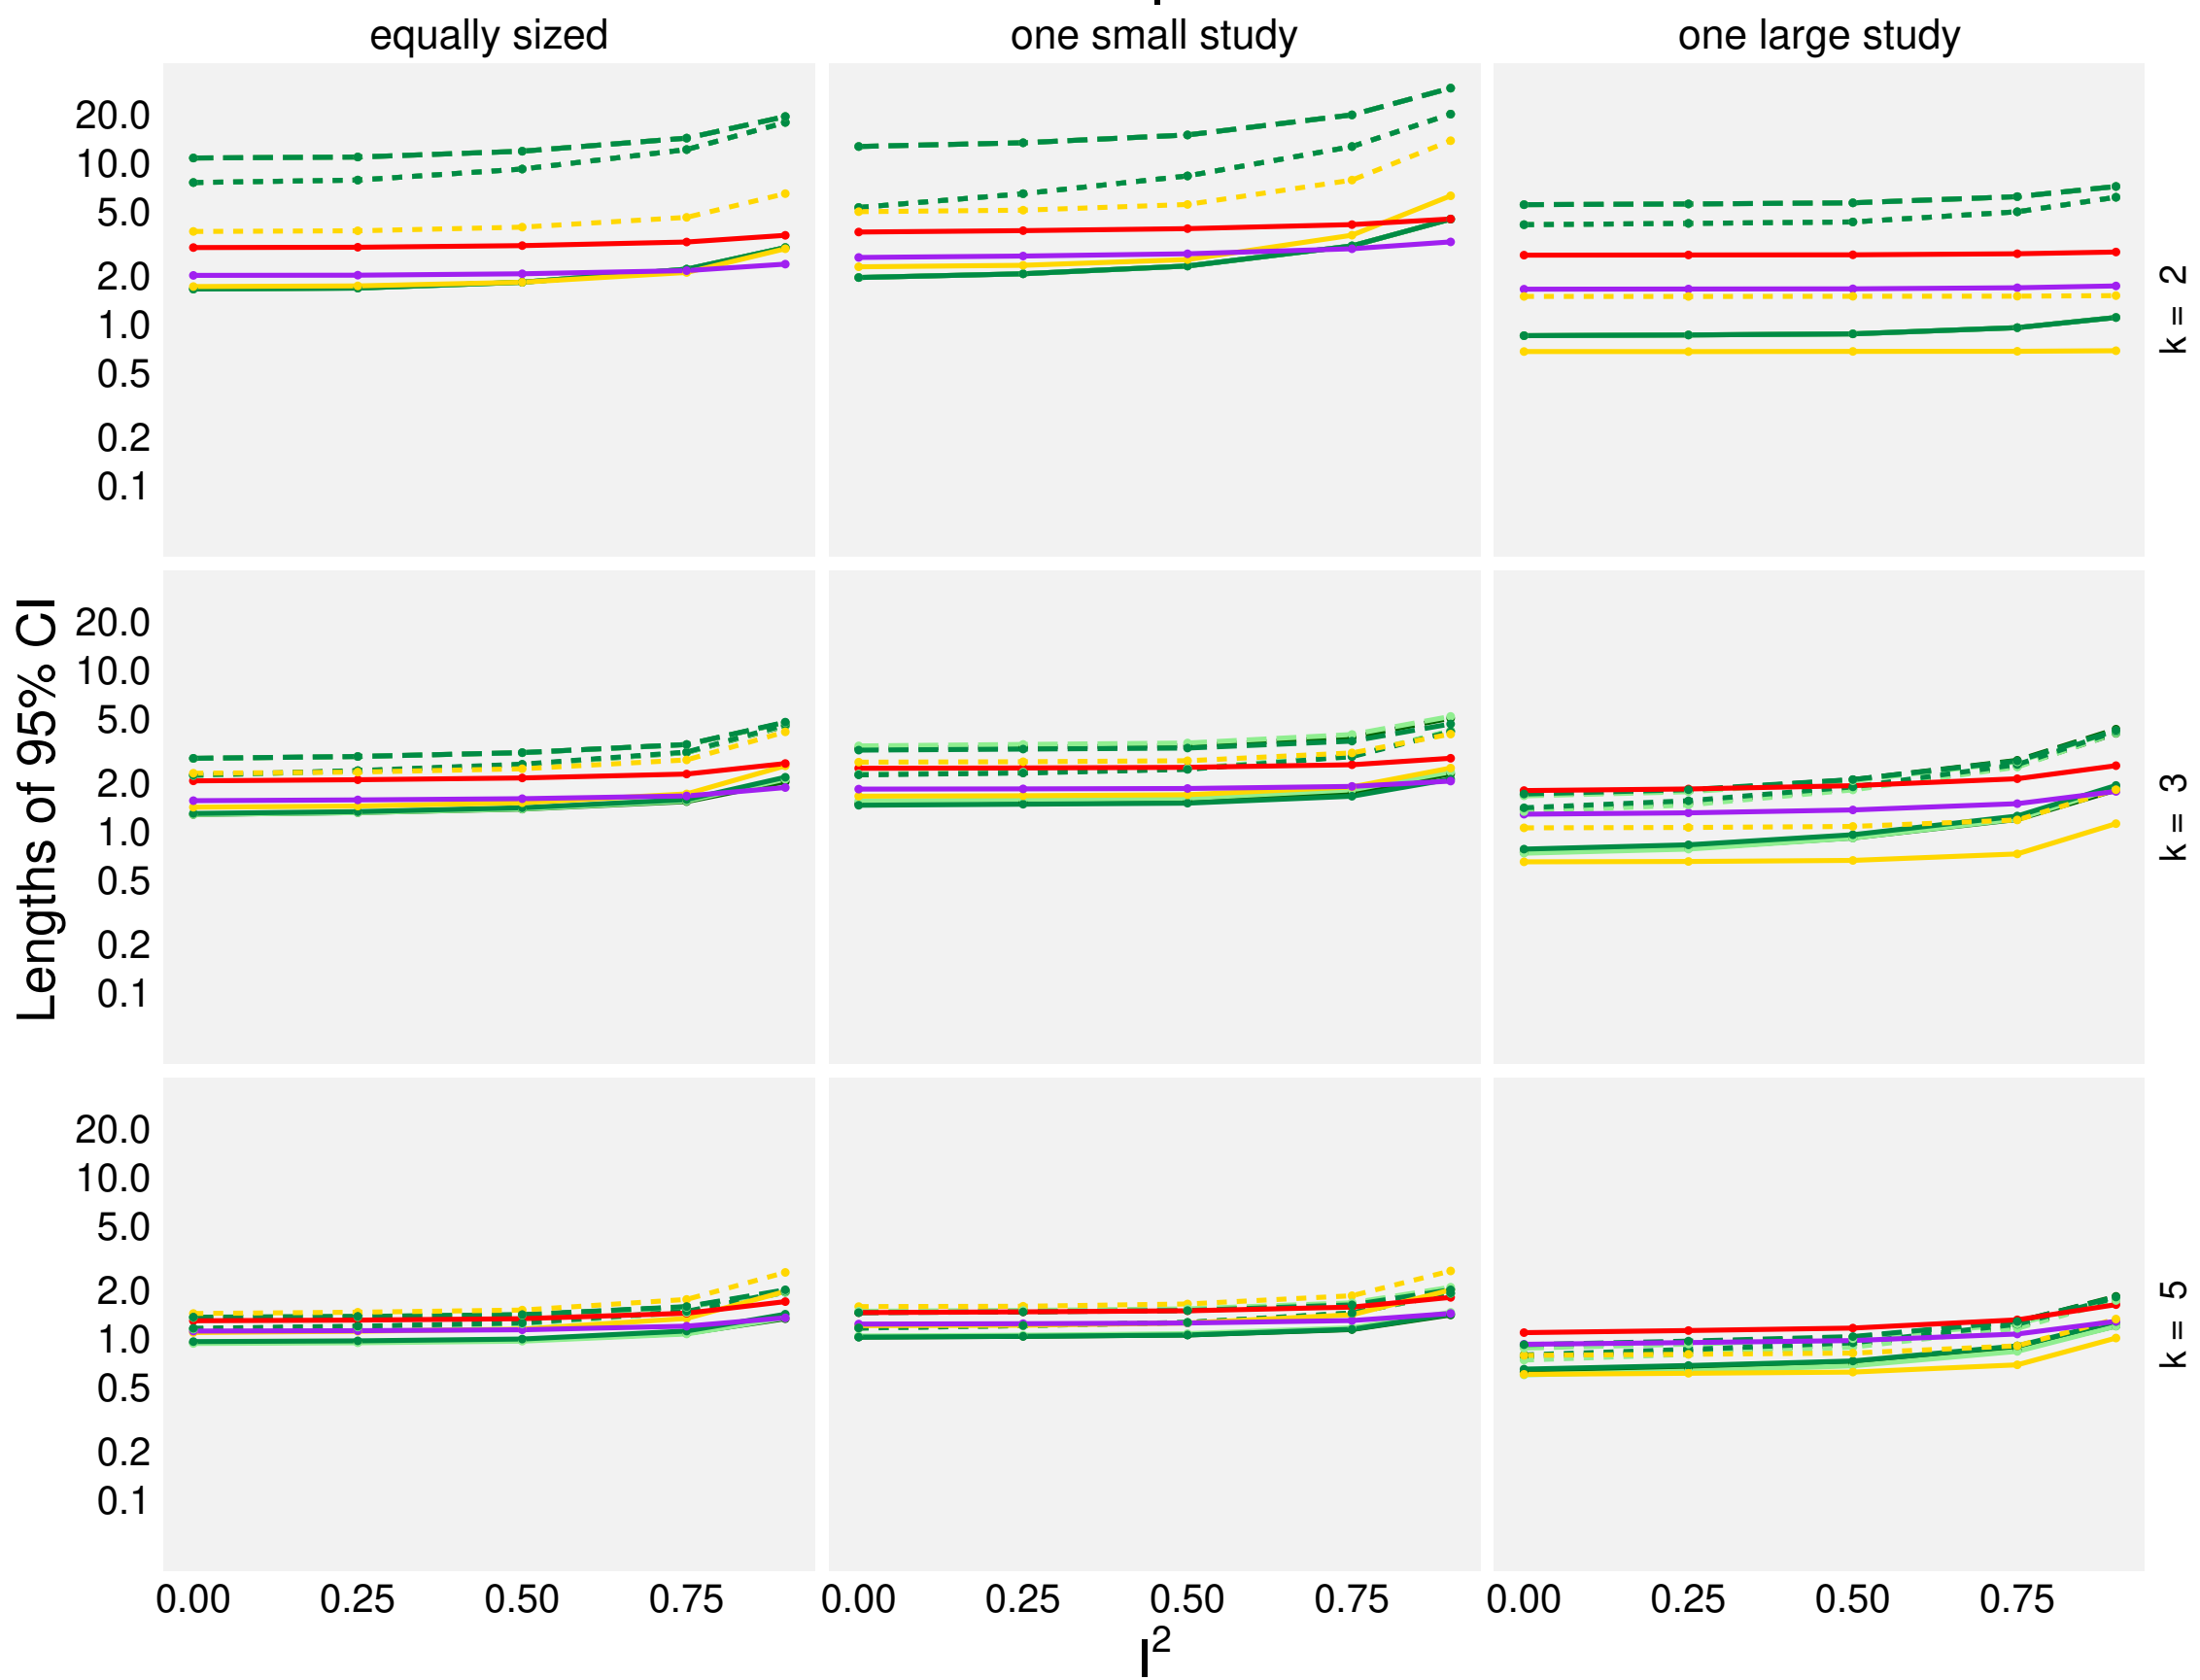

— NN – DL      — PN – PL      — normal quantiles  
 — NN – REML      — NN – Bayes HN(0.5)      - - HKSJ or Student's t  
 — NN – EB      — NN – Bayes HN(1)      - - mHKSJ

RR  
( $n_i=25, \pi_0=0.5$ )

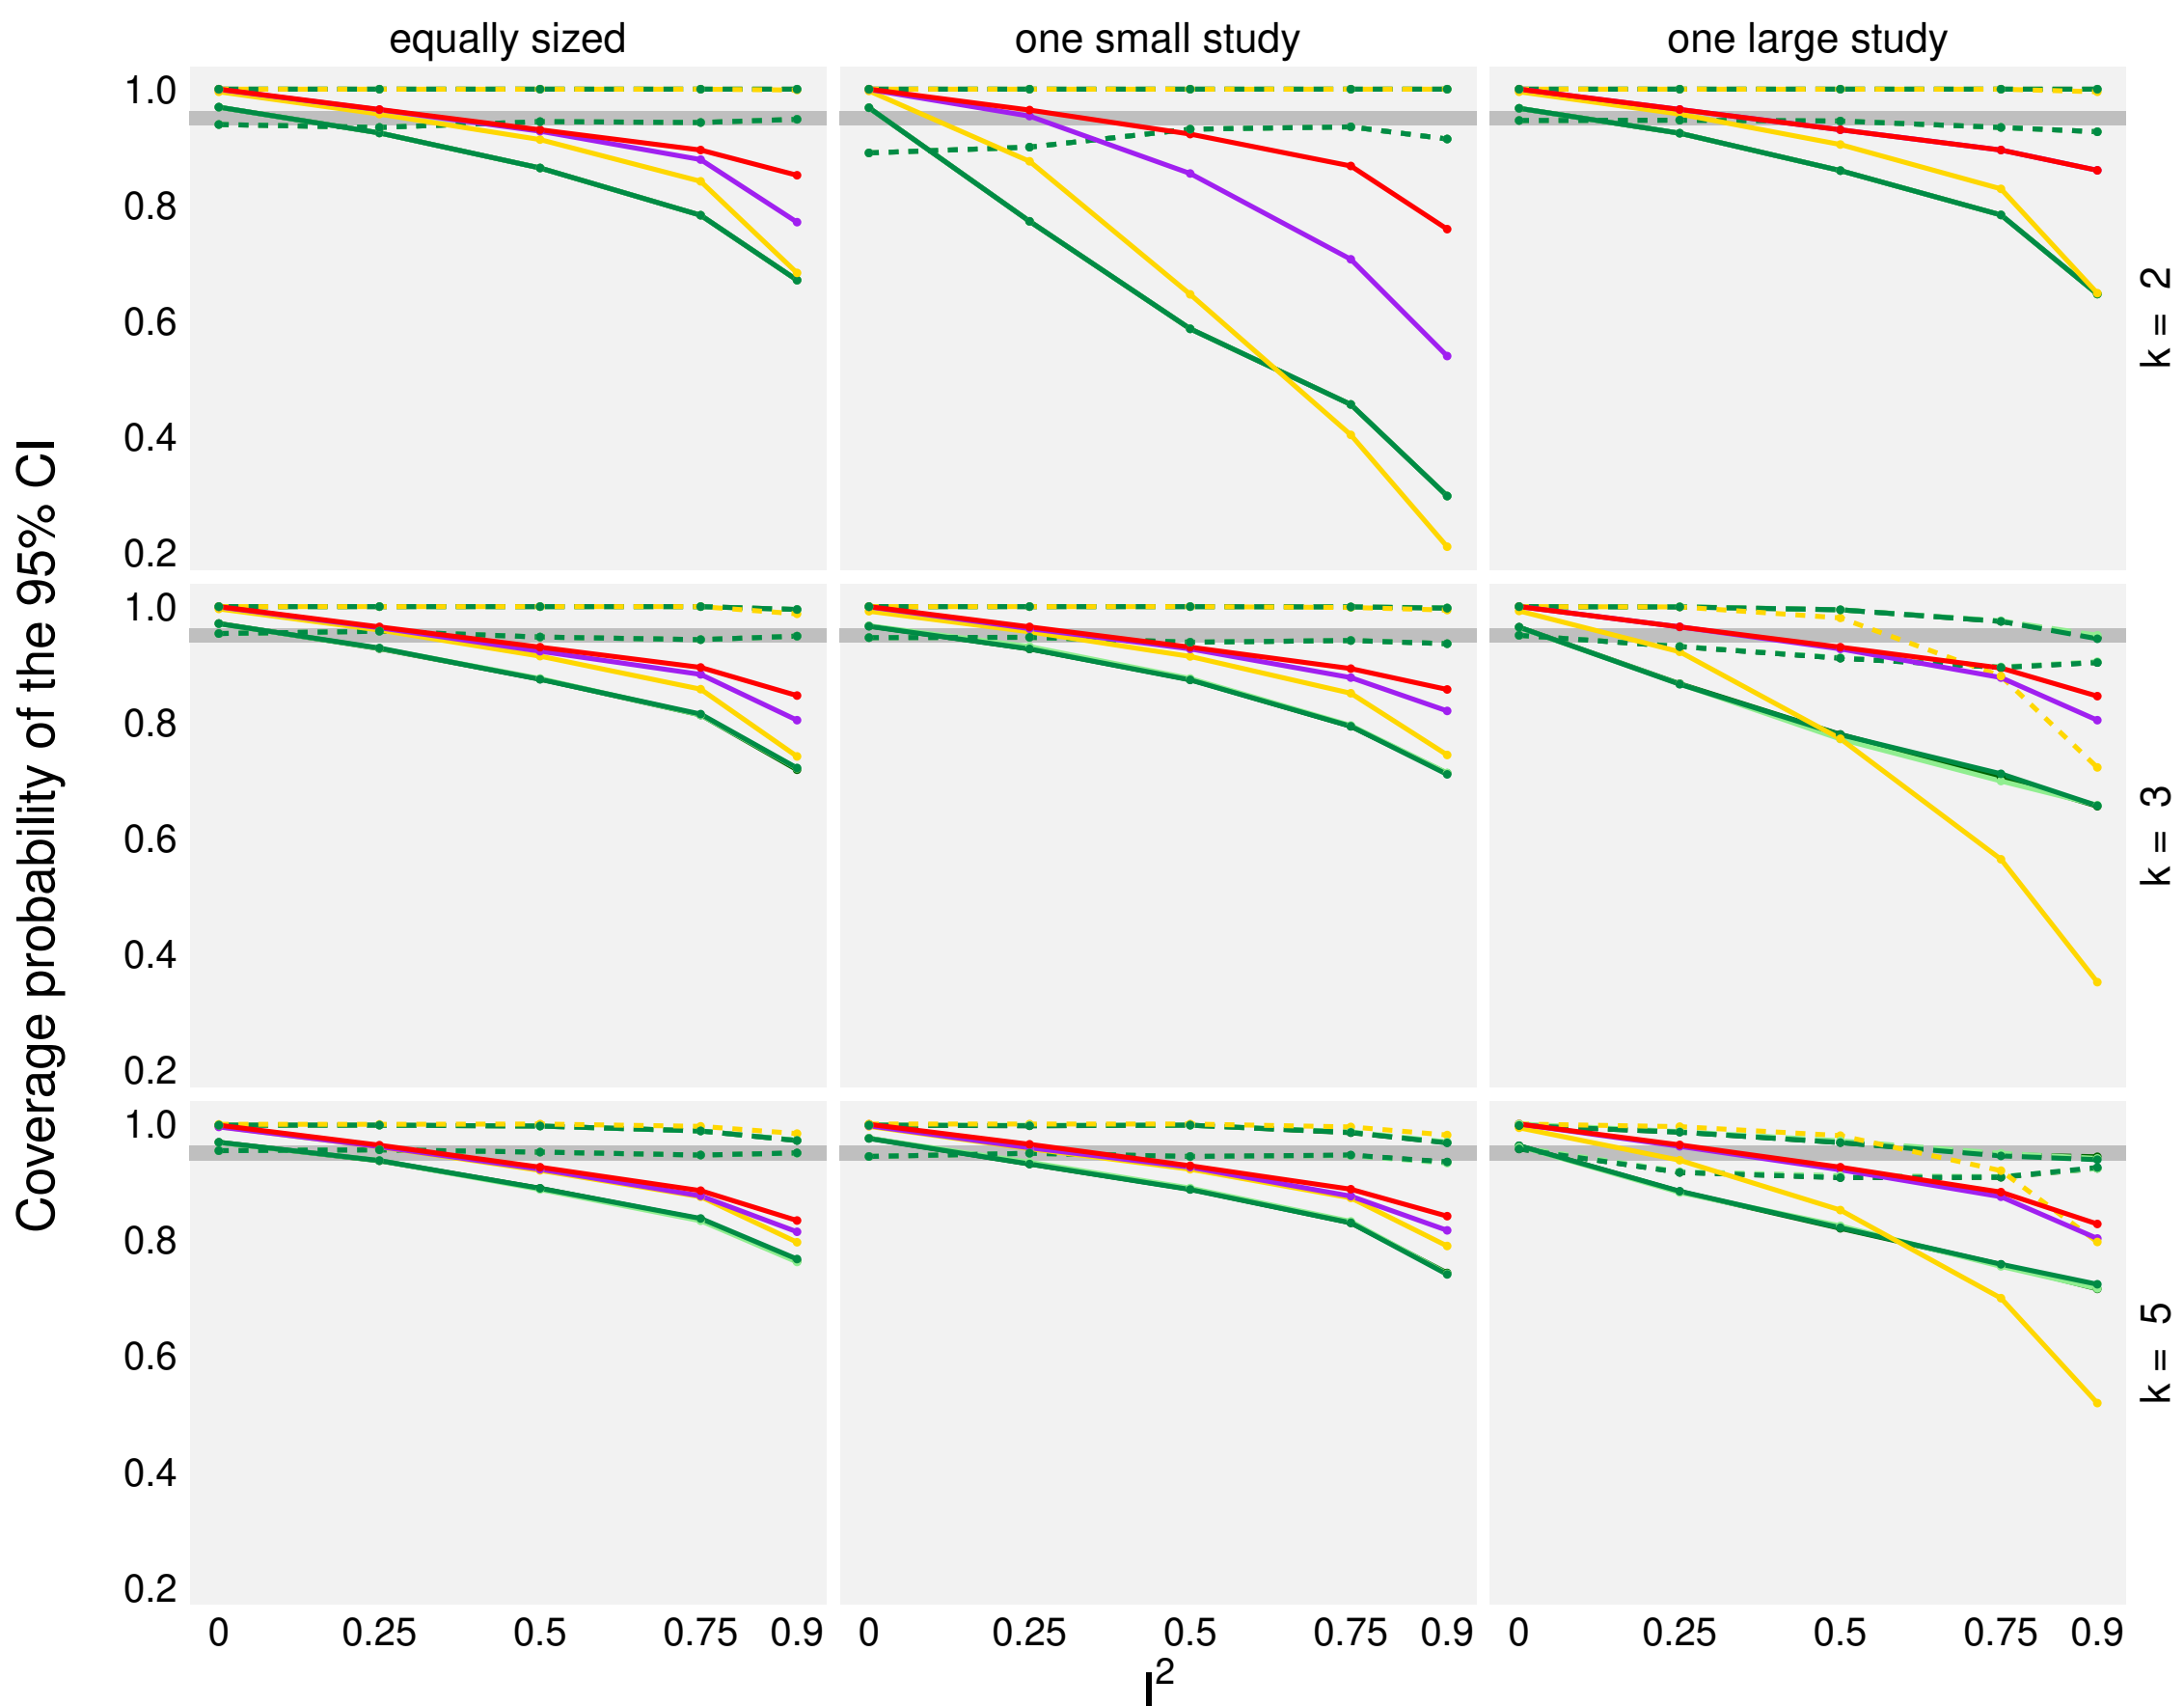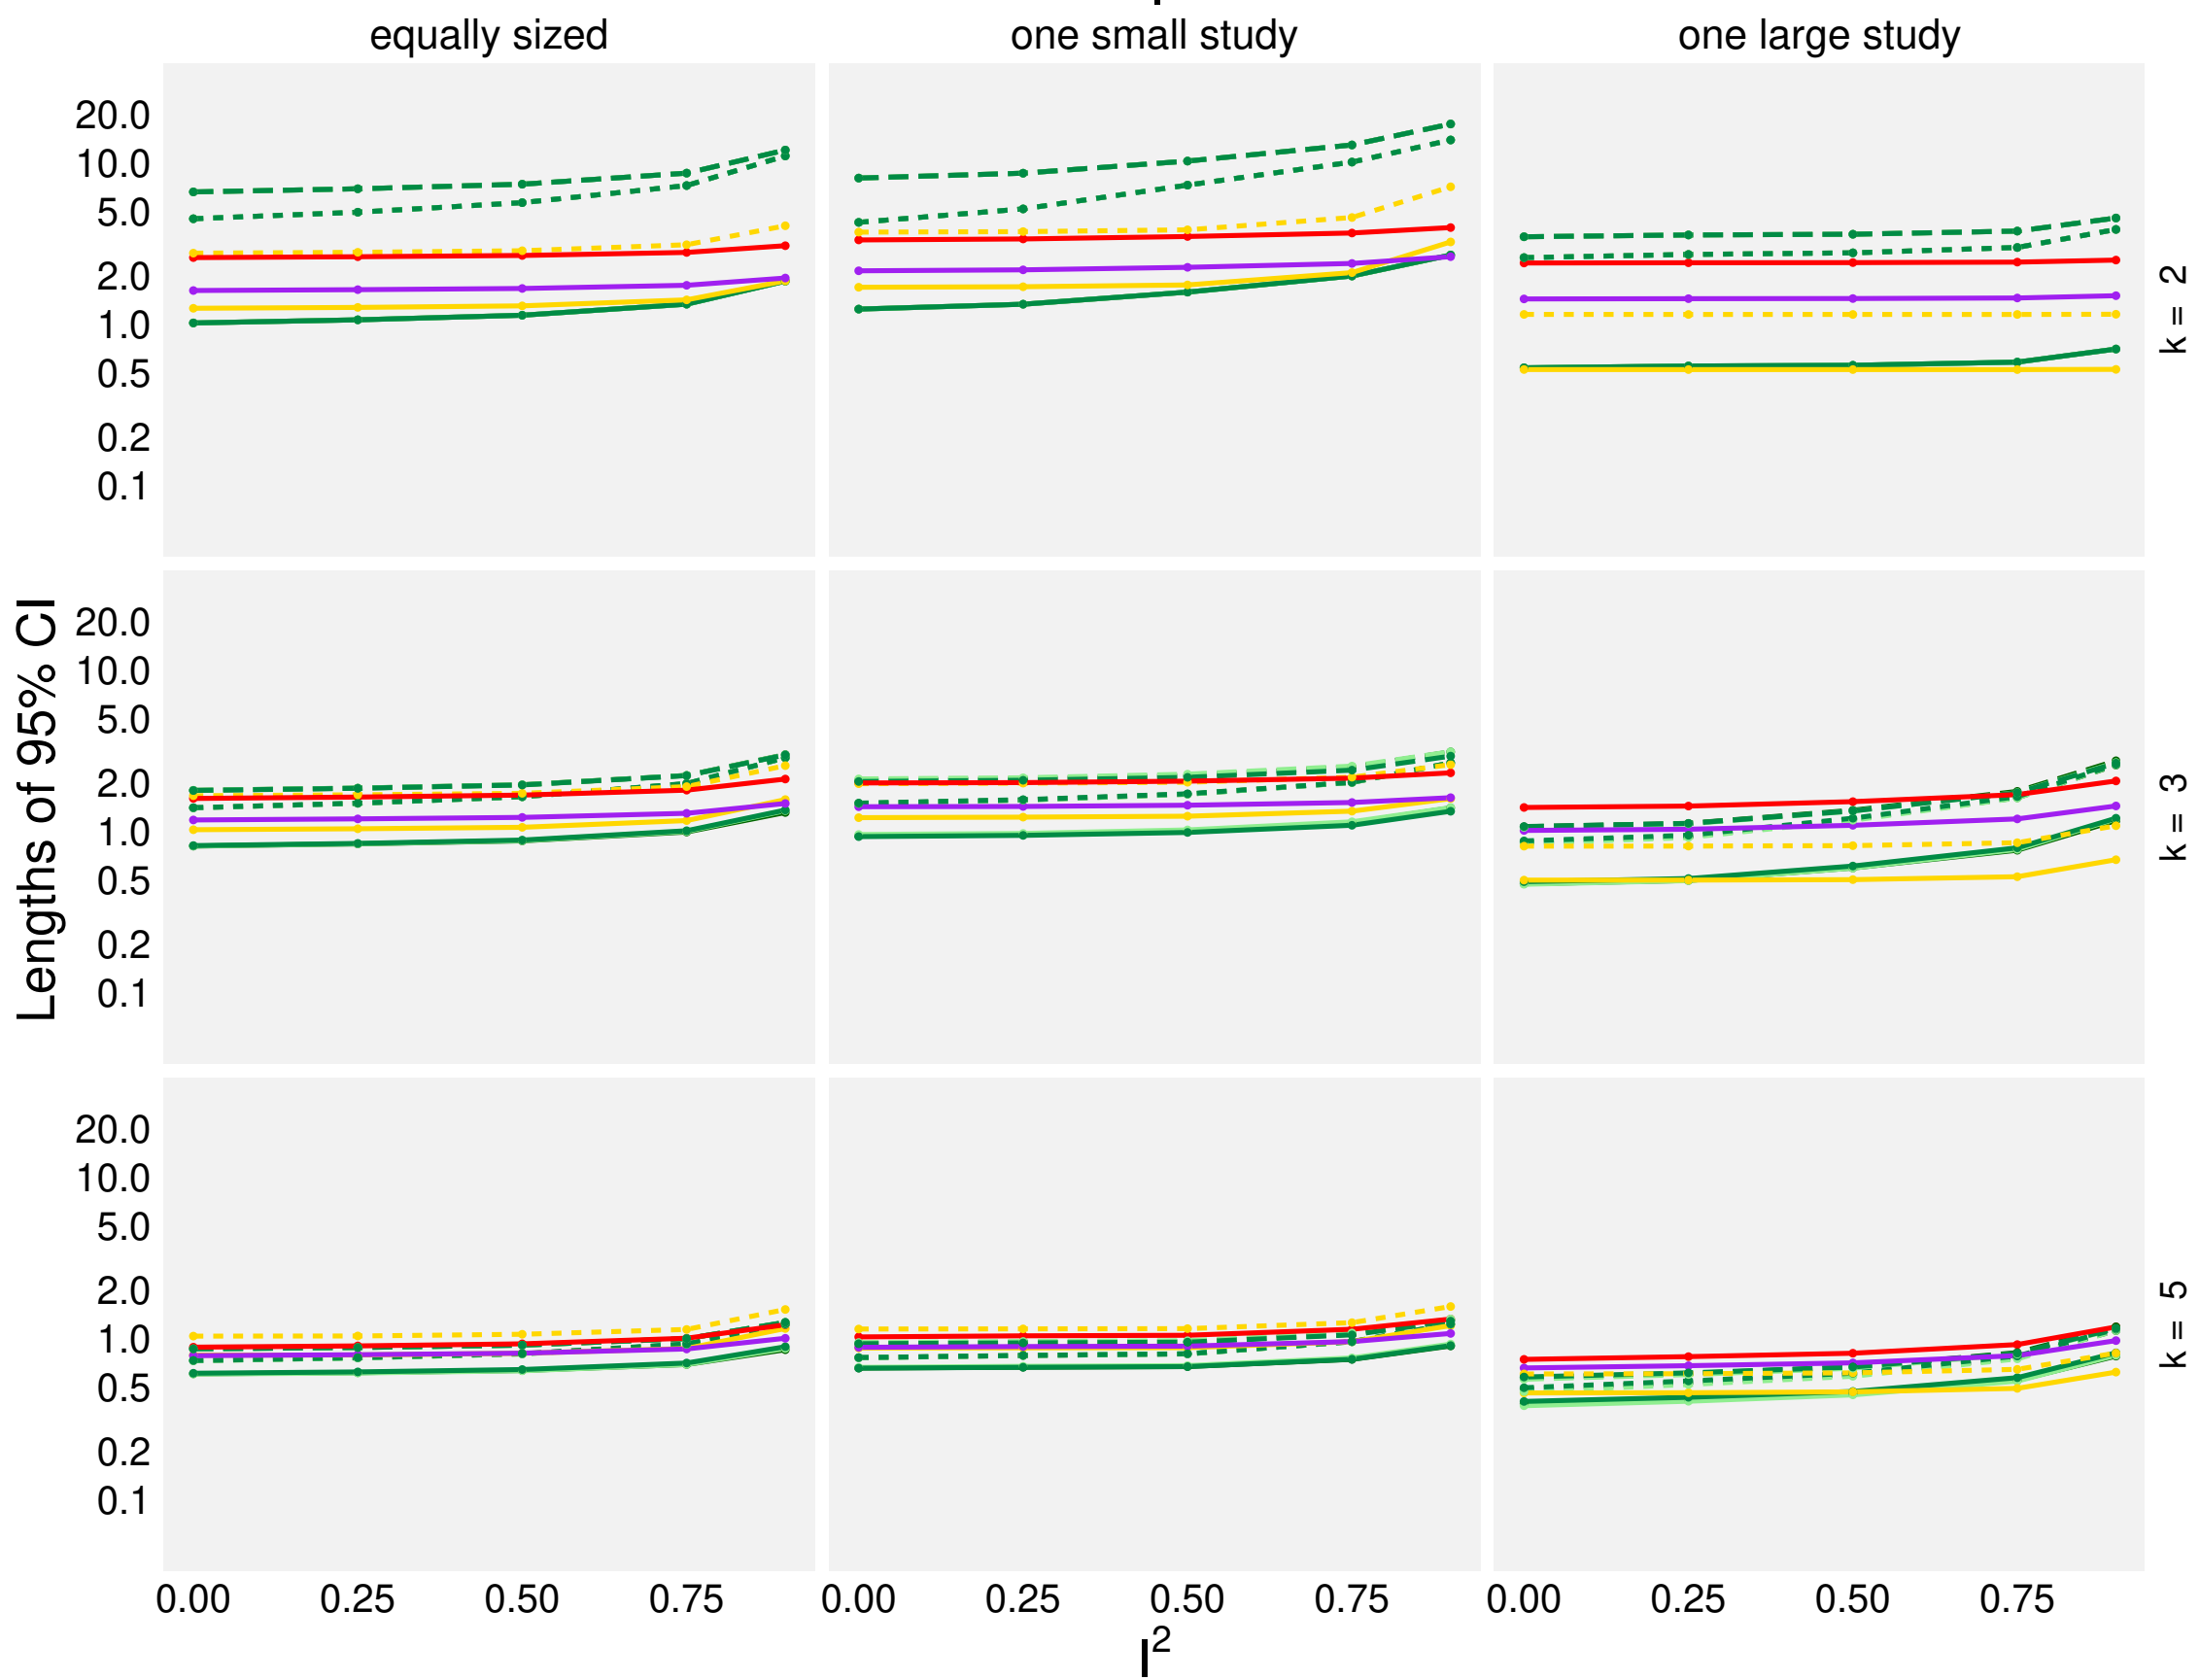

NN - DL      PN - PL  
 NN - REML      NN - Bayes HN(0.5)  
 NN - EB      NN - Bayes HN(1)

— normal quantiles  
 -- HKSJ or Student's t  
 ··· mHKSJ

RR  
( $n_i=25, \pi_0=0.7$ )

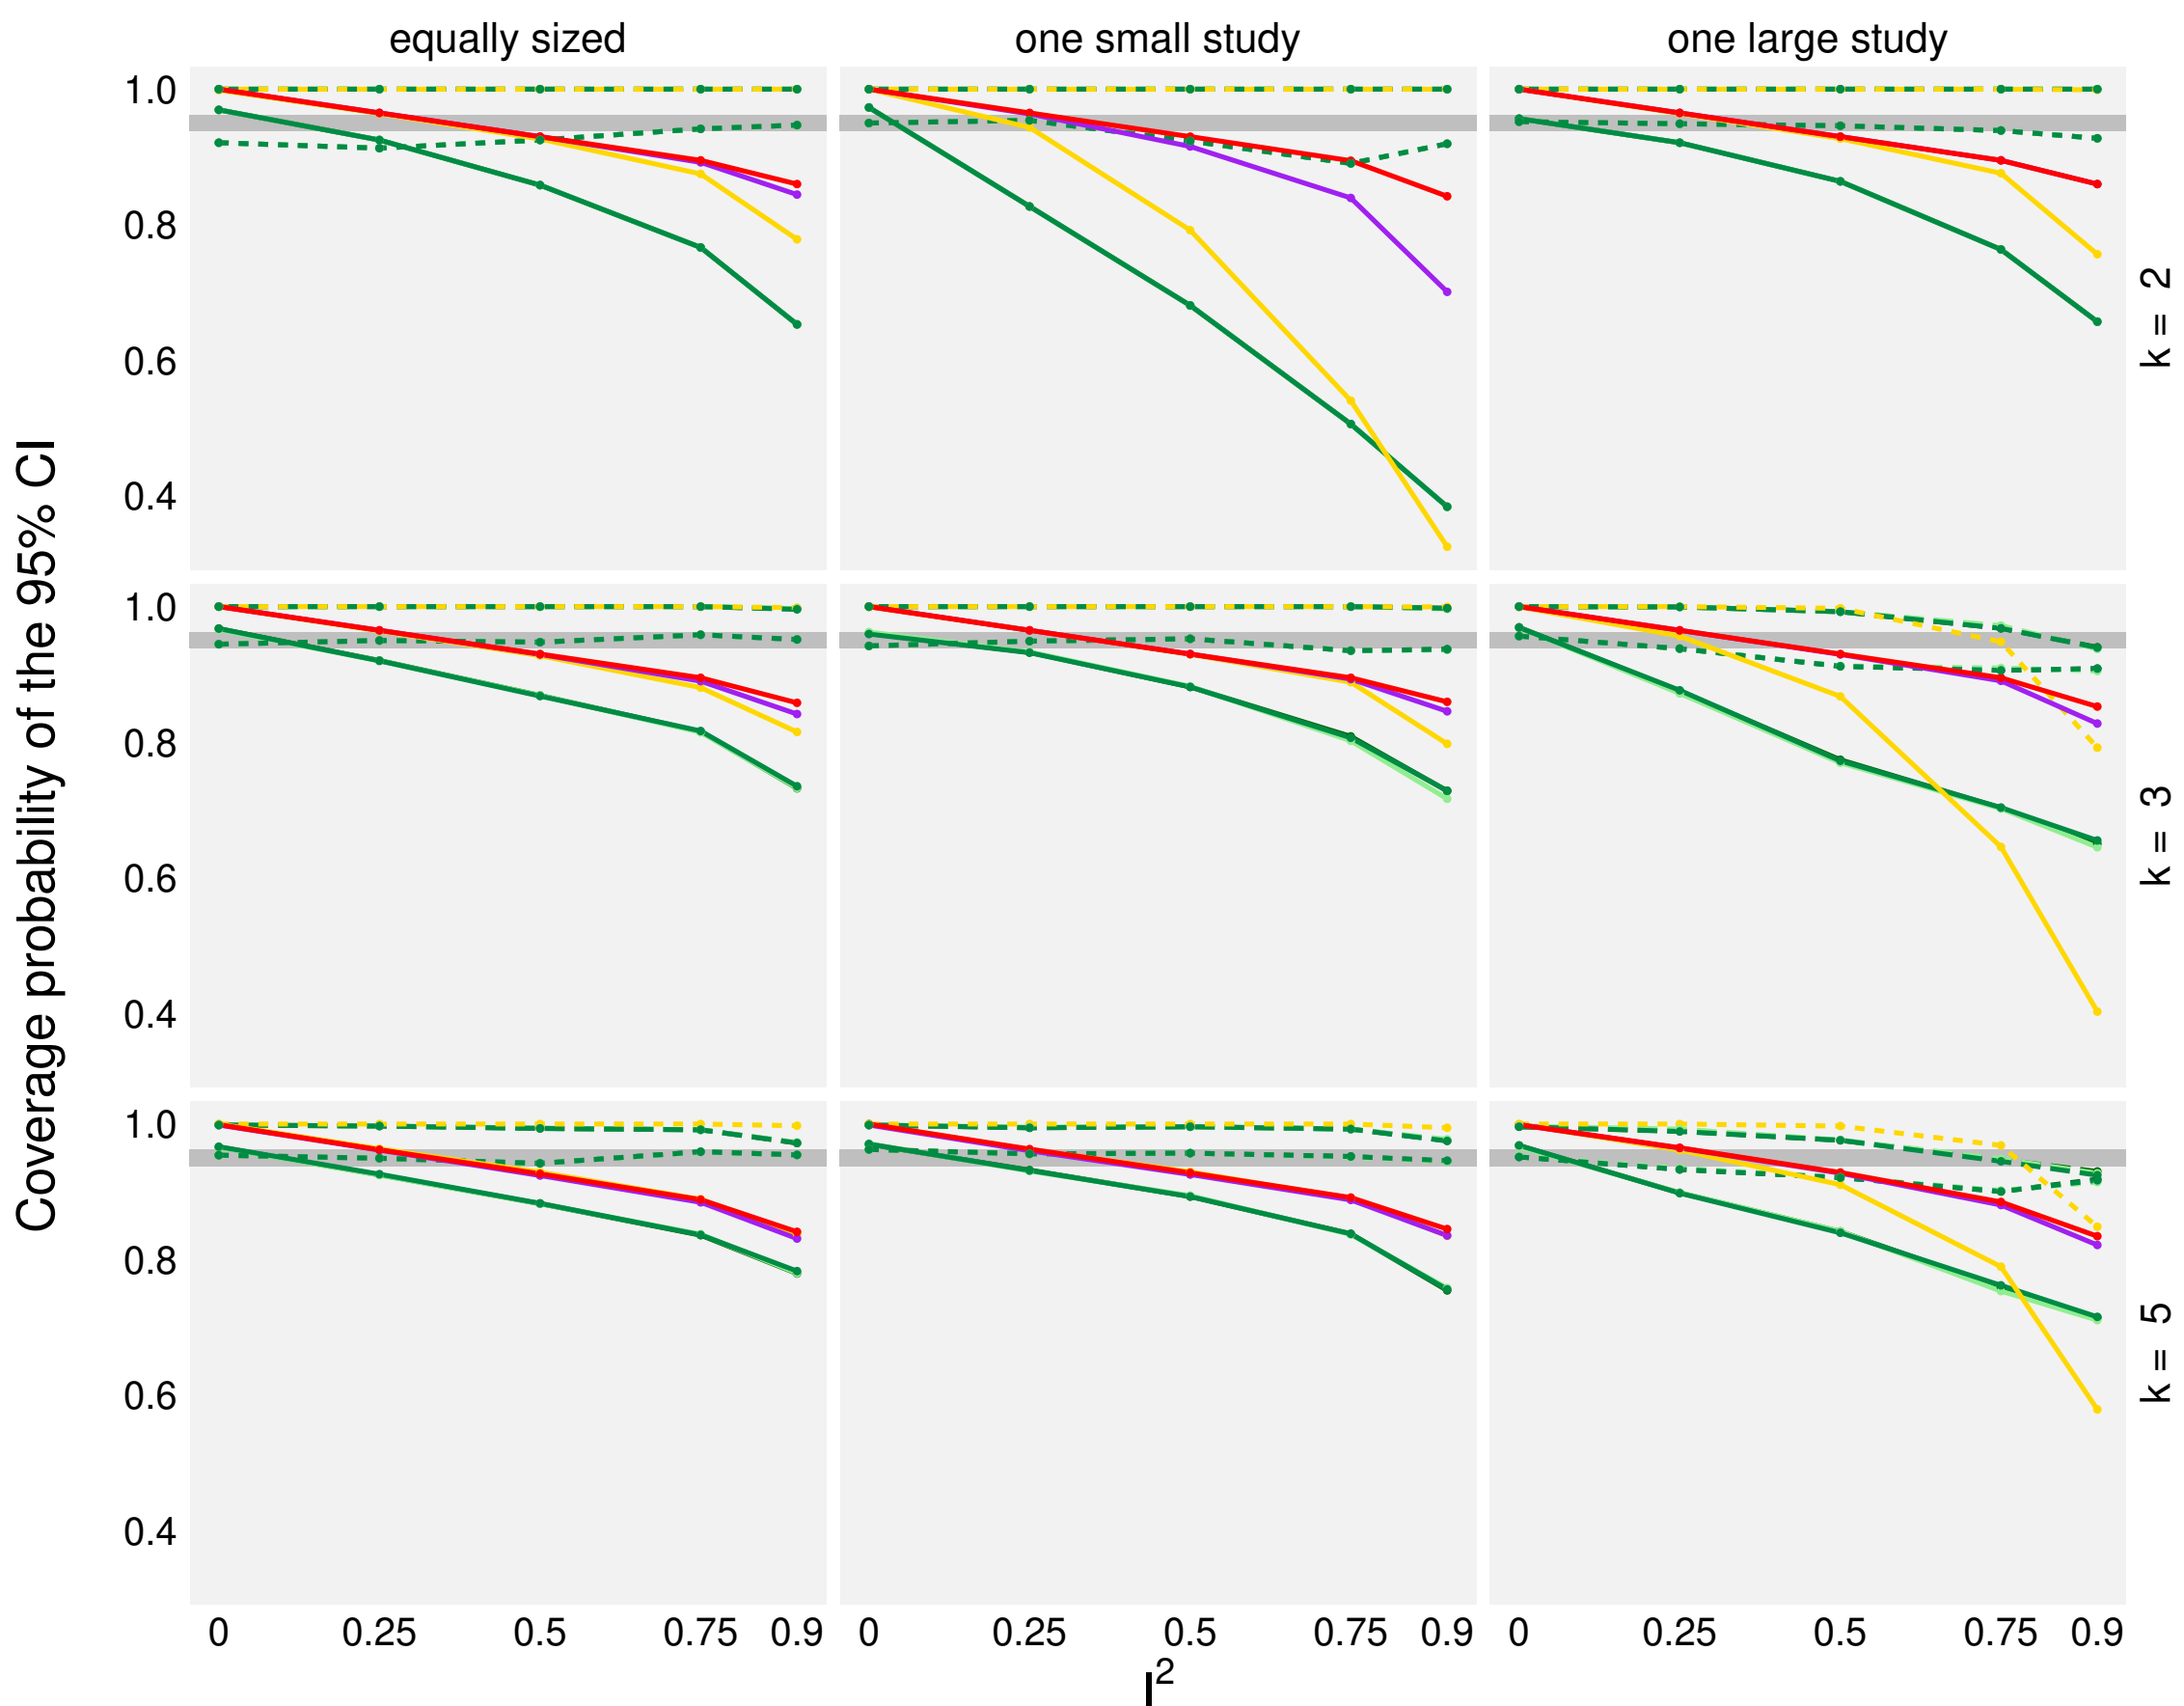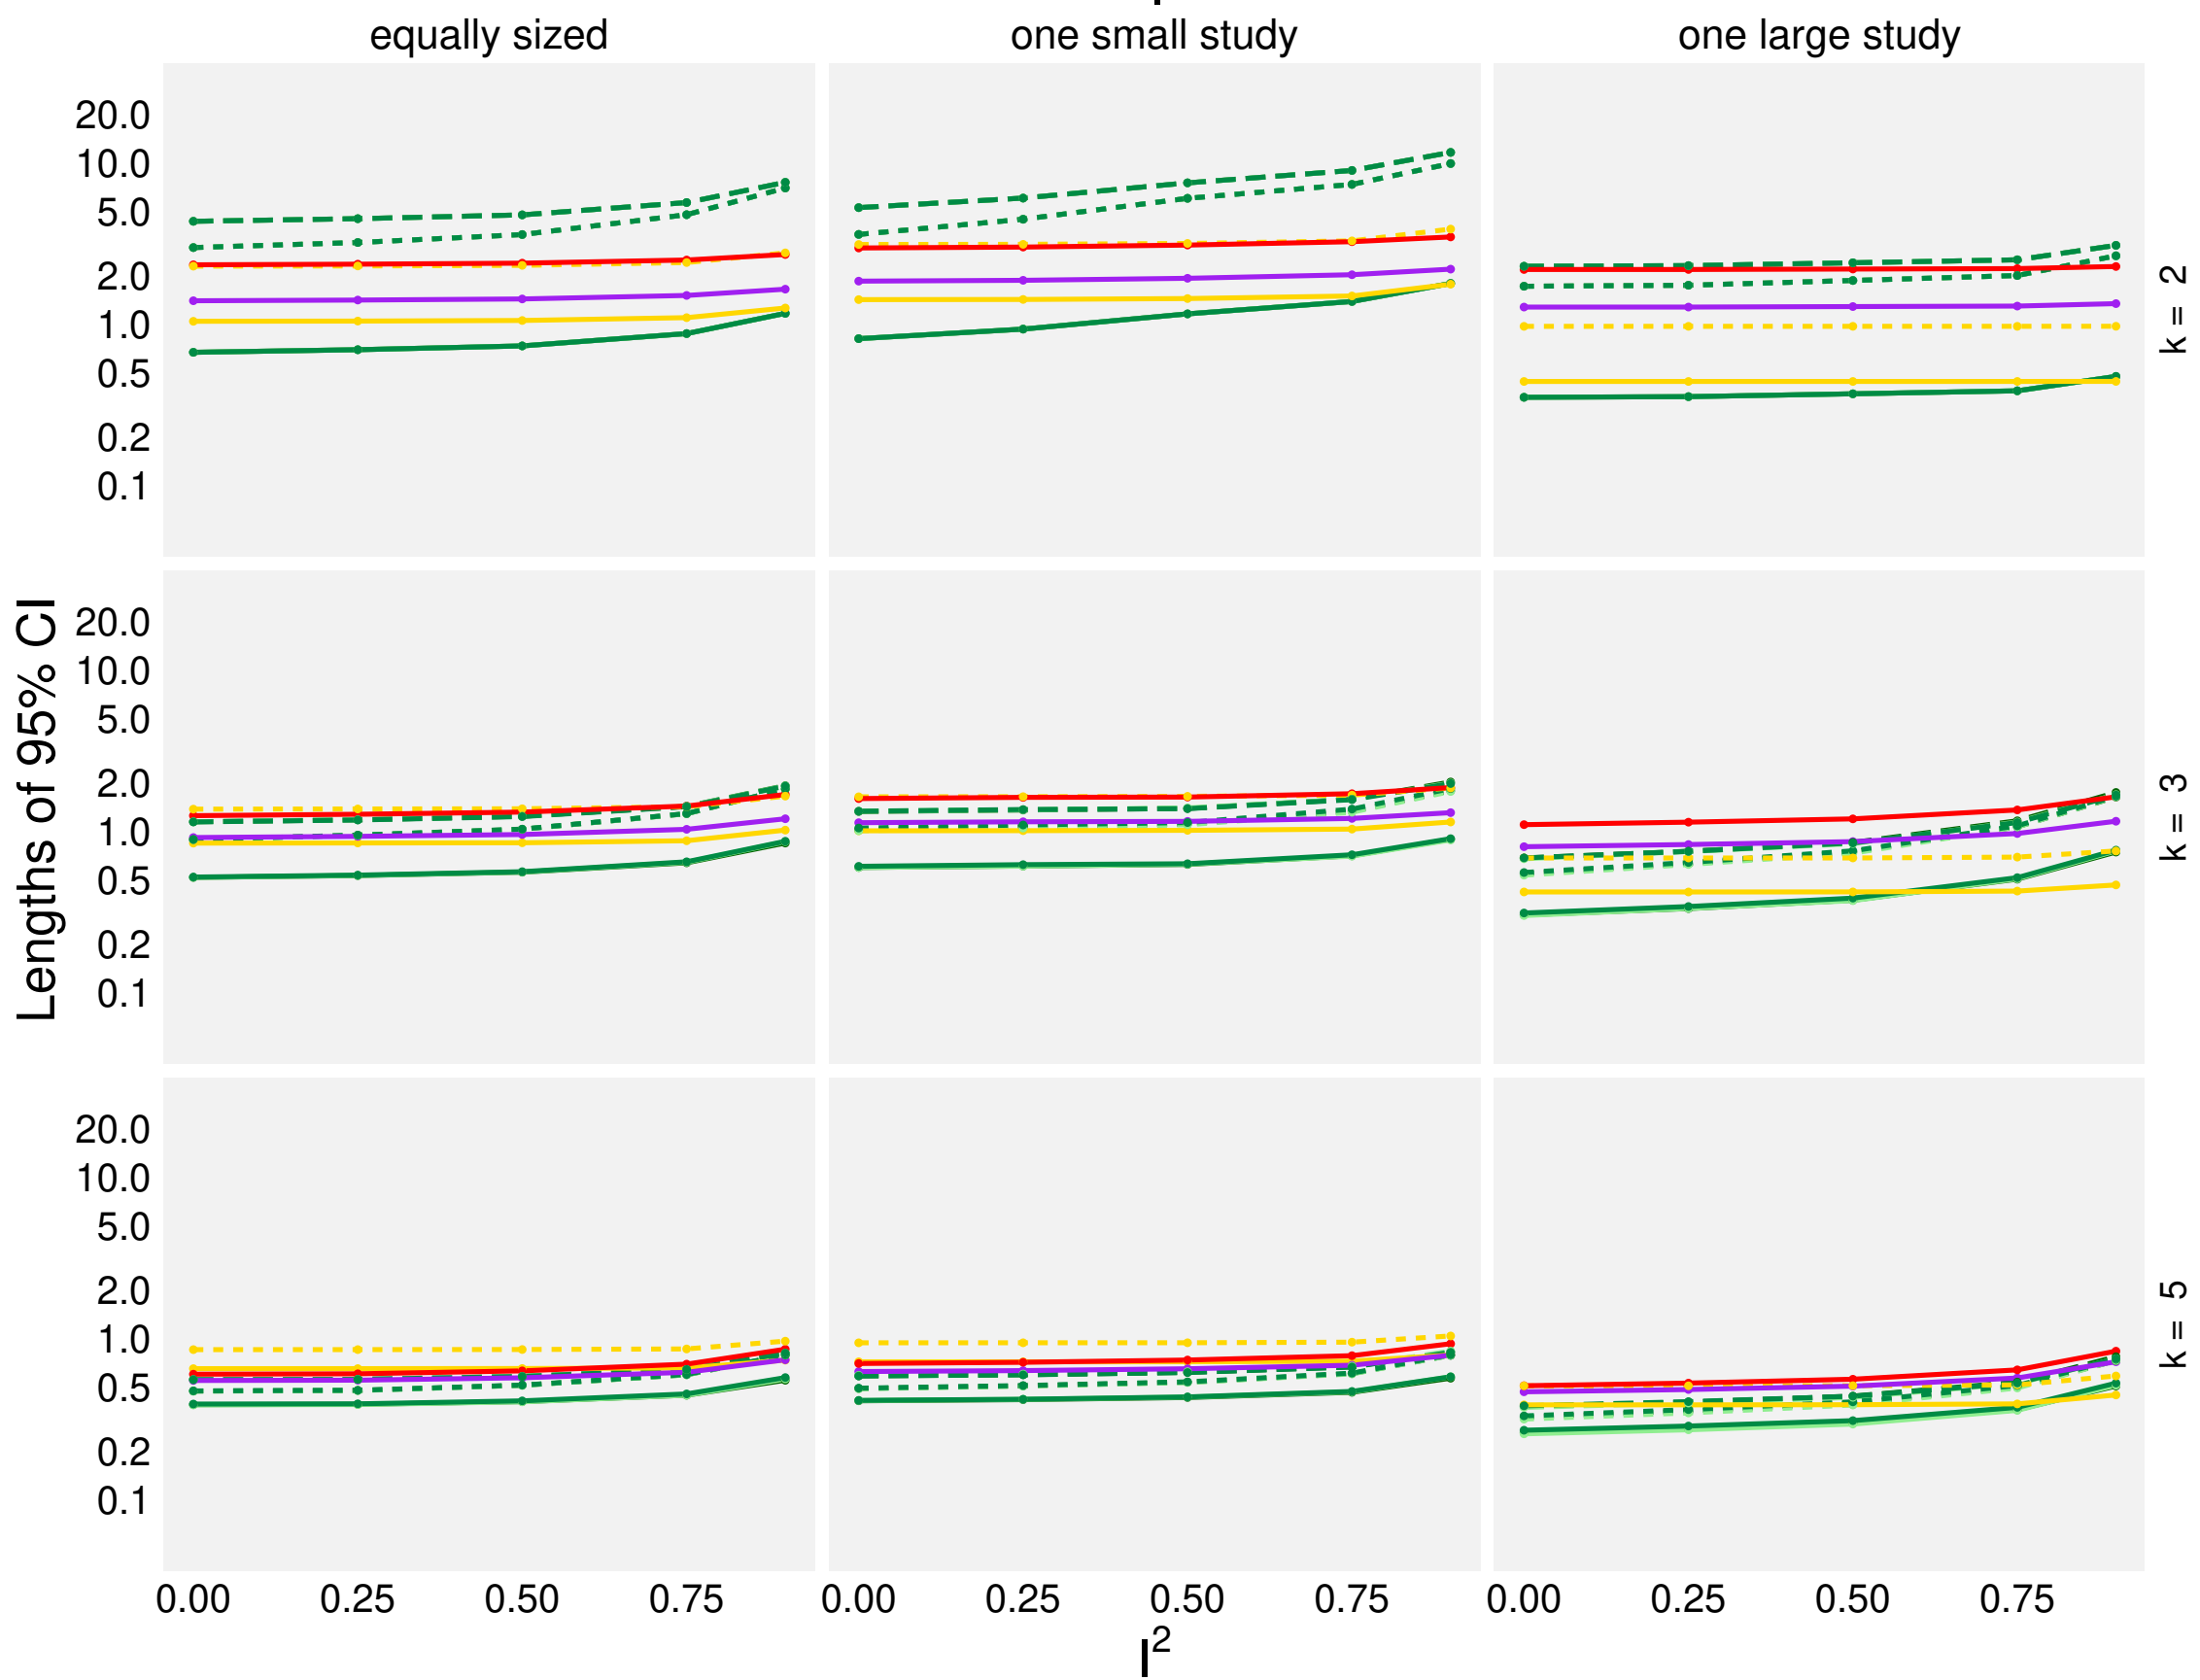

— NN – DL      — PN – PL      — normal quantiles  
 — NN – REML      — NN – Bayes HN(0.5)      - - HKSJ or Student's t  
 — NN – EB      — NN – Bayes HN(1)      - - mHKSJ

RR  
( $n_i=25, \pi_0=0.9$ )

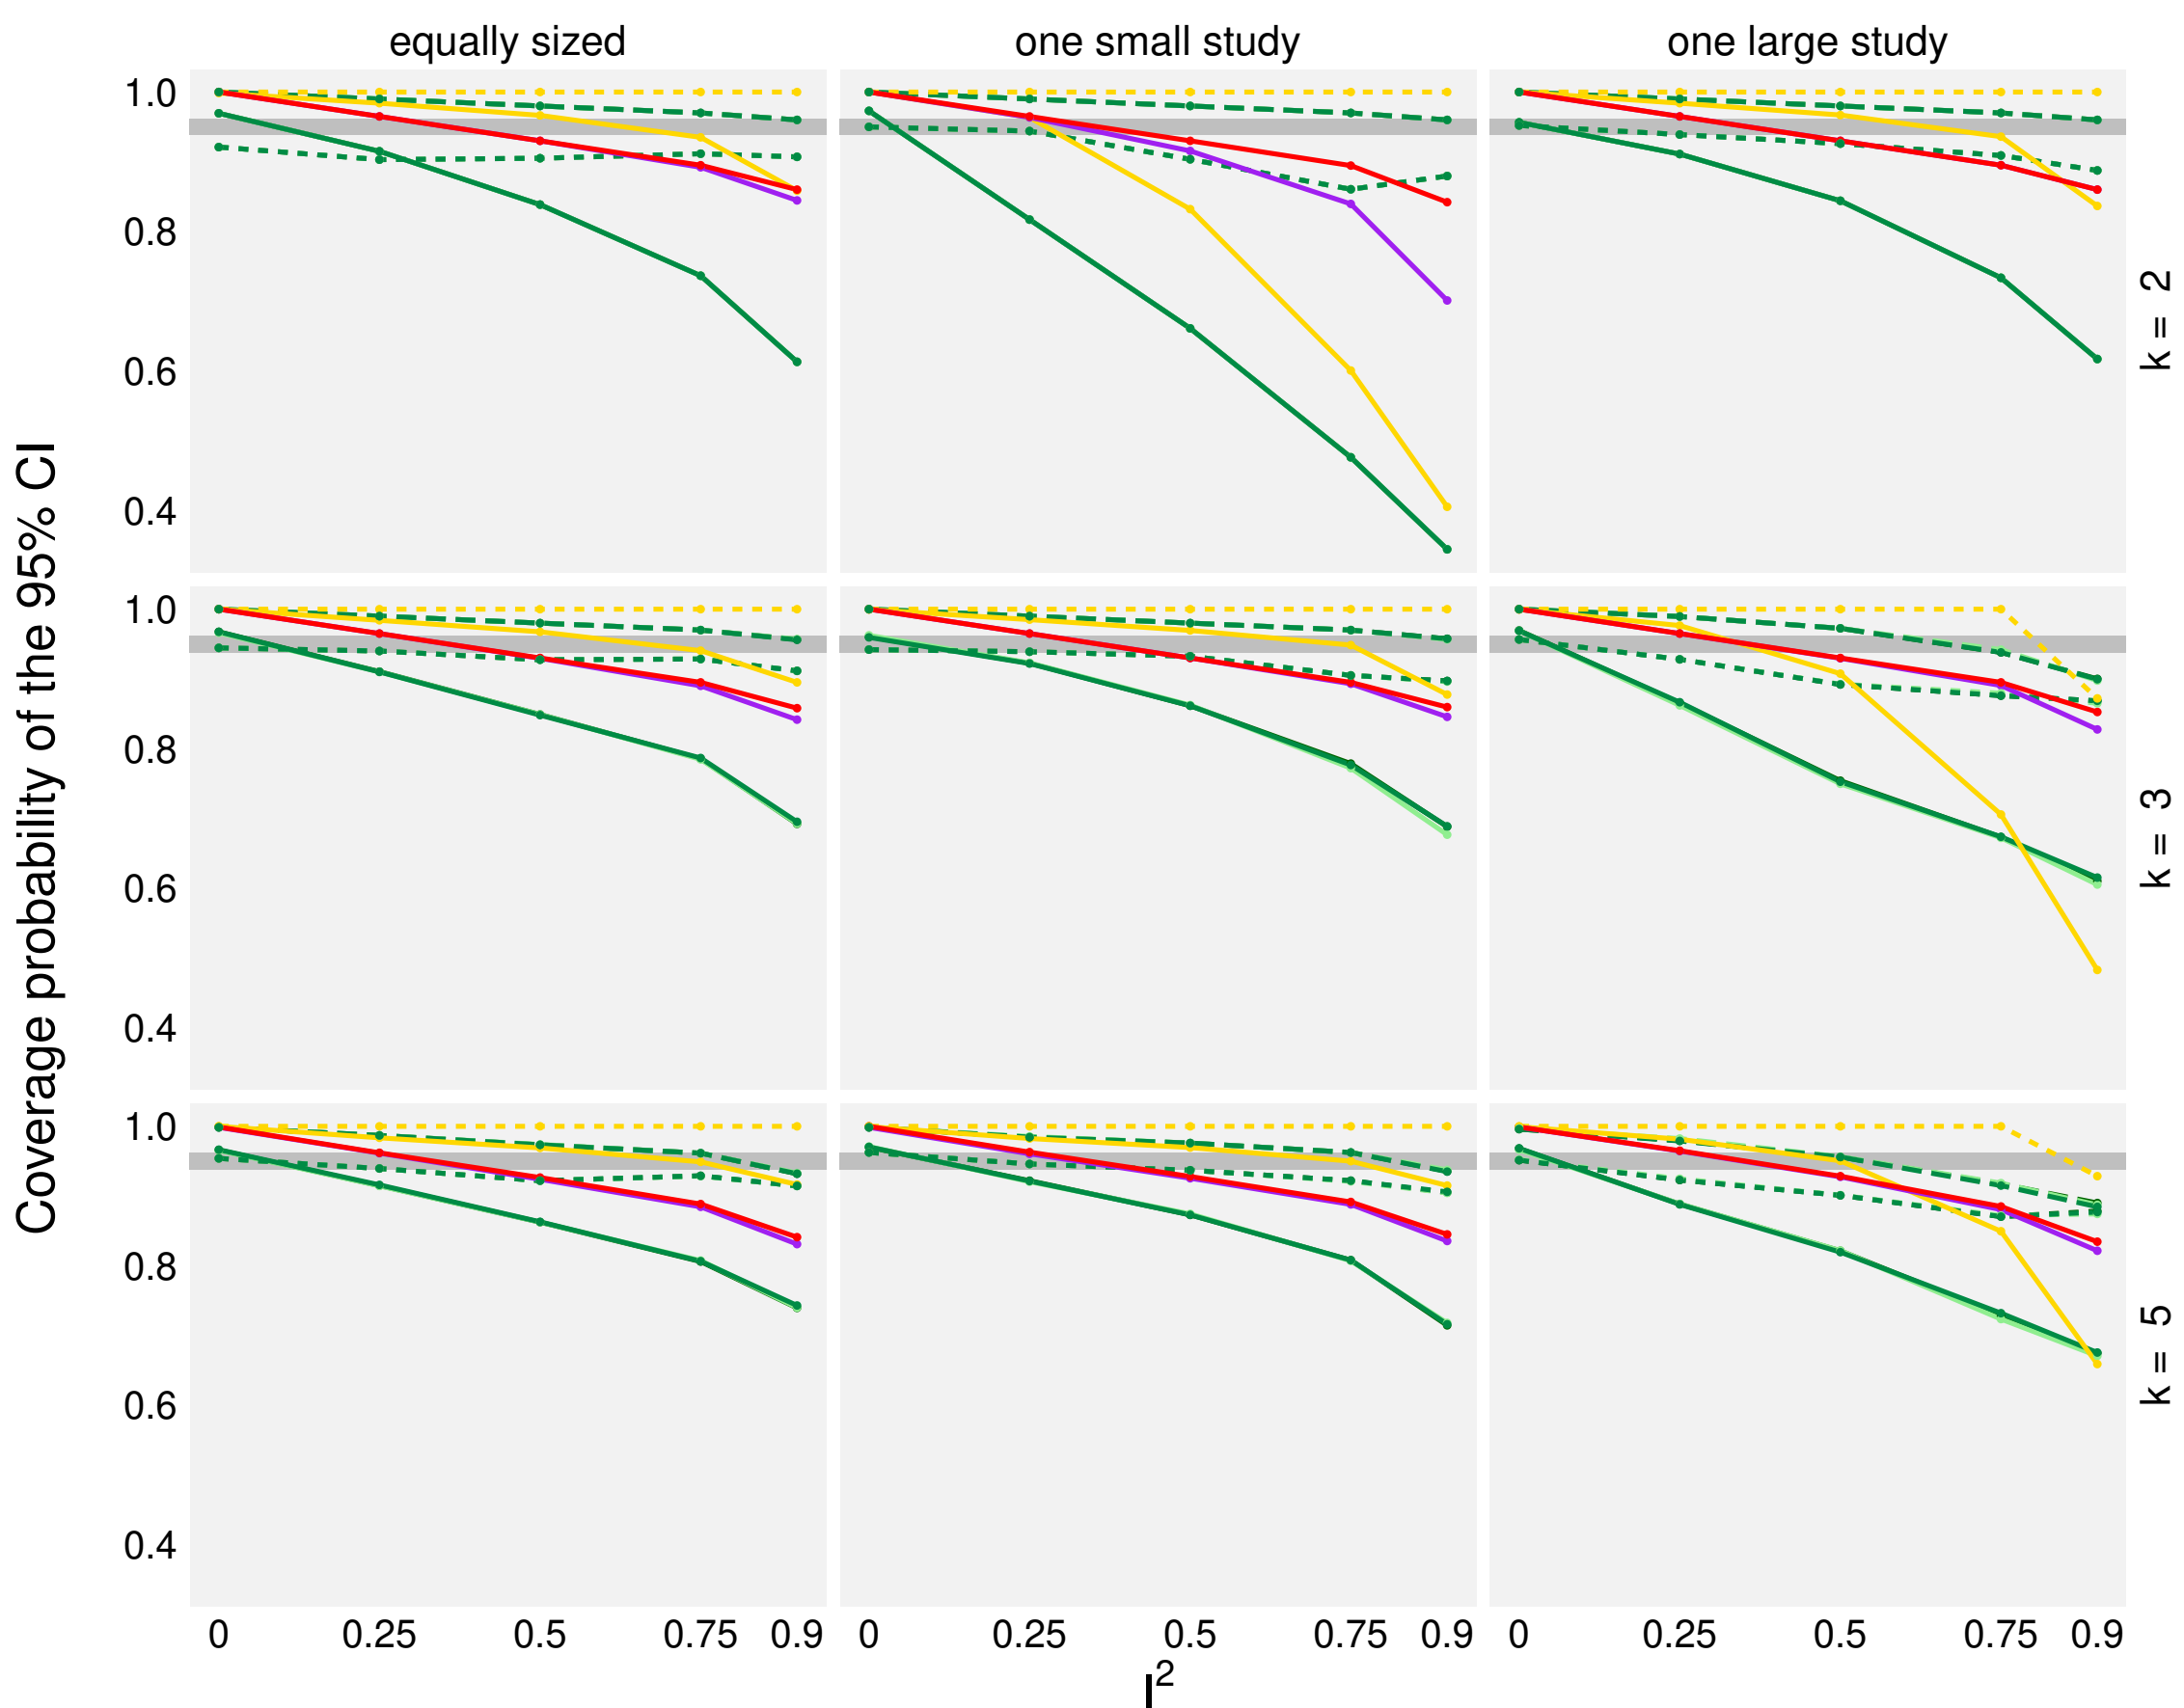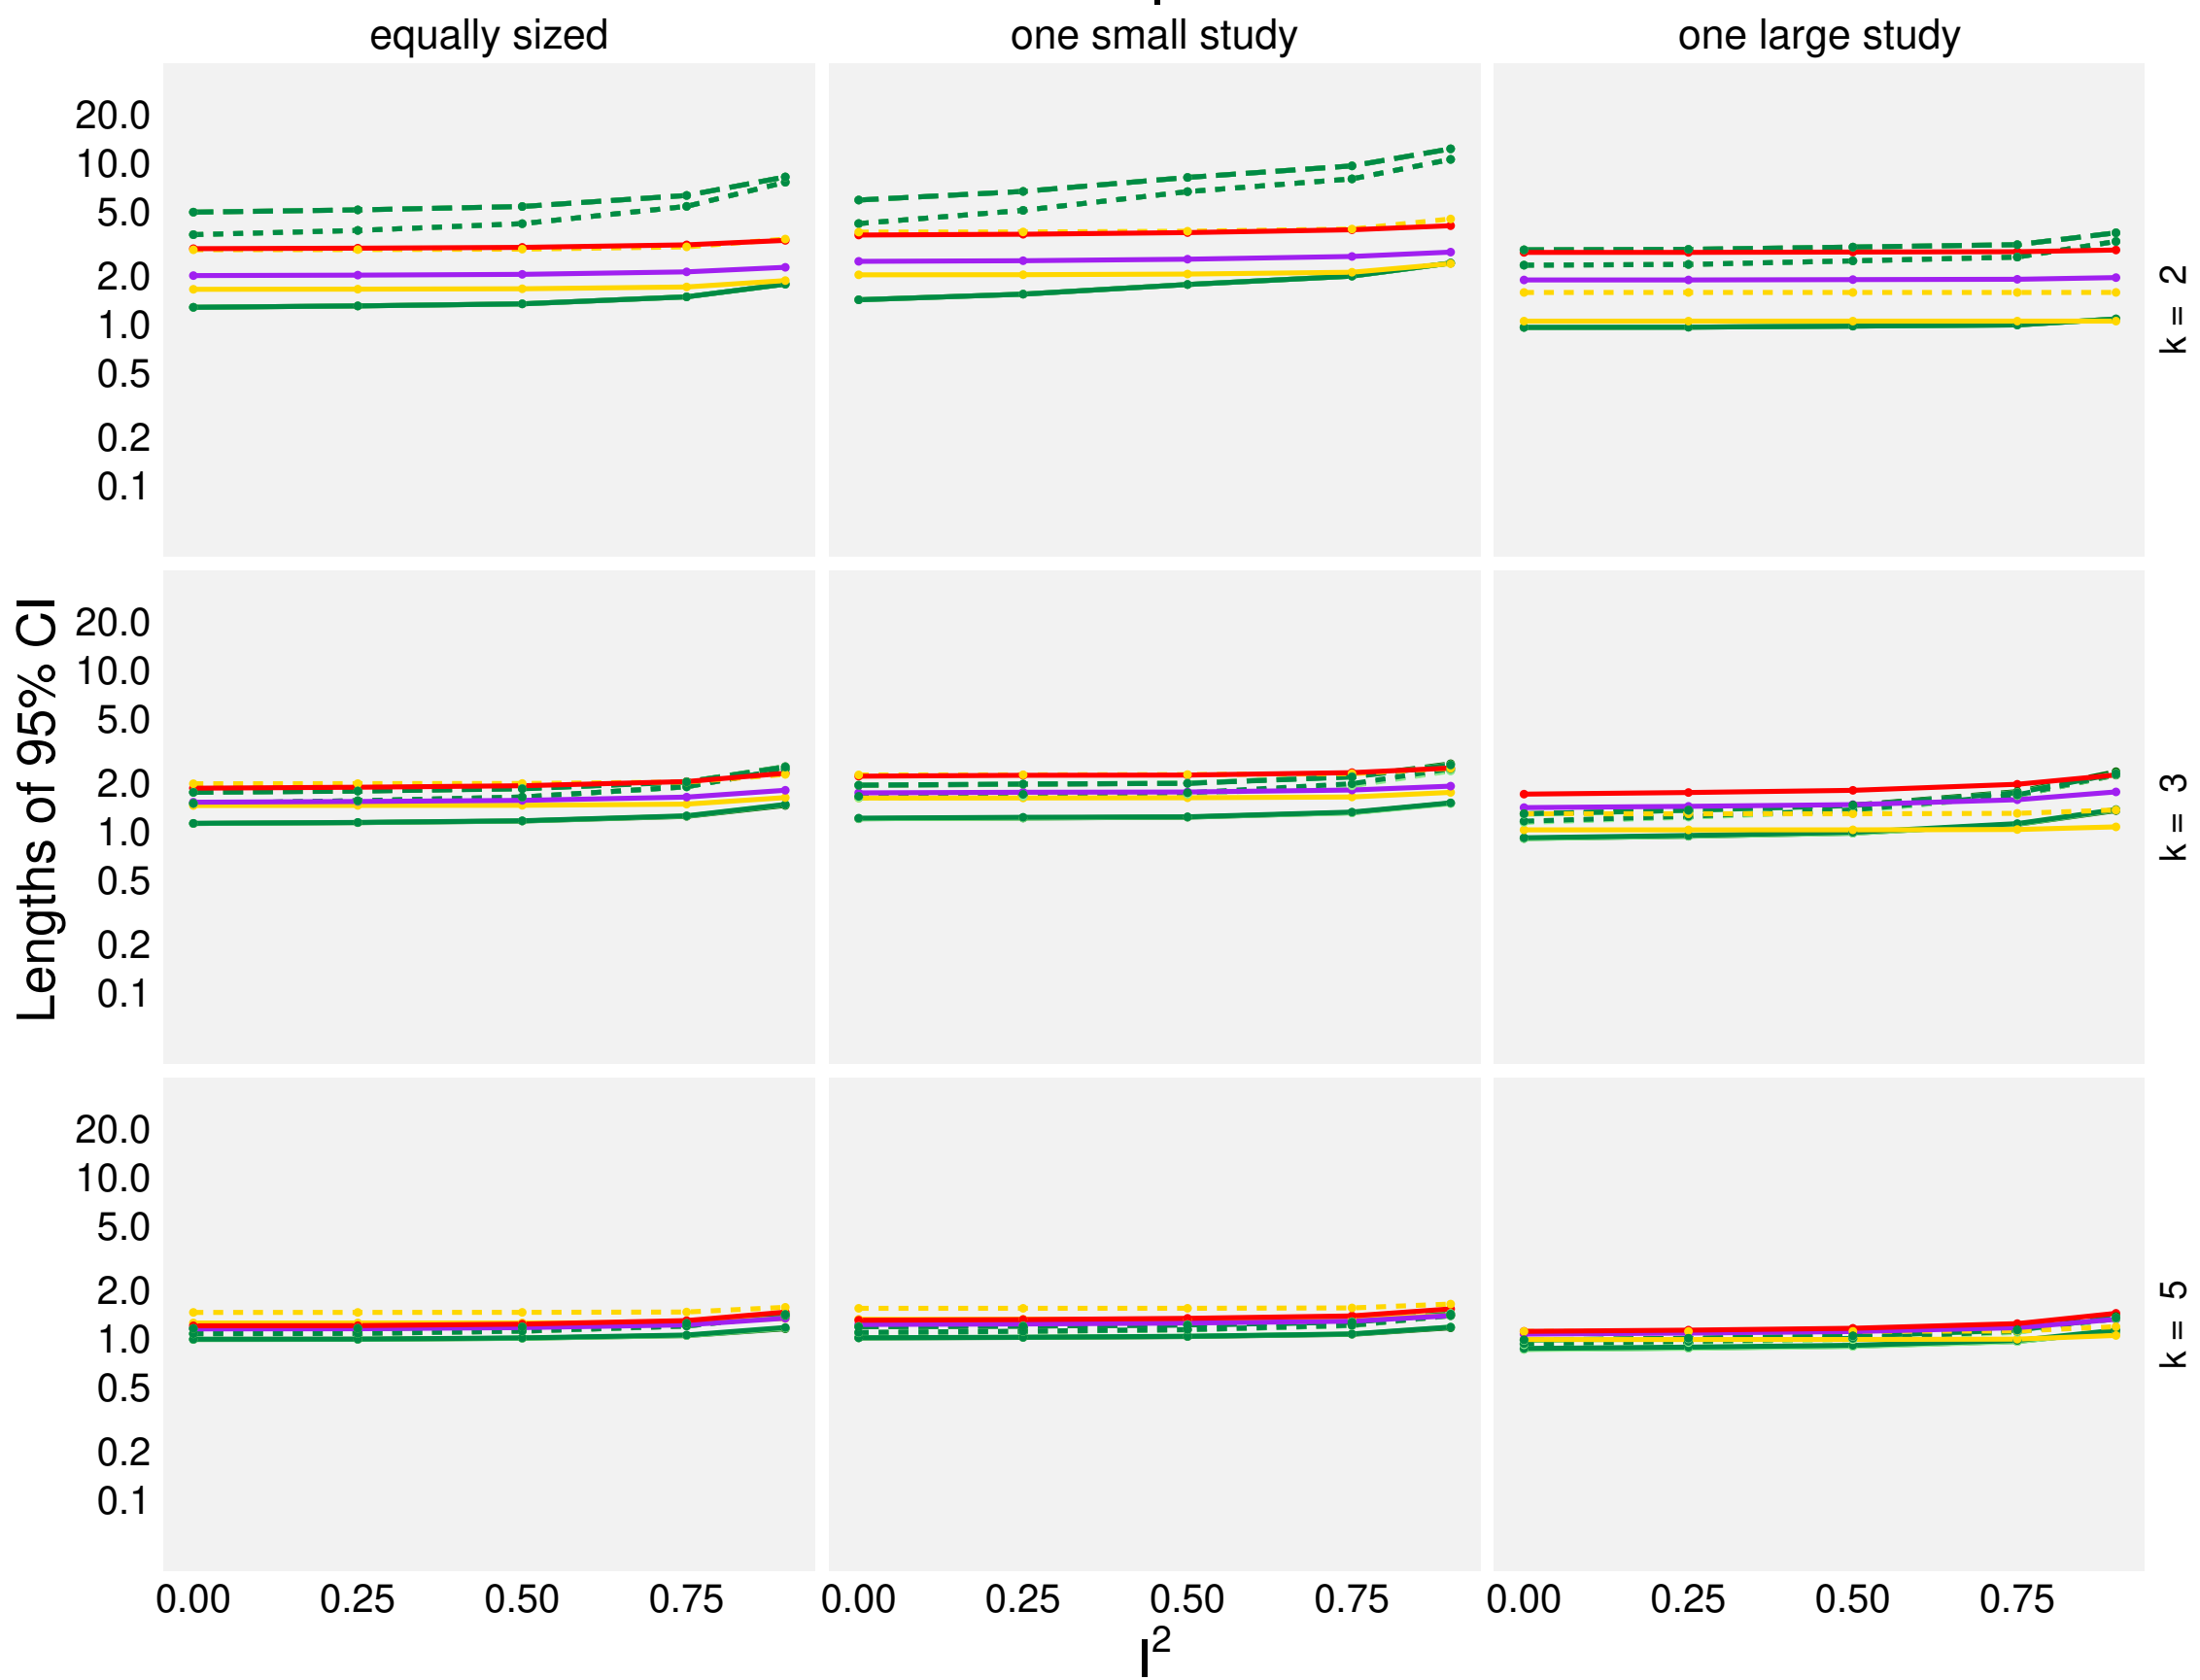

— NN – DL      — PN – PL      — normal quantiles  
 — NN – REML      — NN – Bayes HN(0.5)      - - HKSJ or Student's t  
 — NN – EB      — NN – Bayes HN(1)      - - mHKSJ

RR  
( $n_i=50, \pi_0=0.1$ )

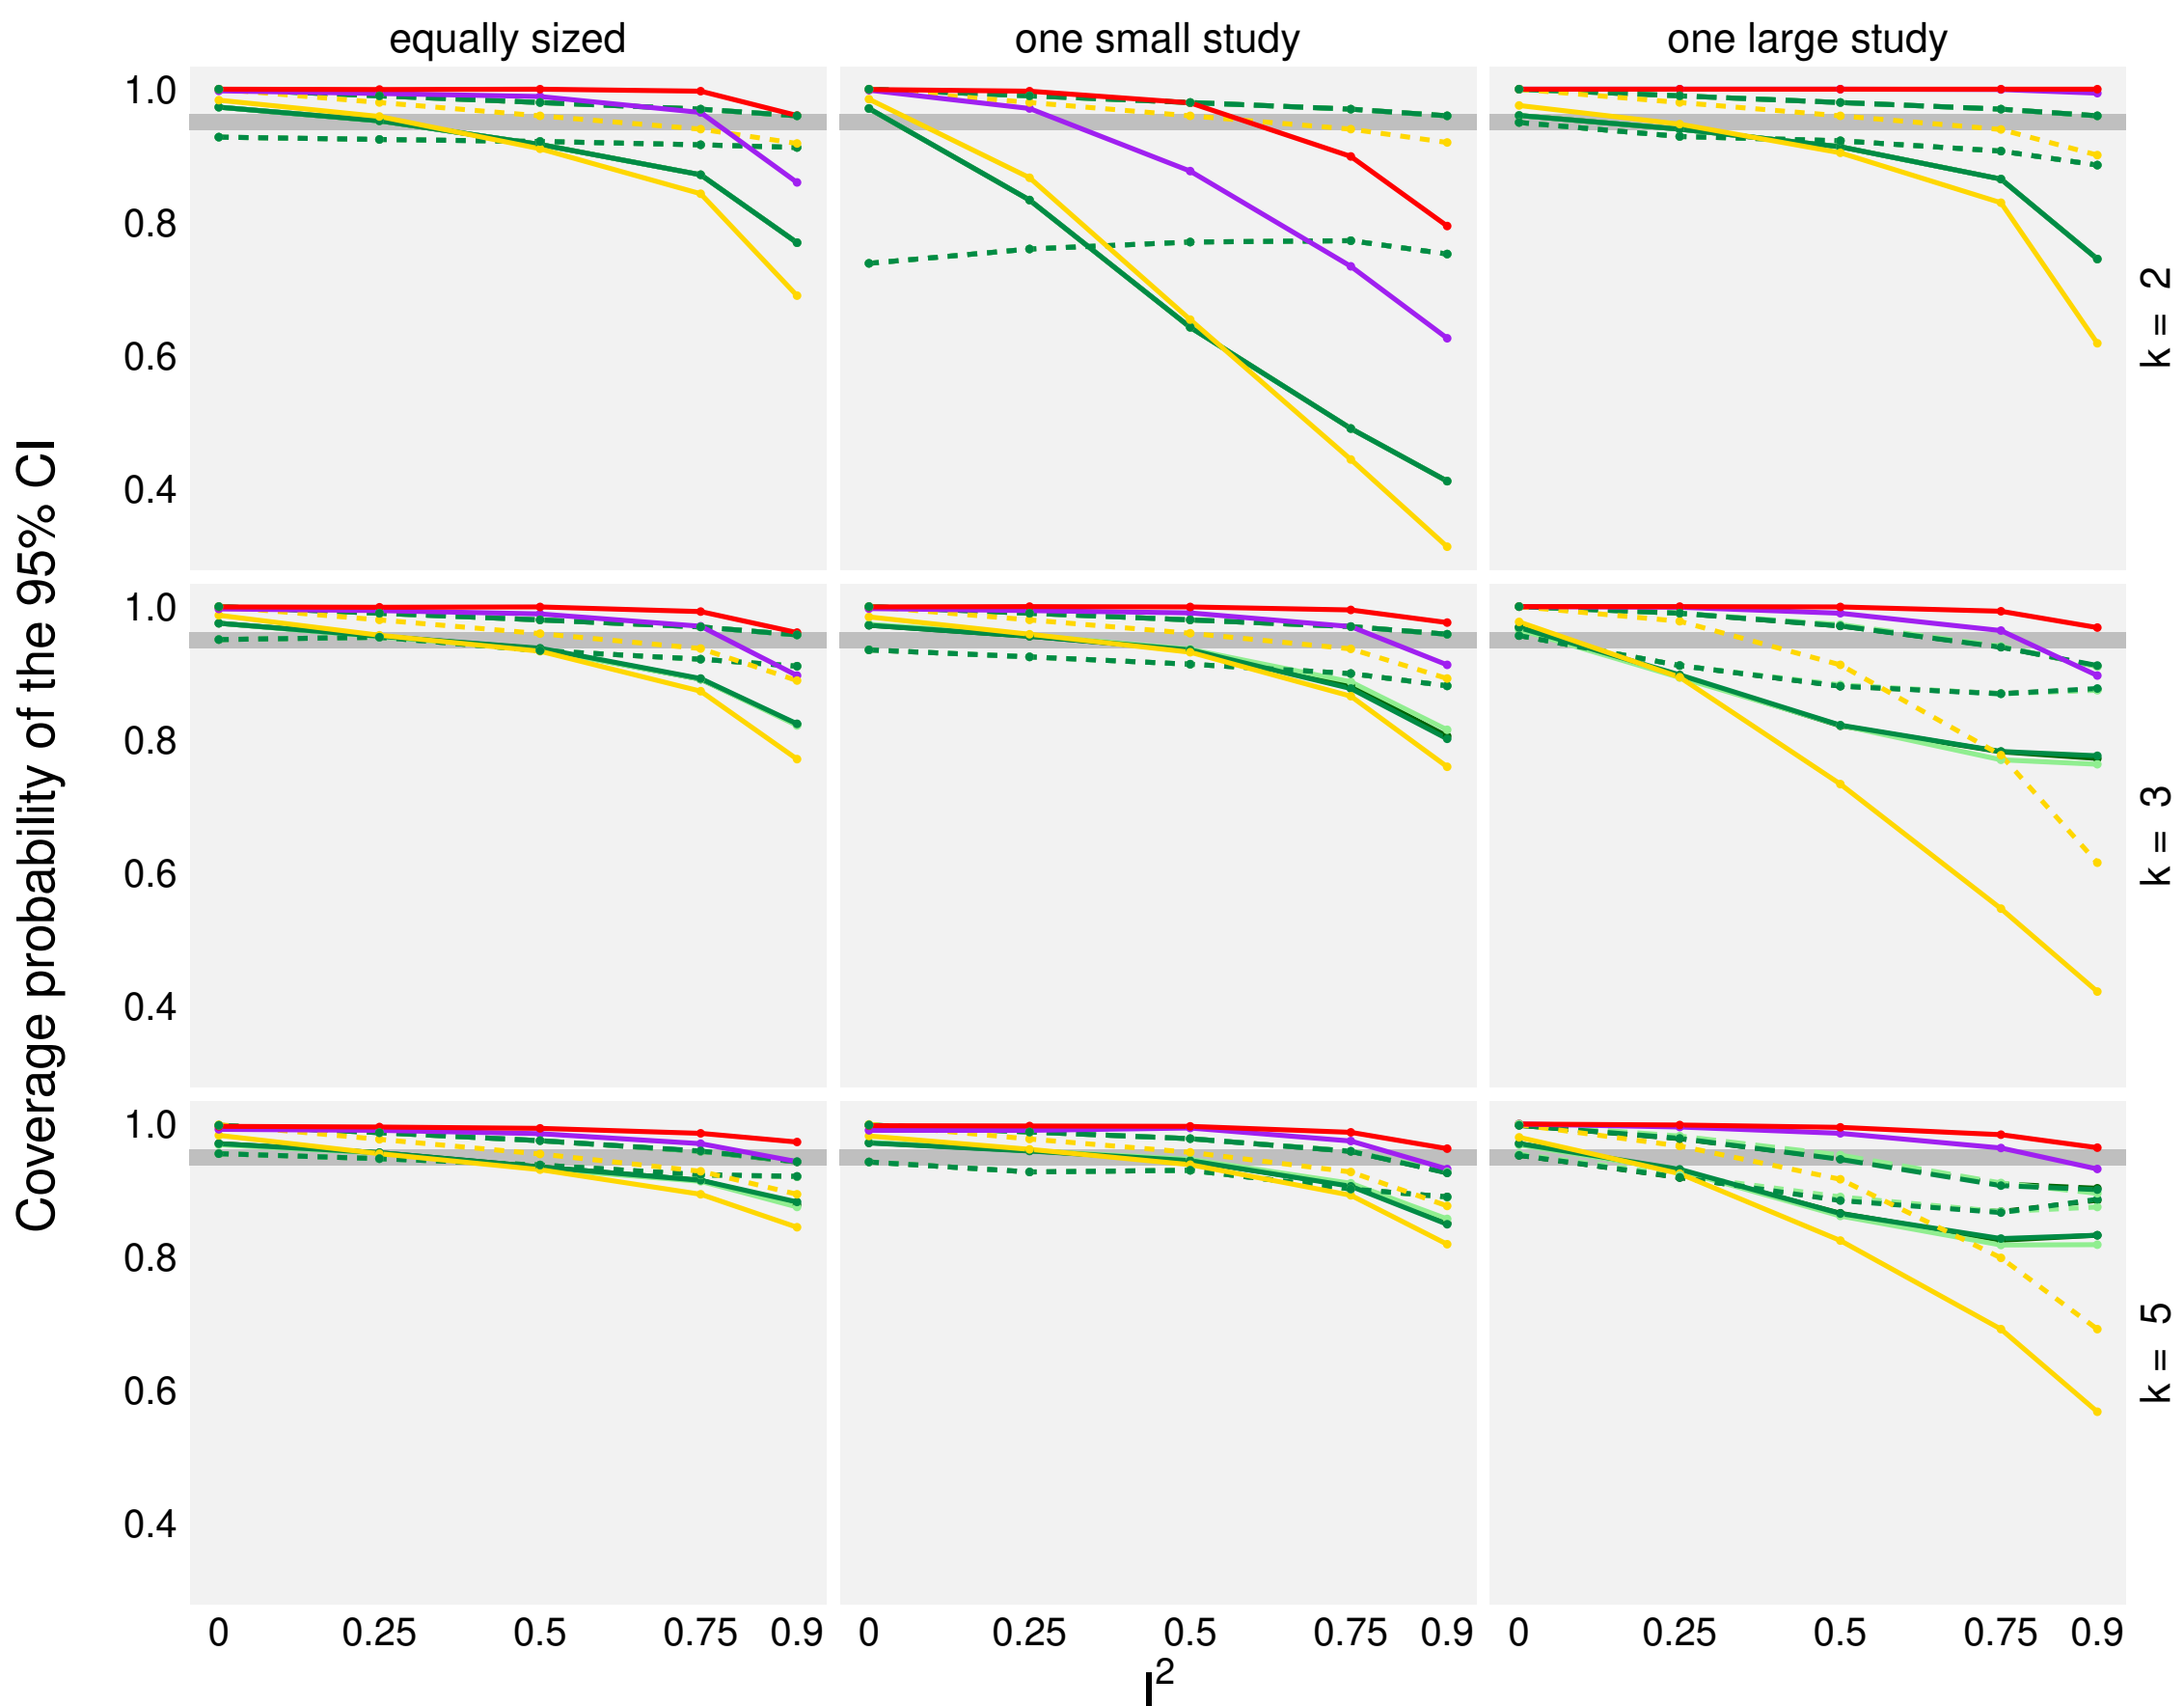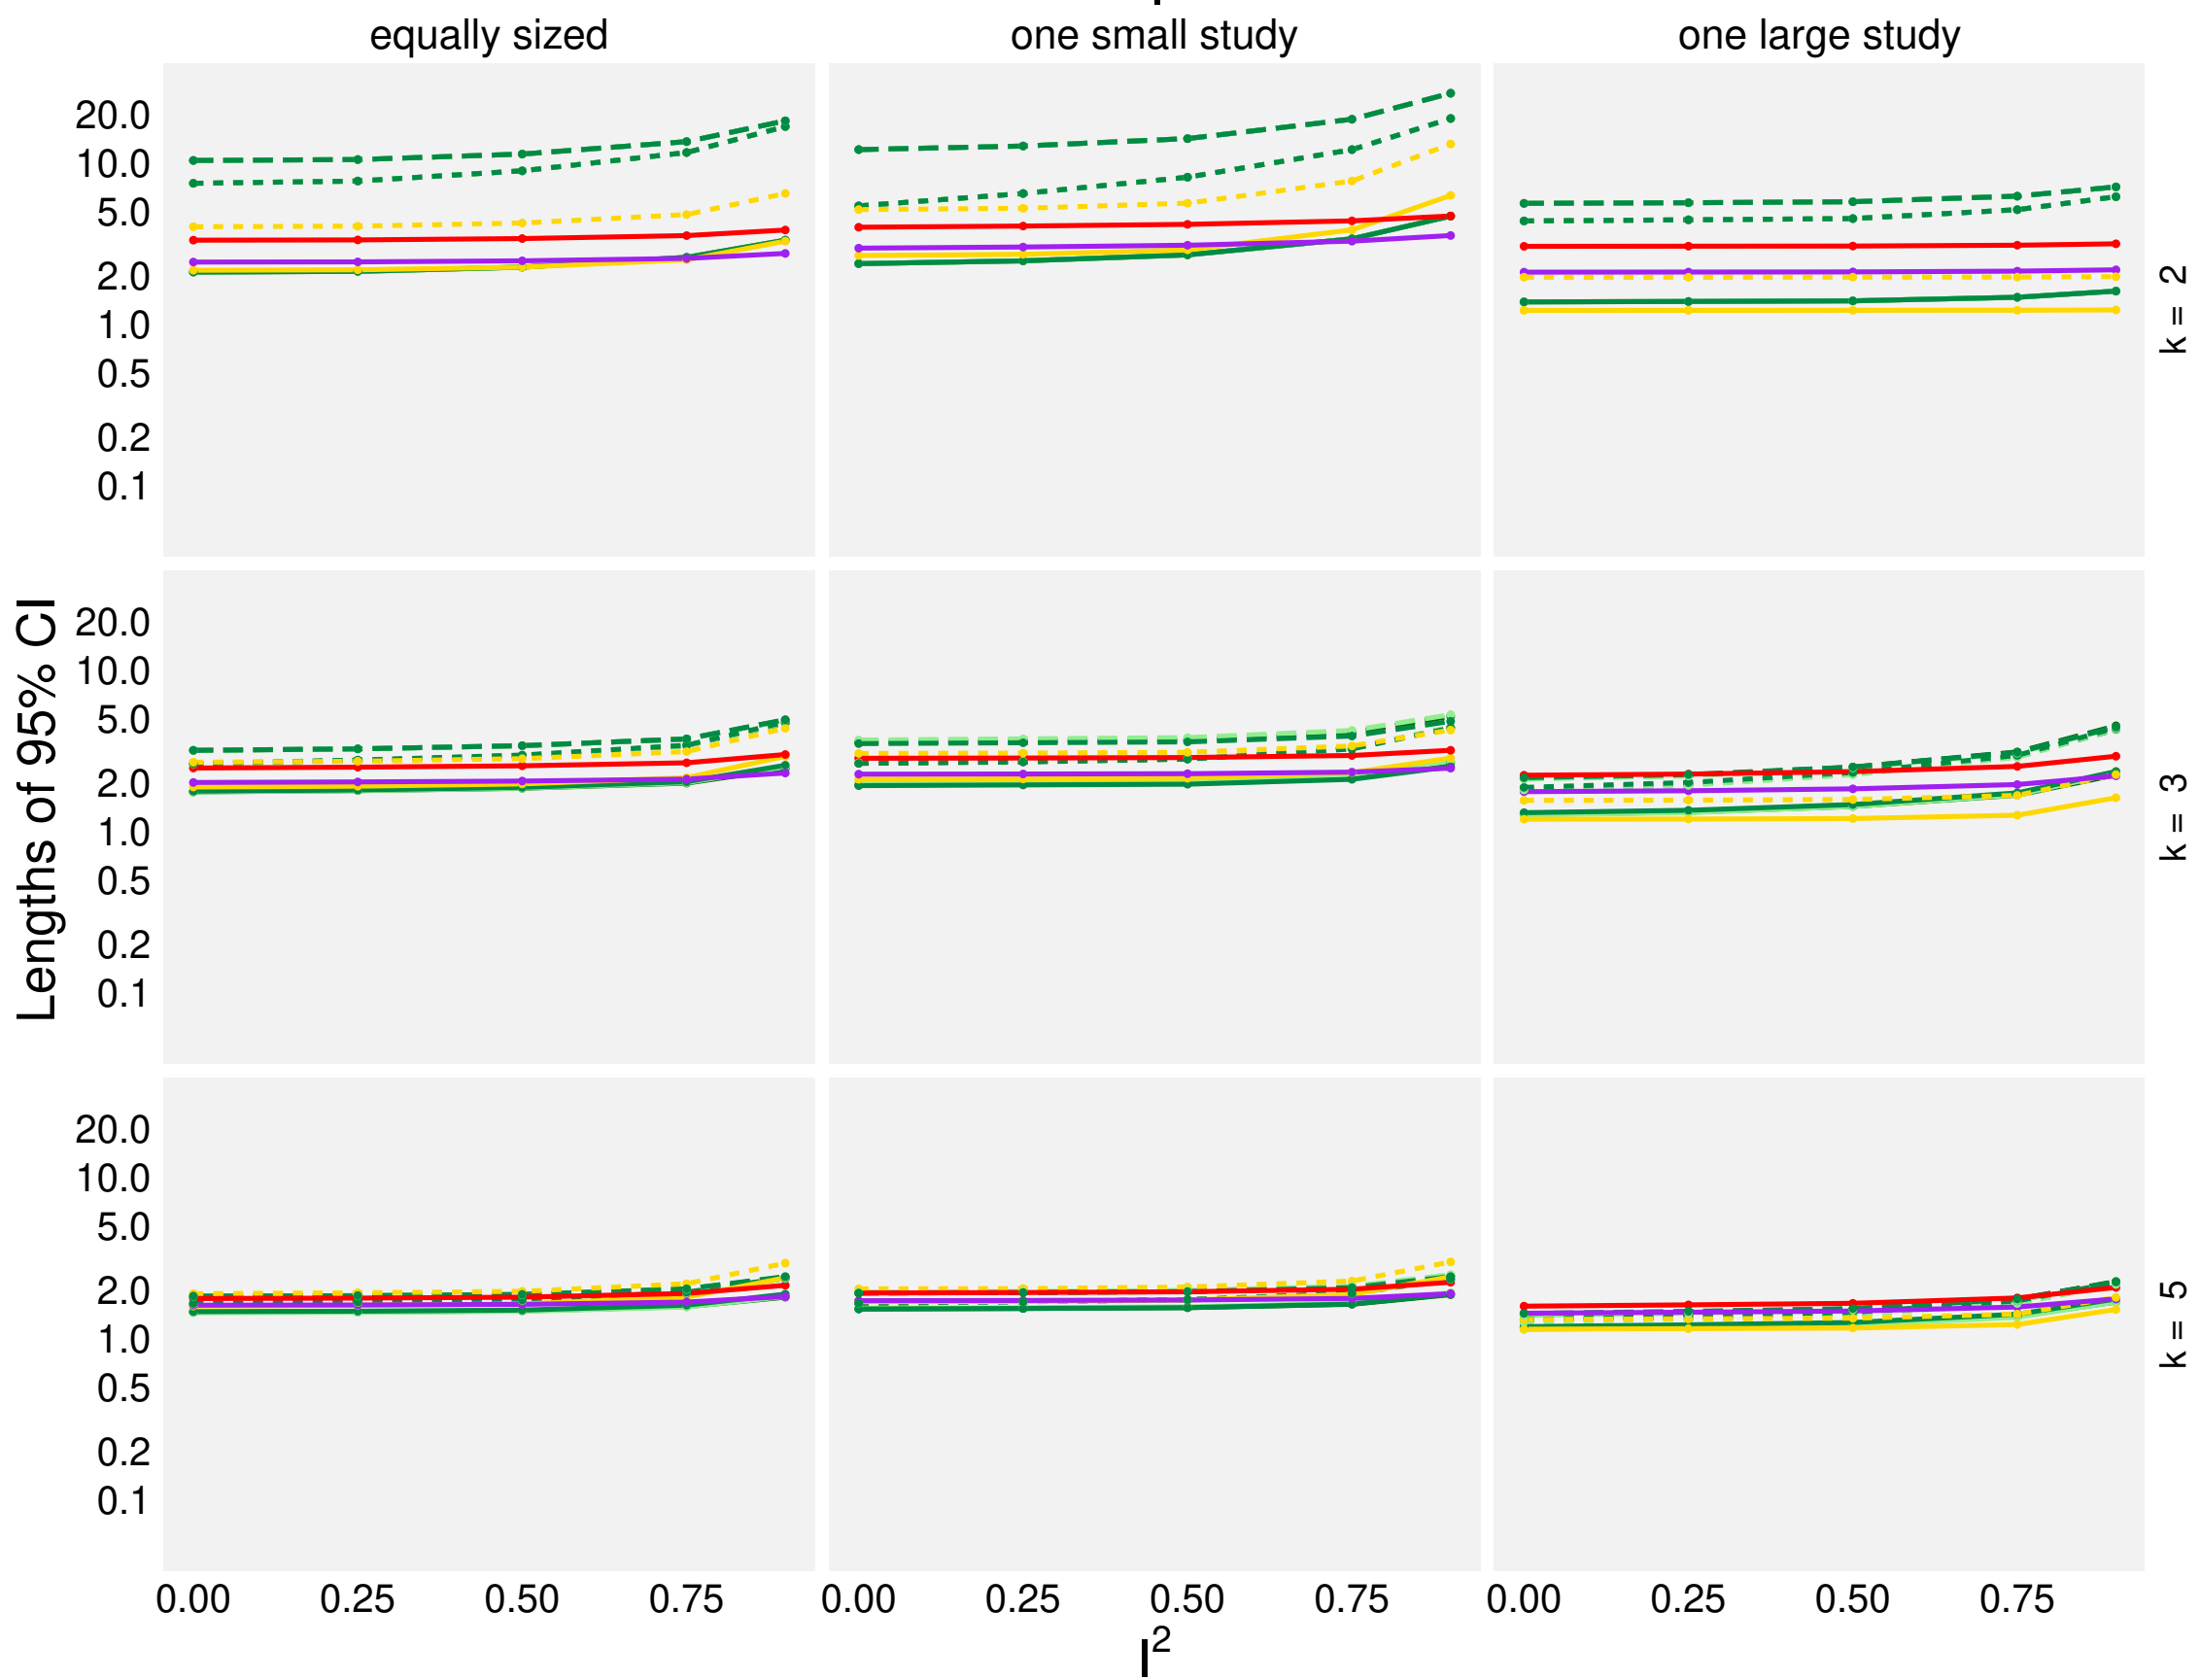

— NN – DL      — PN – PL      — normal quantiles  
 — NN – REML      — NN – Bayes HN(0.5)      - - HKSJ or Student's t  
 — NN – EB      — NN – Bayes HN(1)      - - mHKSJ

RR  
( $n_i=50, \pi_0=0.3$ )

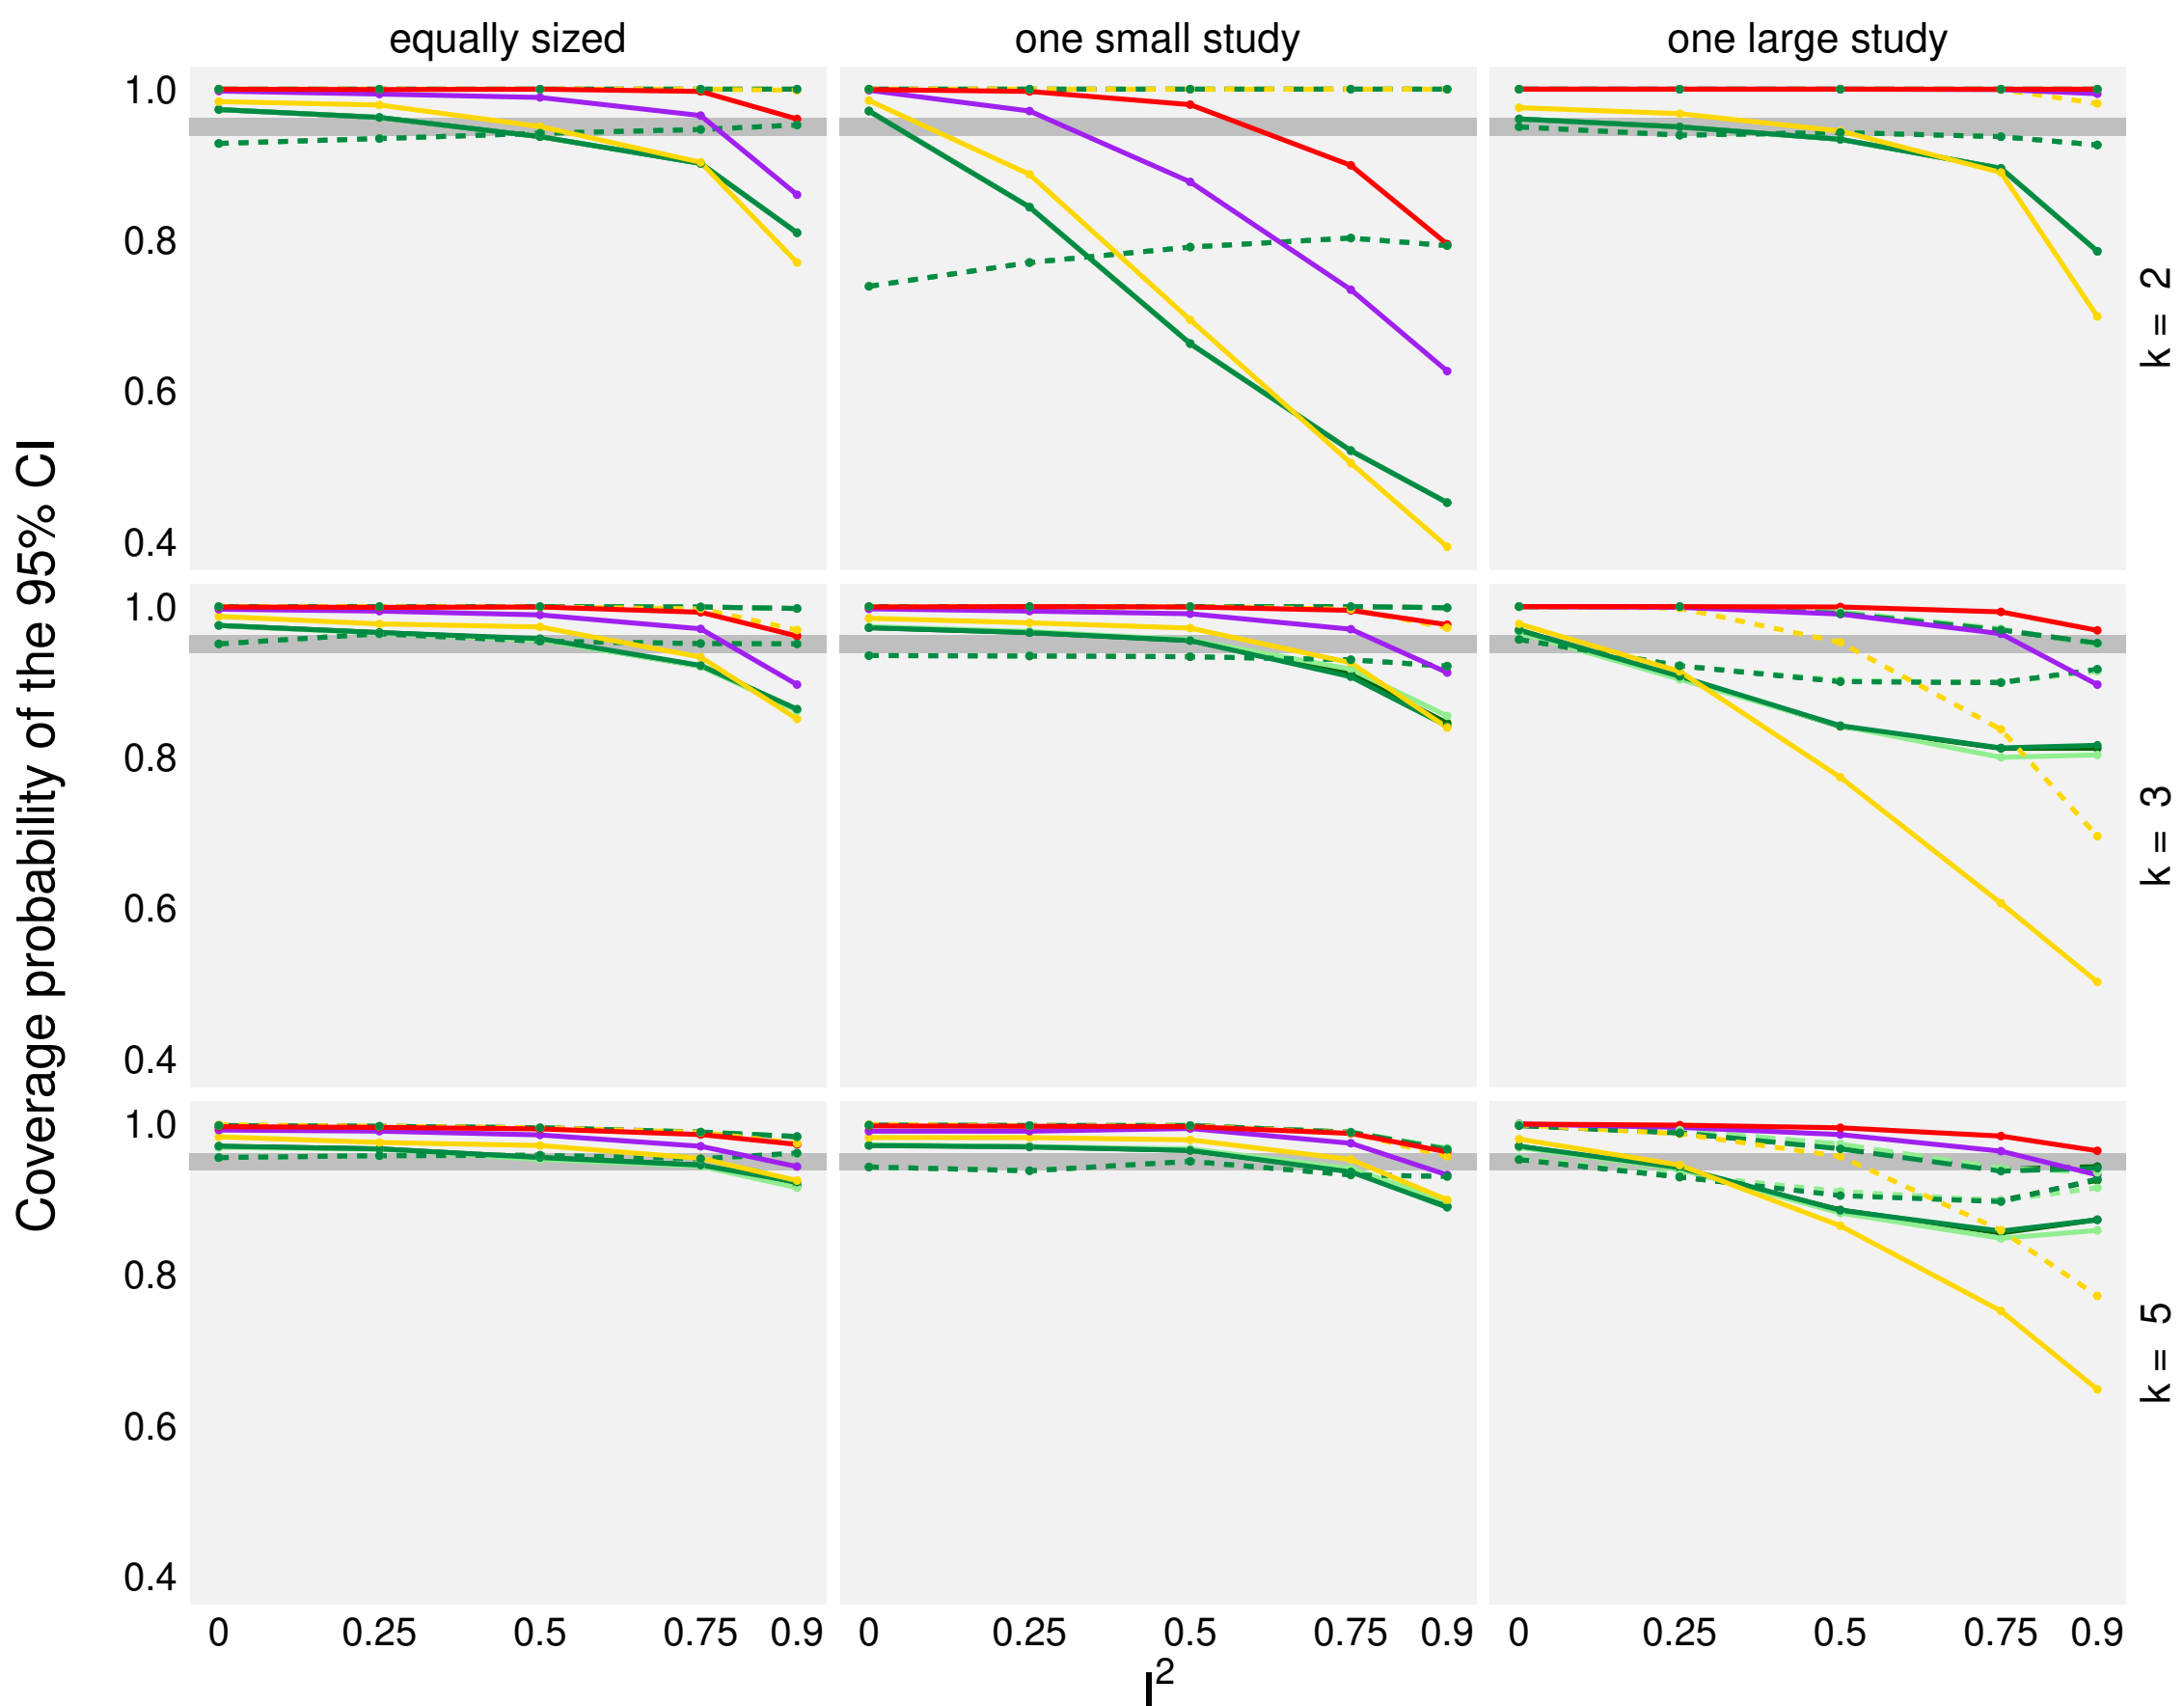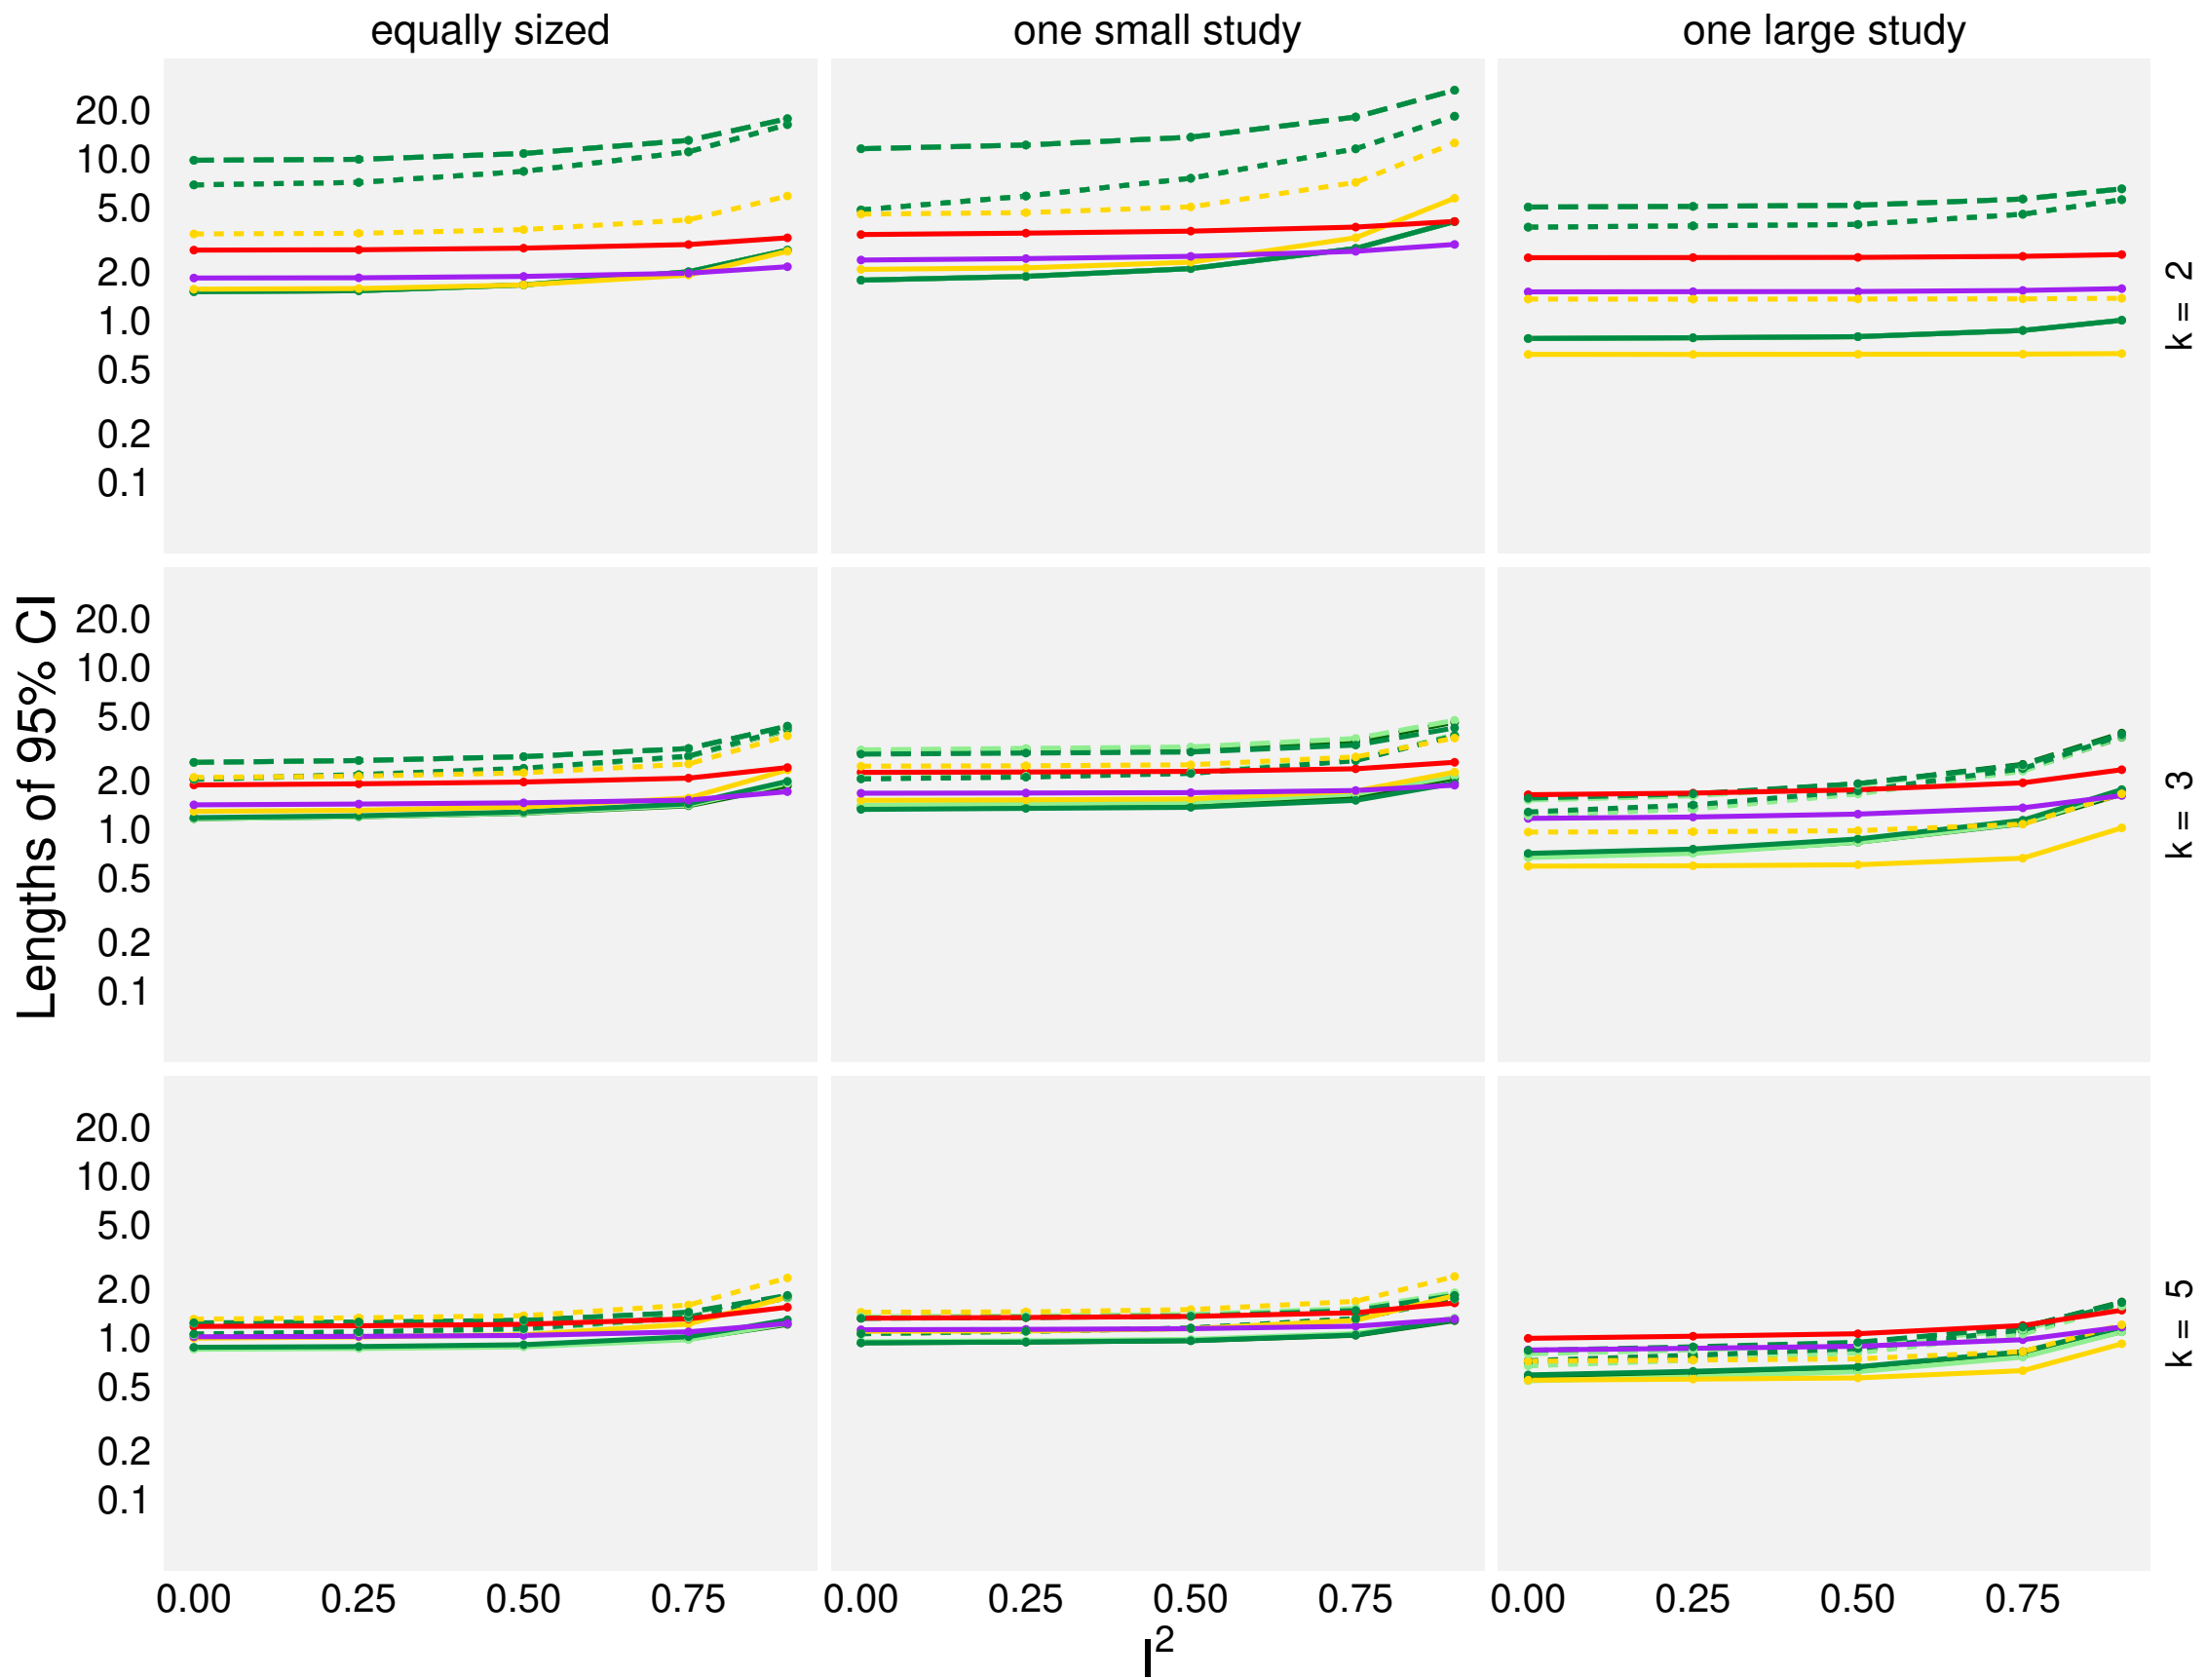

— NN – DL      — PN – PL      — normal quantiles  
 — NN – REML      — NN – Bayes HN(0.5)      - - HKSJ or Student's t  
 — NN – EB      — NN – Bayes HN(1)      - - mHKSJ

RR  
( $n_i=50, \pi_0=0.5$ )

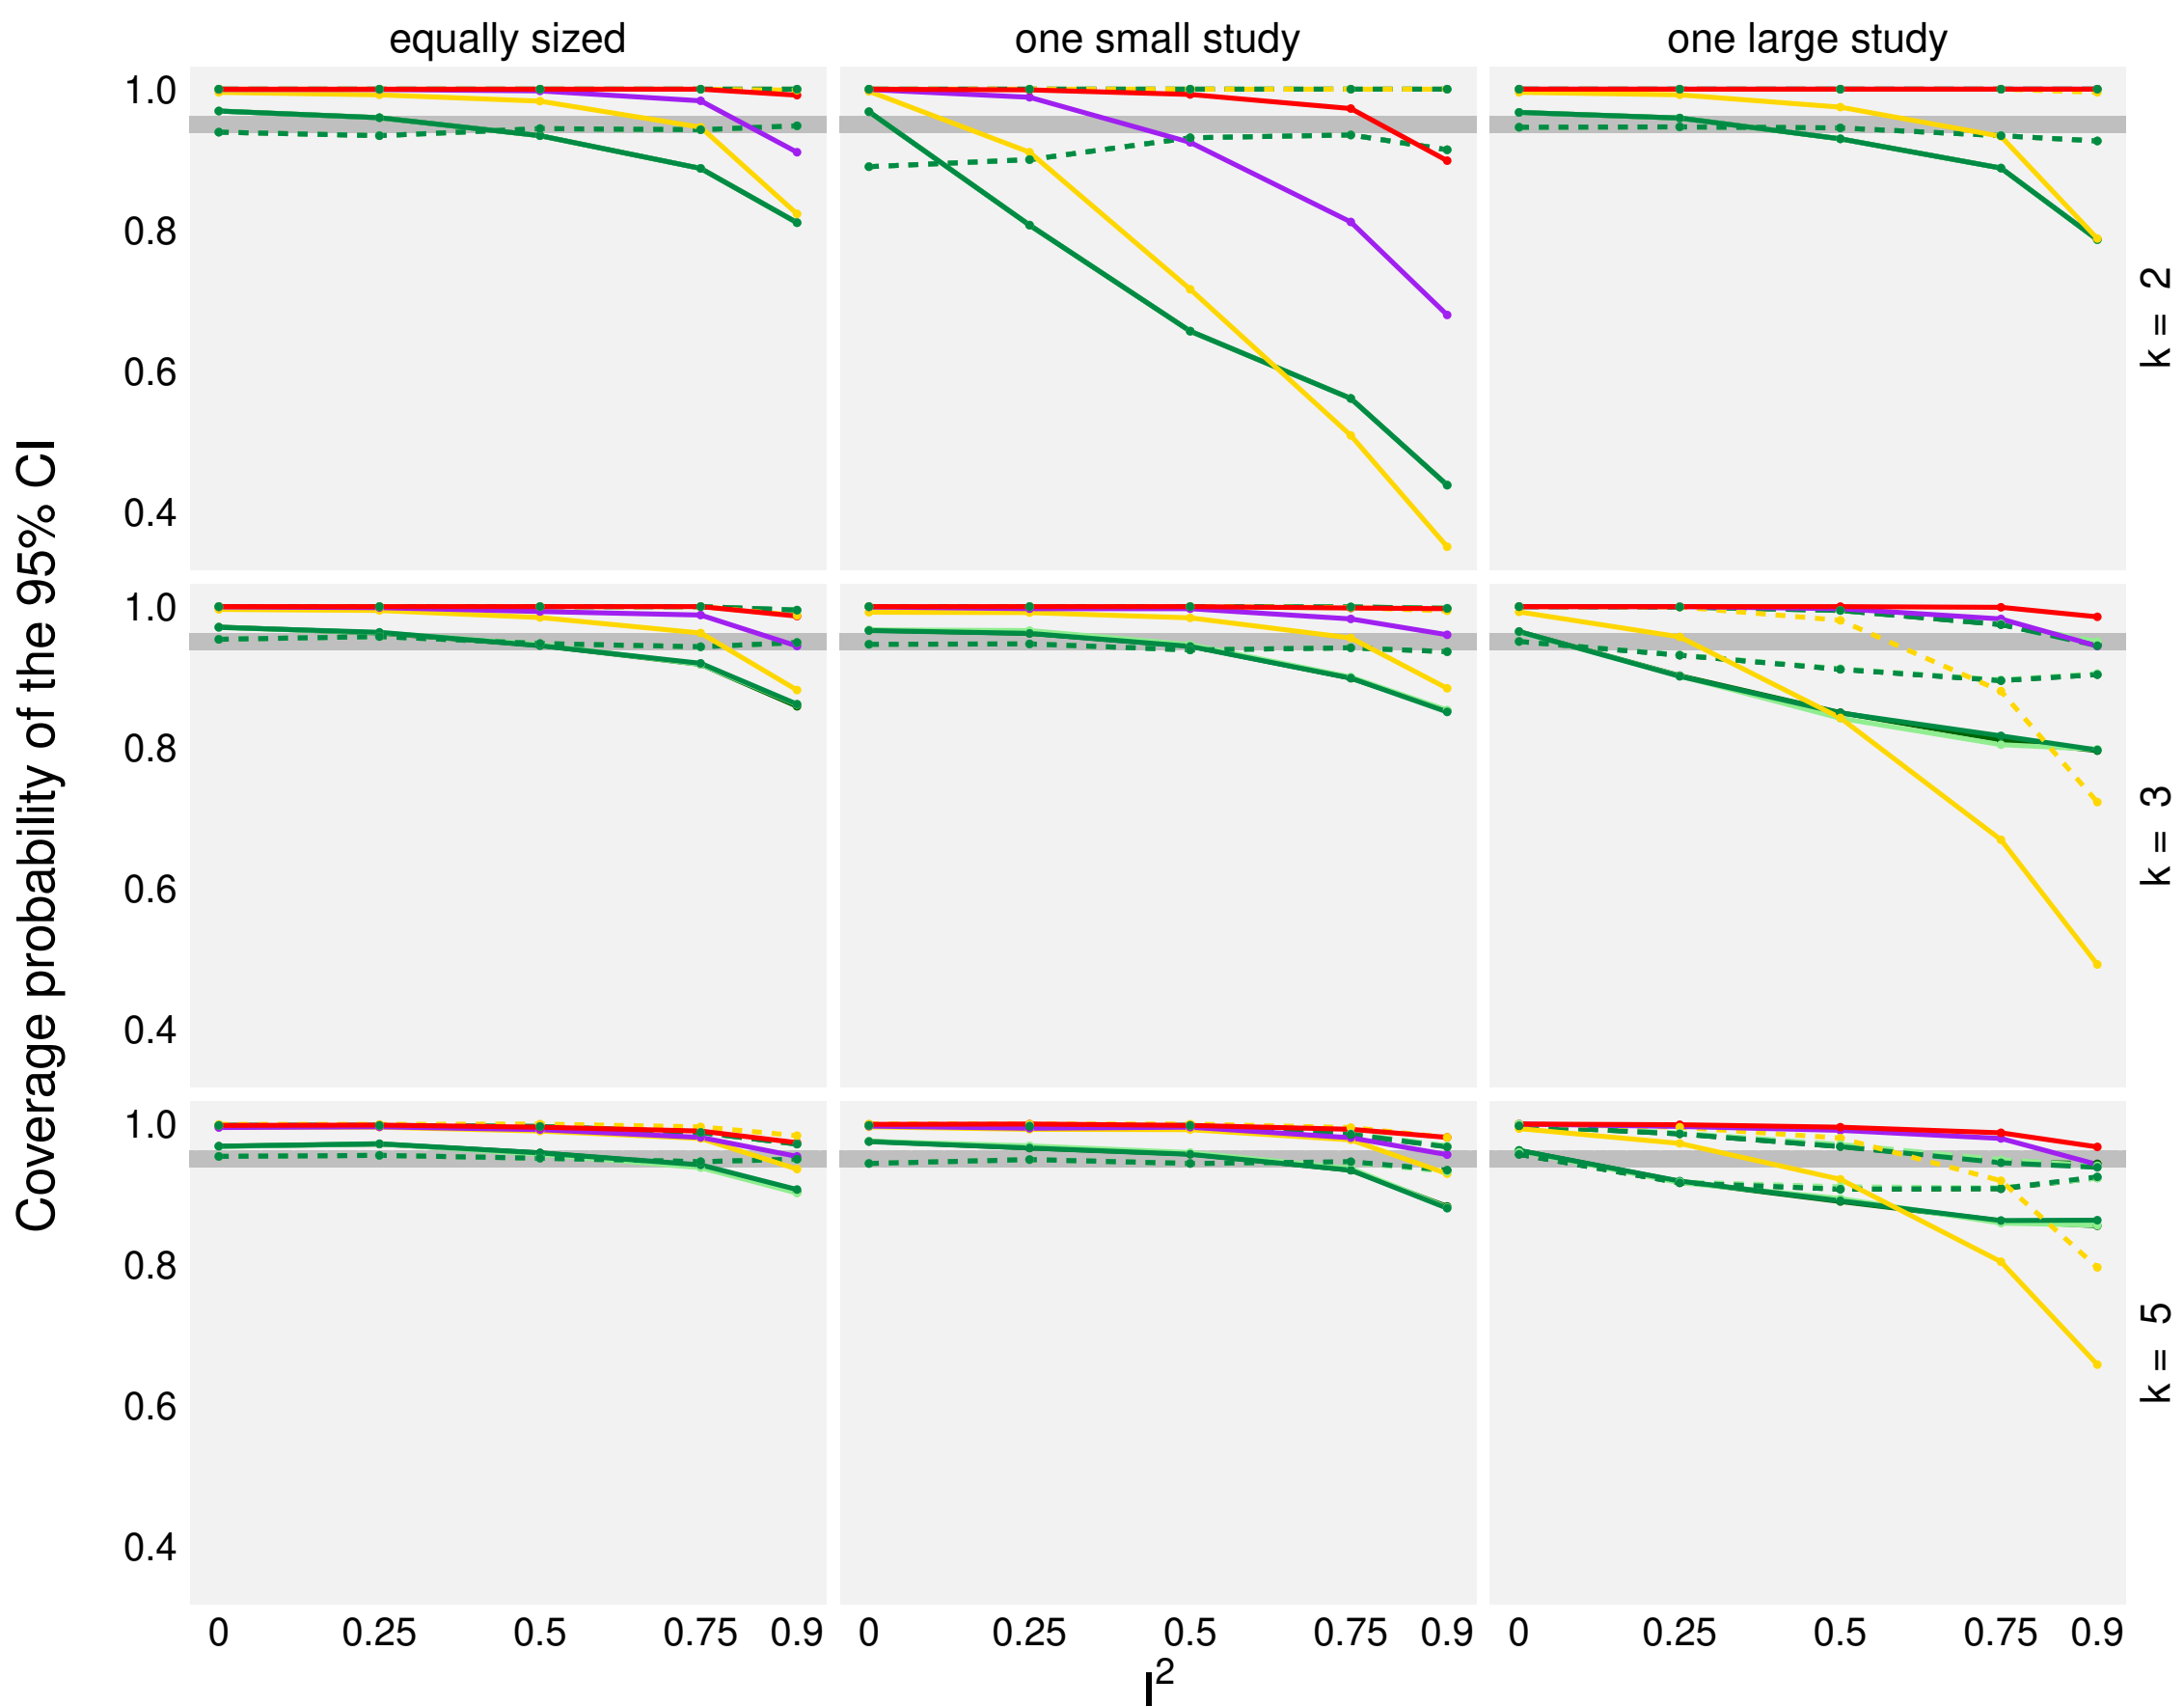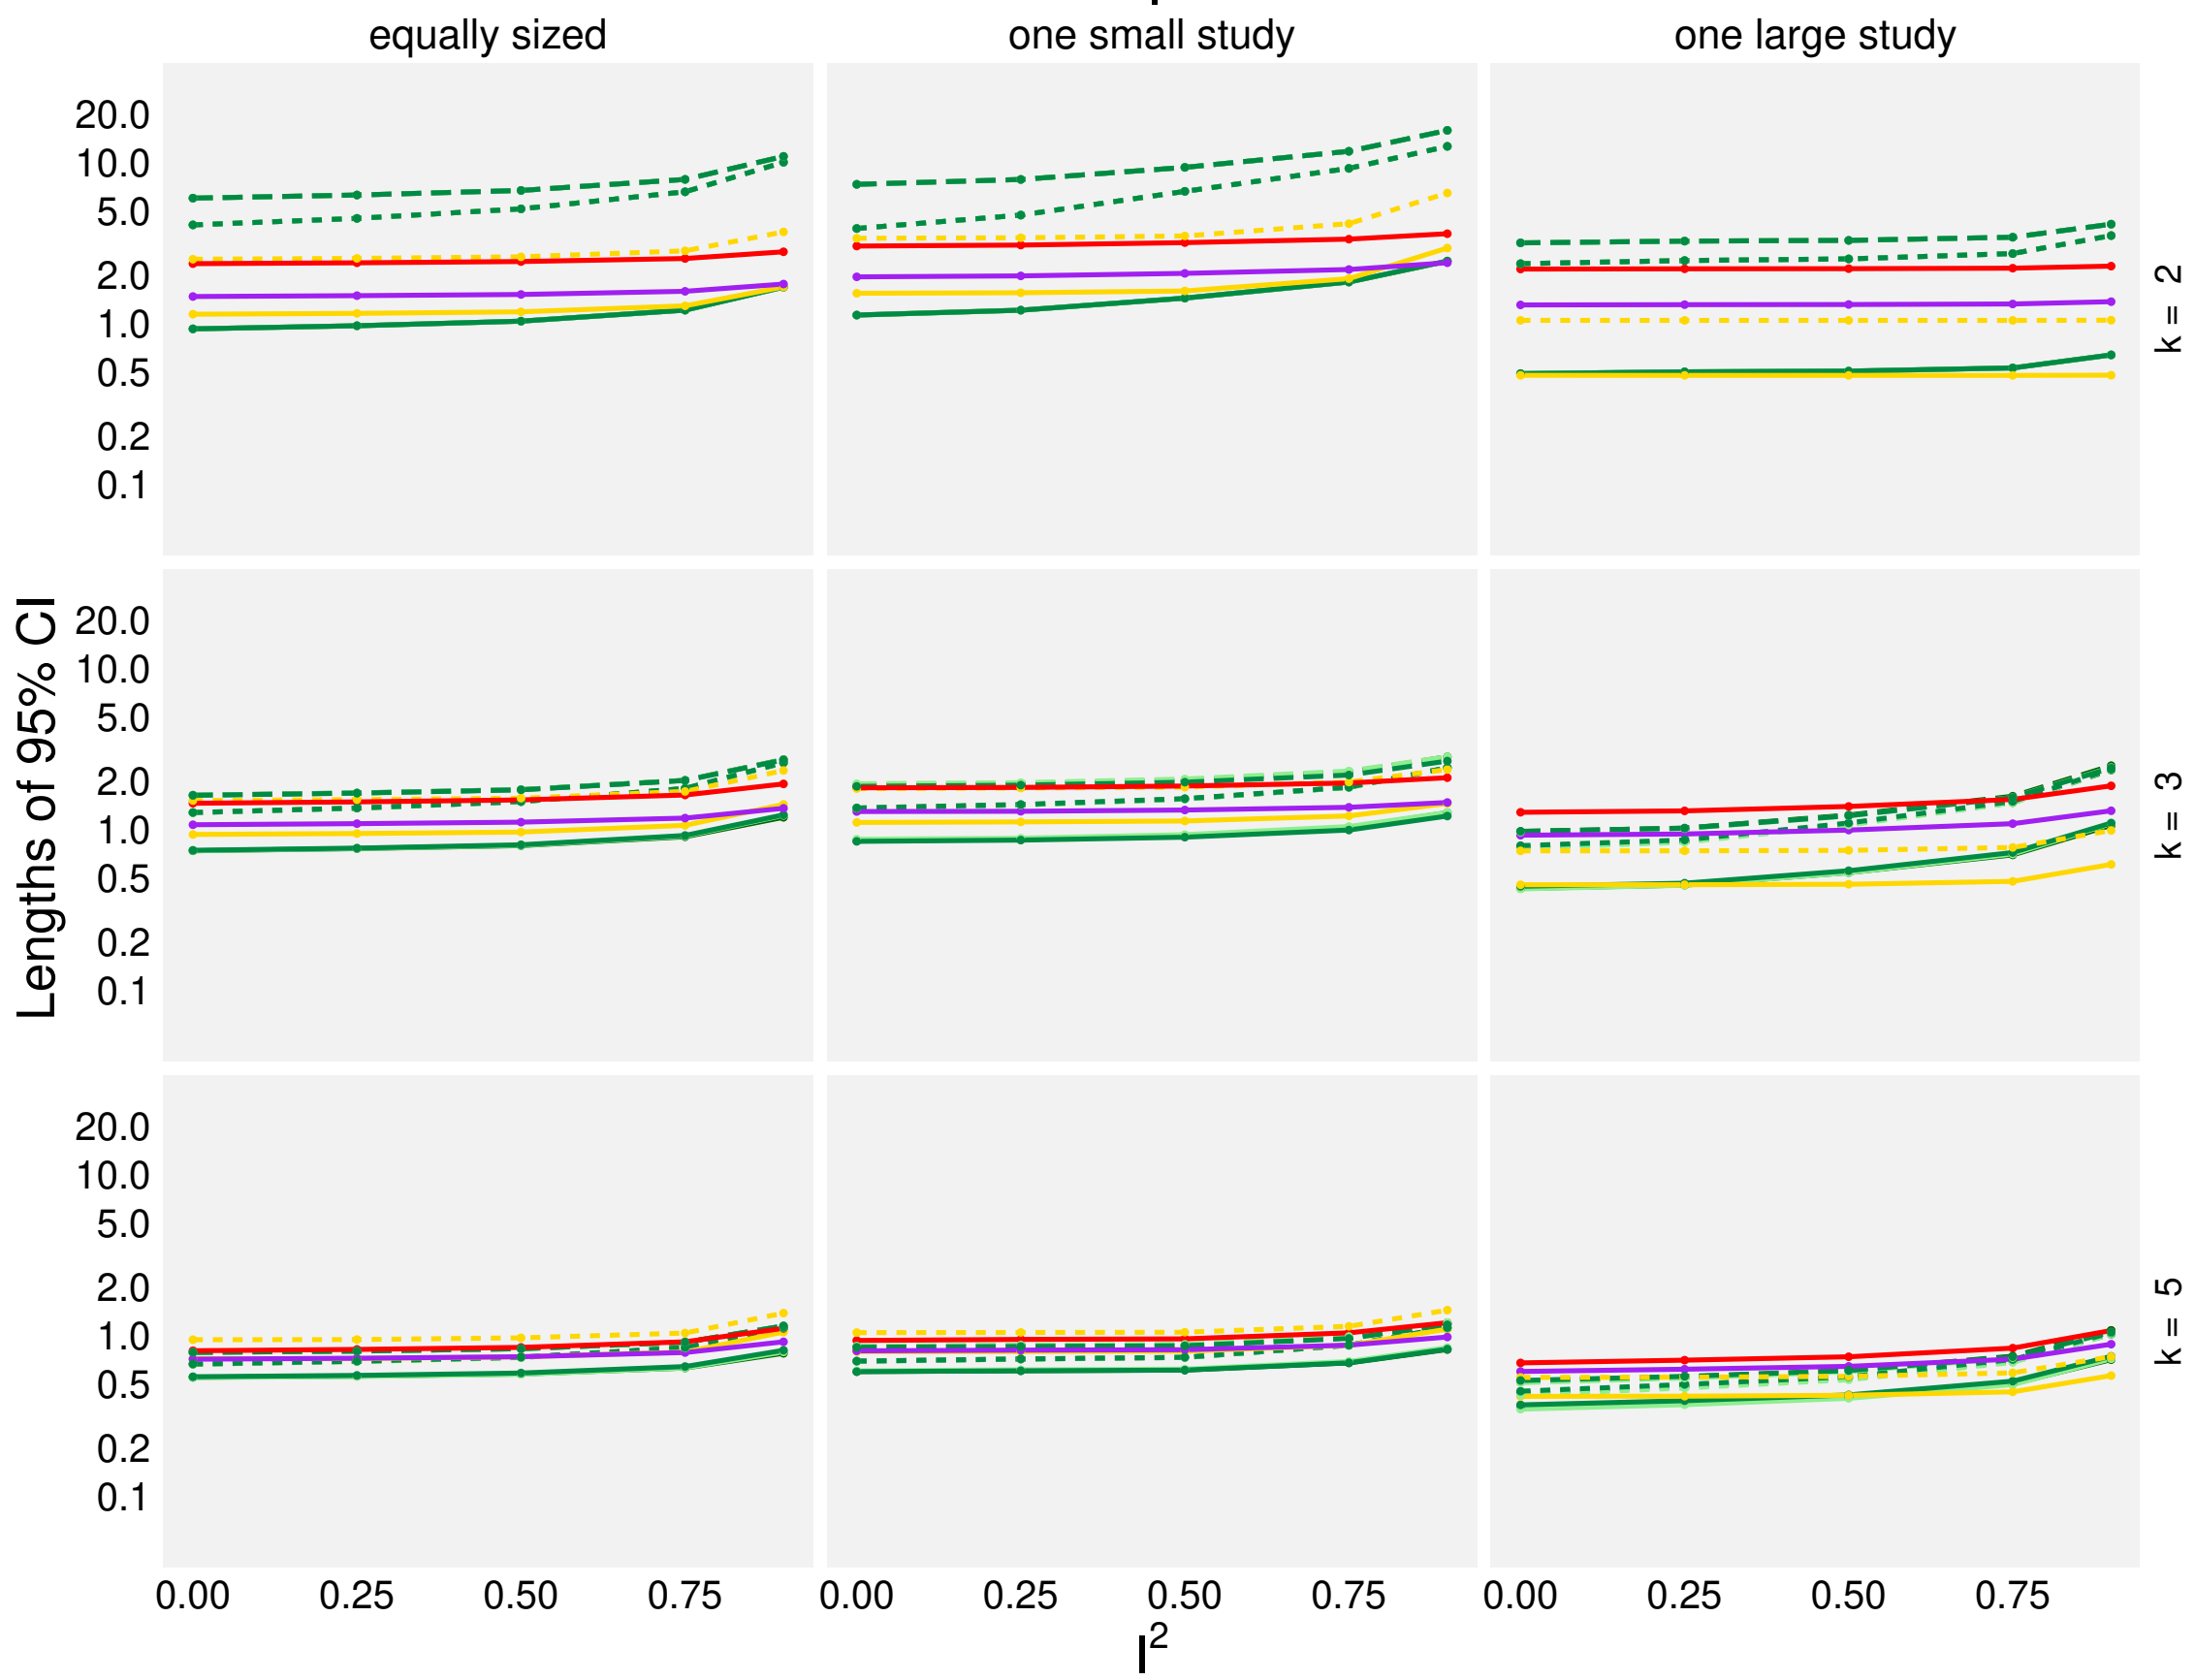

NN - DL      NN - PL      — normal quantiles  
 NN - REML      NN - Bayes HN(0.5)      - - HKSJ or Student's t  
 NN - EB      NN - Bayes HN(1)      ··· mHKSJ

RR  
( $n_i=50, \pi_0=0.7$ )

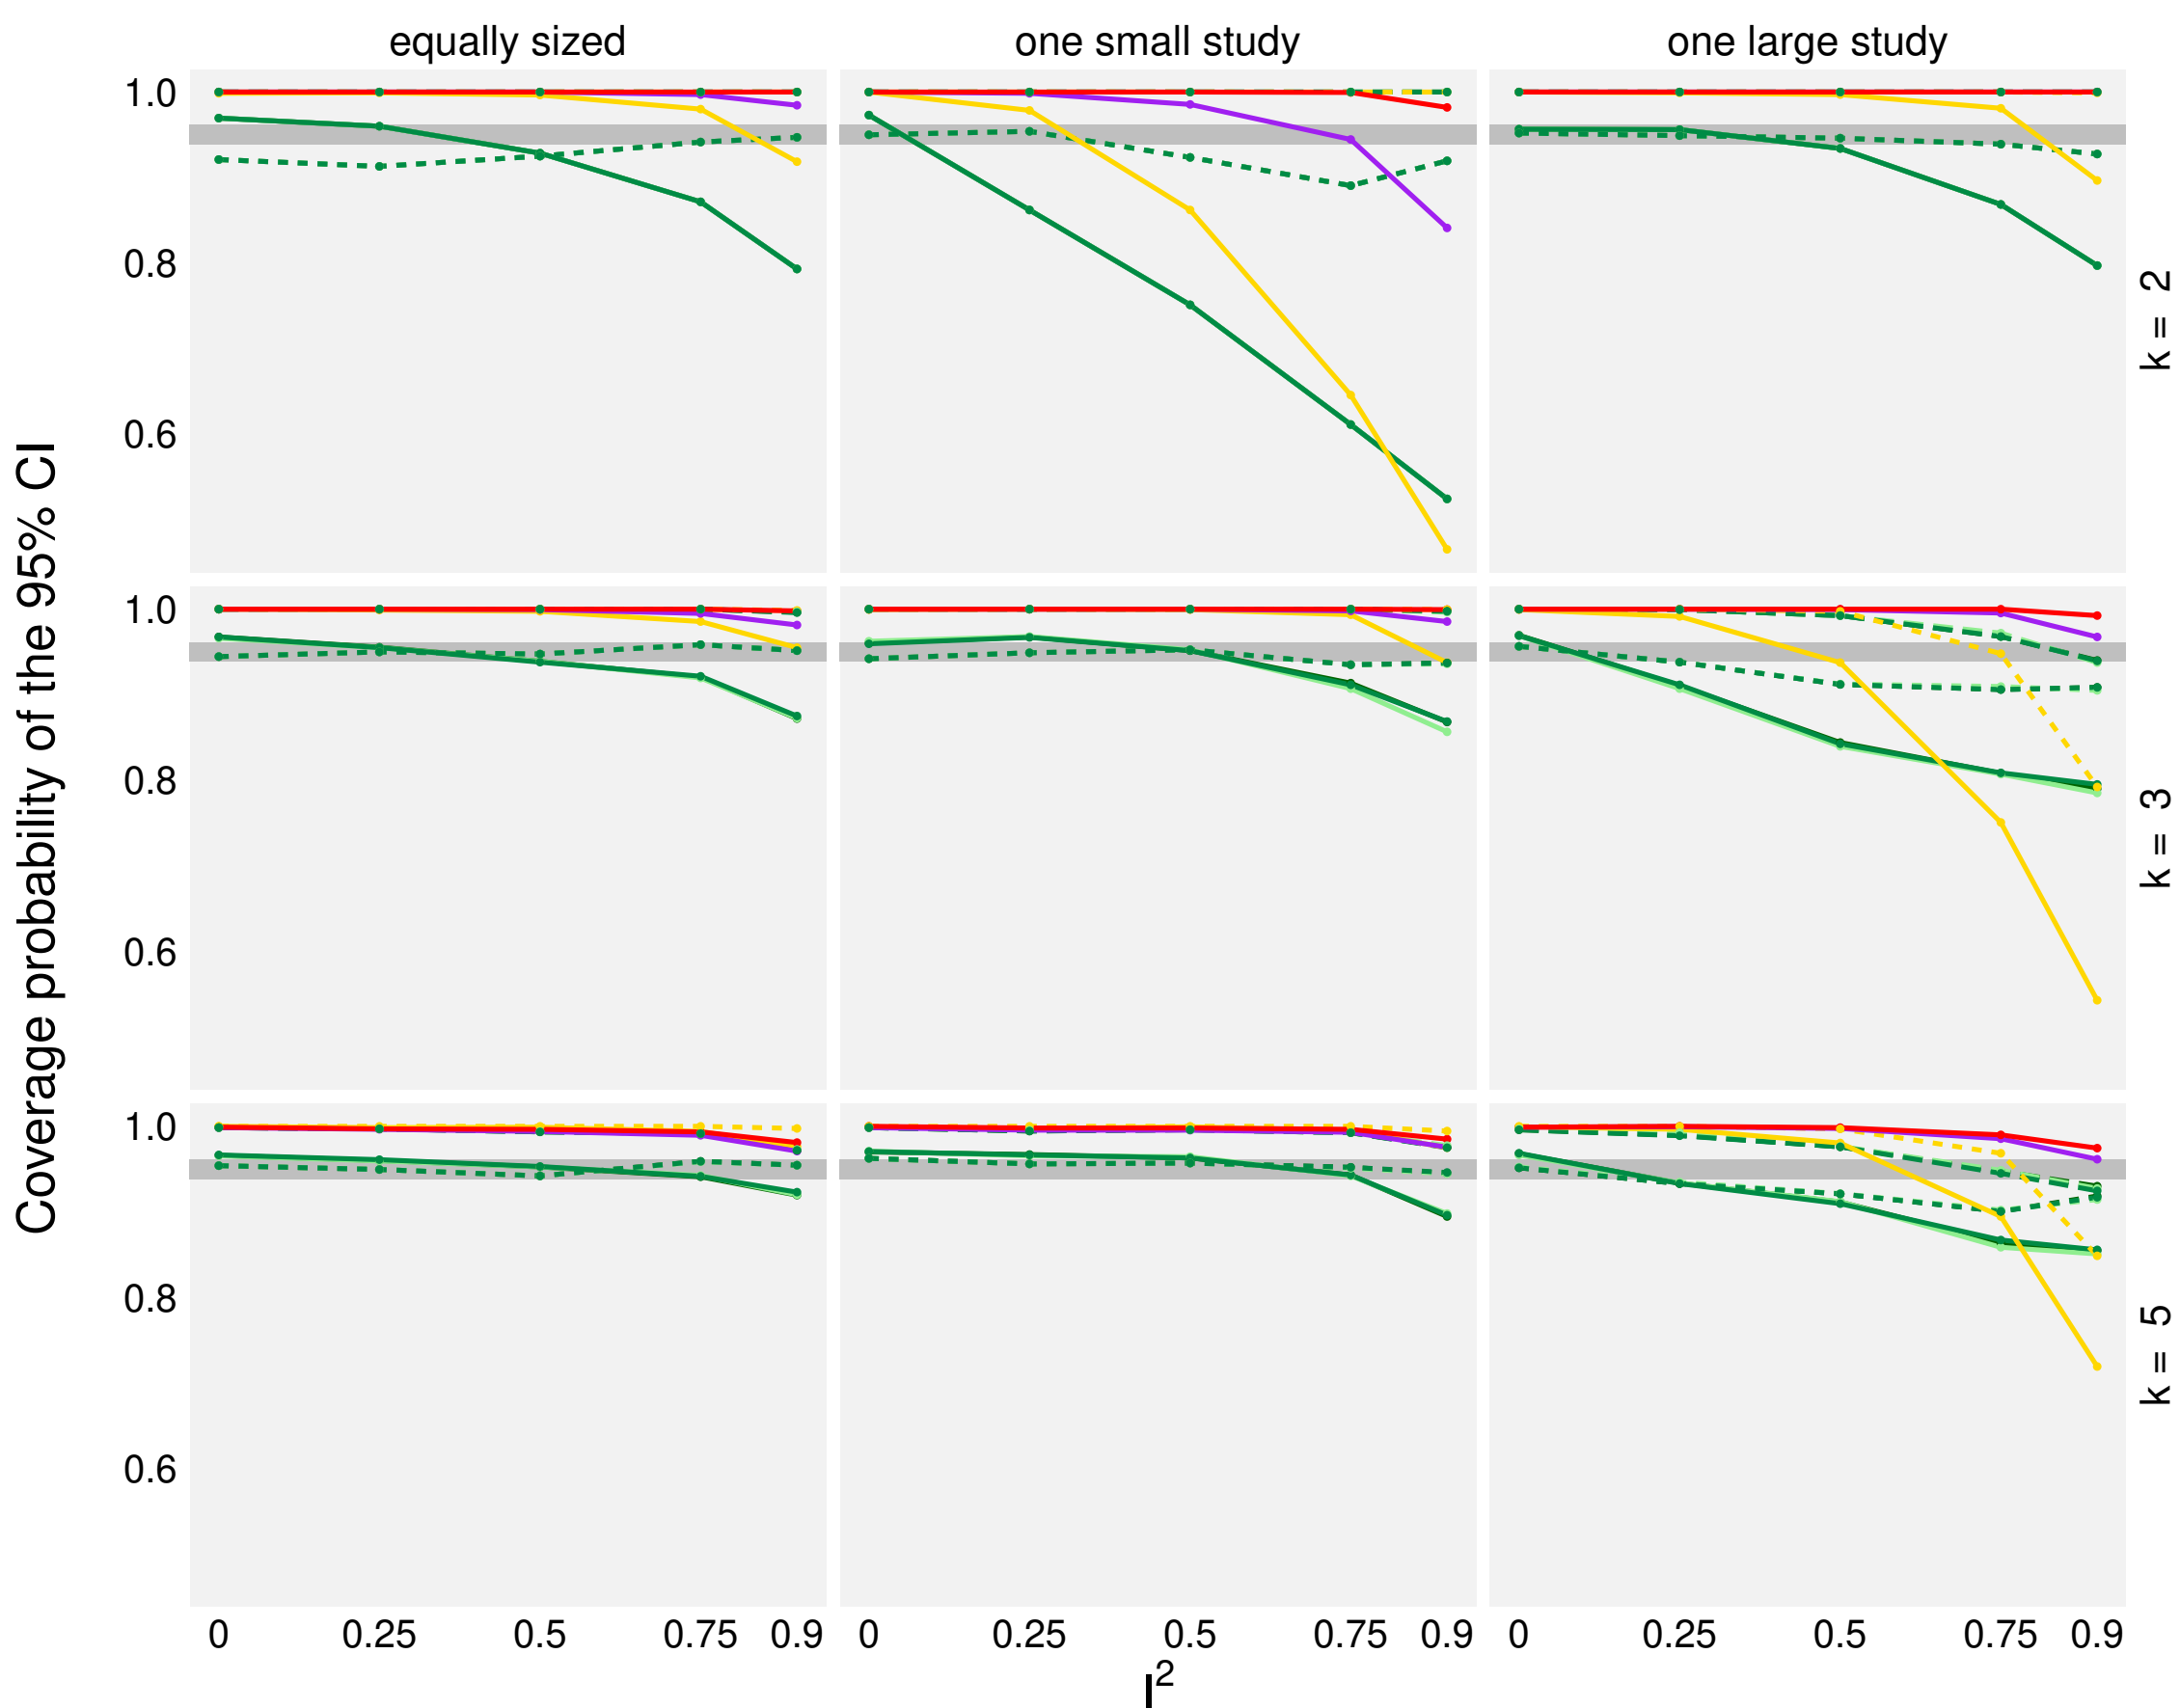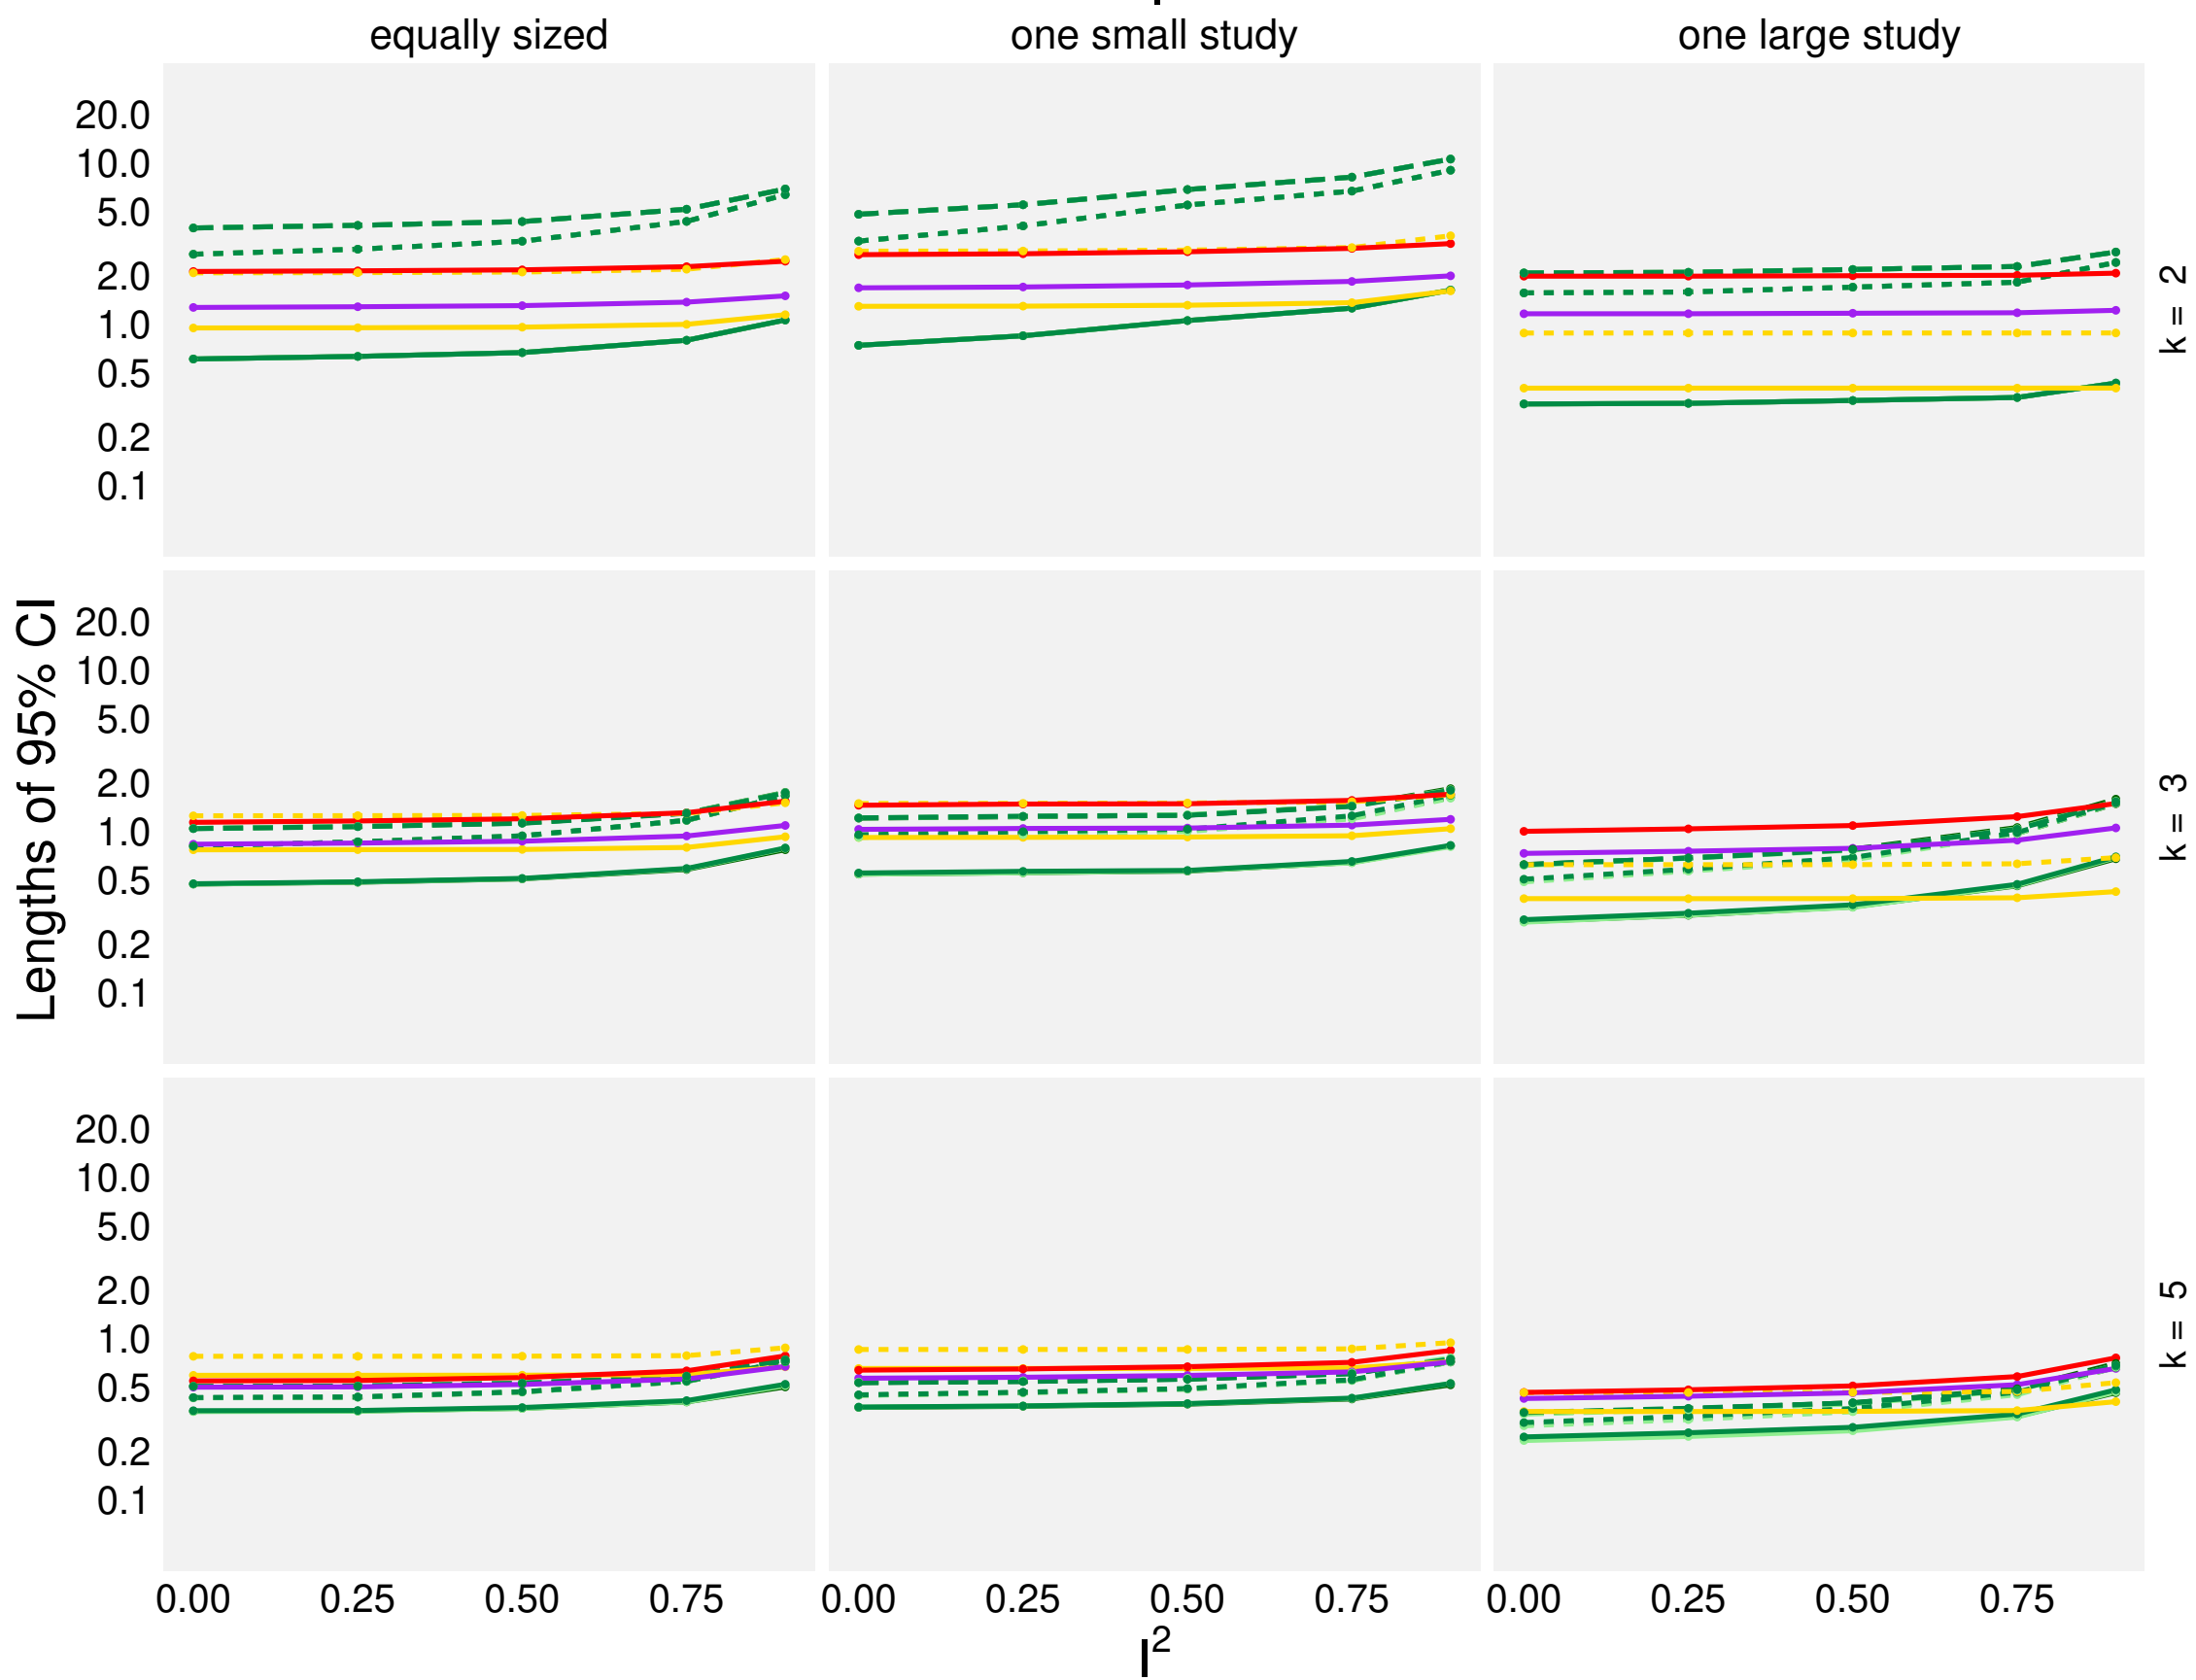

— NN – DL  
 — NN – REML  
 — NN – EB  
 — PN – PL  
 — NN – Bayes HN(0.5)  
 — NN – Bayes HN(1)  
 — normal quantiles  
 - - HKSJ or Student's t  
 - - mHKSJ

RR  
( $n_i=50, \pi_0=0.9$ )

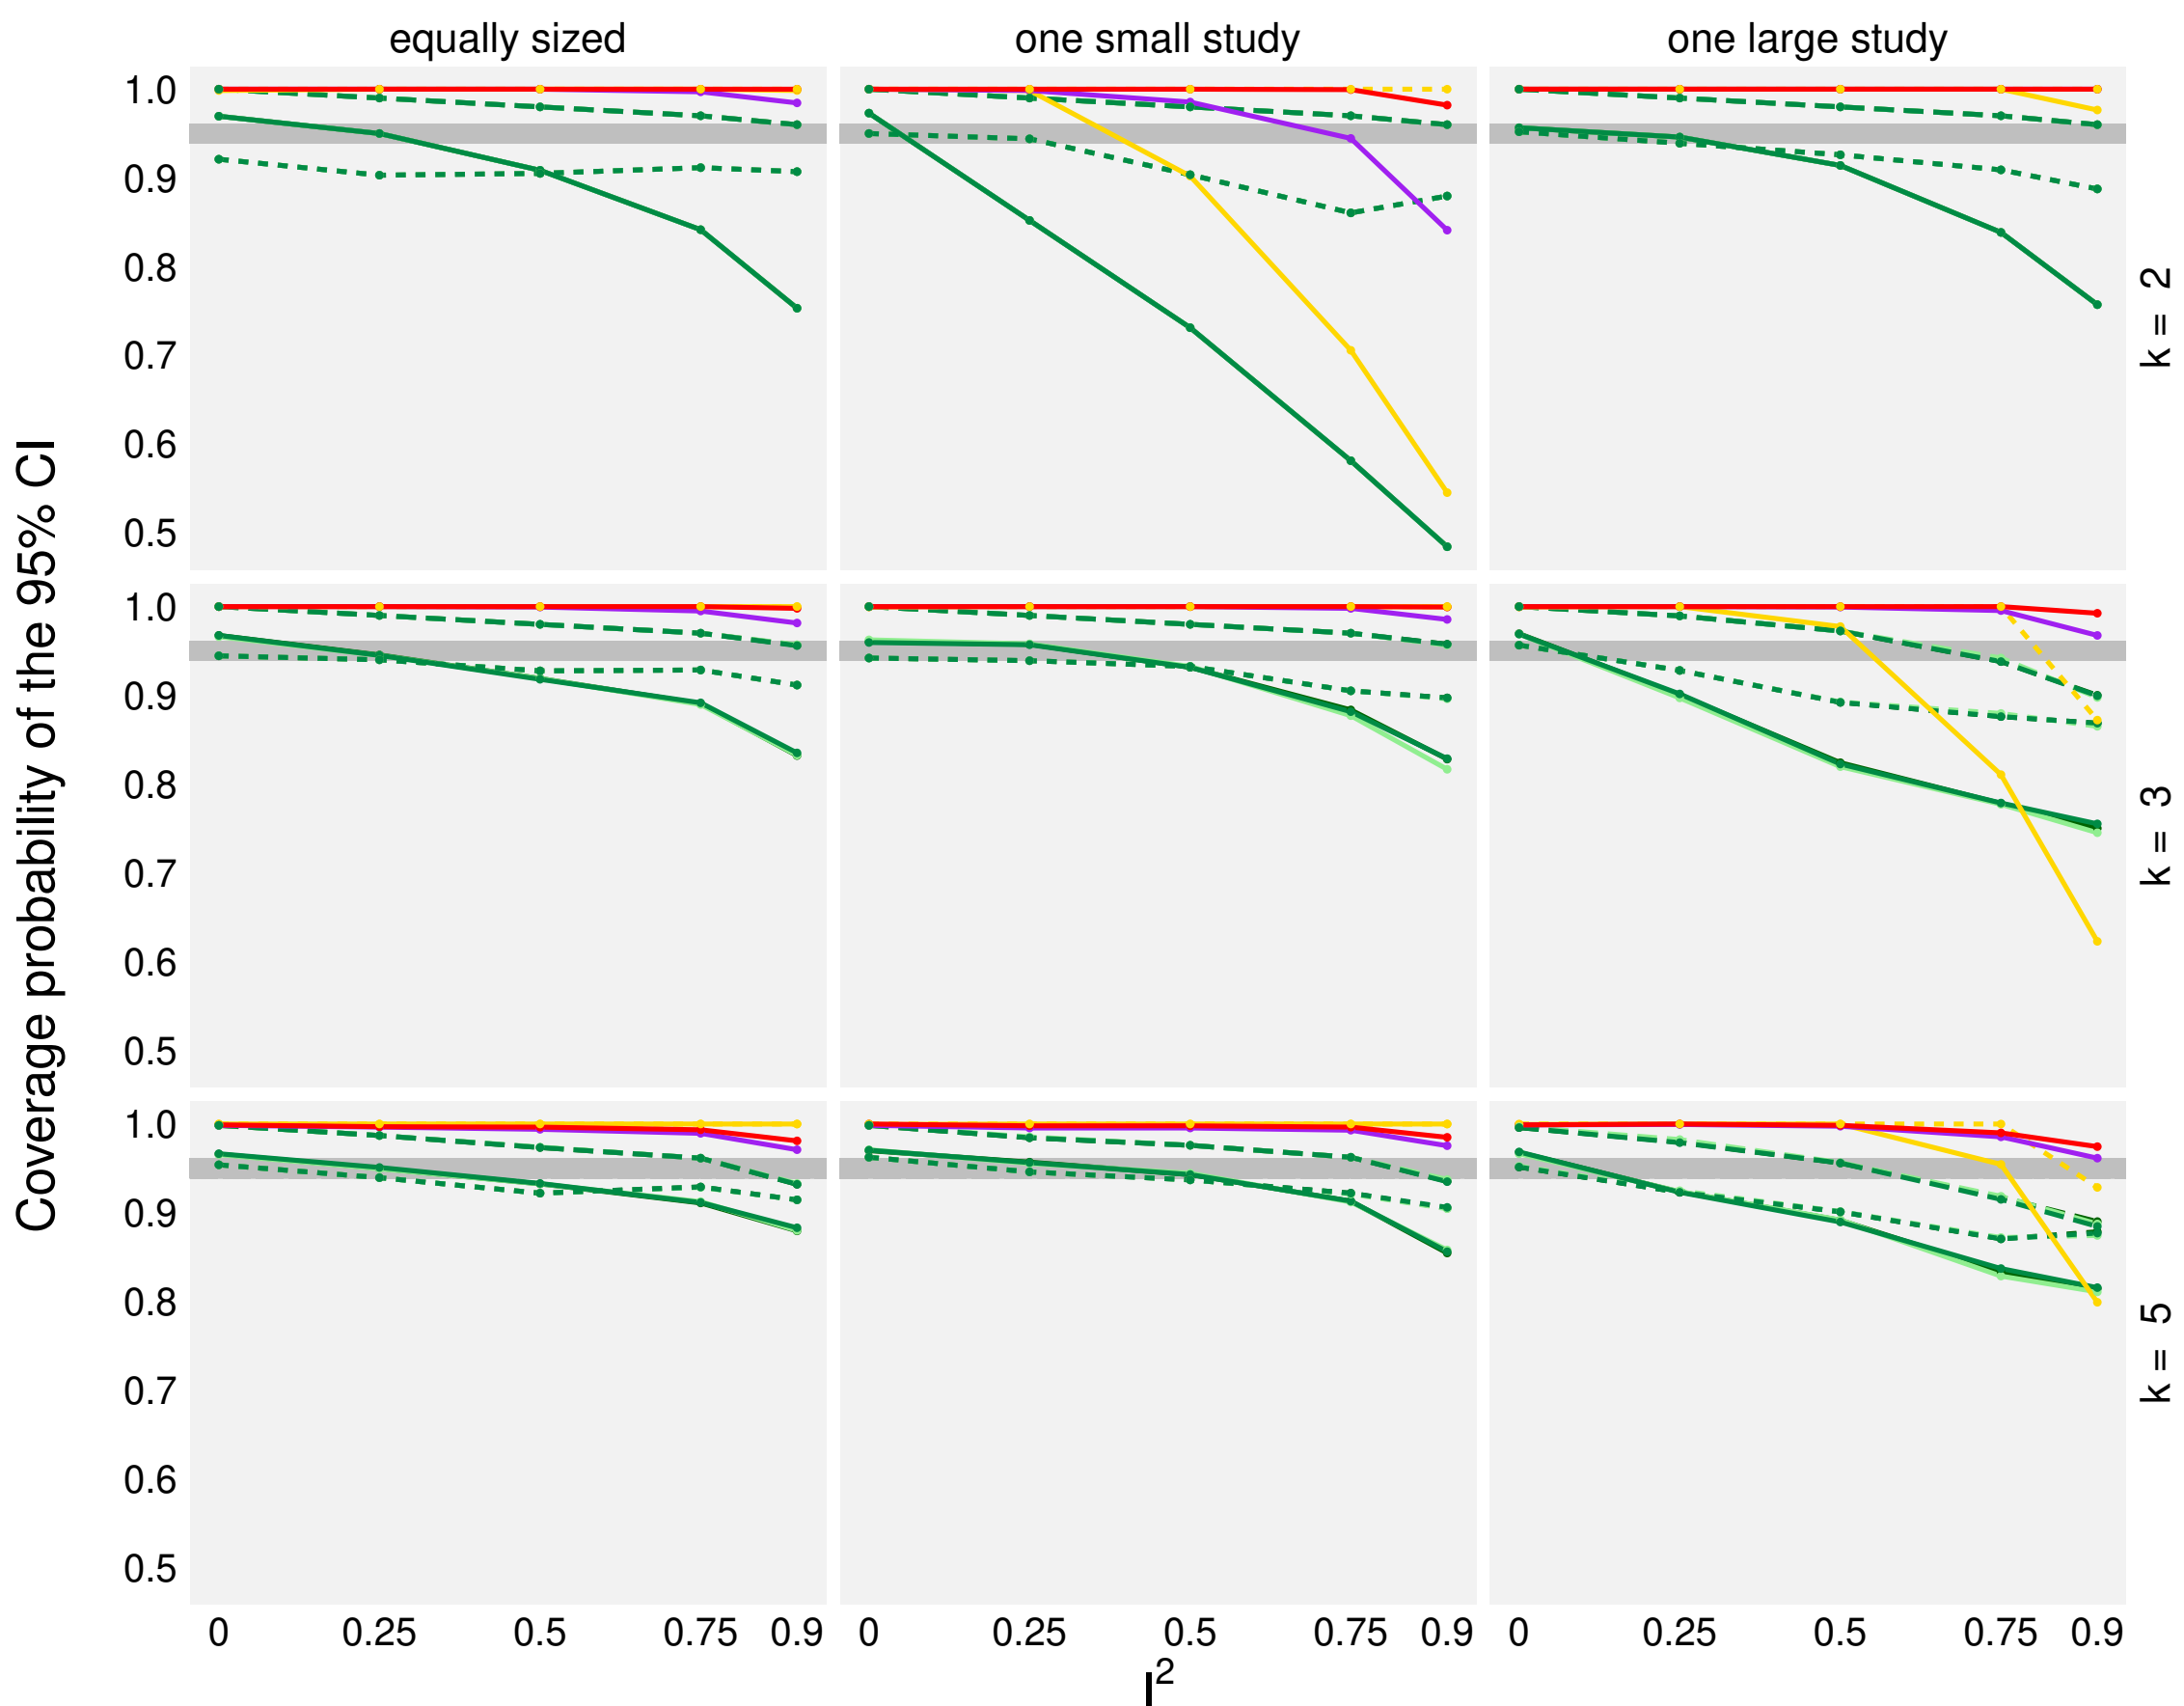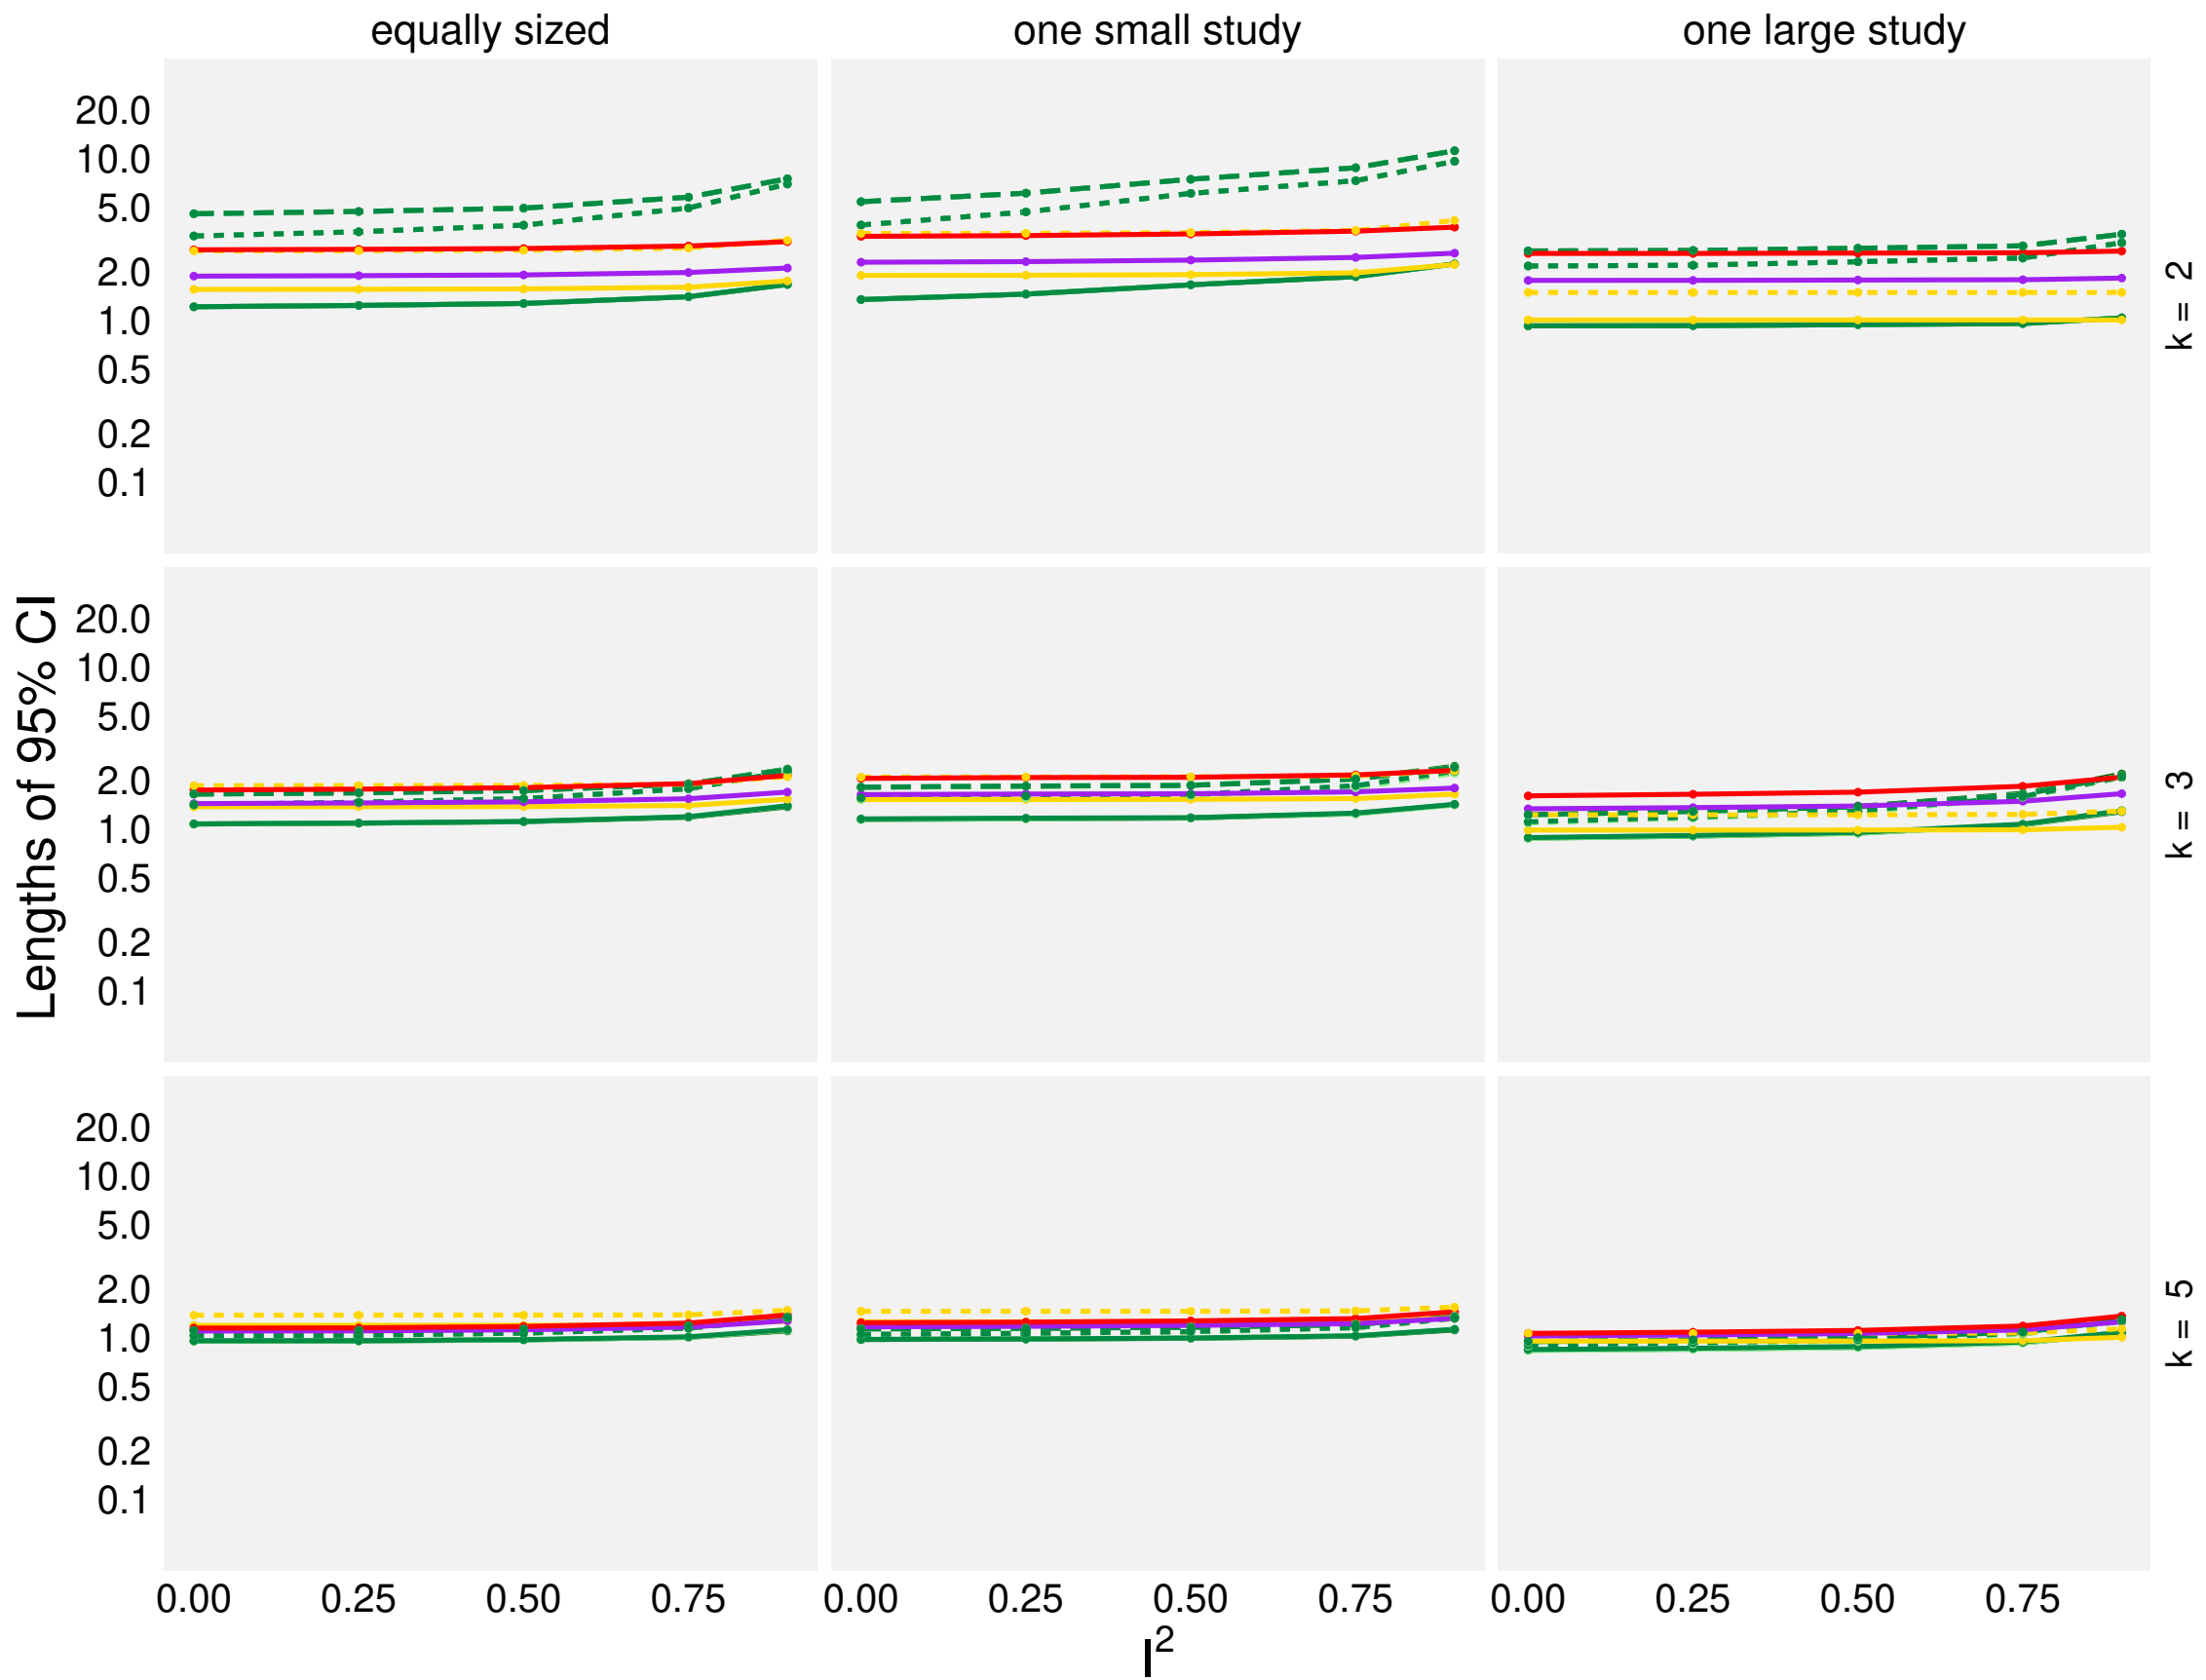

— NN – DL  
 — NN – REML  
 — NN – EB  
 — PN – PL  
 — NN – Bayes HN(0.5)  
 — NN – Bayes HN(1)  
 — normal quantiles  
 - - HKSJ or Student's t  
 - - mHKSJ

RR  
( $n_i=100, \pi_0=0.1$ )

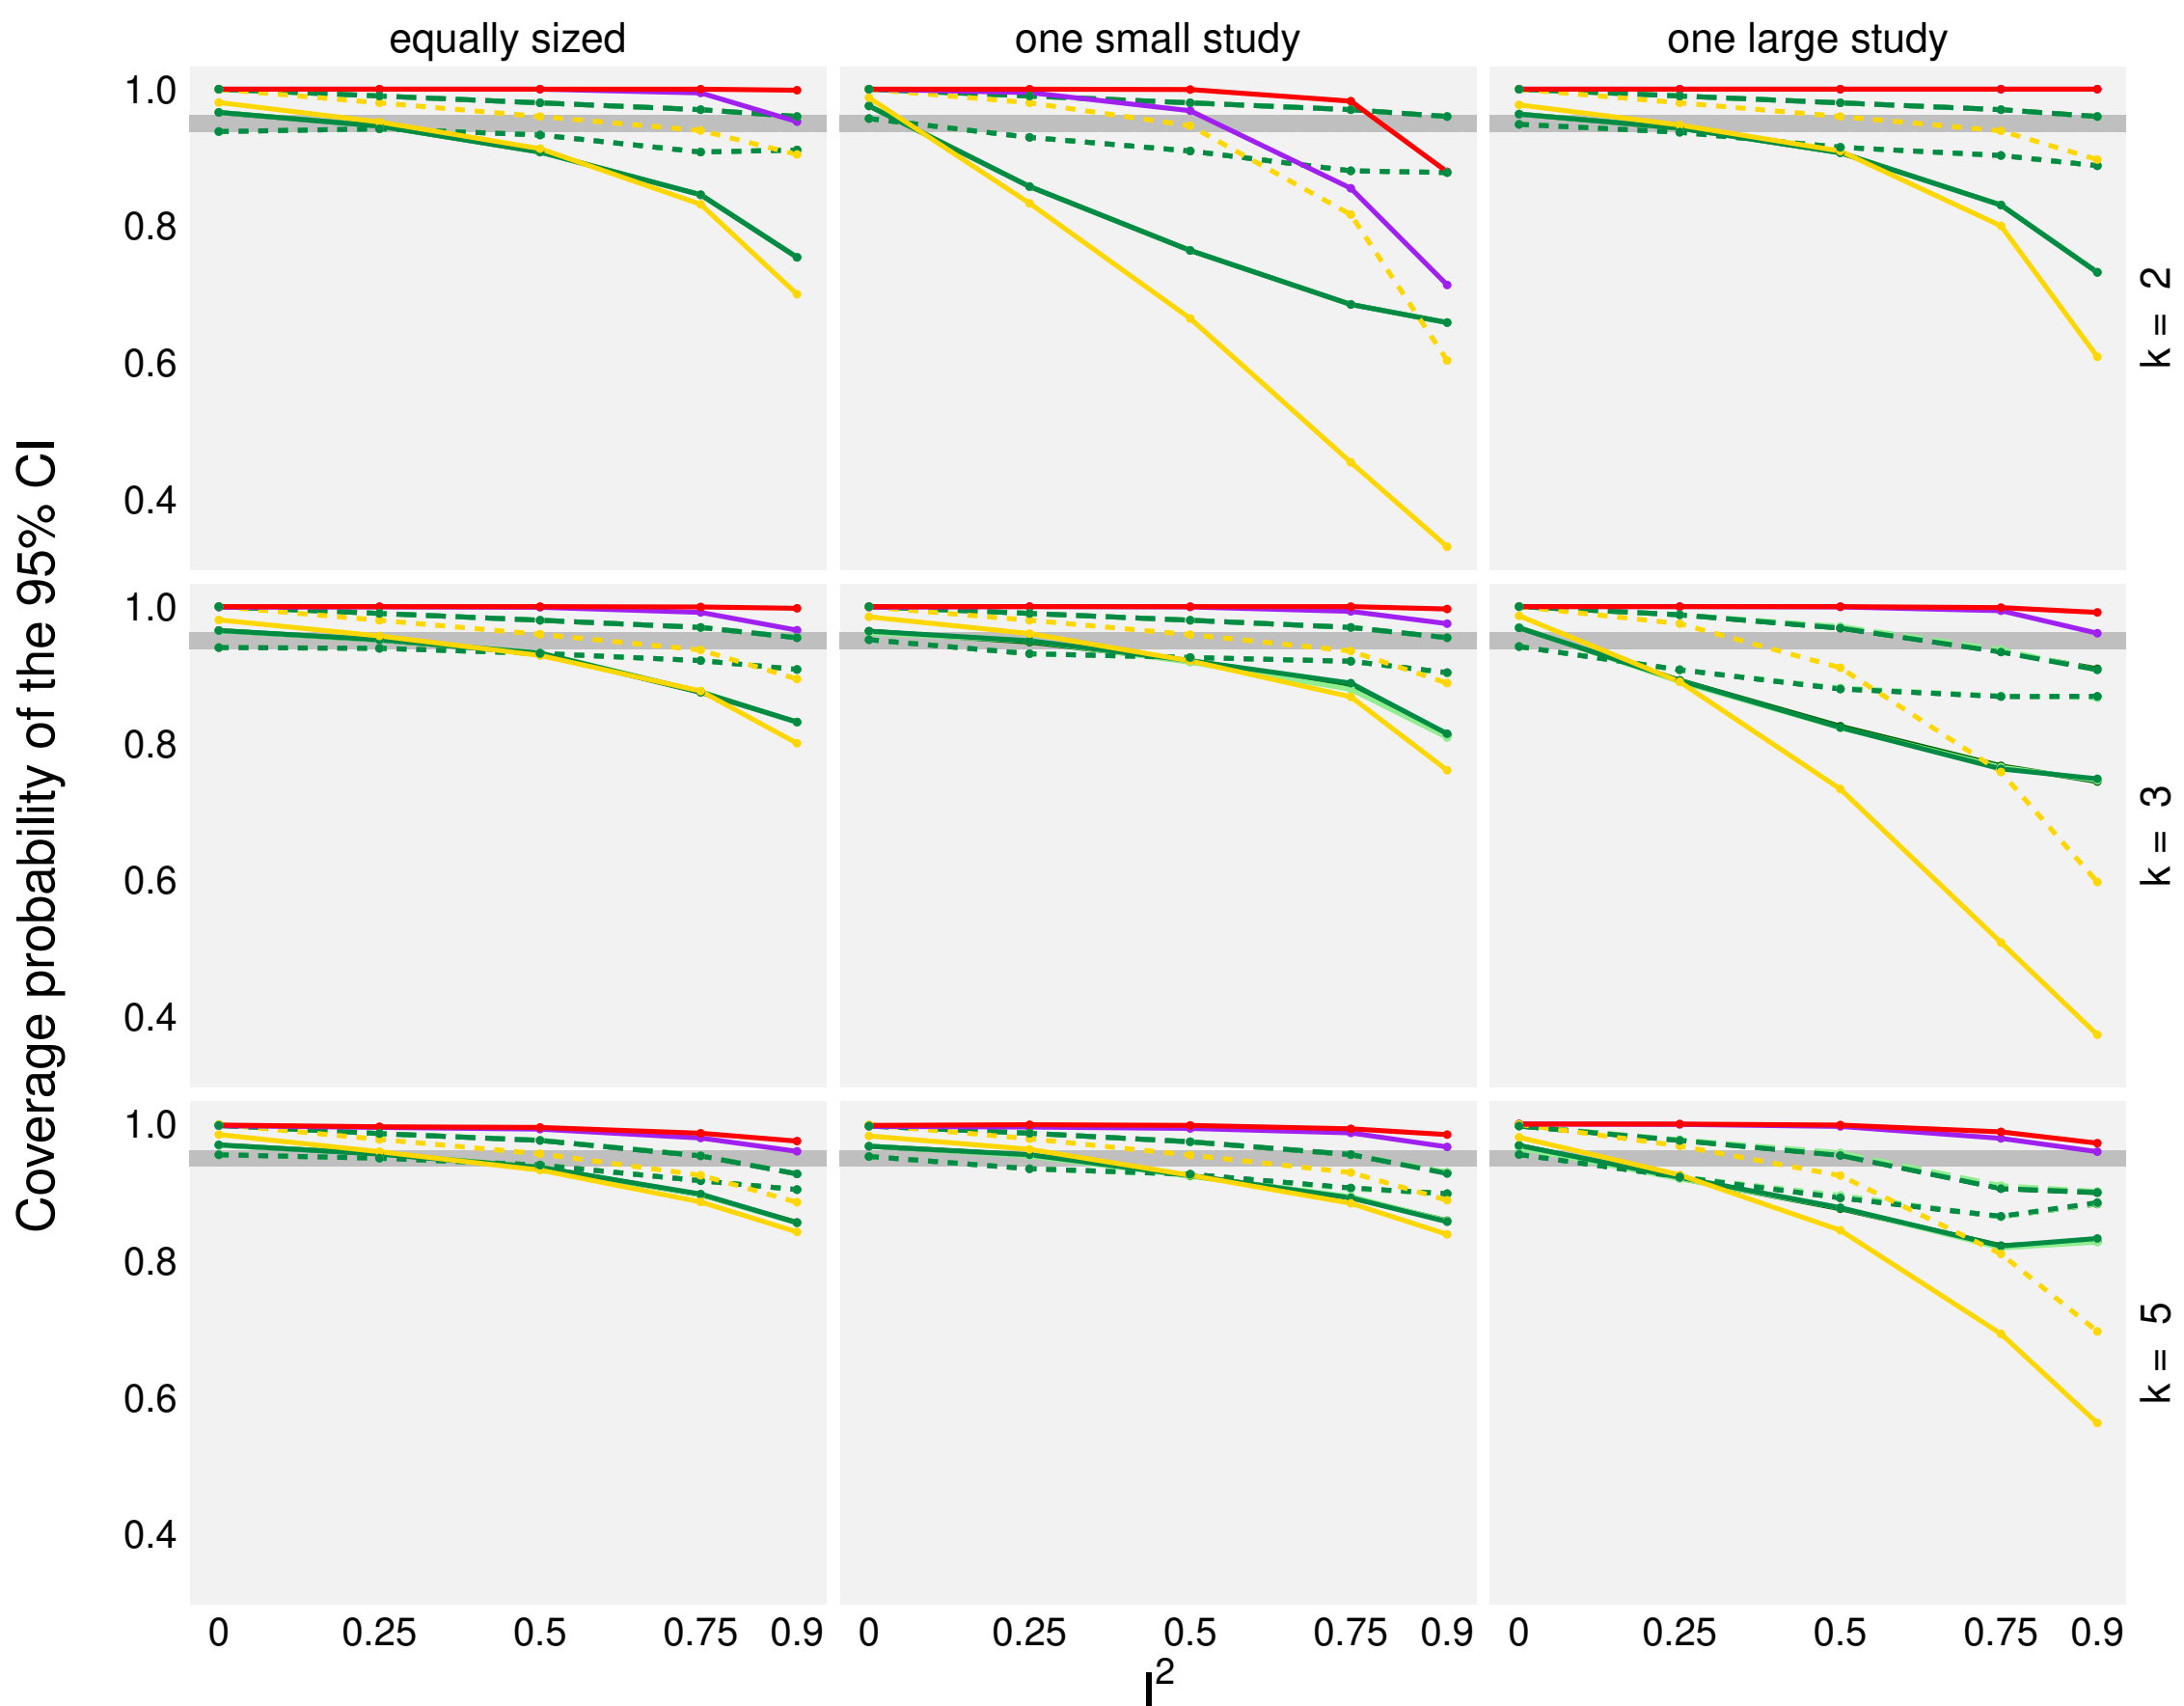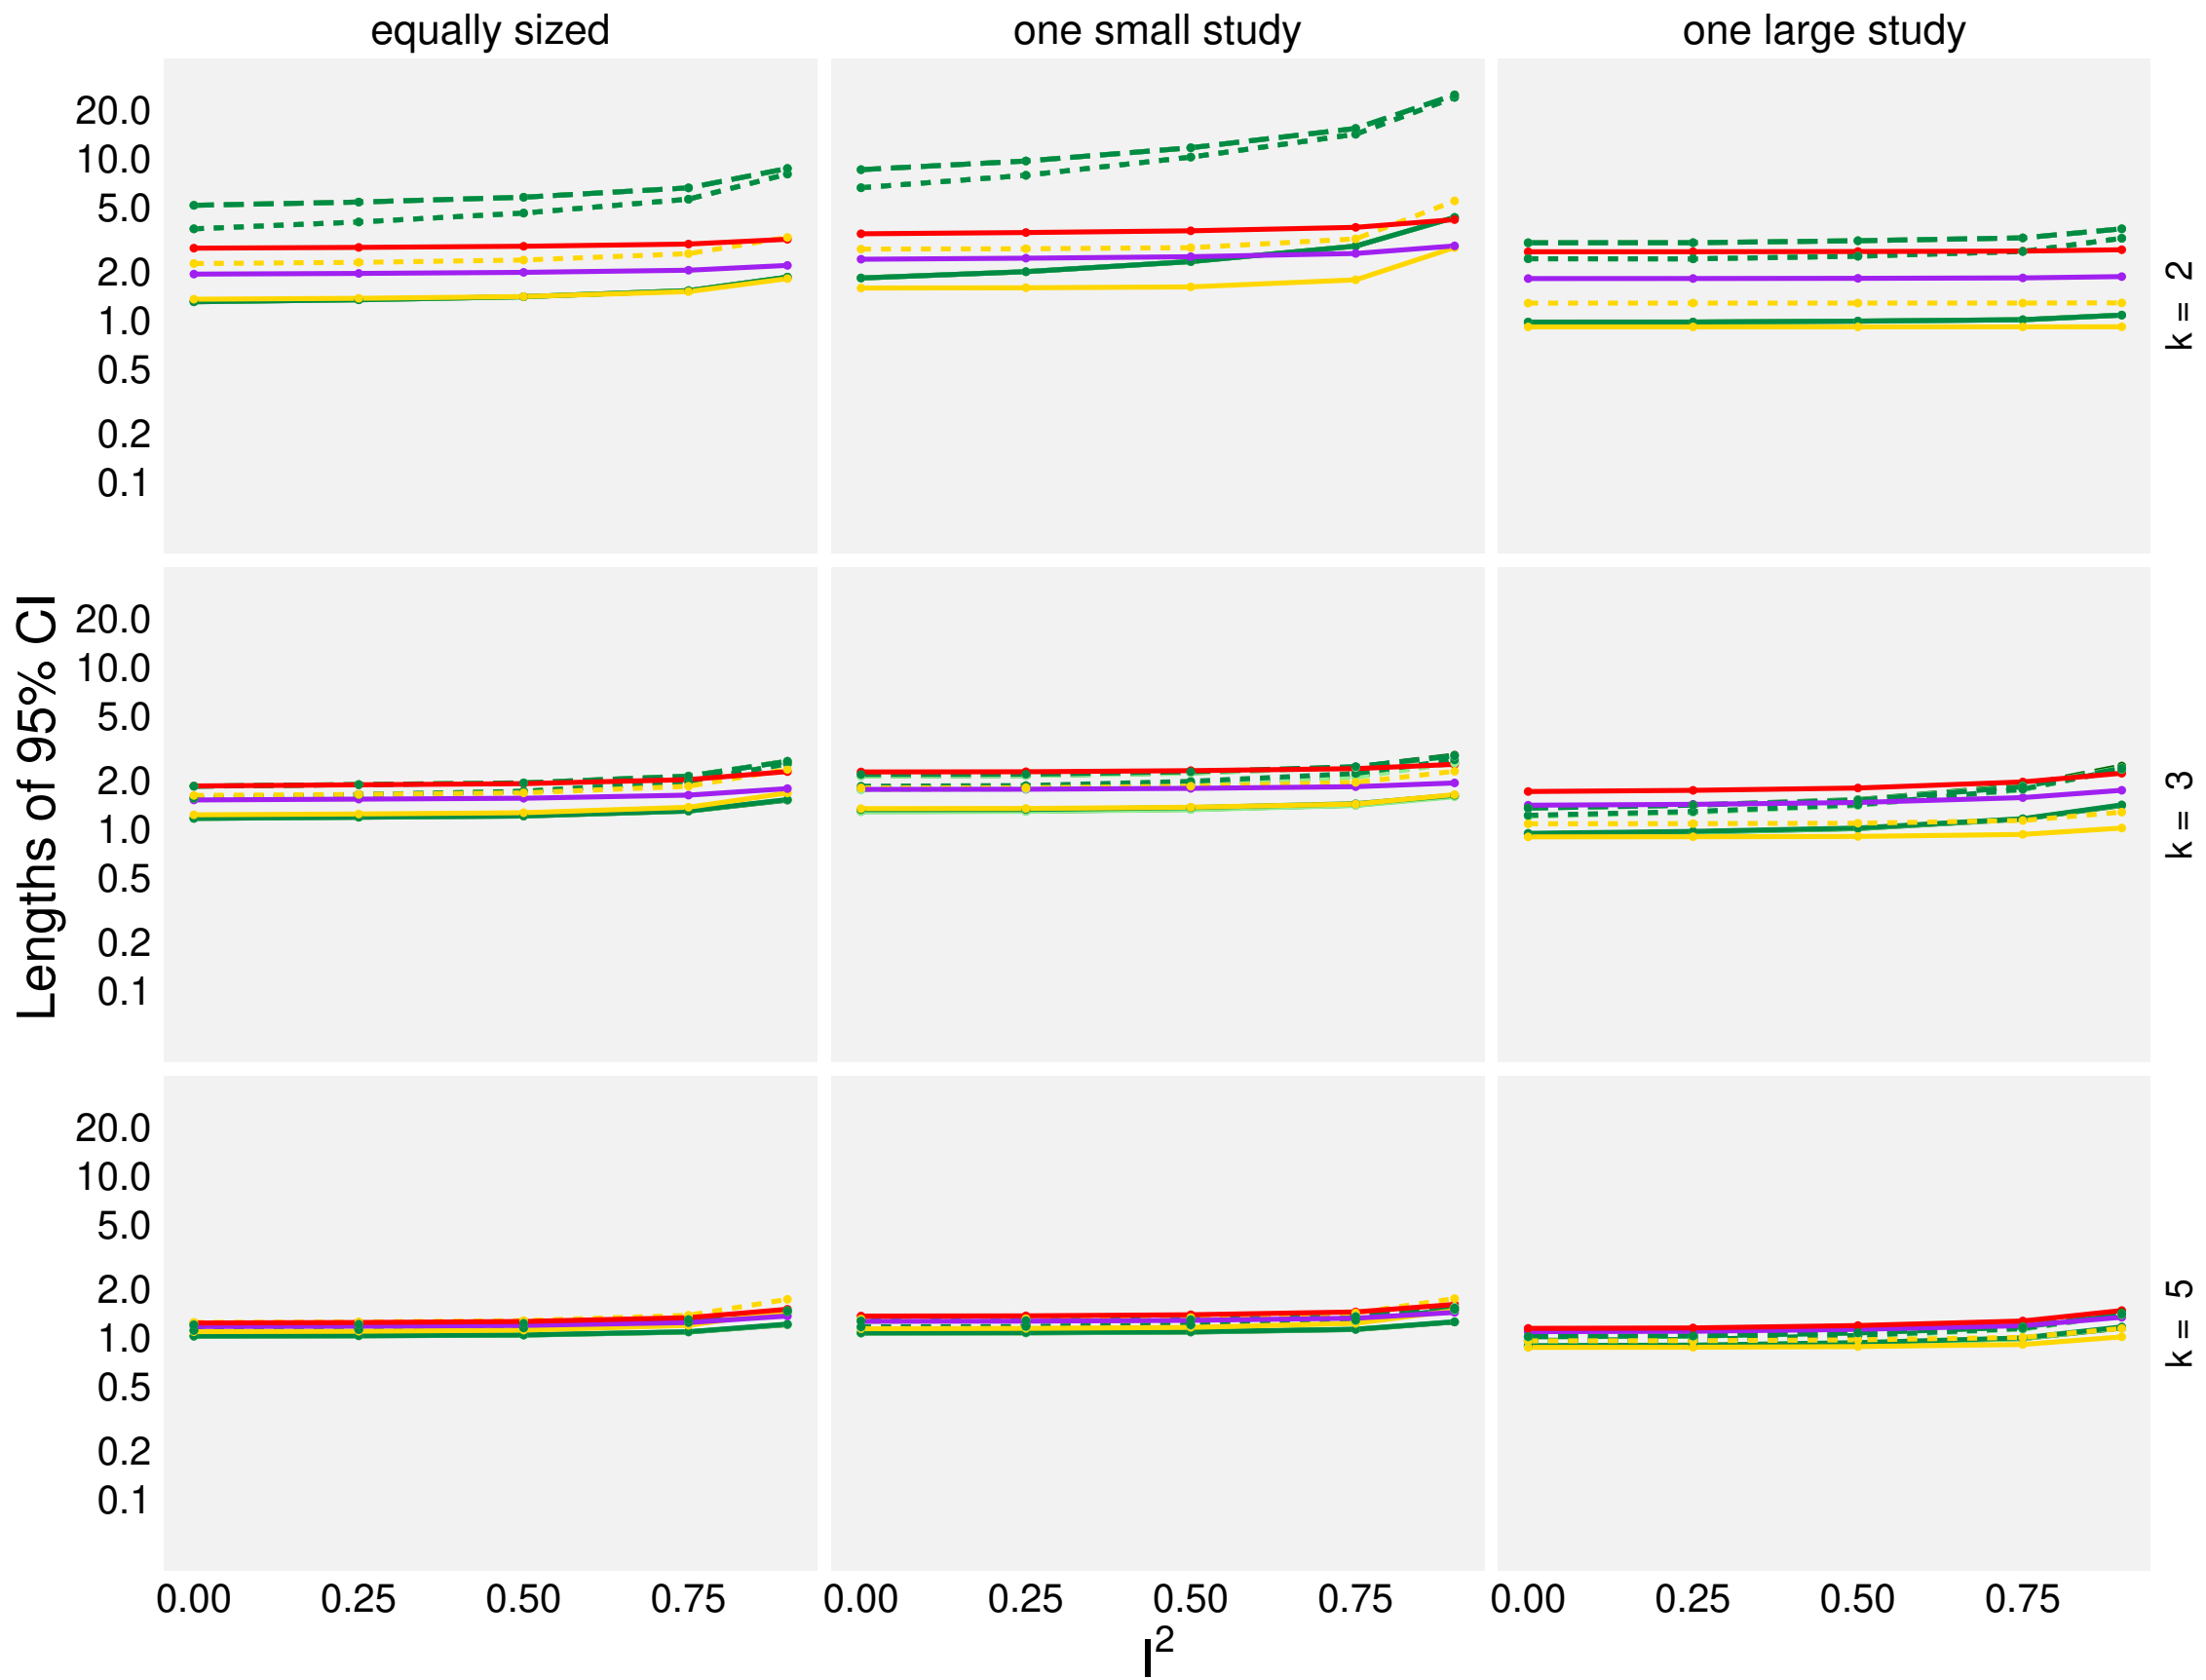

NN - DL      PN - PL      normal quantiles  
 NN - REML      NN - Bayes HN(0.5)      HKSJ or Student's t  
 NN - EB      NN - Bayes HN(1)      mHKSJ

RR  
( $n_i=100, \pi_0=0.3$ )

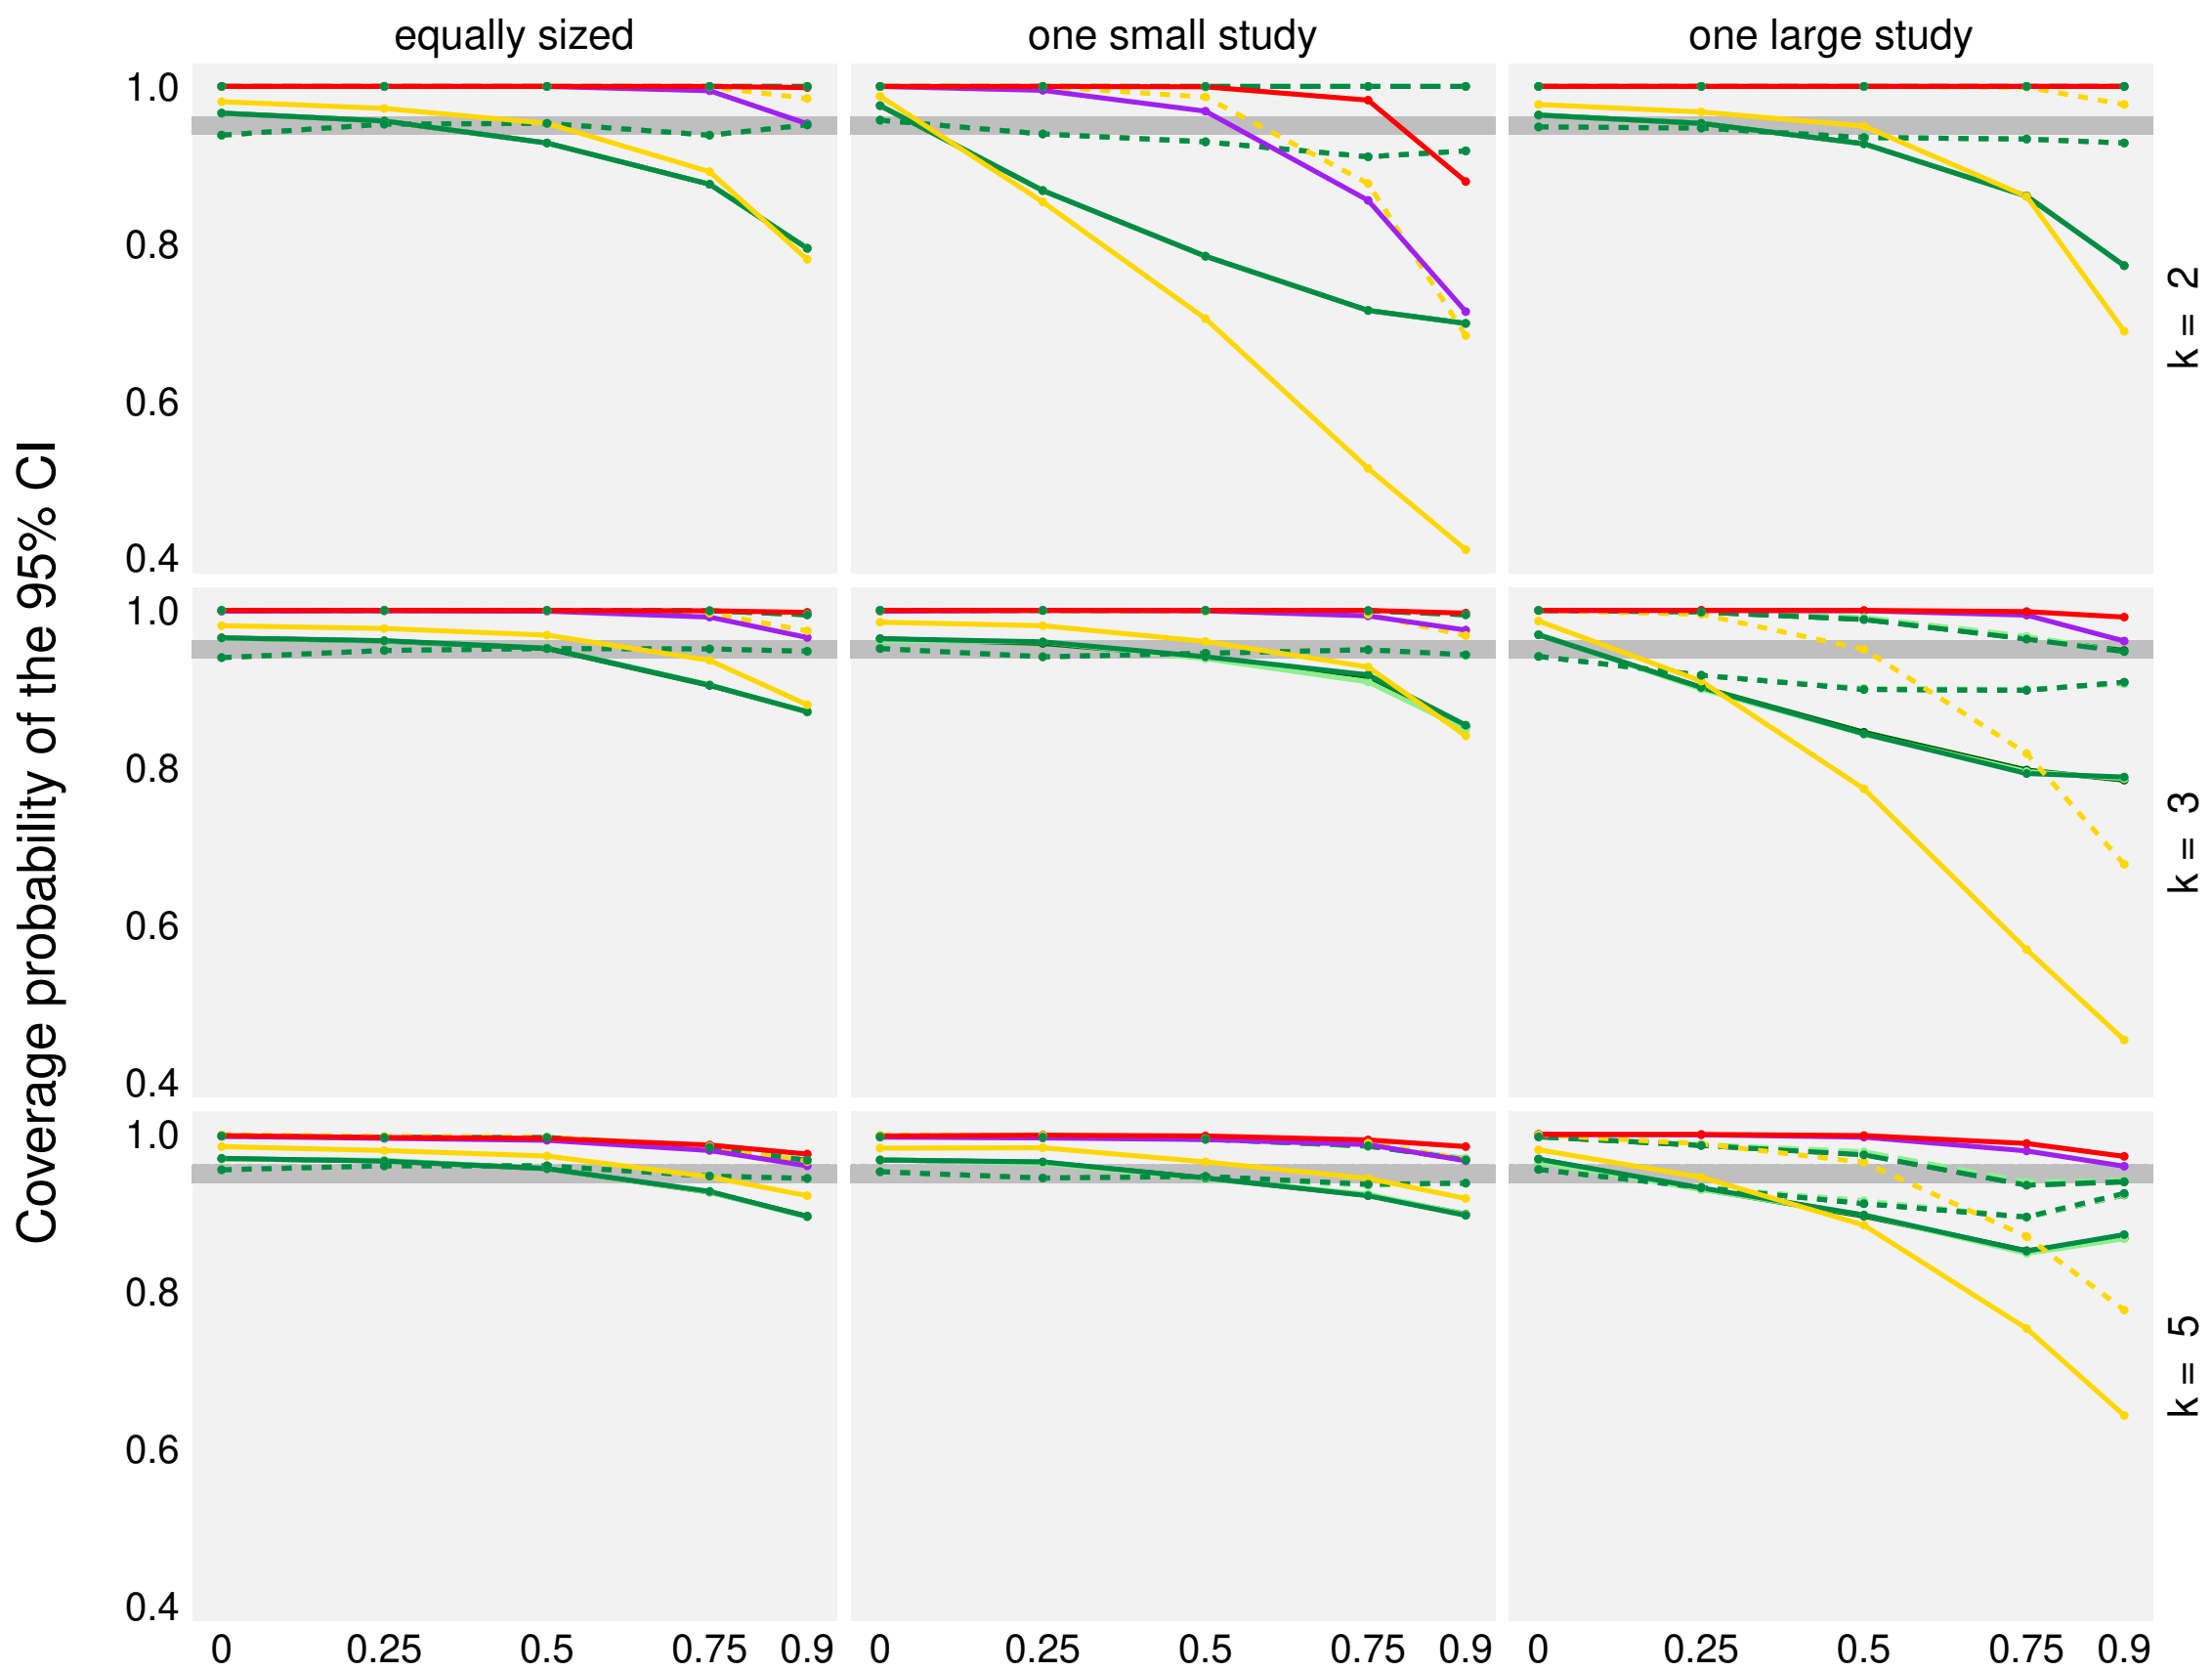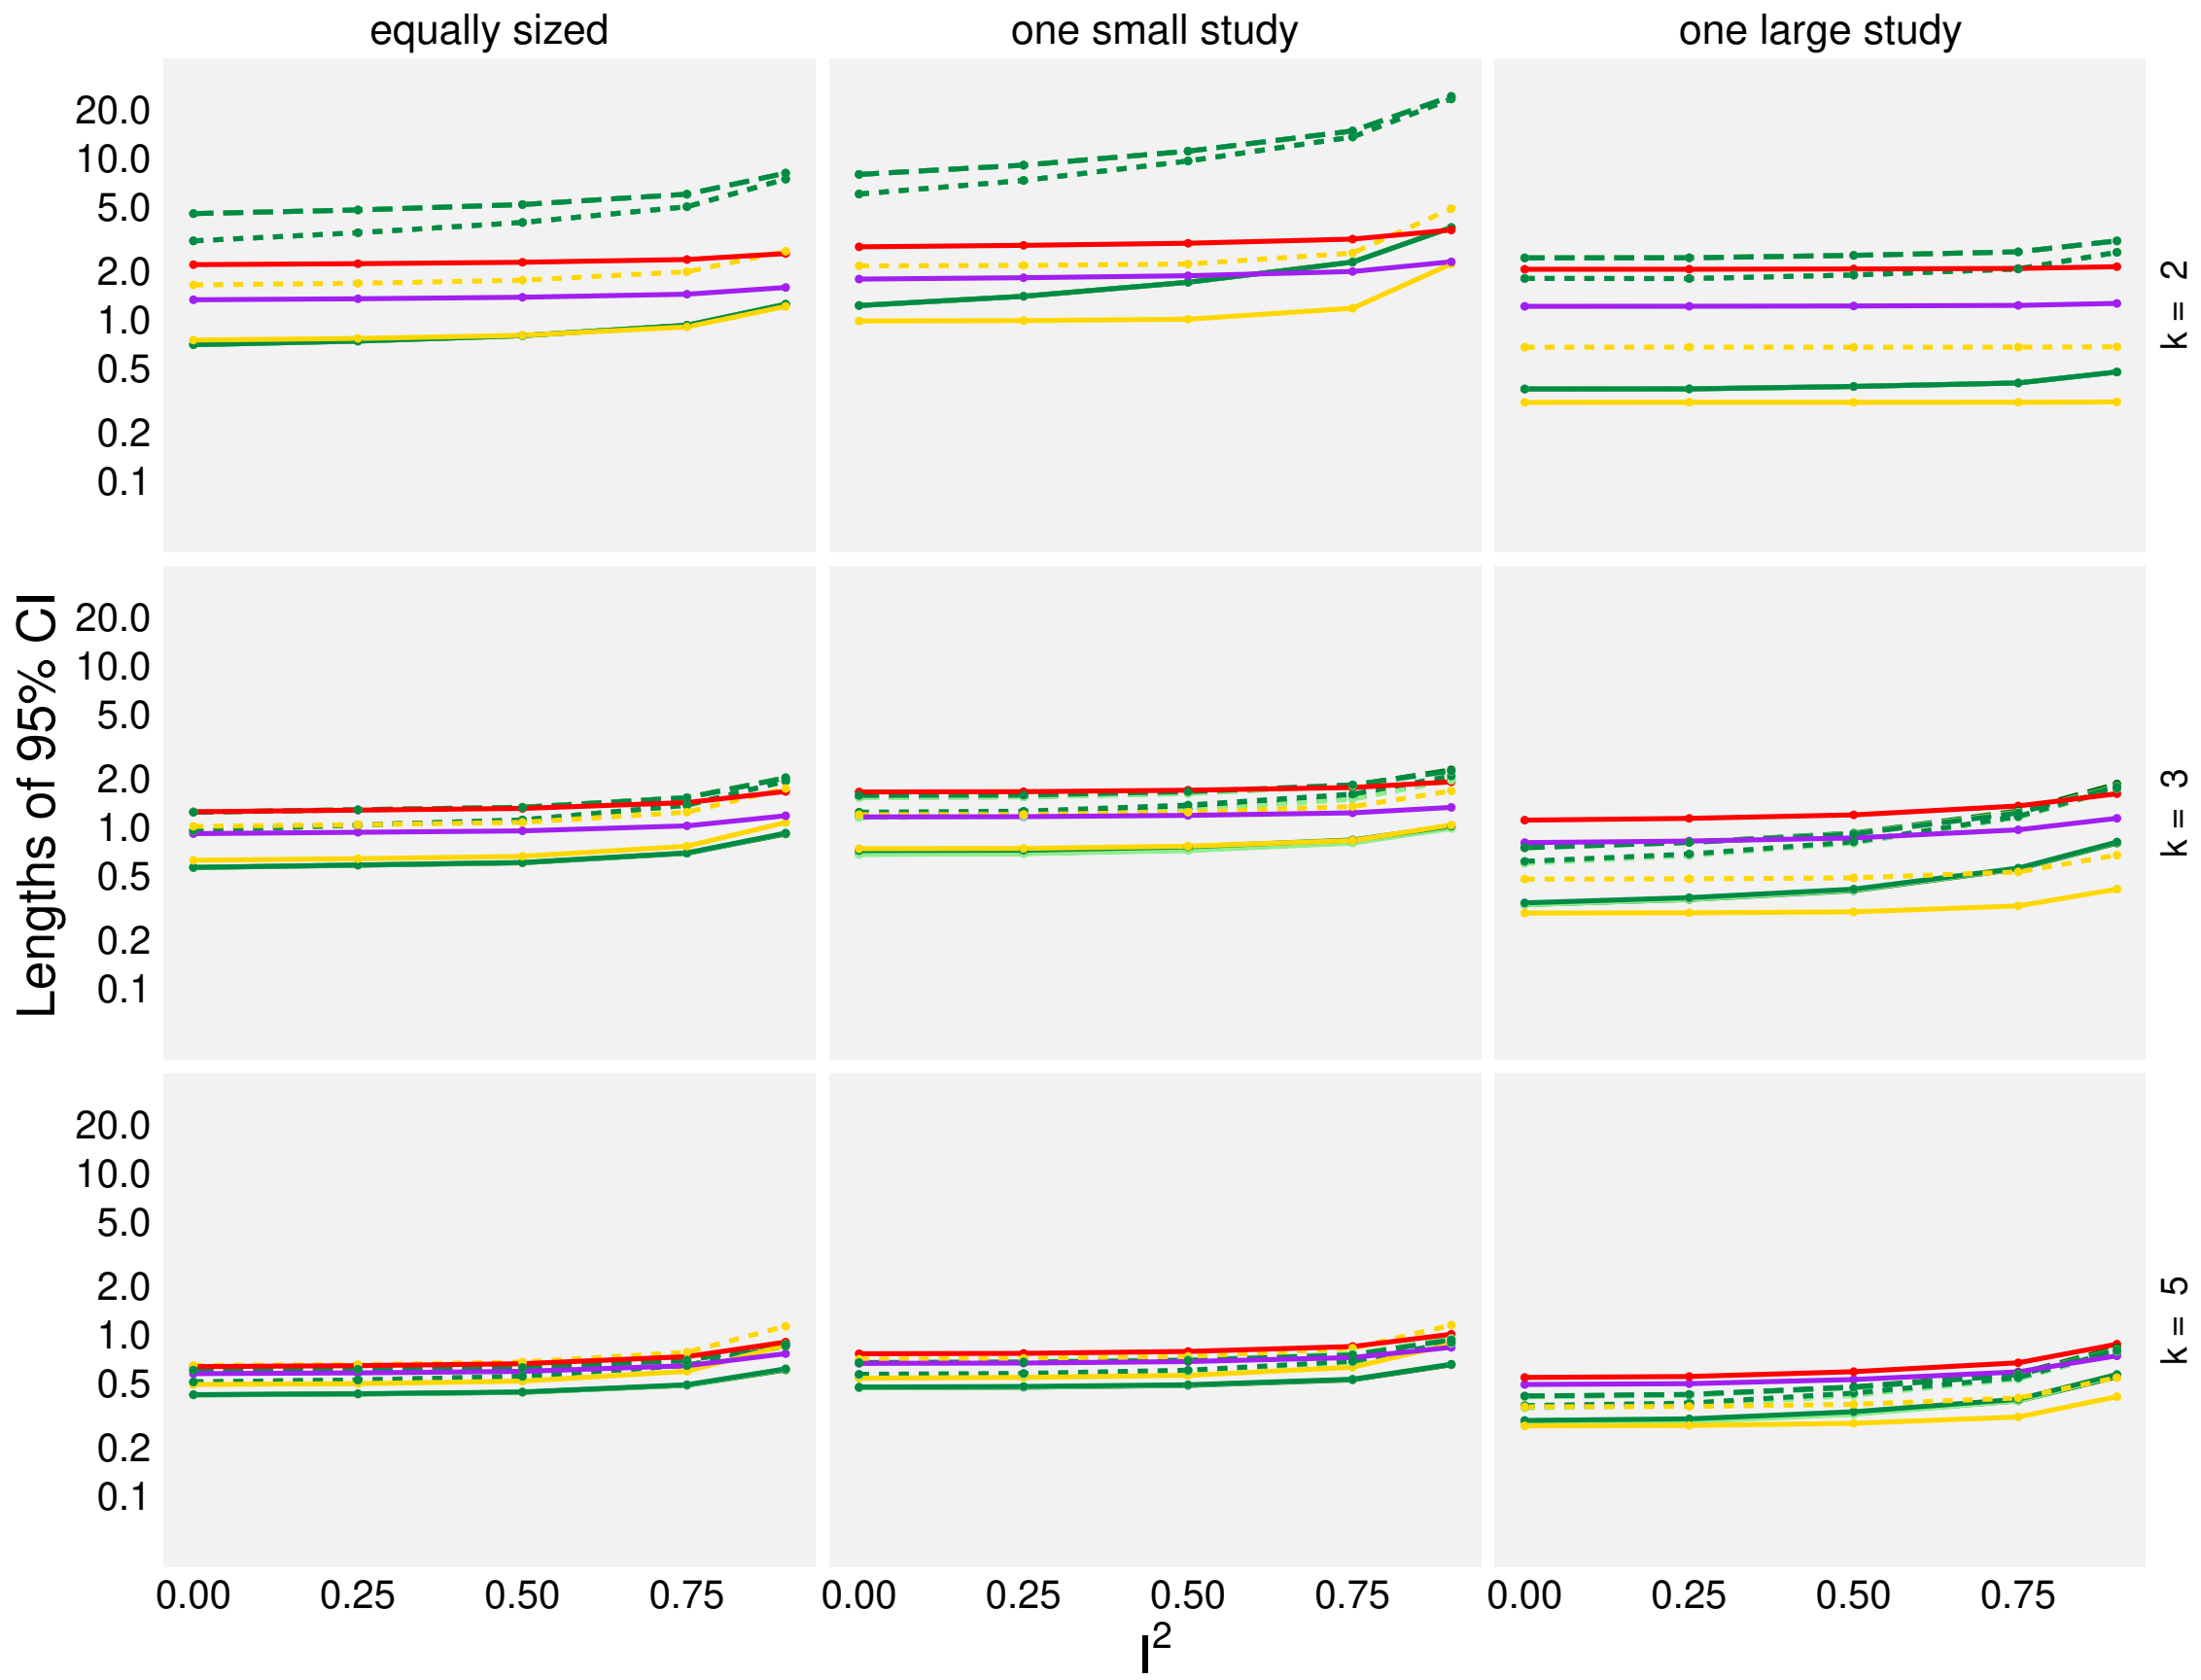

— NN – DL      — PN – PL      — normal quantiles  
 — NN – REML      — NN – Bayes HN(0.5)      - - HKSJ or Student's t  
 — NN – EB      — NN – Bayes HN(1)      - - mHKSJ

RR  
( $n_i=100, \pi_0=0.5$ )

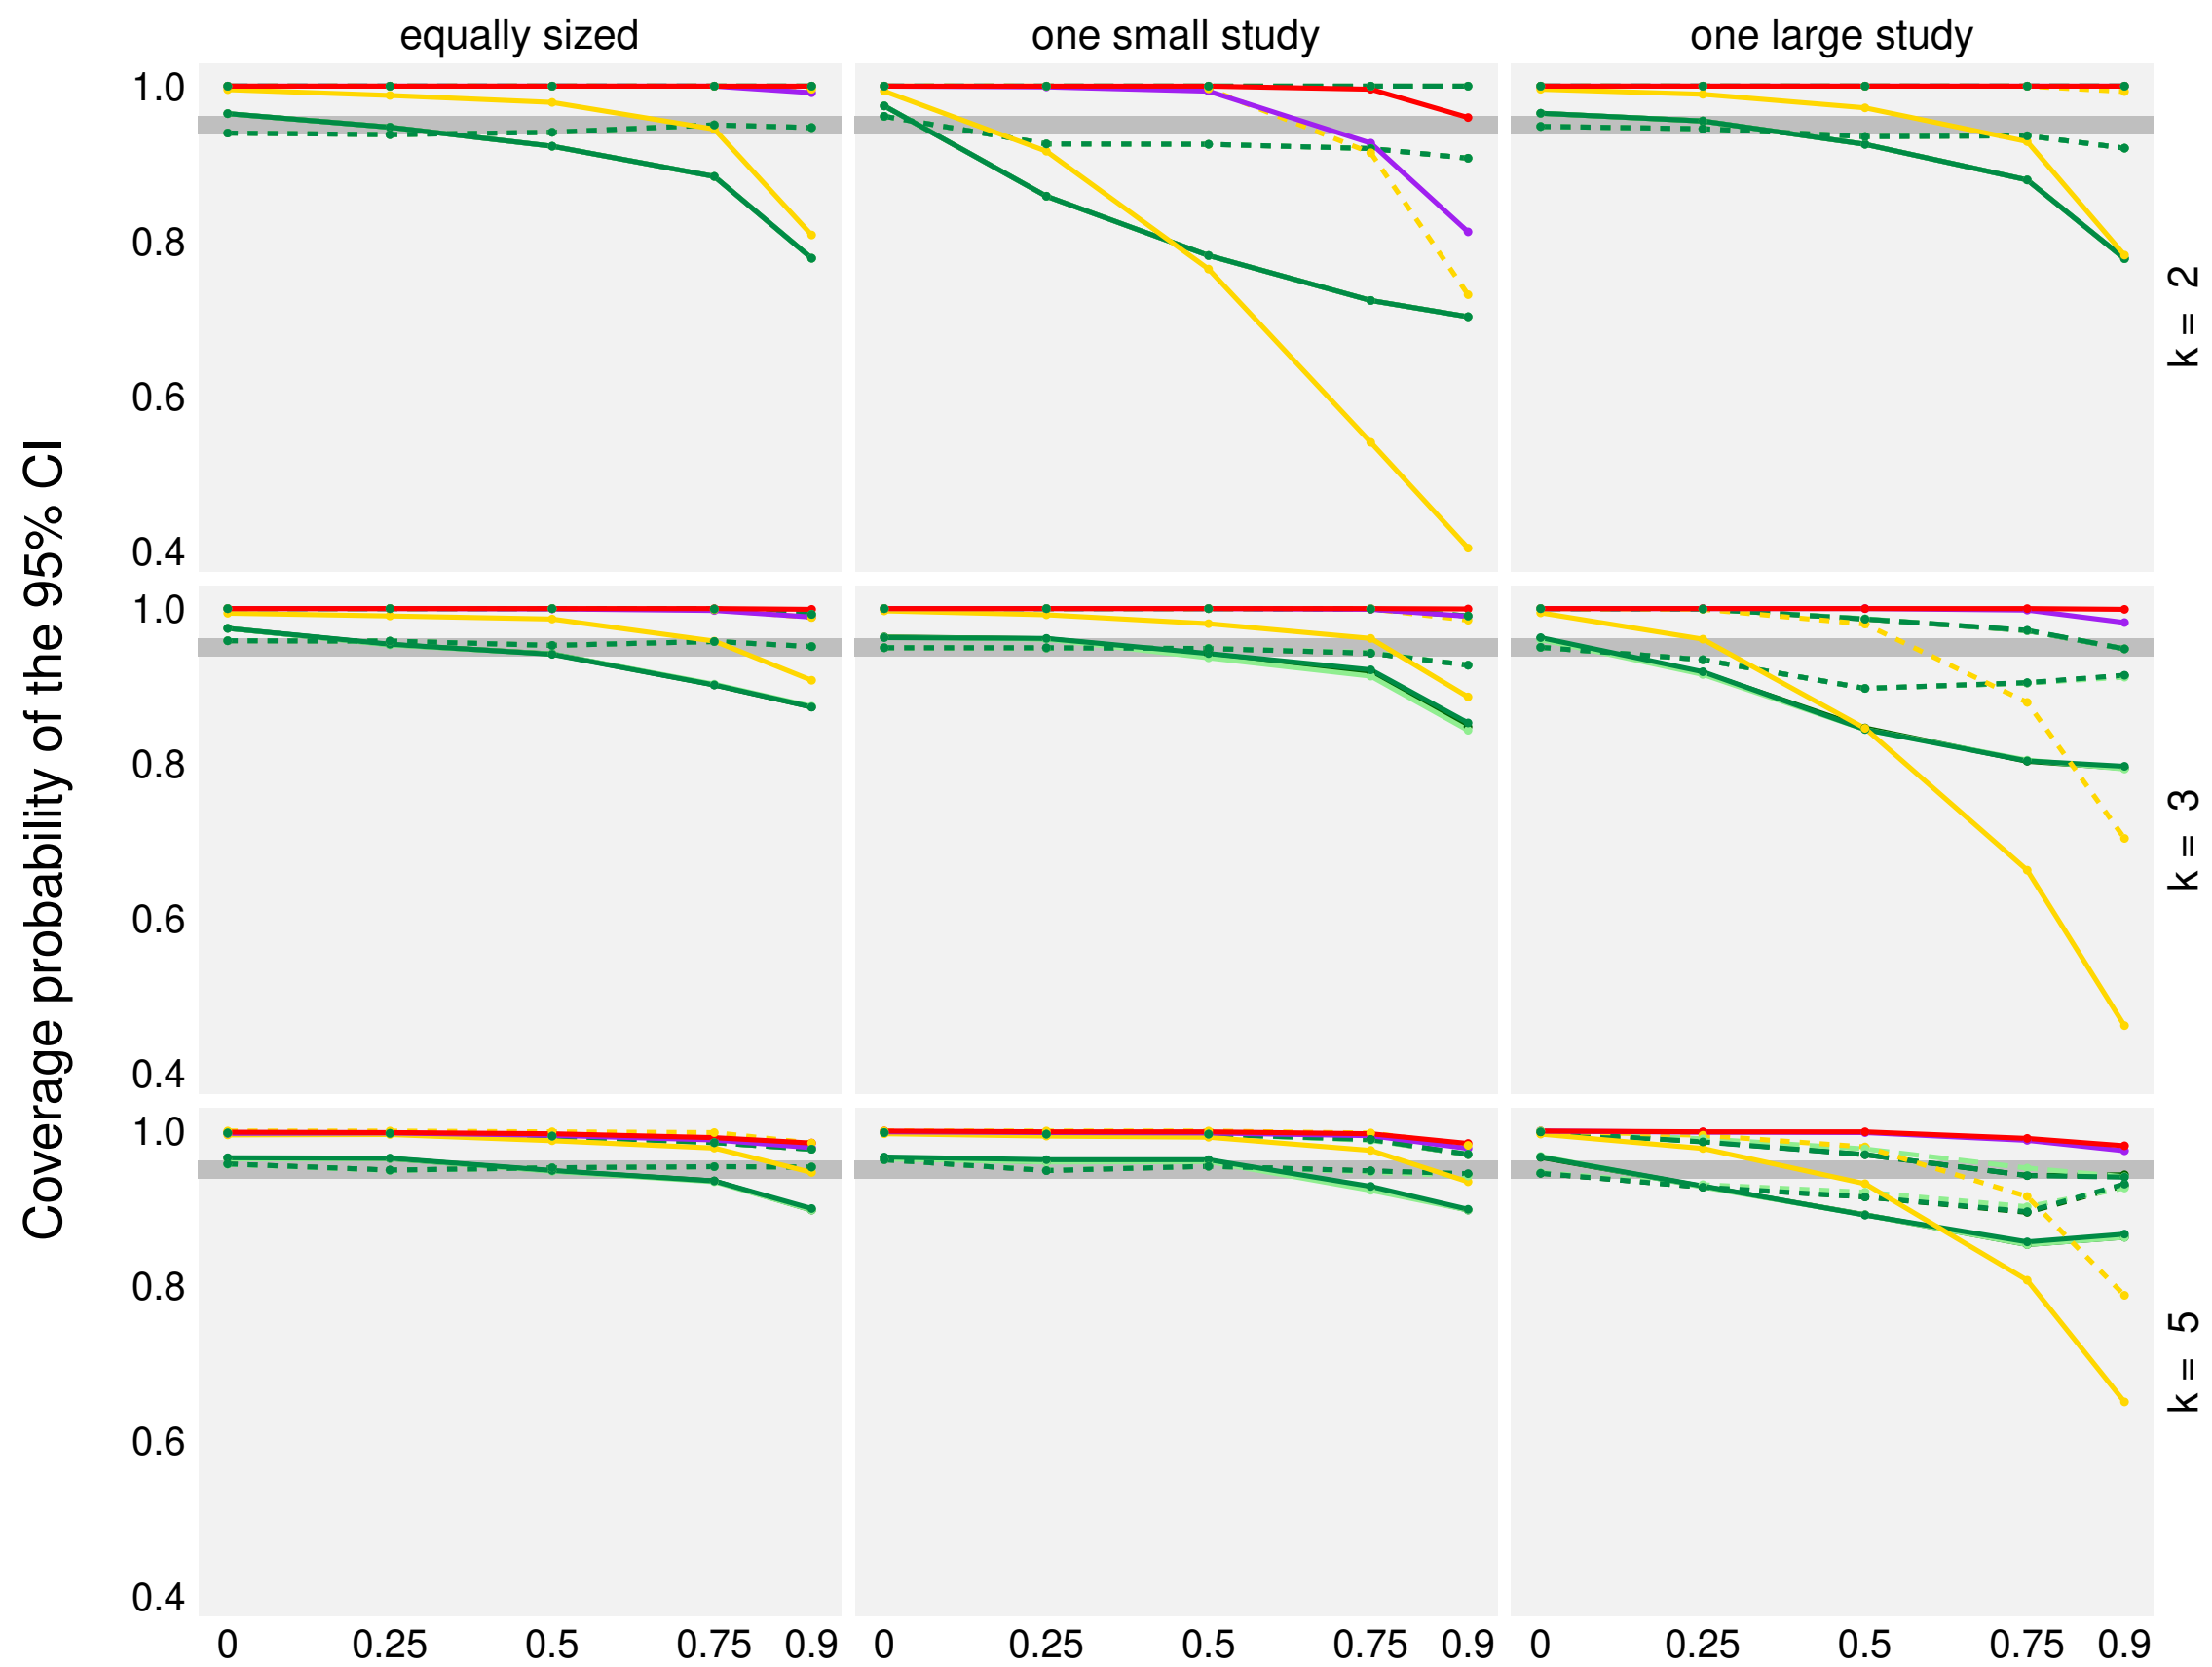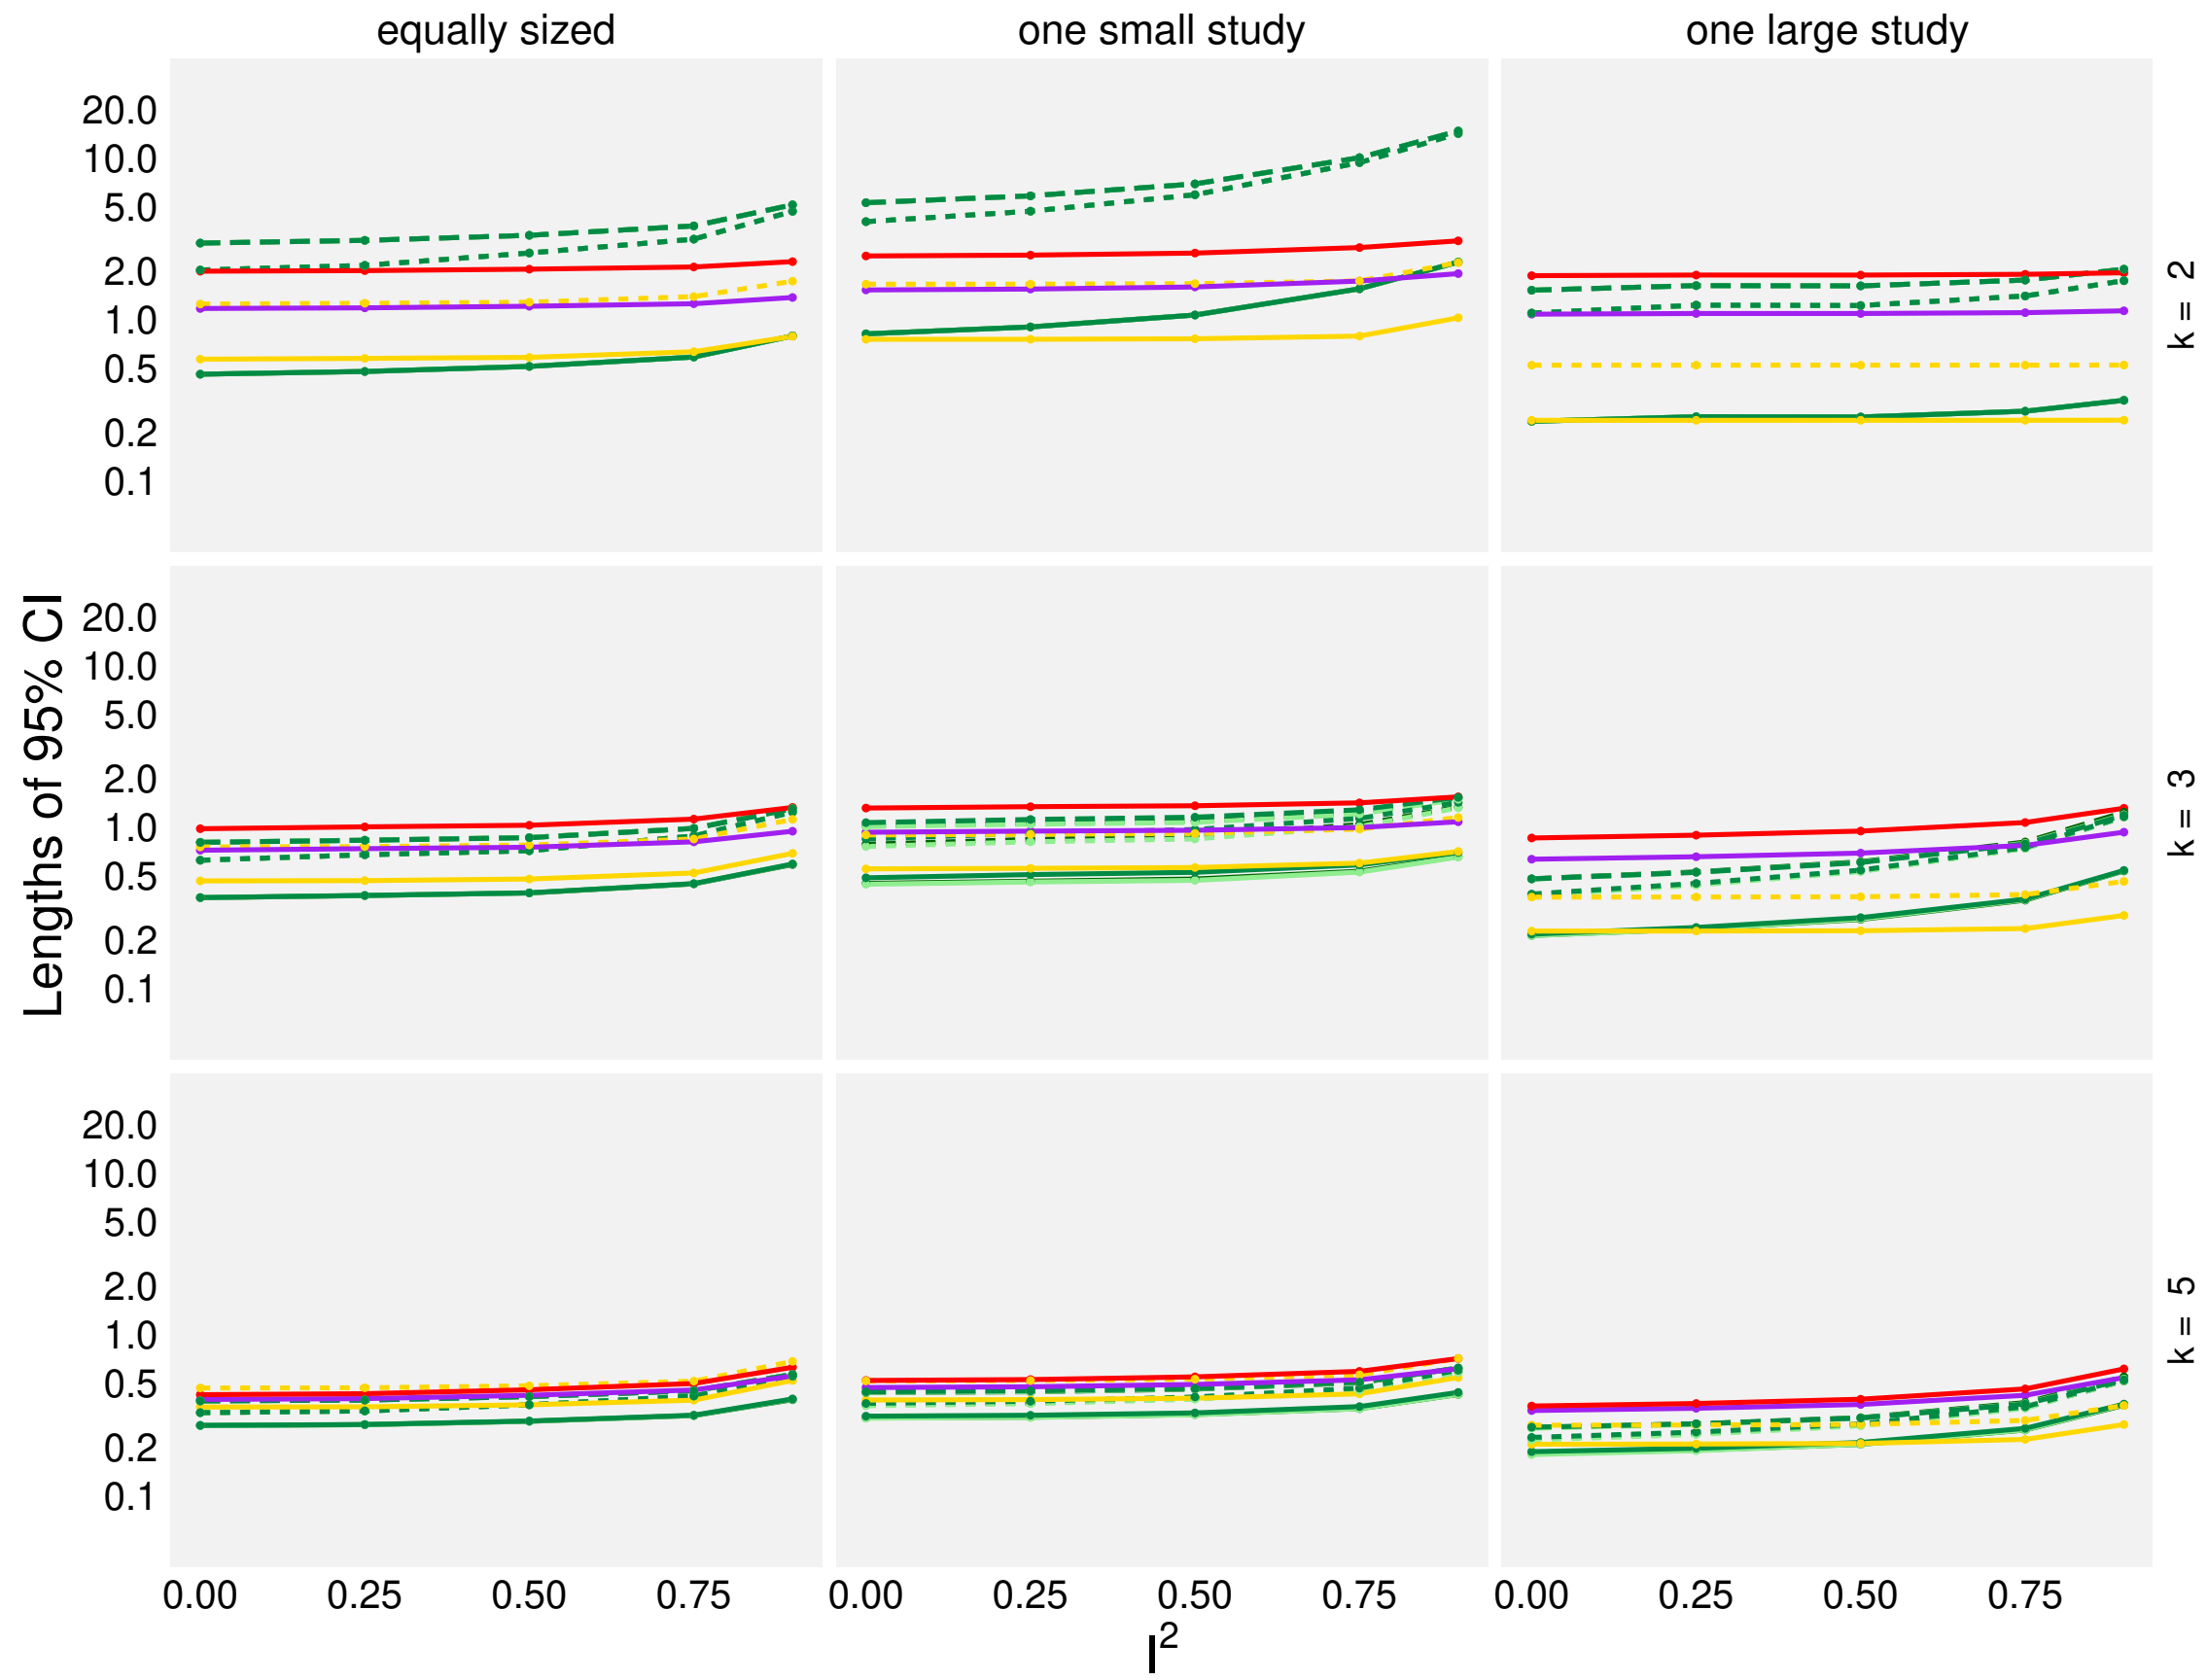

— NN – DL      — PN – PL      — normal quantiles  
 — NN – REML      — NN – Bayes HN(0.5)      - - HKSJ or Student's t  
 — NN – EB      — NN – Bayes HN(1)      - - mHKSJ

RR  
( $n_i=100, \pi_0=0.7$ )

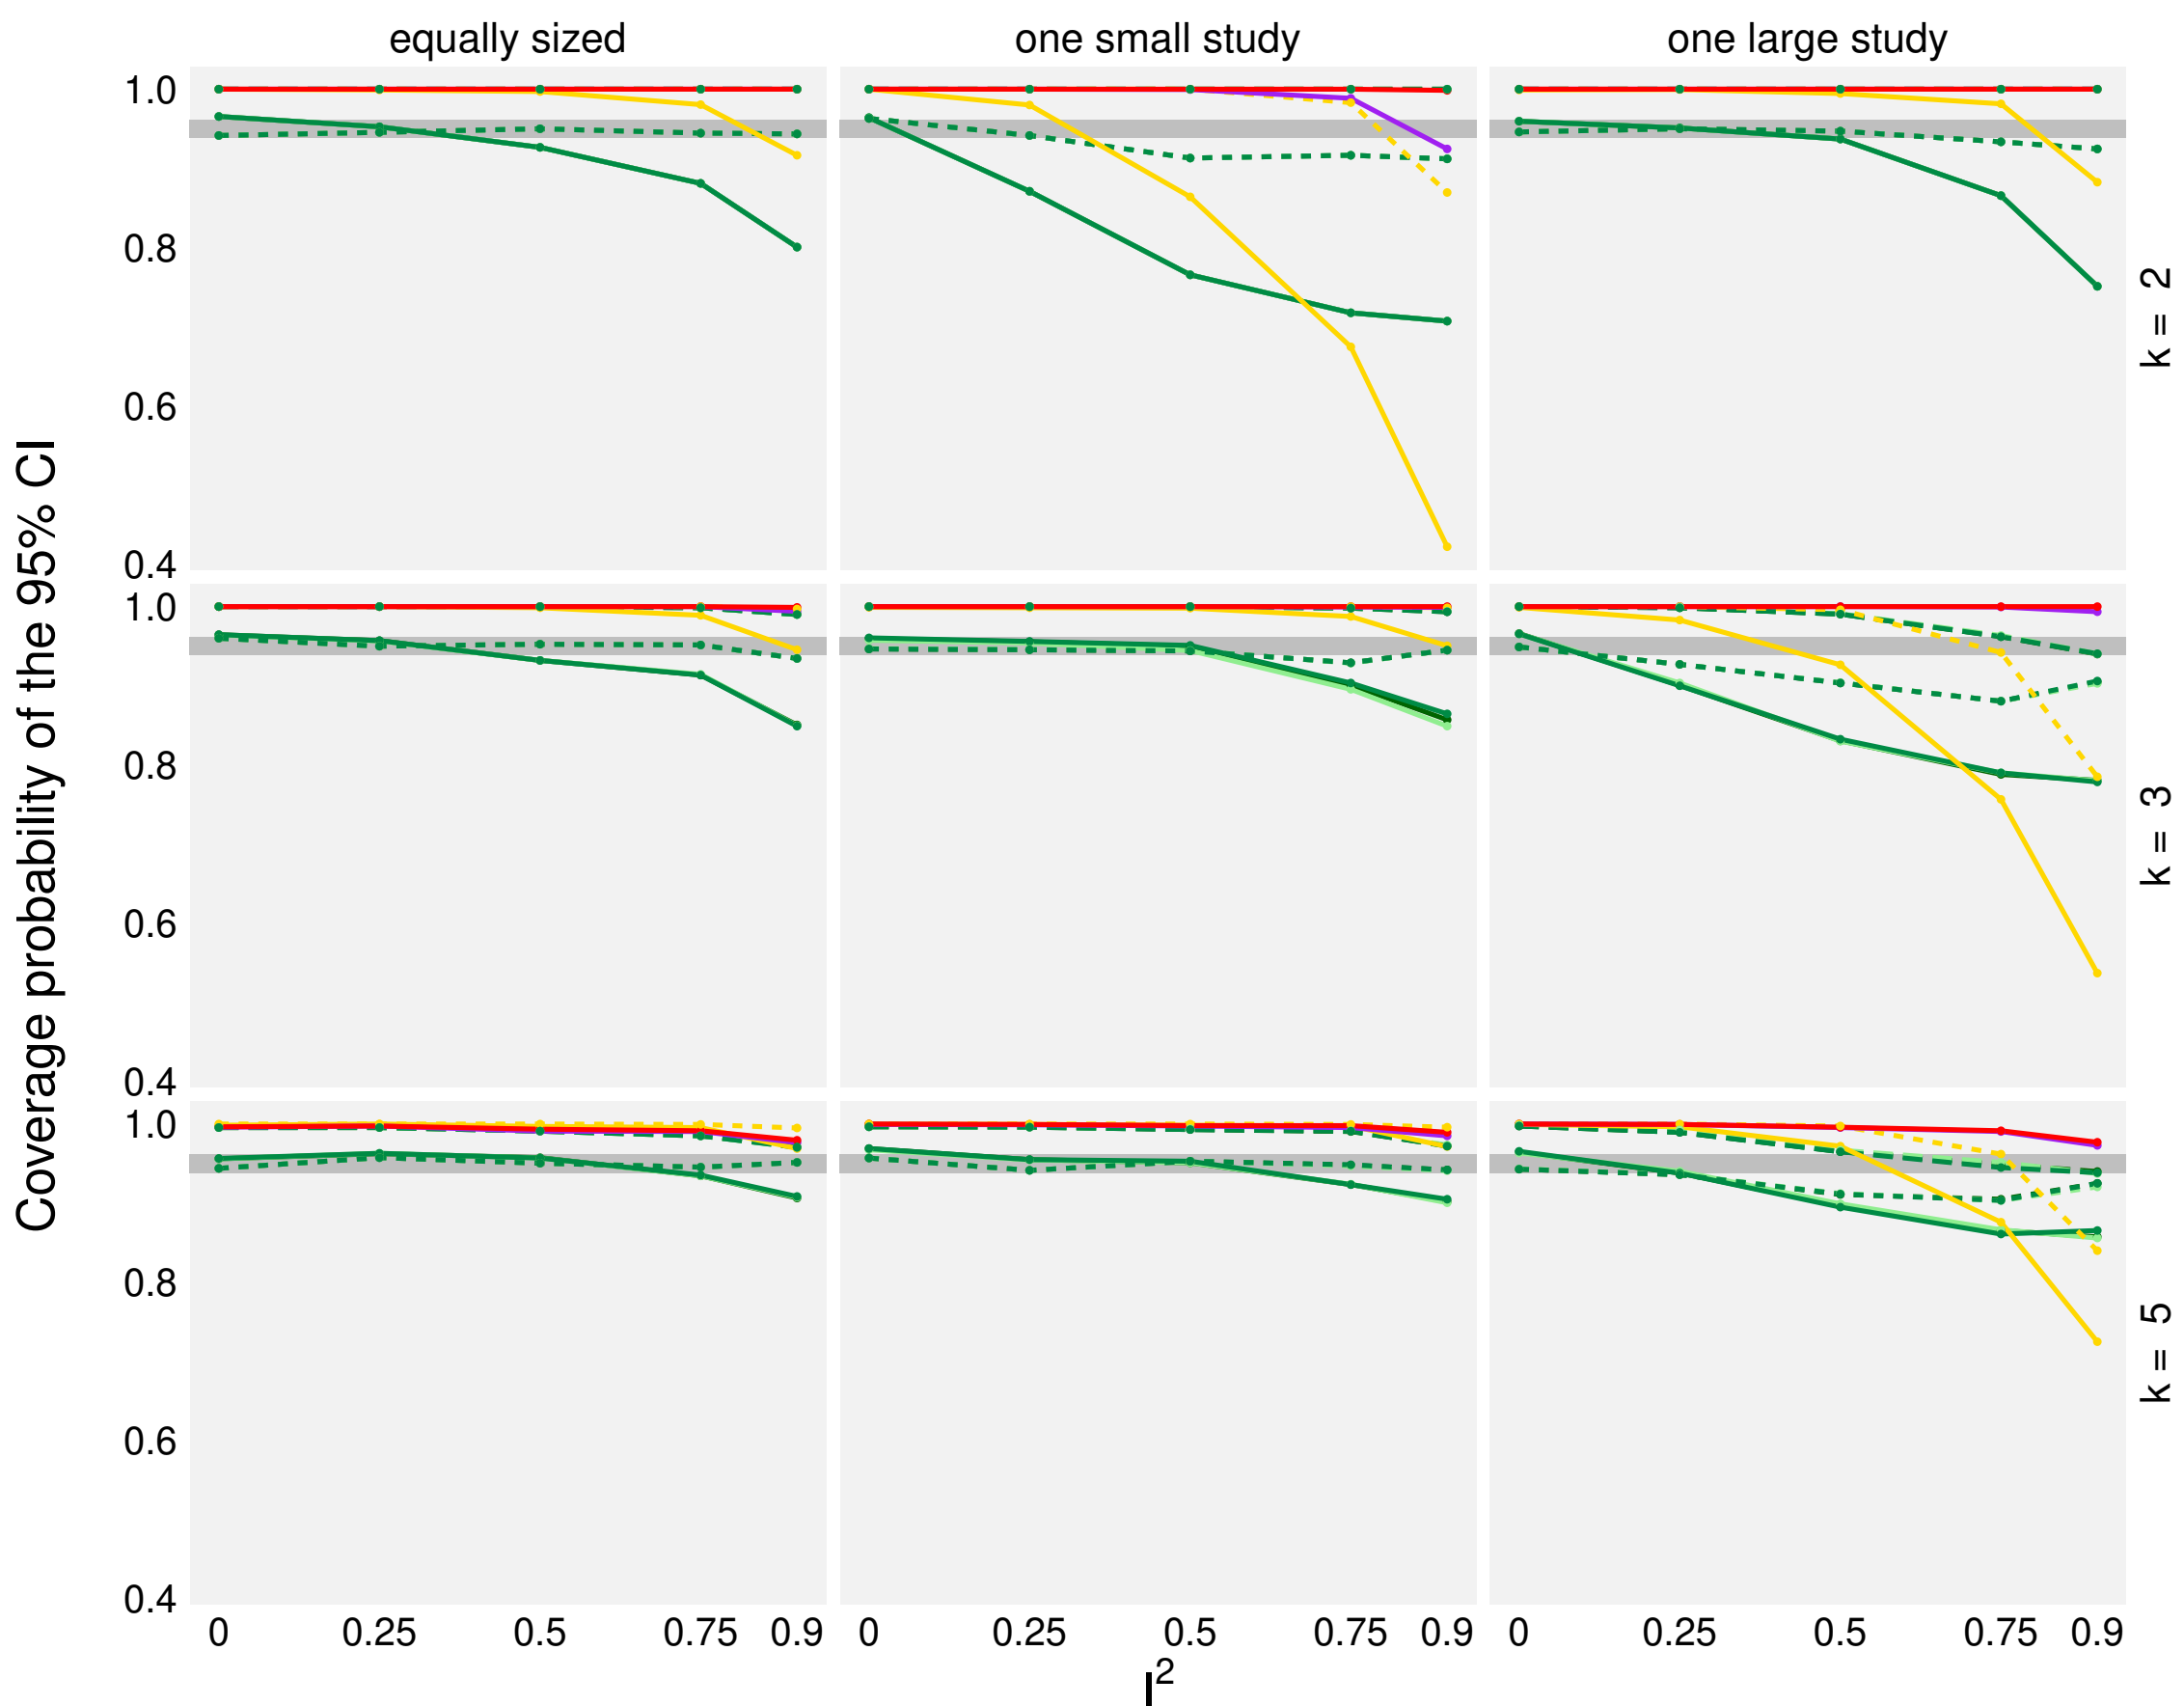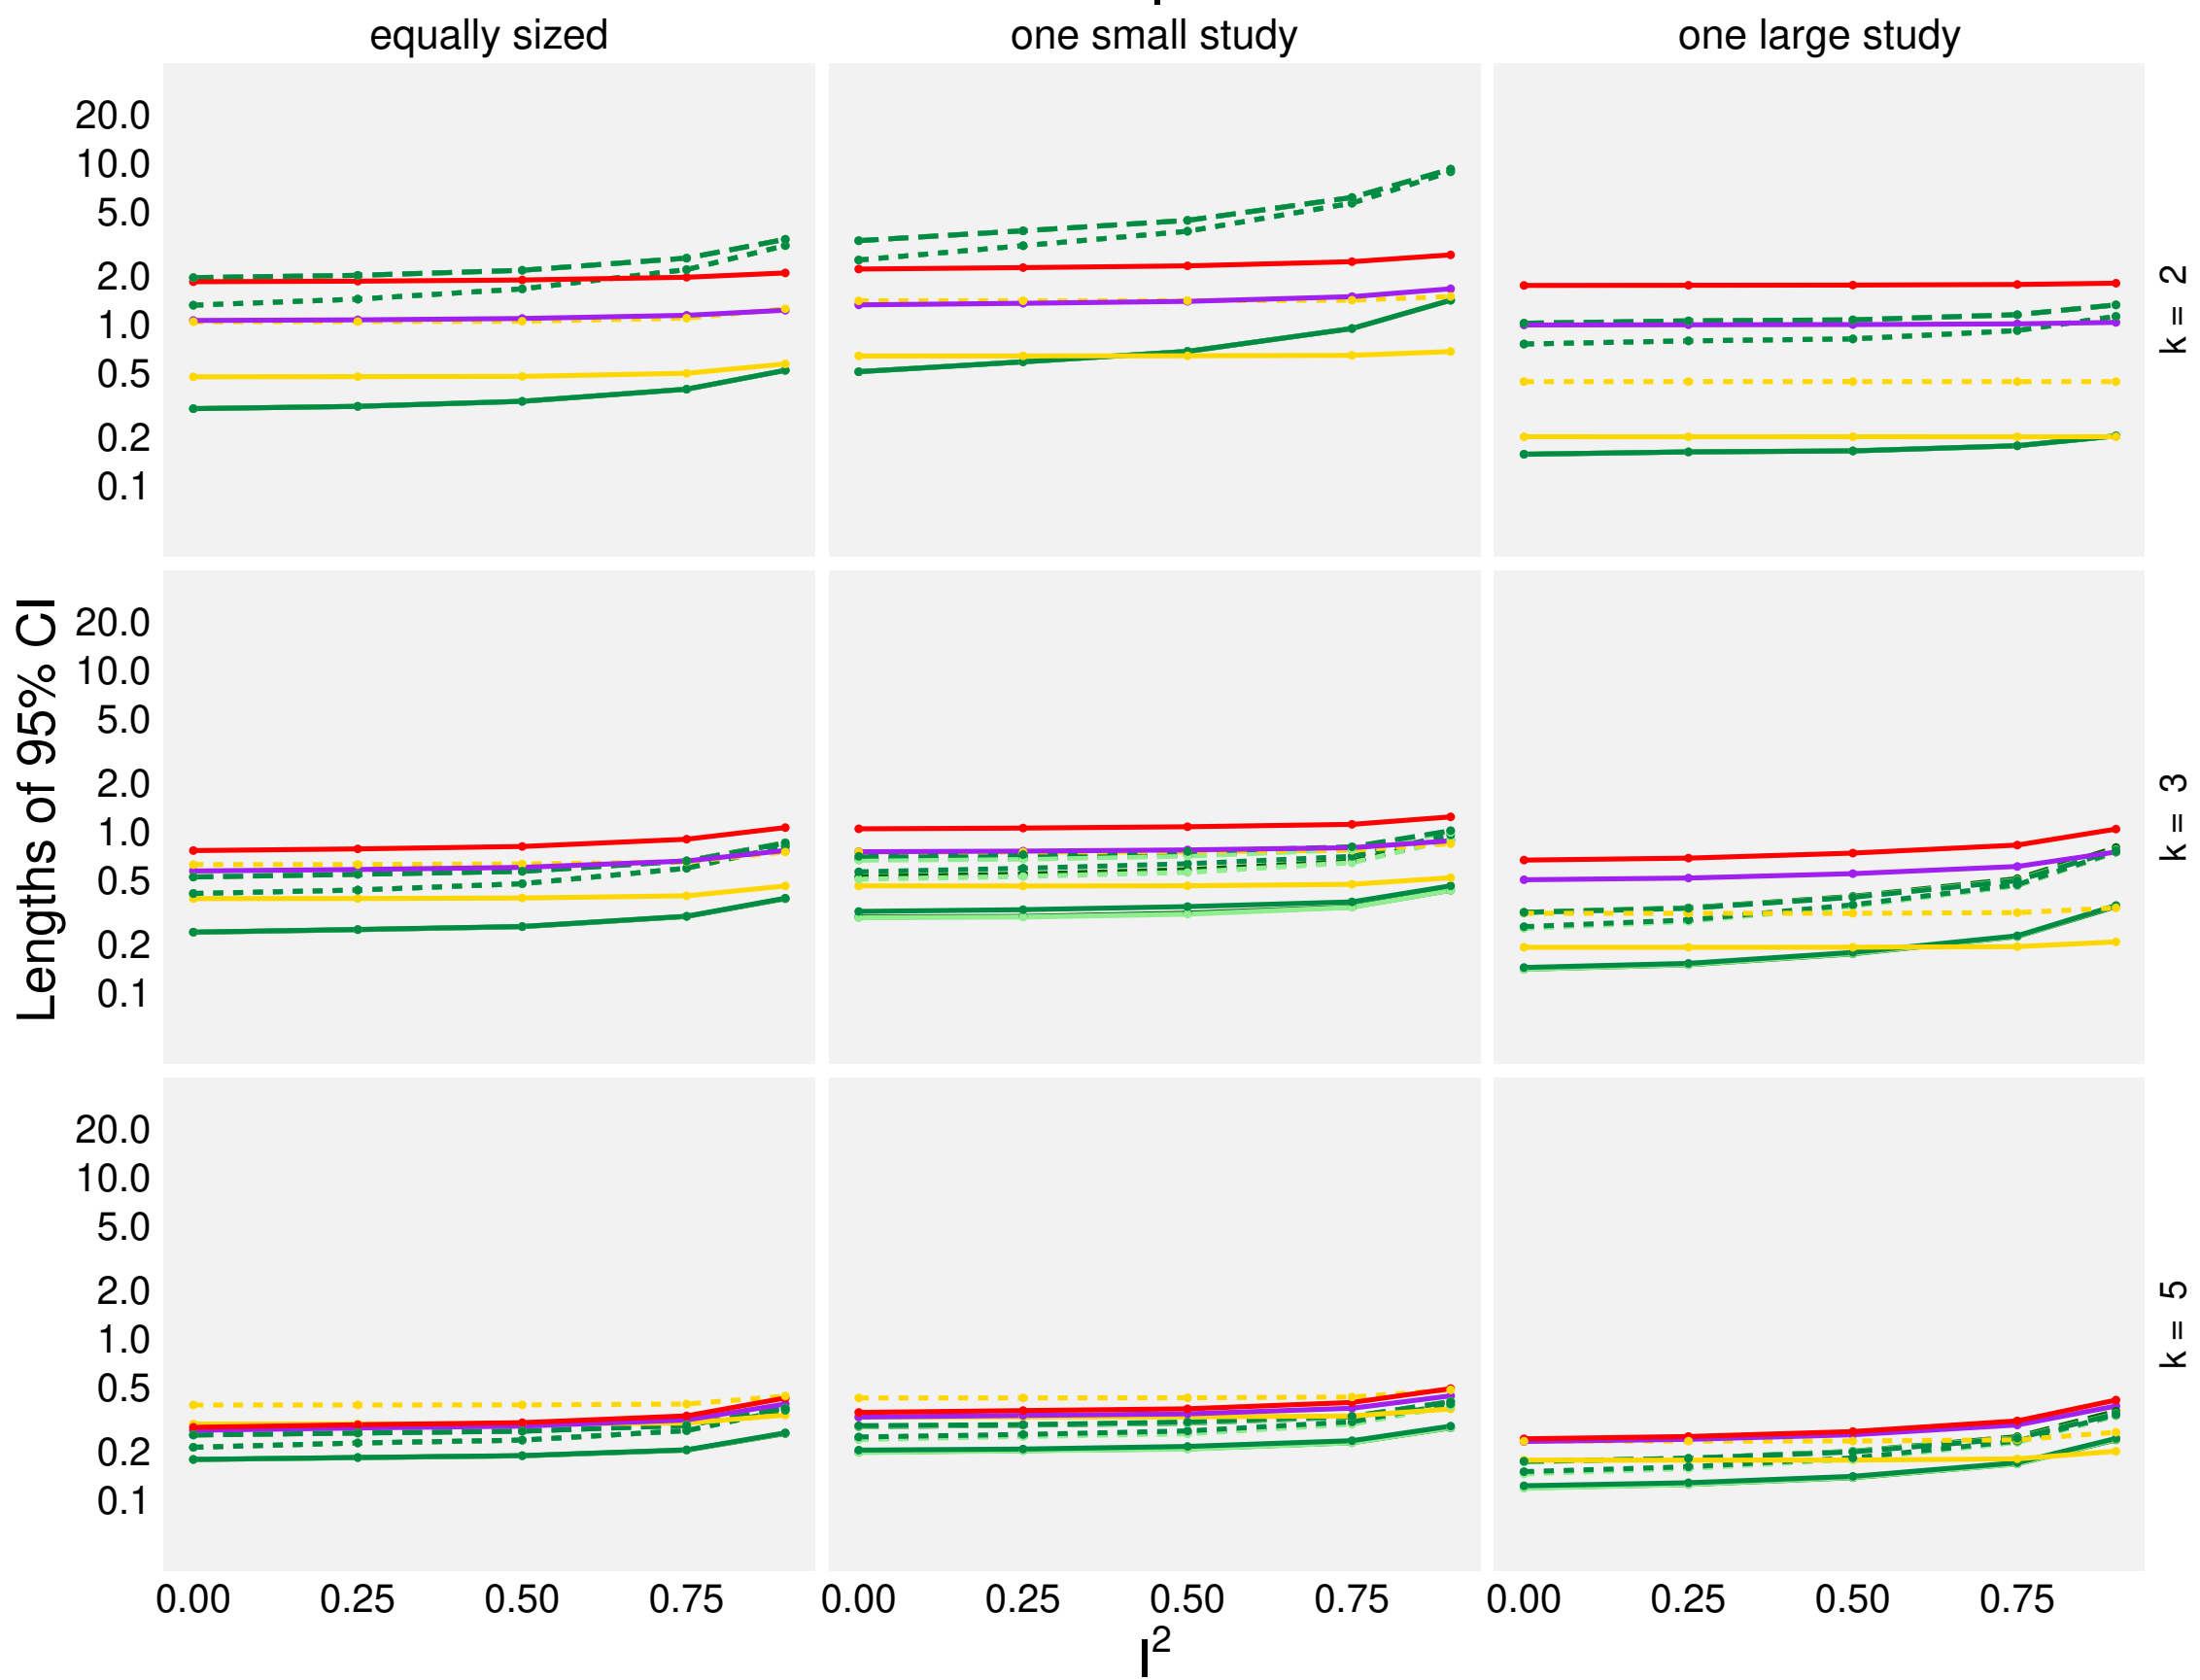

NN – DL  
 NN – REML  
 NN – EB  
 PN – PL  
 NN – Bayes HN(0.5)  
 NN – Bayes HN(1)  
 — normal quantiles  
 - - HKSJ or Student's t  
 - - mHKSJ

RR  
( $n_i=100, \pi_0=0.9$ )

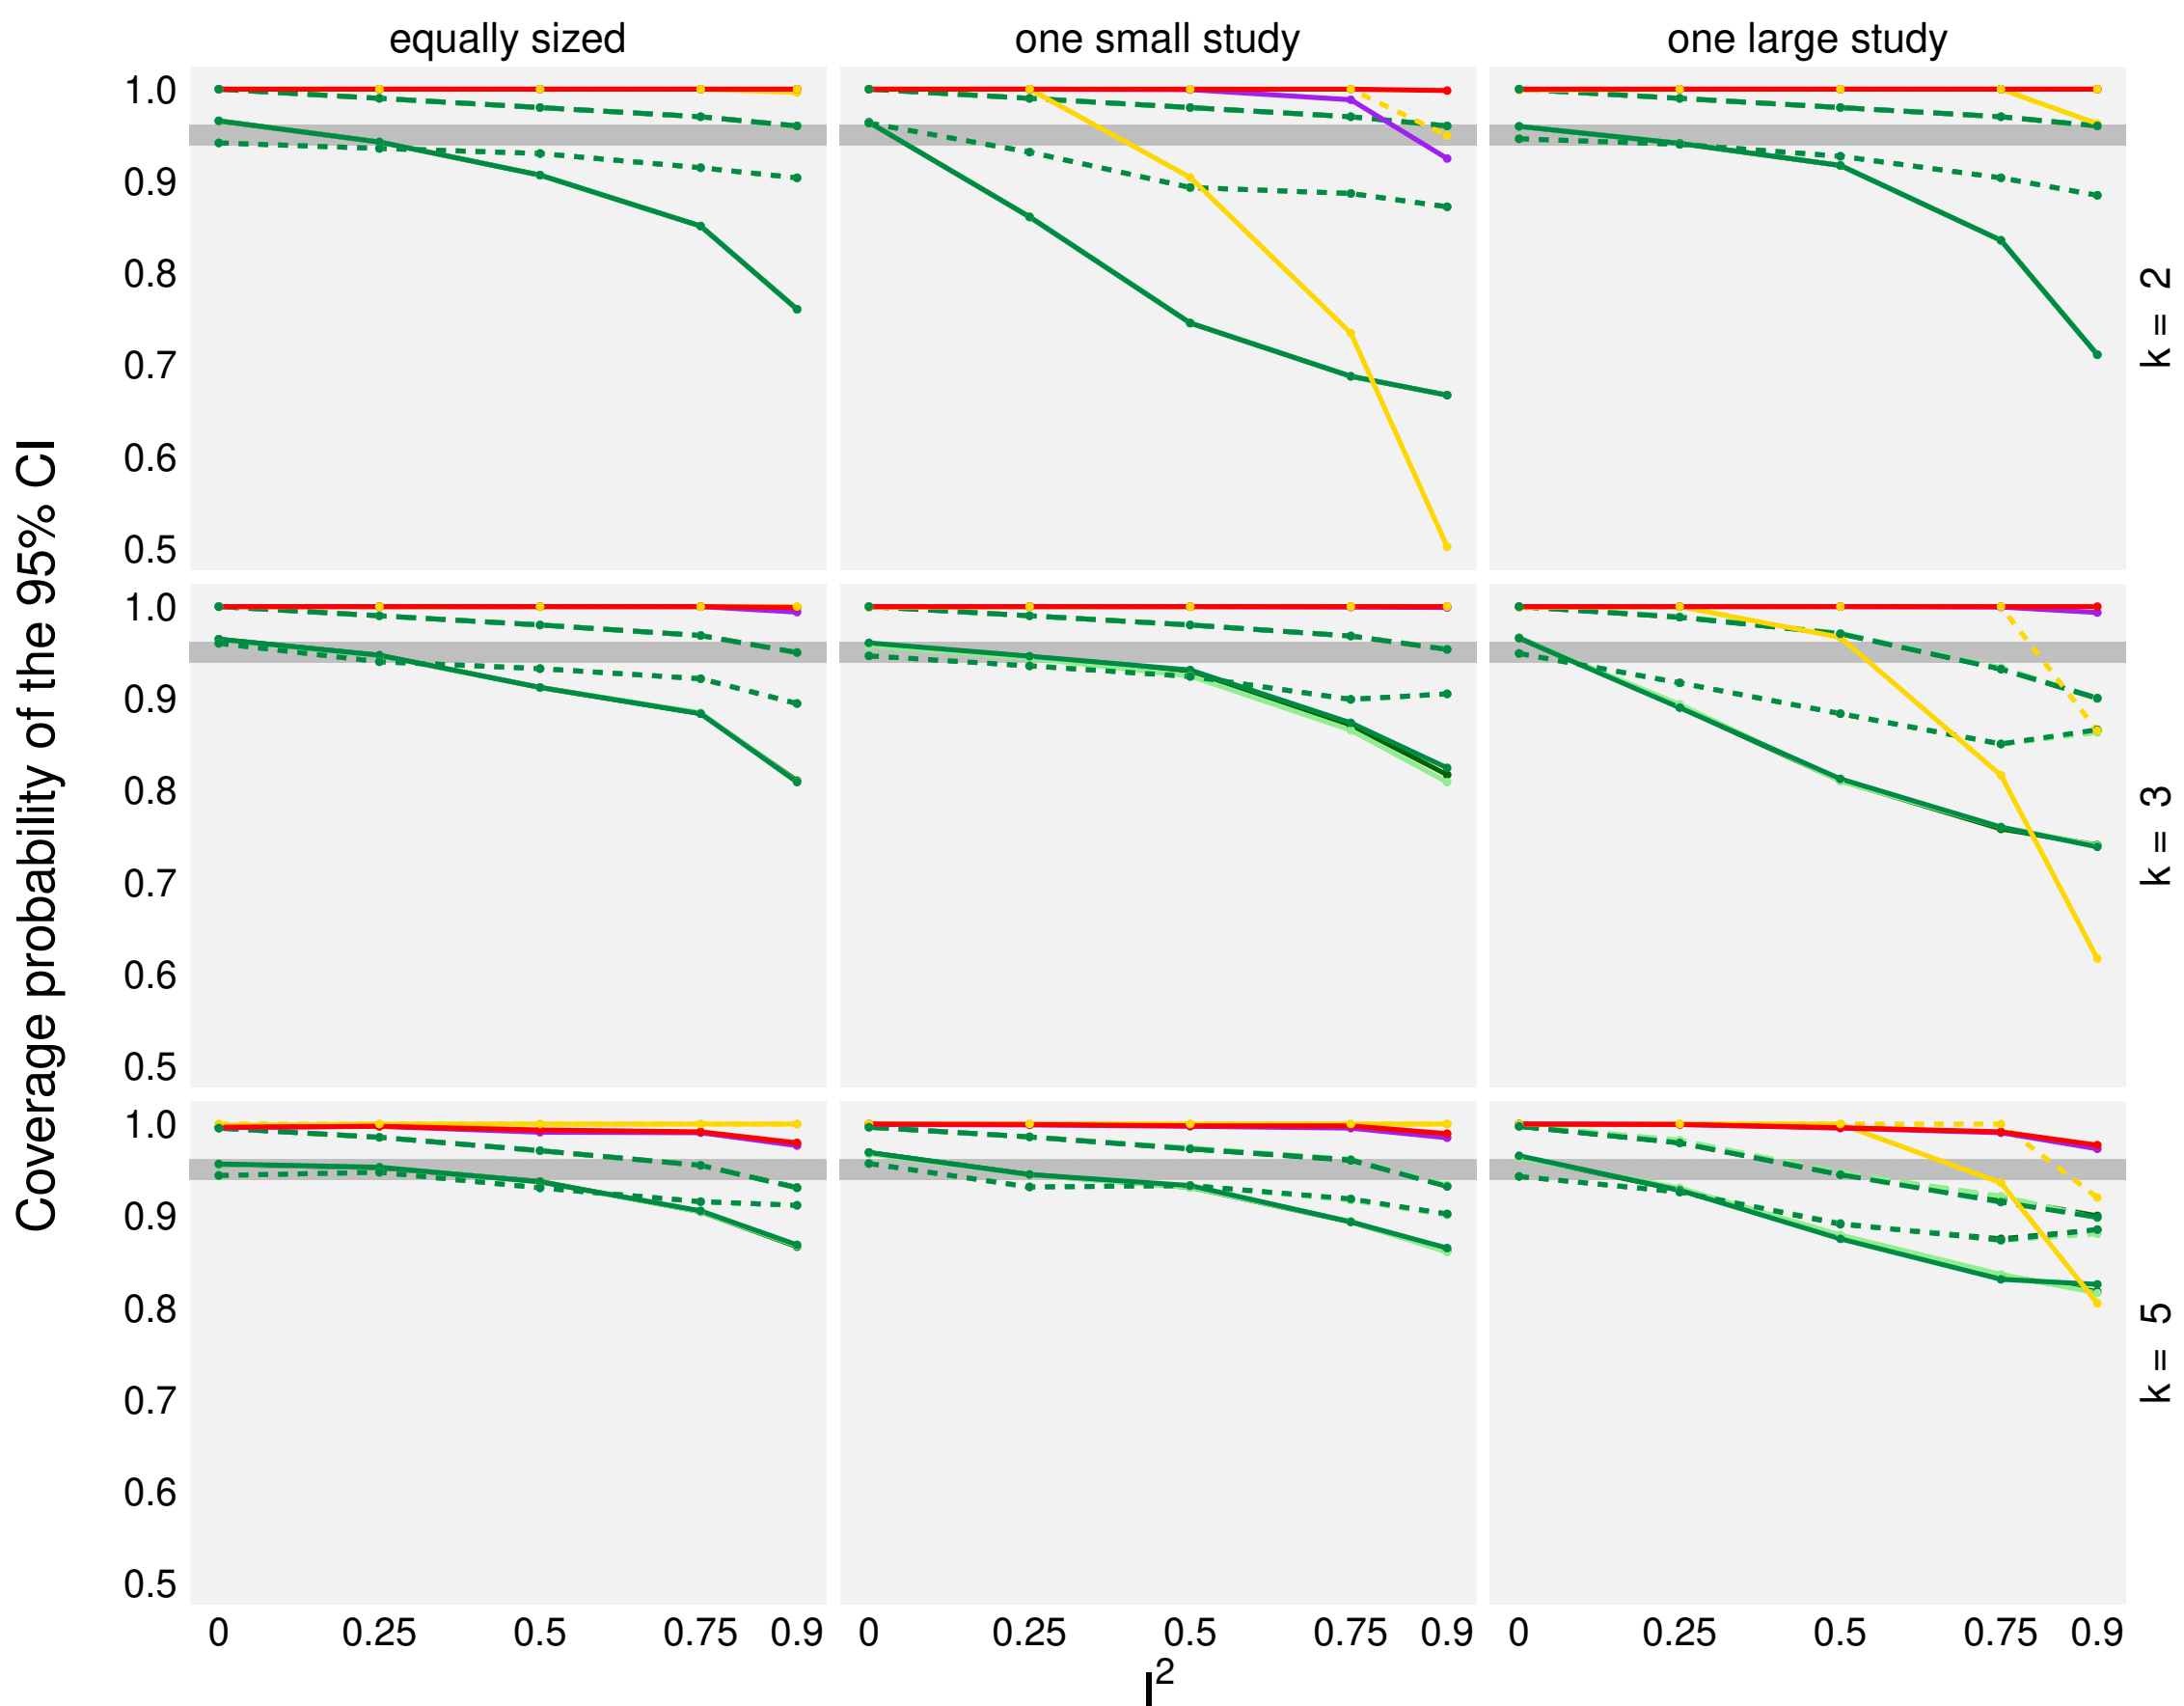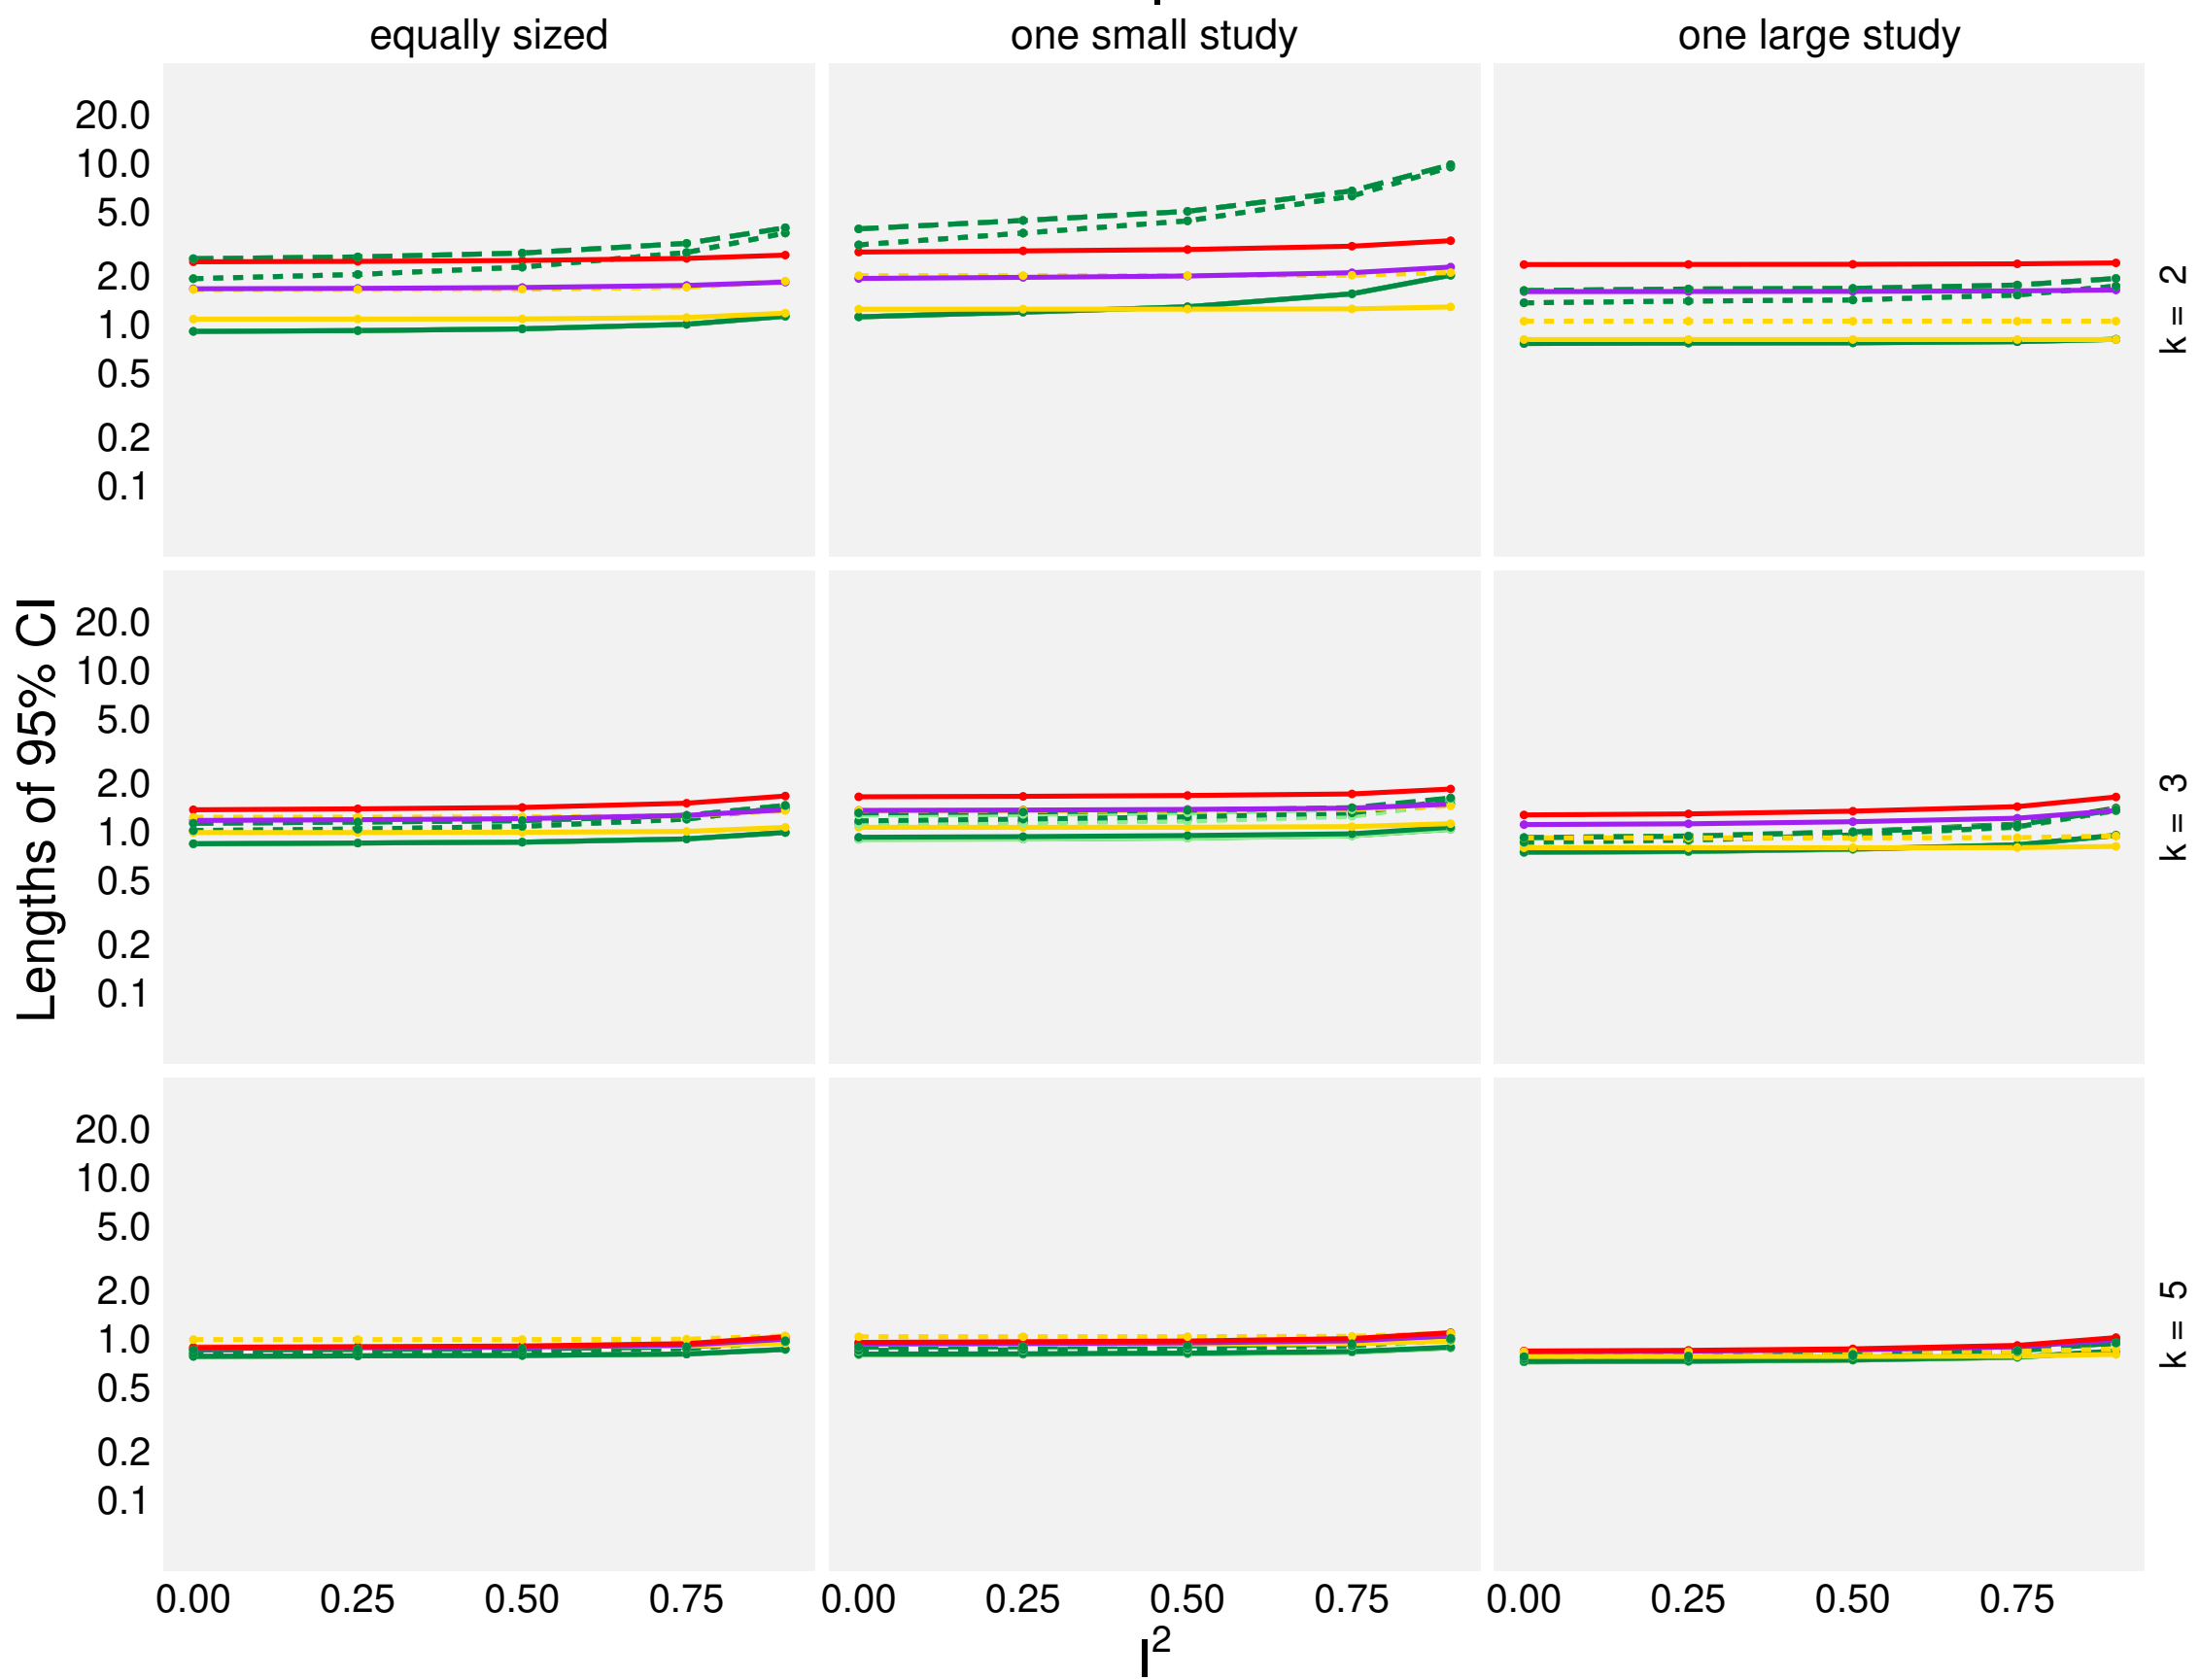

NN - DL    NN - PL  
 NN - REML    NN - Bayes HN(0.5)  
 NN - EB    NN - Bayes HN(1)

— normal quantiles  
 -- HKSJ or Student's t  
 ··· mHKSJ

RR  
( $n_i=250, \pi_0=0.1$ )

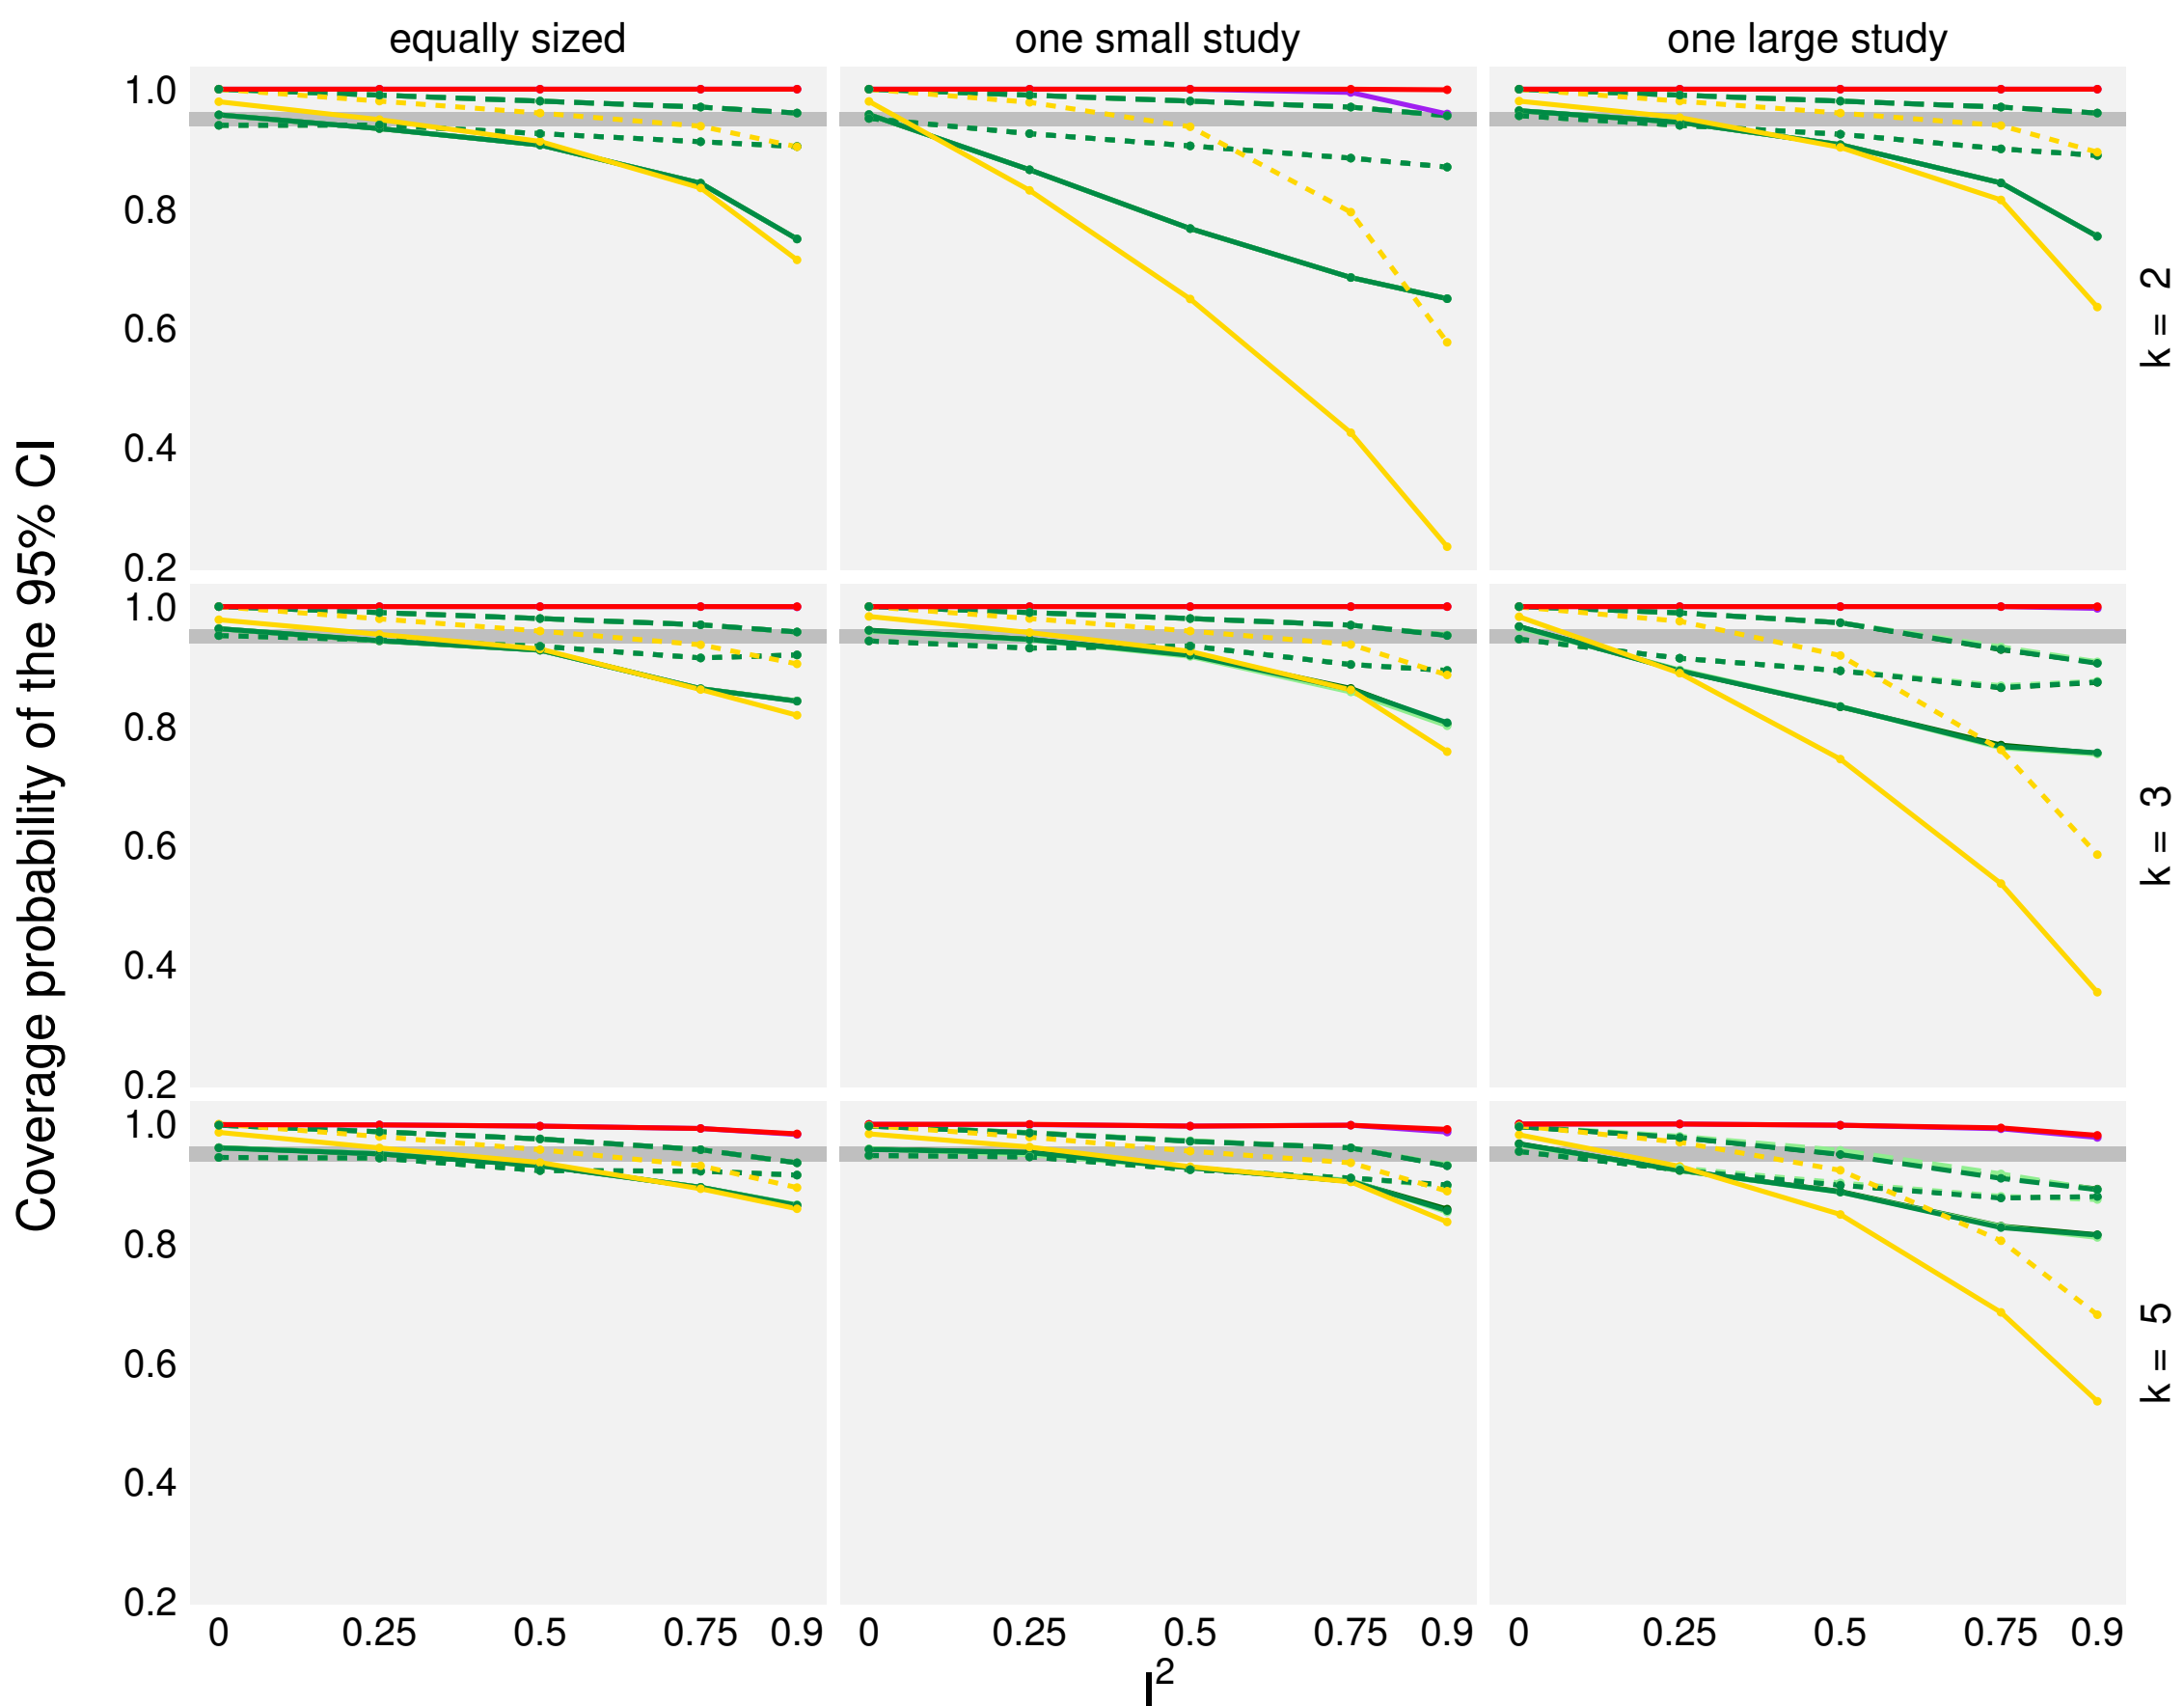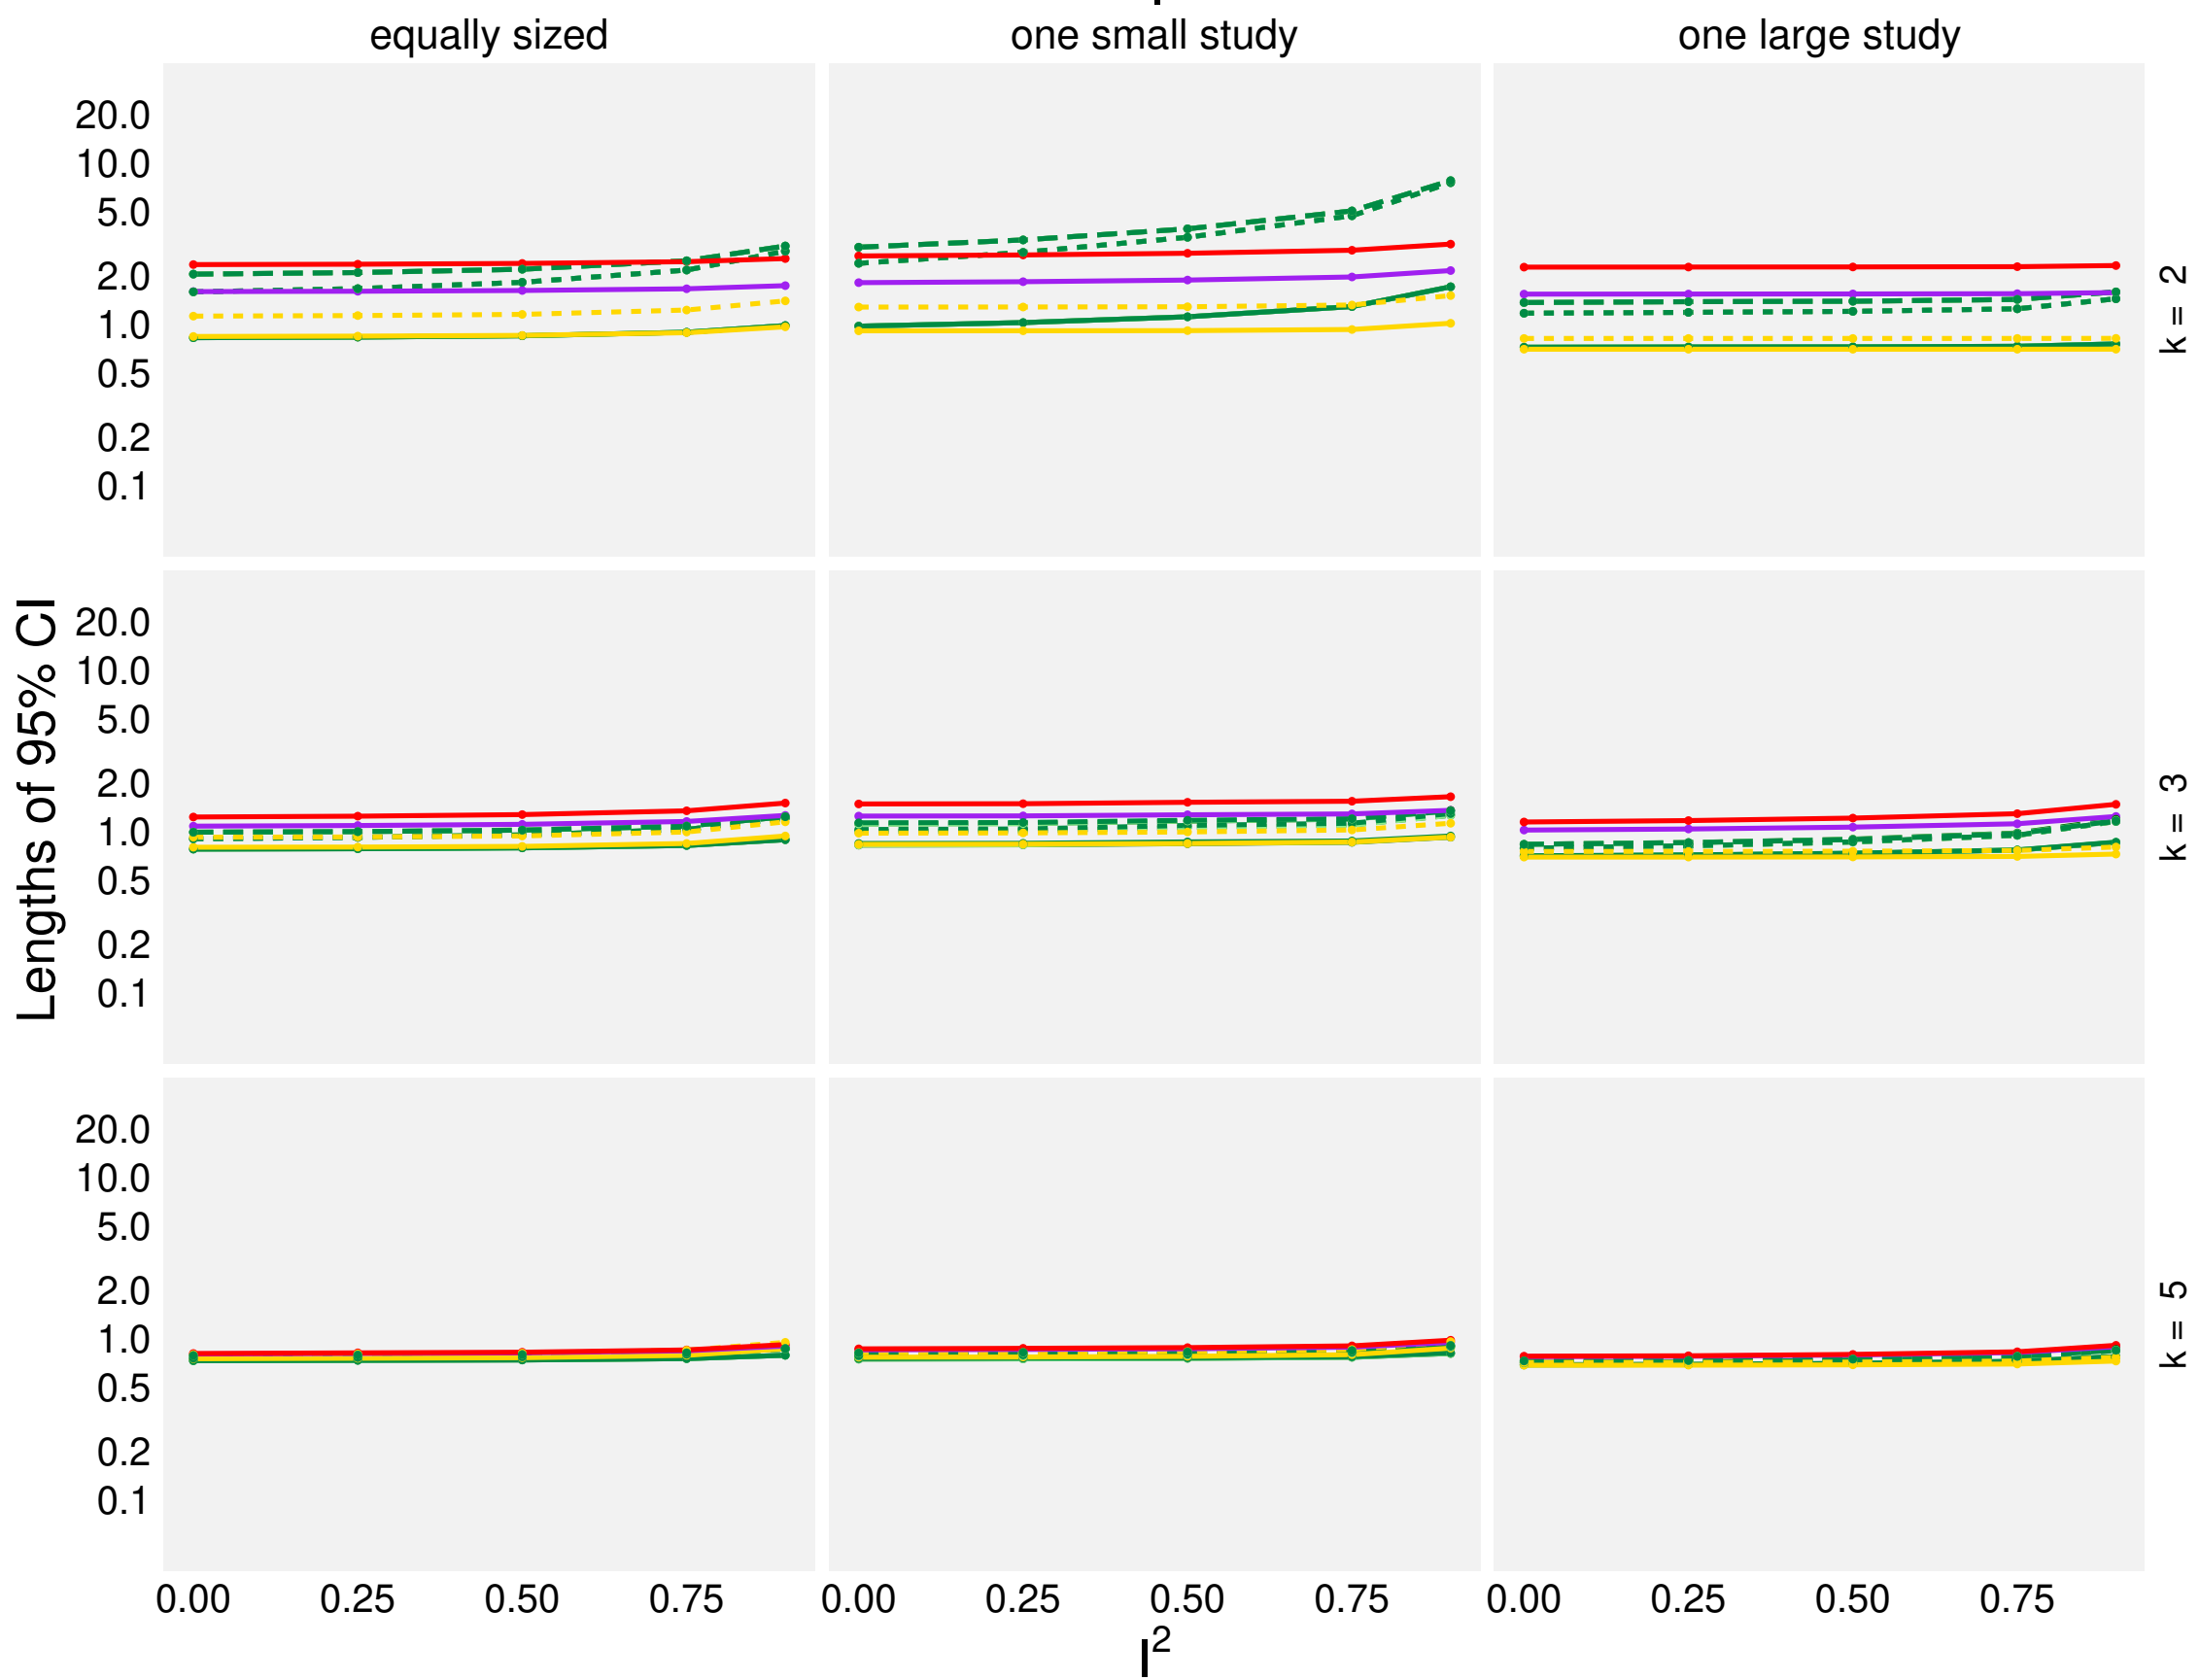

NN - DL  
 NN - REML  
 NN - EB  
 PN - PL  
 NN - Bayes HN(0.5)  
 NN - Bayes HN(1)  
 — normal quantiles  
 -- HKSJ or Student's t  
 -·- mHKSJ

RR  
( $n_i=250, \pi_0=0.3$ )

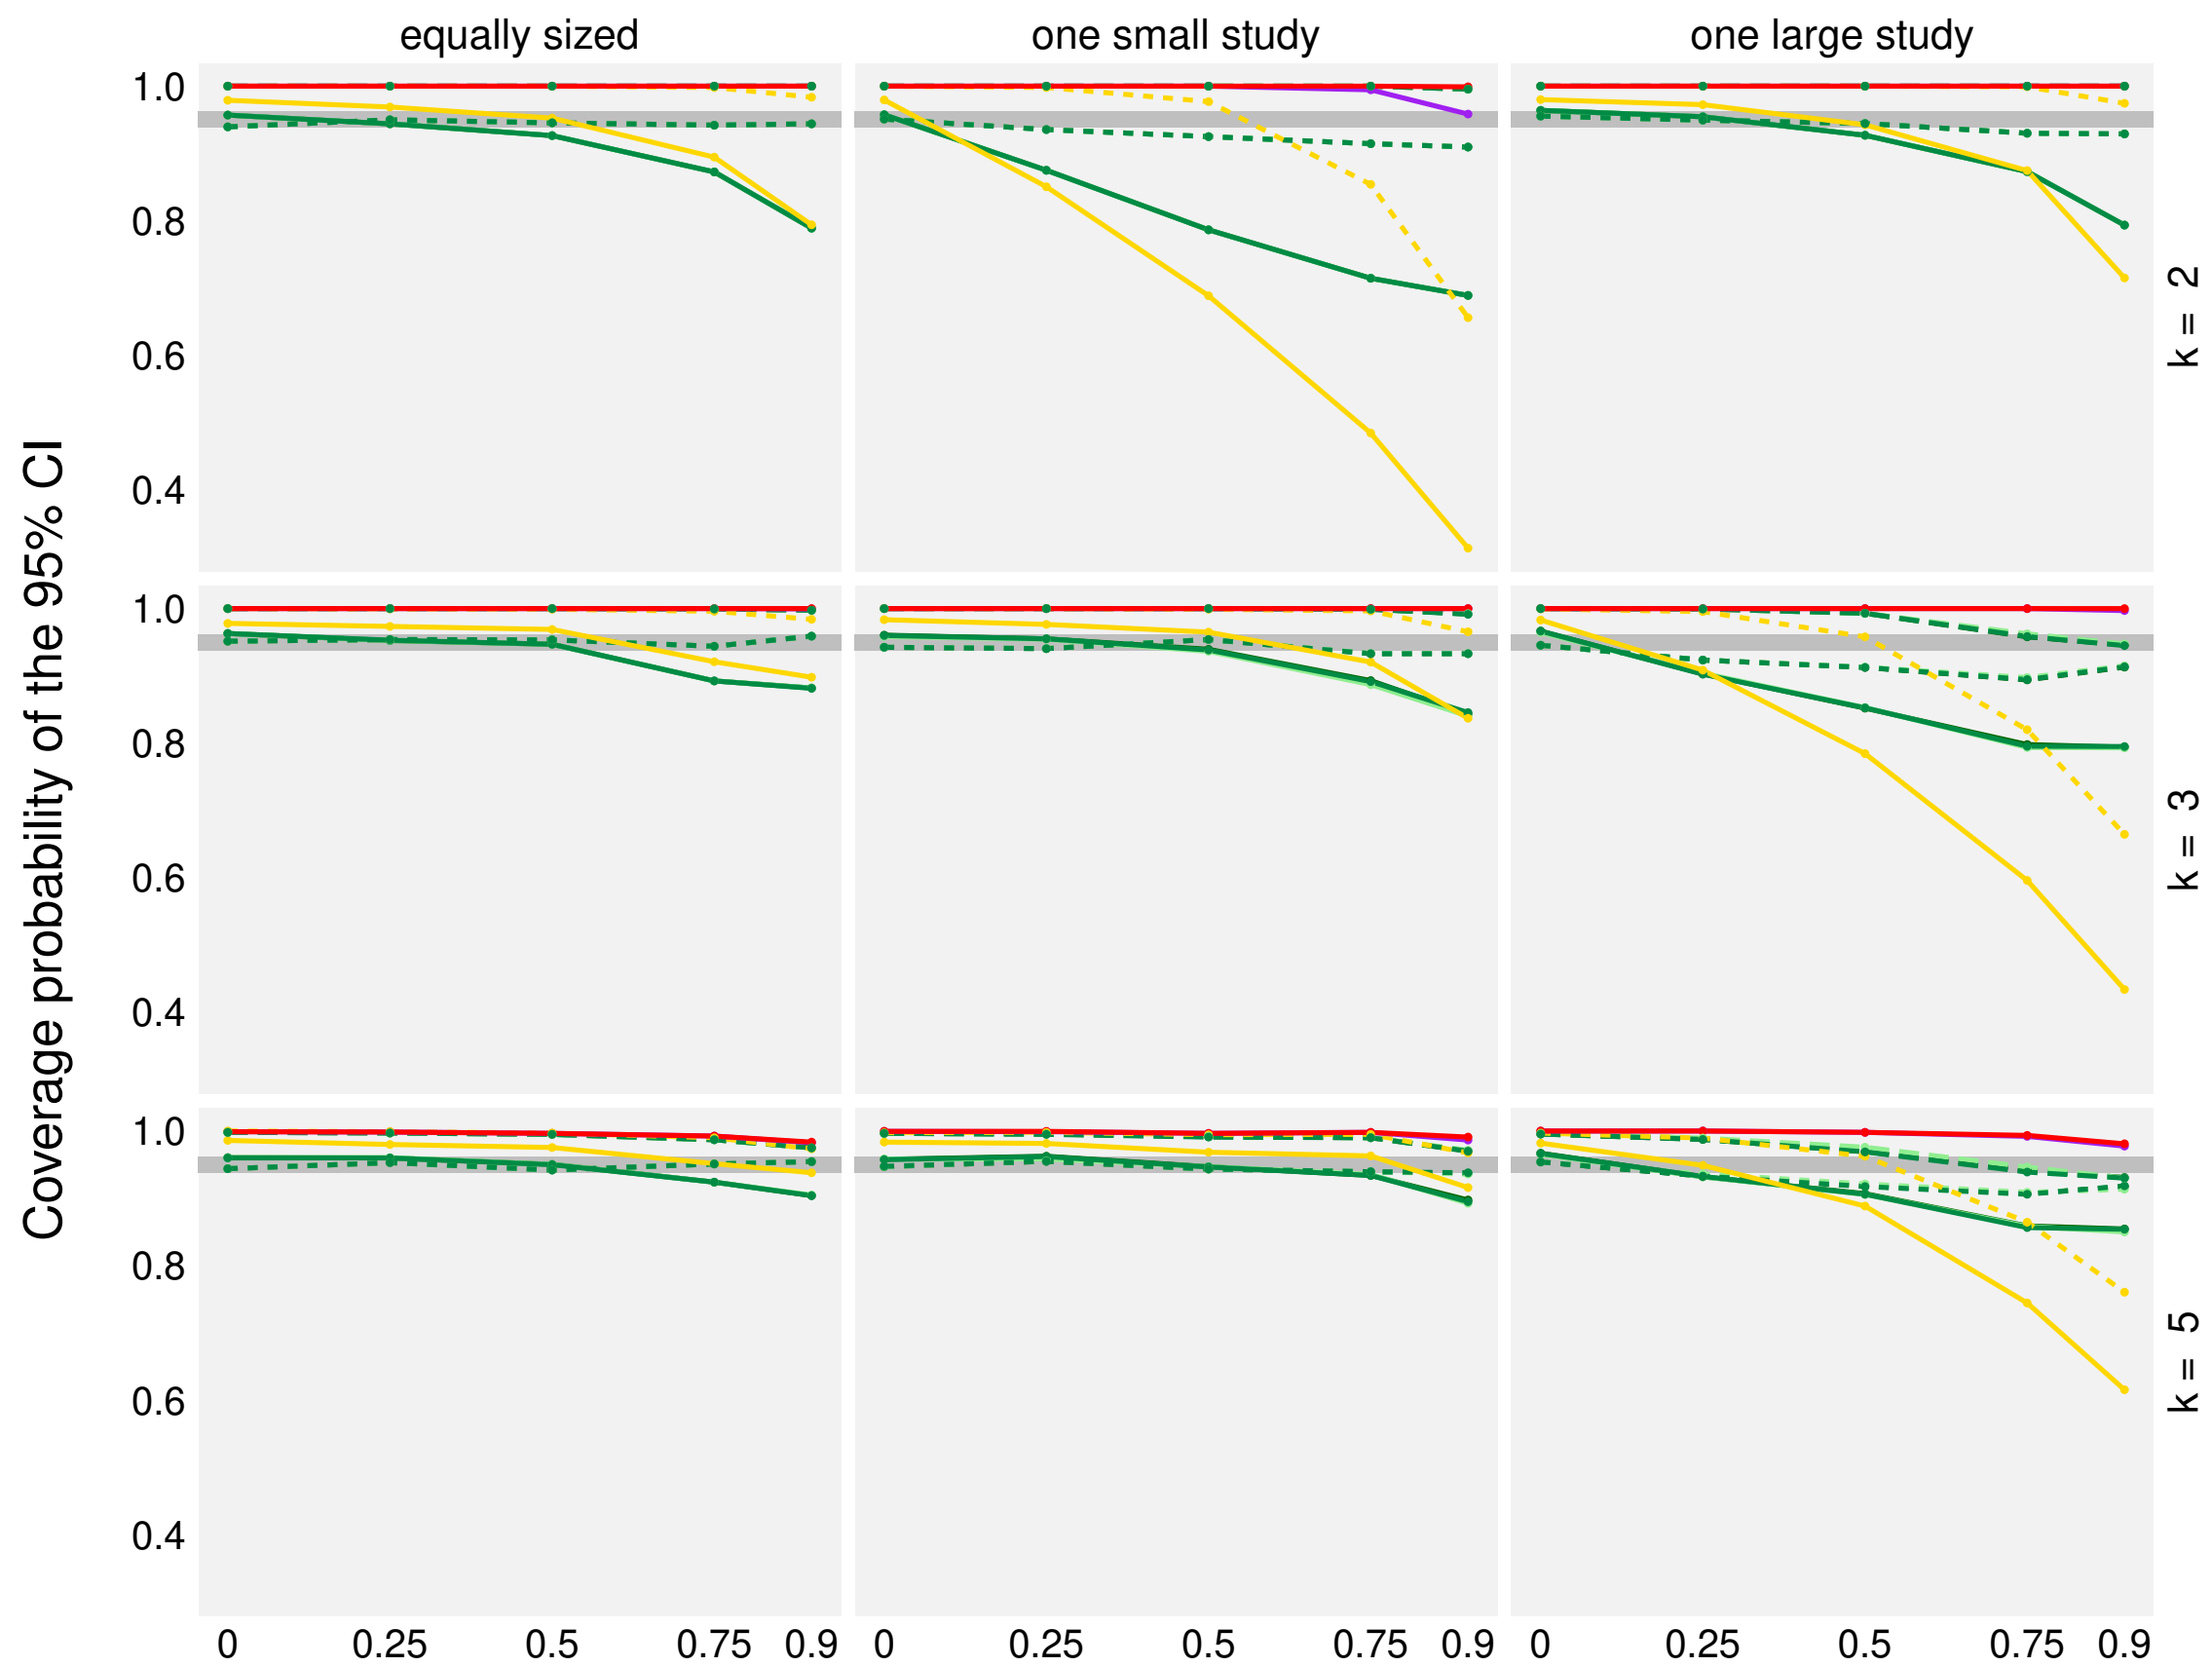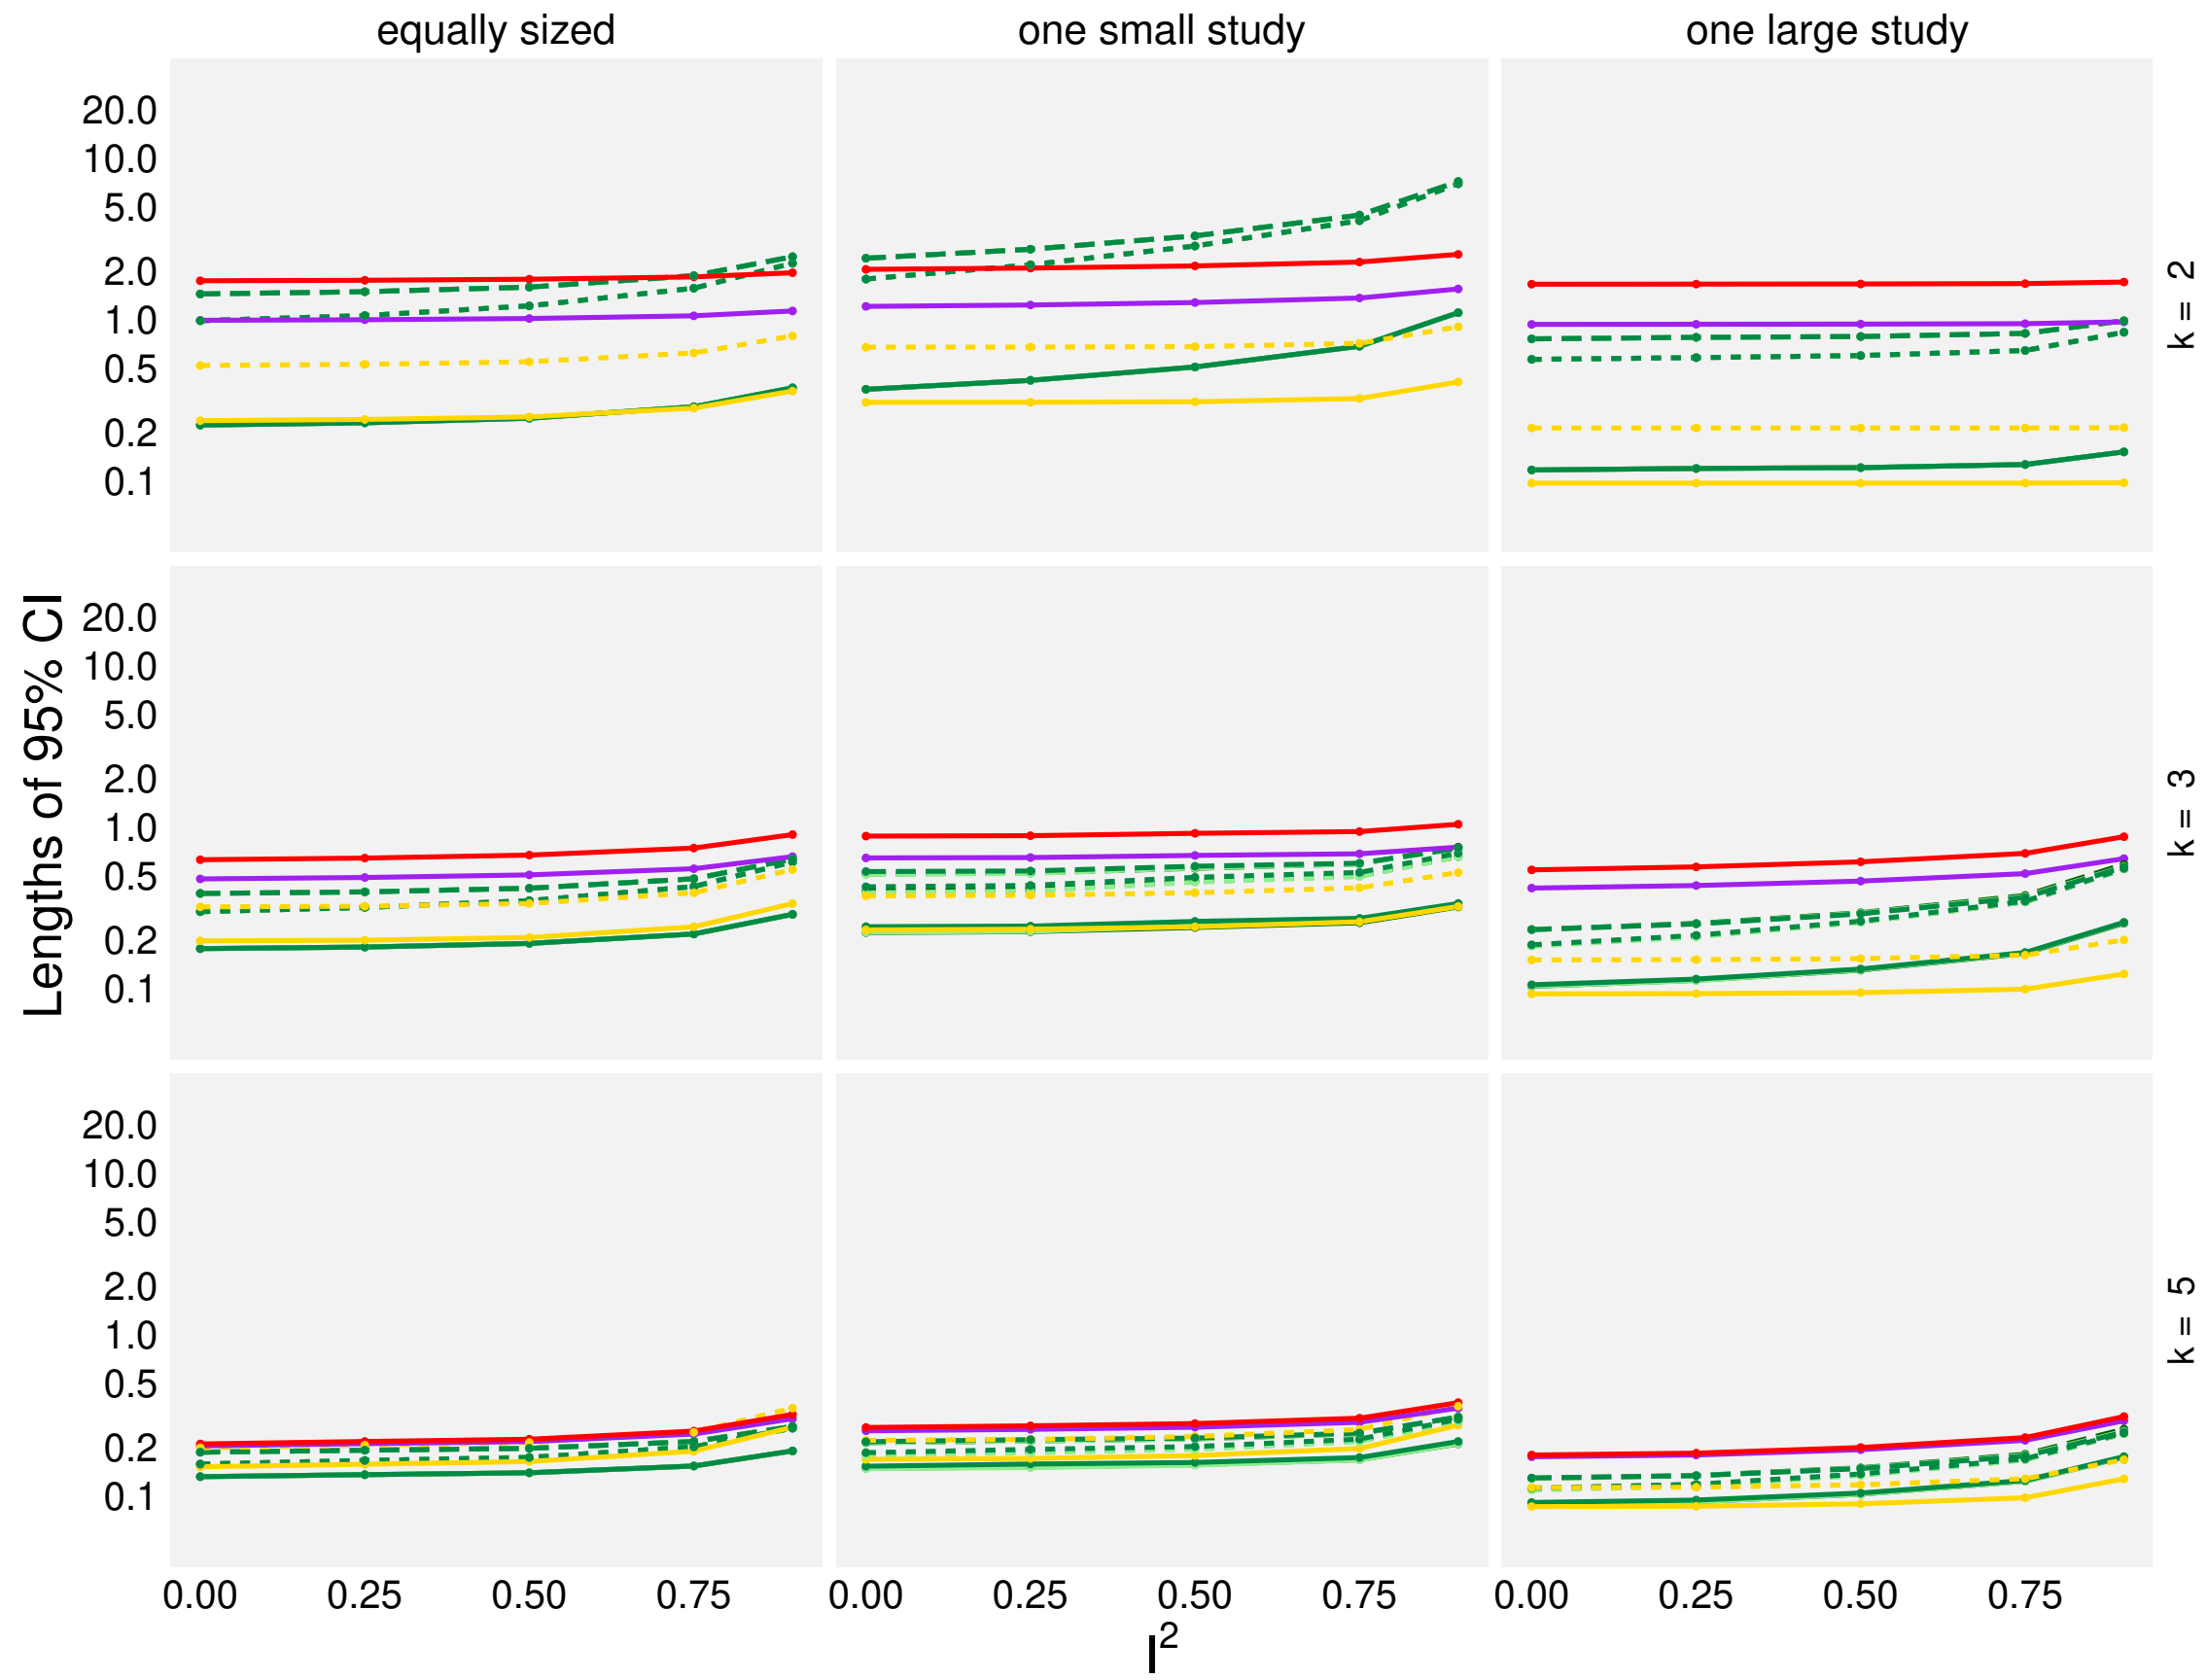

— NN – DL      — PN – PL      — normal quantiles  
 — NN – REML      — NN – Bayes HN(0.5)      - - HKSJ or Student's t  
 — NN – EB      — NN – Bayes HN(1)      - - mHKSJ

RR  
( $n_i=250, \pi_0=0.5$ )

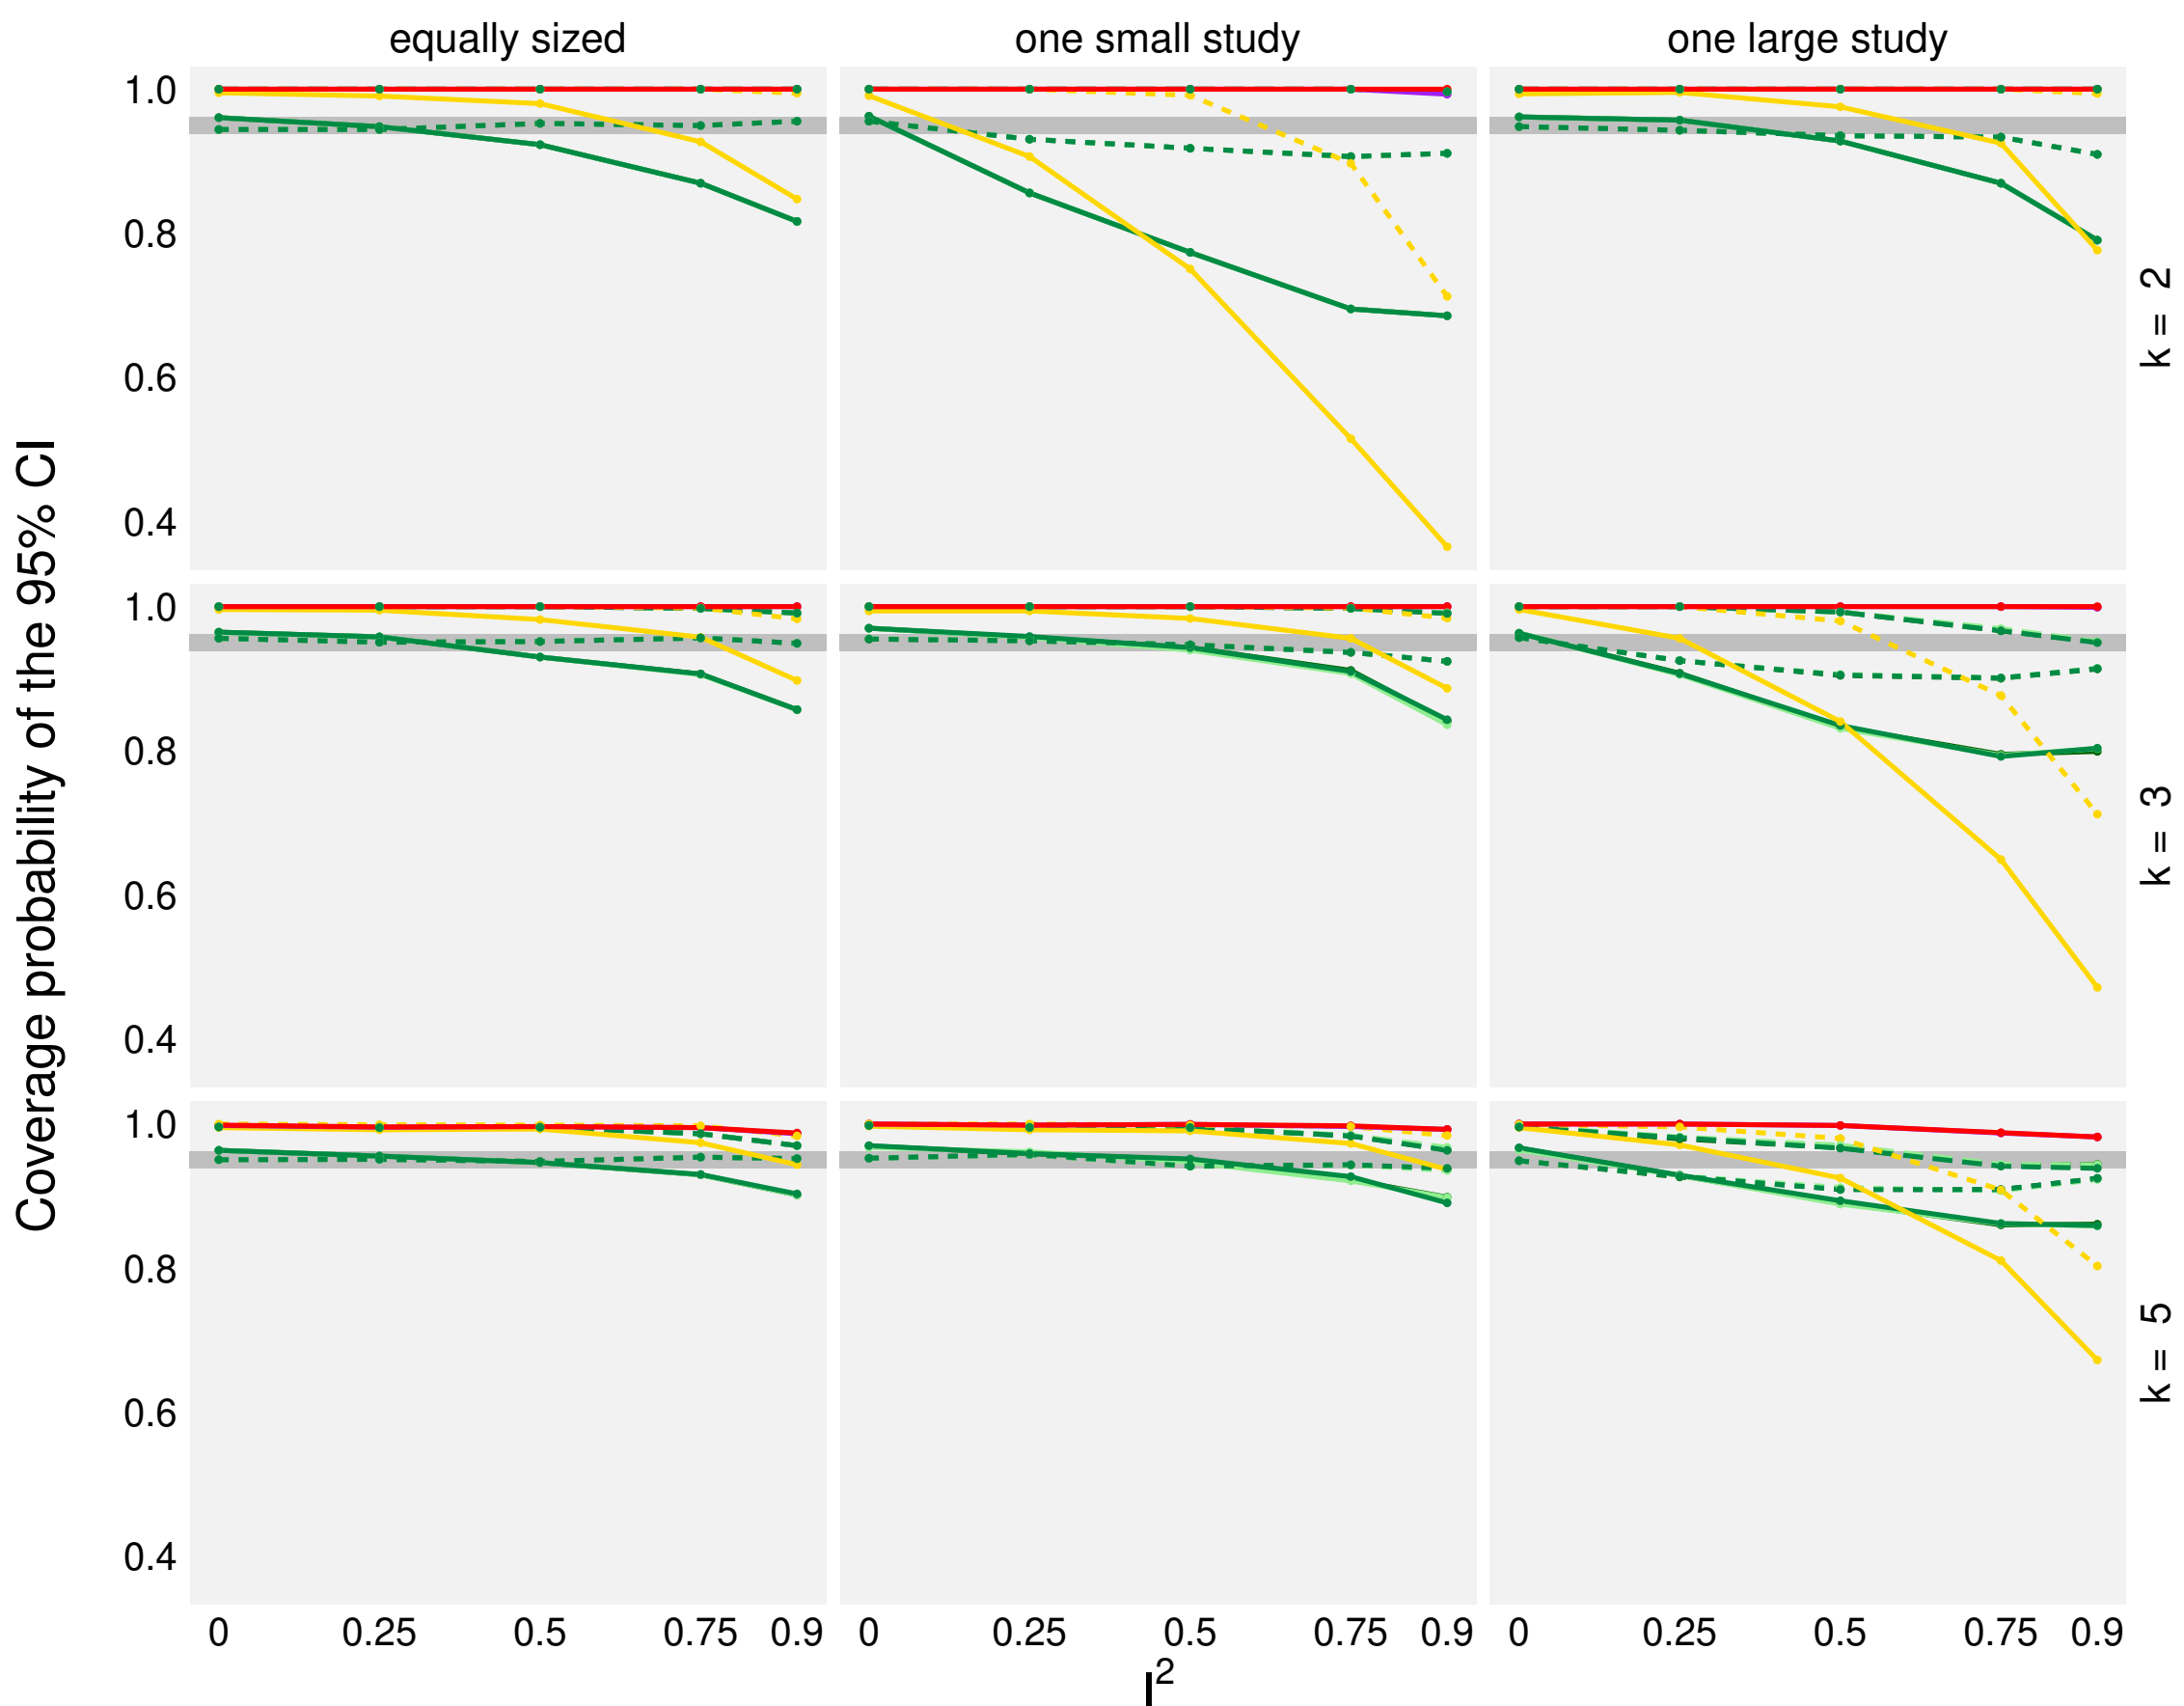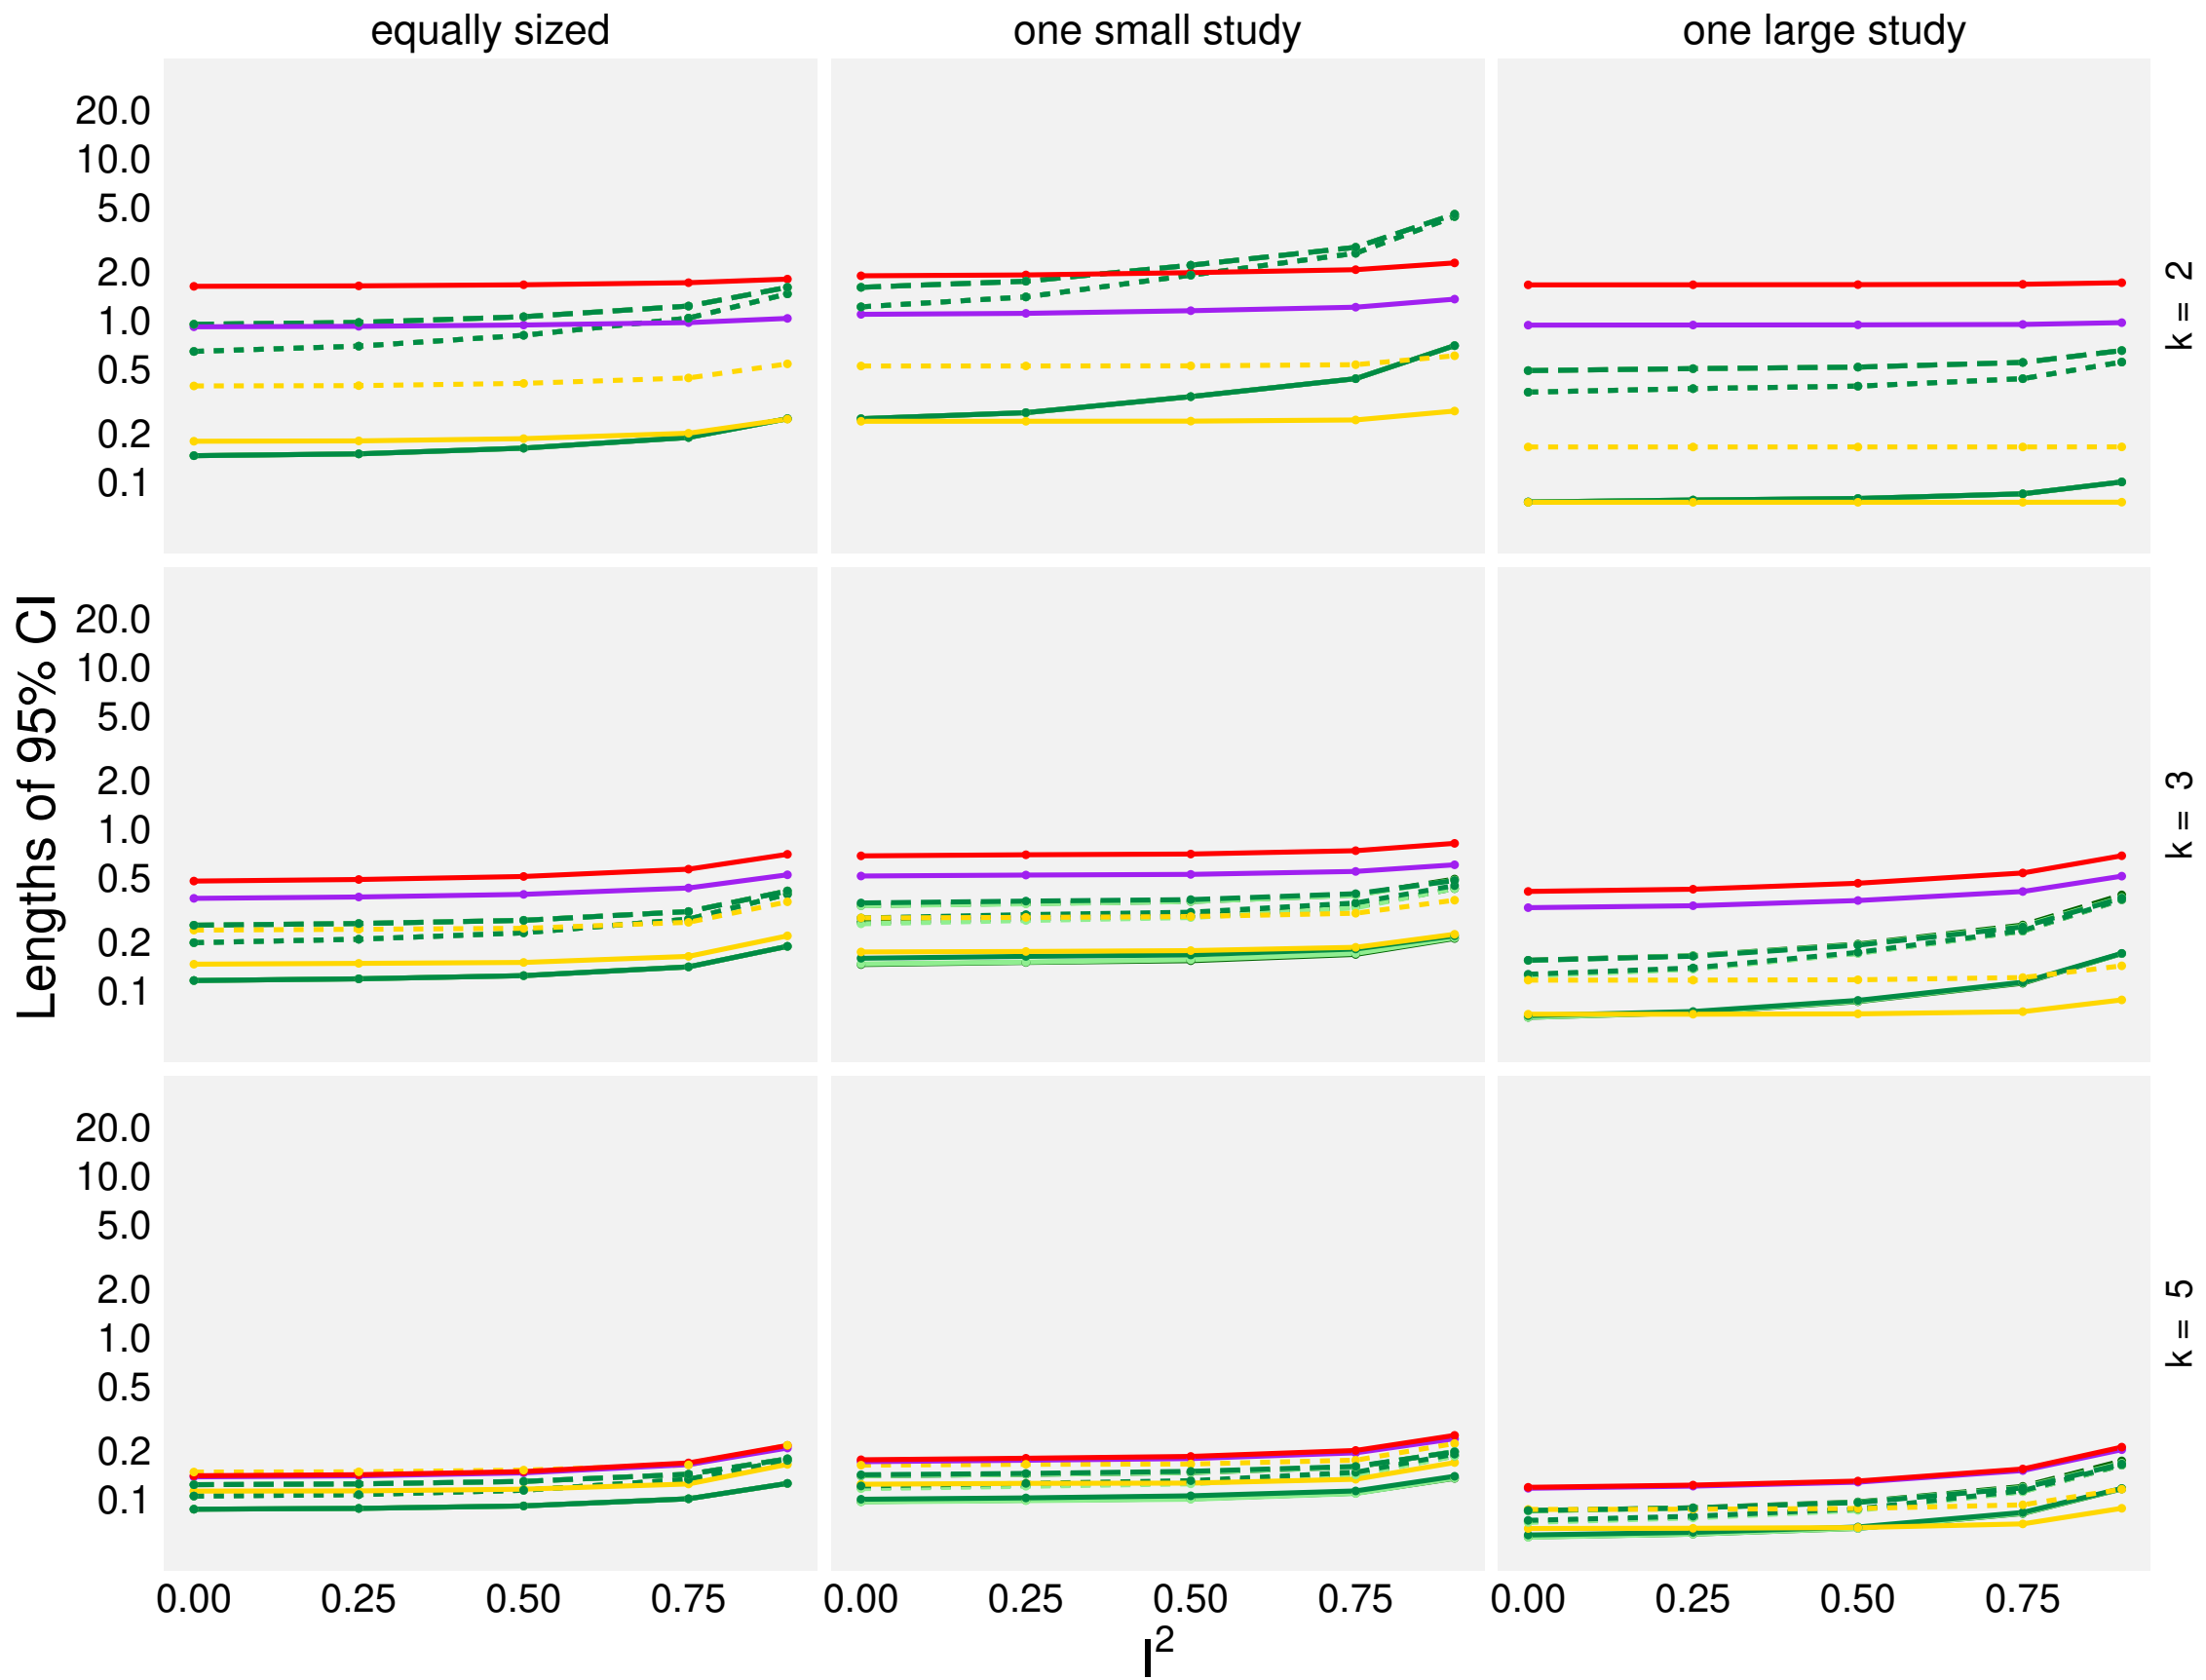

NN – DL  
 NN – REML  
 NN – EB  
 PN – PL  
 NN – Bayes HN(0.5)  
 NN – Bayes HN(1)  
 — normal quantiles  
 - - HKSJ or Student's t  
 - - mHKSJ

RR  
( $n_i=250, \pi_0=0.7$ )

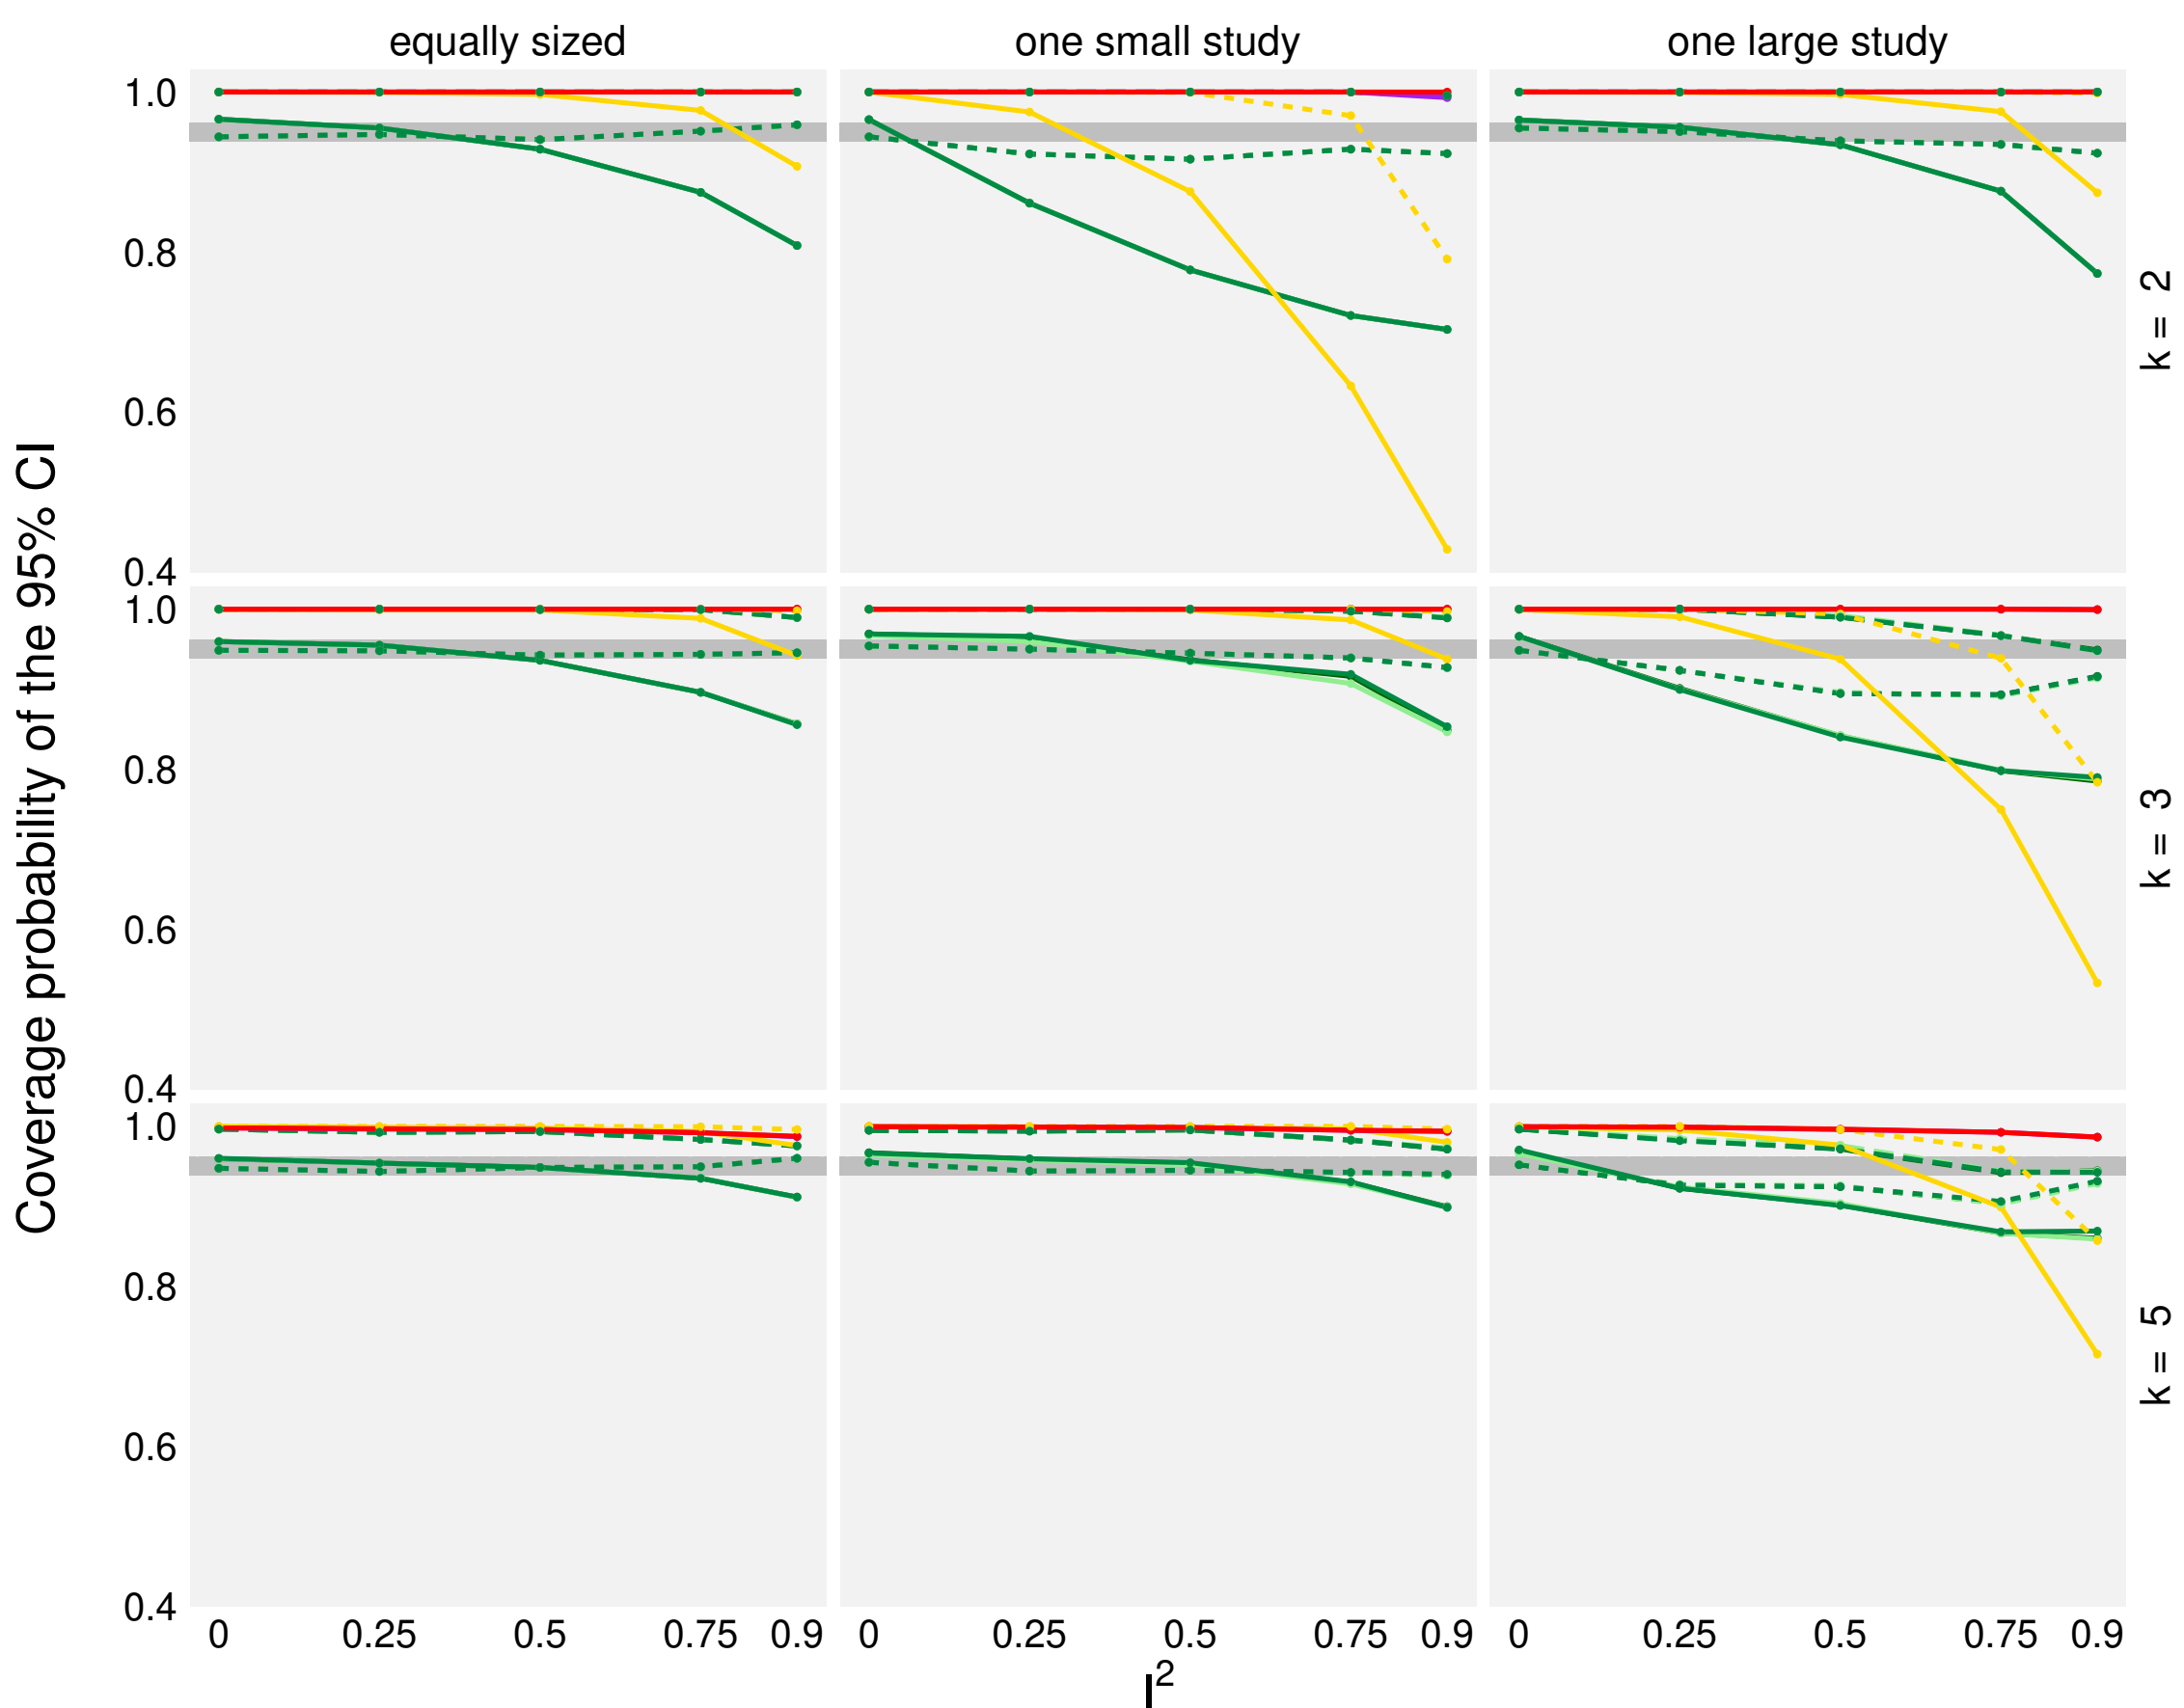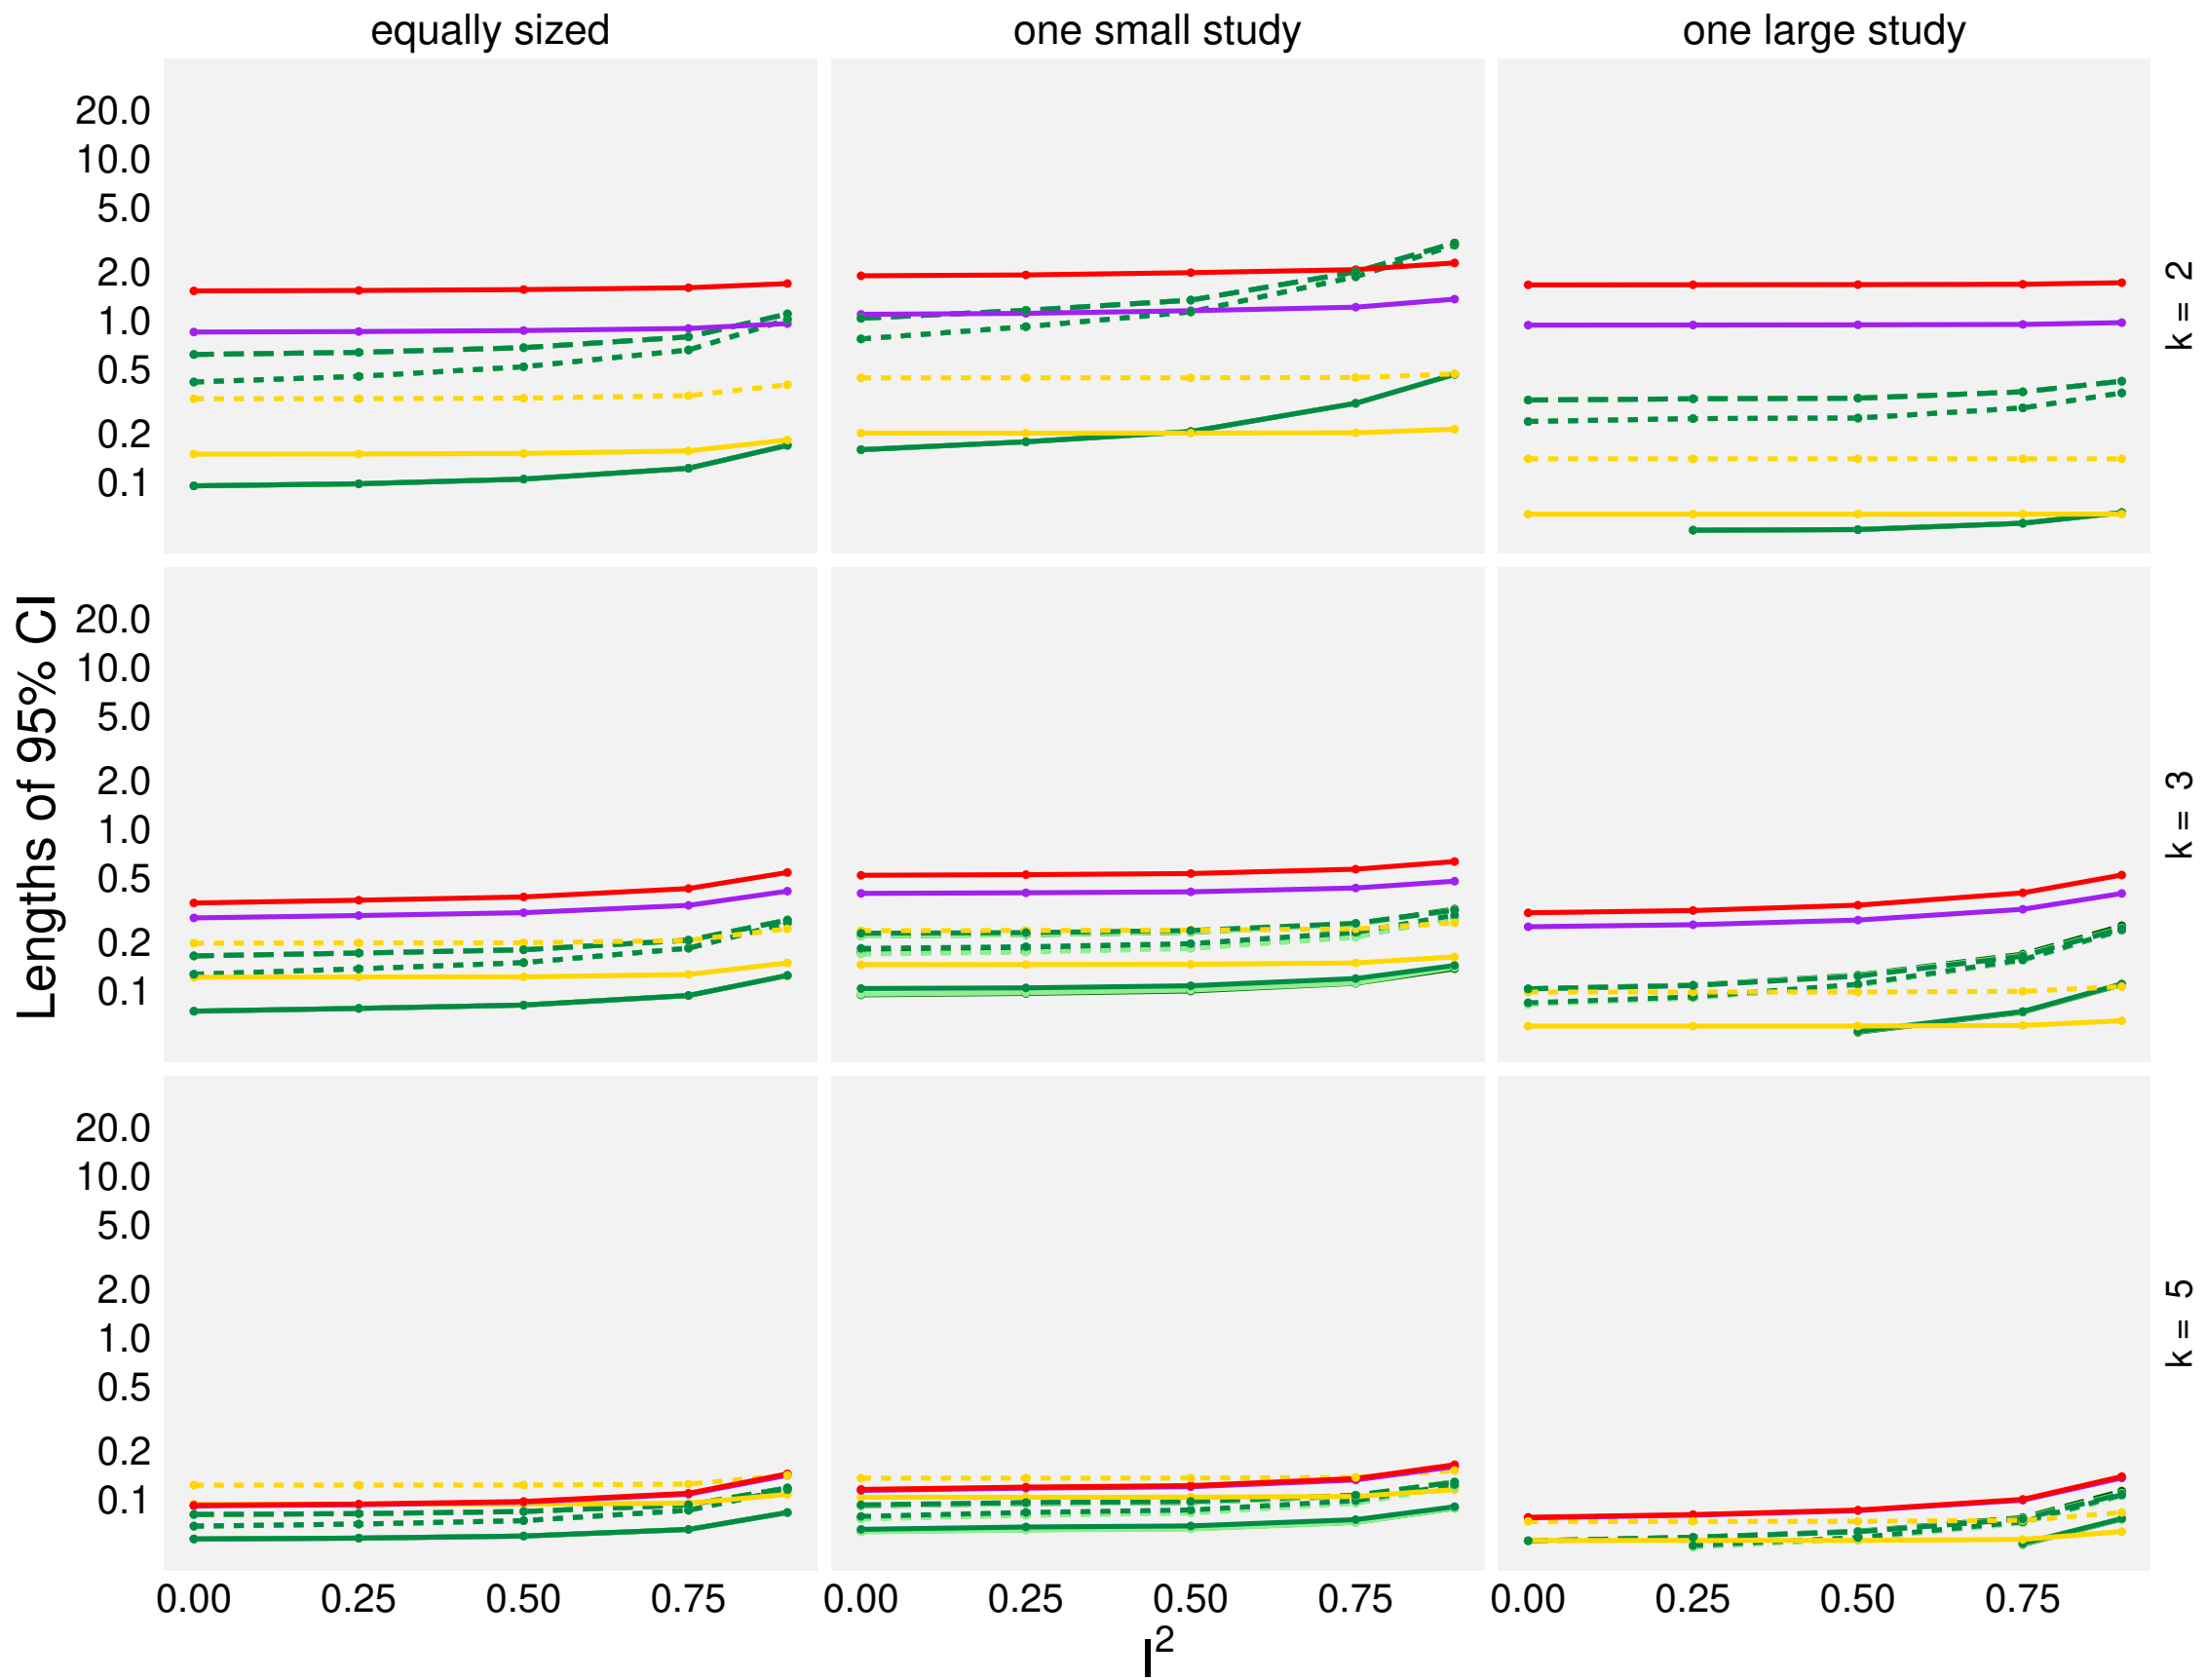

NN - DL    PN - PL    — normal quantiles  
 NN - REML    NN - Bayes HN(0.5)    -- HKSJ or Student's t  
 NN - EB    NN - Bayes HN(1)    -- mHKSJ

RR  
( $n_i=250, \pi_0=0.9$ )

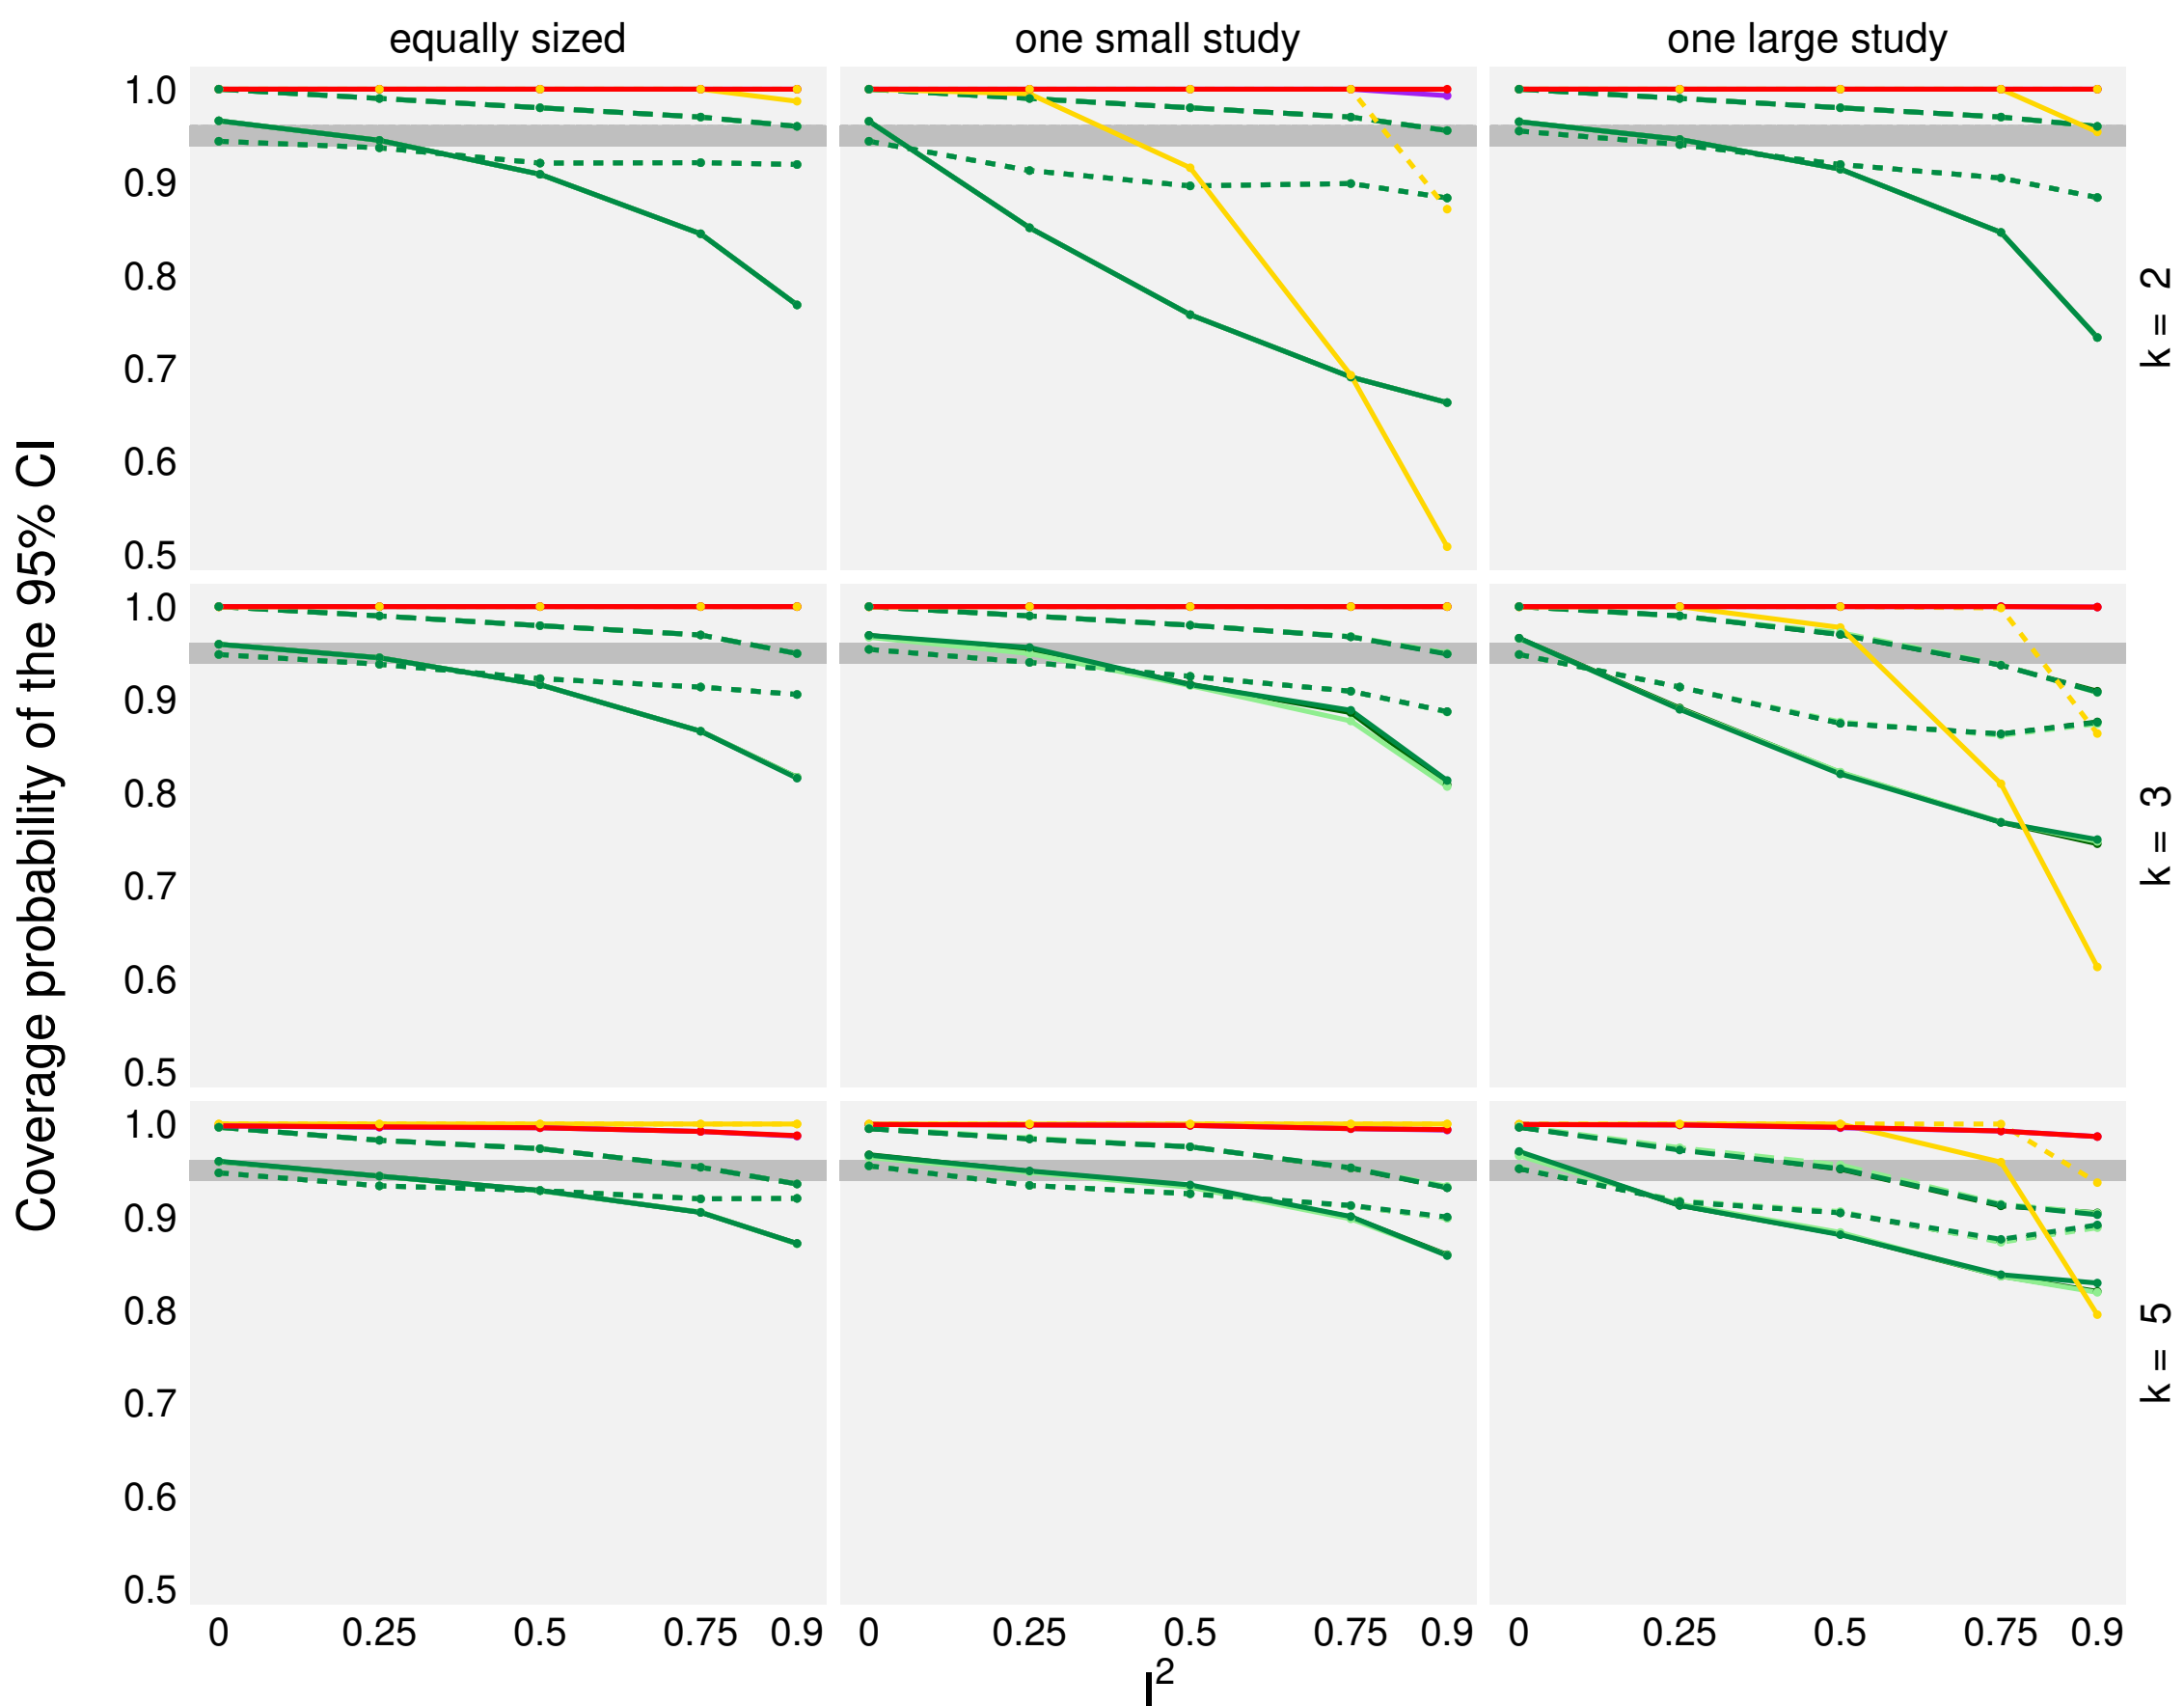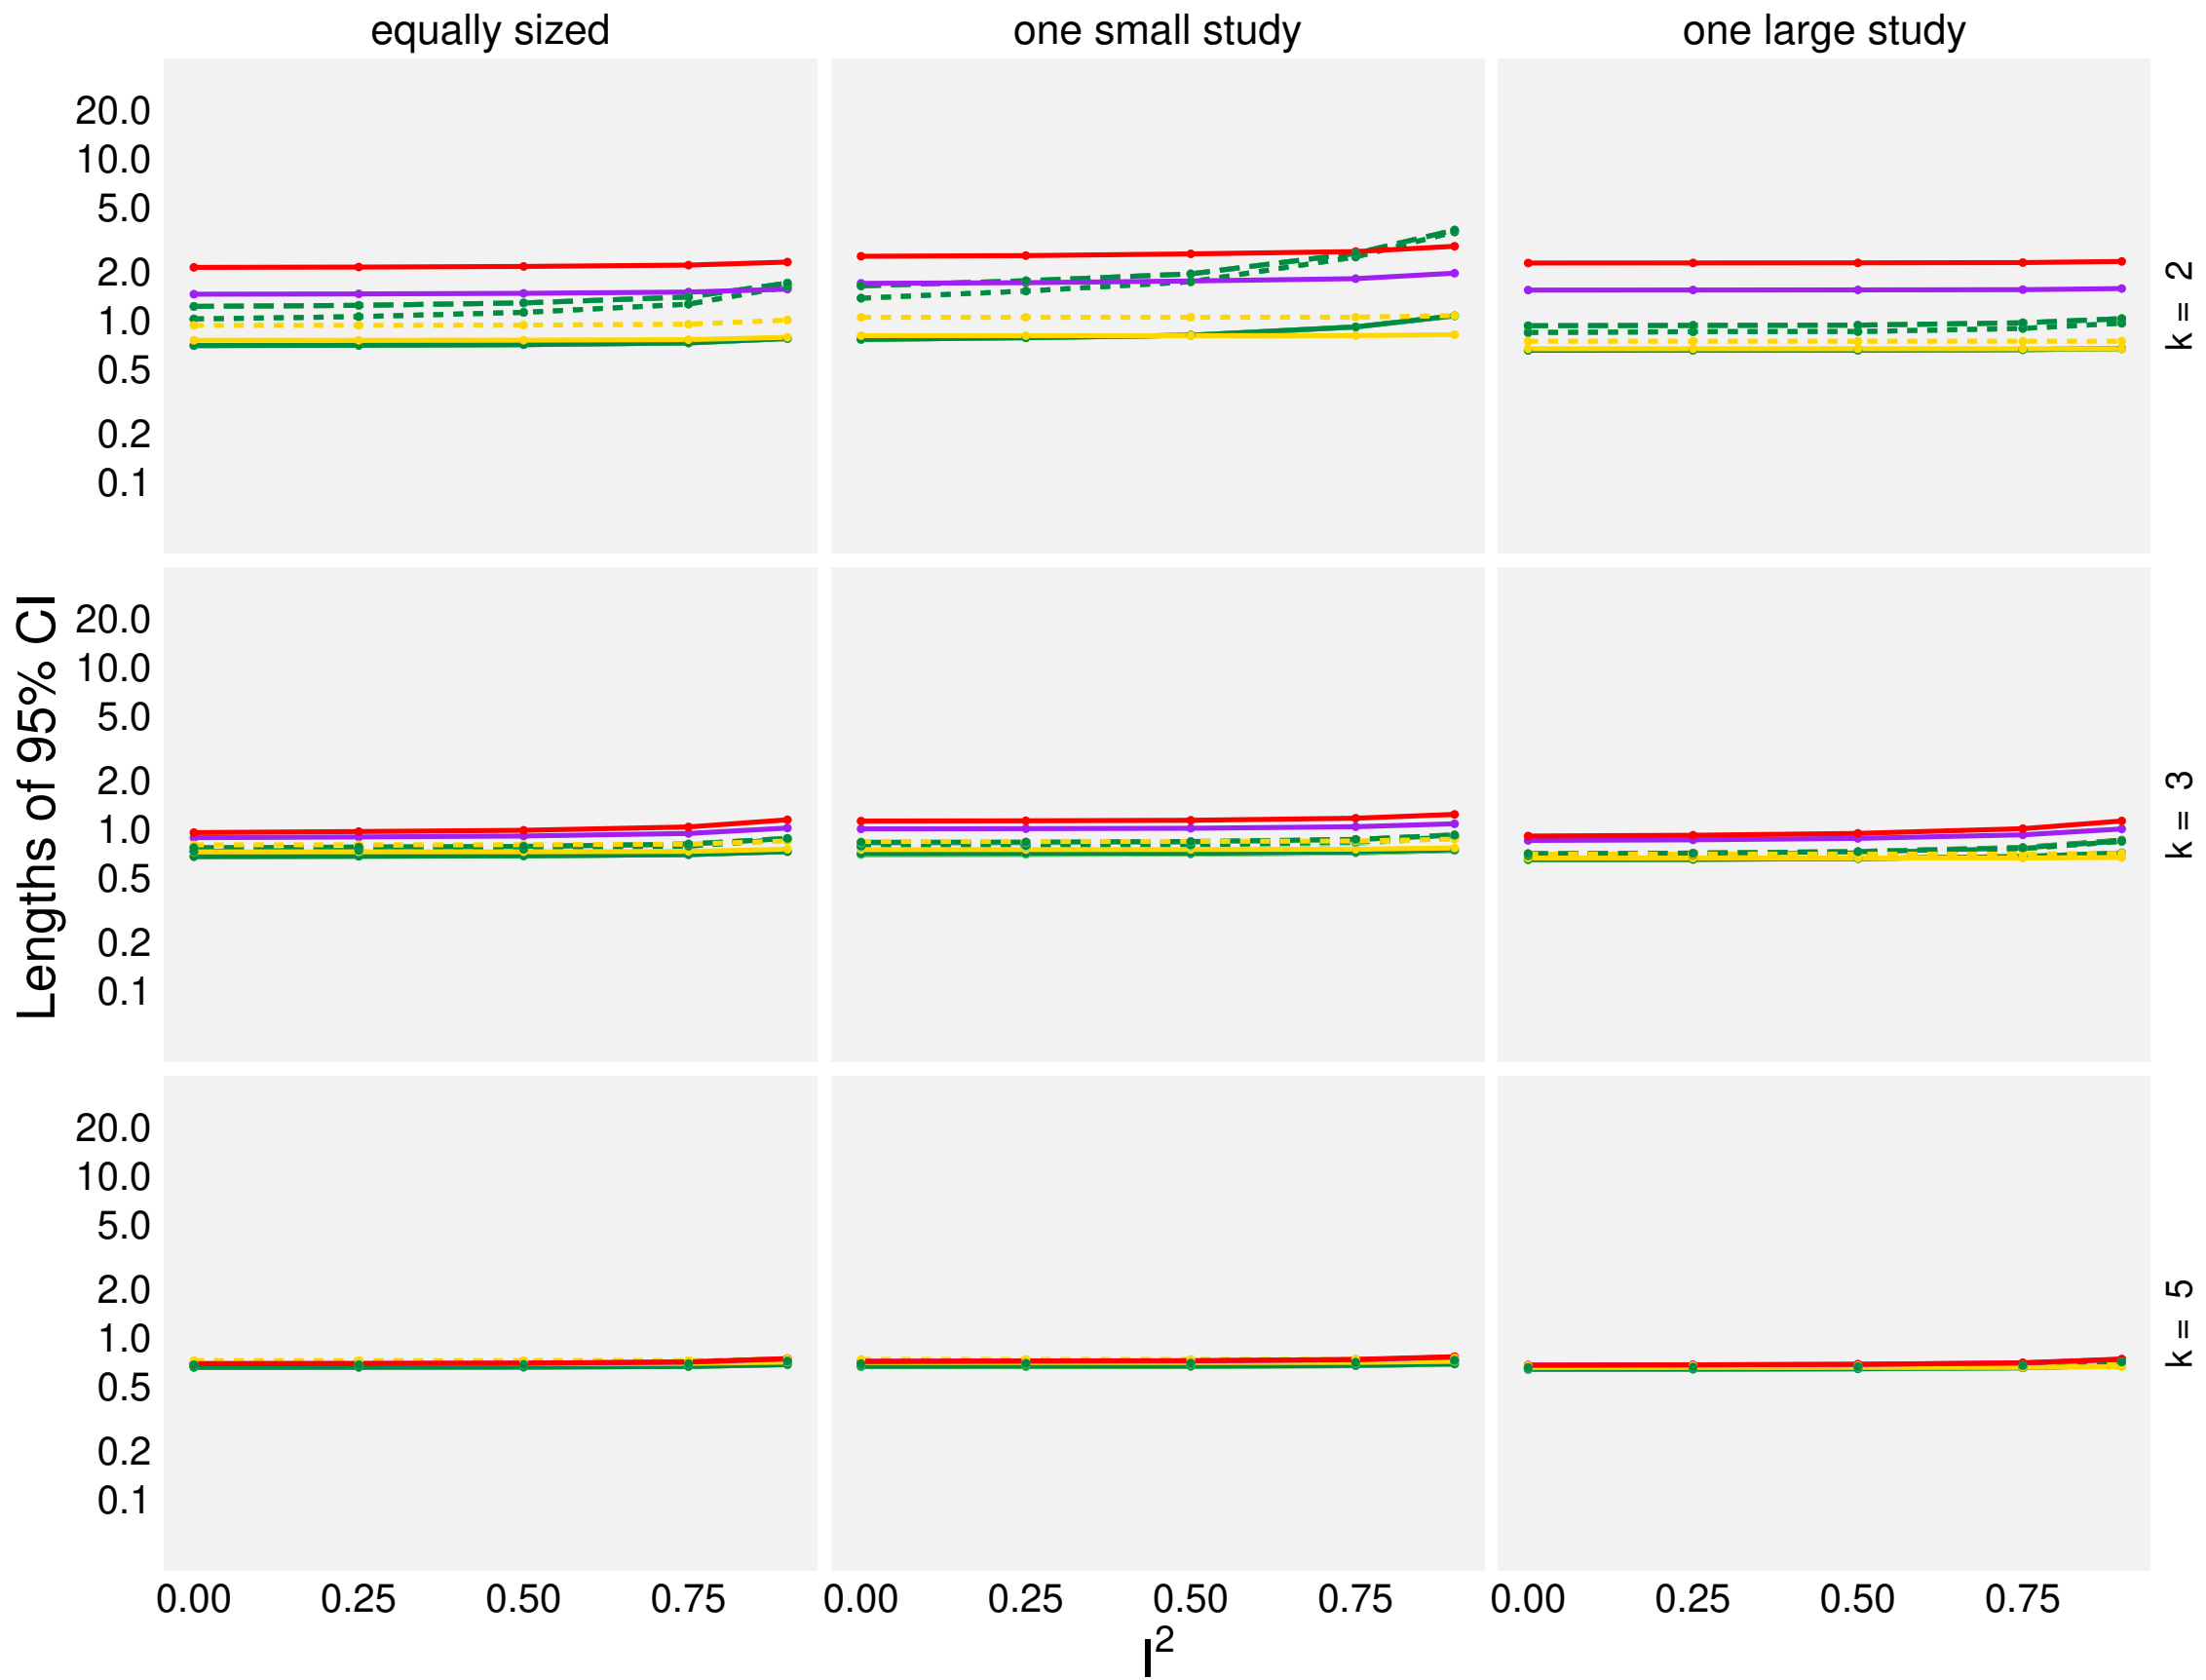

NN - DL  
 NN - REML  
 NN - EB  
 PN - PL  
 NN - Bayes HN(0.5)  
 NN - Bayes HN(1)  
 — normal quantiles  
 -- HKSJ or Student's t  
 ··· mHKSJ

RR  
( $n_i=500, \pi_0=0.1$ )

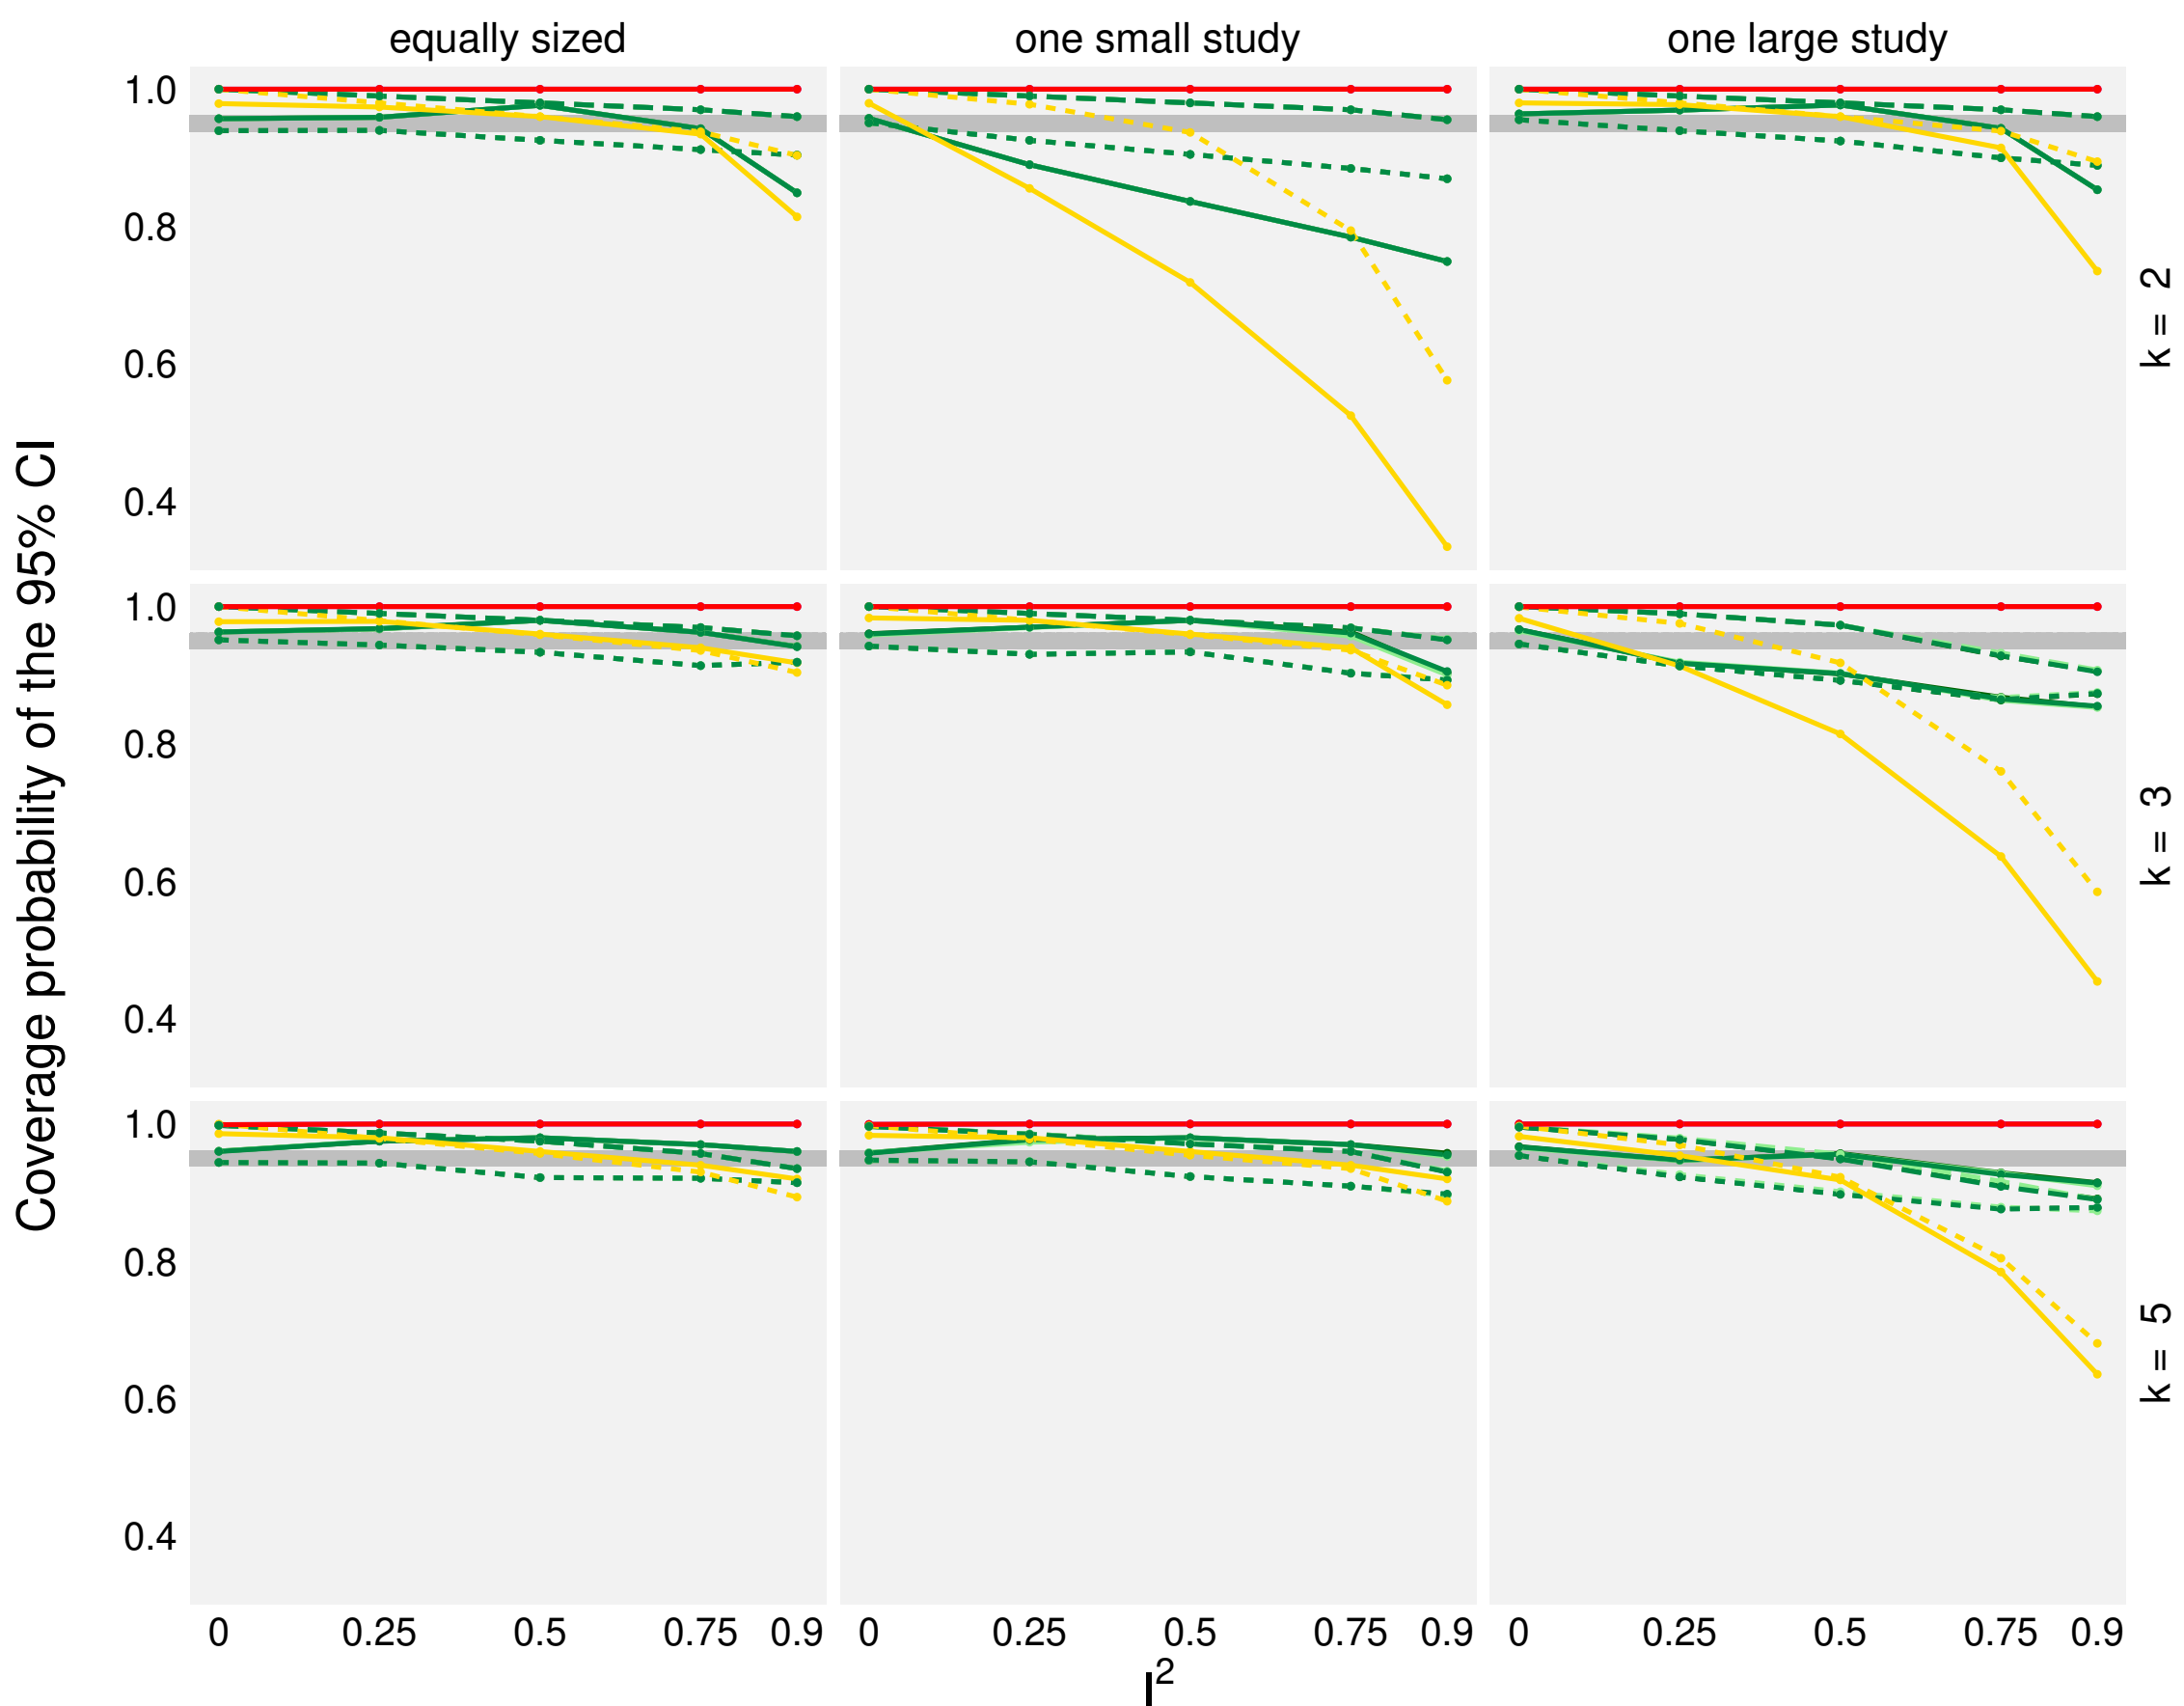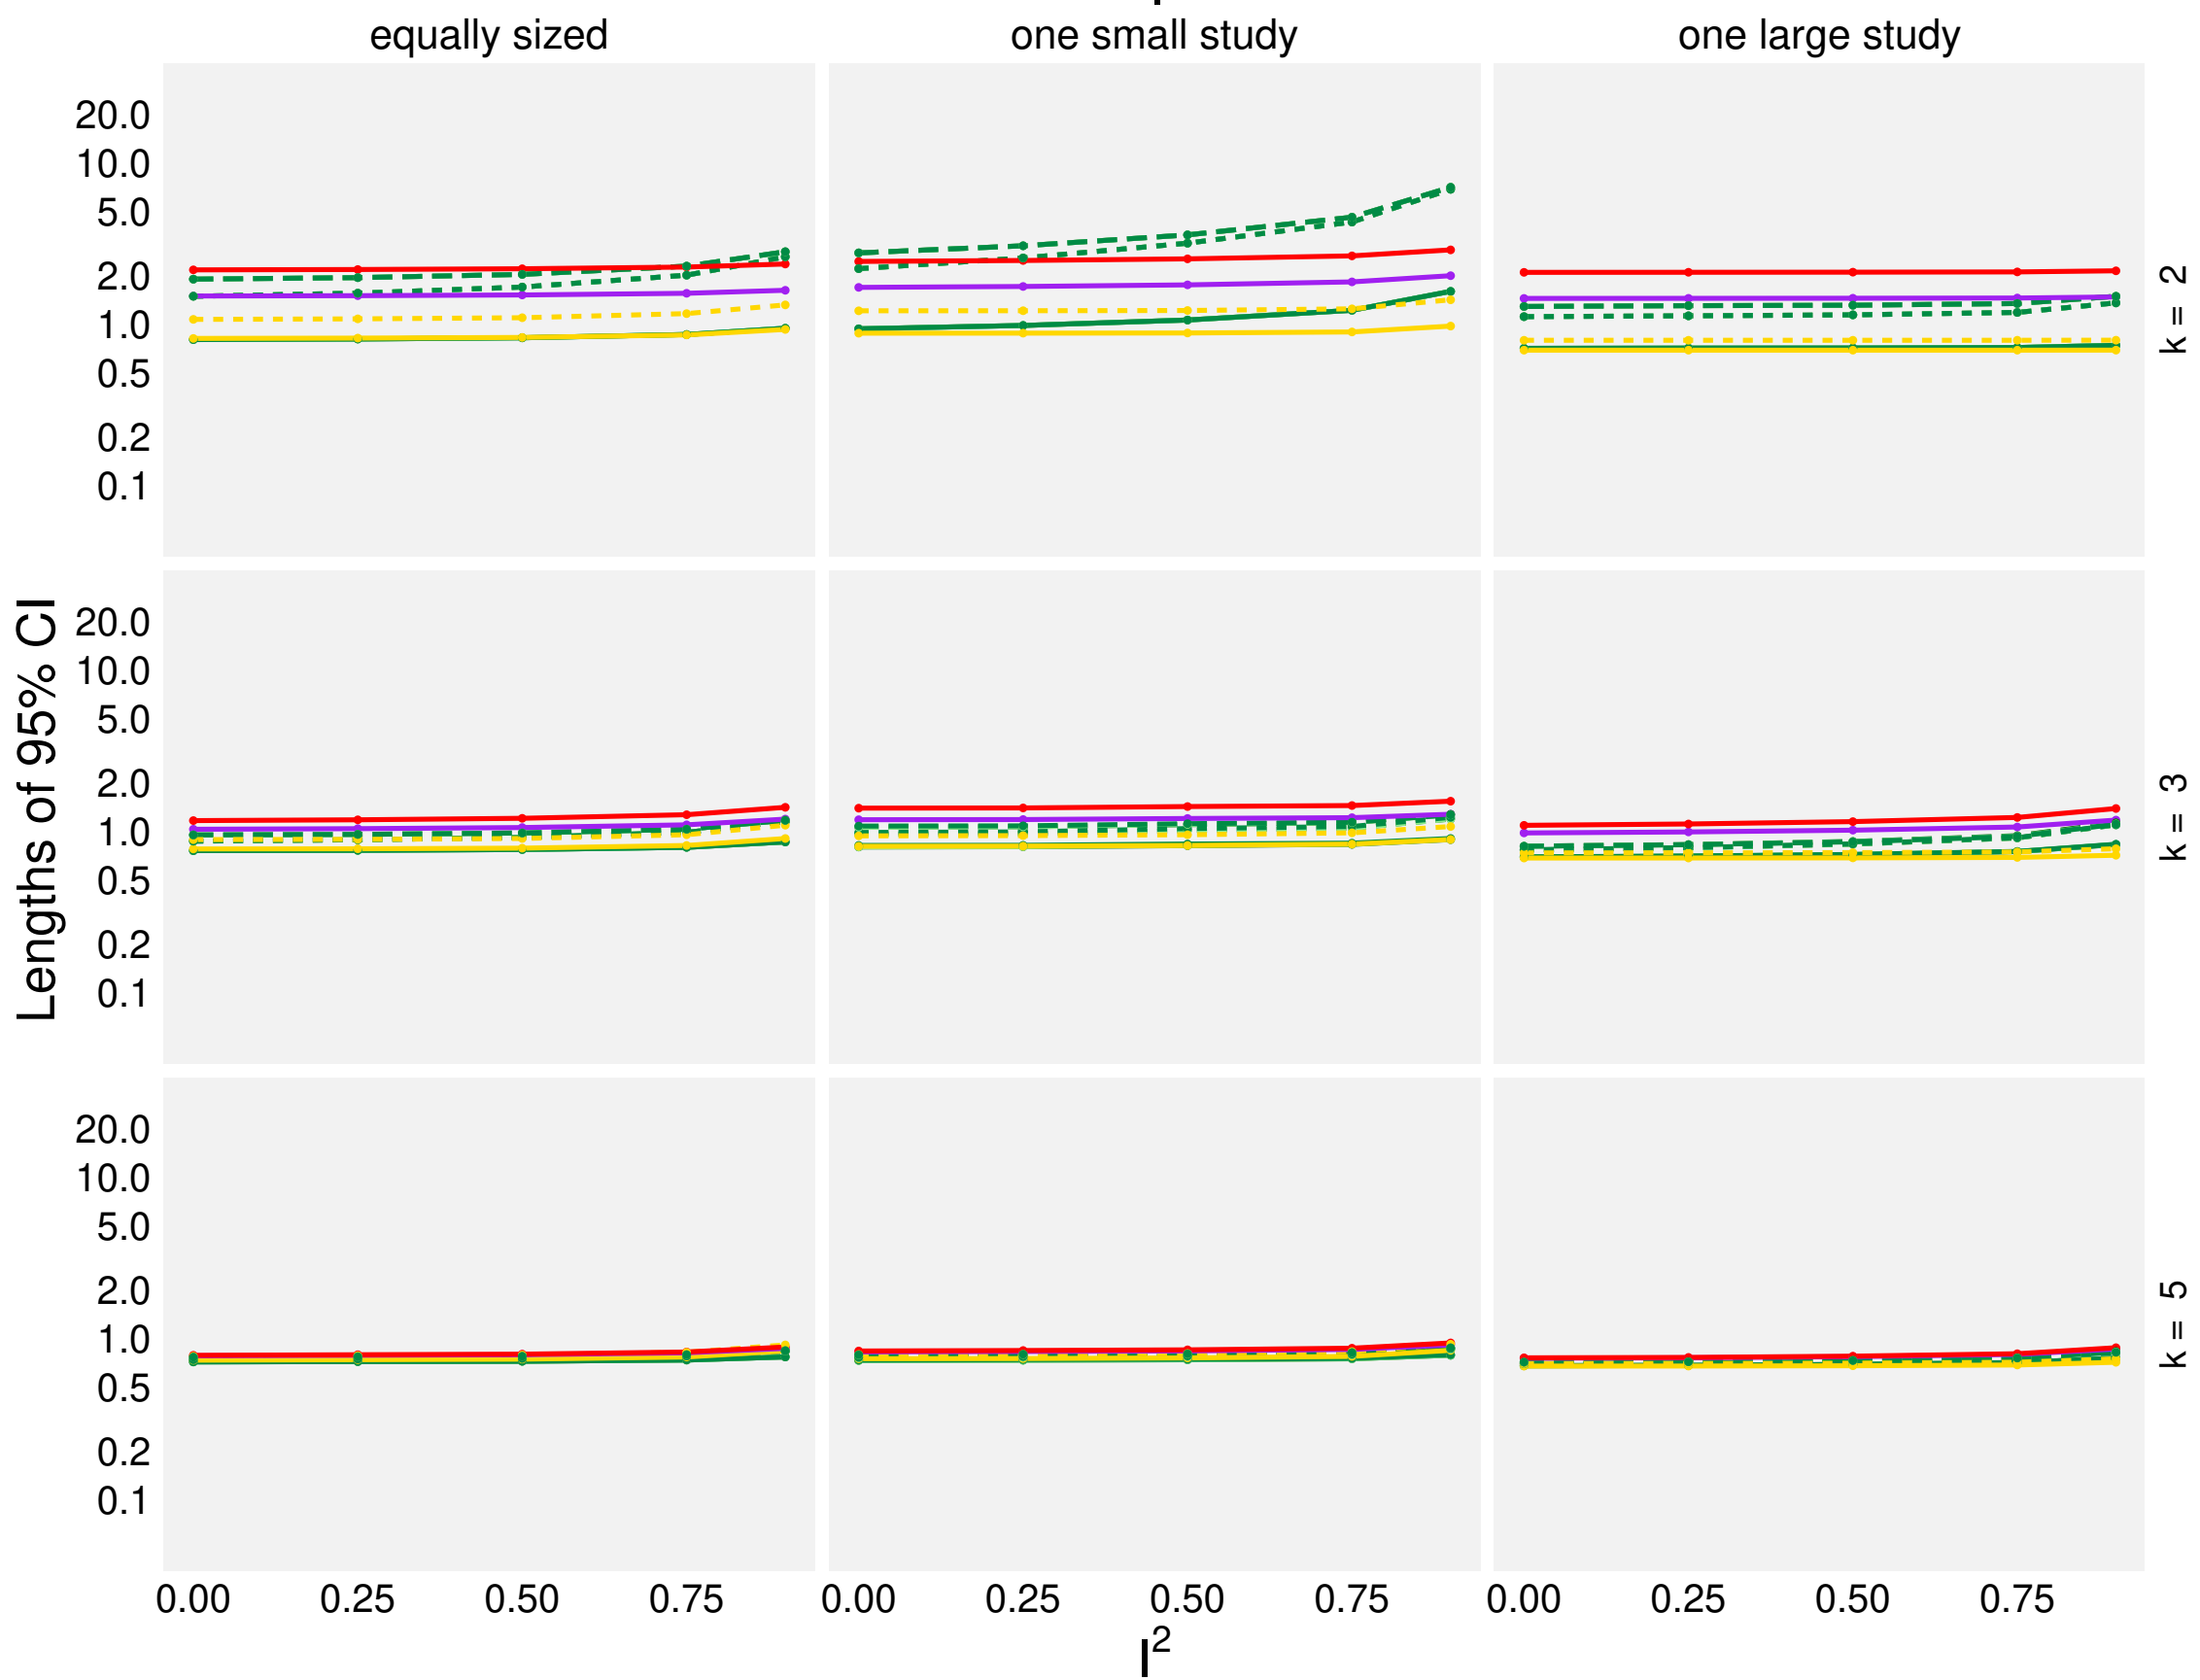

NN – DL  
 NN – REML  
 NN – EB  
 PN – PL  
 NN – Bayes HN(0.5)  
 NN – Bayes HN(1)  
 — normal quantiles  
 - - HKSJ or Student's t  
 . . mHKSJ

RR  
( $n_i=500, \pi_0=0.3$ )

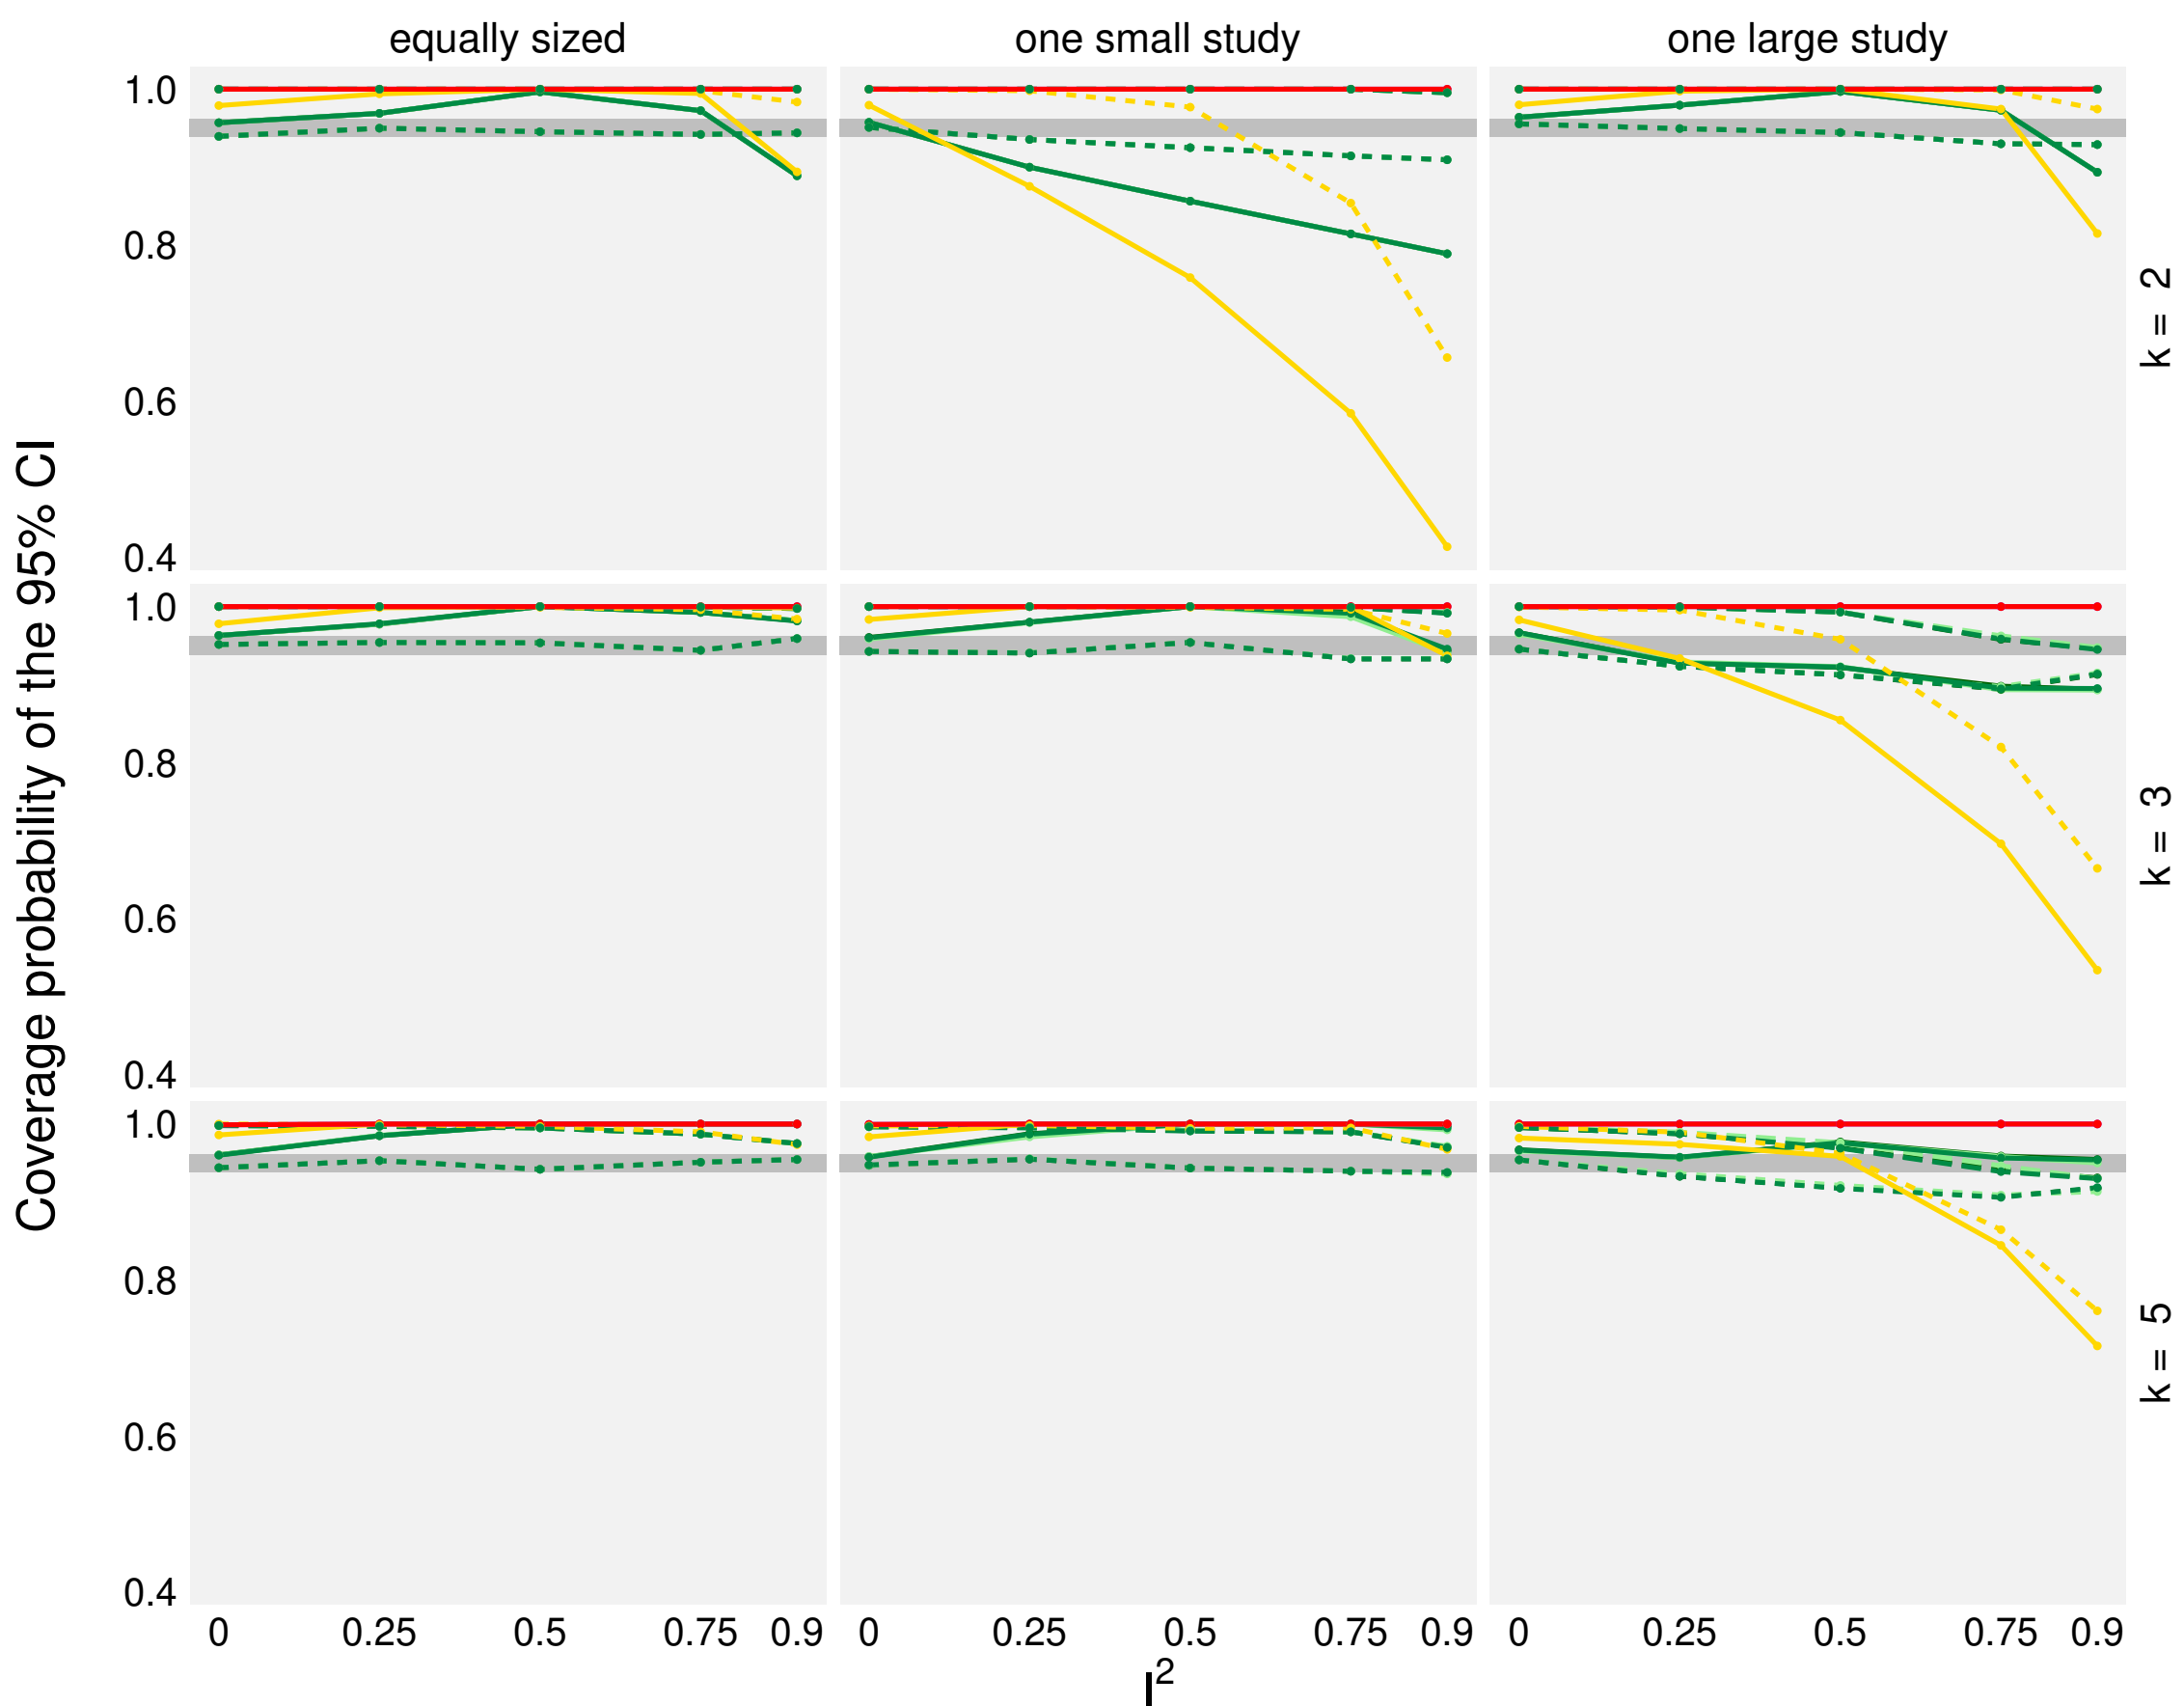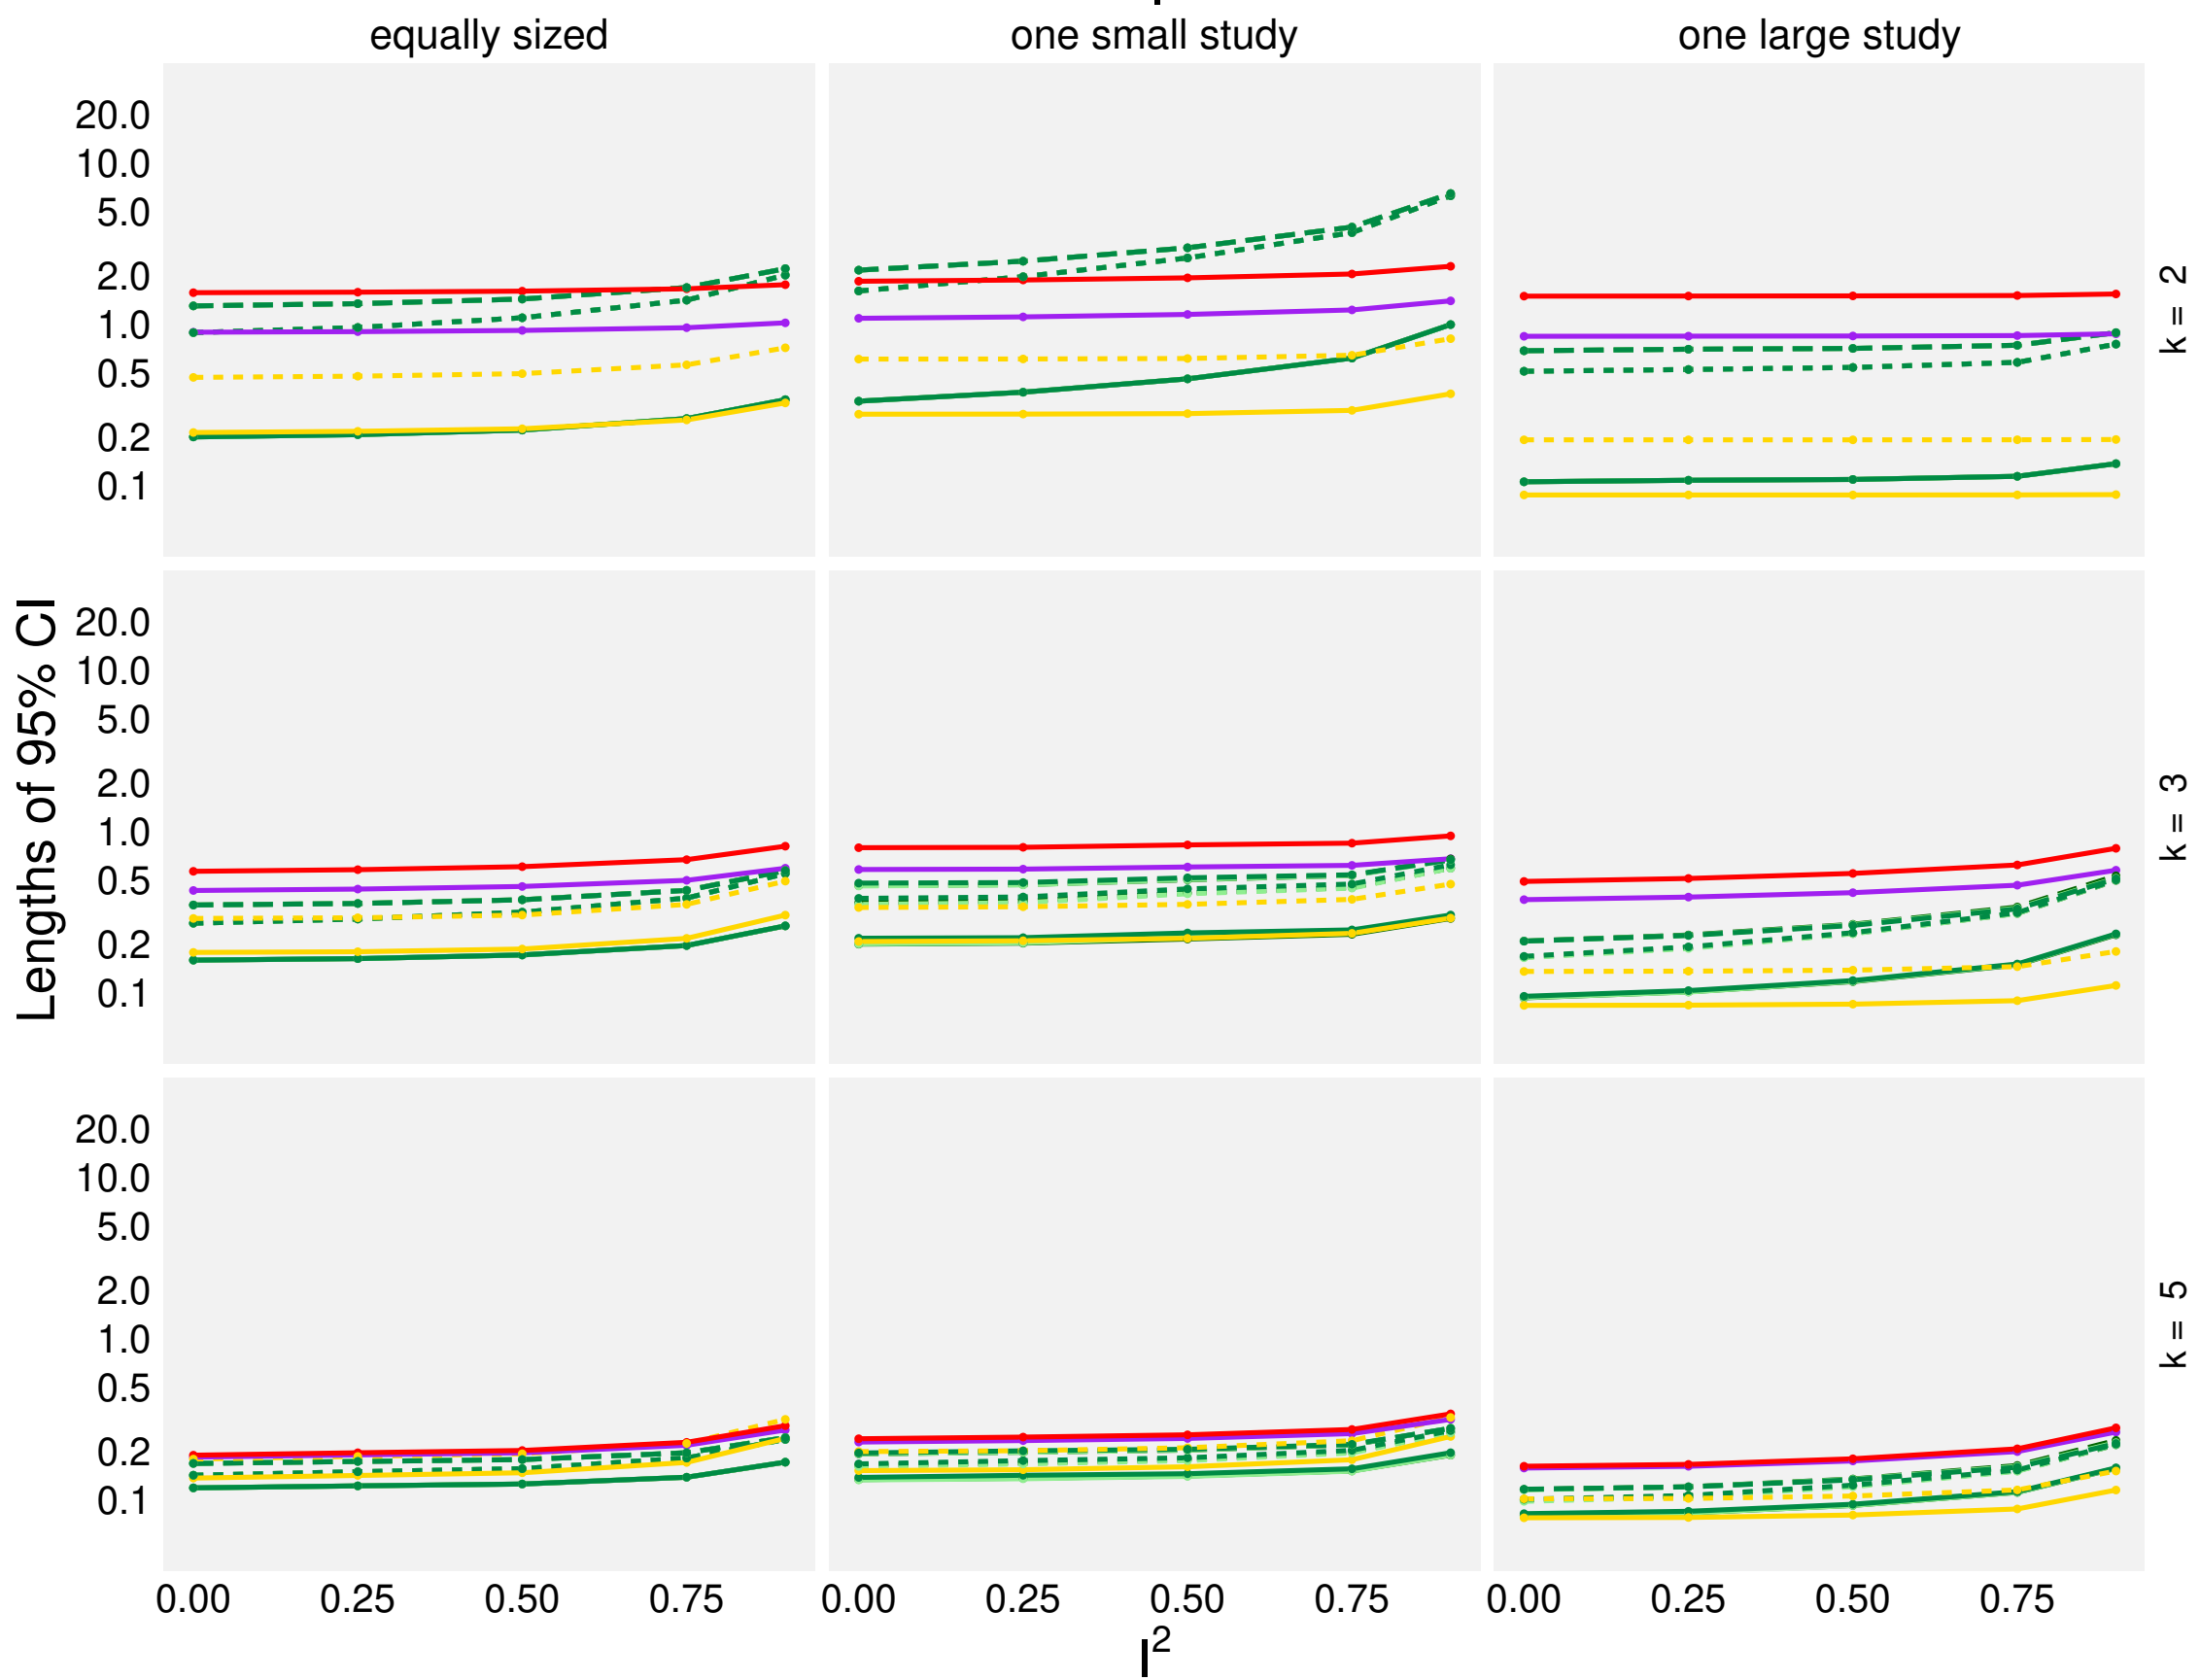

NN - DL  
 NN - REML  
 NN - EB  
 PN - PL  
 NN - Bayes HN(0.5)  
 NN - Bayes HN(1)  
 — normal quantiles  
 - - HKSJ or Student's t  
 - - mHKSJ

RR  
( $n_i=500, \pi_0=0.5$ )

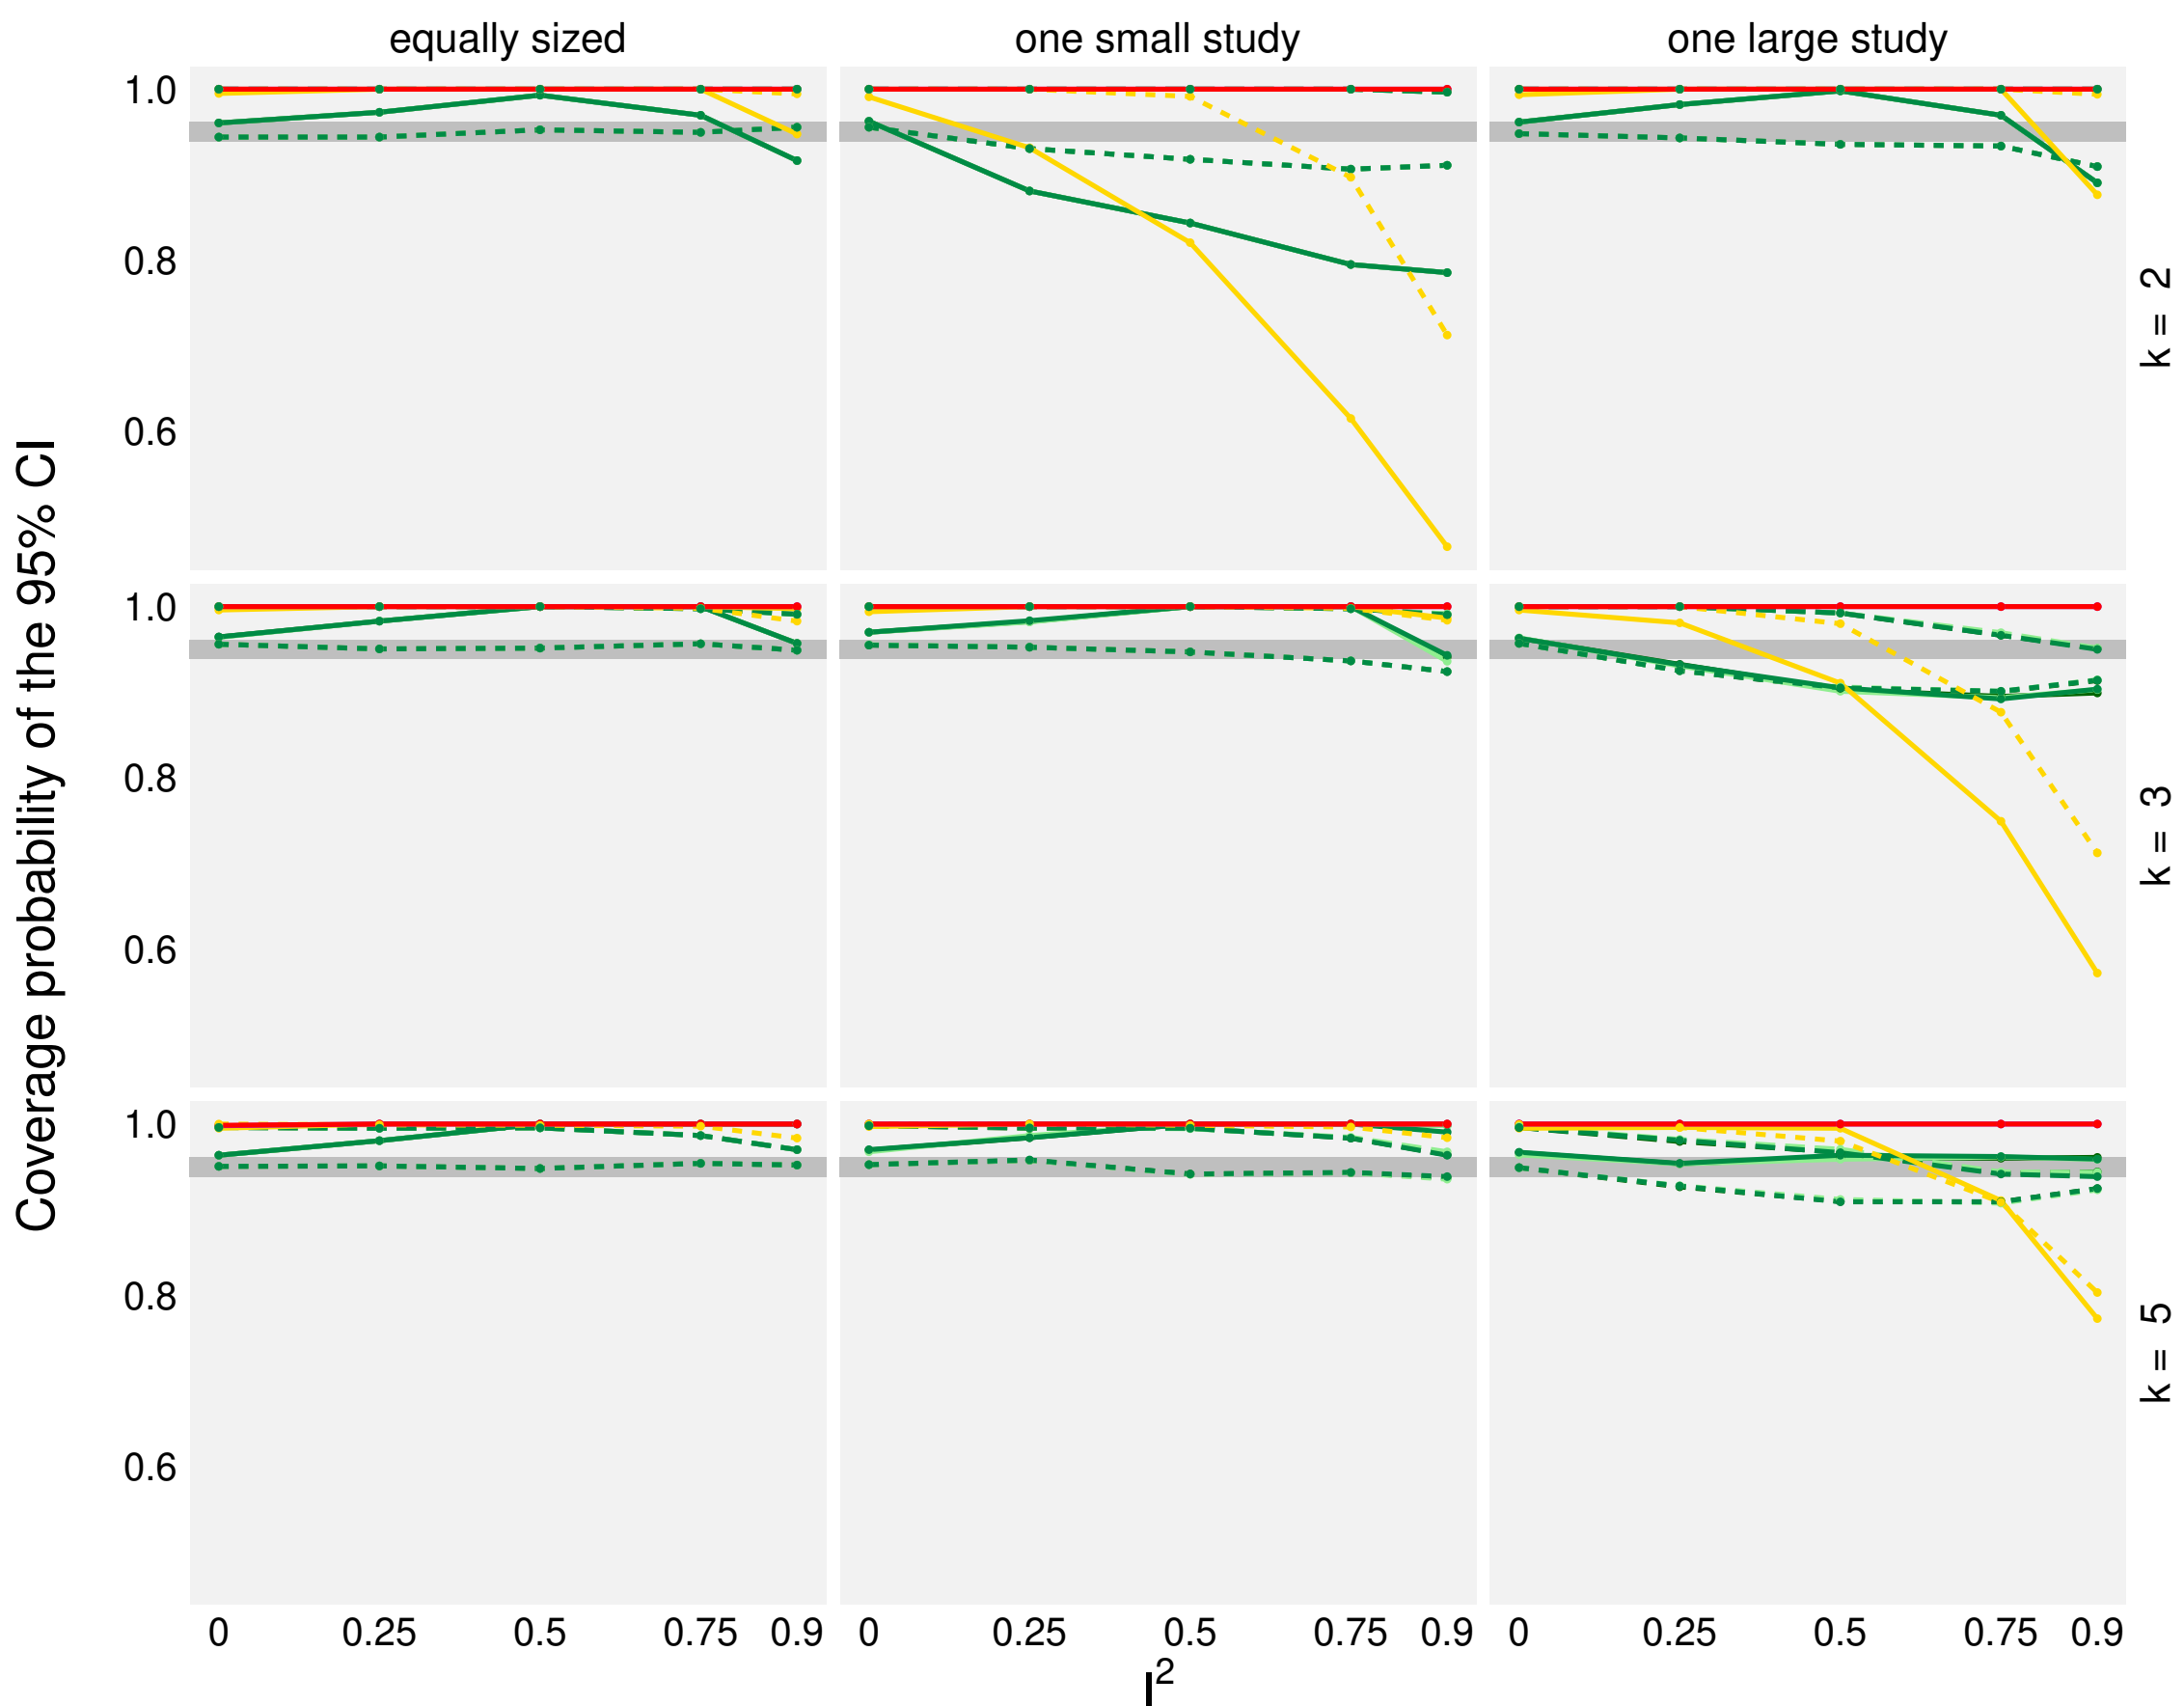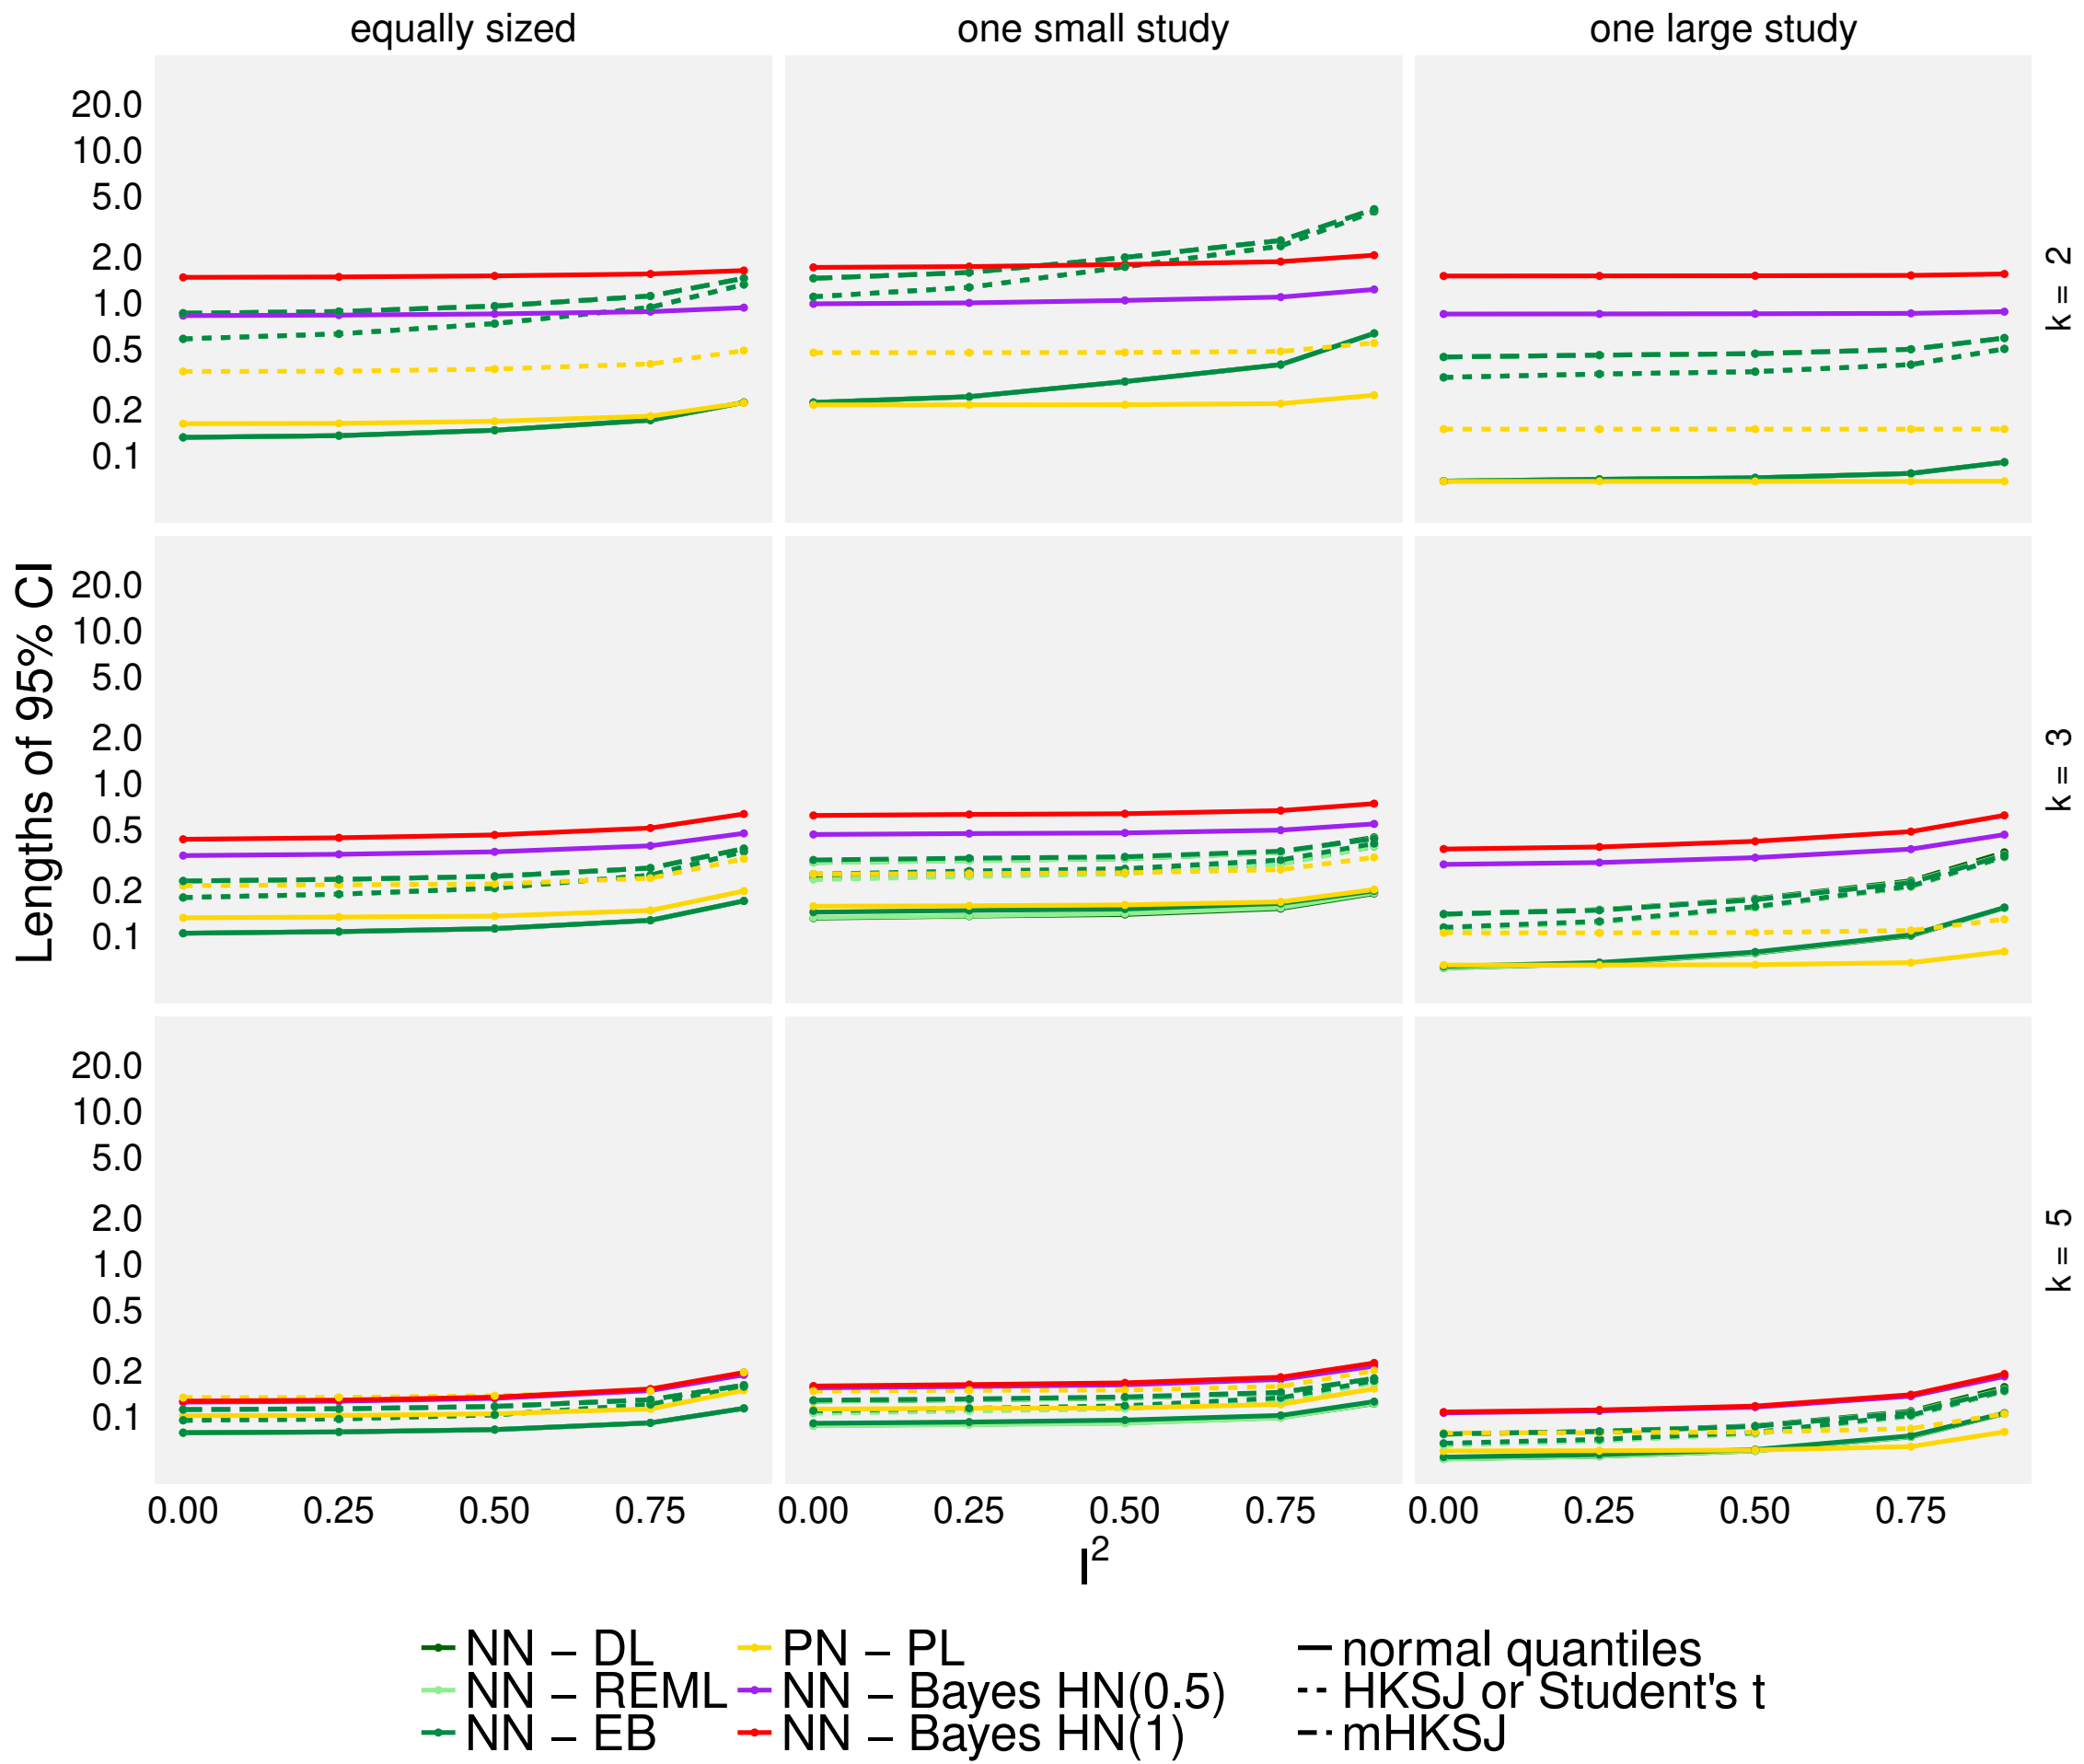

NN - DL  
 NN - REML  
 NN - EB  
 PN - PL  
 NN - Bayes HN(0.5)  
 NN - Bayes HN(1)  
 — normal quantiles  
 -- HKSJ or Student's t  
 - - mHKSJ

RR  
( $n_i=500, \pi_0=0.7$ )

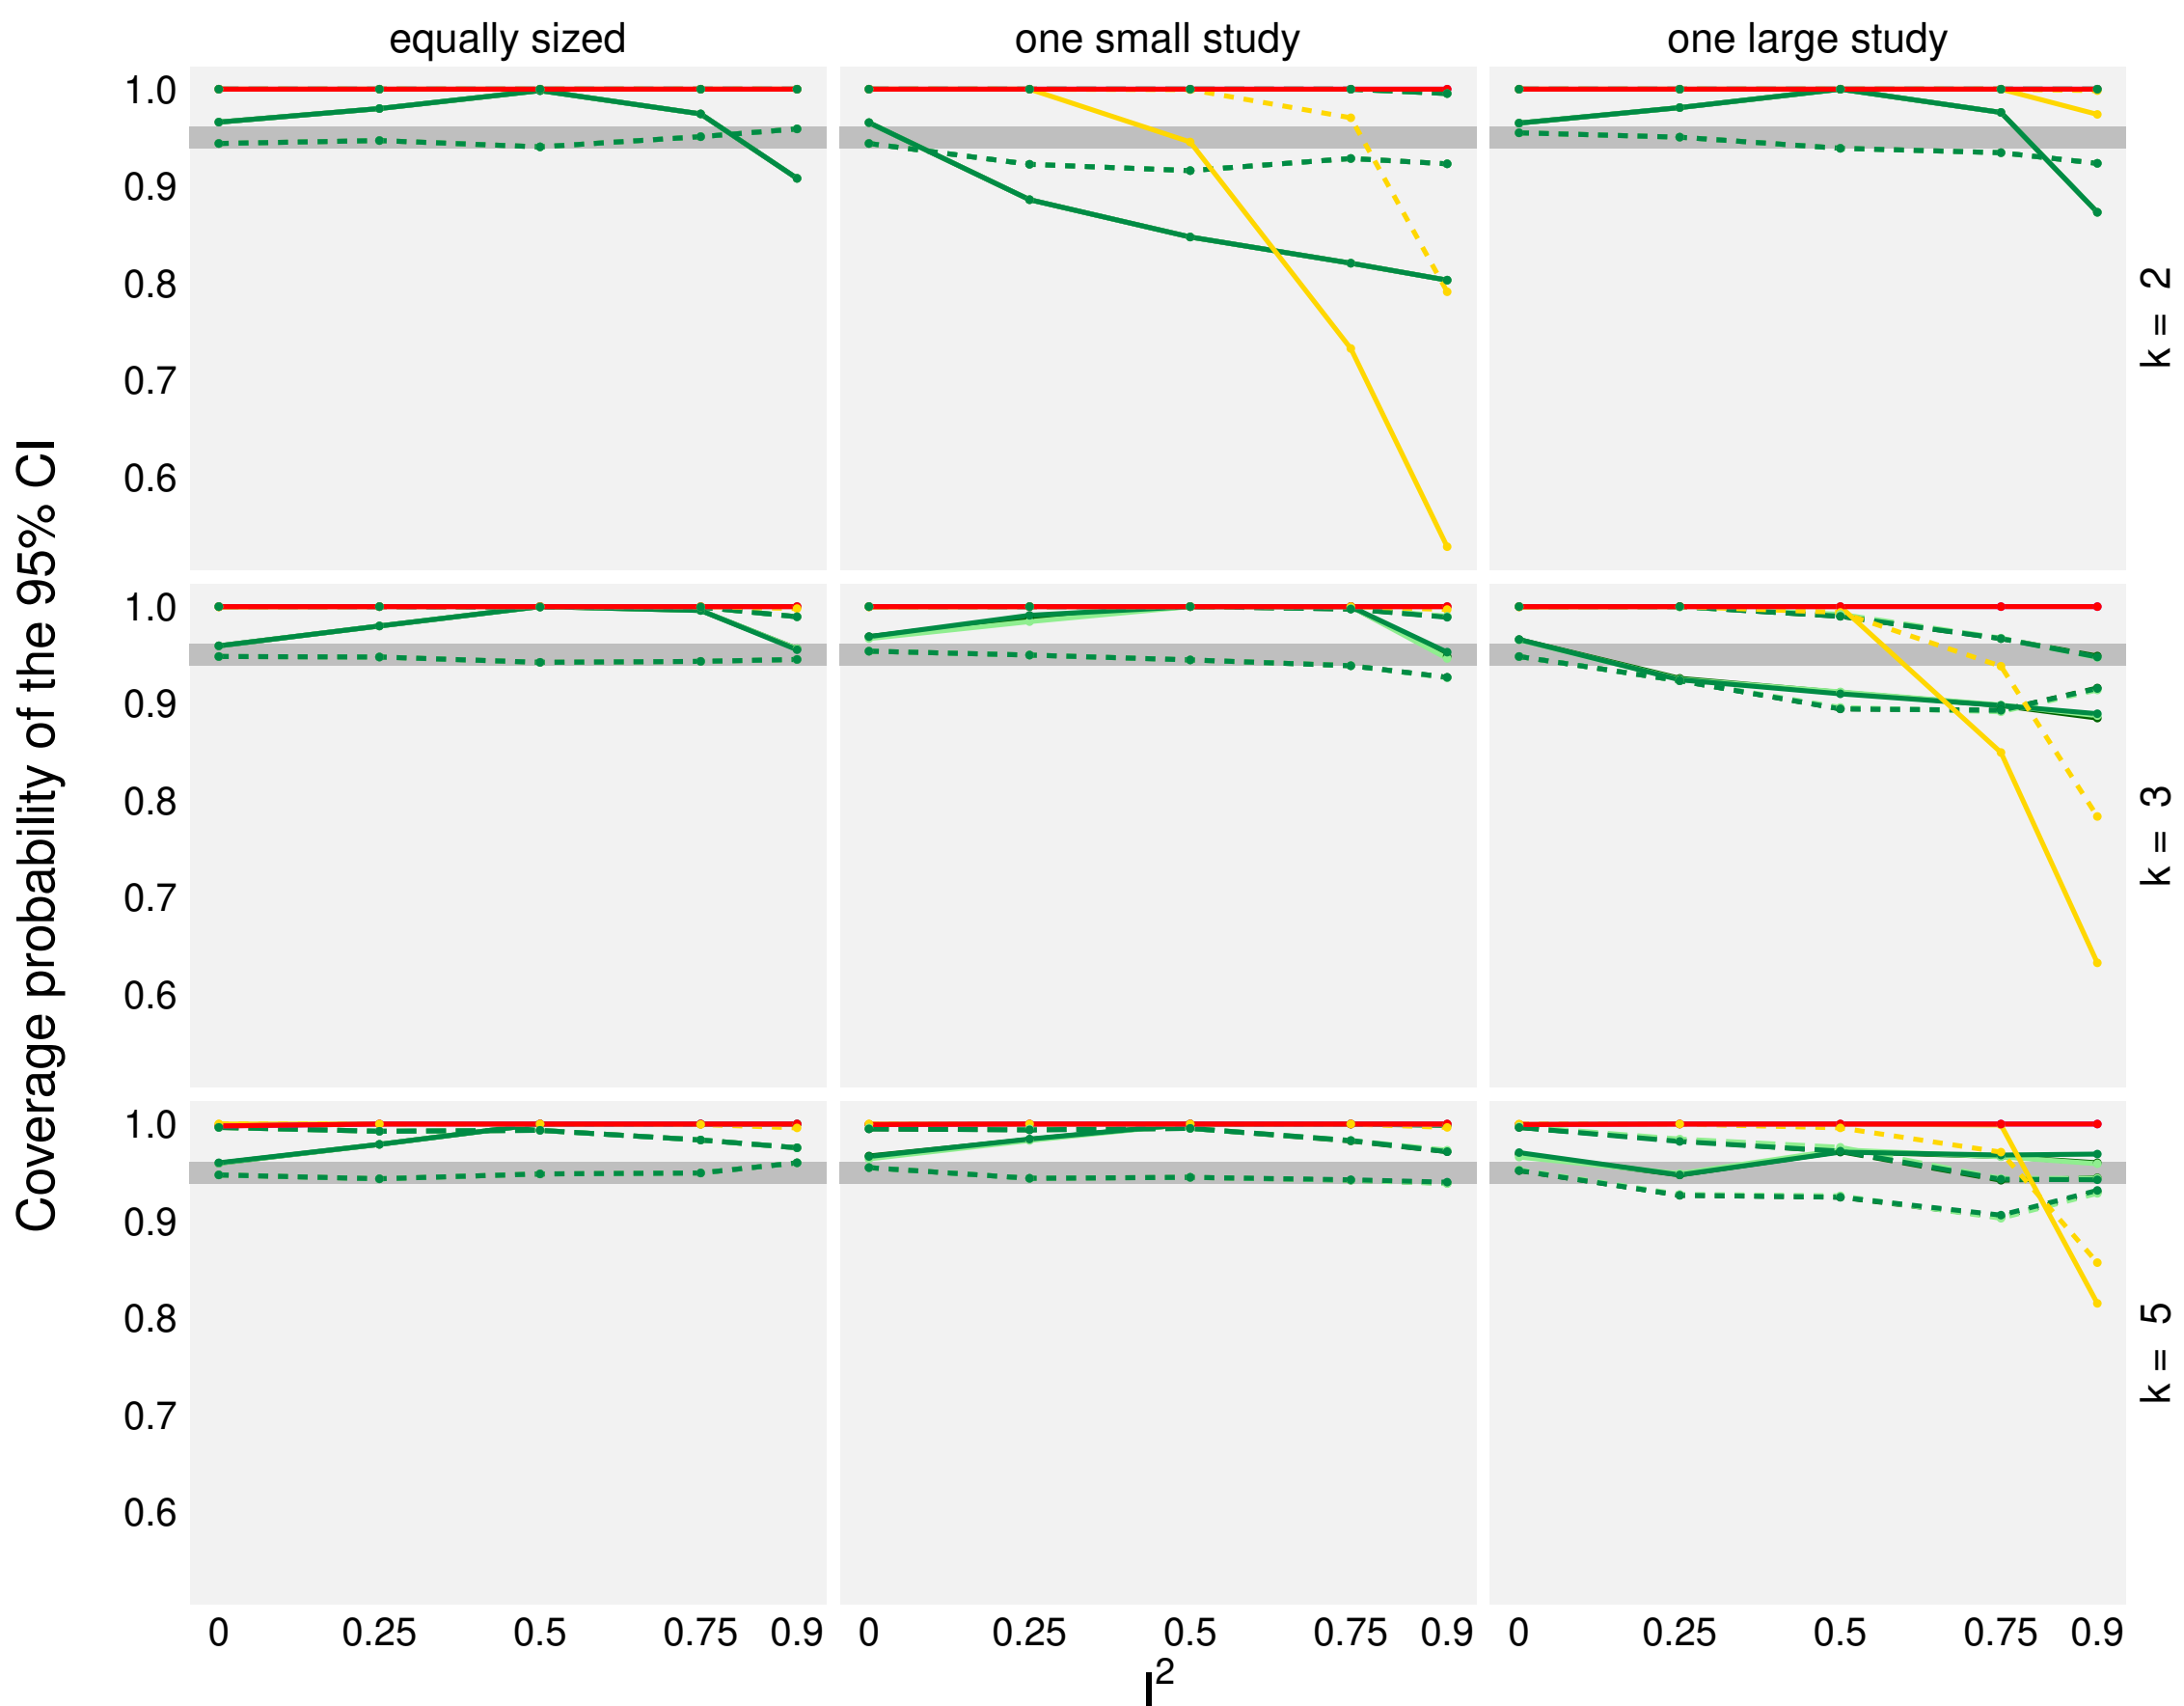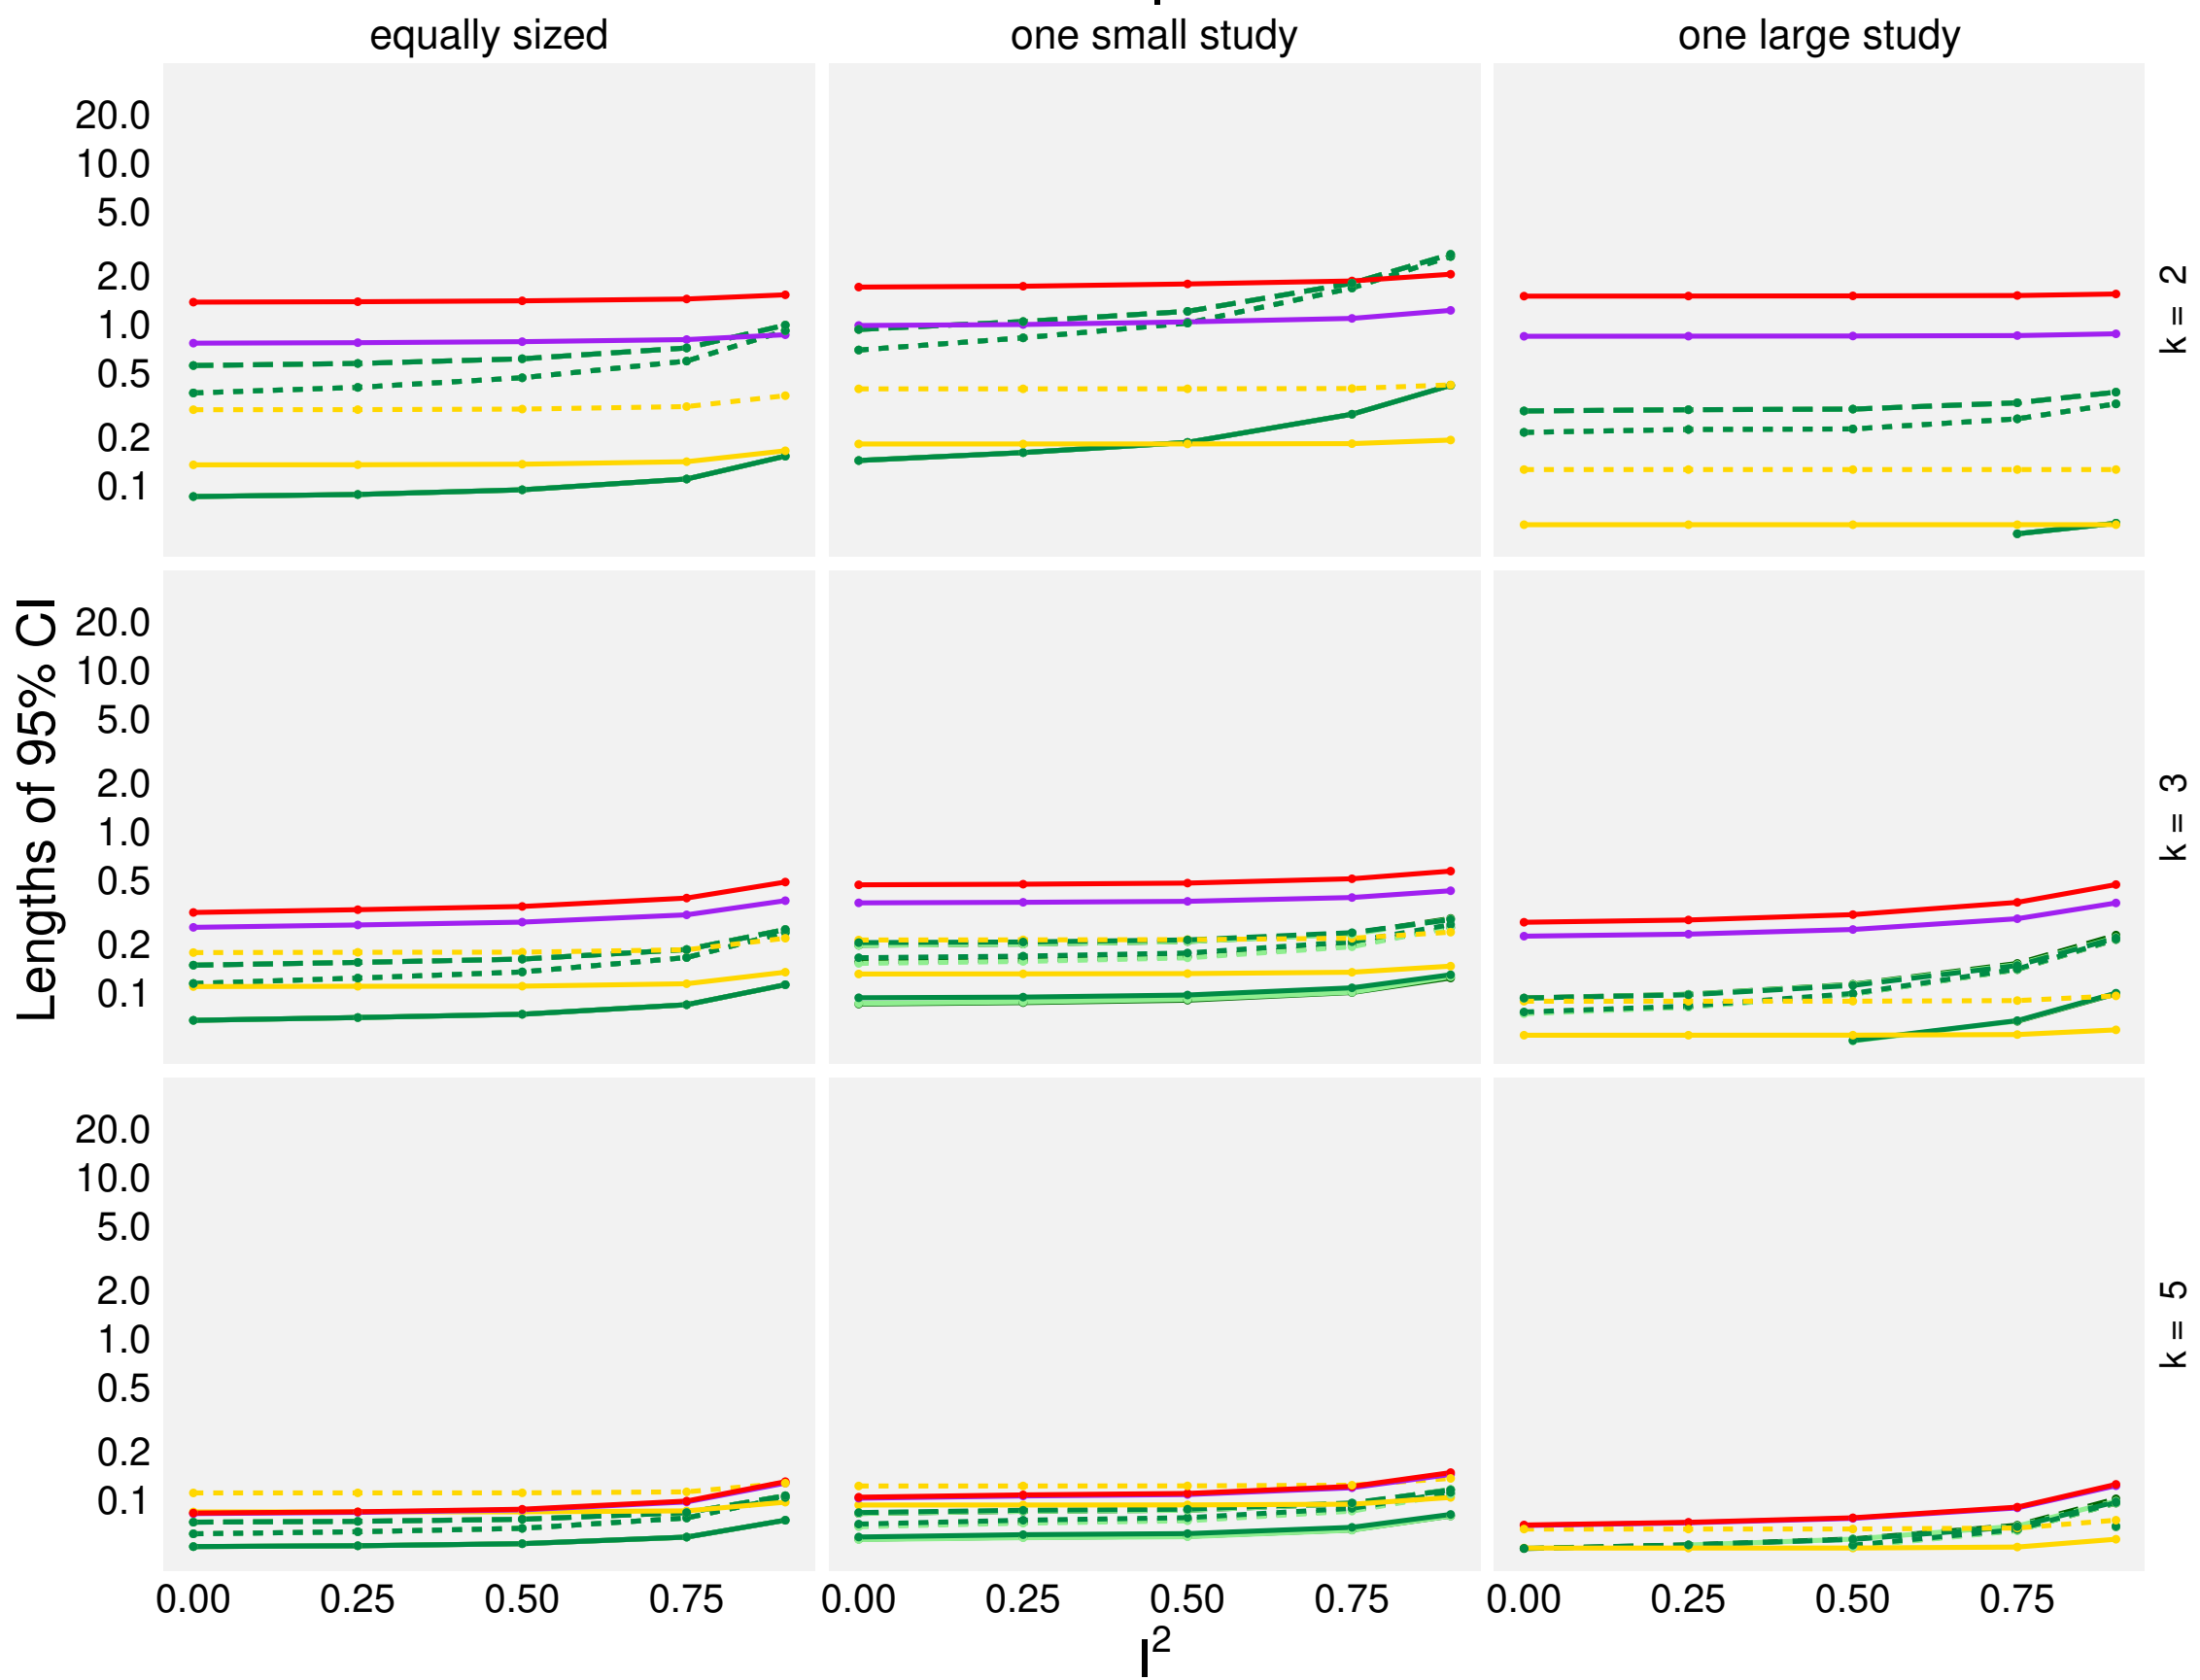

NN - DL  
 NN - REML  
 NN - EB  
 PN - PL  
 NN - Bayes HN(0.5)  
 NN - Bayes HN(1)  
 — normal quantiles  
 - - HKSJ or Student's t  
 - - mHKSJ

RR  
( $n_i=500, \pi_0=0.9$ )

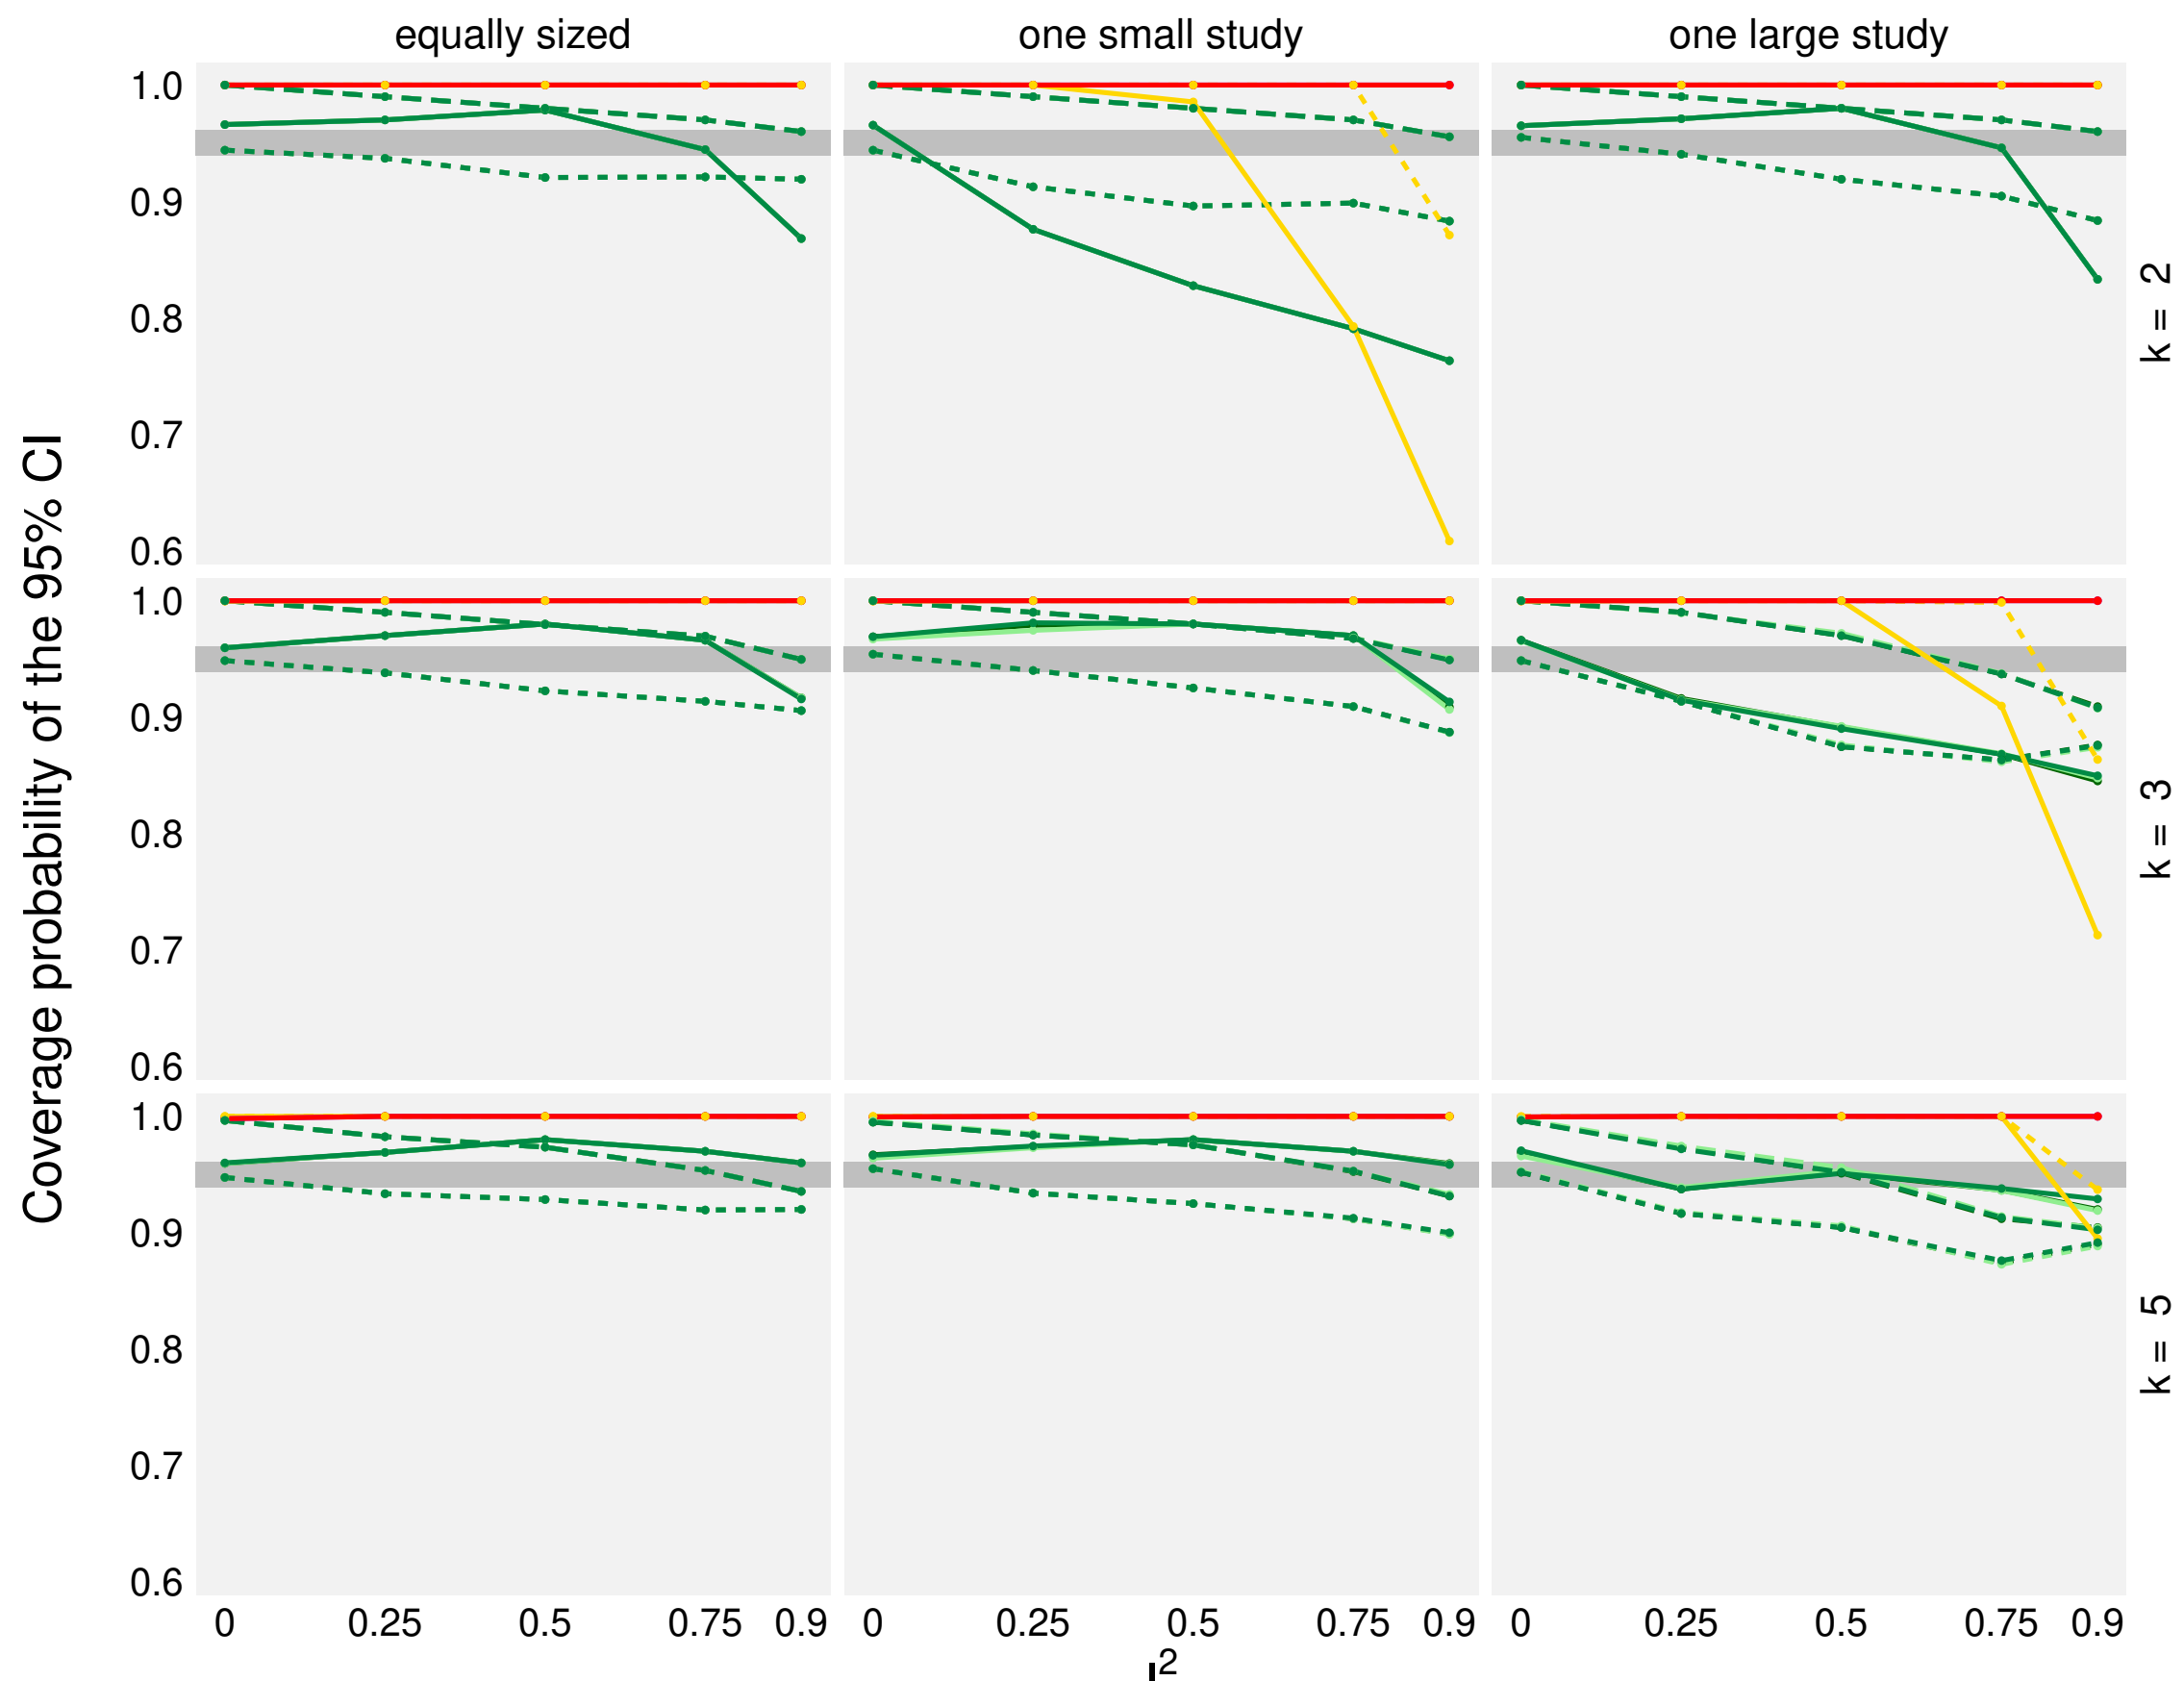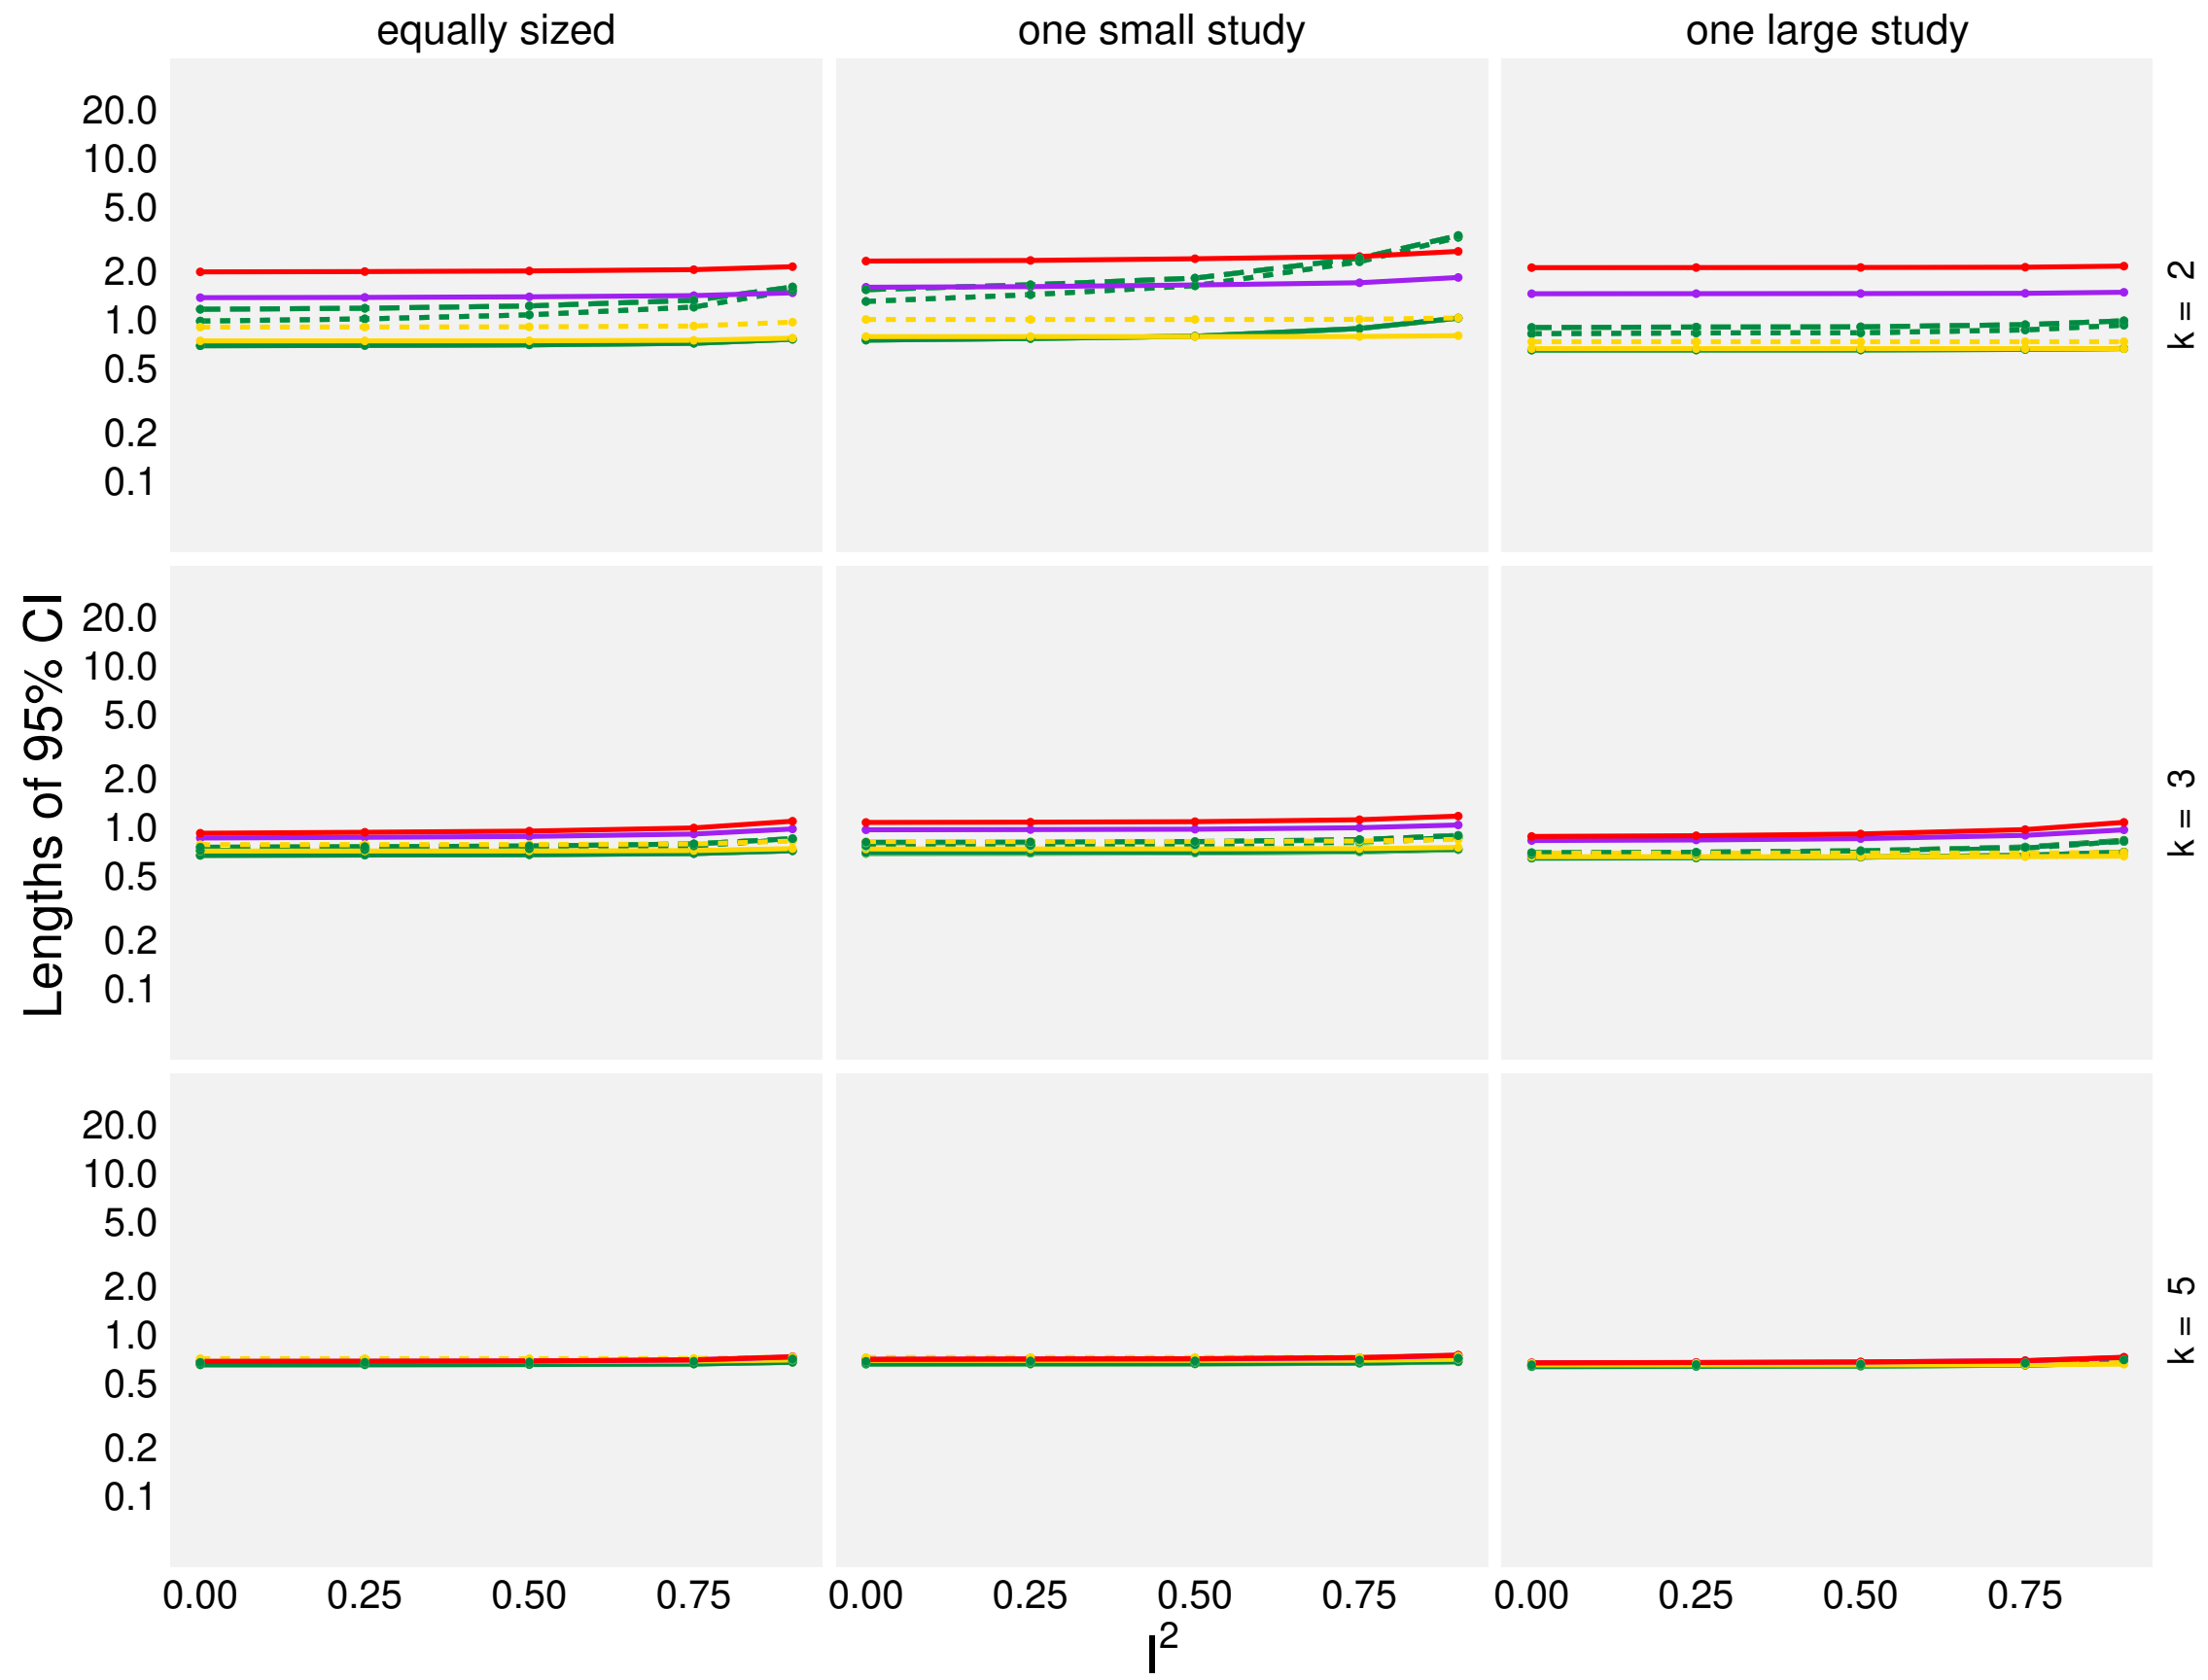

— NN – DL      — PN – PL      — normal quantiles  
 — NN – REML      — NN – Bayes HN(0.5)      - - HKSJ or Student's t  
 — NN – EB      — NN – Bayes HN(1)      - - mHKSJ

RR  
( $n_i=1000, \pi_0=0.1$ )

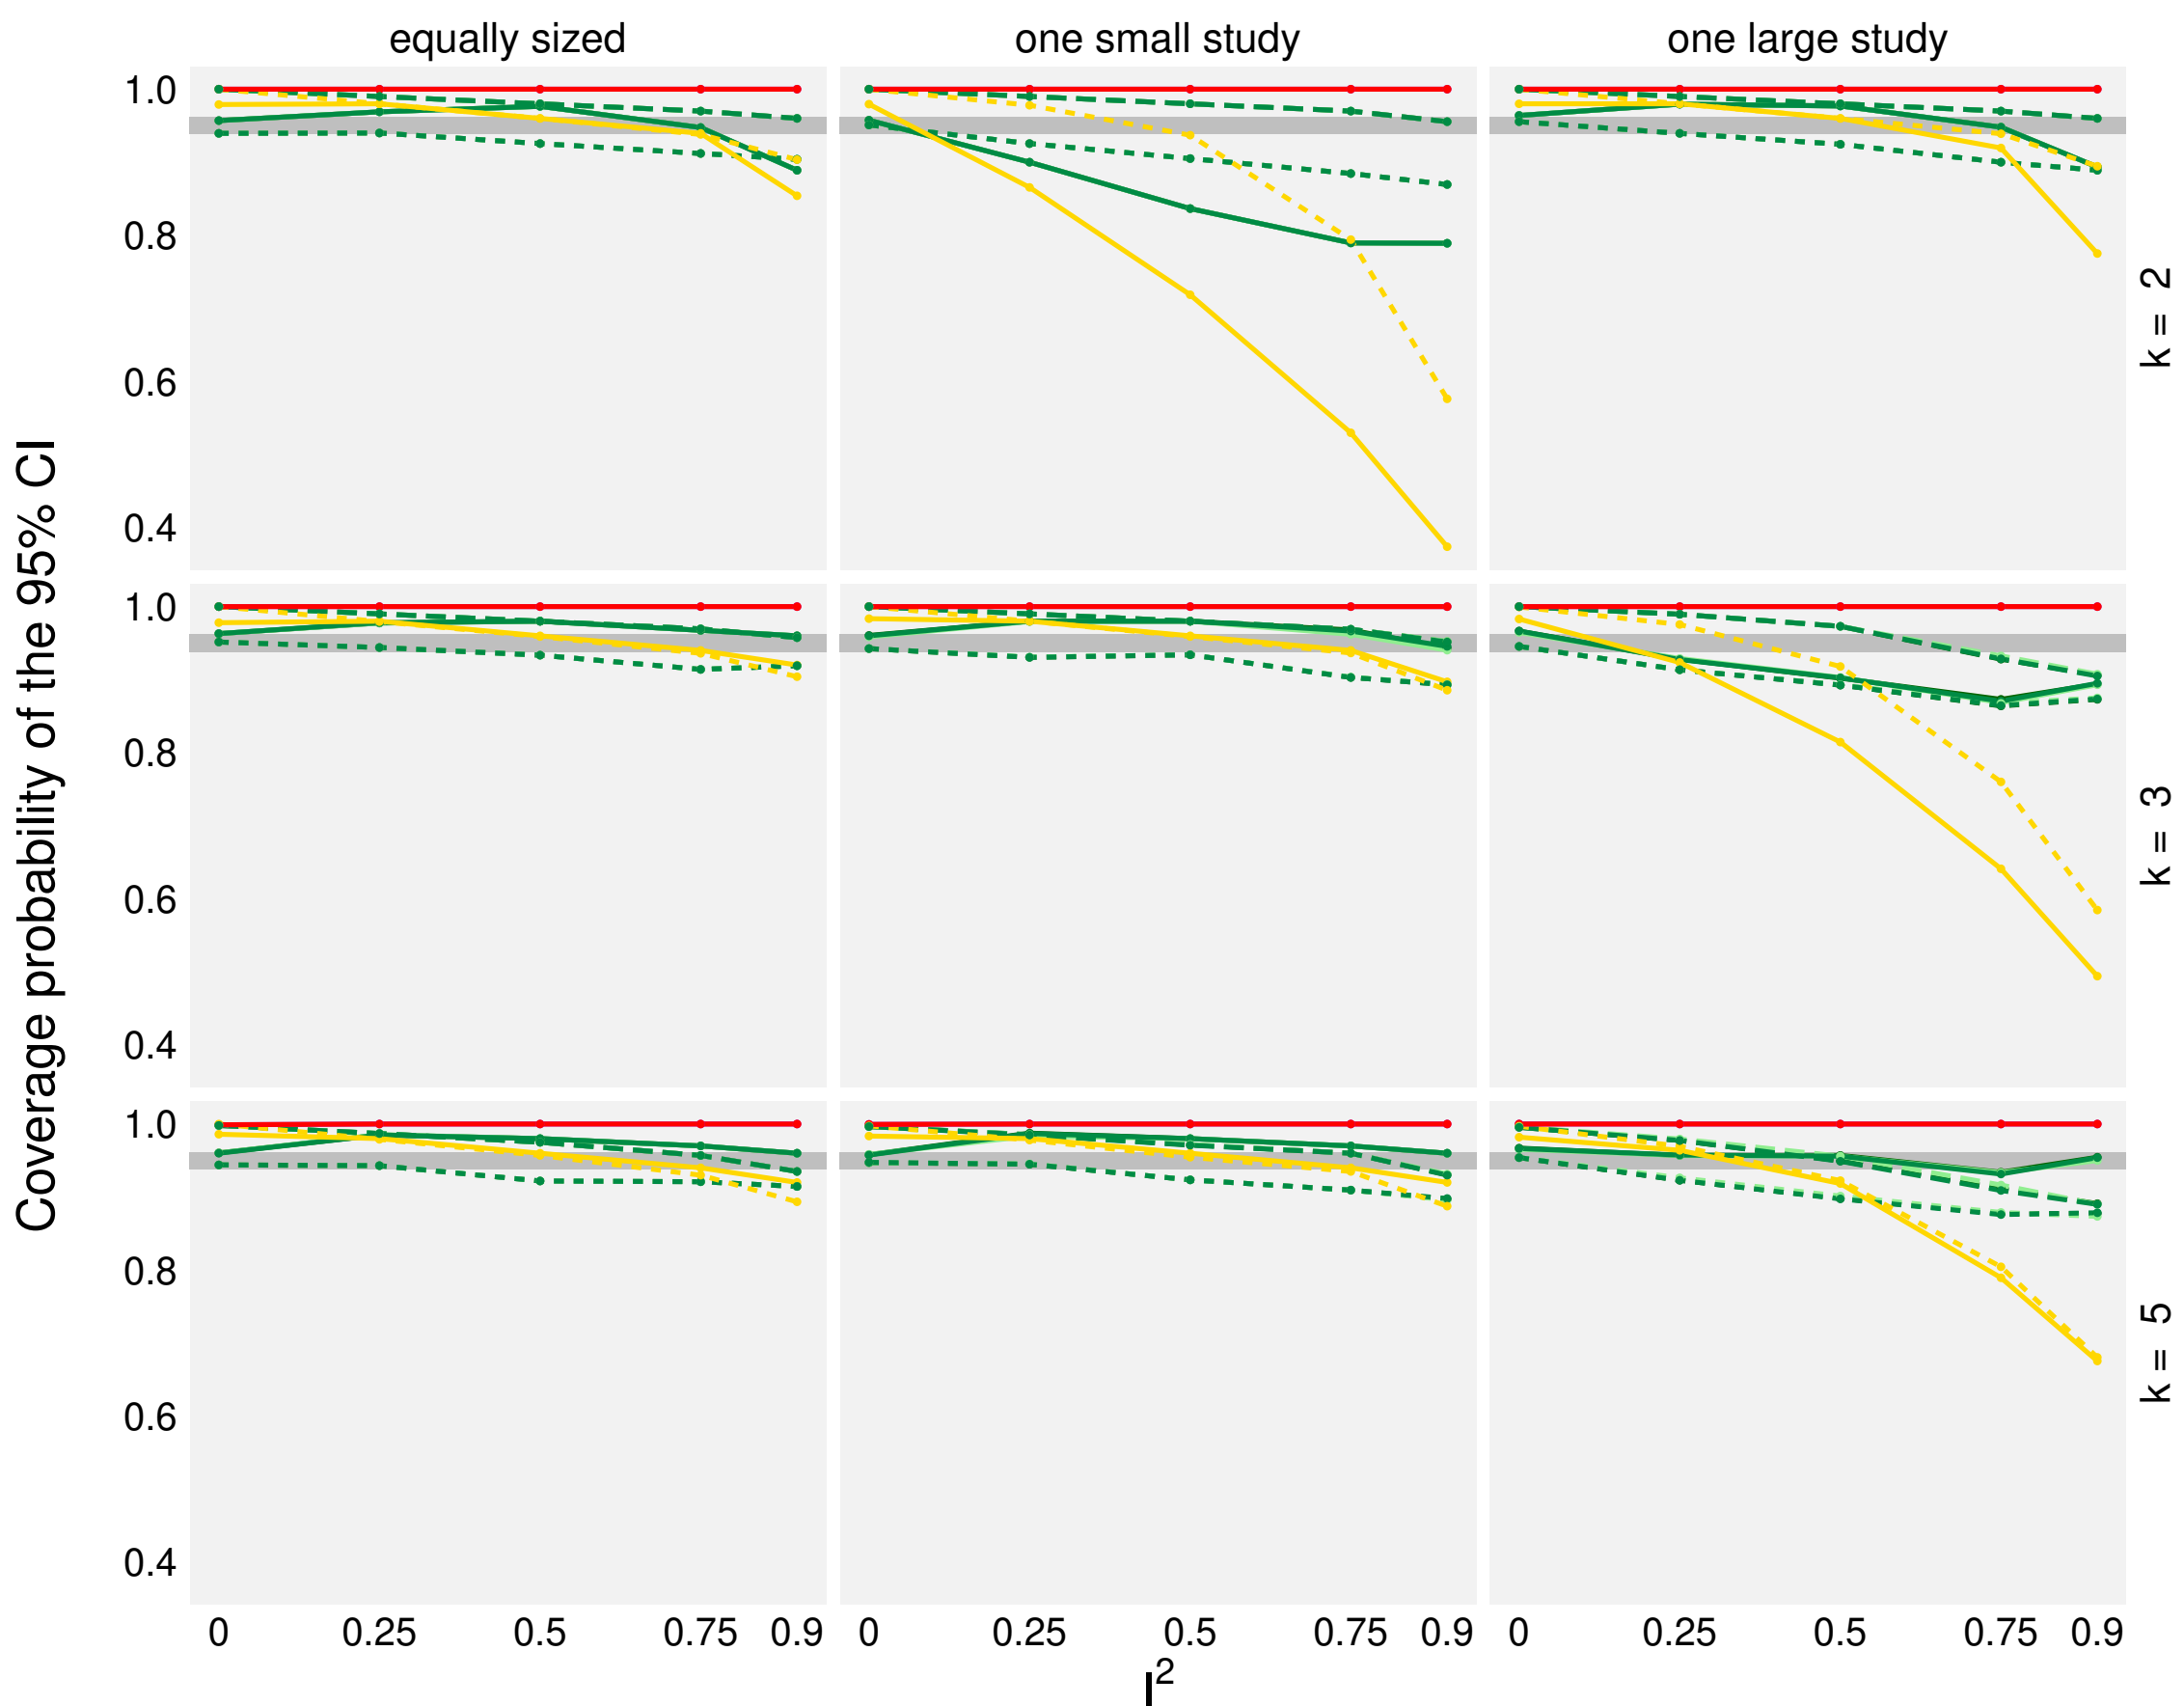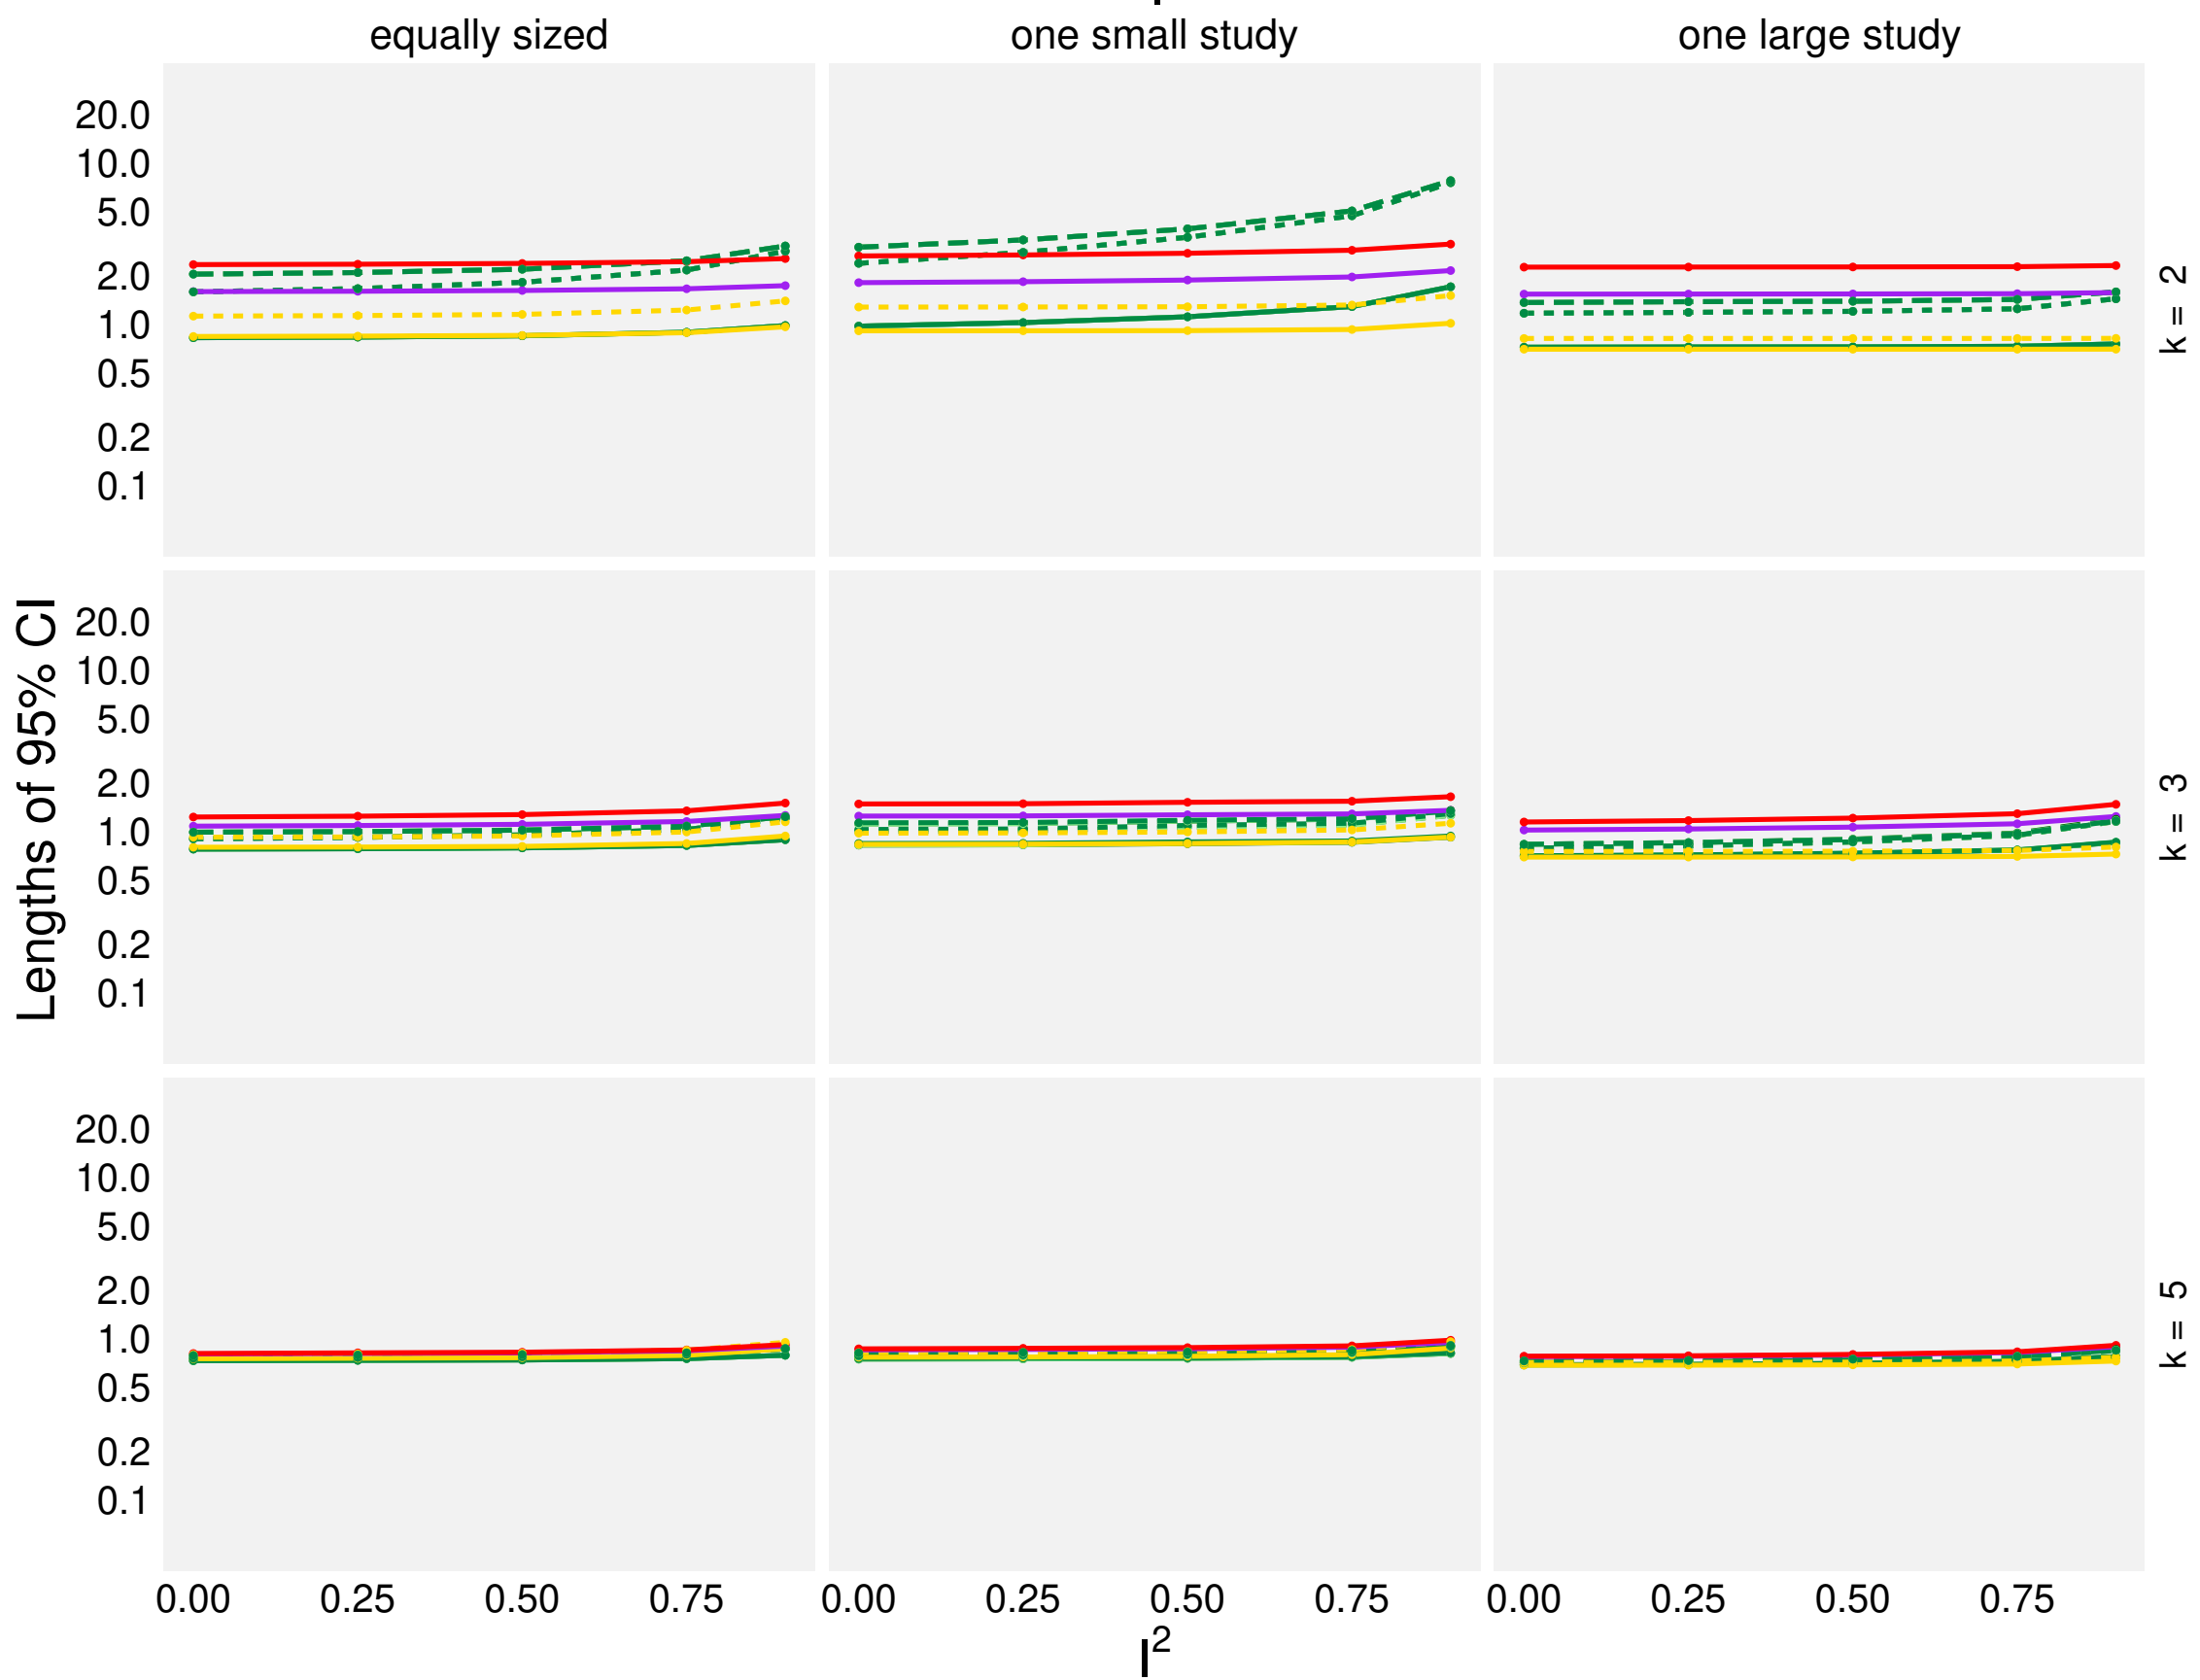

— NN – DL  
 — NN – REML  
 — NN – EB  
 — PN – PL  
 — NN – Bayes HN(0.5)  
 — NN – Bayes HN(1)  
 — normal quantiles  
 - - HKSJ or Student's t  
 - - mHKSJ

RR  
( $n_i=1000, \pi_0=0.3$ )

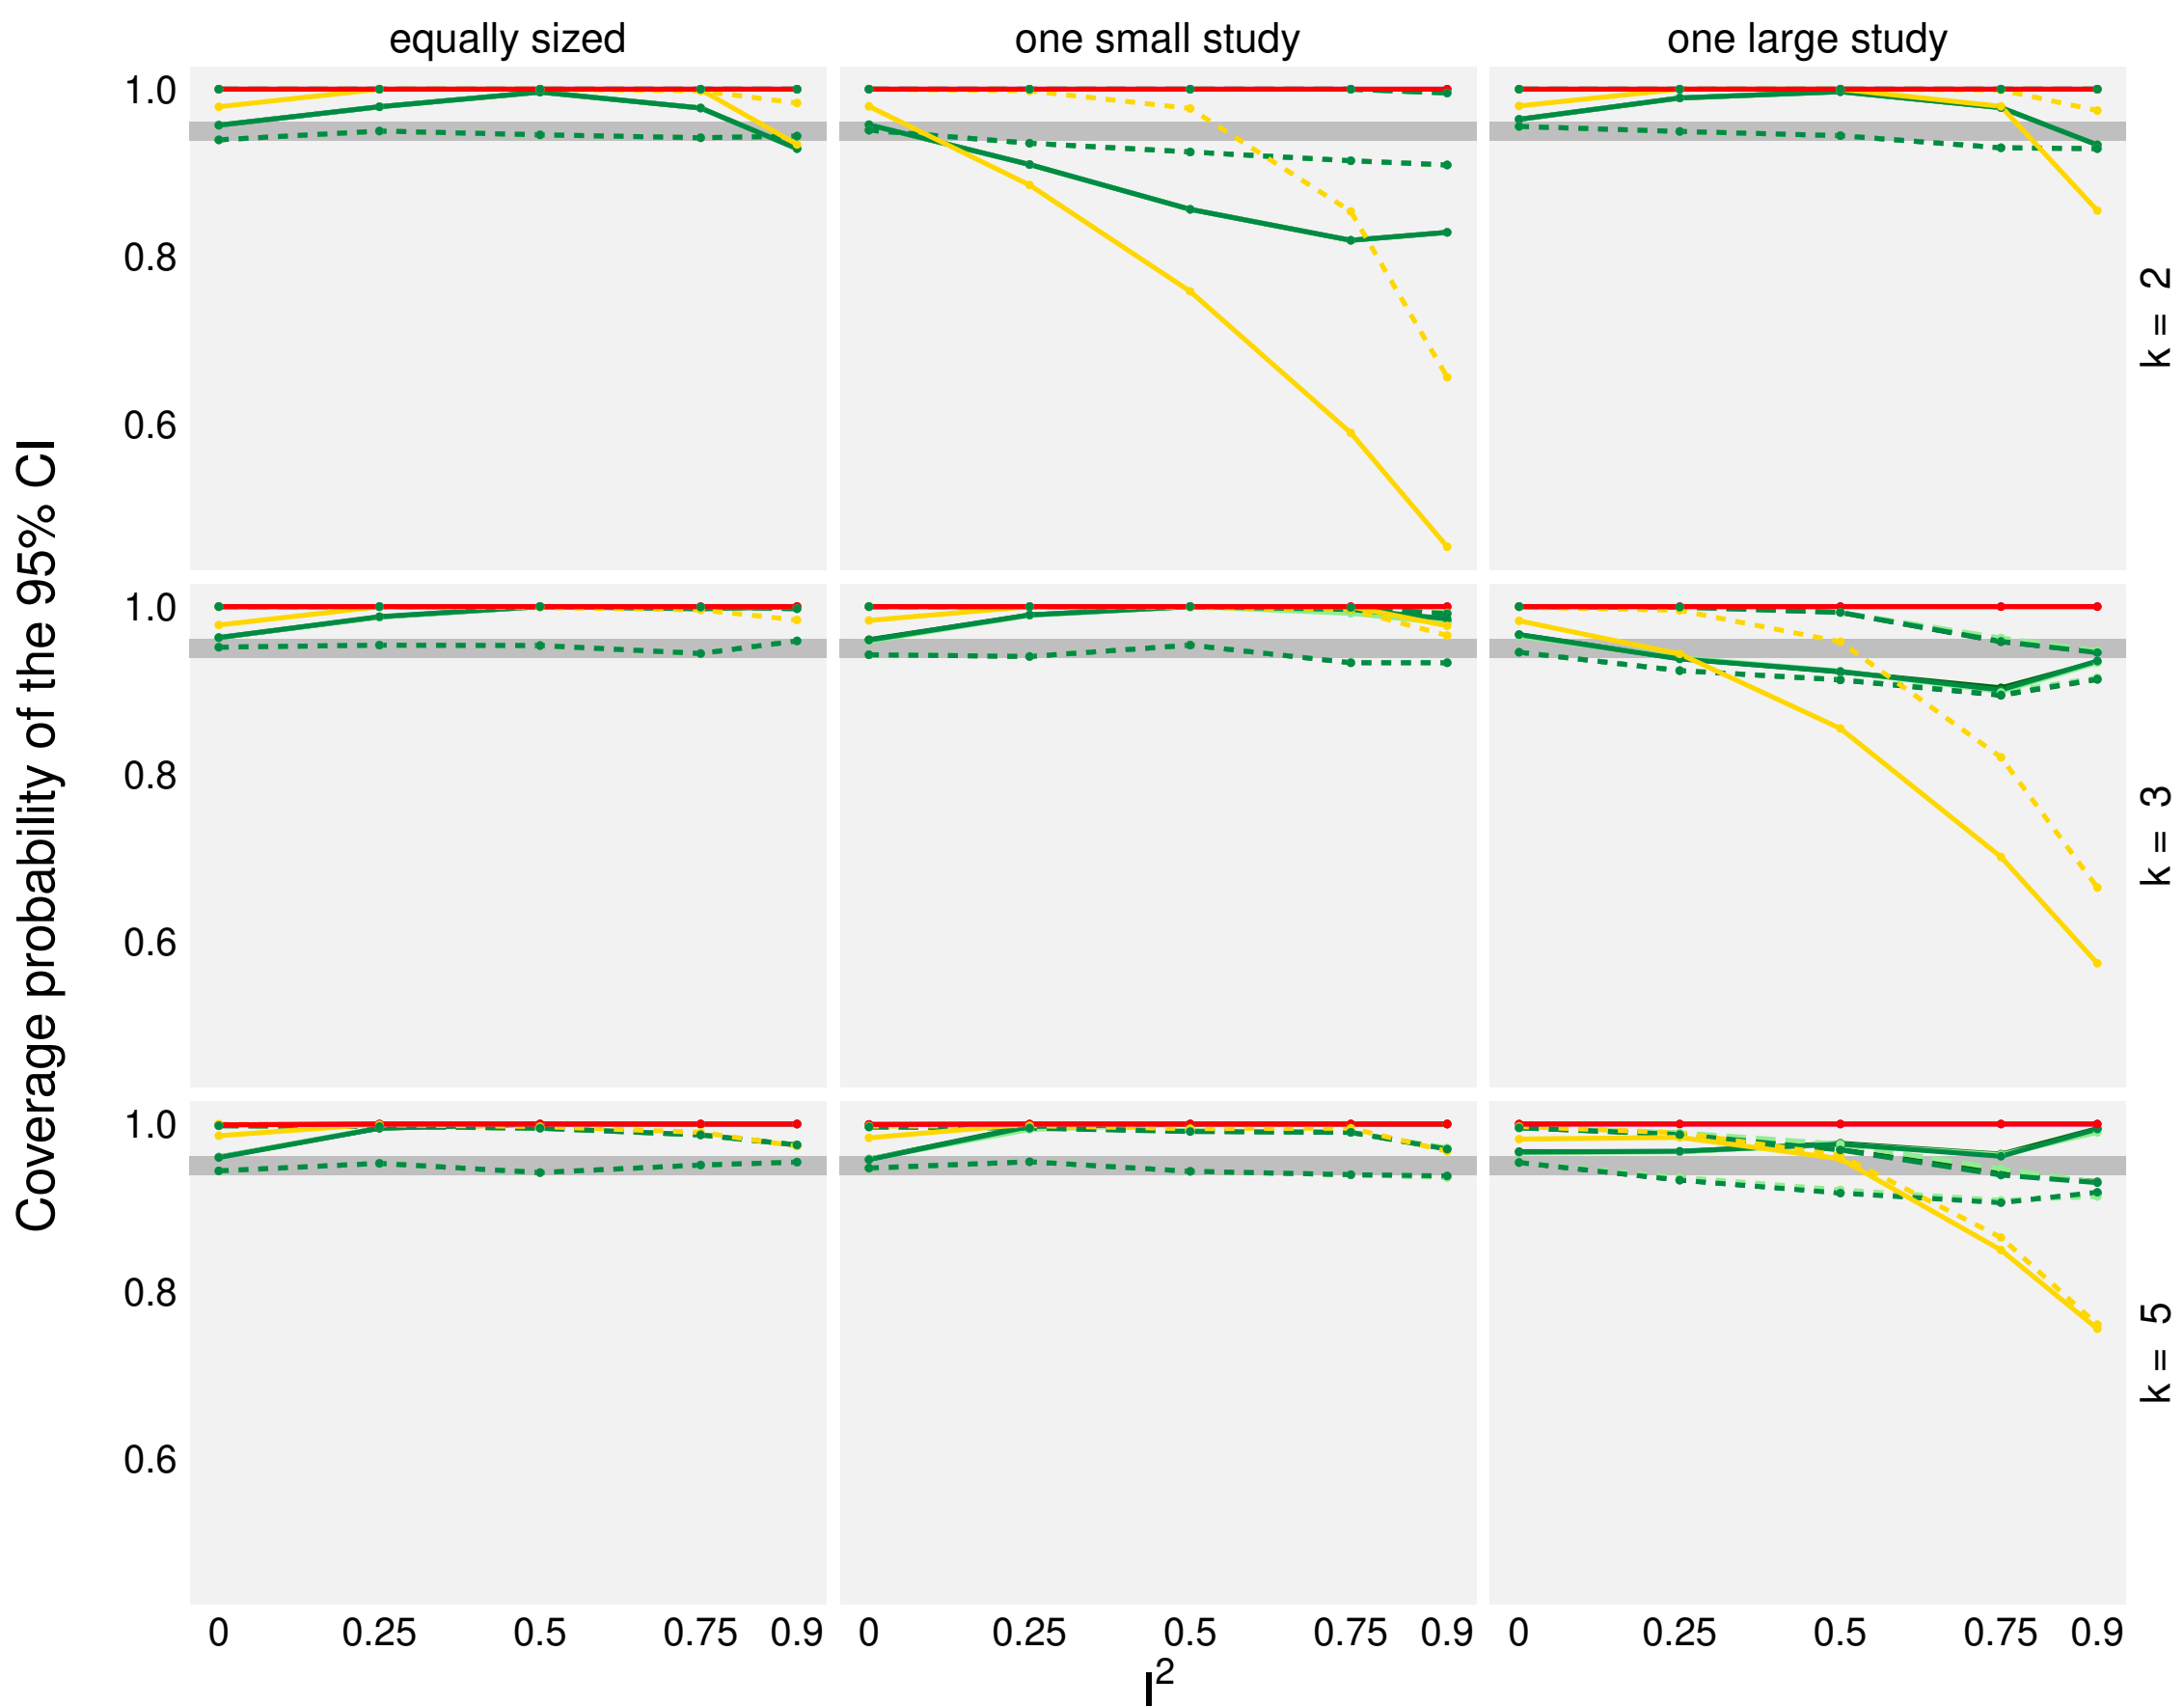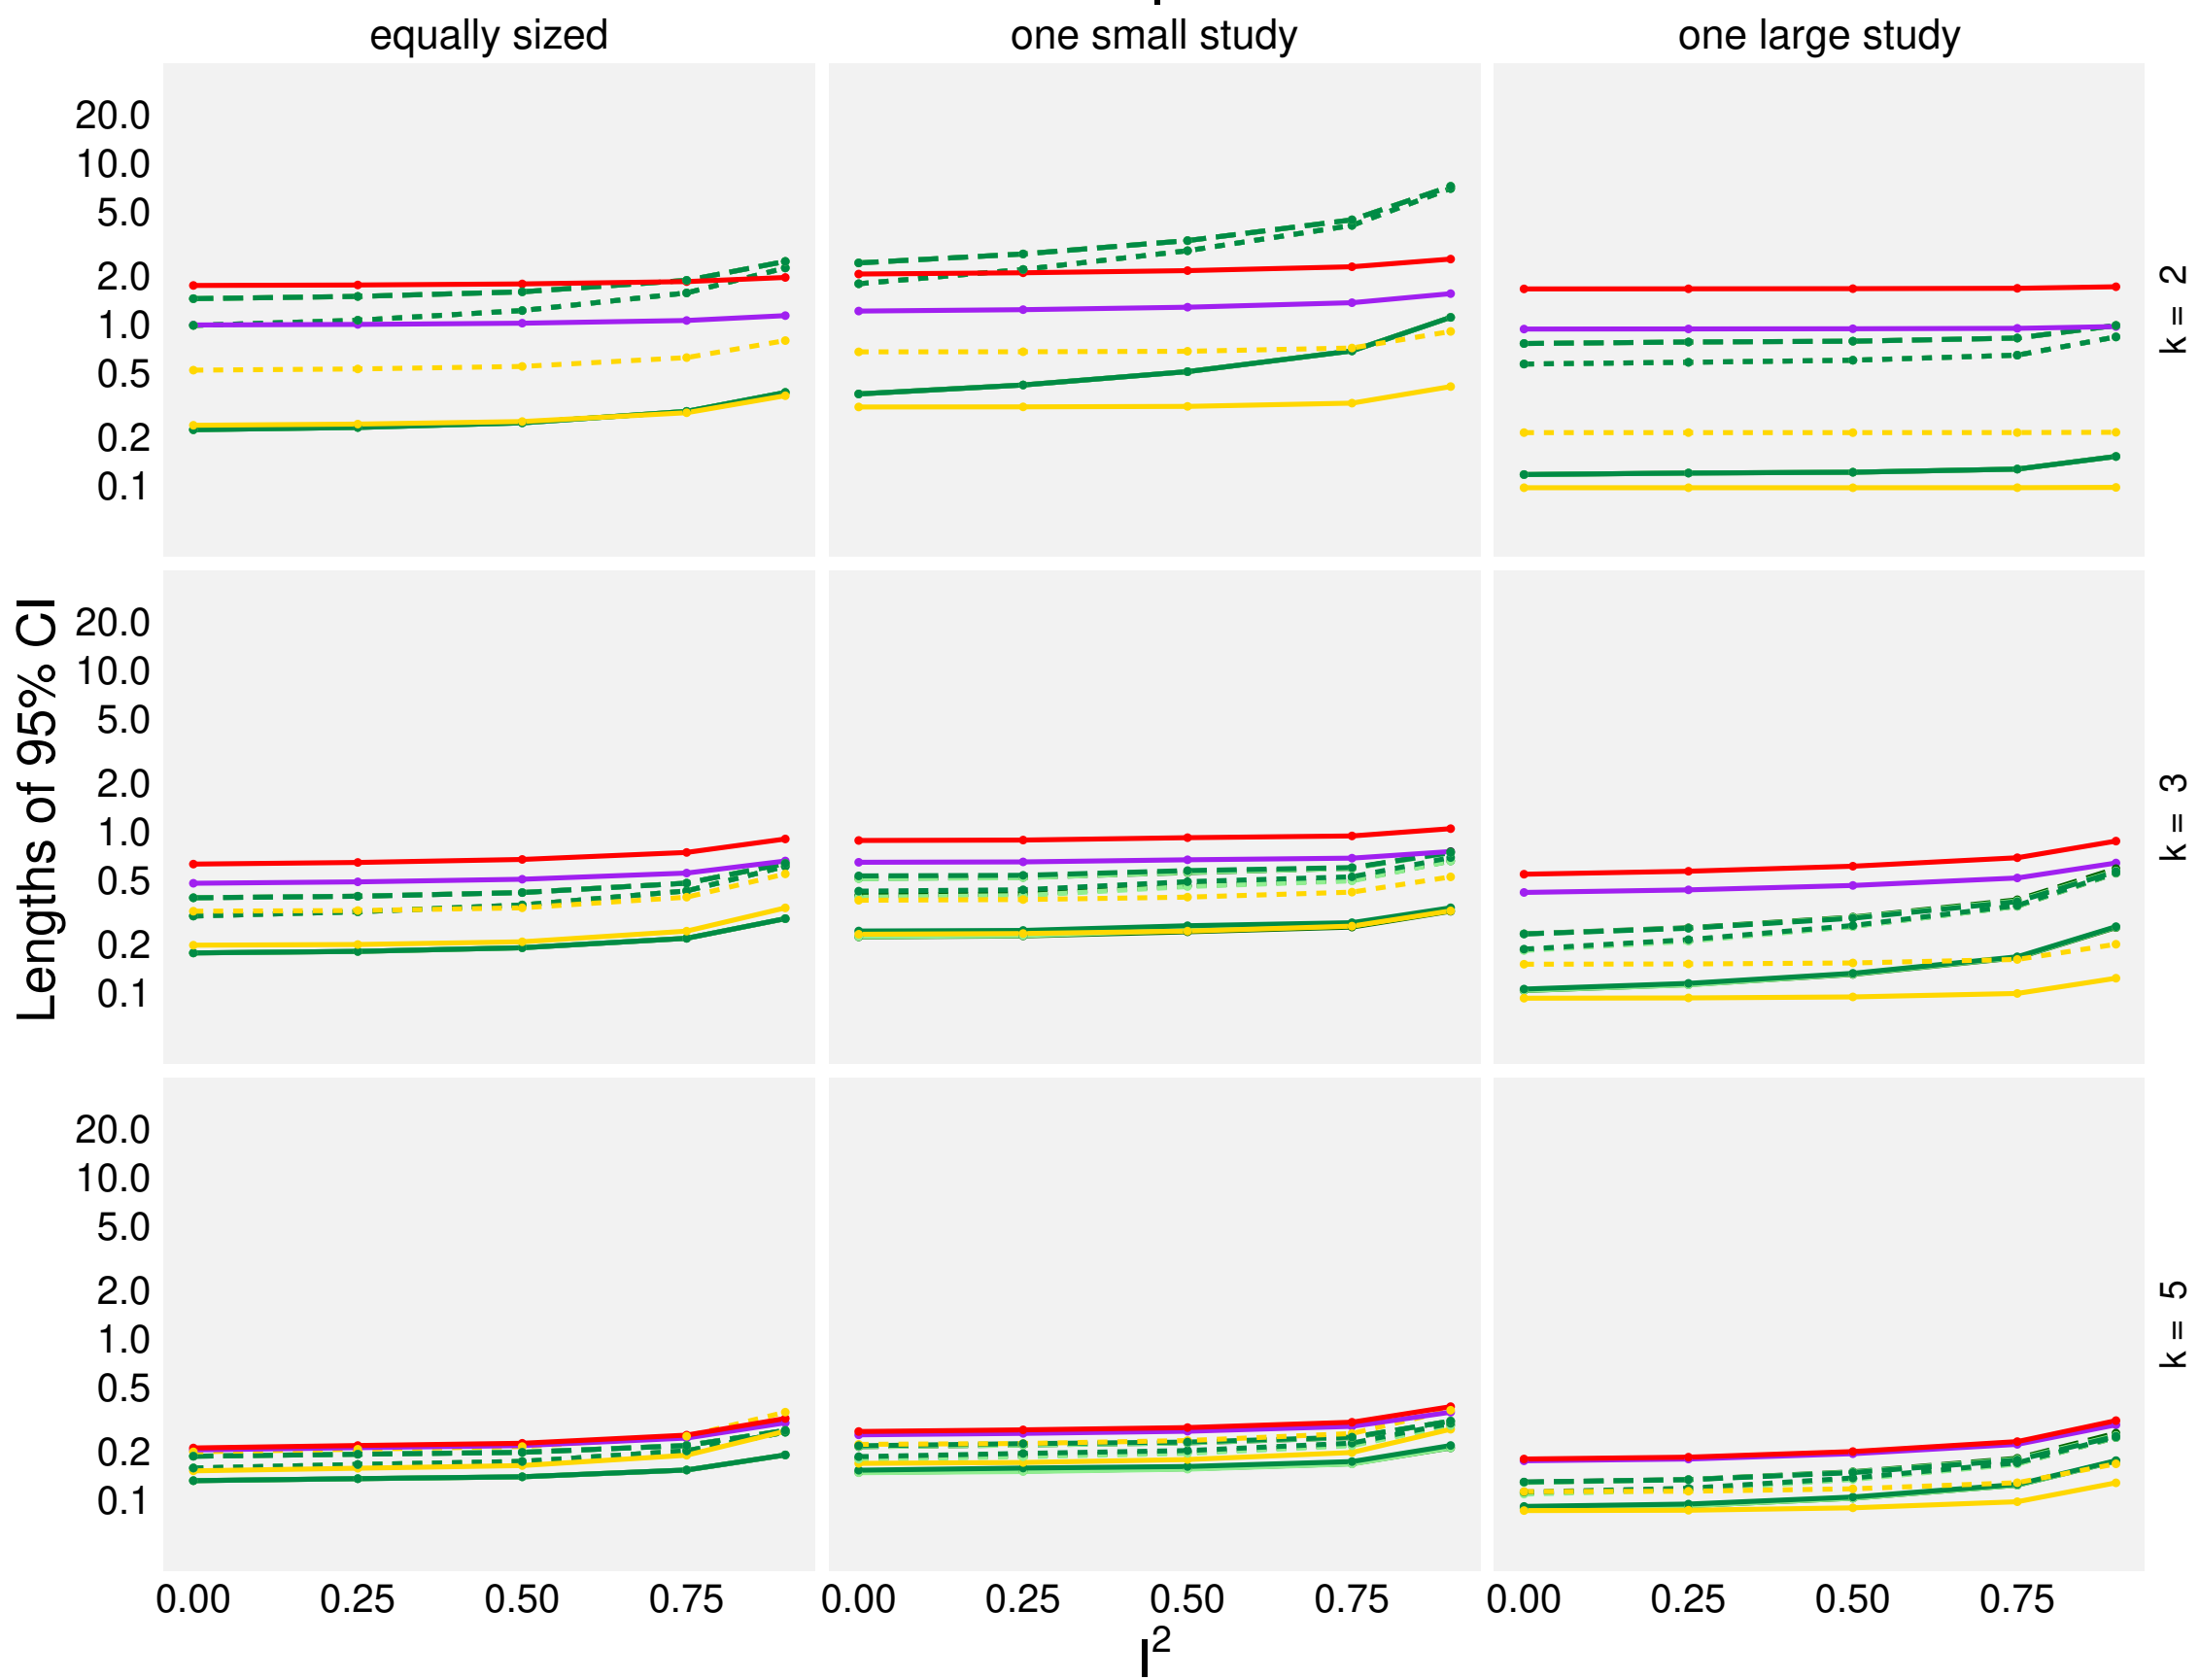

— NN — DL  
 — NN — REML  
 — NN — EB  
 — PN — PL  
 — NN — Bayes HN(0.5)  
 — NN — Bayes HN(1)  
 — normal quantiles  
 - - HKSJ or Student's t  
 - - mHKSJ

RR  
( $n_i=1000, \pi_0=0.5$ )

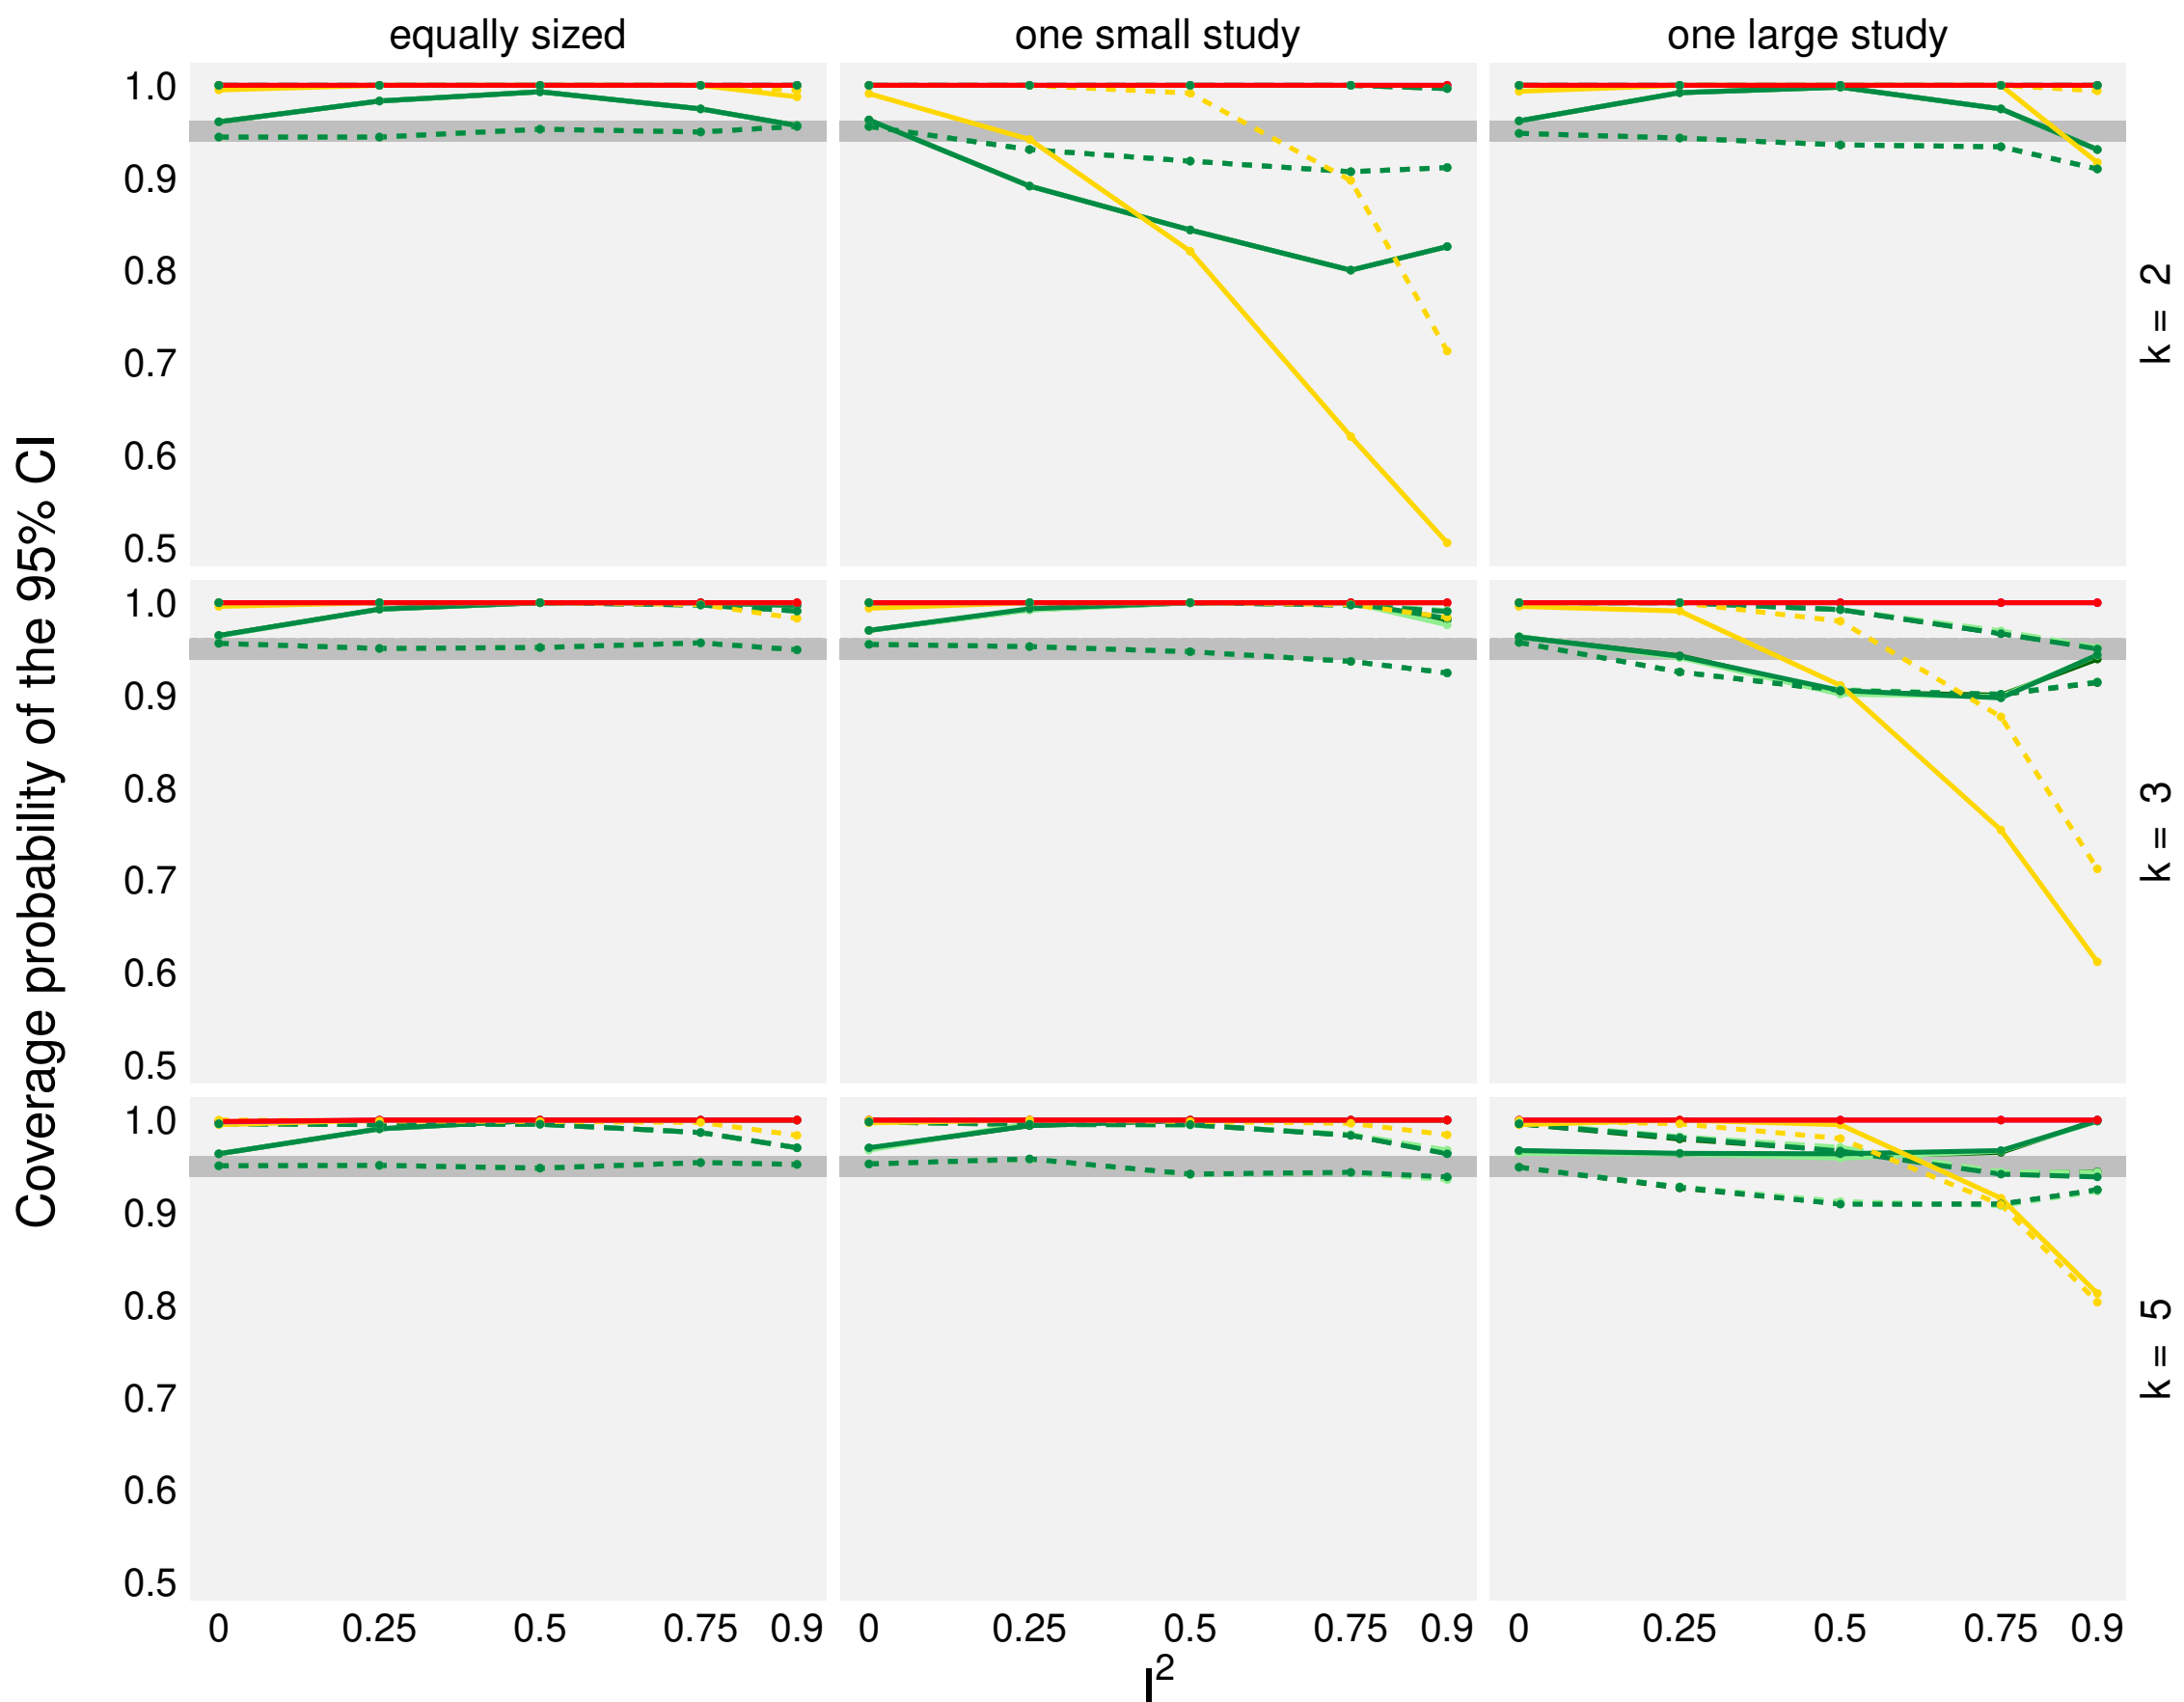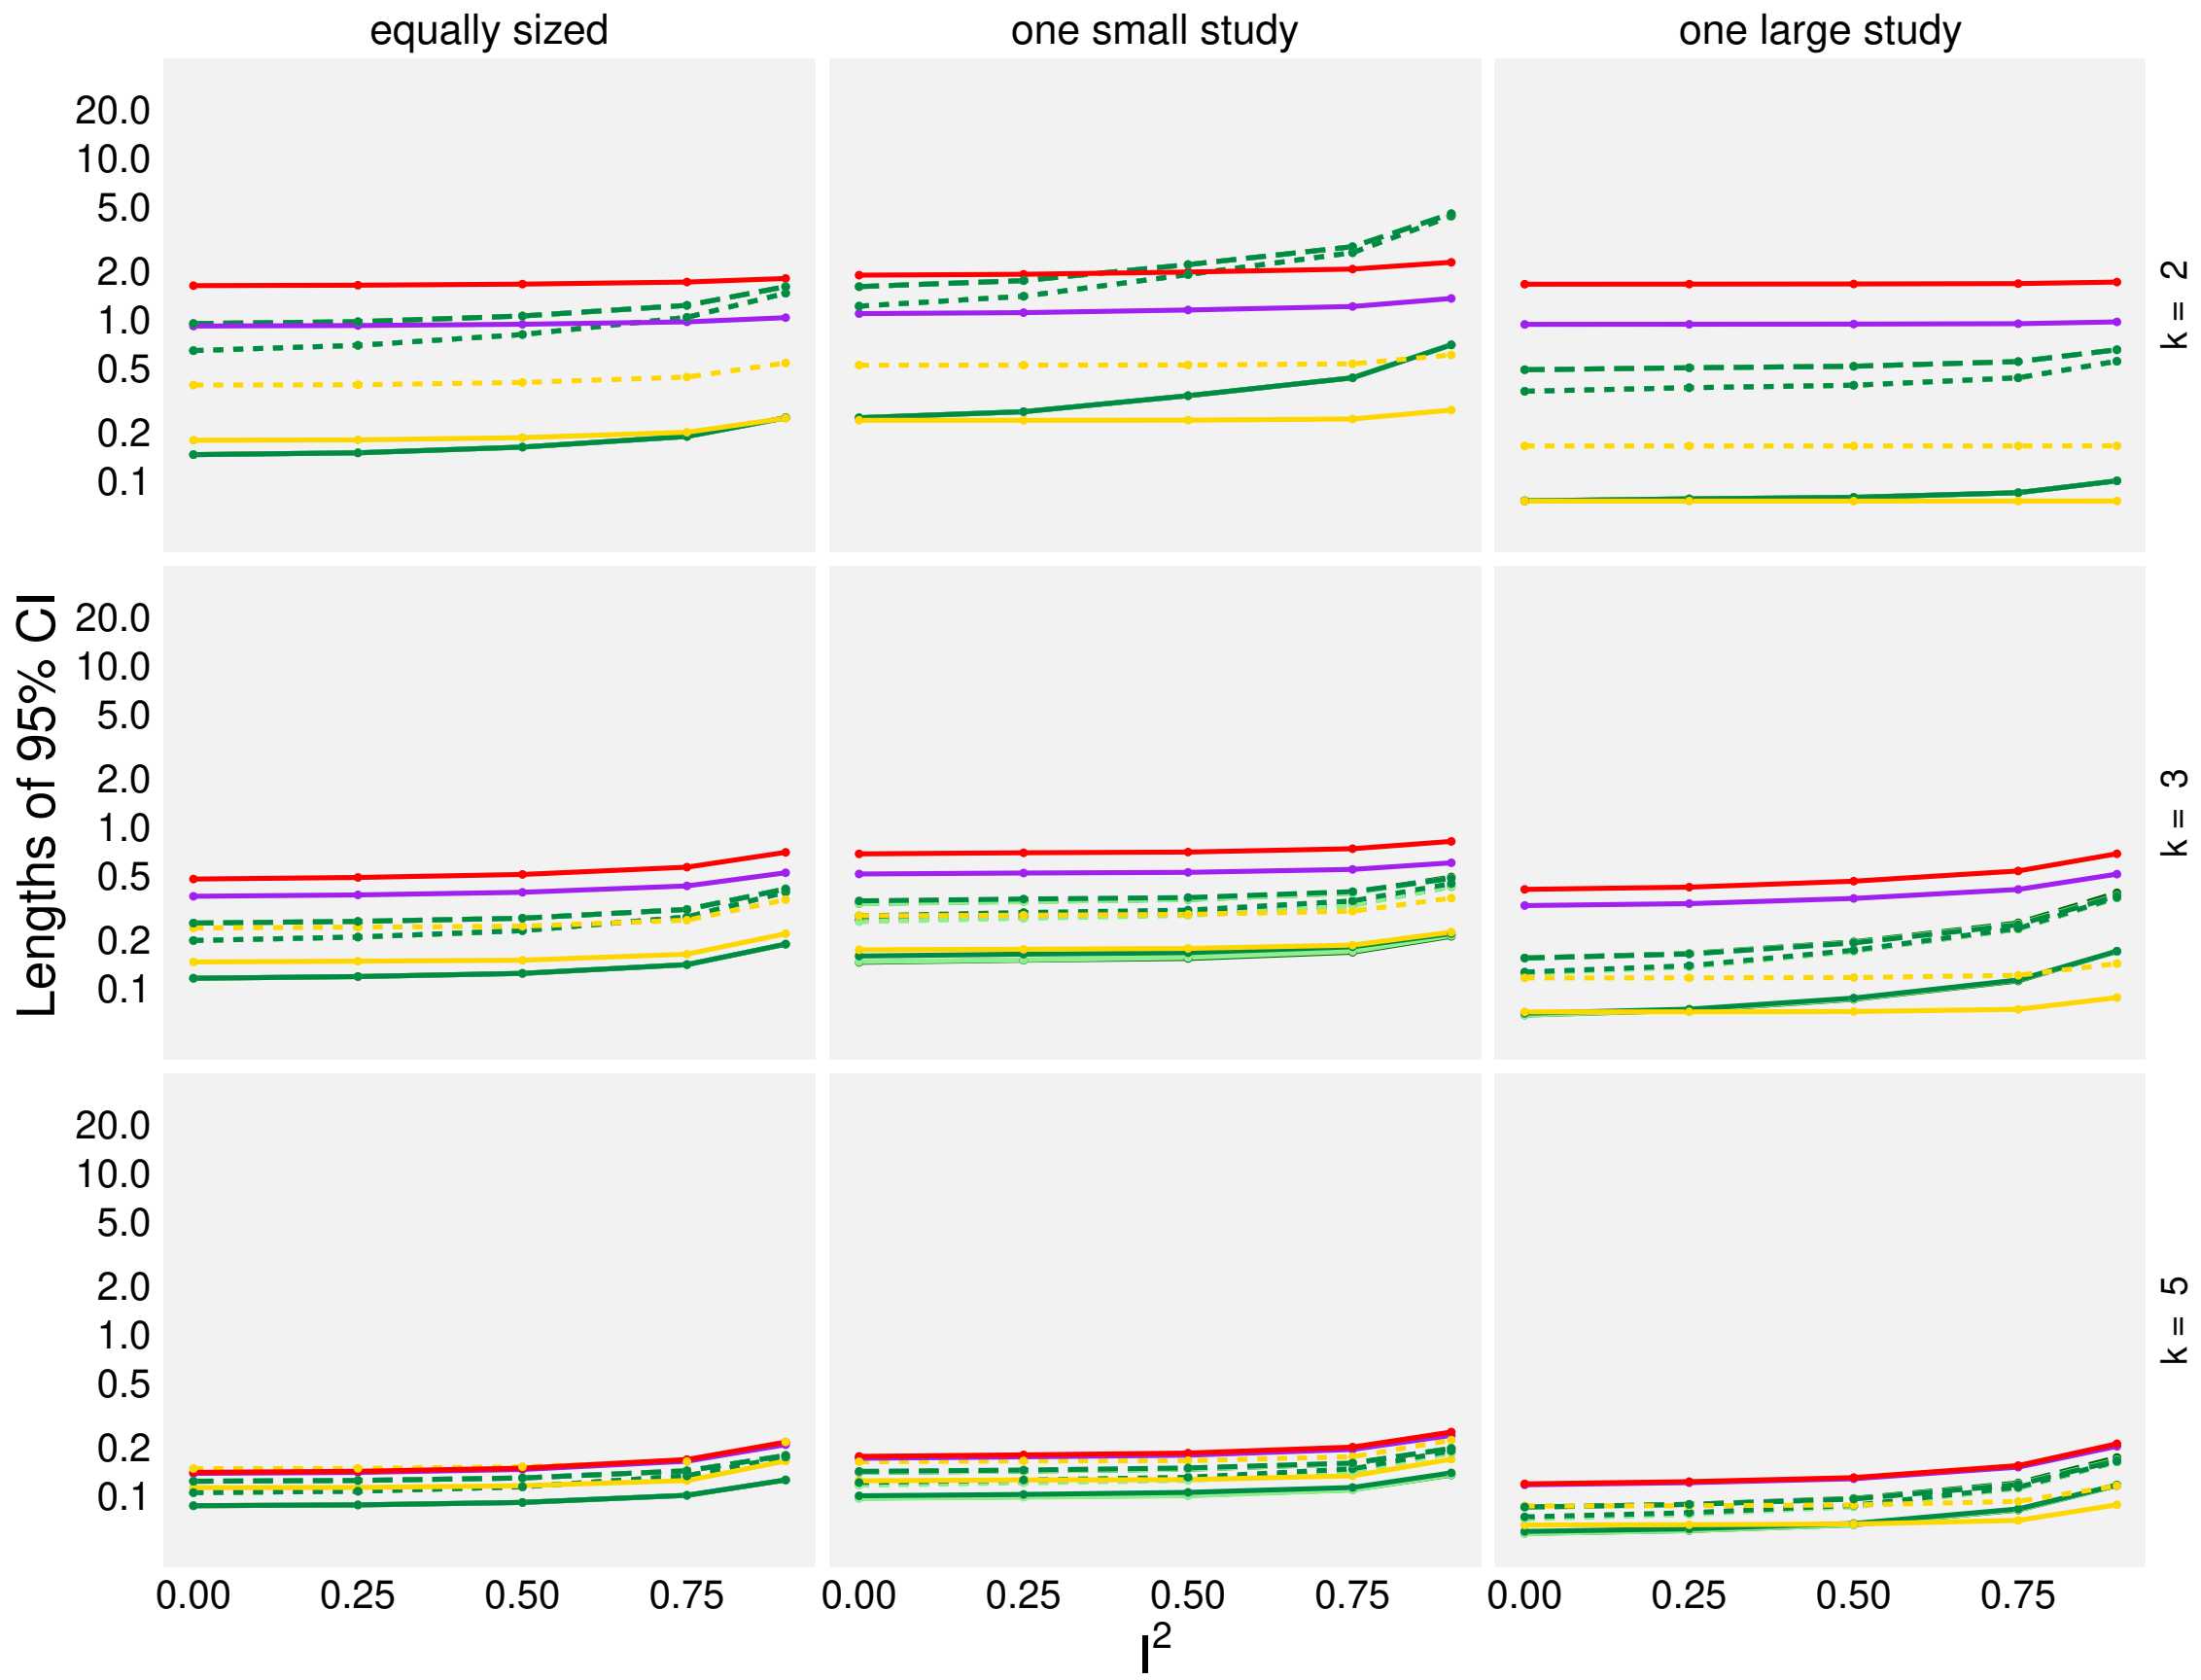

NN – DL      PN – PL      — normal quantiles  
 NN – REML      NN – Bayes HN(0.5)      - - HKSJ or Student's t  
 NN – EB      NN – Bayes HN(1)      - - mHKSJ

RR  
( $n_i=1000, \pi_0=0.7$ )

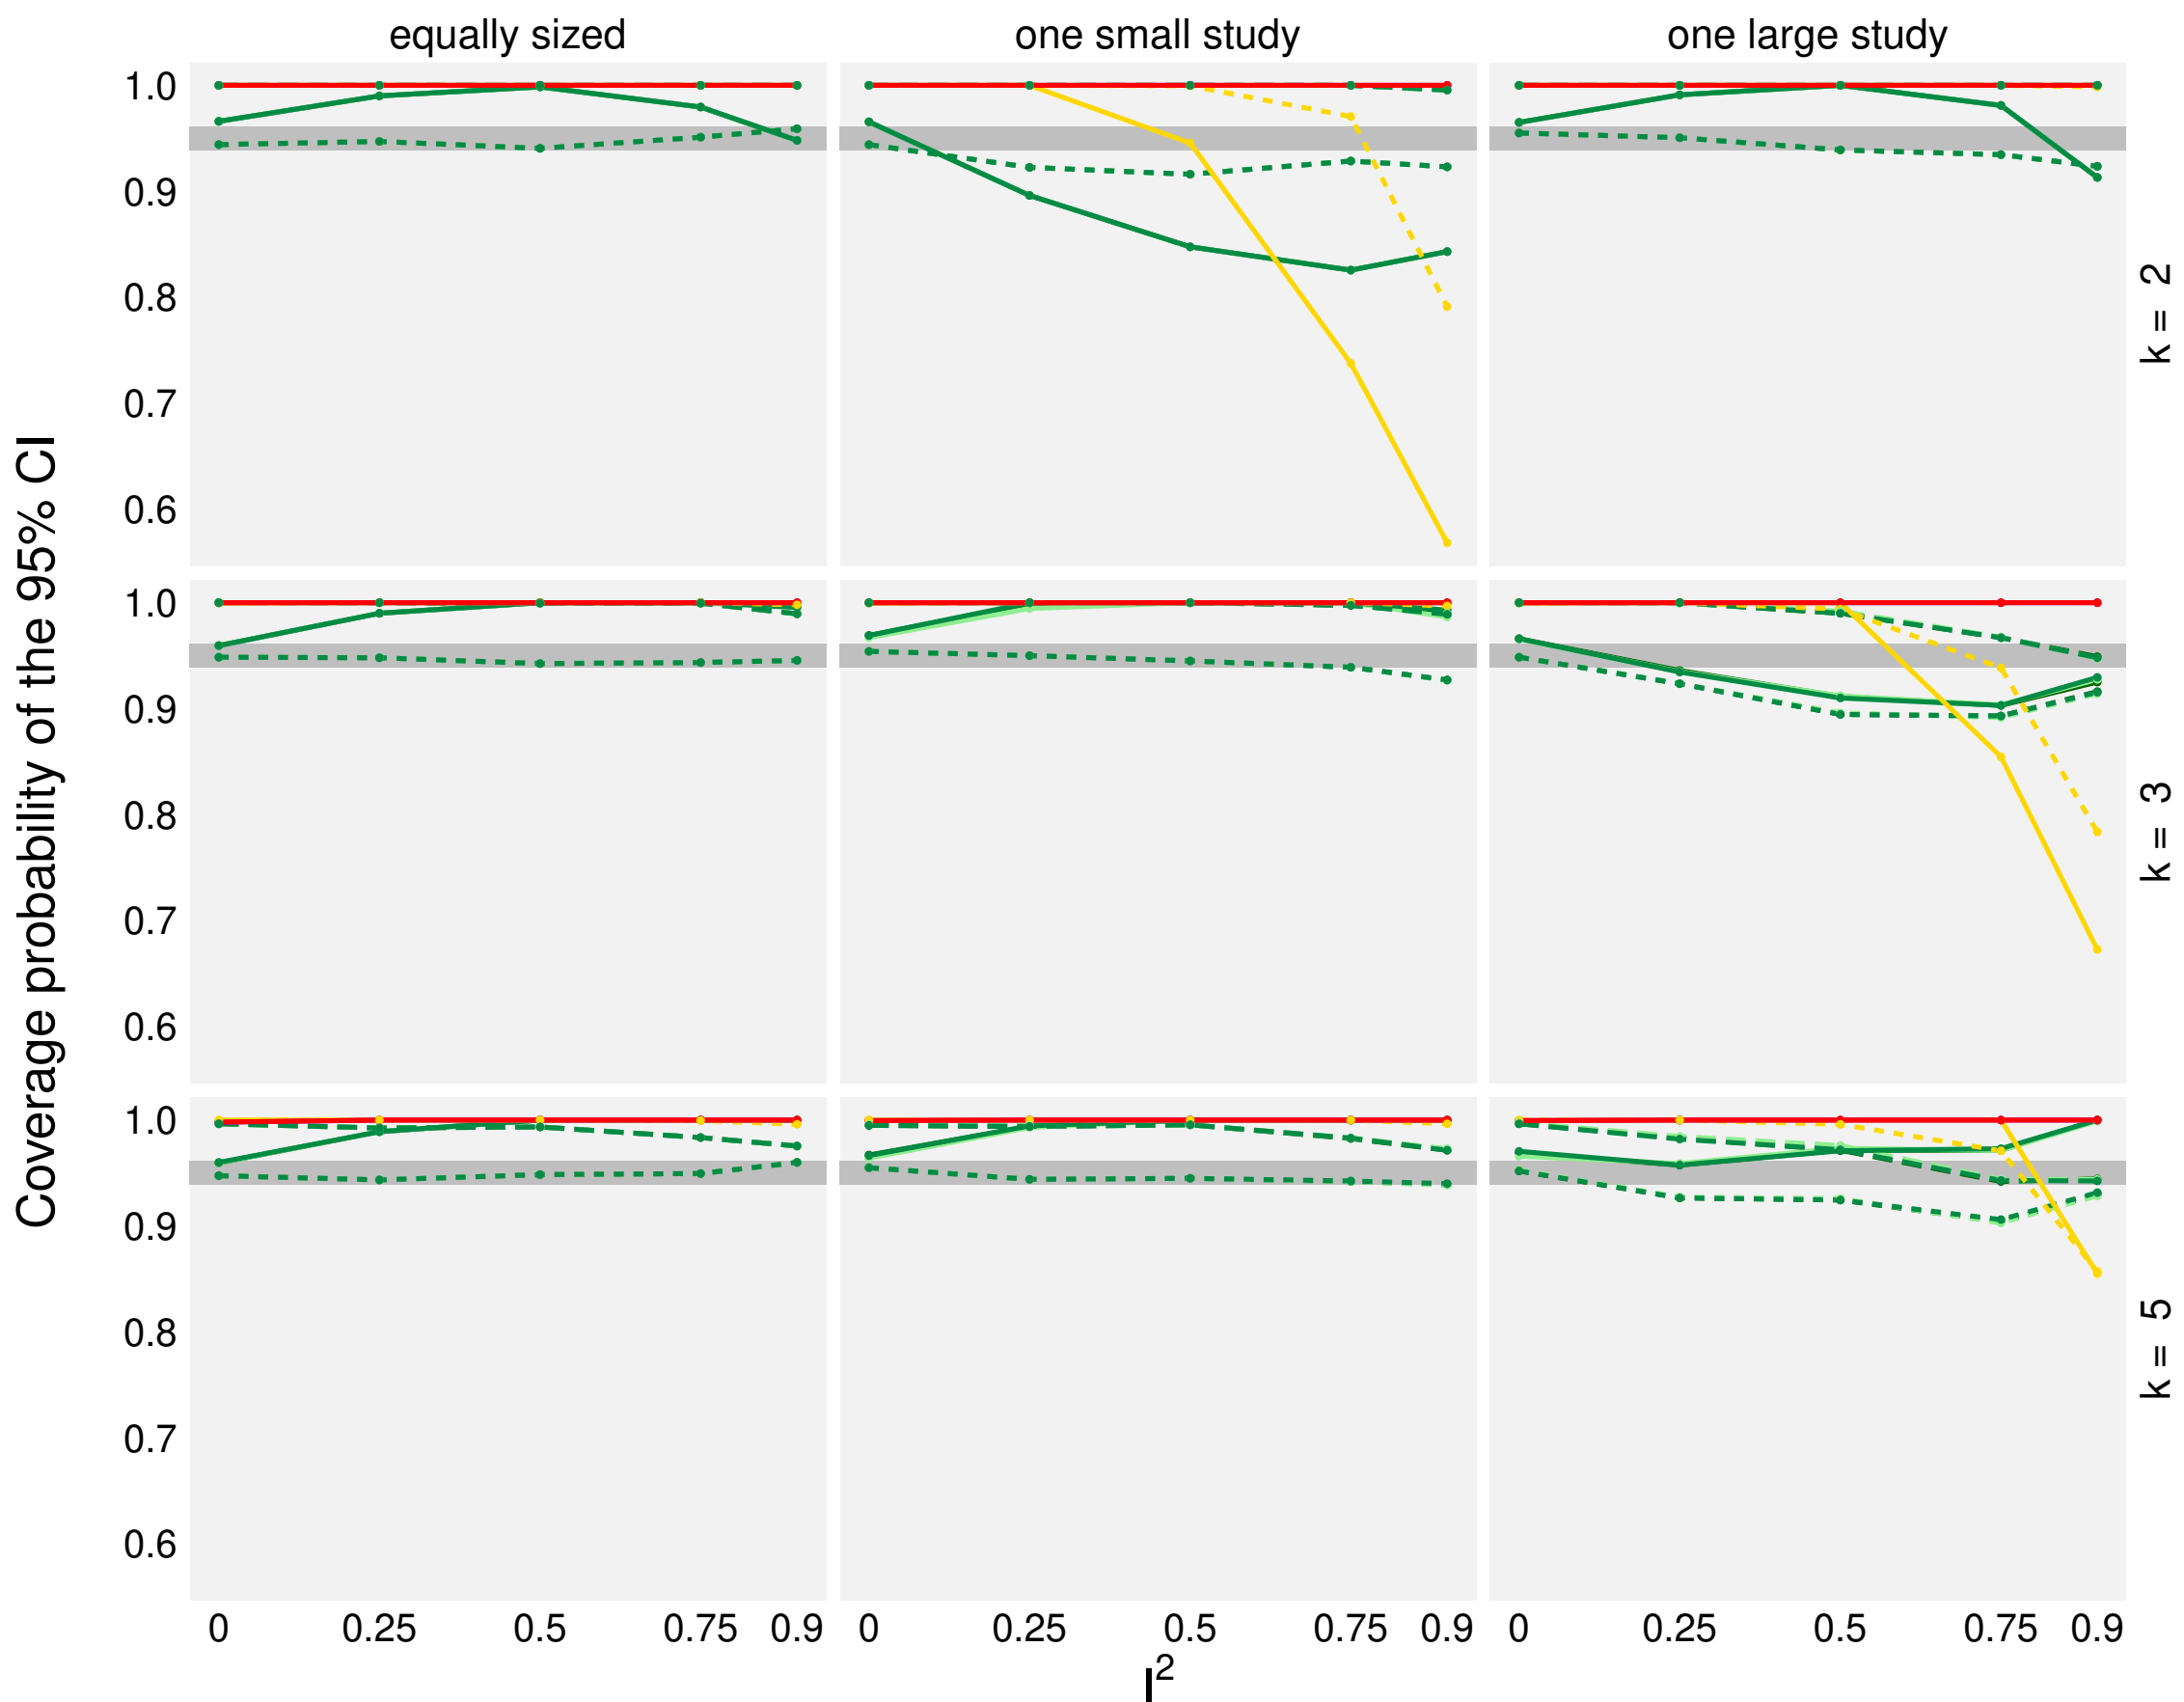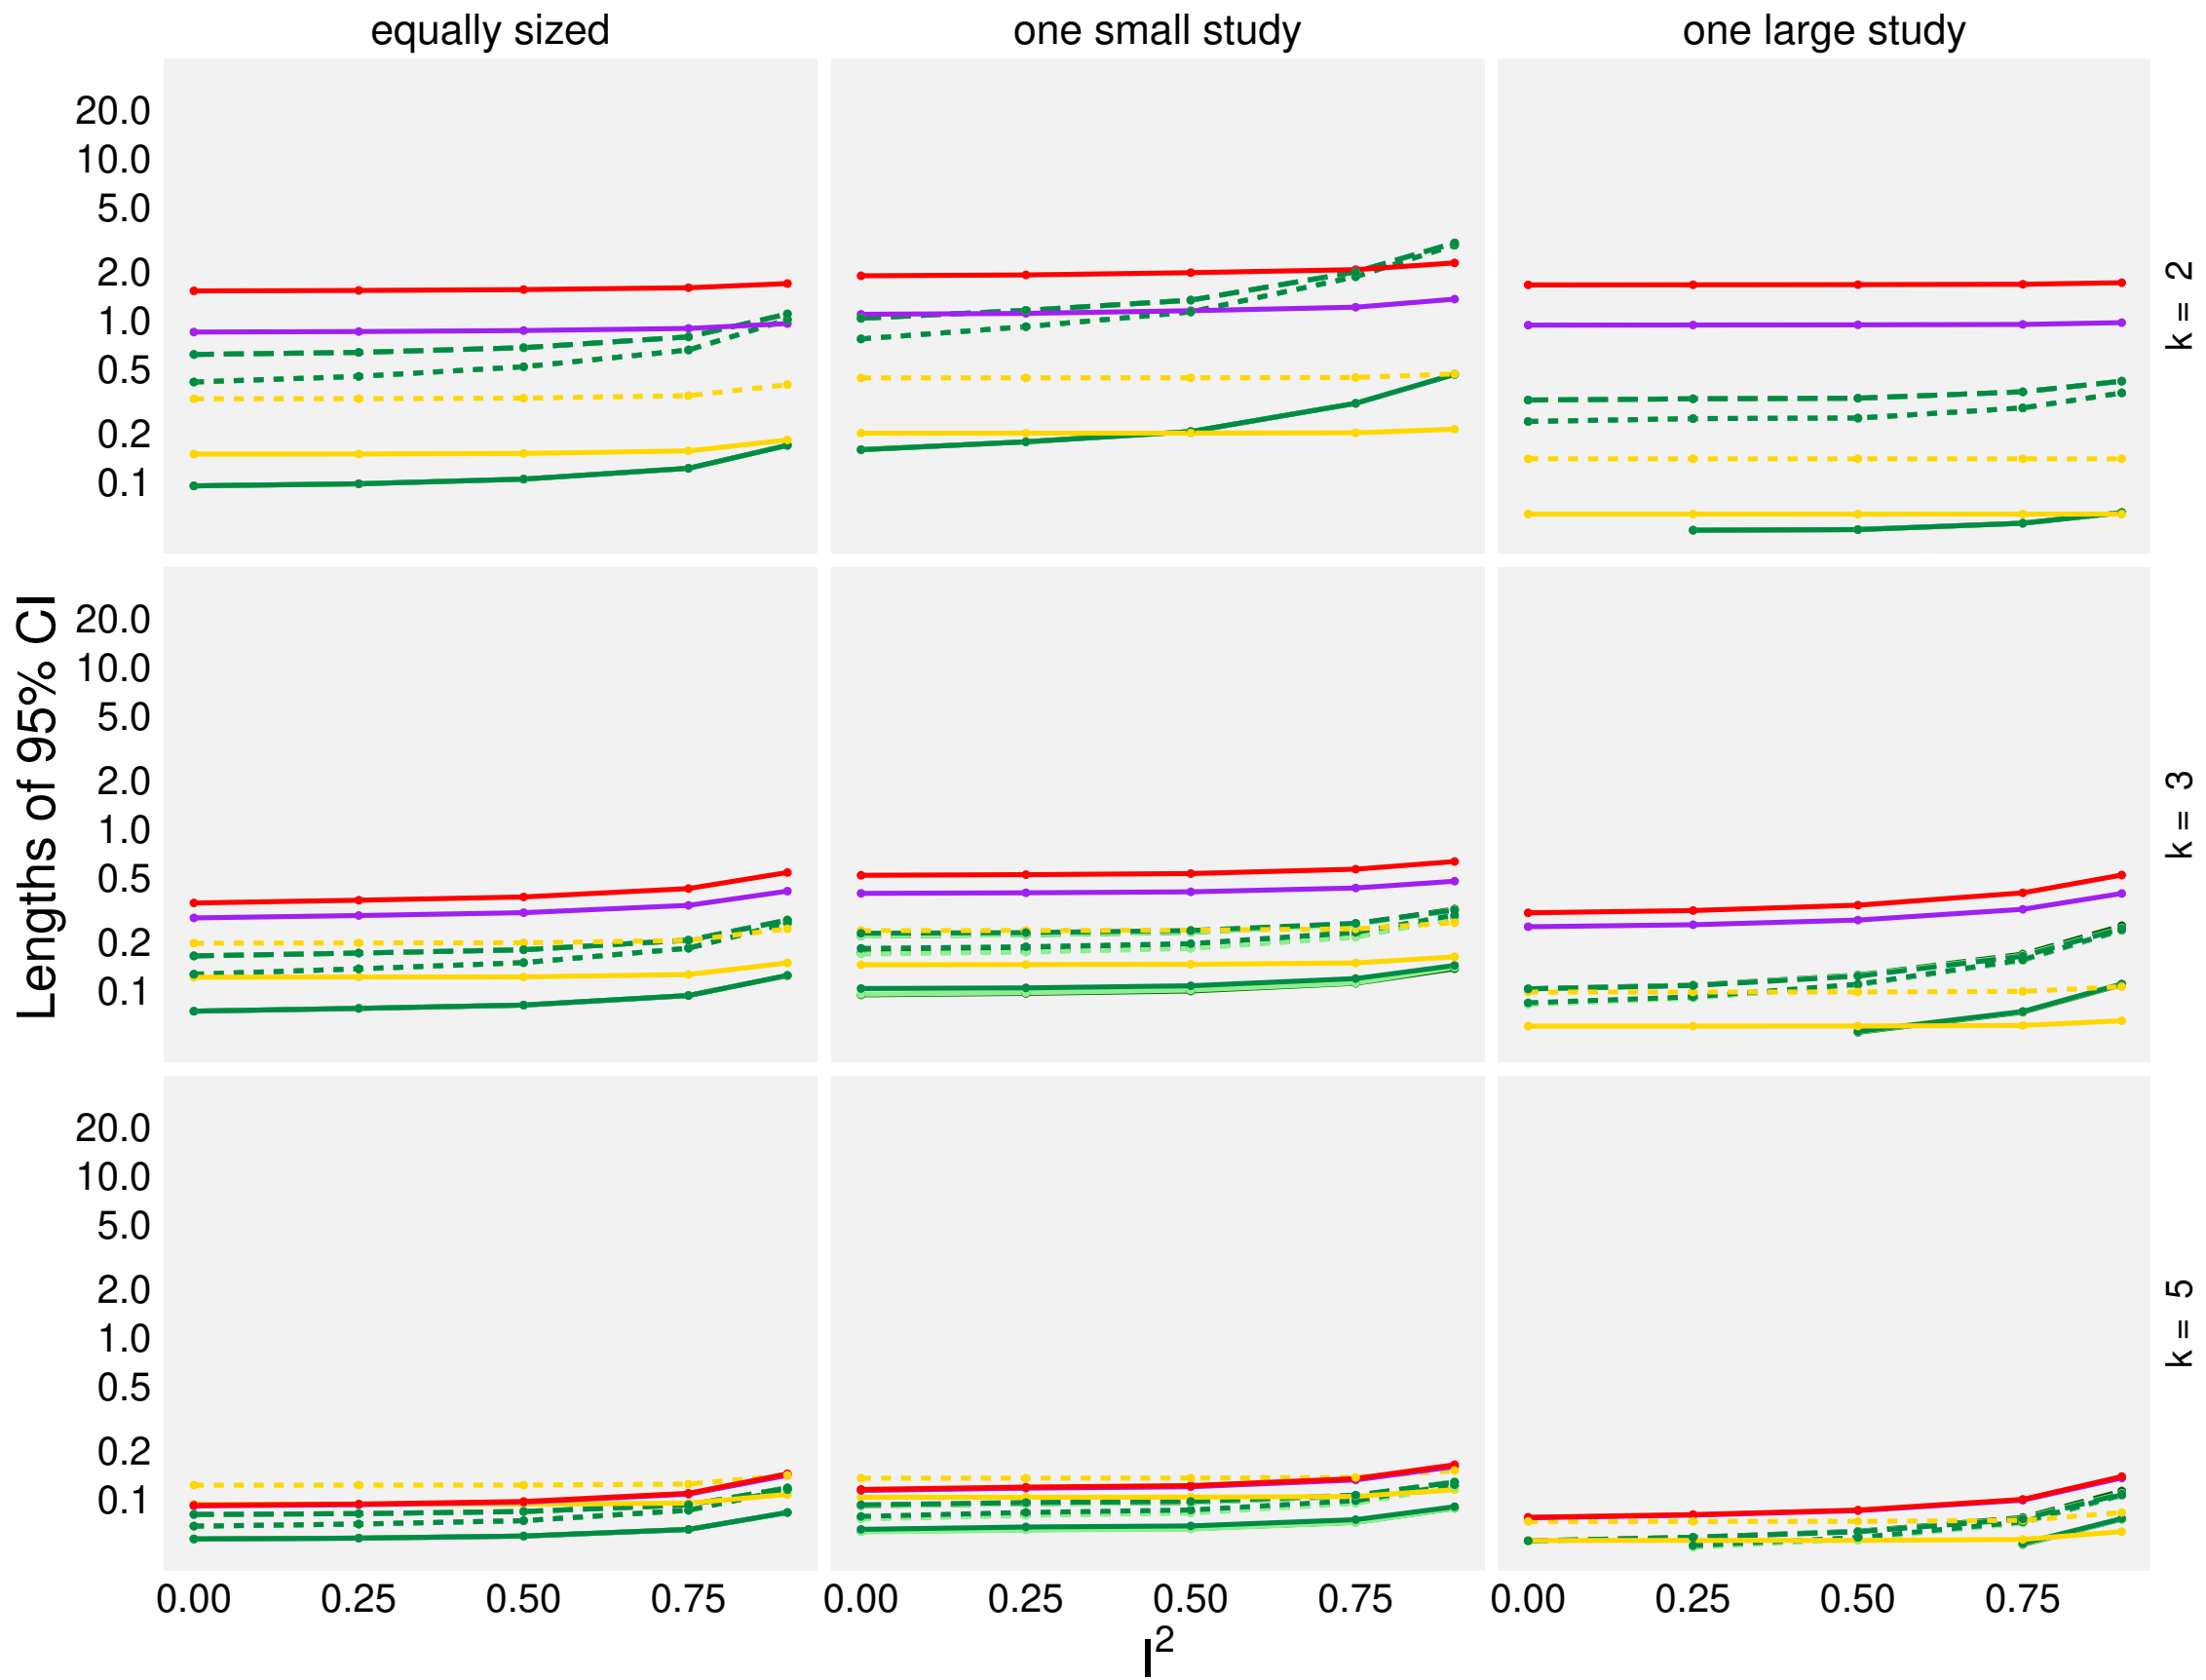

NN - DL  
 NN - REML  
 NN - EB  
 PN - PL  
 NN - Bayes HN(0.5)  
 NN - Bayes HN(1)  
 — normal quantiles  
 -- HKSJ or Student's t  
 -- mHKSJ

RR  
( $n_i=1000, \pi_0=0.9$ )

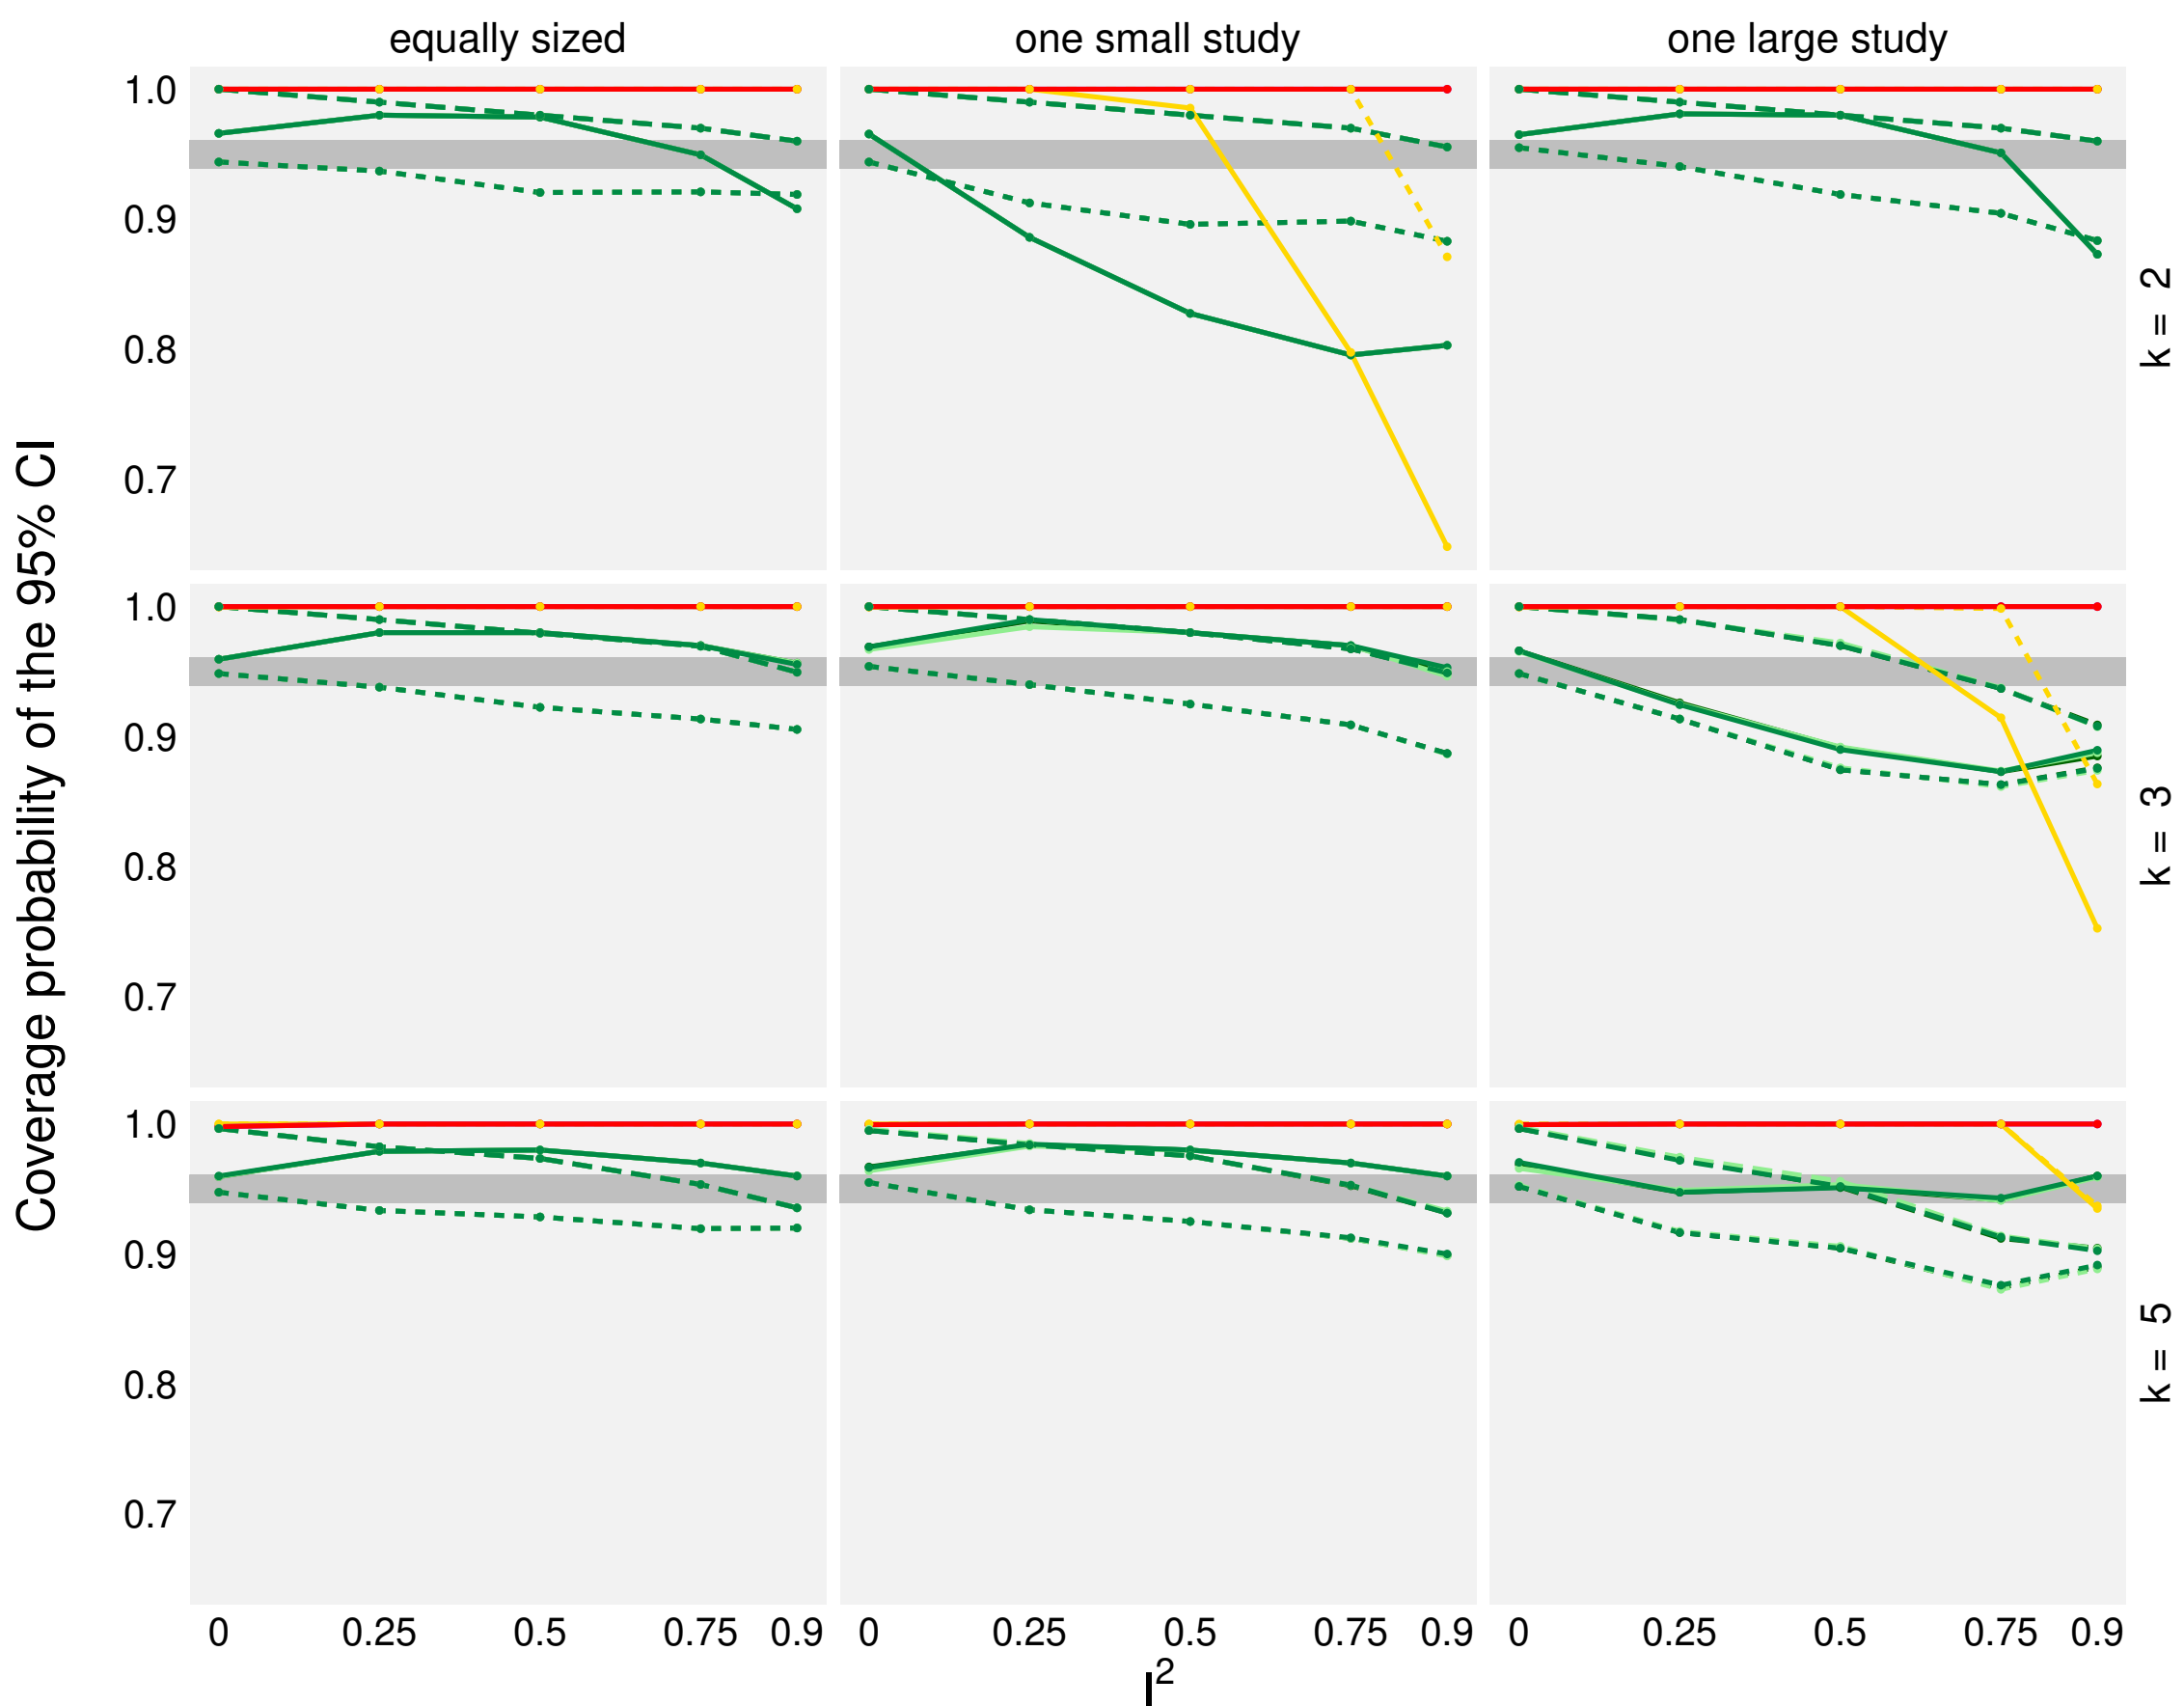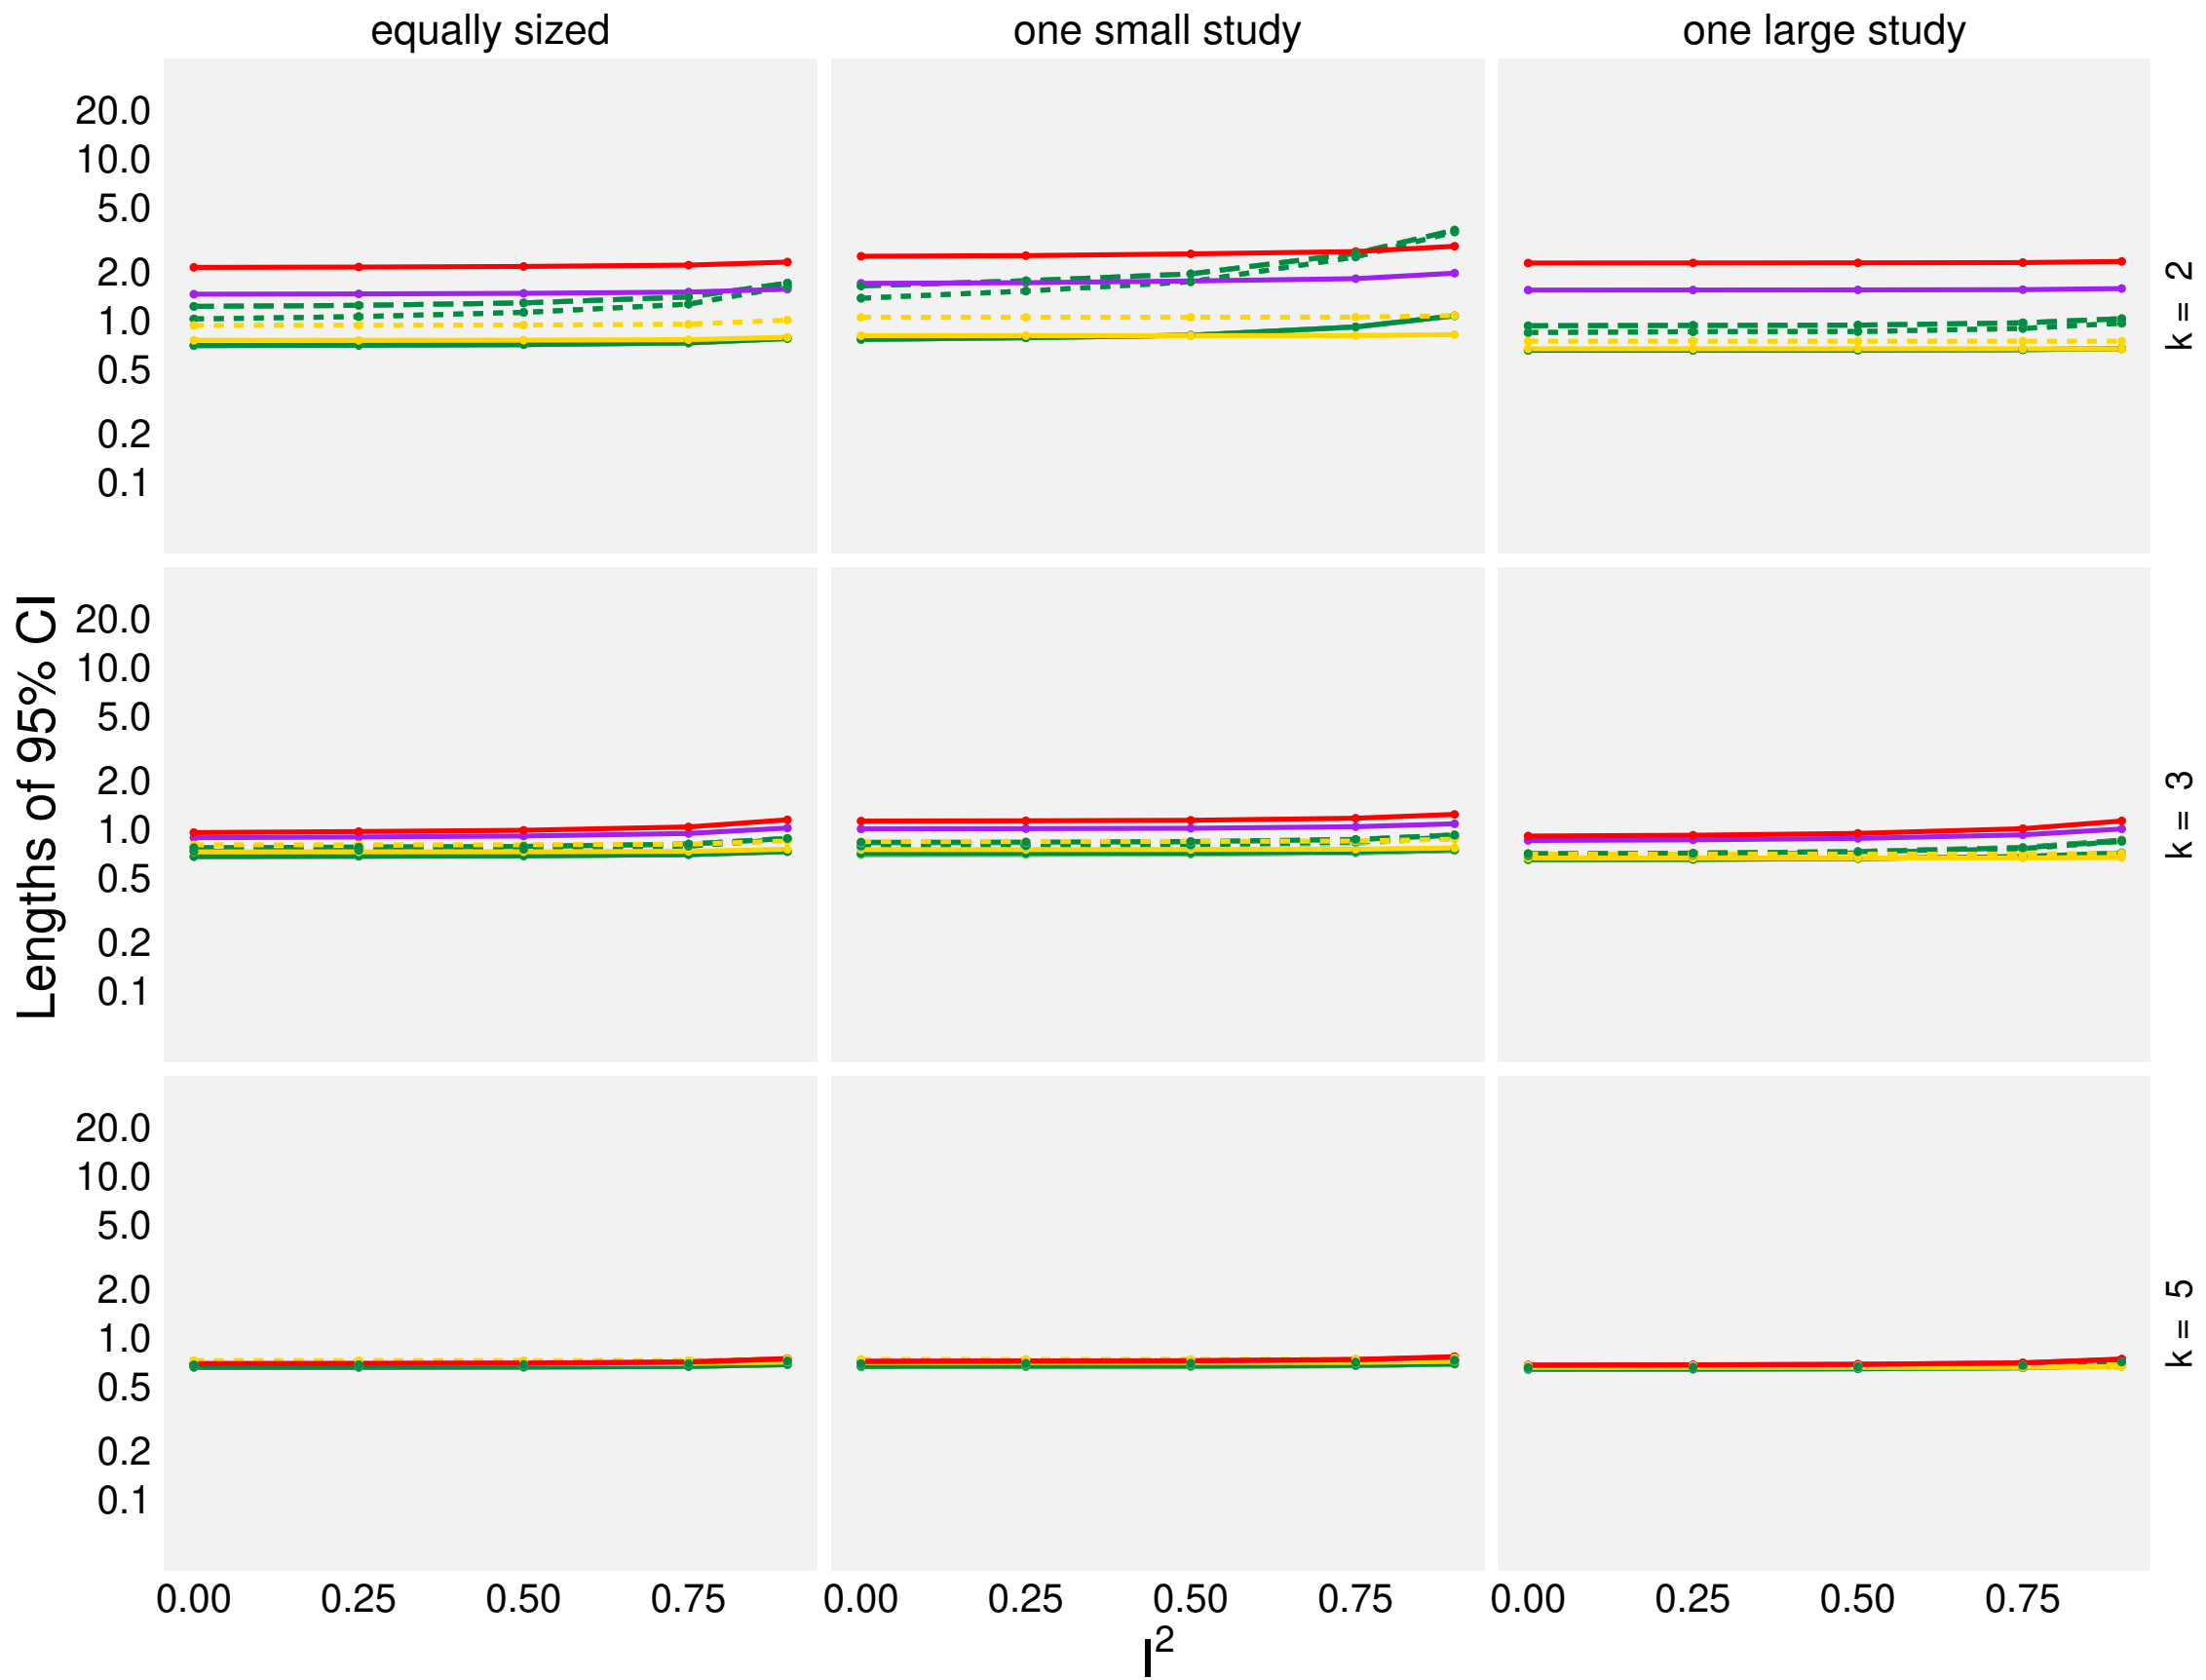

NN - DL  
 NN - REML  
 NN - EB  
 PN - PL  
 NN - Bayes HN(0.5)  
 NN - Bayes HN(1)  
 — normal quantiles  
 -- HKSJ or Student's t  
 ··· mHKSJ
