# Supplementary material for: Likelihood-based meta-analysis with few studies: Empirical and simulation studies
Source: arXiv:1807.09037 source file (2018-10-30)
Supplement: Supplementary file 2 [file Supplement-2.pdf]

OR  
( $n_i=25, \pi_0=0.1$ )

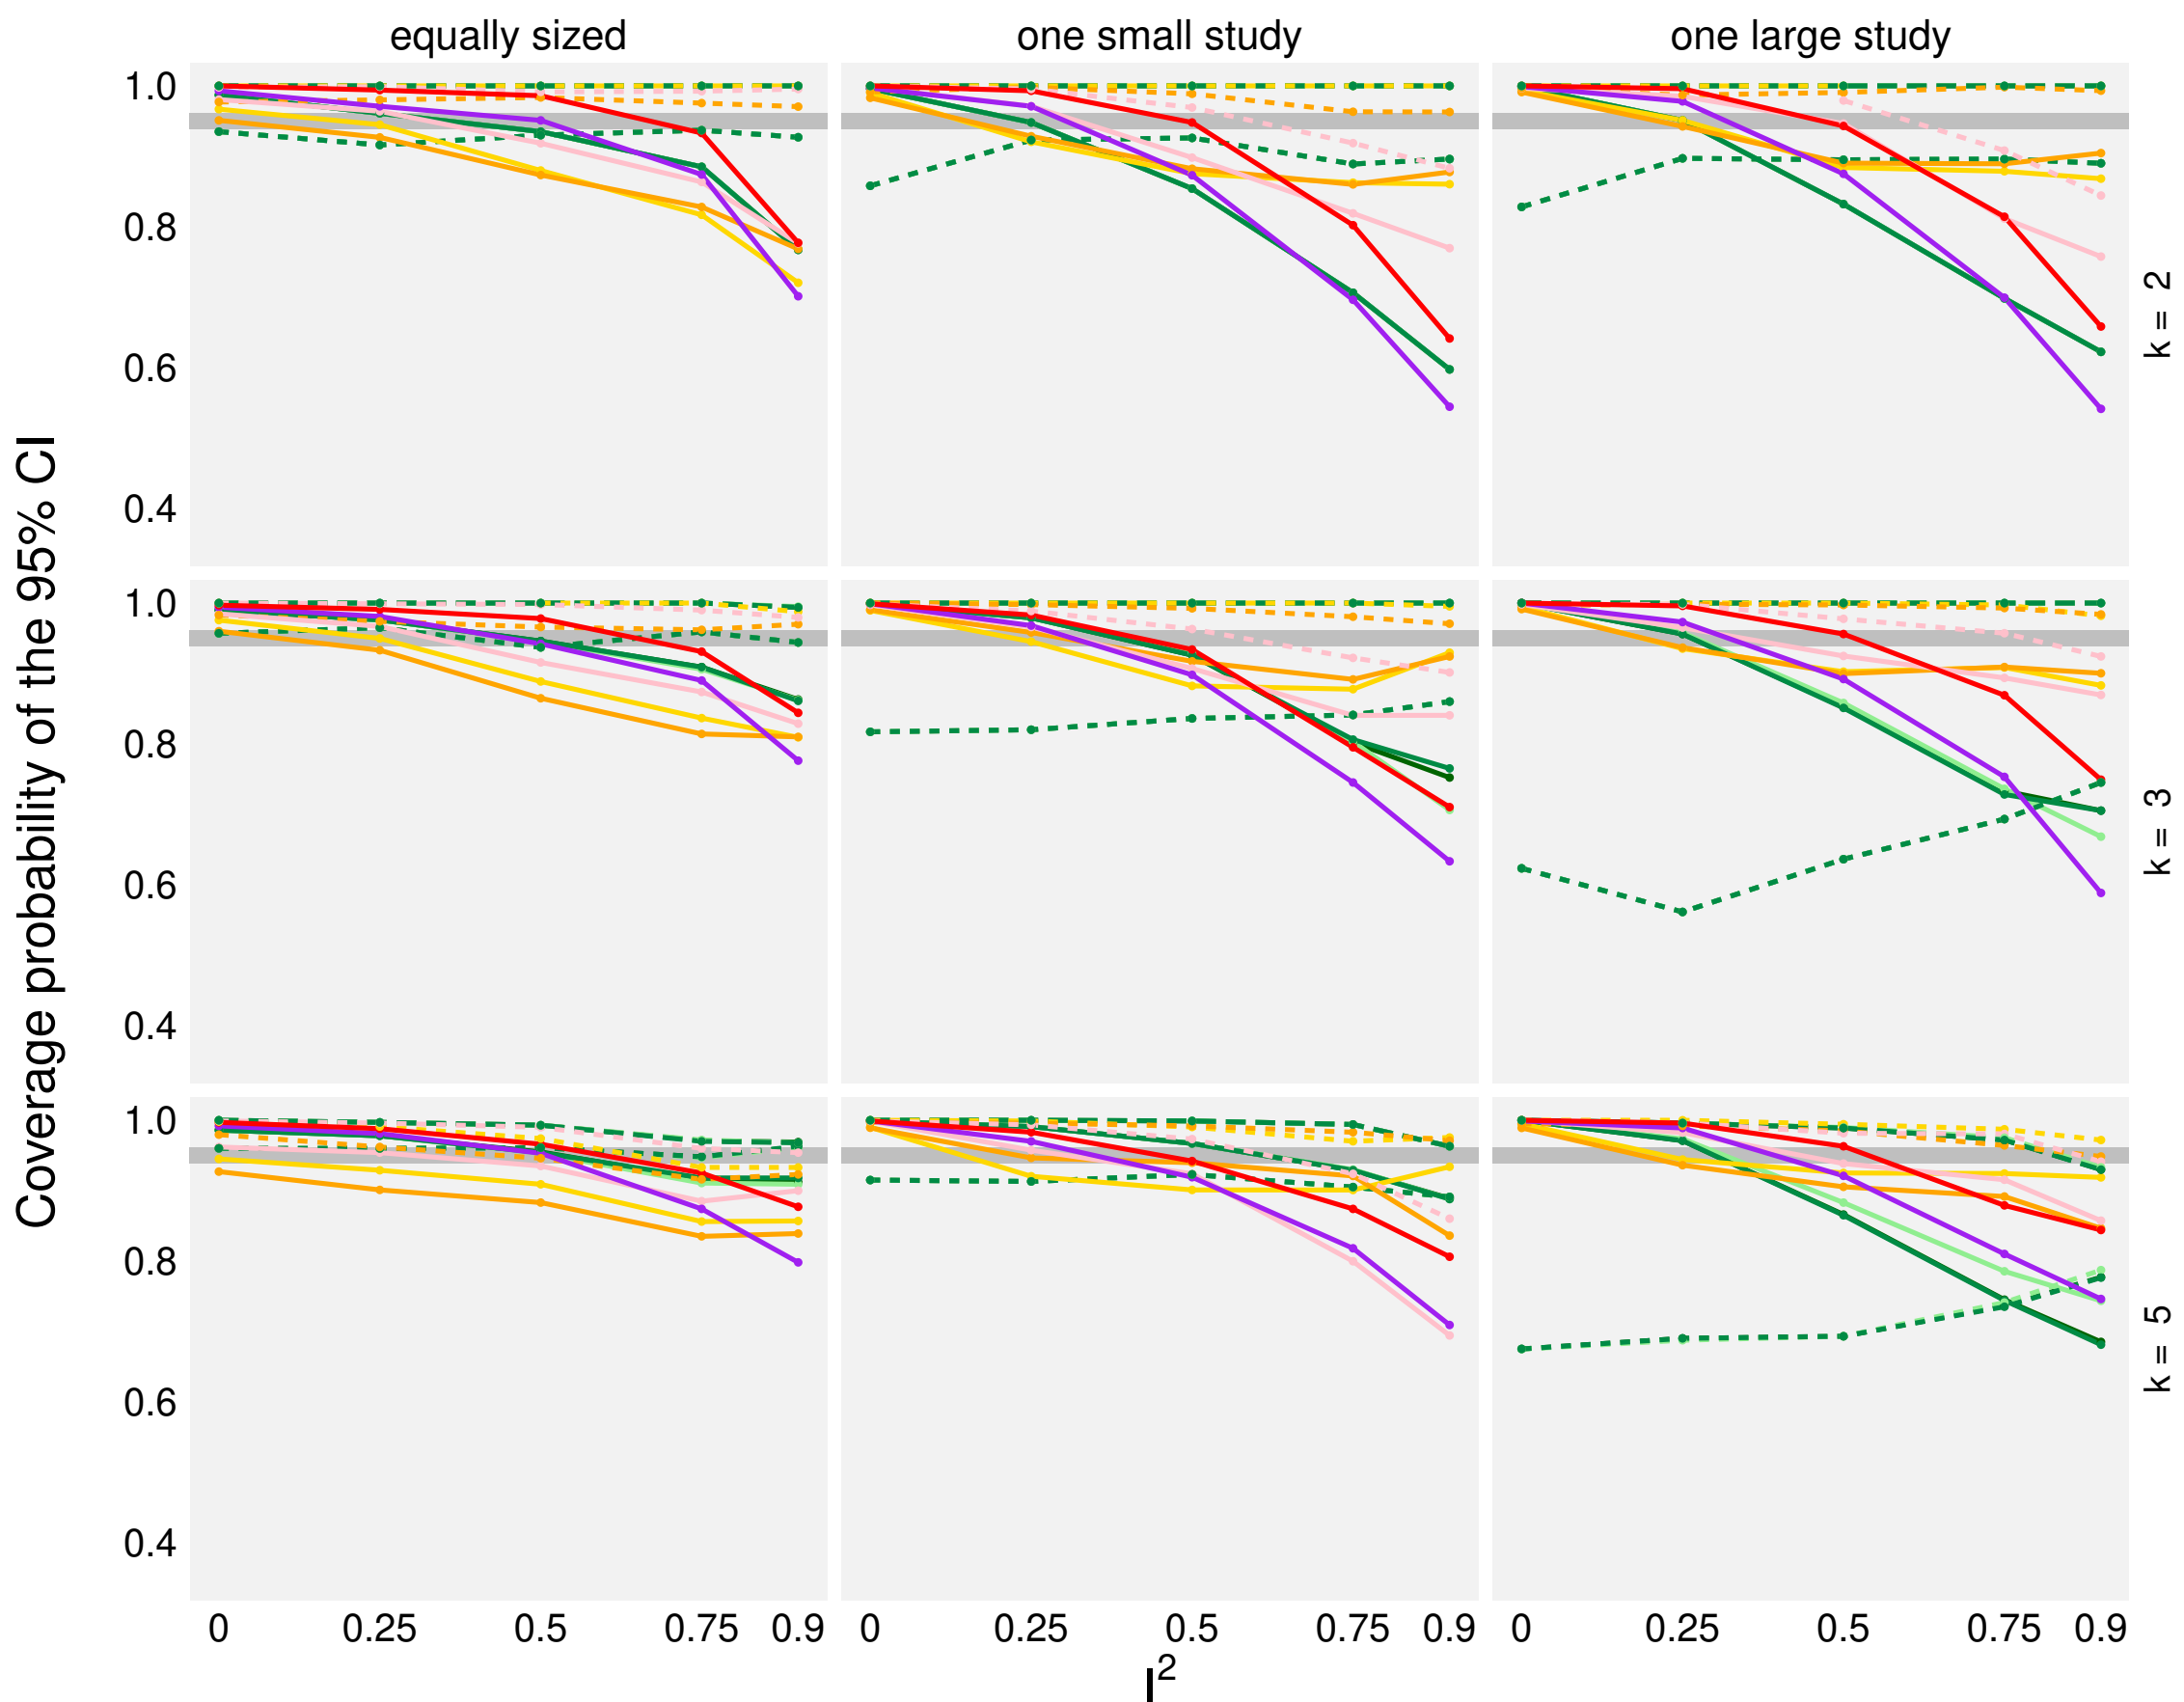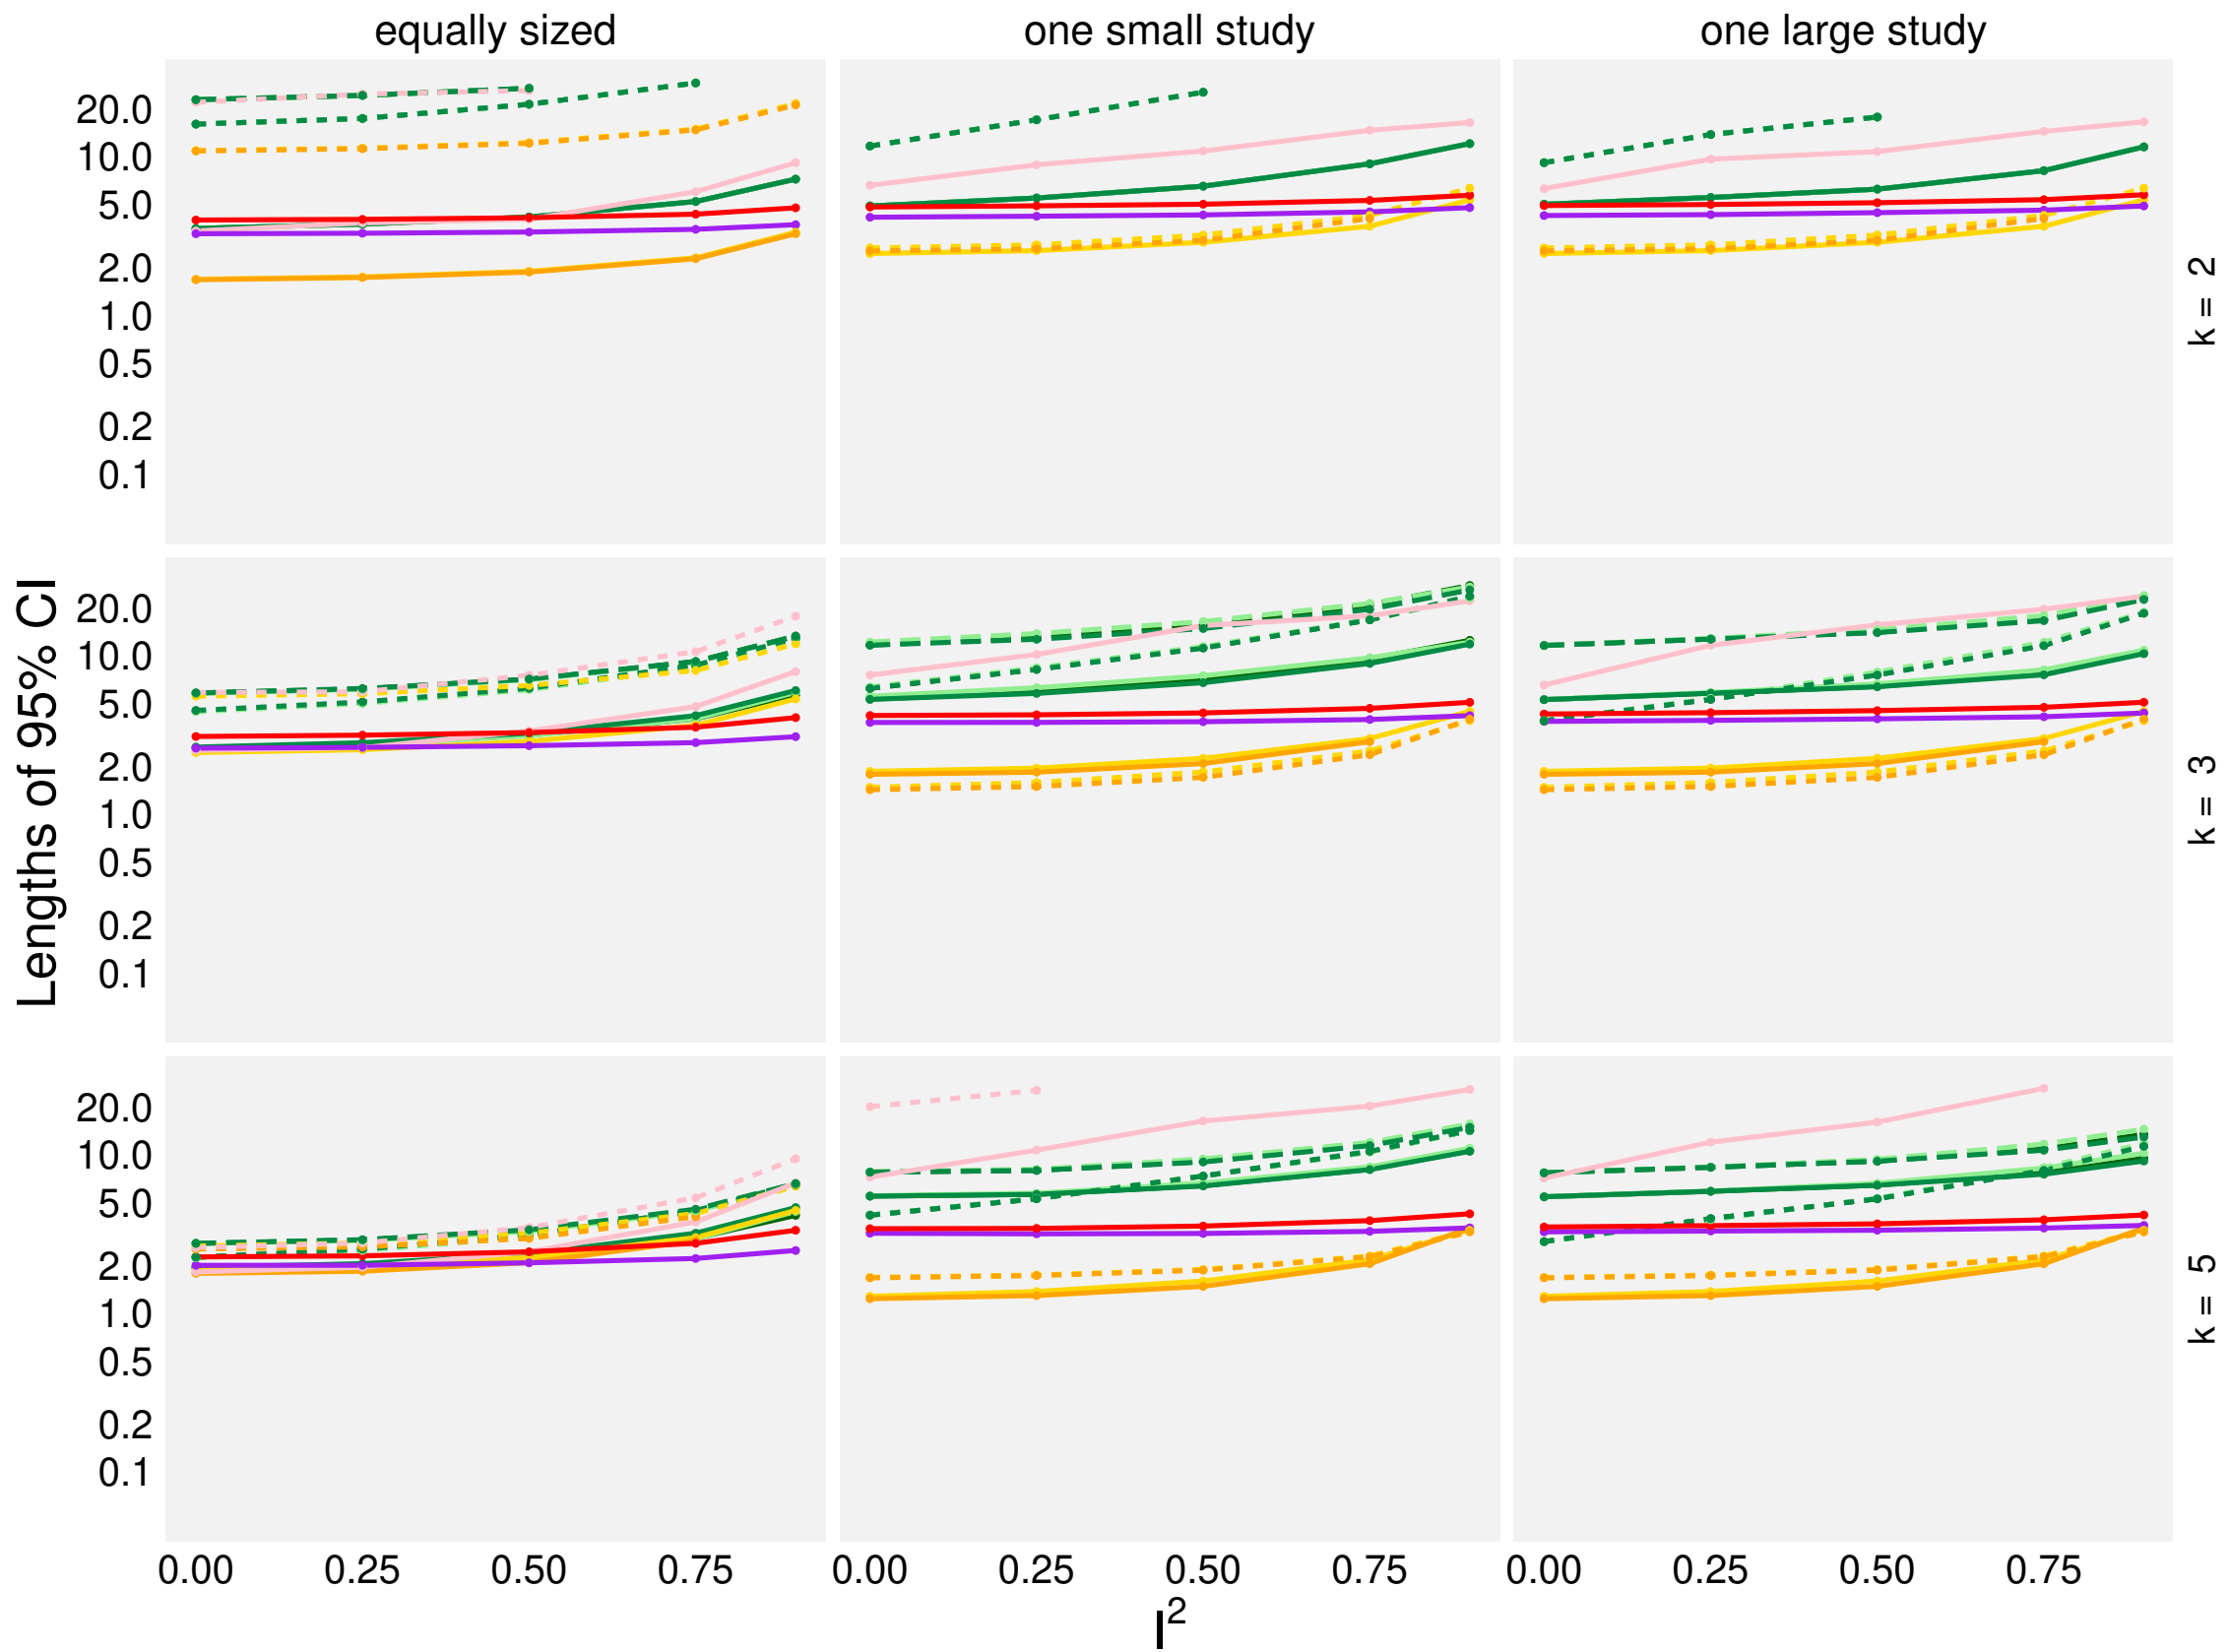

— NN — DL      — BN — UM.RS      — normal quantiles  
 — NN — REML      — BN — CM.AL      -- HKSJ or Student's t  
 — NN — EB      — NN — Bayes HN(0.5)      -- mHKSJ  
 — BN — UM.FS      — NN — Bayes HN(1)

OR  
( $n_i=25, \pi_0=0.3$ )

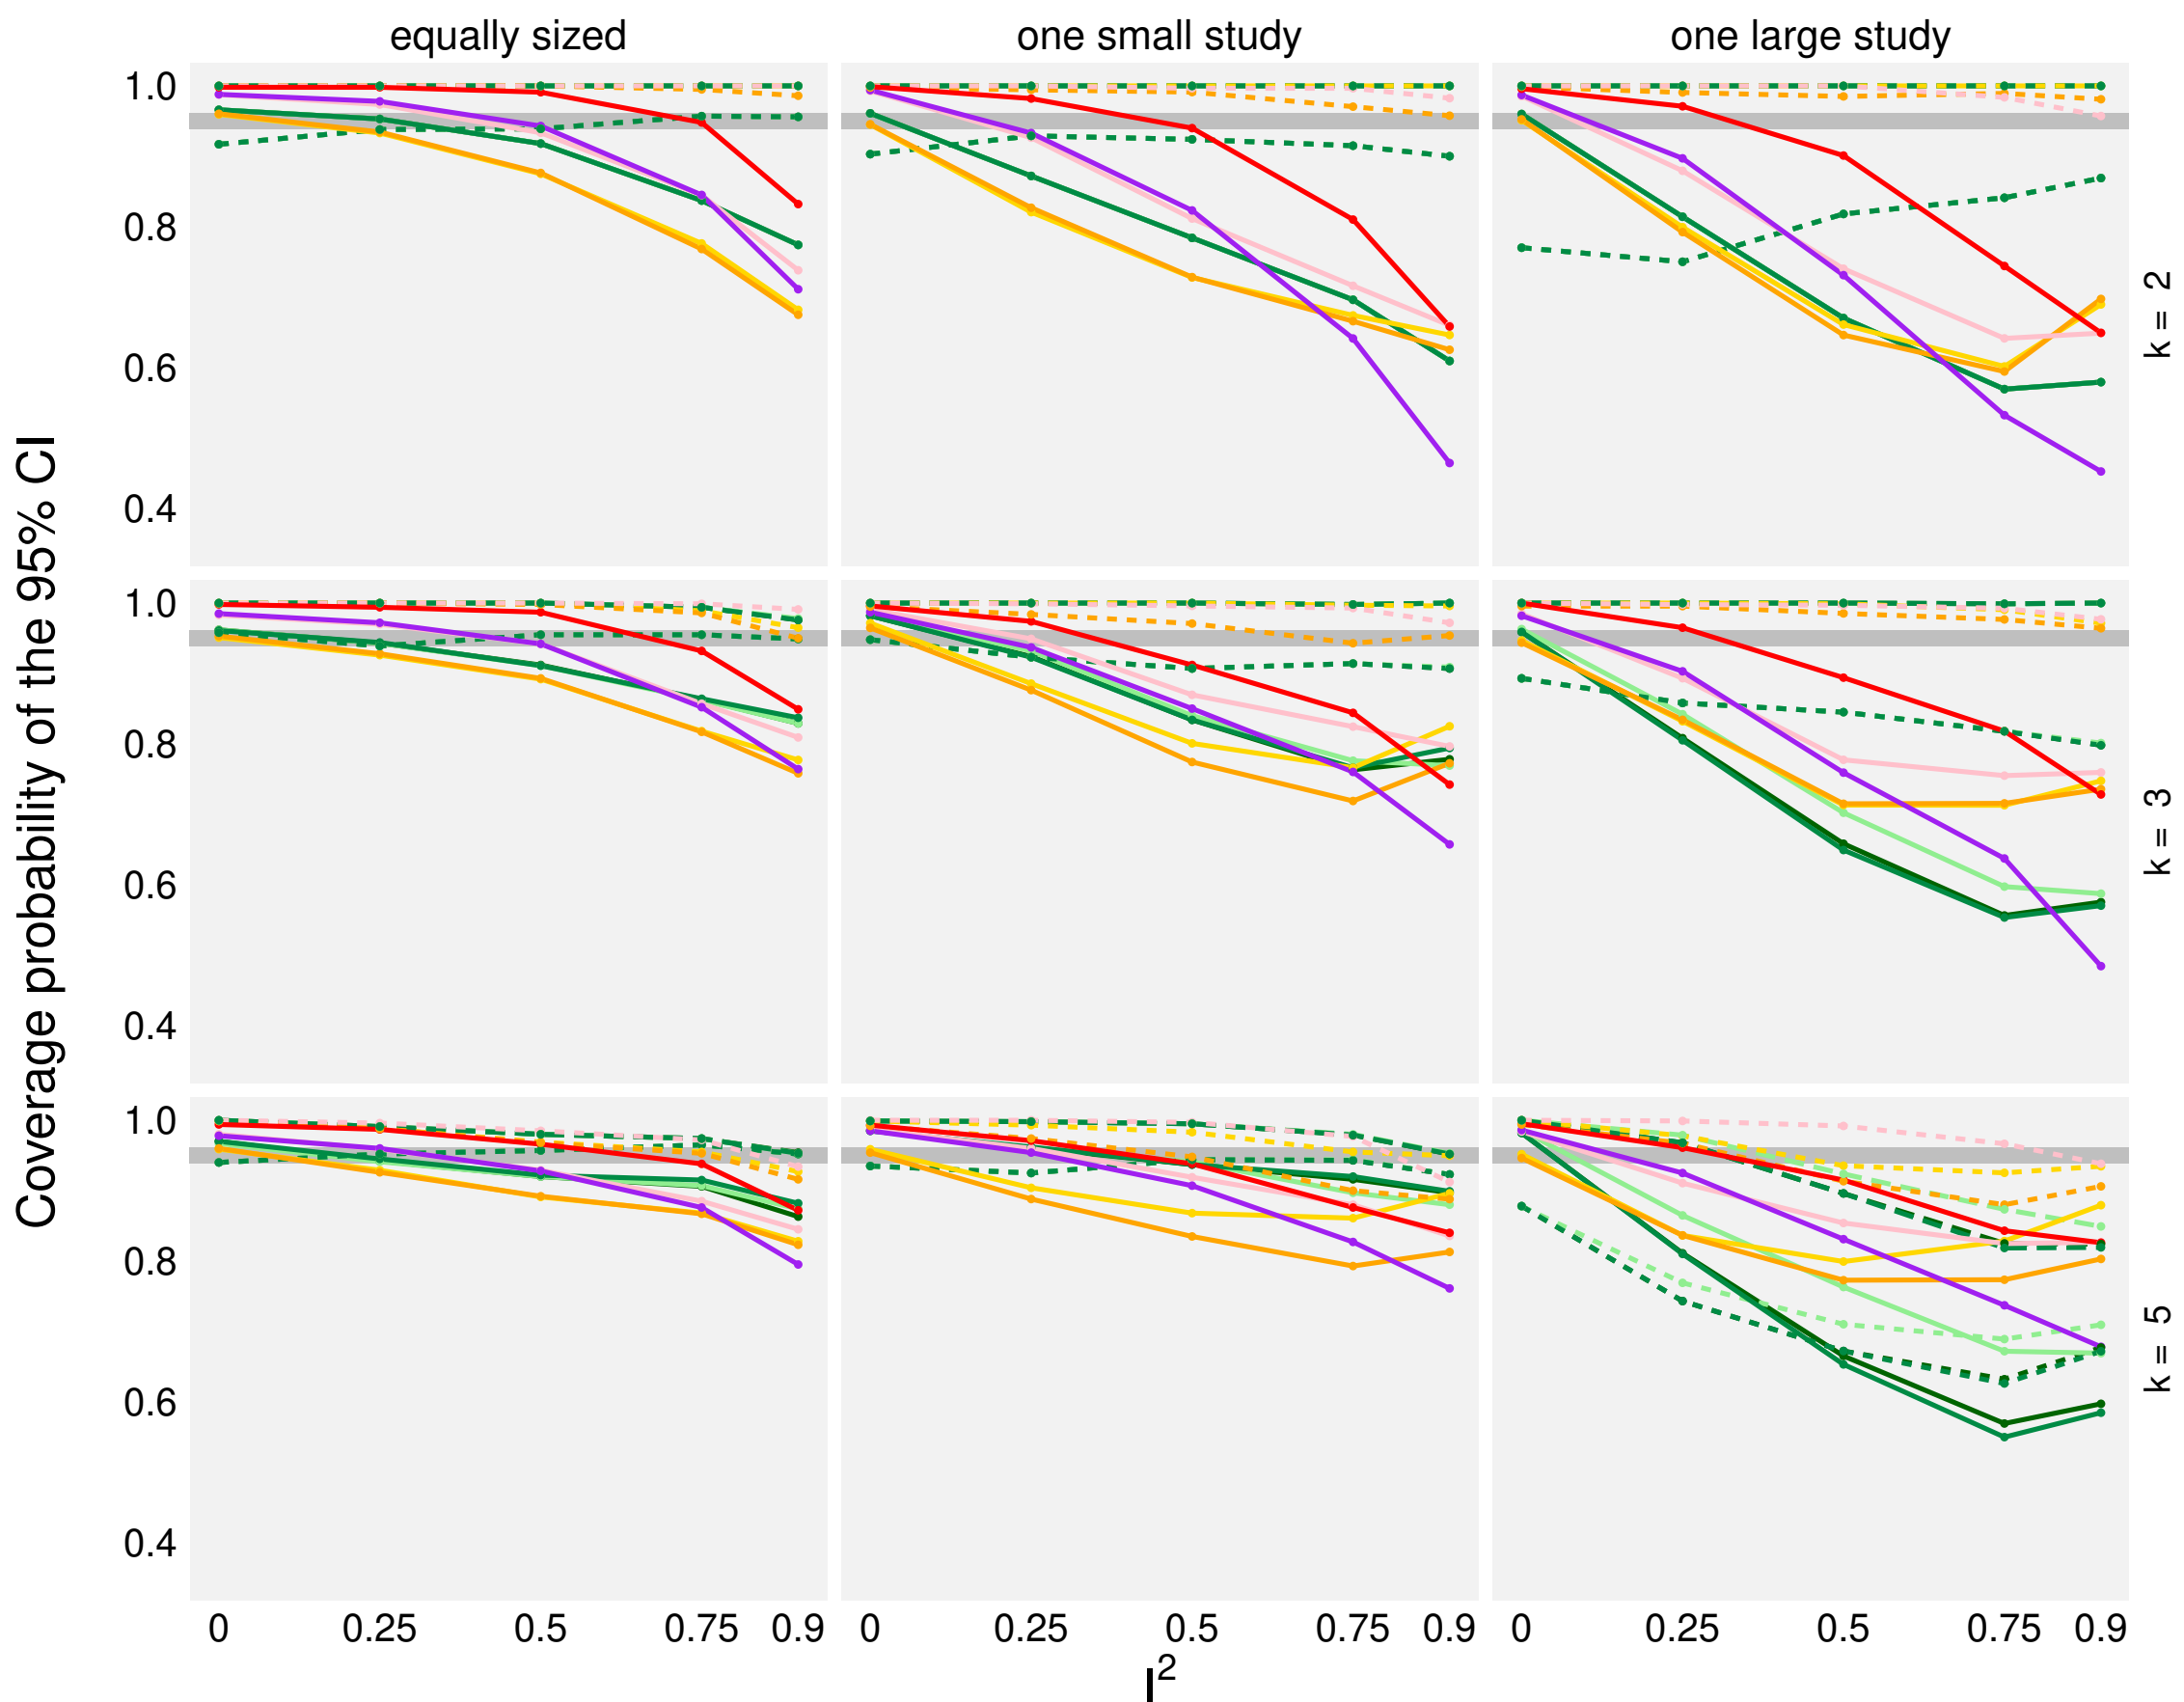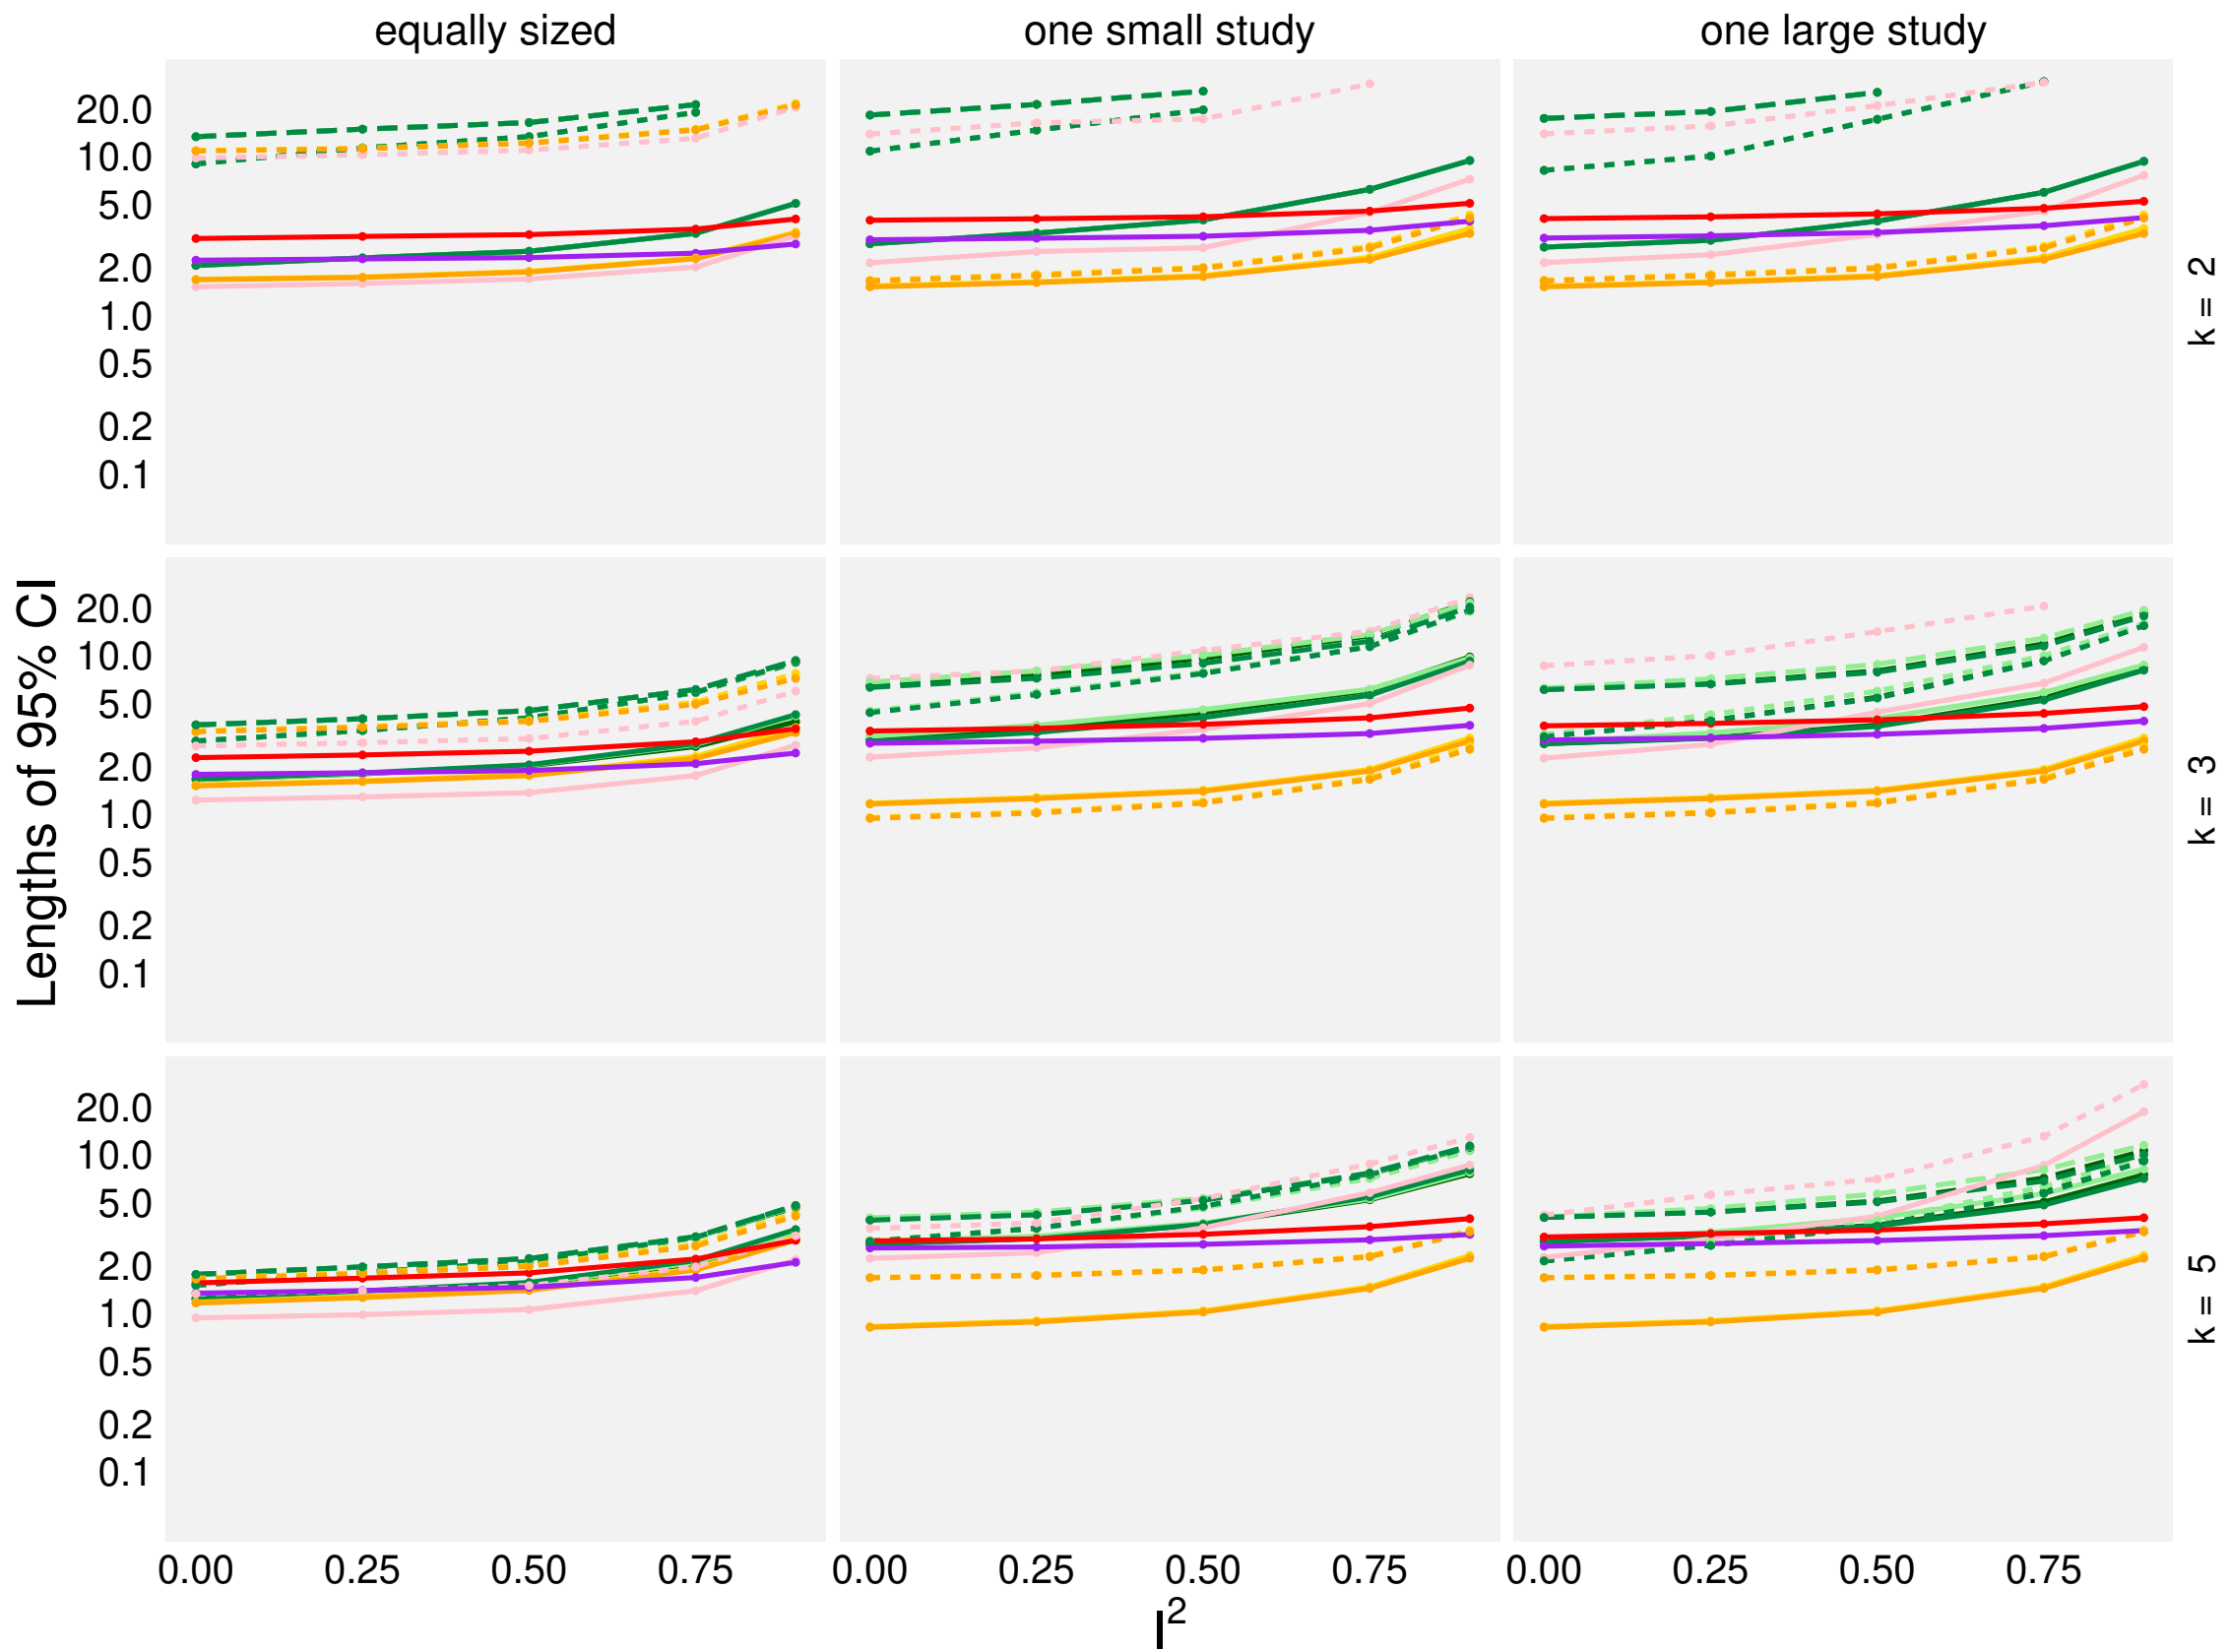

— NN — DL  
 — NN — REML  
 — NN — EB  
 — BN — UM.FS  
 — BN — UM.RS  
 — BN — CM.AL  
 — NN — Bayes HN(0.5)  
 — NN — Bayes HN(1)

— normal quantiles  
 - - HKSJ or Student's t  
 - · mHKSJ

OR  
( $n_i=25, \pi_0=0.5$ )

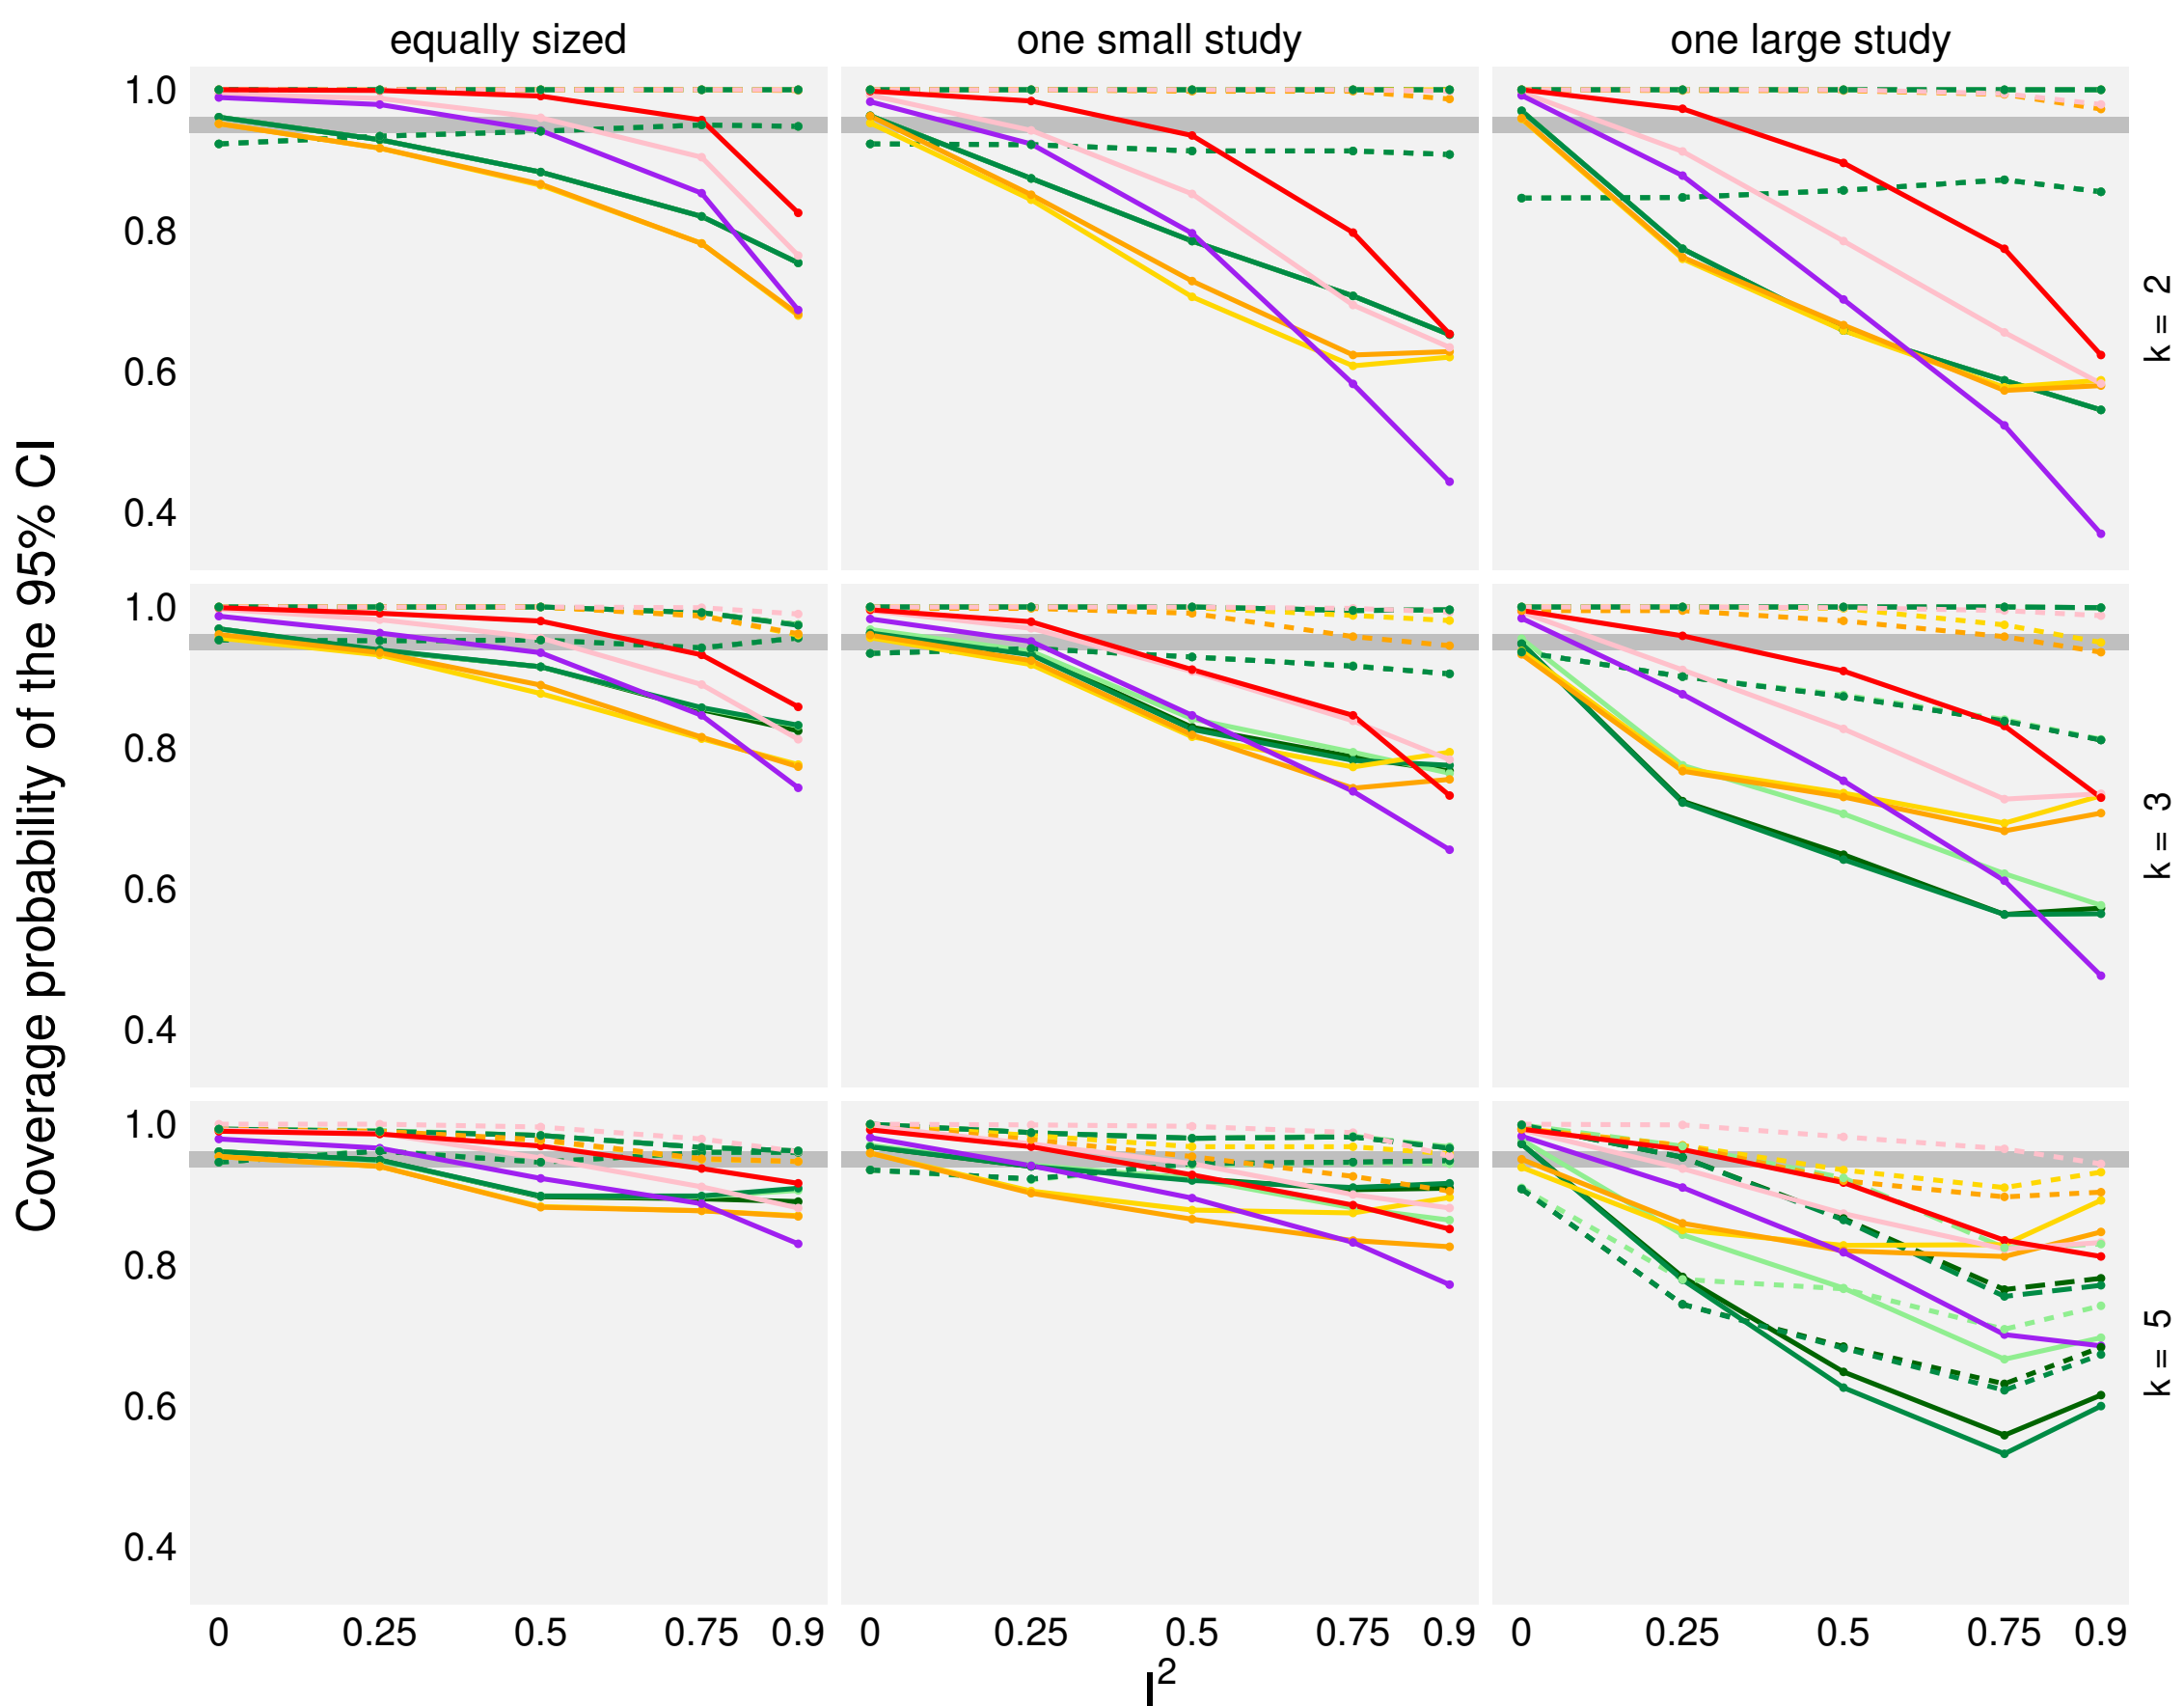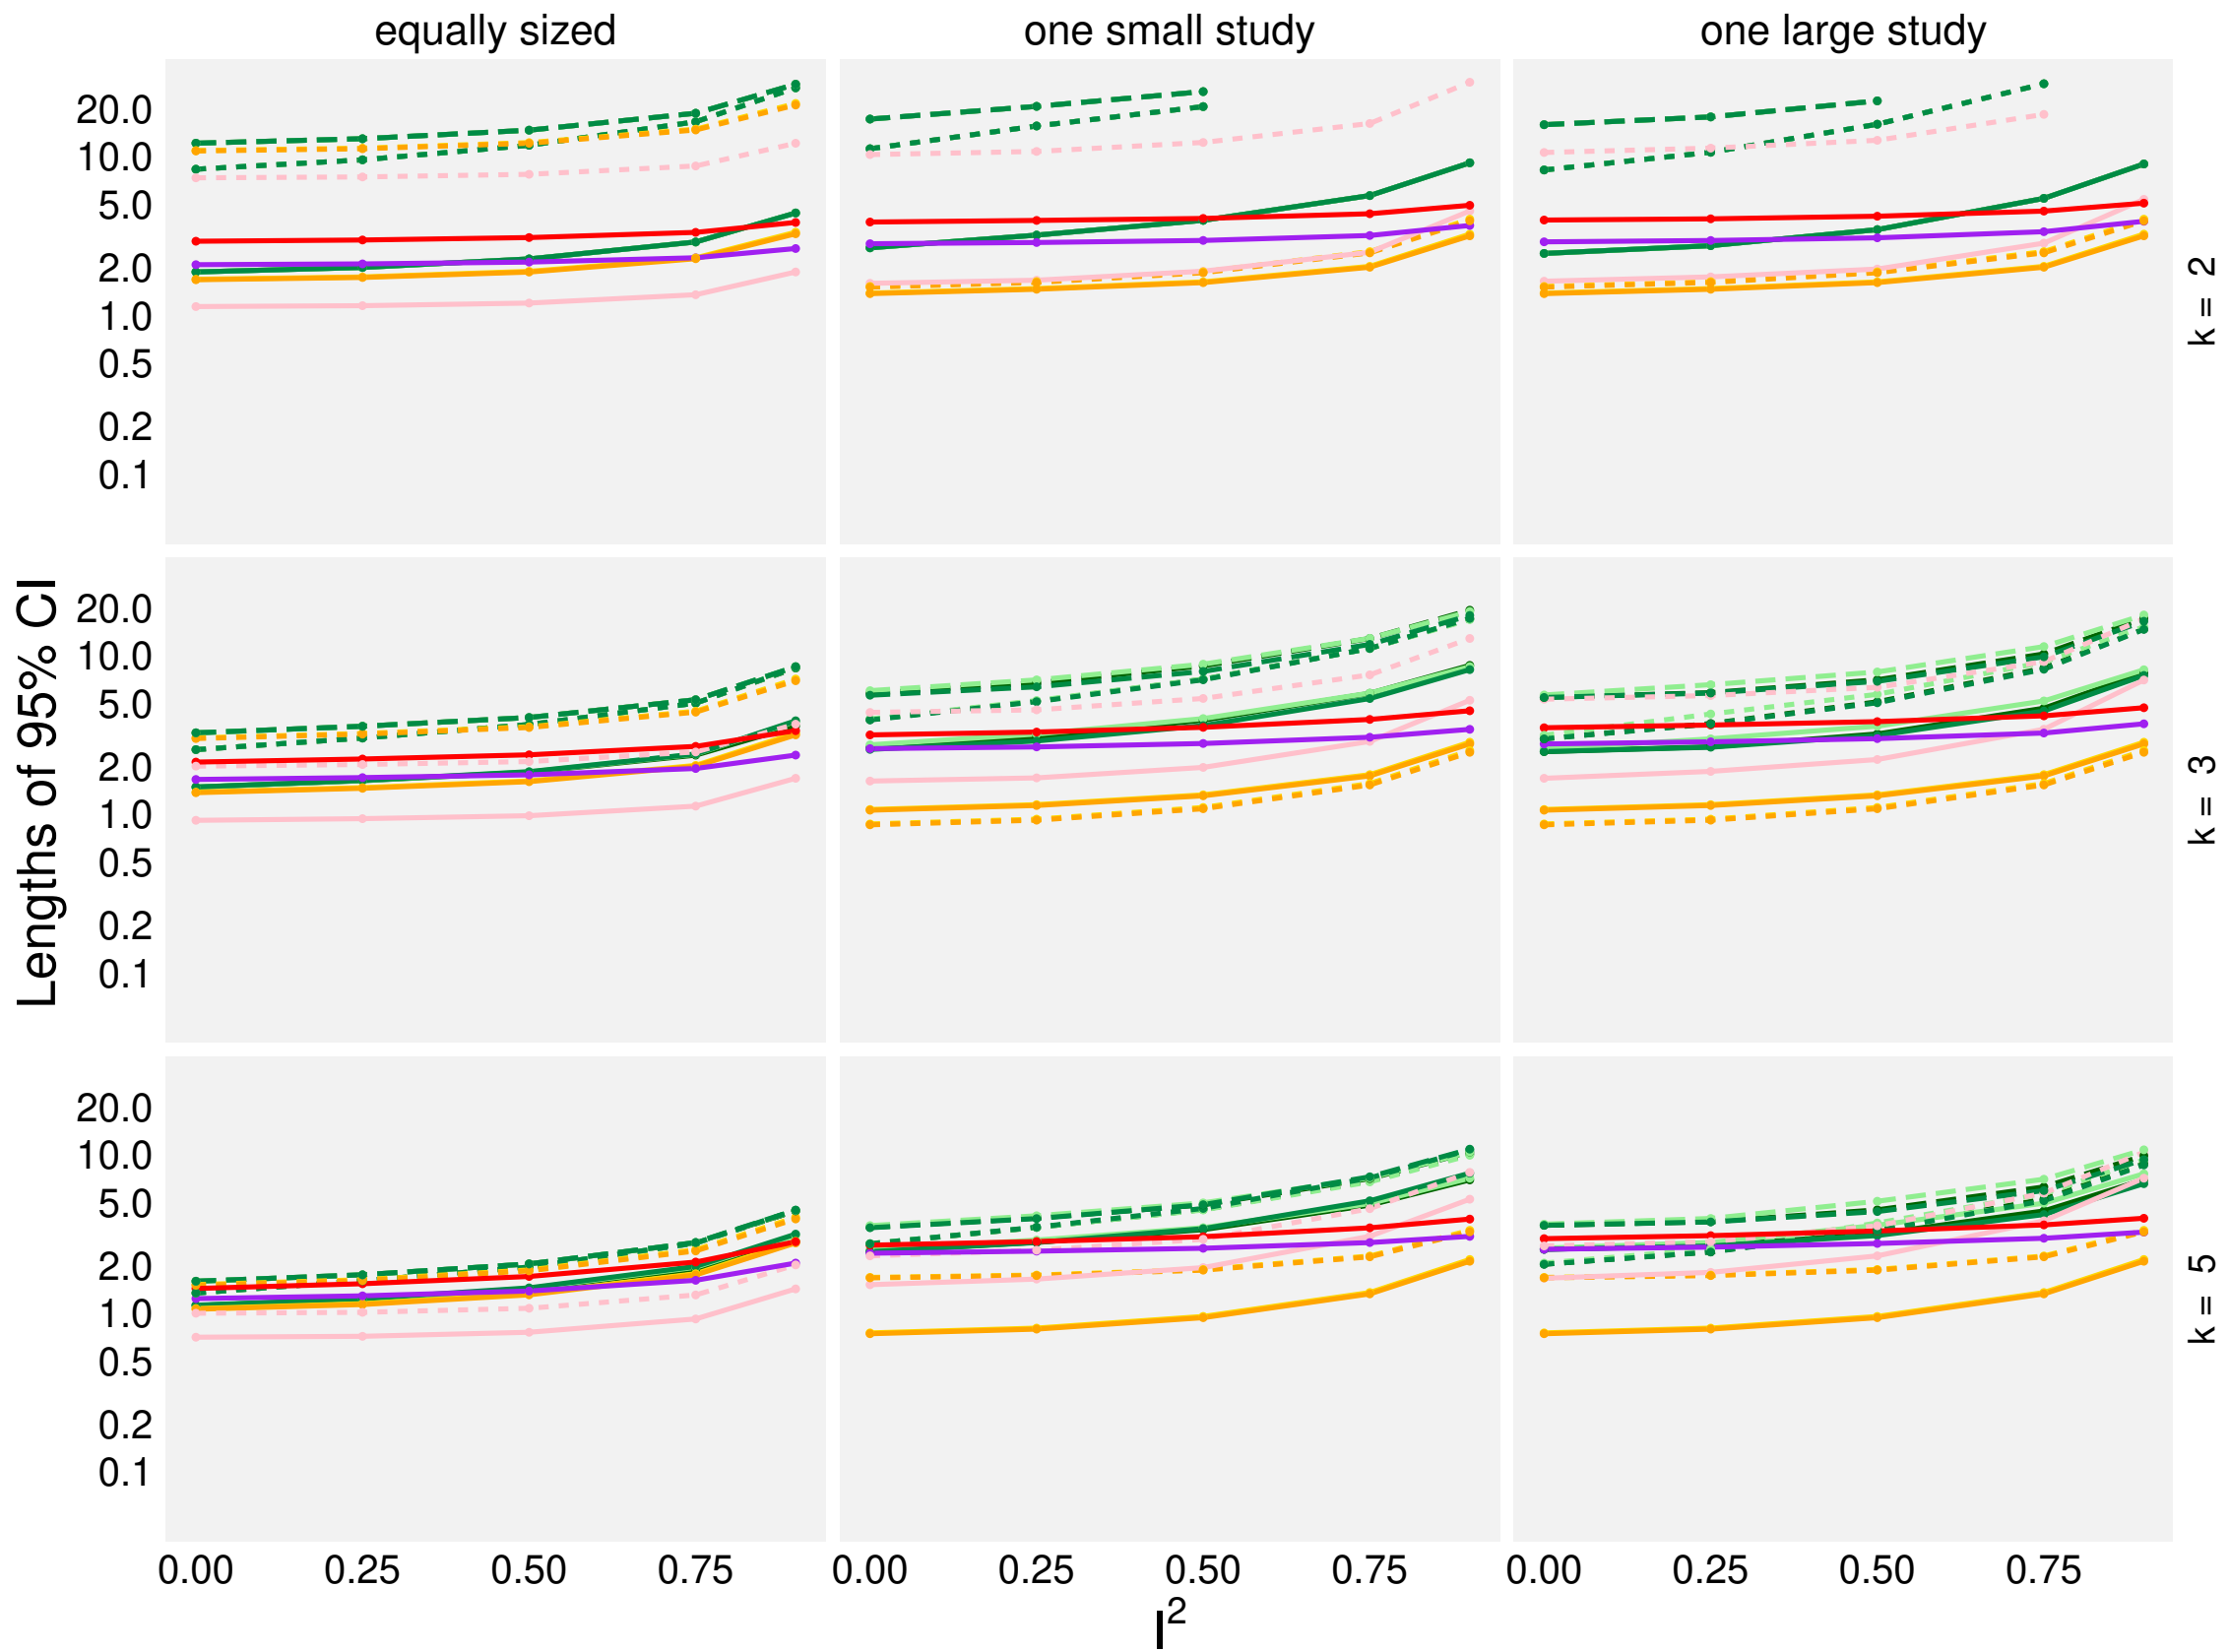

— NN — DL  
 — NN — REML  
 — NN — EB  
 — BN — UM.FS  
 — BN — UM.RS  
 — BN — CM.AL  
 — NN — Bayes HN(0.5)  
 — NN — Bayes HN(1)

— normal quantiles  
 - - HKSJ or Student's t  
 - - mHKSJ

OR  
( $n_i=25, \pi_0=0.7$ )

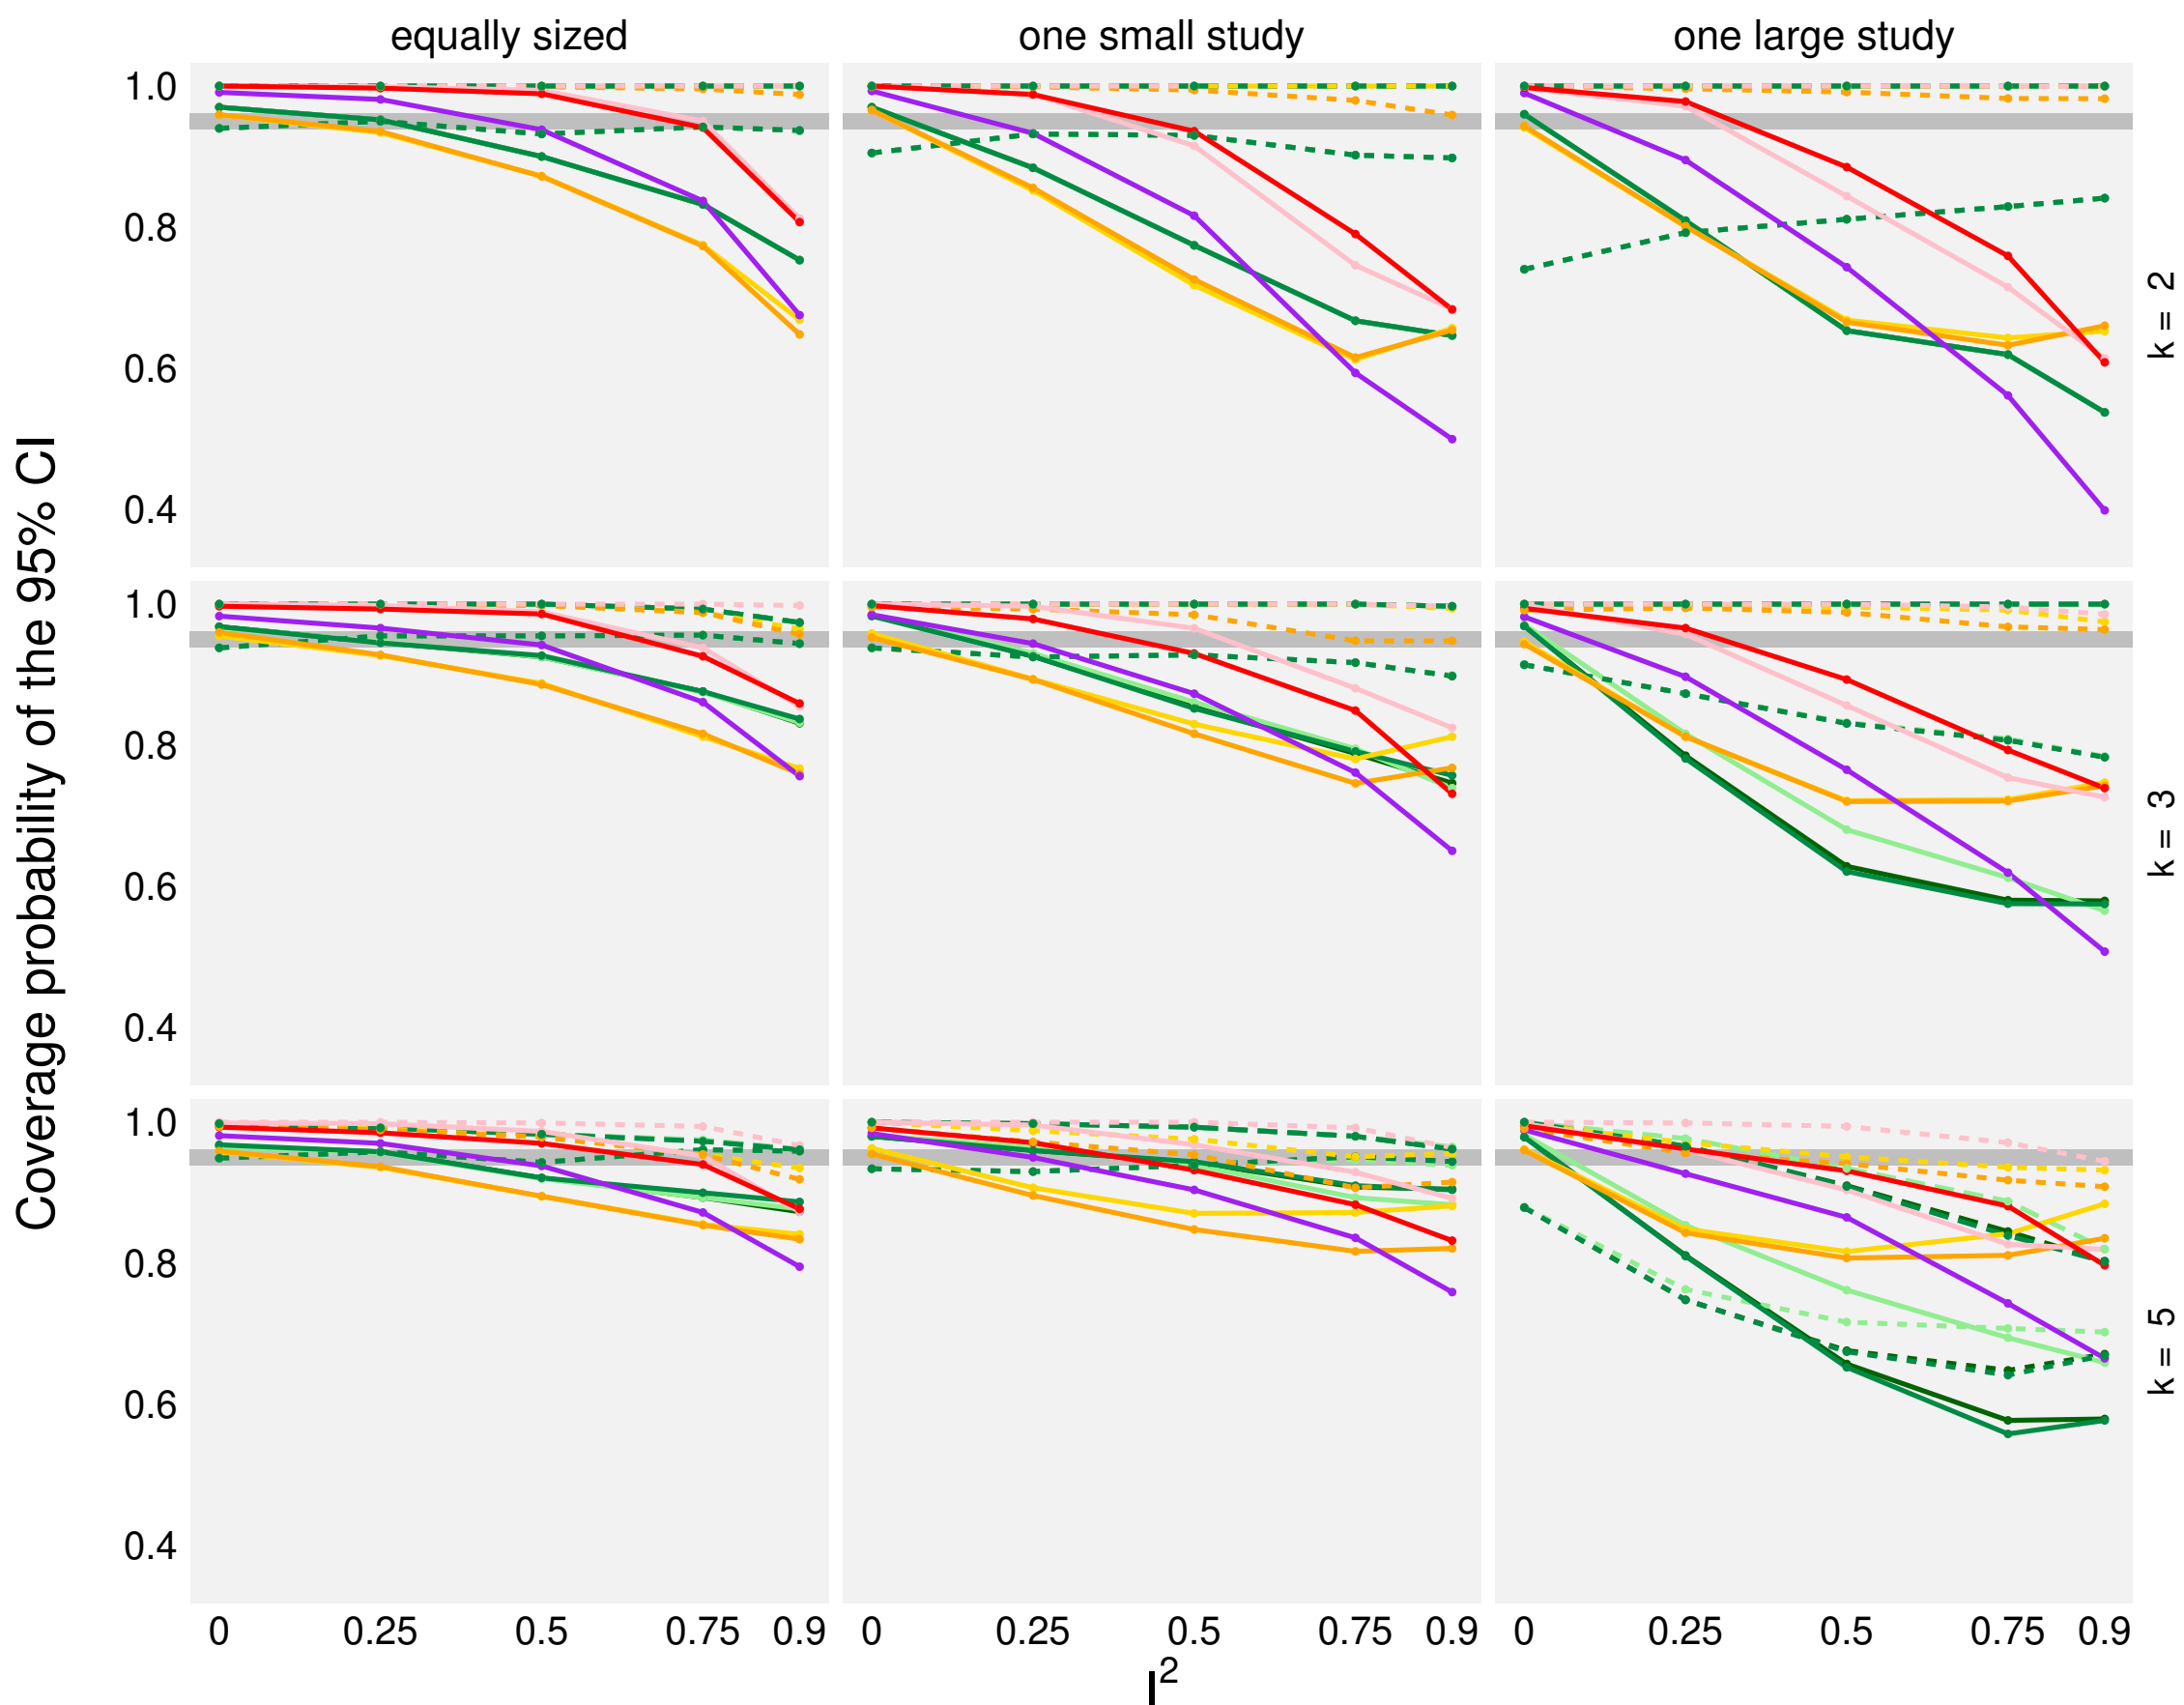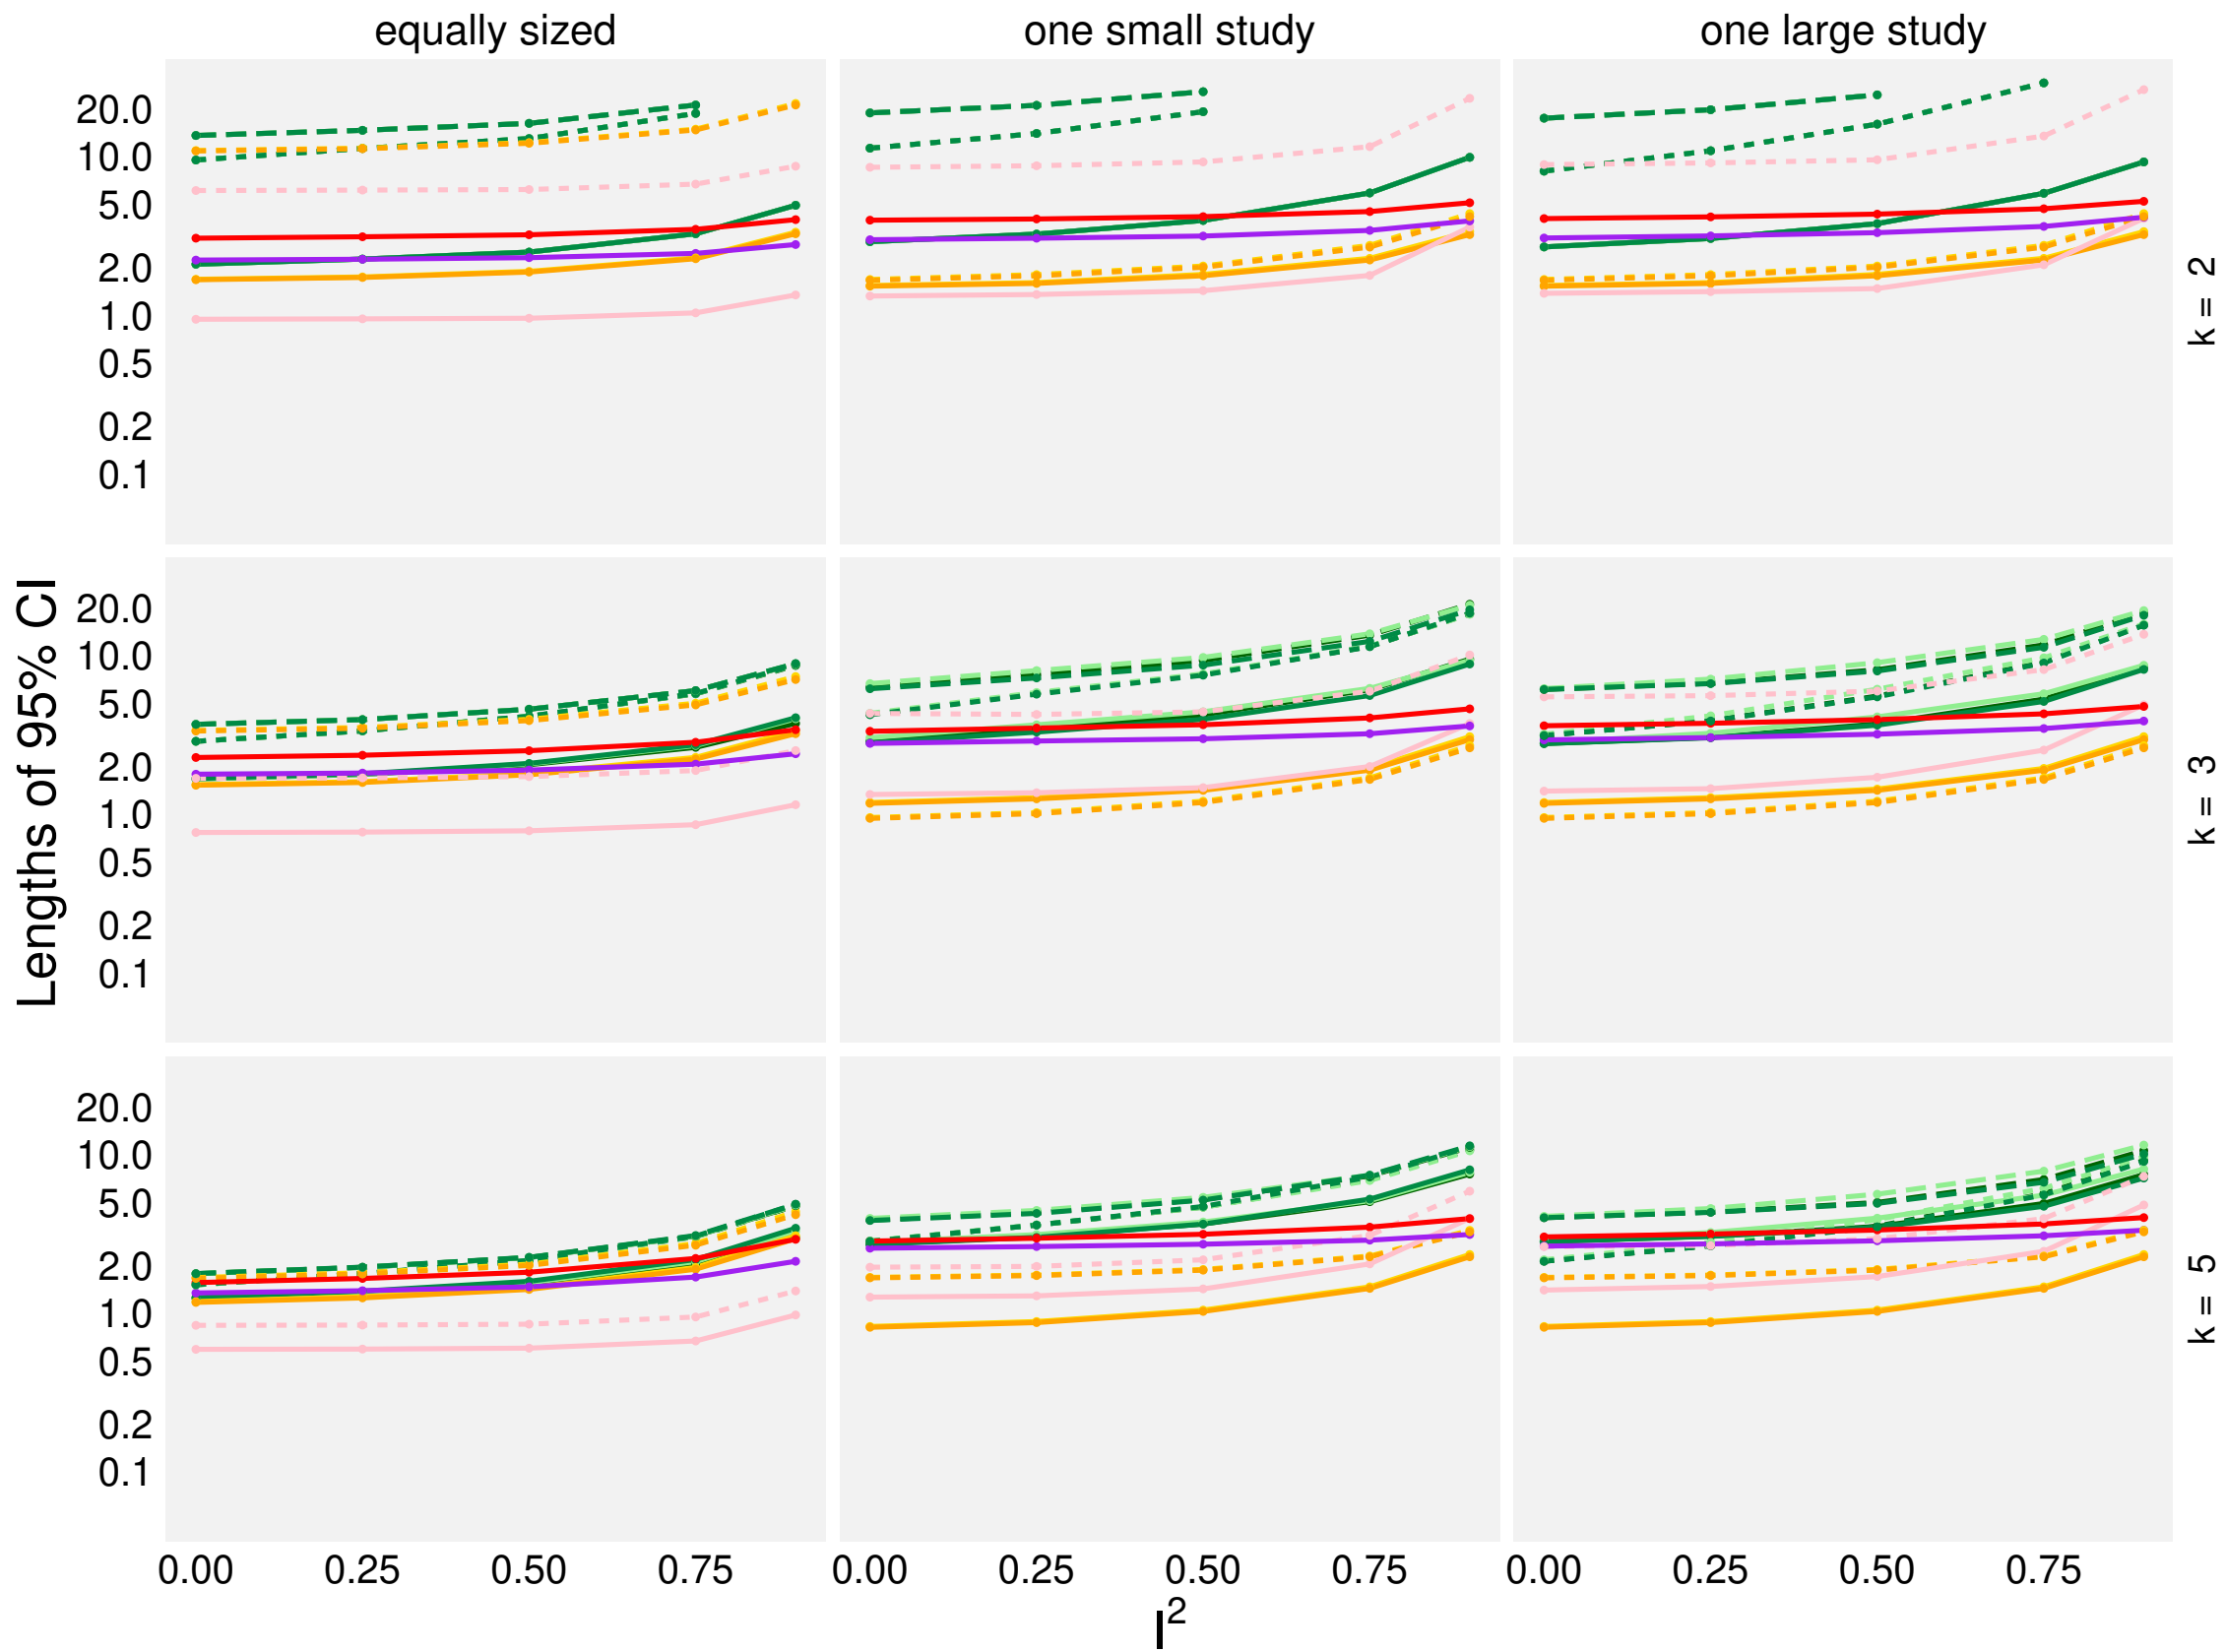

— NN — DL  
 — NN — REML  
 — NN — EB  
 — BN — UM.FS  
 — BN — UM.RS  
 — BN — CM.AL  
 — NN — Bayes HN(0.5)  
 — NN — Bayes HN(1)

— normal quantiles  
 - - HKSJ or Student's t  
 - - mHKSJ

OR  
( $n_i=25, \pi_0=0.9$ )

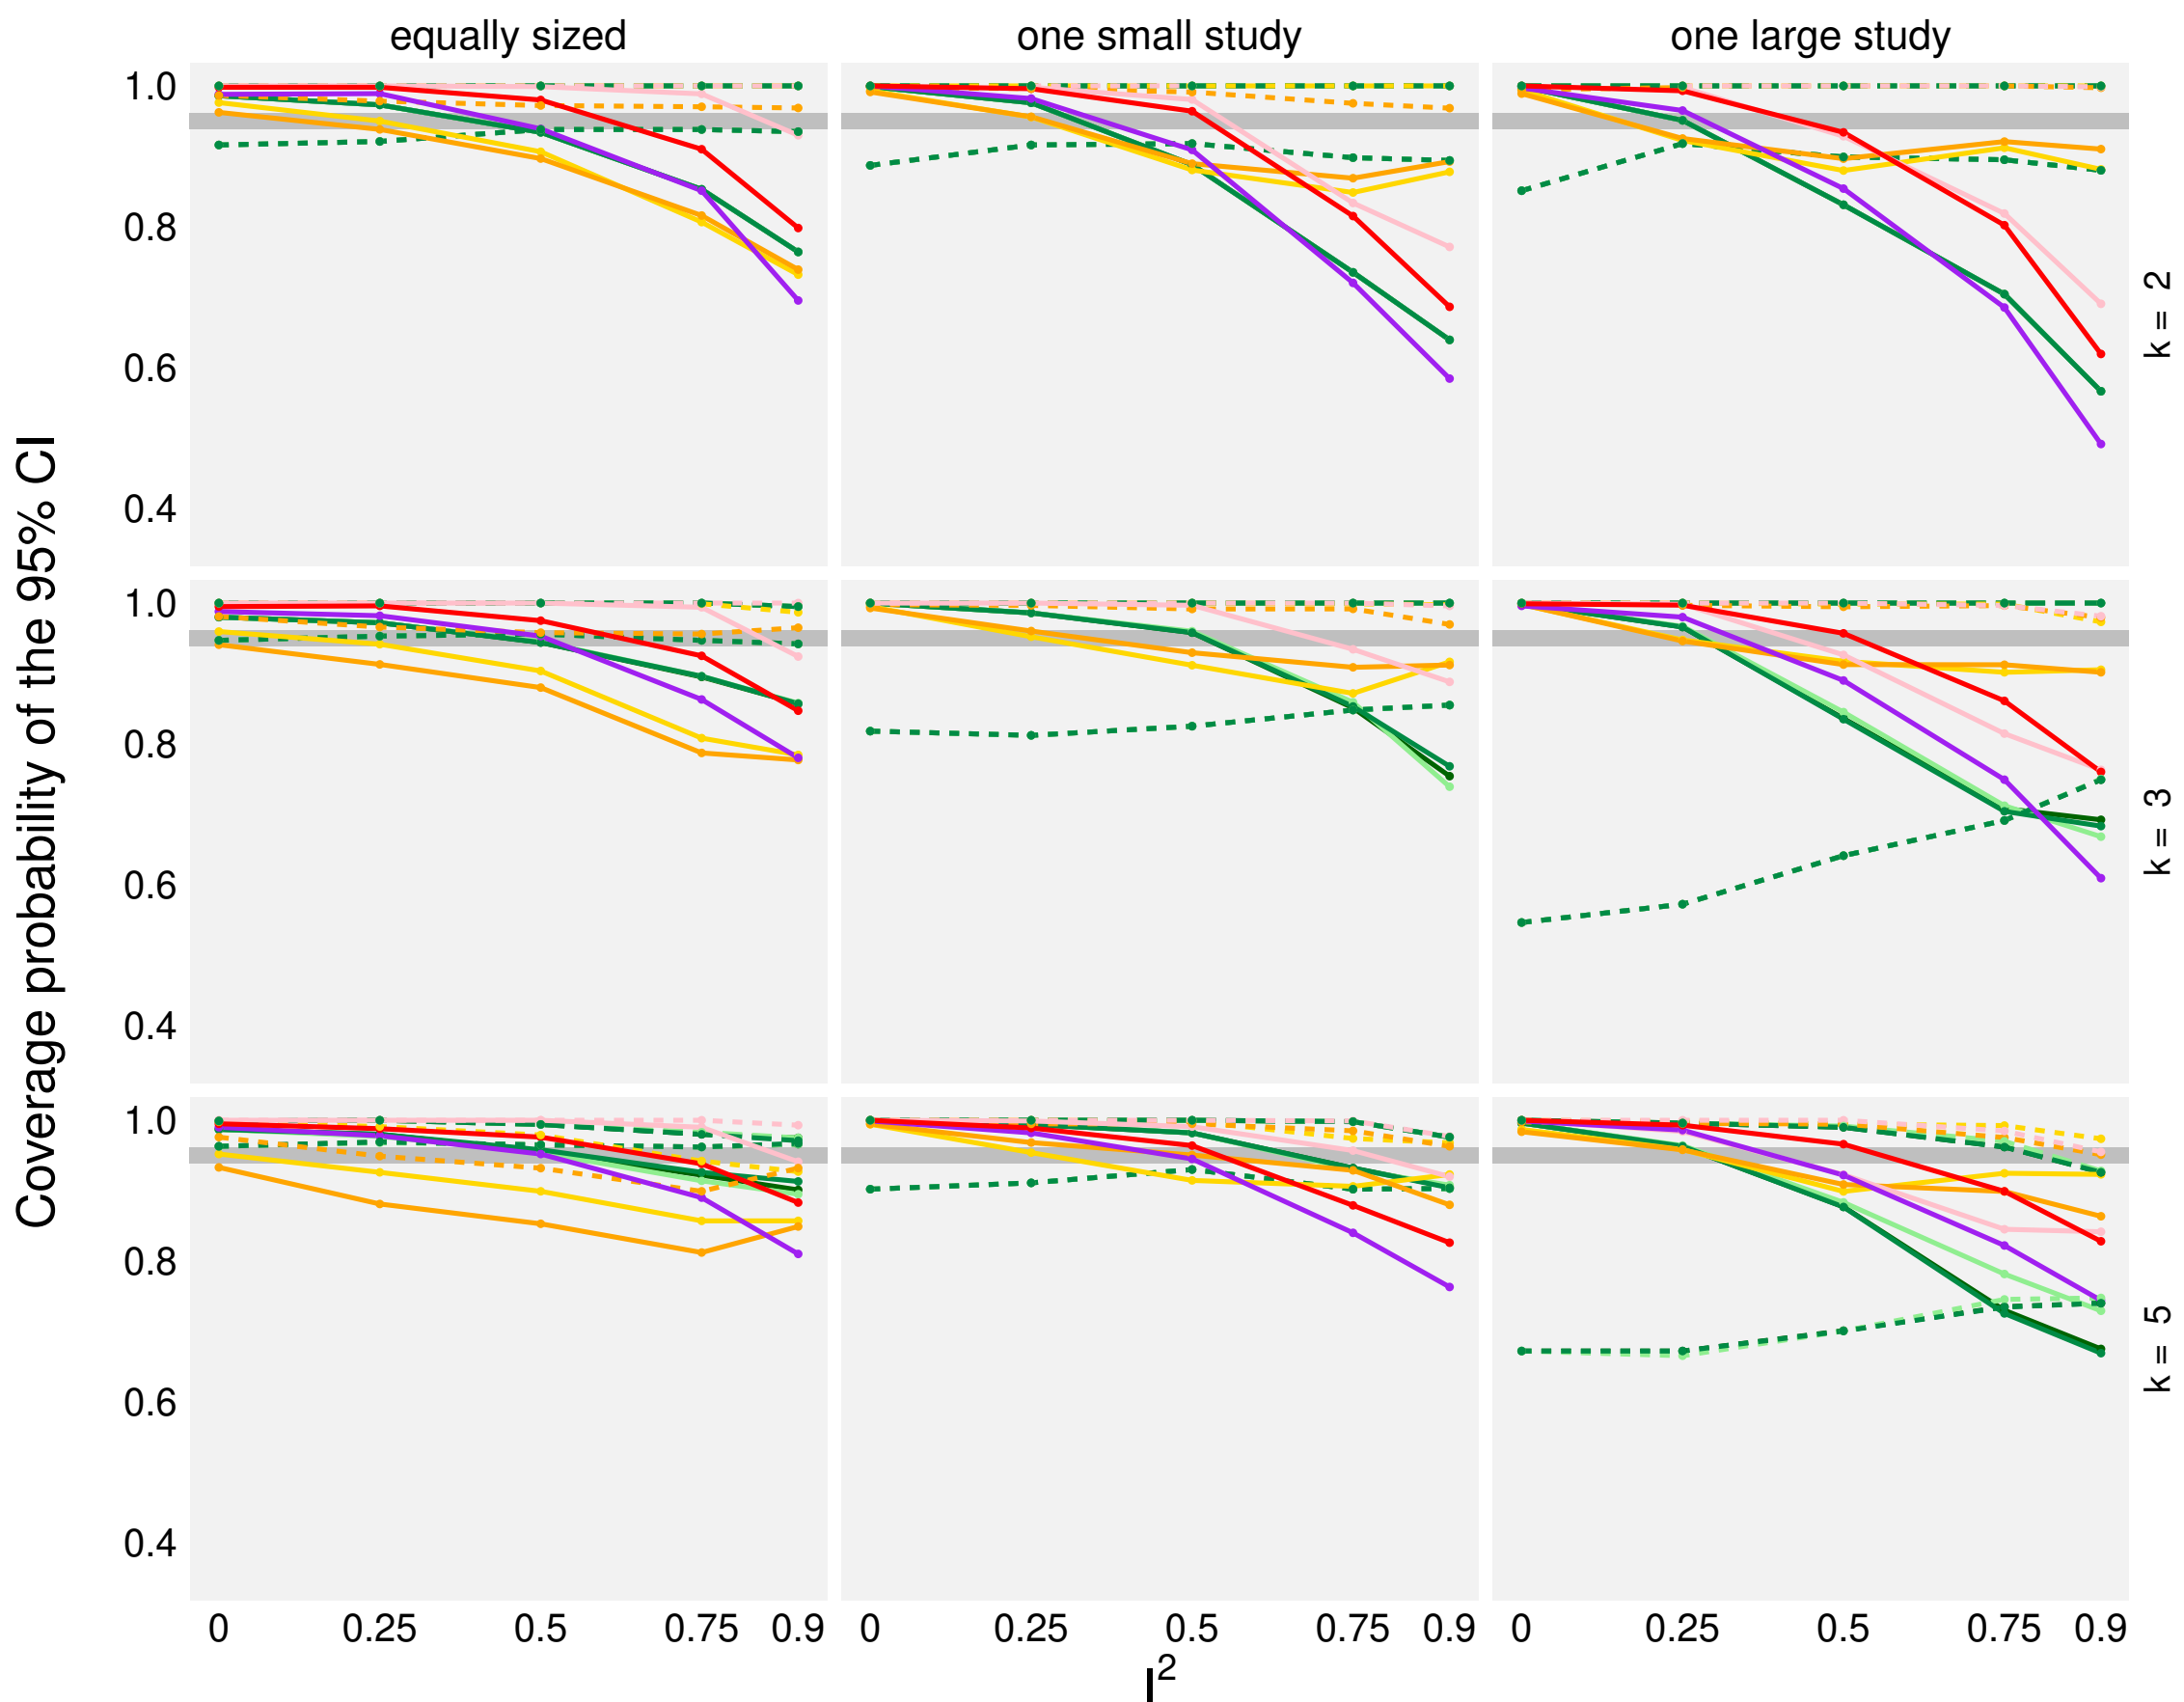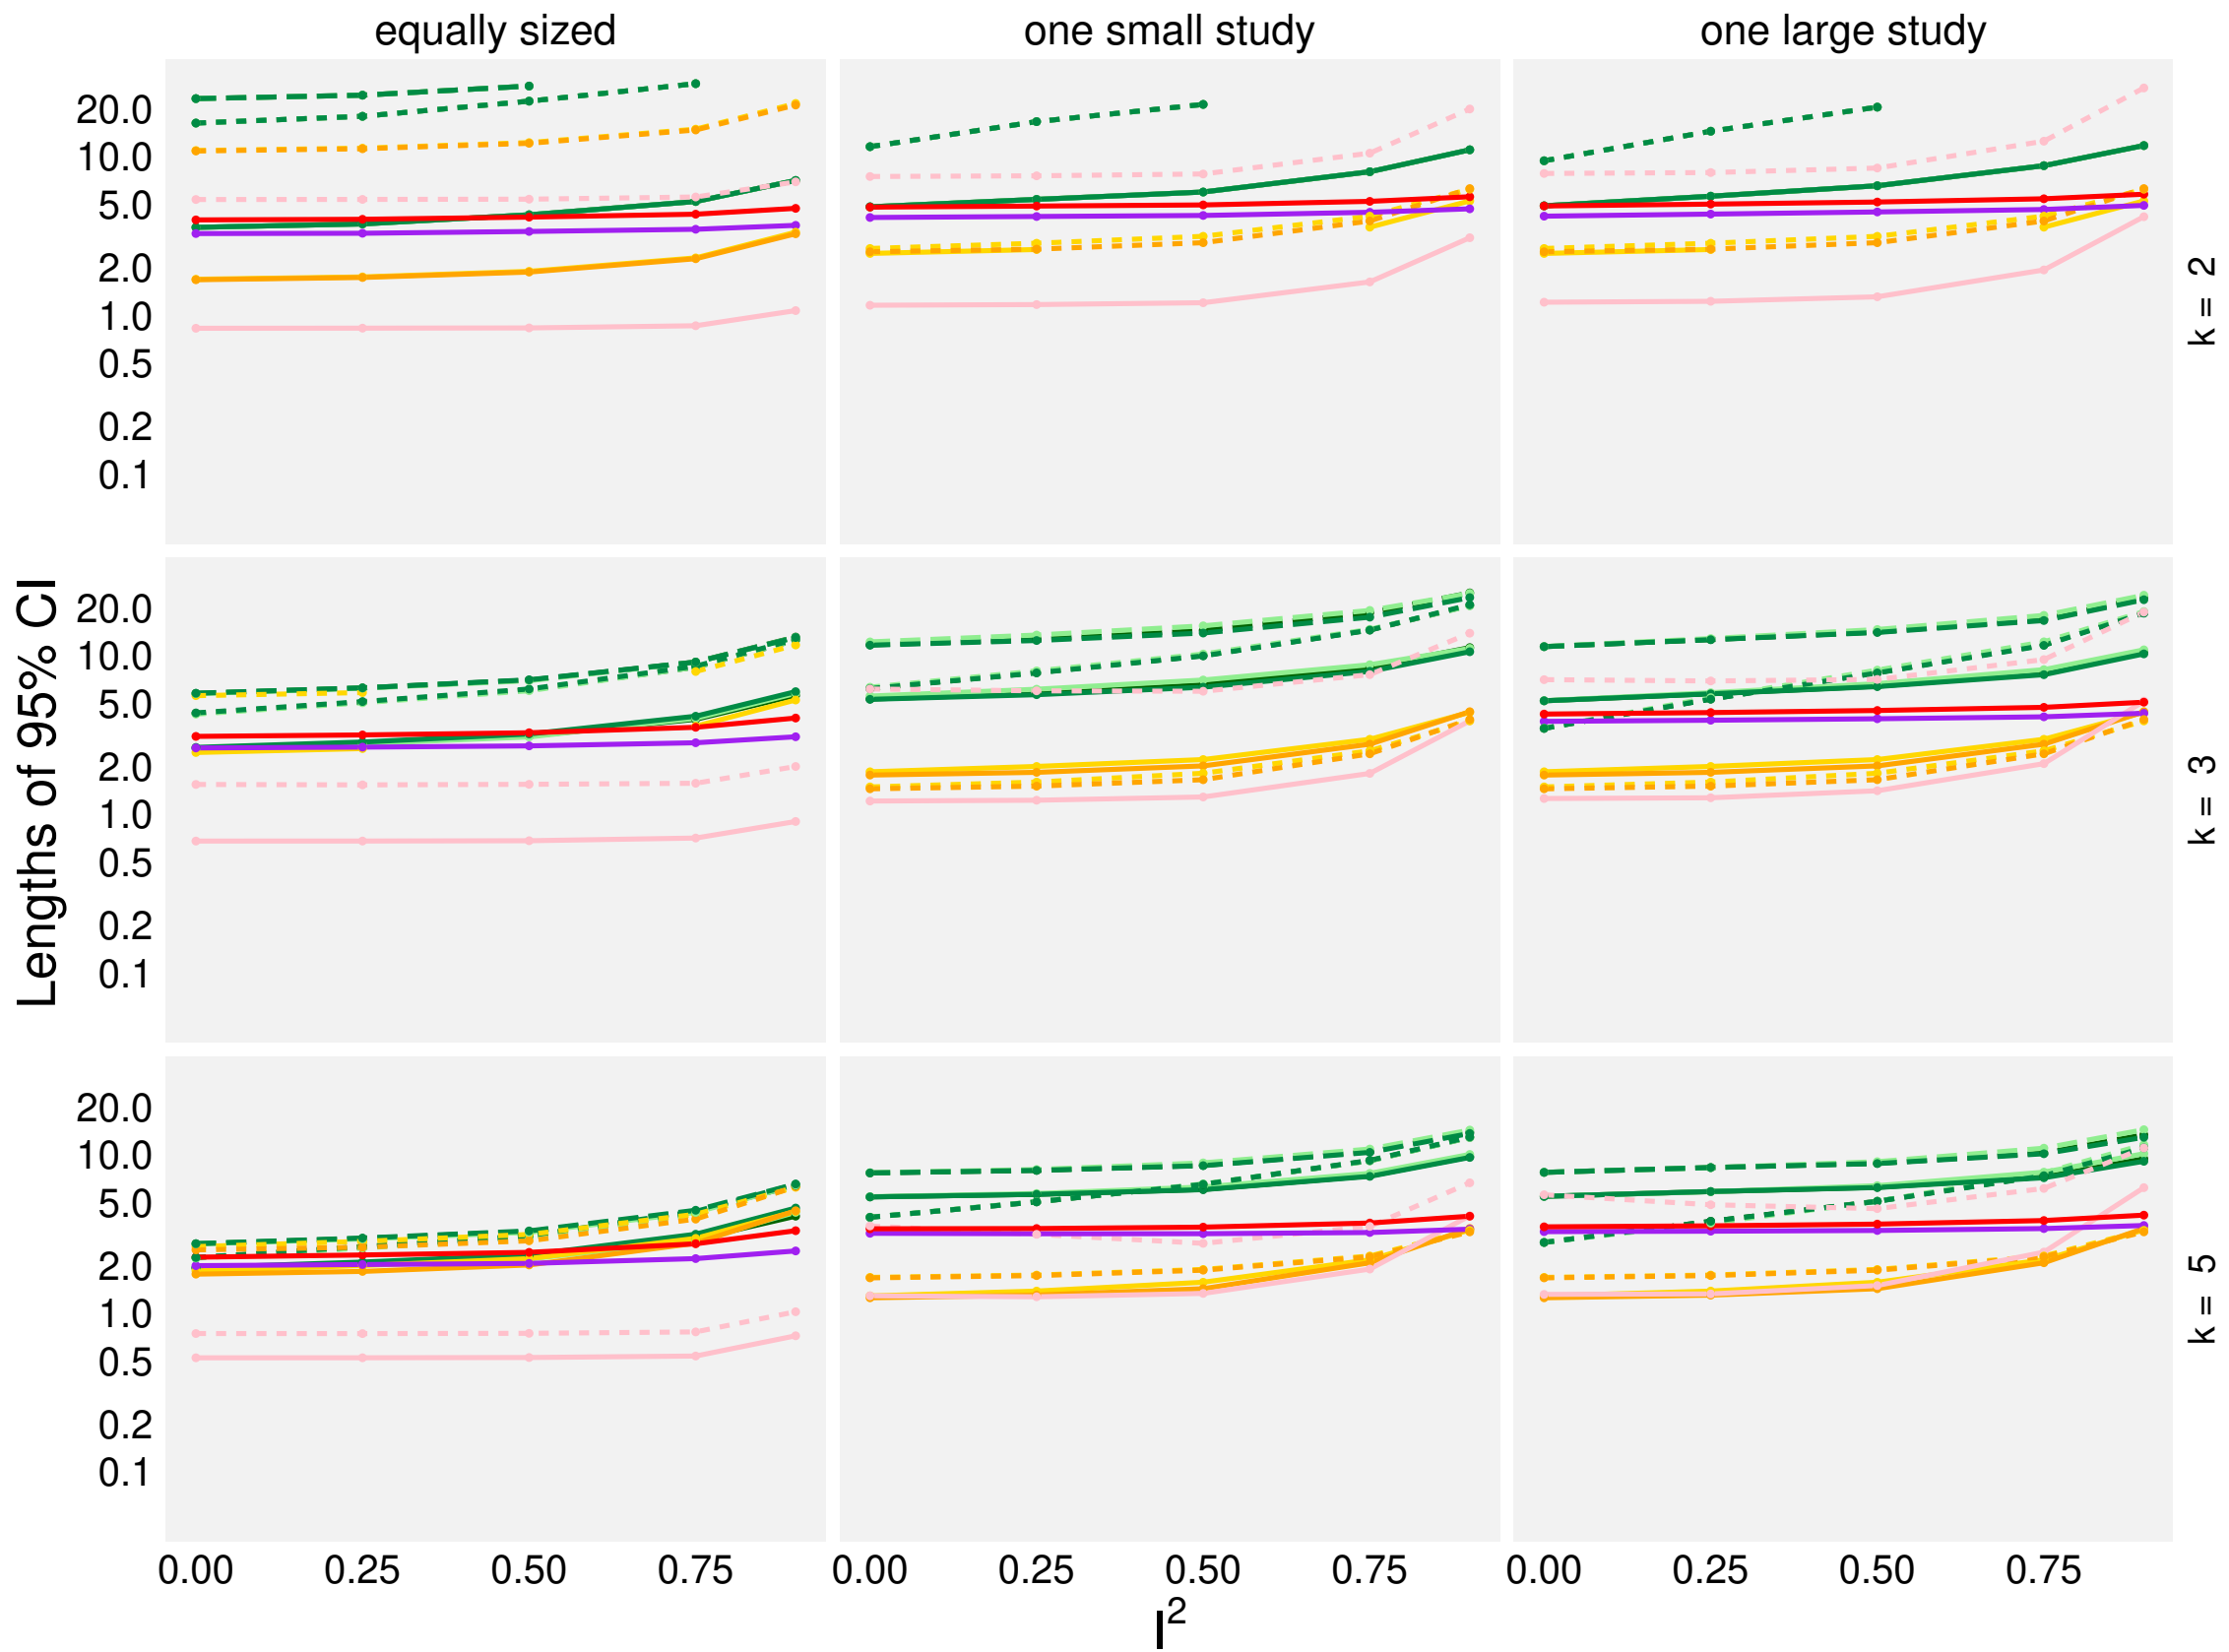

— NN — DL  
 — NN — REML  
 — NN — EB  
 — BN — UM.FS  
 — BN — UM.RS  
 — BN — CM.AL  
 — NN — Bayes HN(0.5)  
 — NN — Bayes HN(1)

— normal quantiles  
 -- HKSJ or Student's t  
 -- mHKSJ

OR  
( $n_i=50, \pi_0=0.1$ )

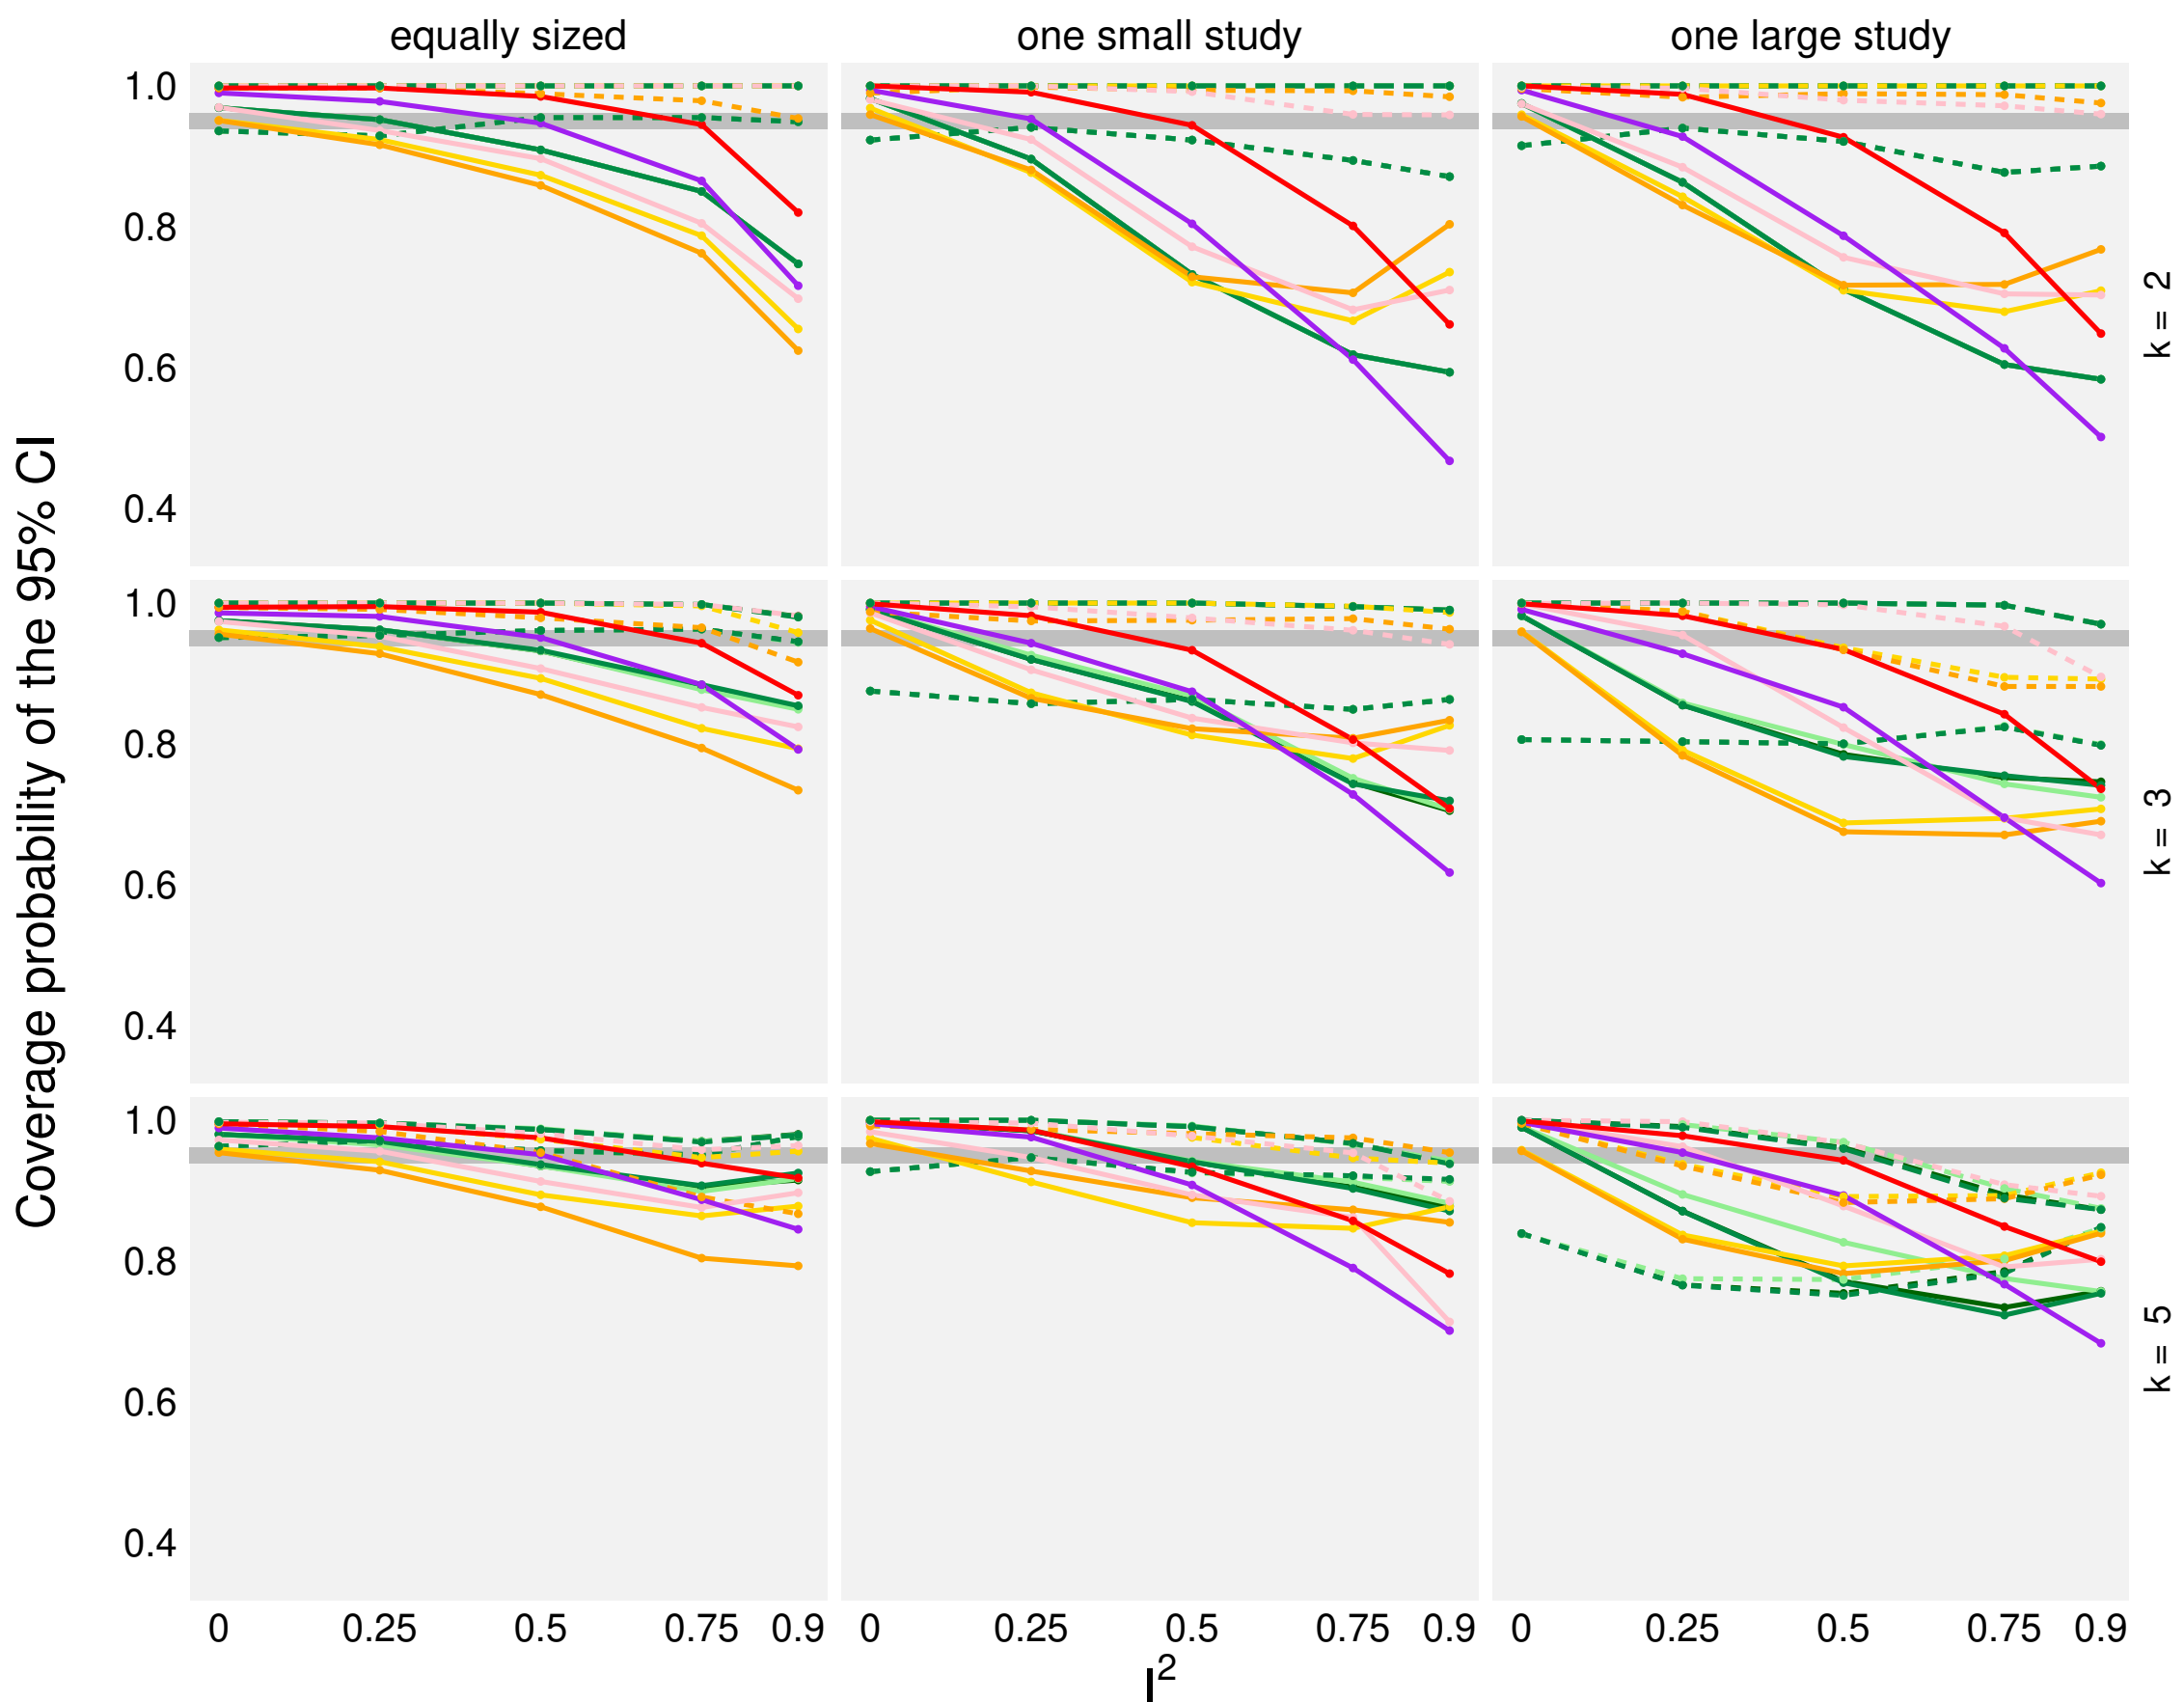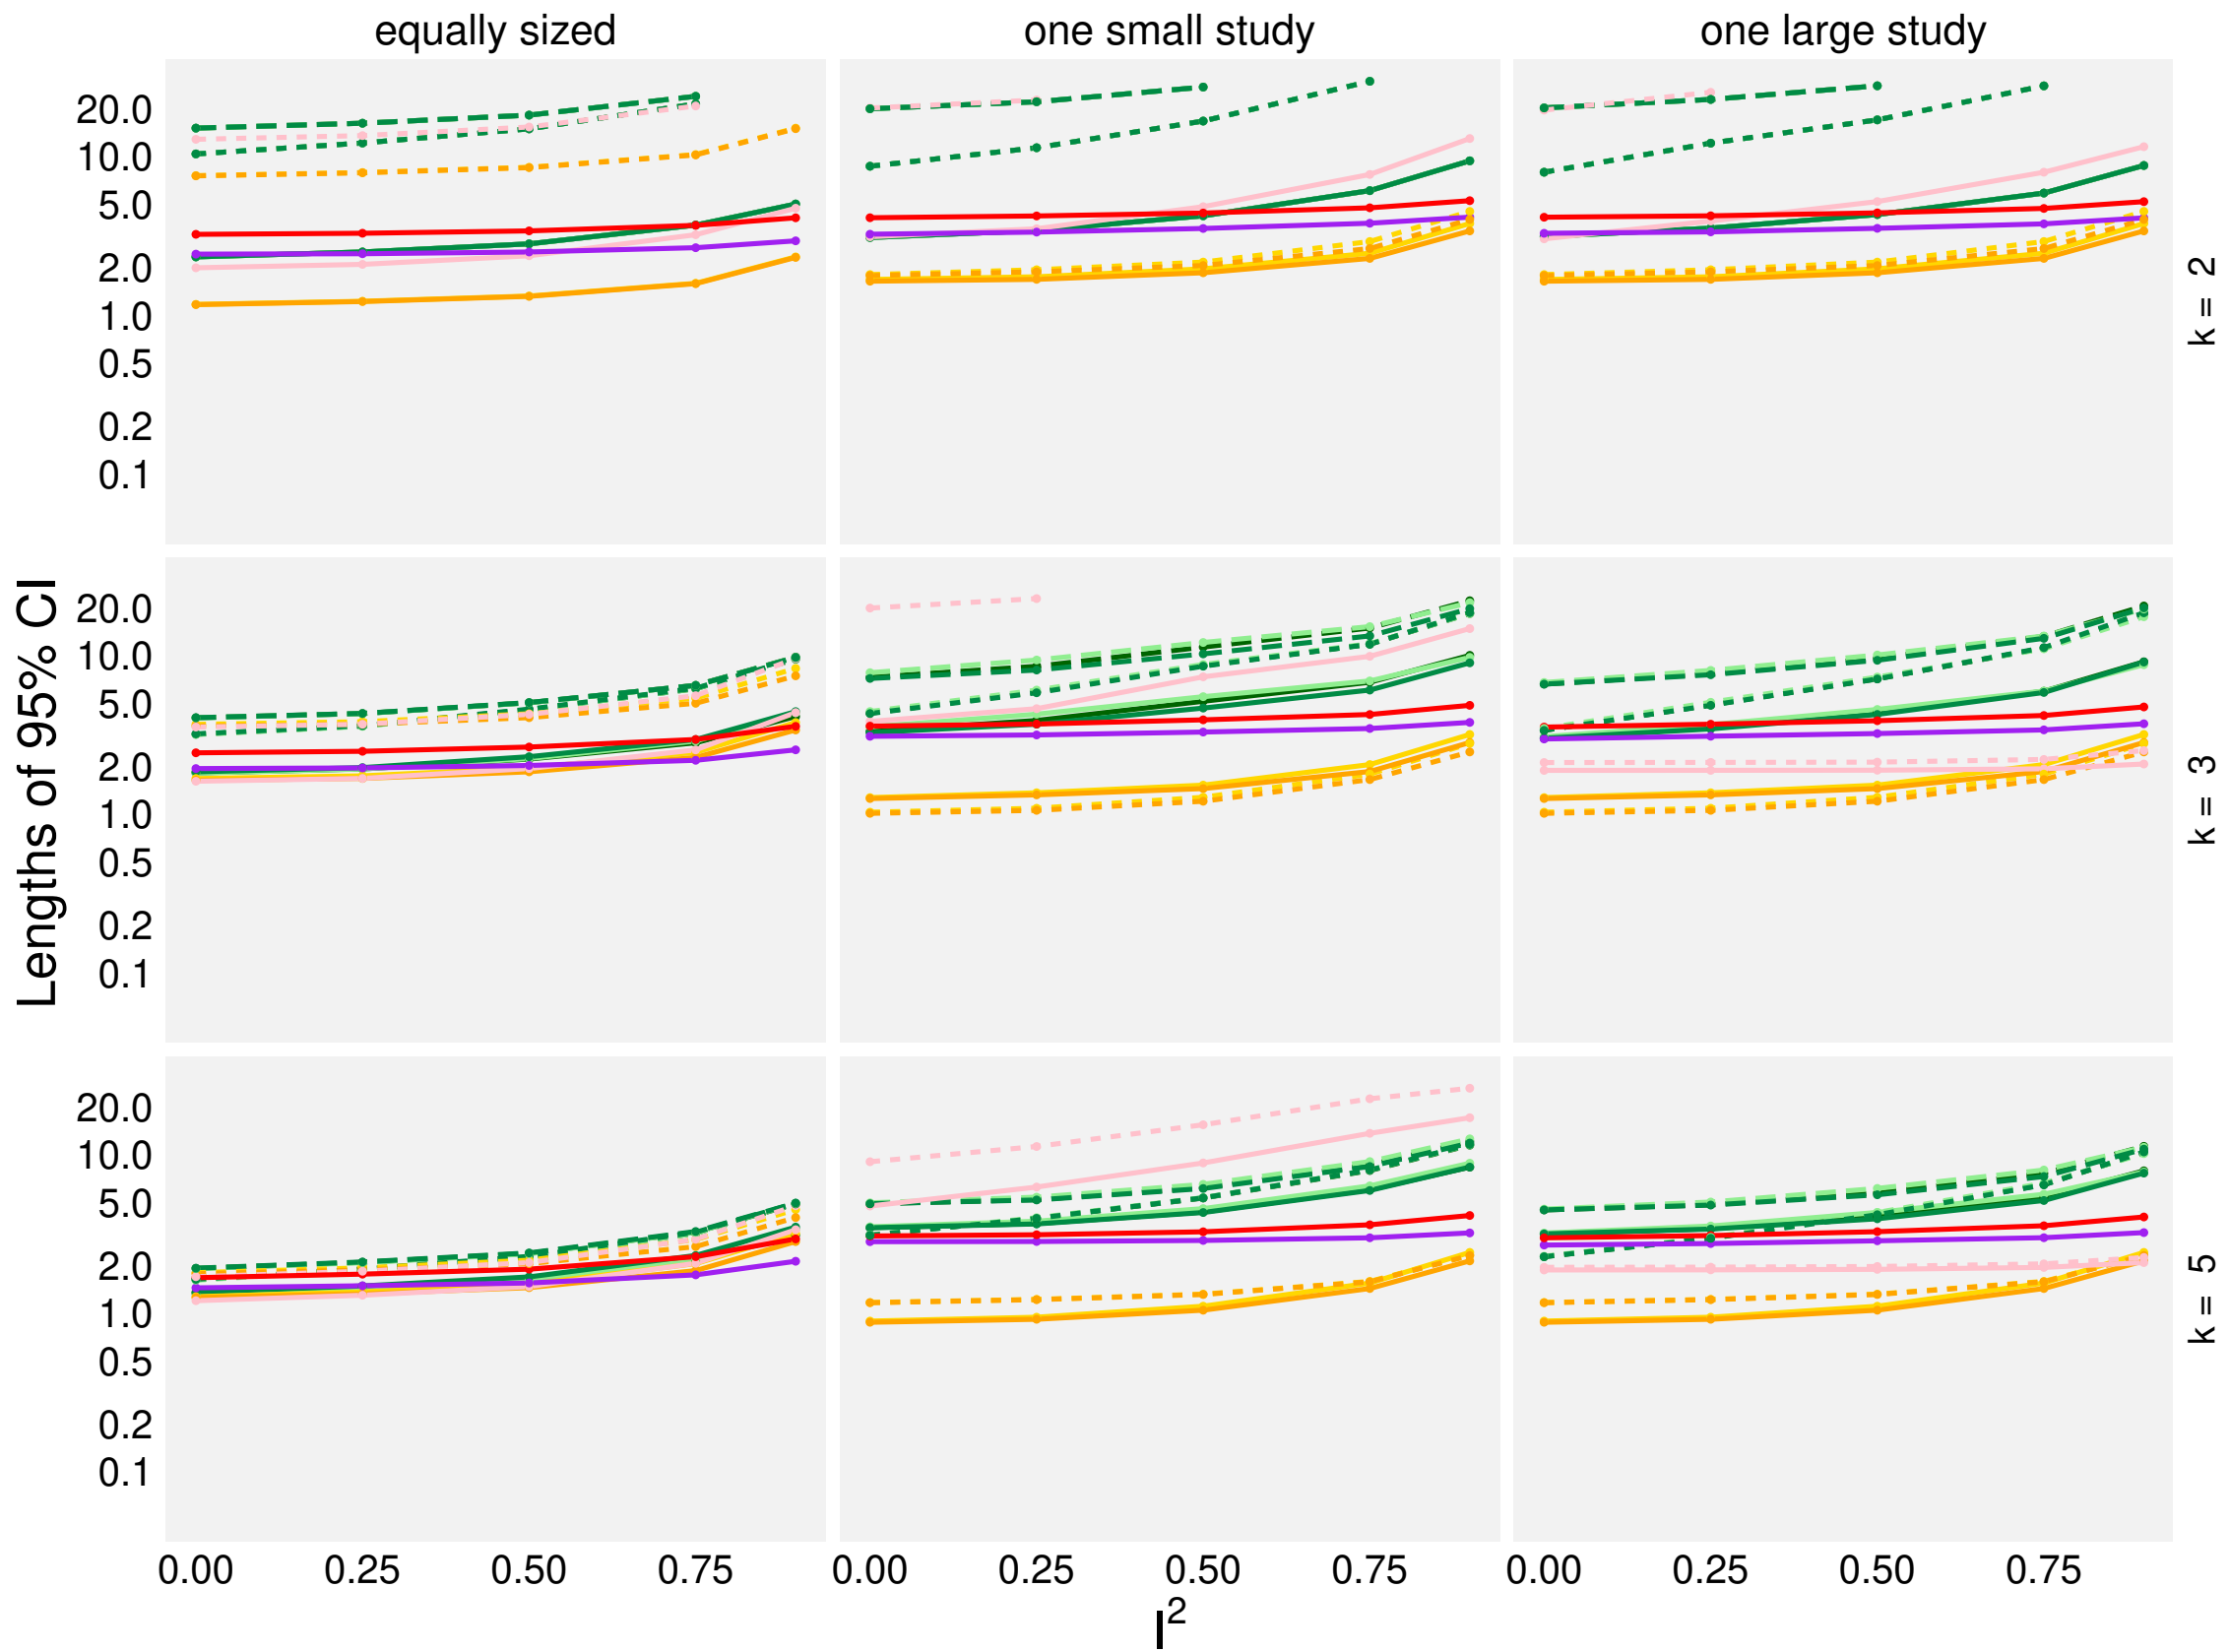

NN – DL  
 NN – REML  
 NN – EB  
 BN – UM.FS  
 BN – UM.RS  
 BN – CM.AL  
 NN – Bayes HN(0.5)  
 NN – Bayes HN(1)

— normal quantiles  
 -- HKSJ or Student's t  
 -·- mHKSJ

OR  
( $n_i=50, \pi_0=0.3$ )

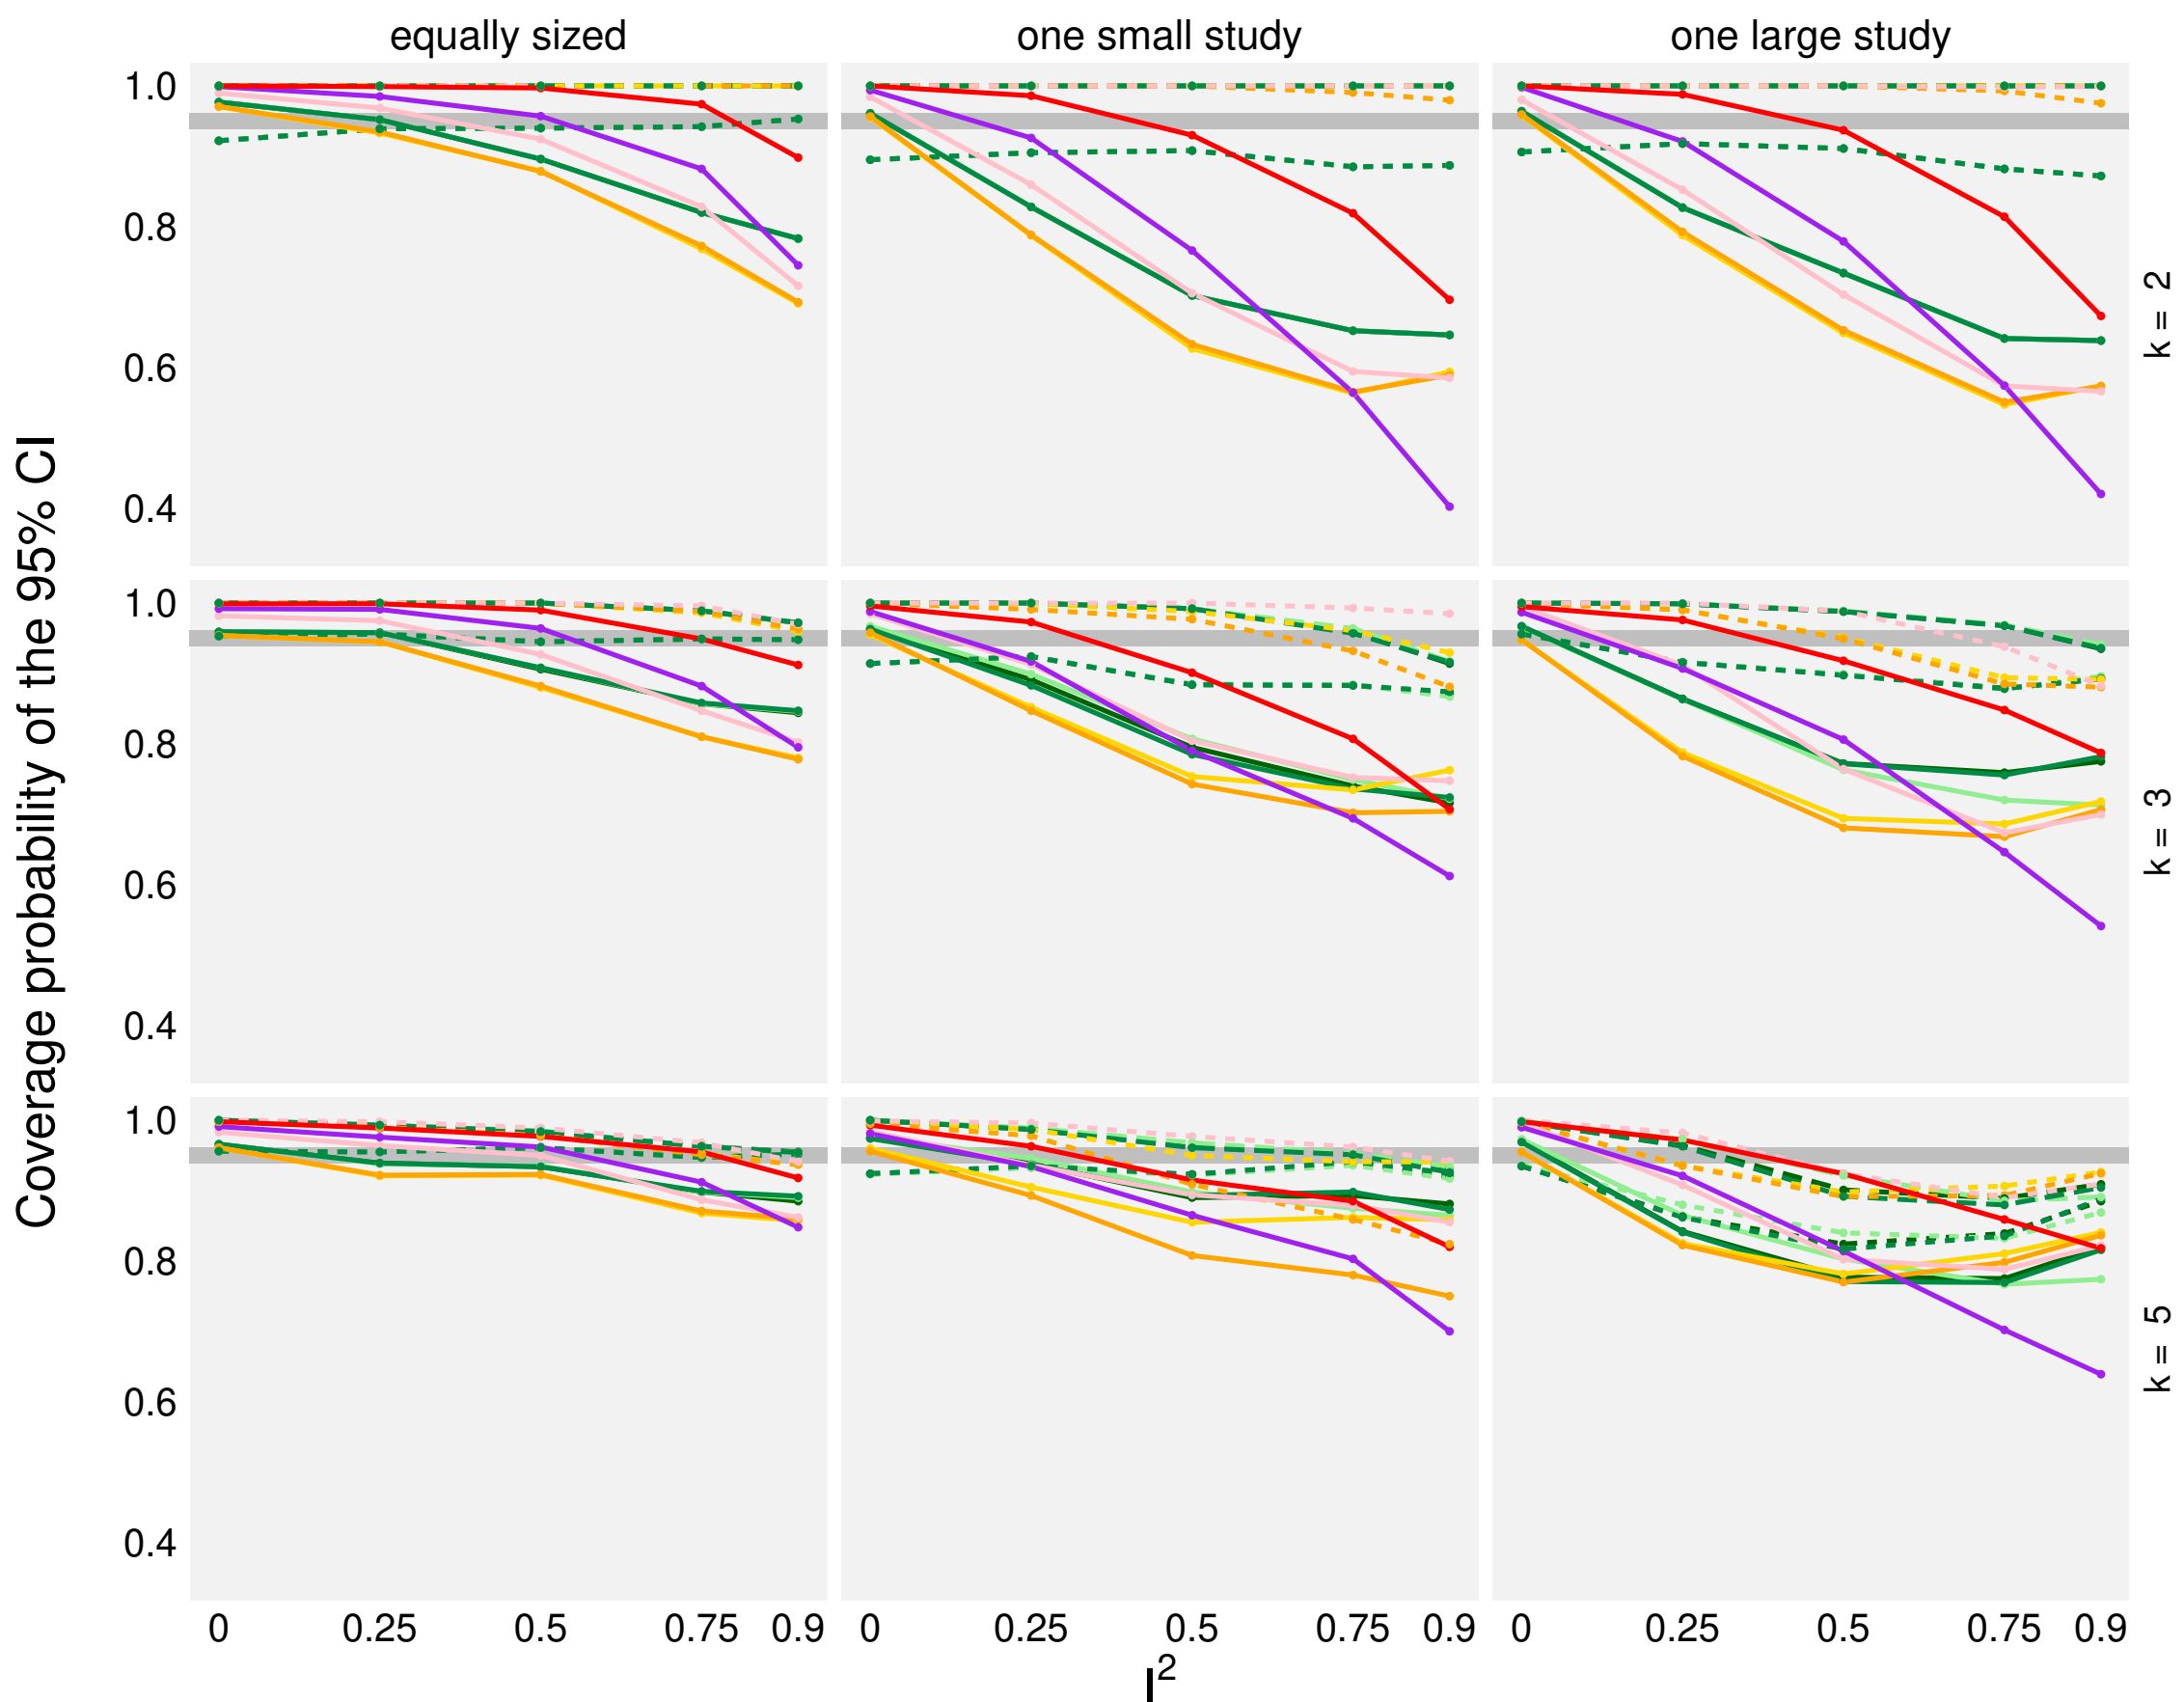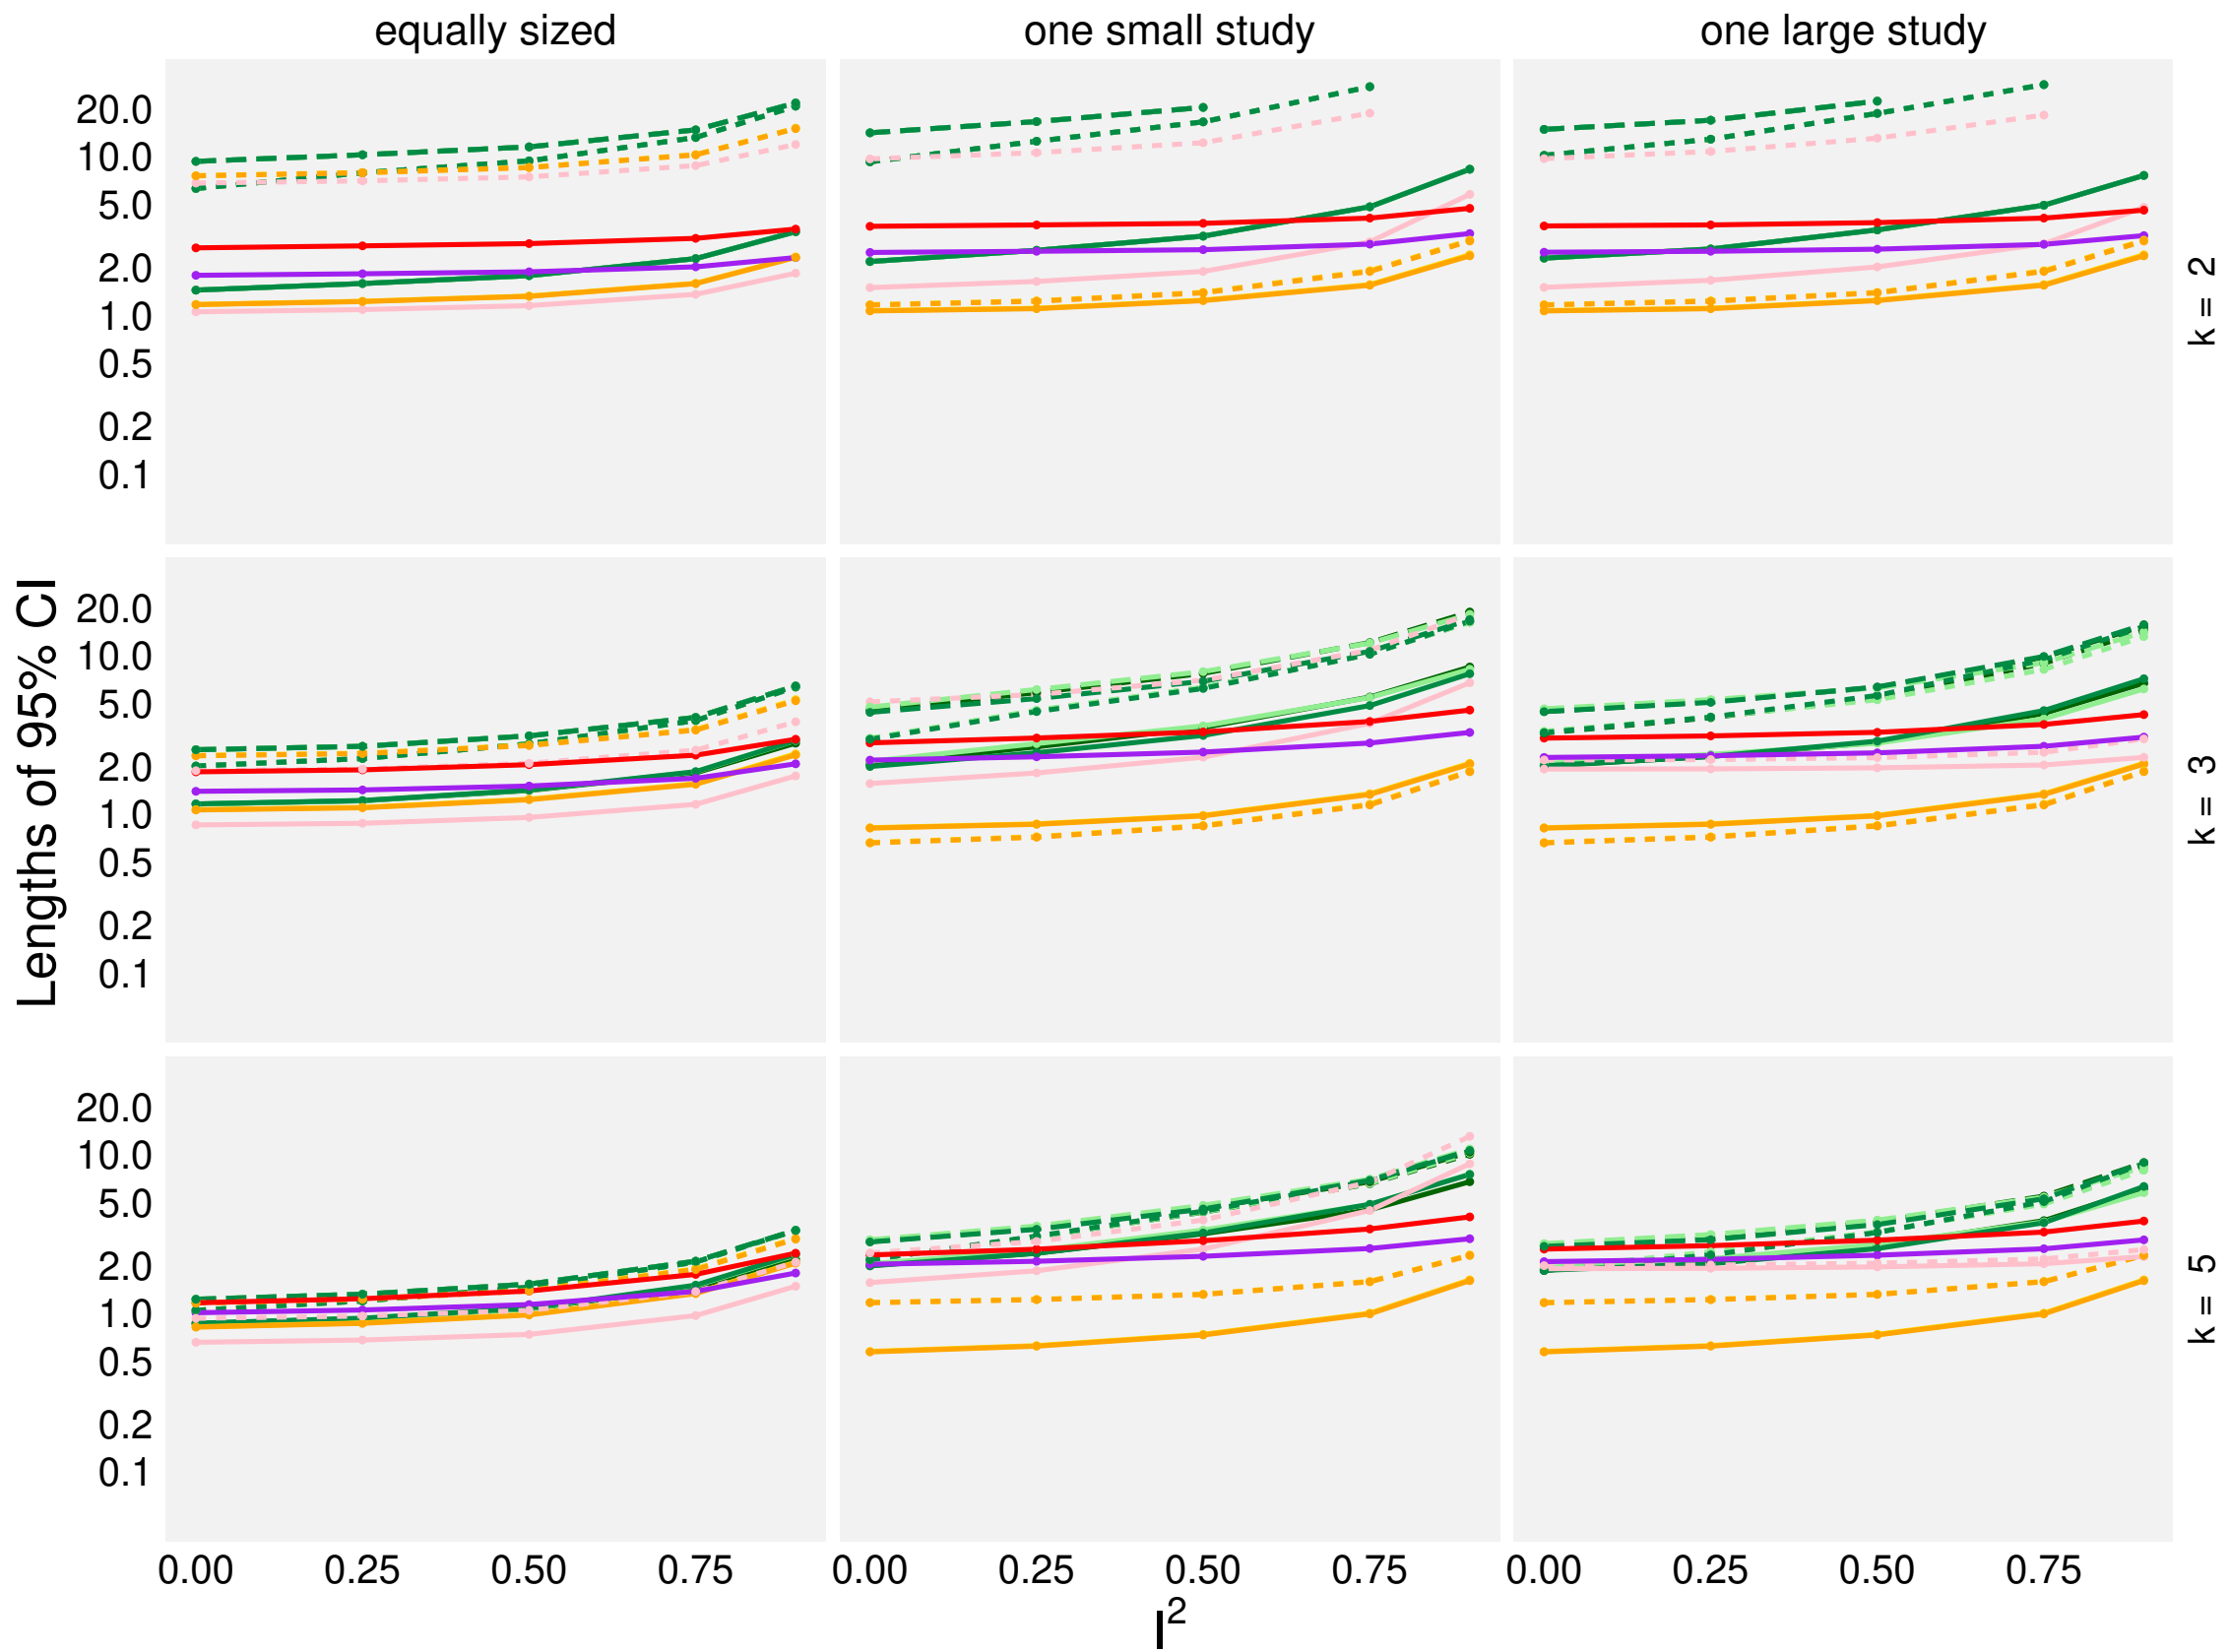

— NN — DL  
 — NN — REML  
 — NN — EB  
 — BN — UM.FS  
 — BN — UM.RS  
 — BN — CM.AL  
 — NN — Bayes HN(0.5)  
 — NN — Bayes HN(1)

— normal quantiles  
 - - HKSJ or Student's t  
 - - mHKSJ

OR  
( $n_i=50, \pi_0=0.5$ )

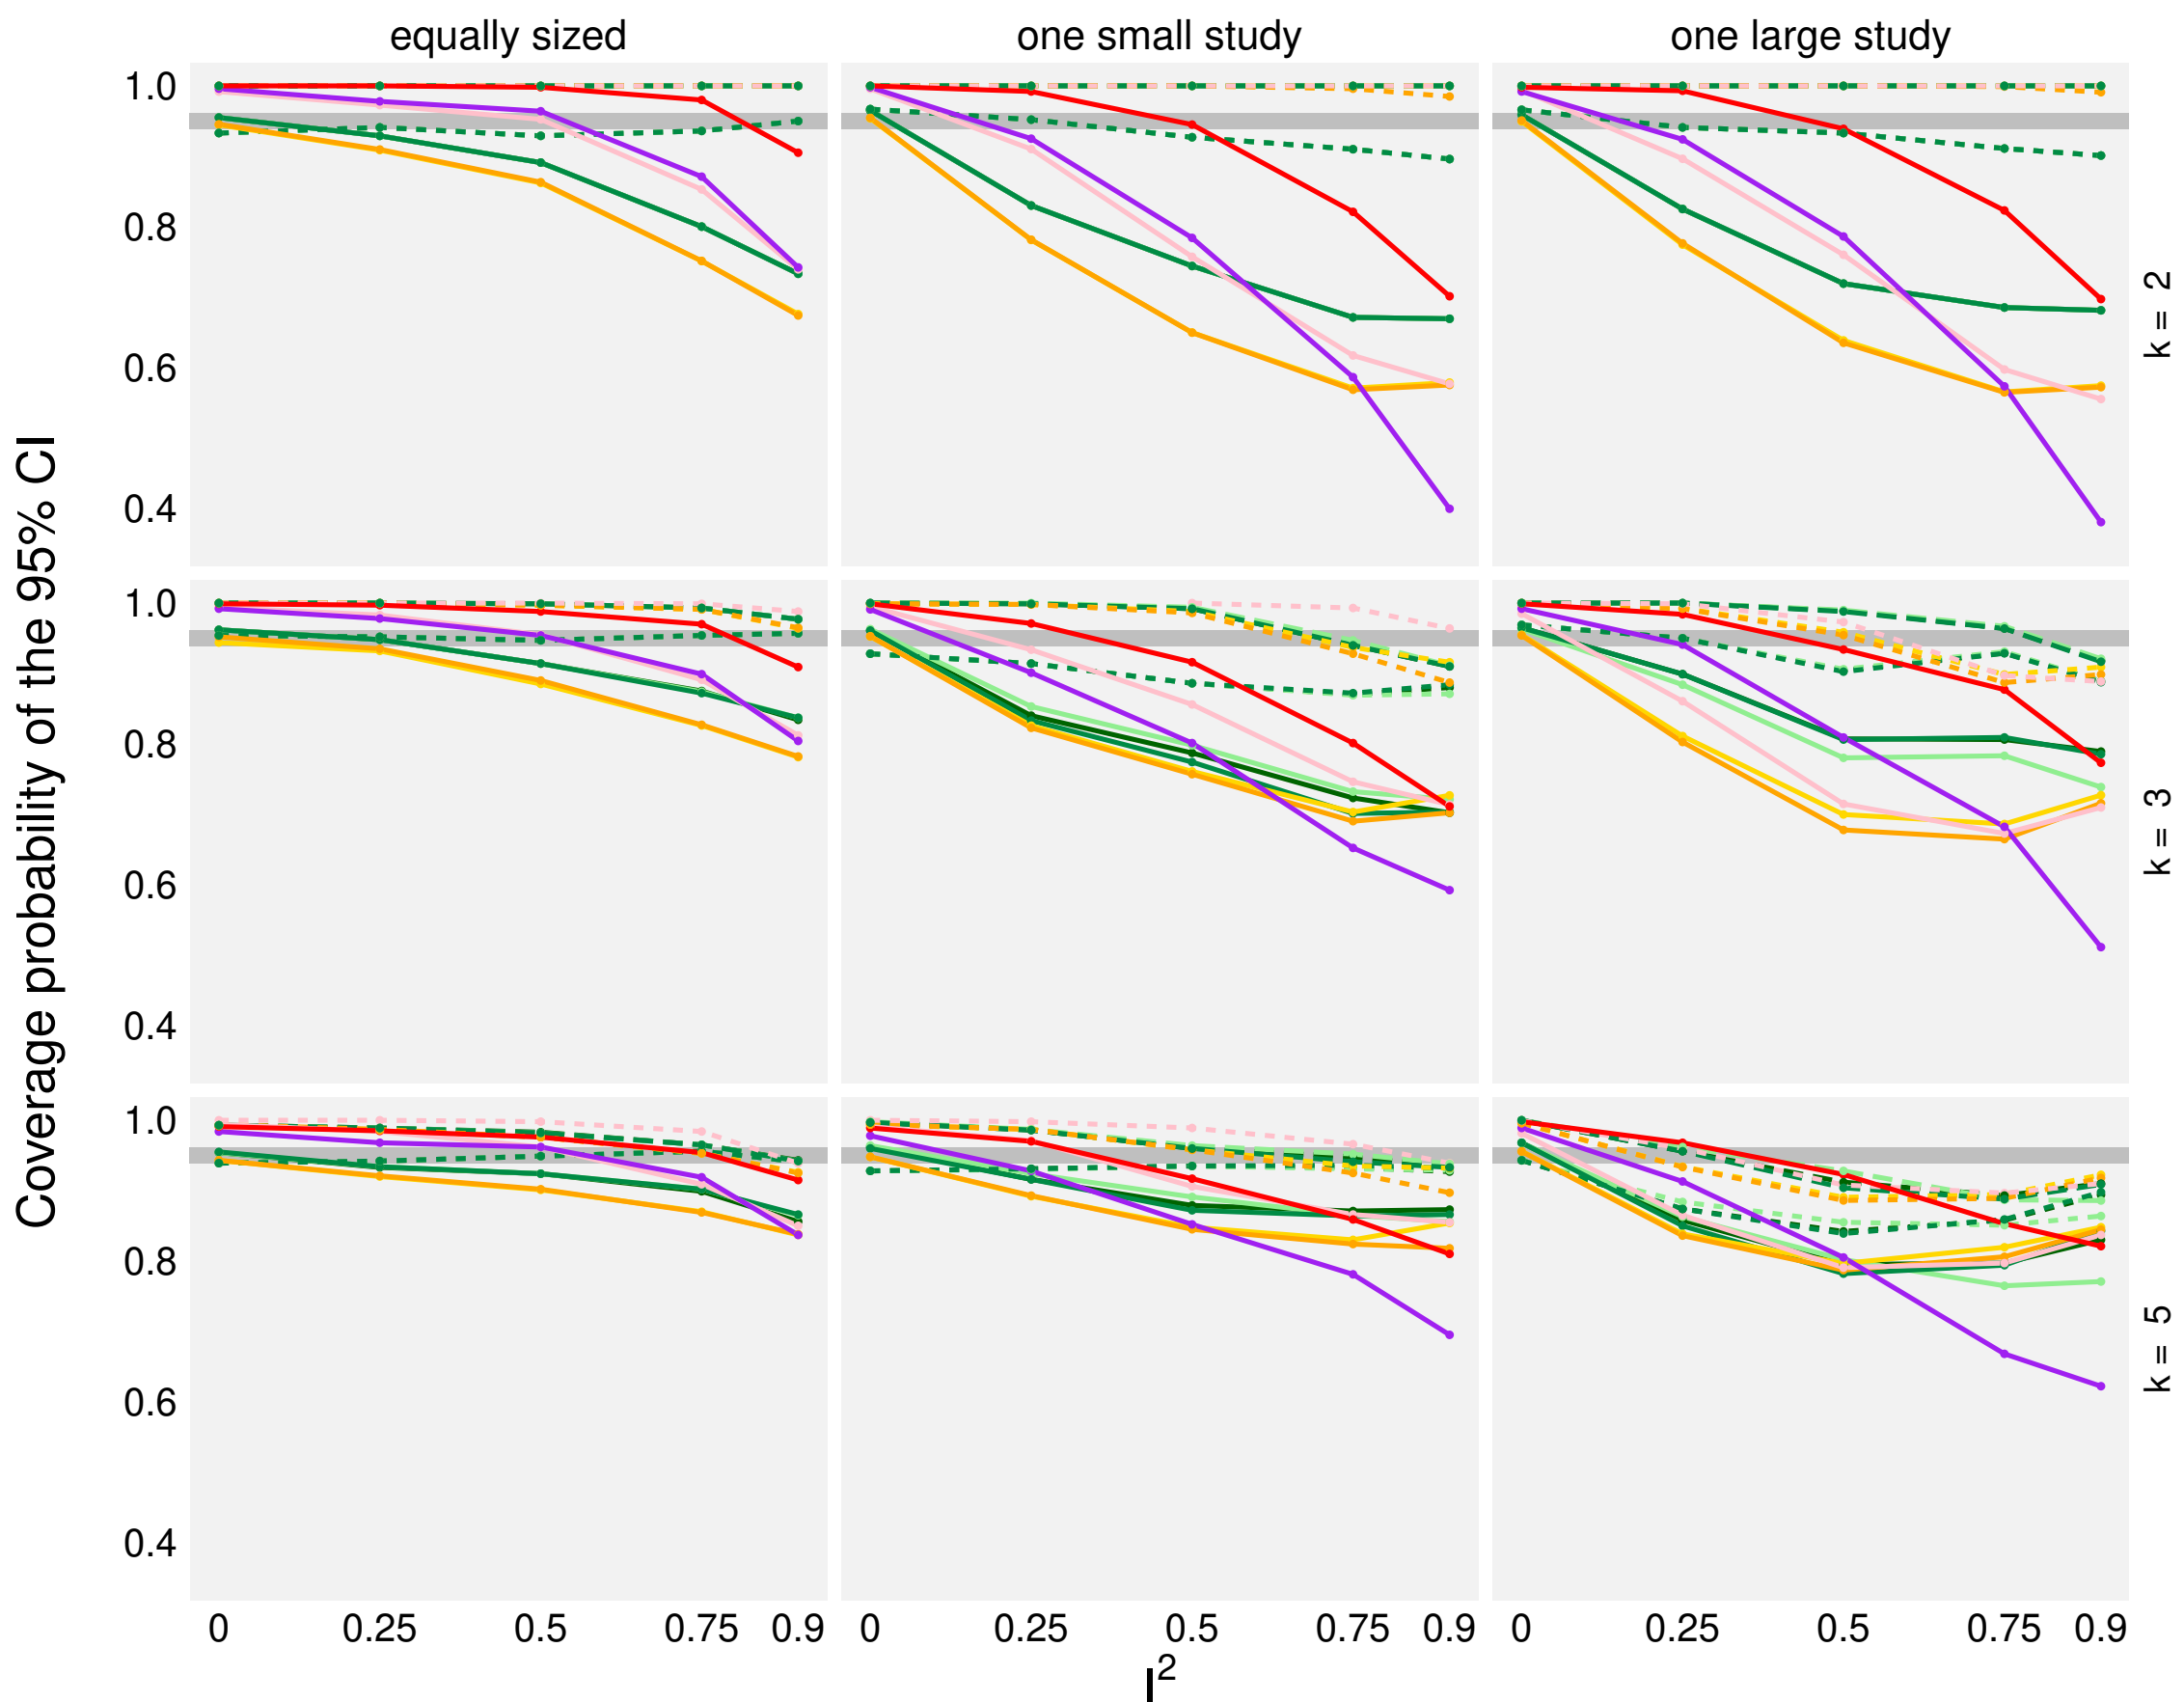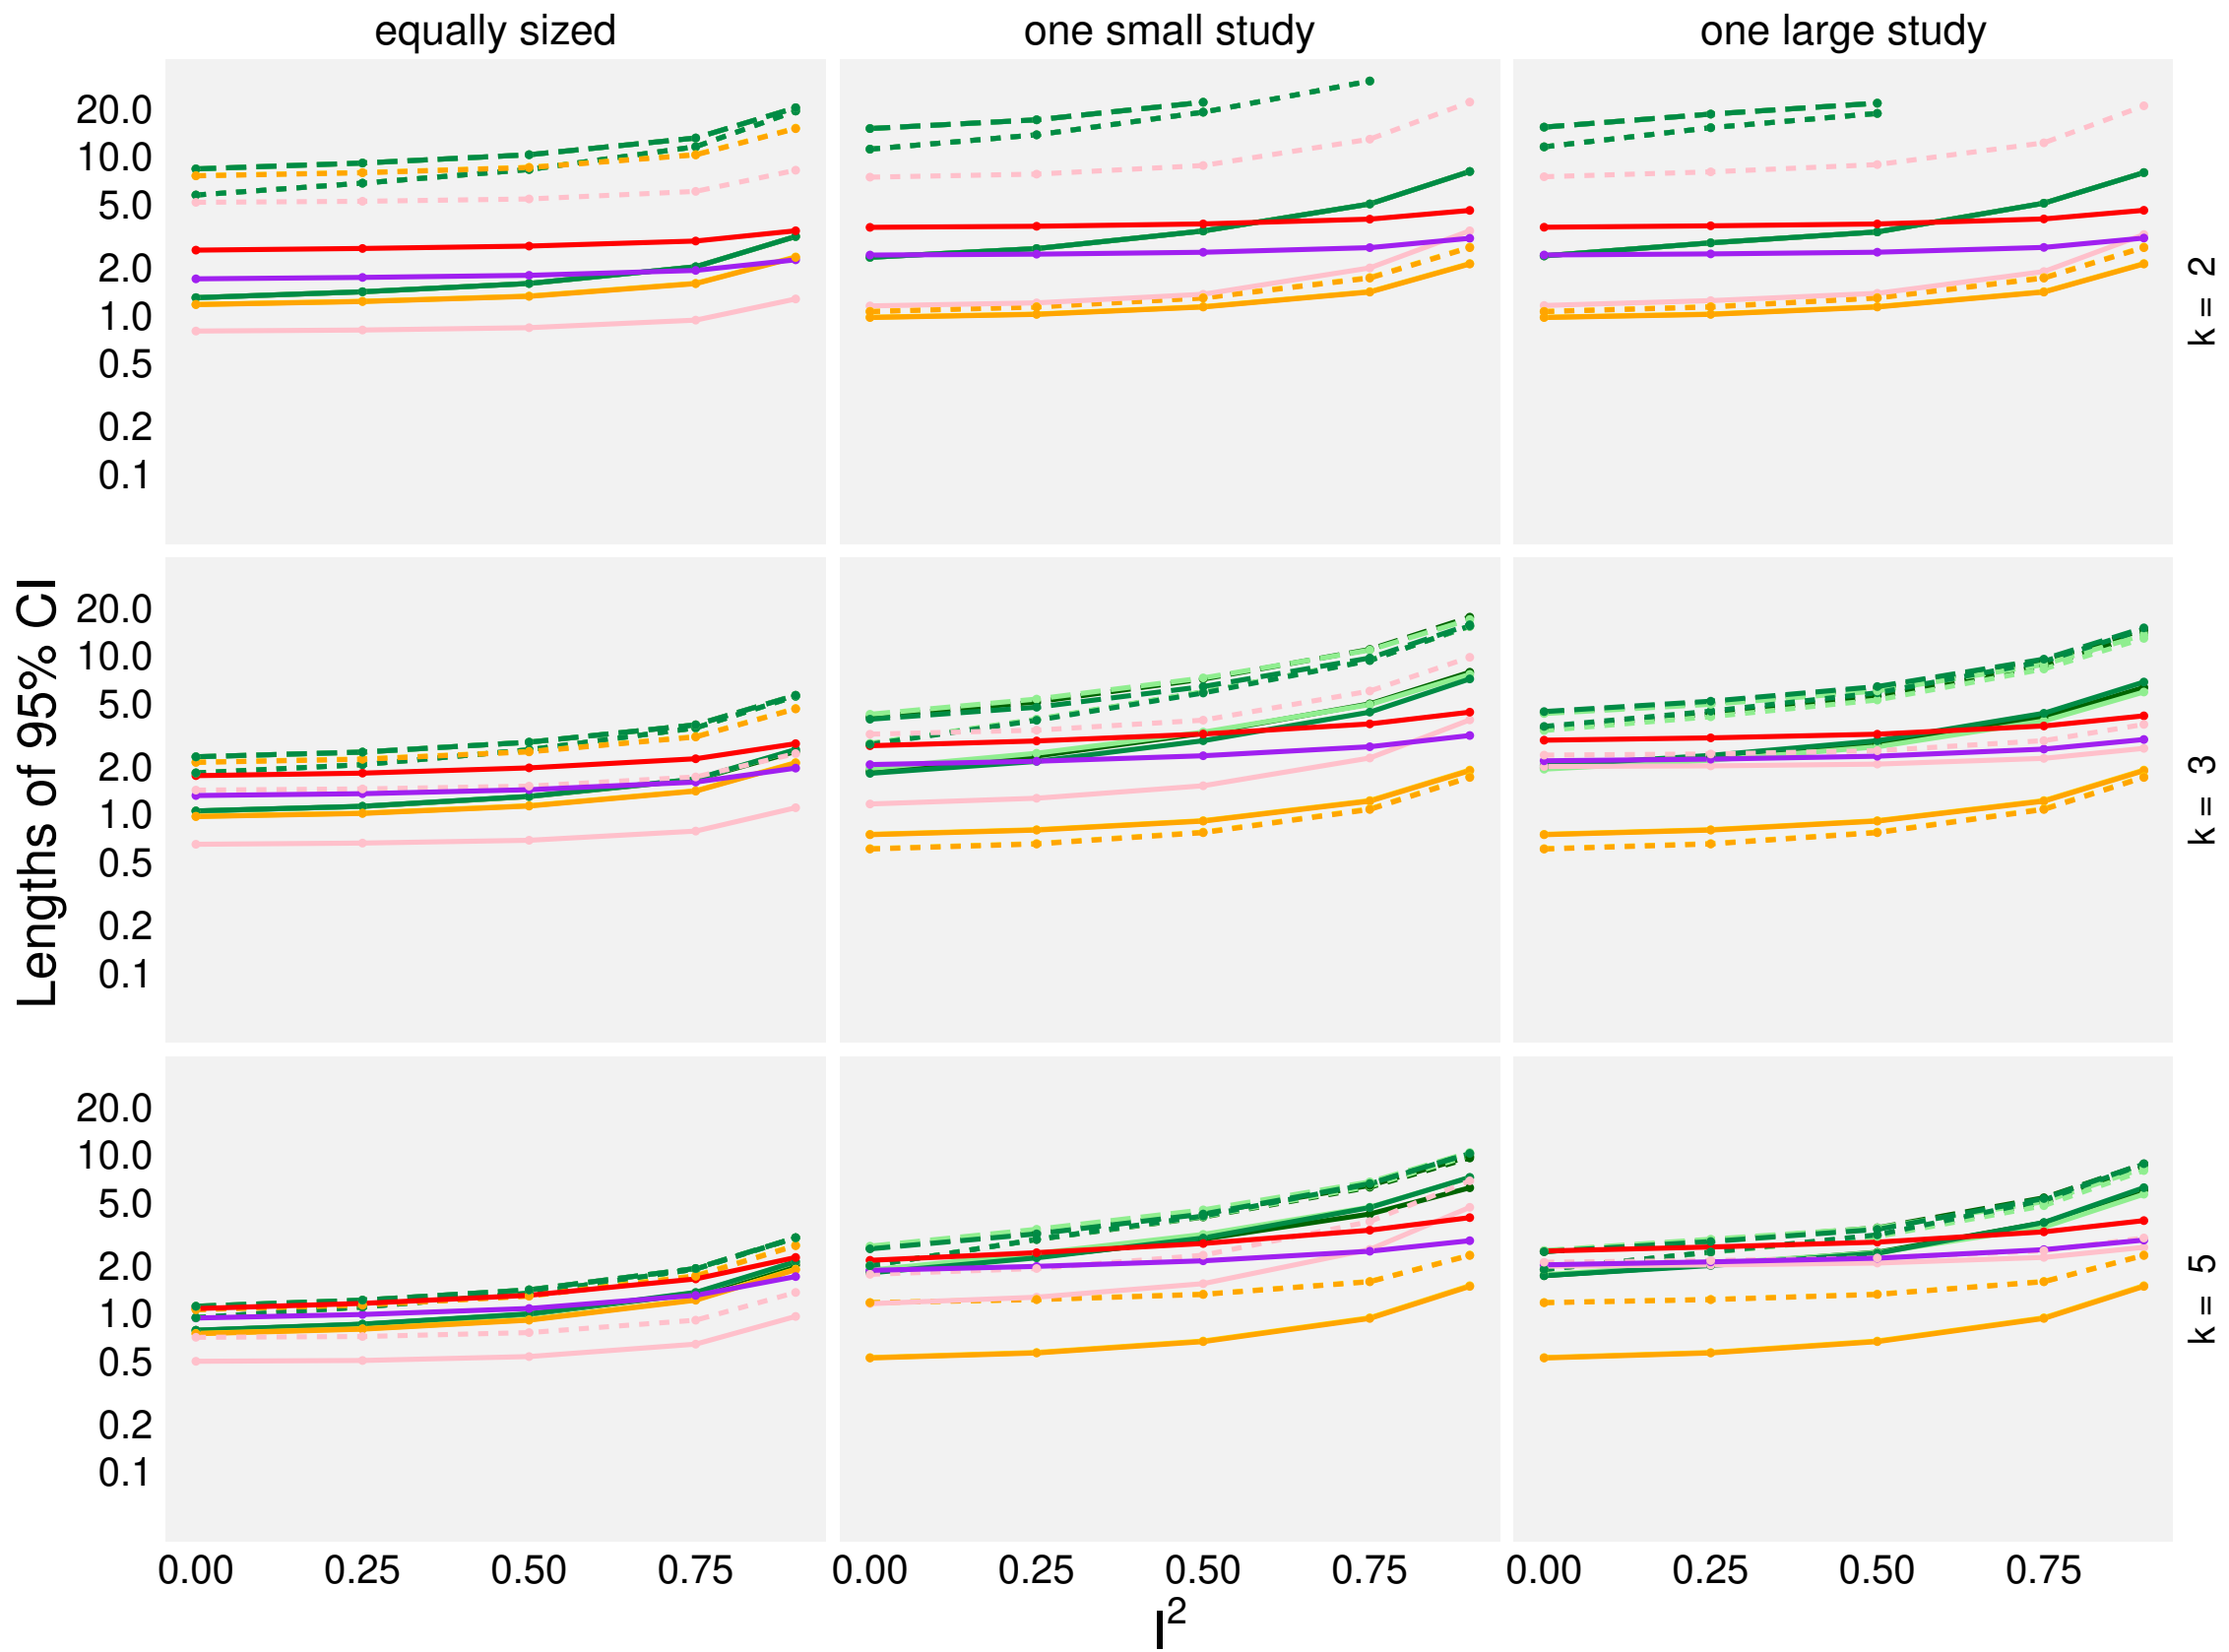

— NN — DL      — BN — UM.RS      — normal quantiles  
 — NN — REML      — BN — CM.AL      -- HKSJ or Student's t  
 — NN — EB      — NN — Bayes HN(0.5)      -- mHKSJ  
 — BN — UM.FS      — NN — Bayes HN(1)

OR  
( $n_i=50, \pi_0=0.7$ )

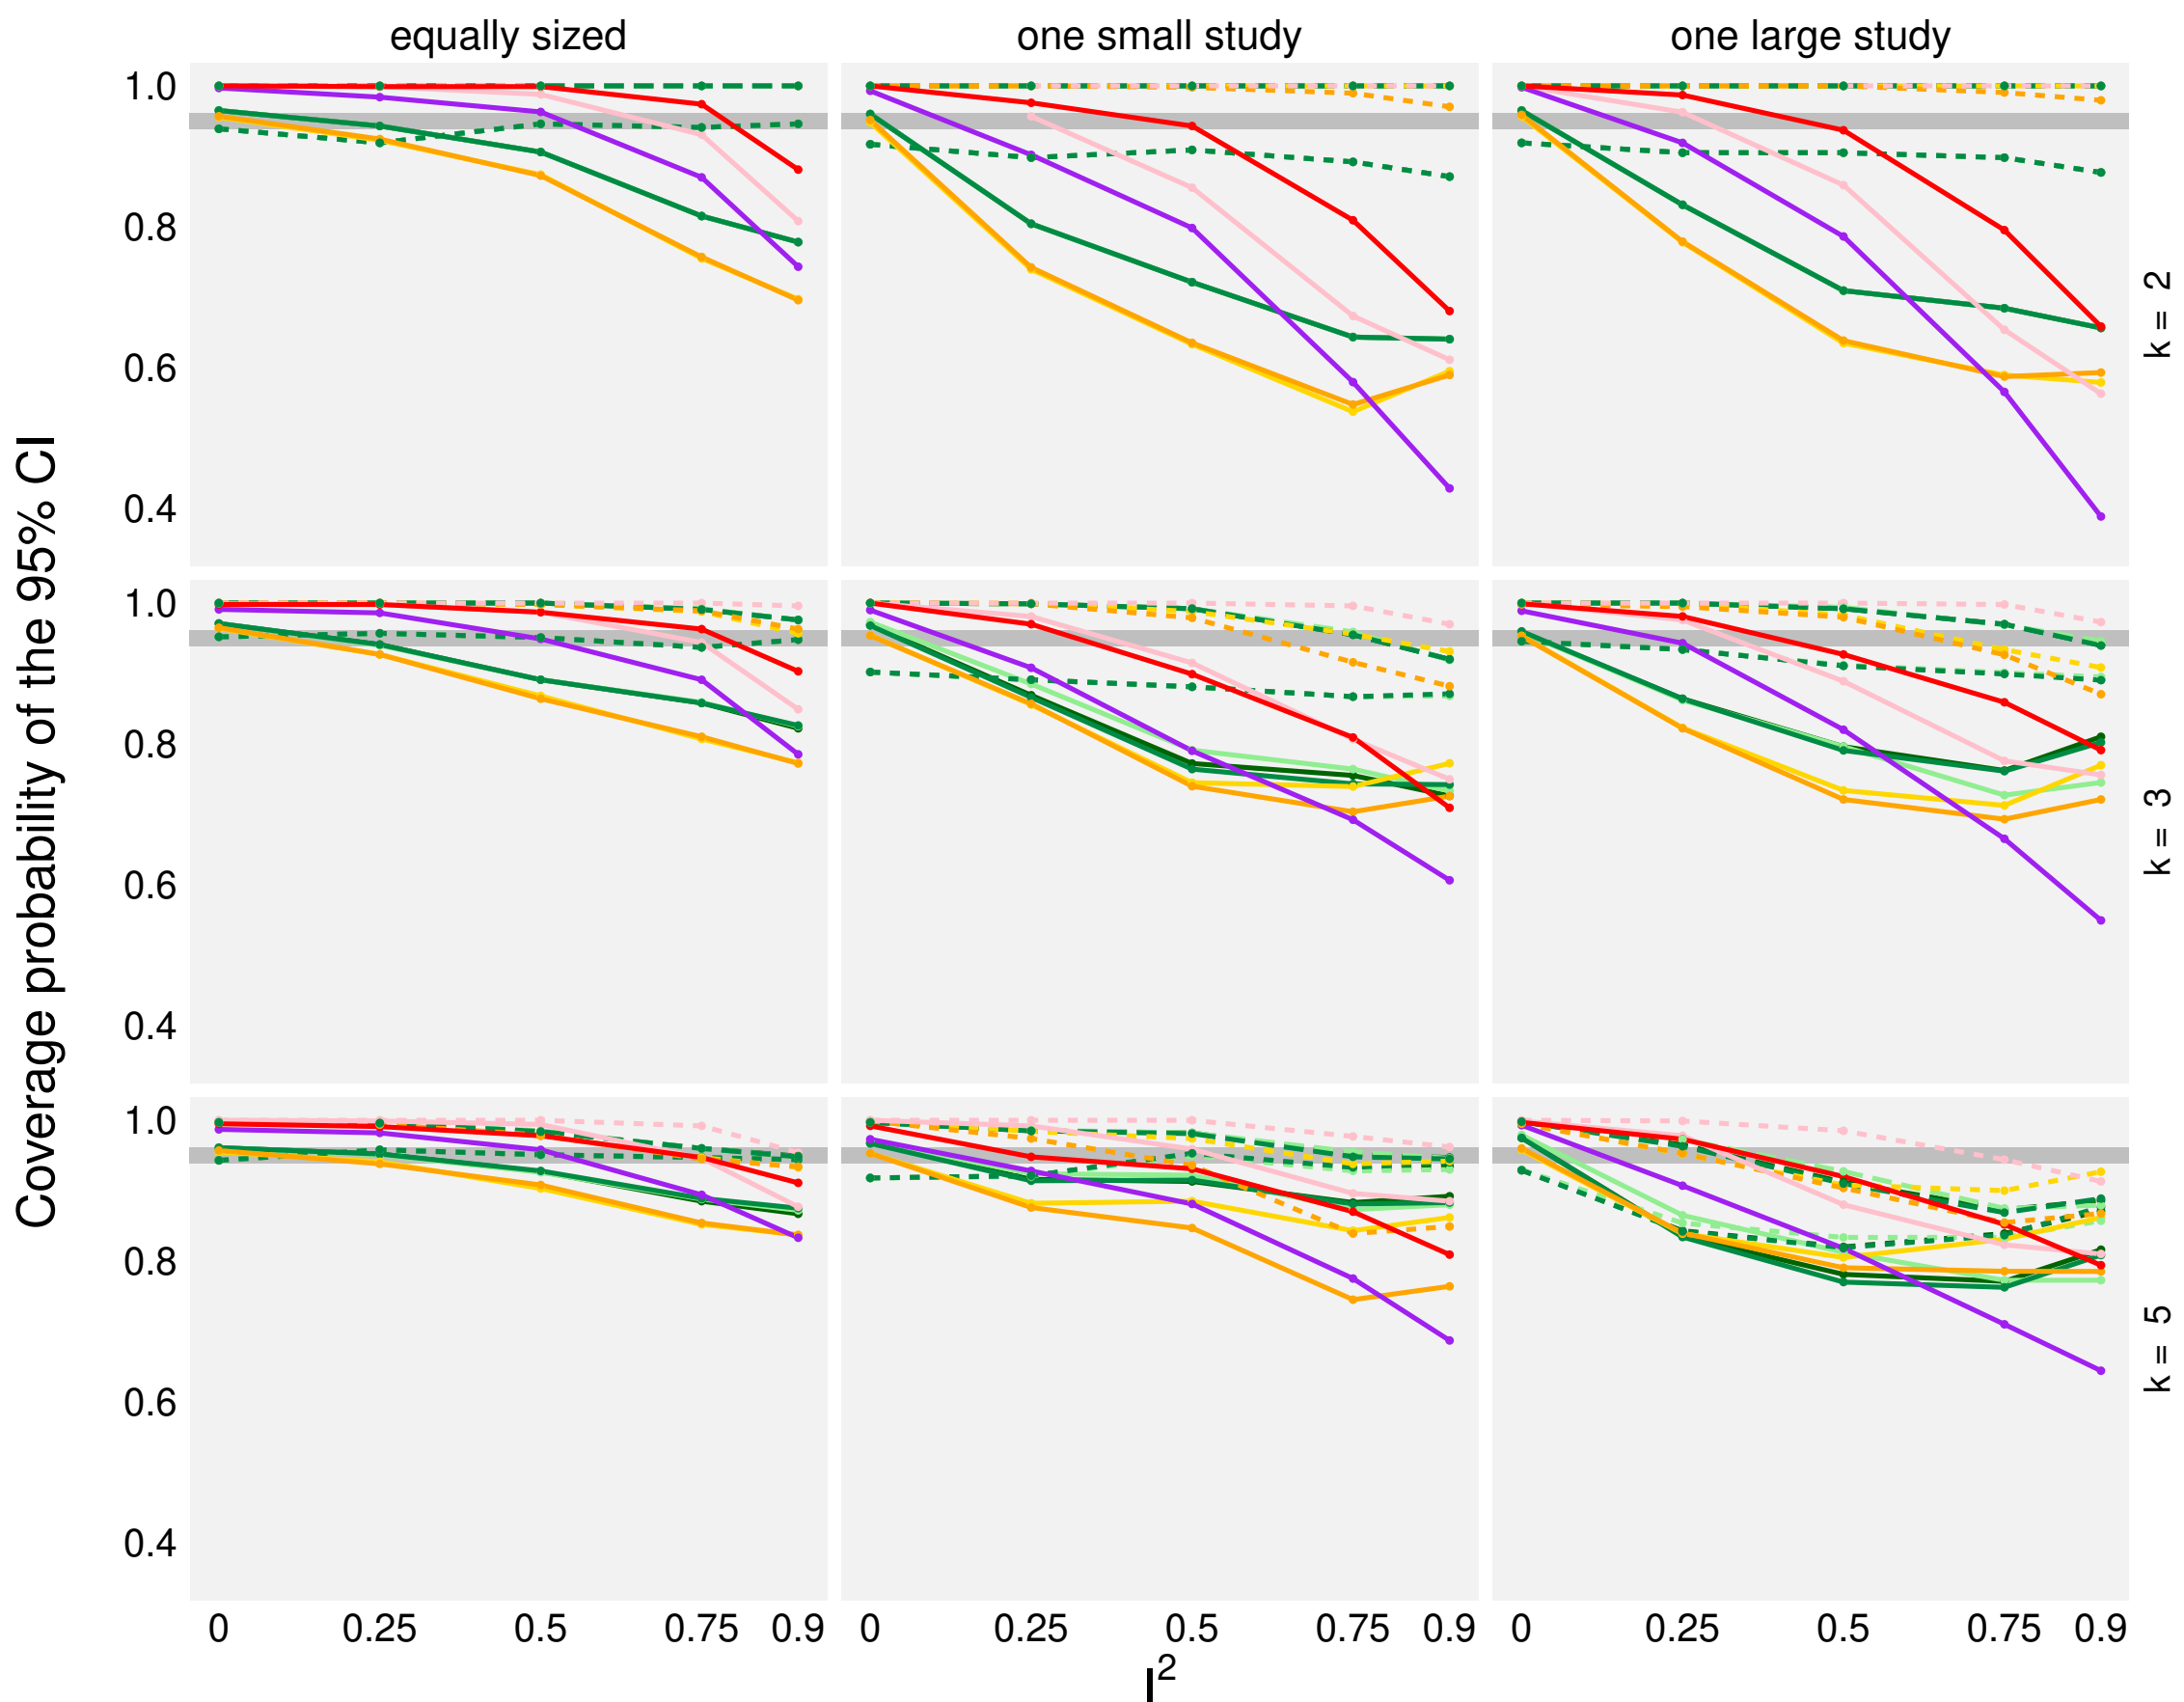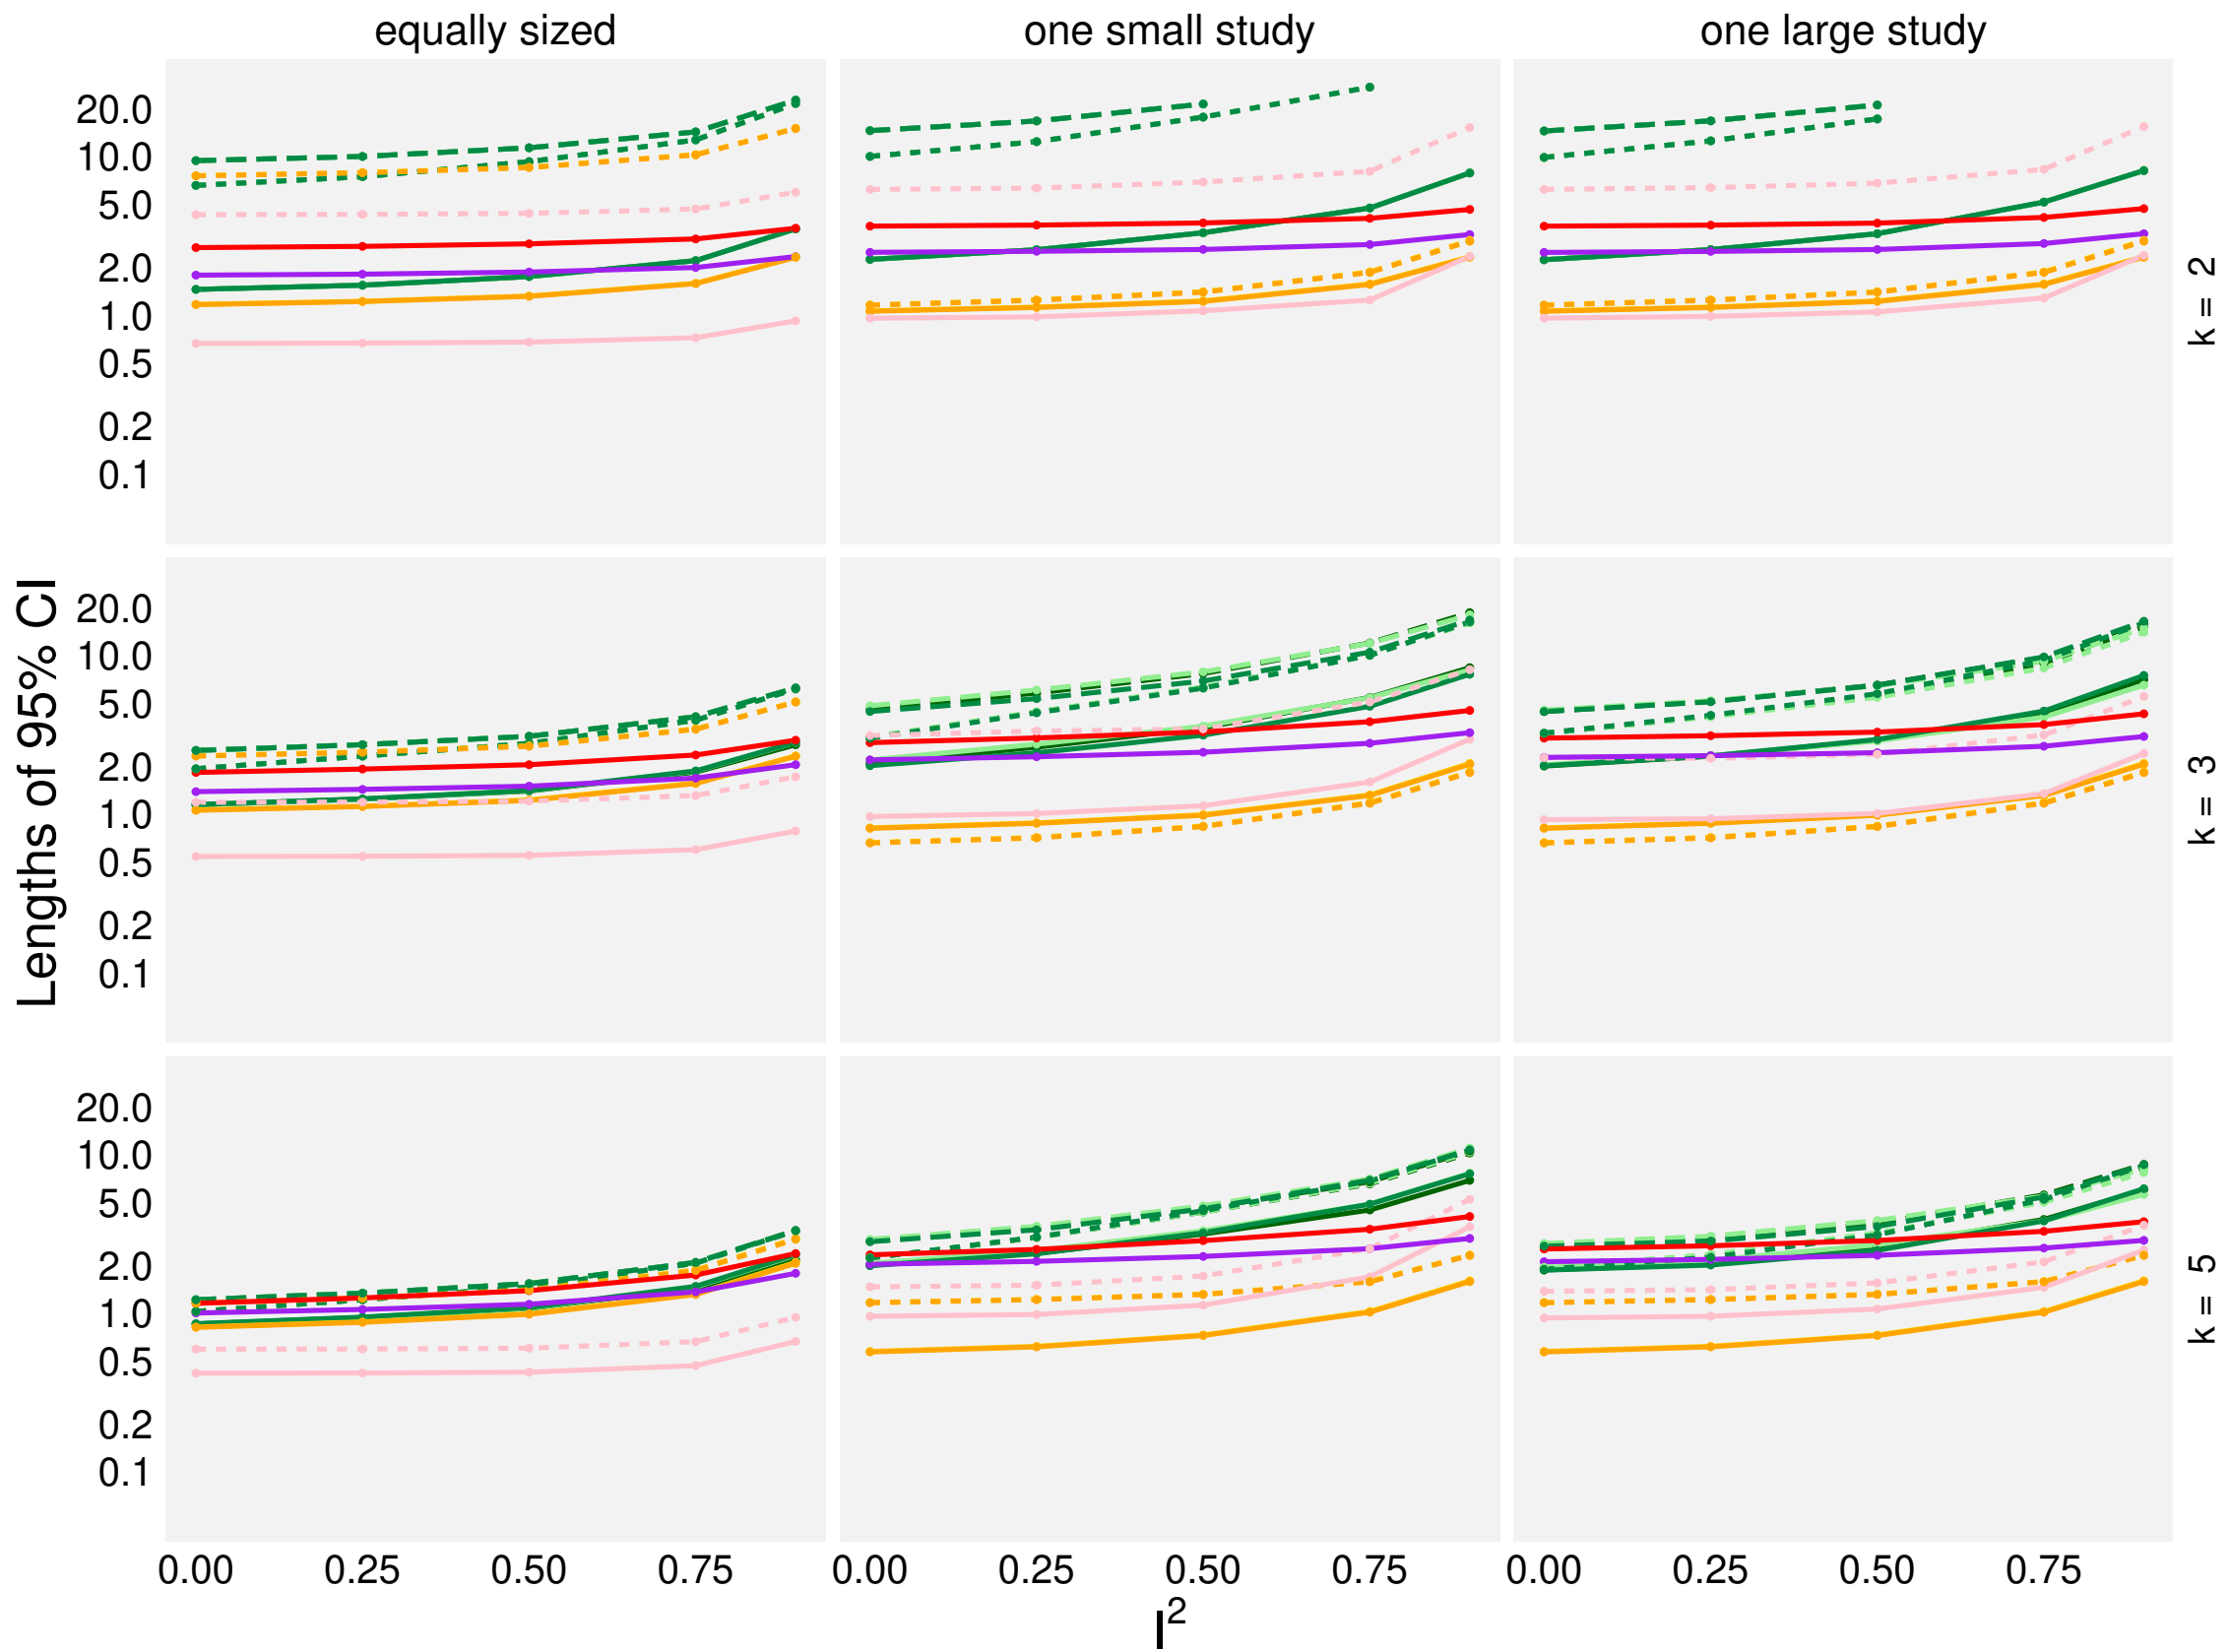

— NN — DL  
 — NN — REML  
 — NN — EB  
 — BN — UM.FS  
 — BN — UM.RS  
 — BN — CM.AL  
 — NN — Bayes HN(0.5)  
 — NN — Bayes HN(1)

— normal quantiles  
 -- HKSJ or Student's t  
 -- mHKSJ

OR  
( $n_i=50, \pi_0=0.9$ )

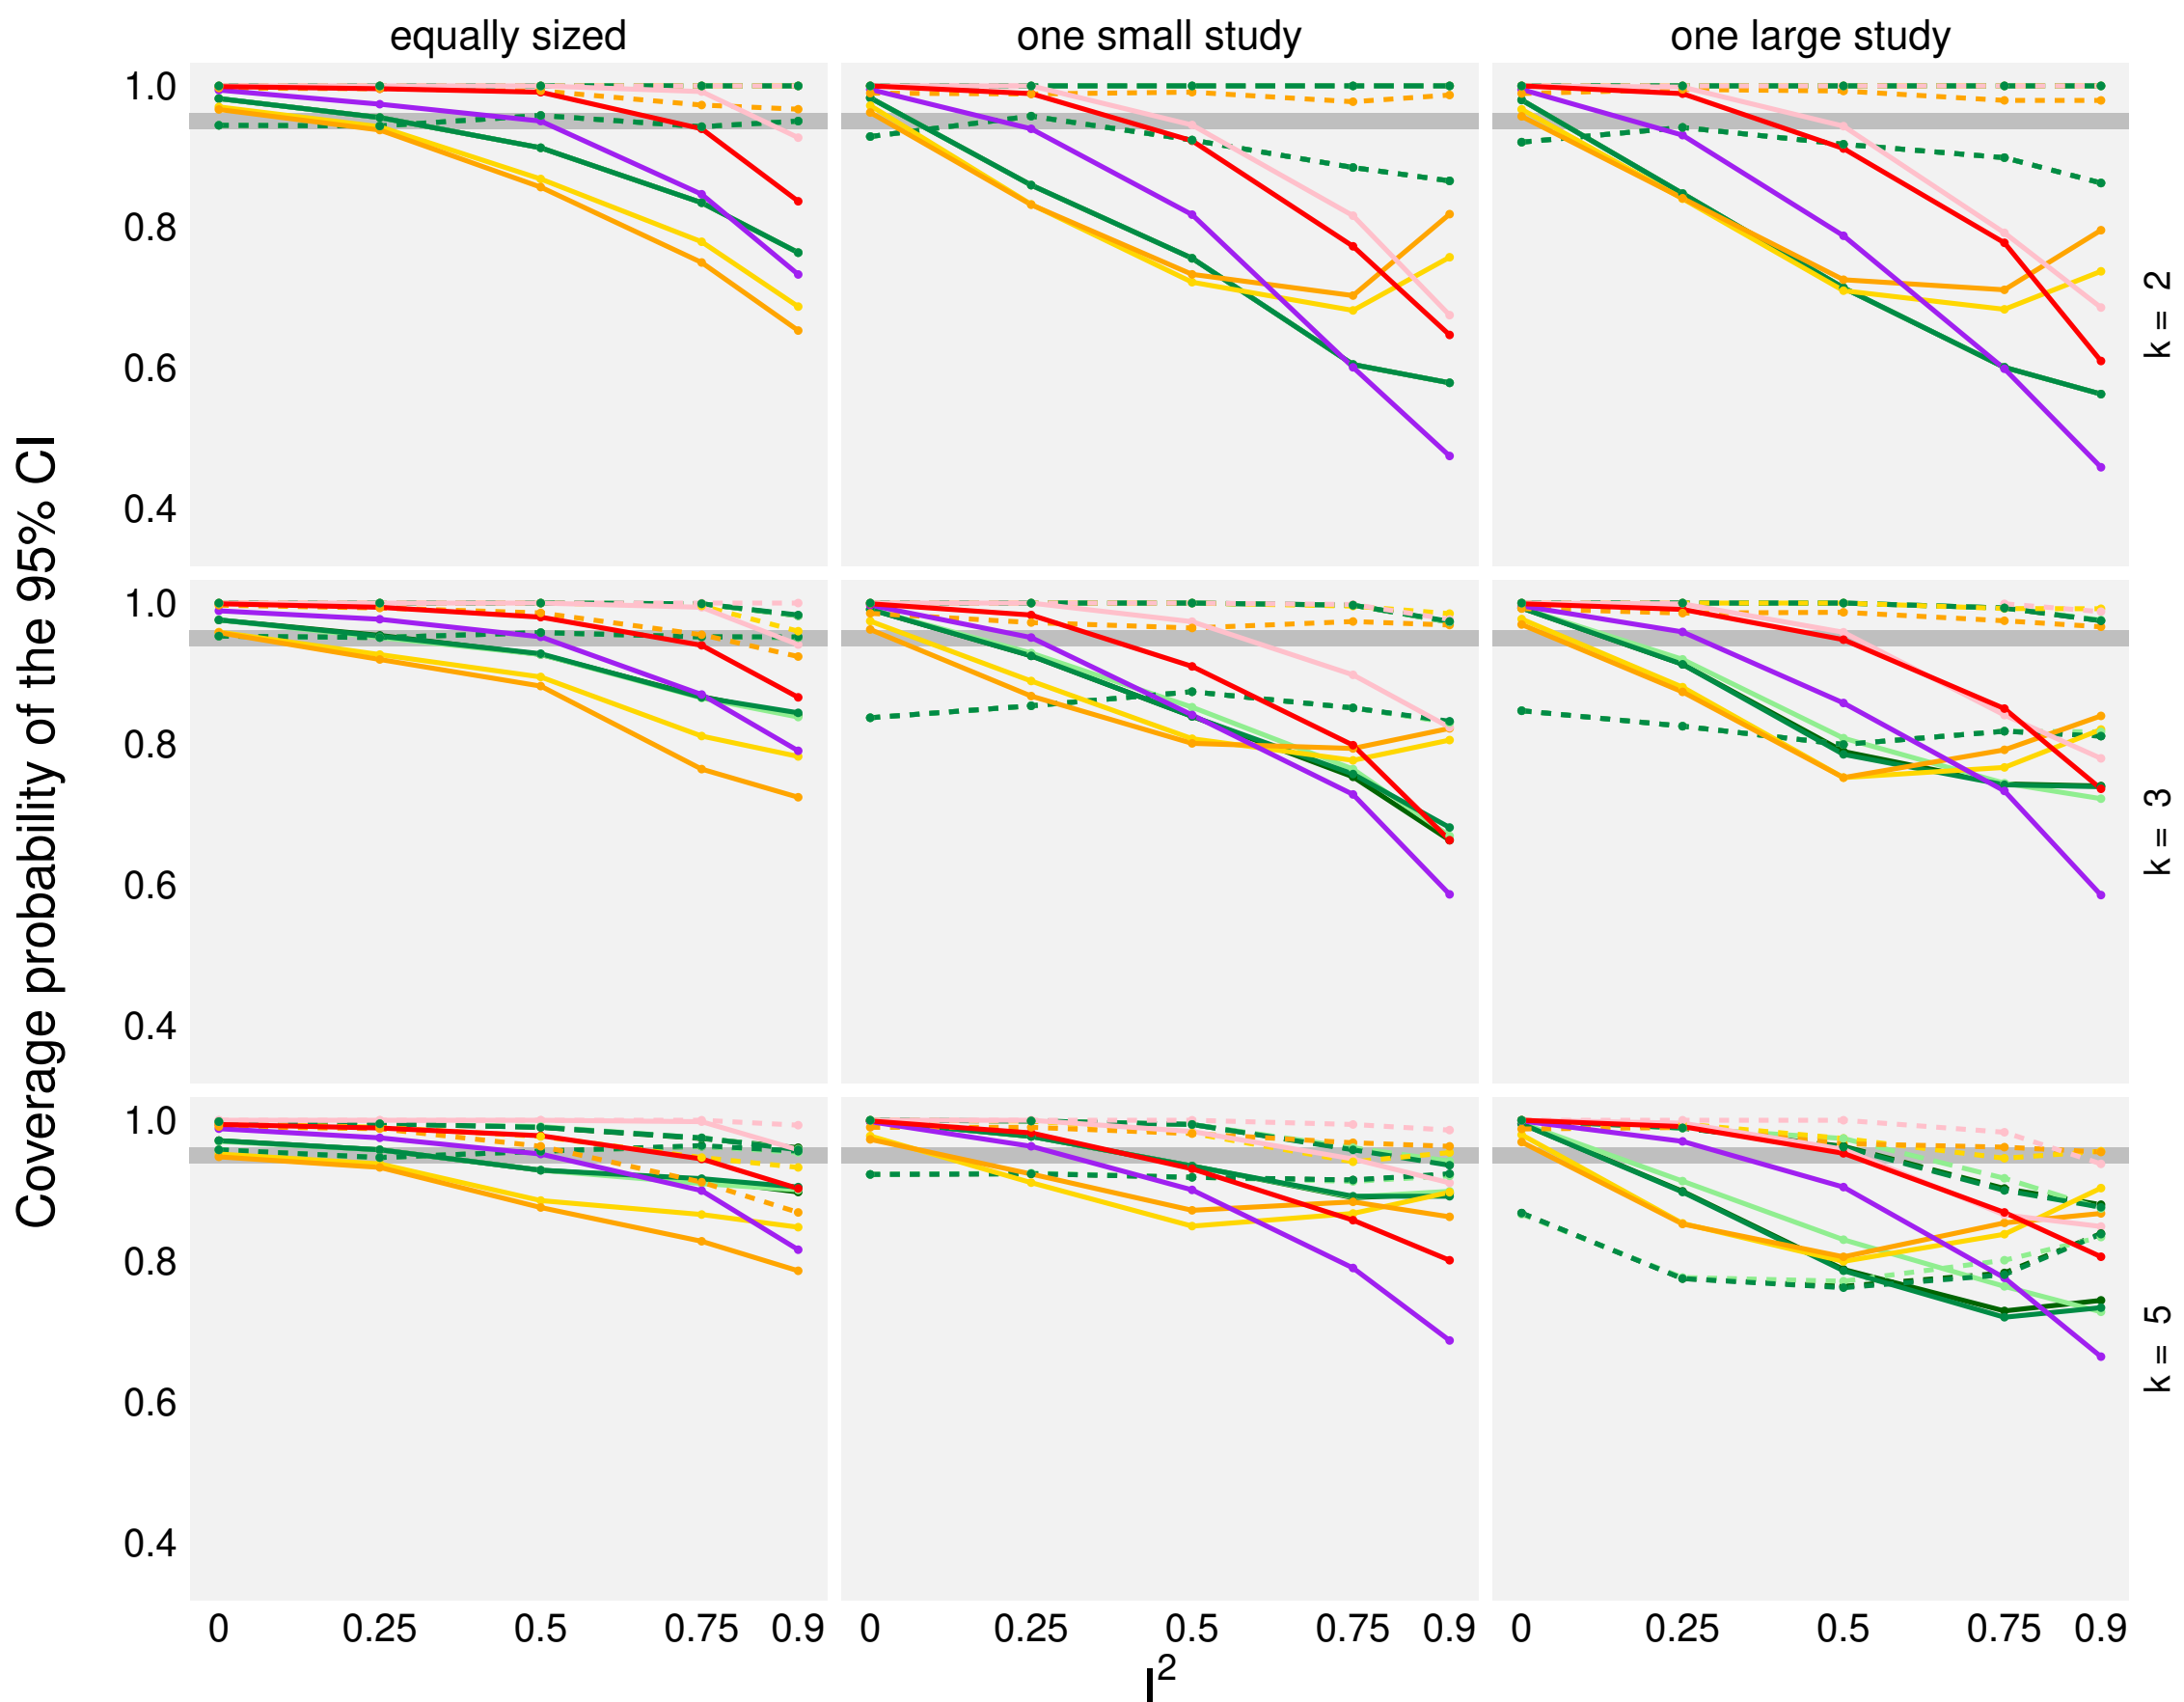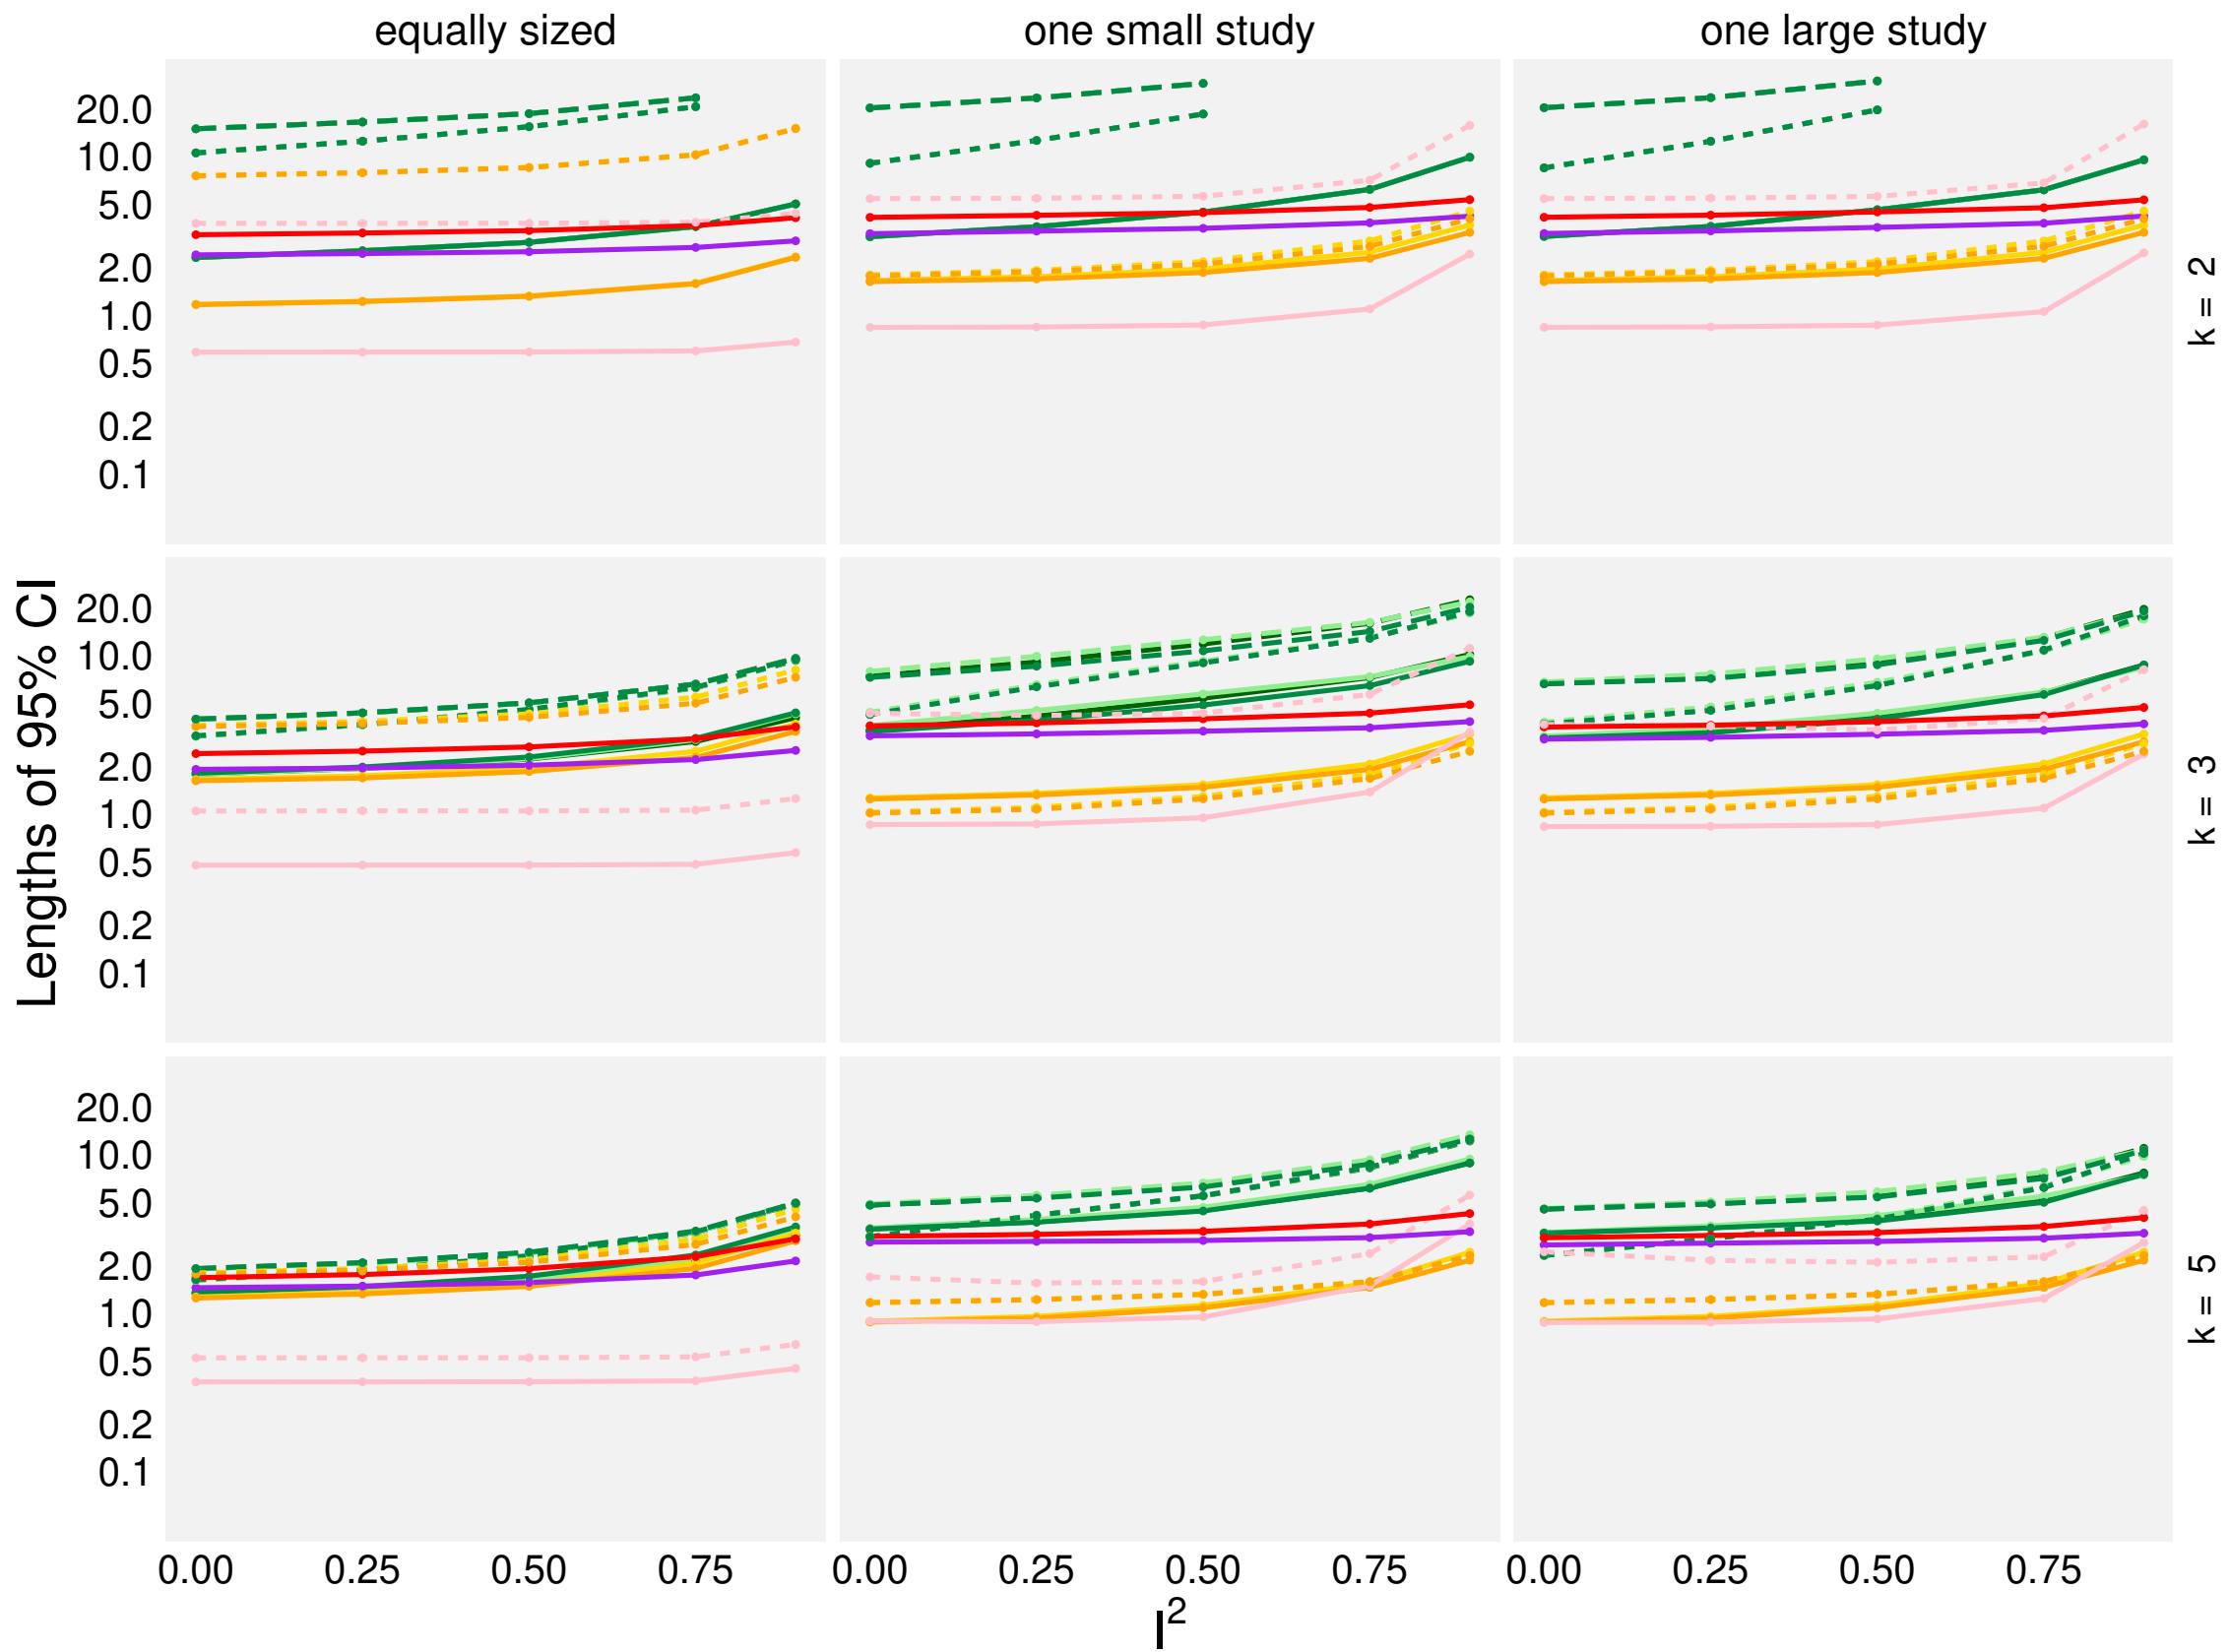

— NN — DL  
 — NN — REML  
 — NN — EB  
 — BN — UM.FS  
 — BN — UM.RS  
 — BN — CM.AL  
 — NN — Bayes HN(0.5)  
 — NN — Bayes HN(1)

— normal quantiles  
 - - HKSJ or Student's t  
 - - mHKSJ

OR

( $n_i=100, \pi_0=0.1$ )

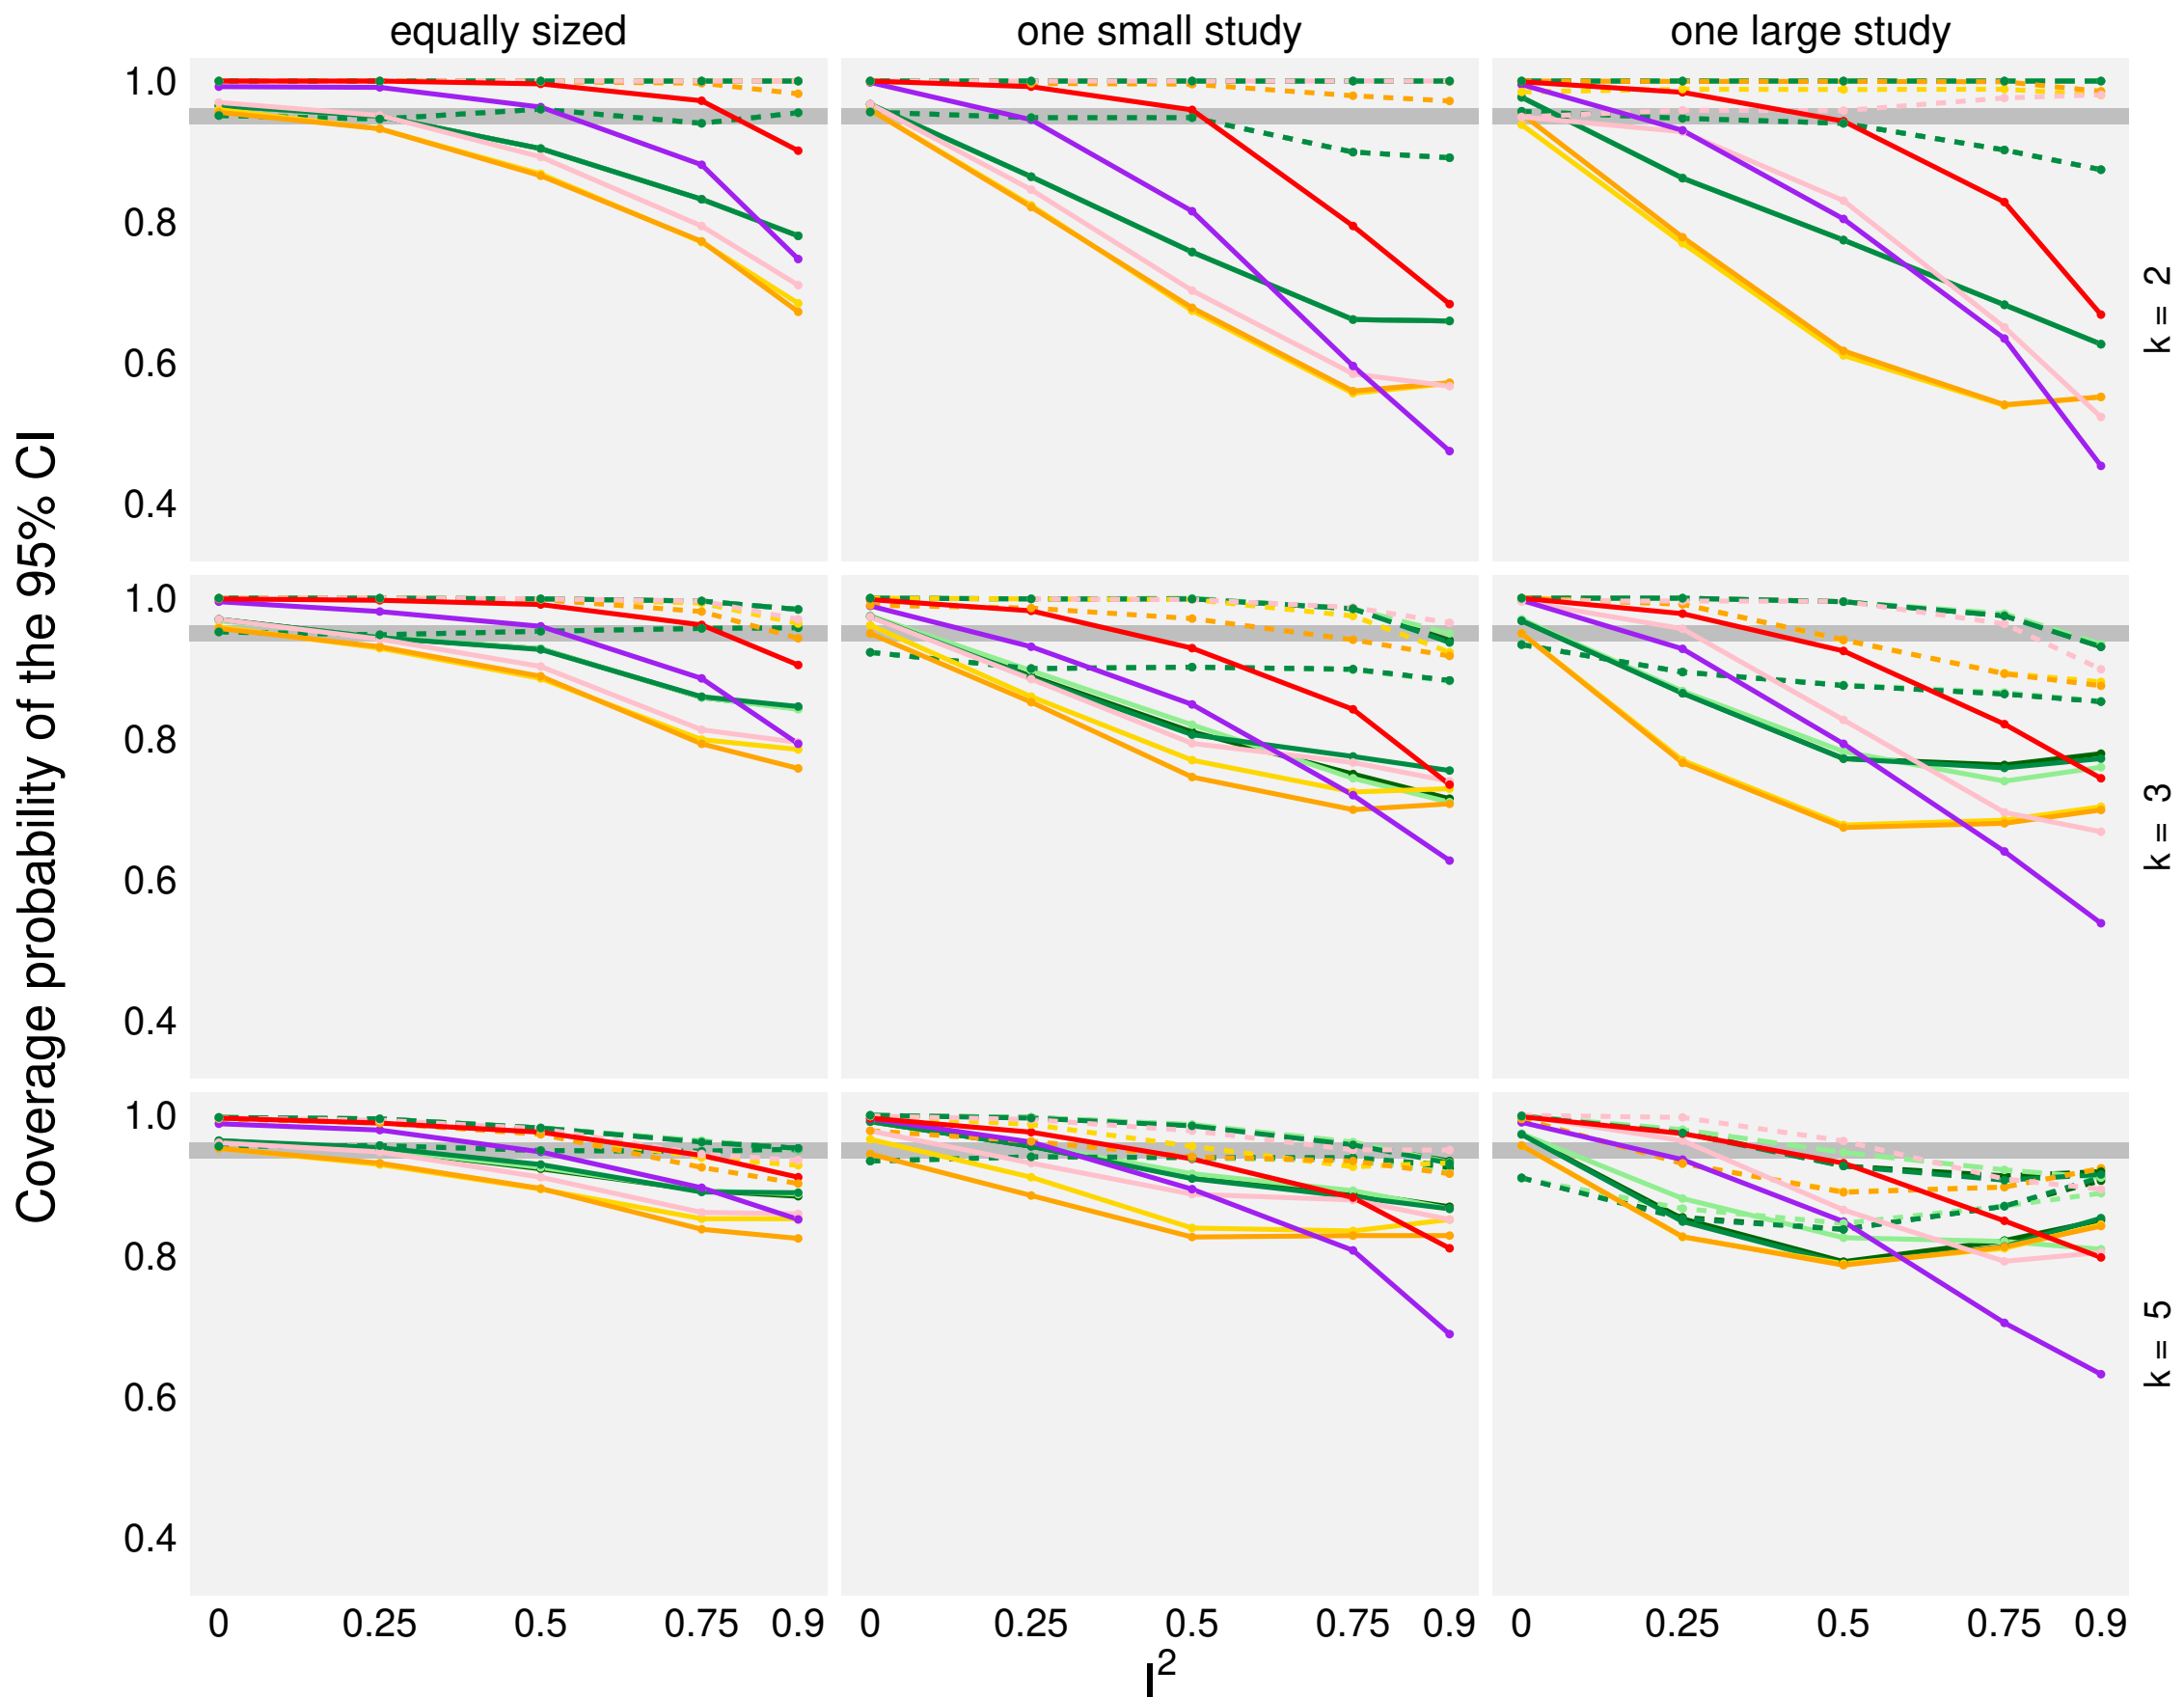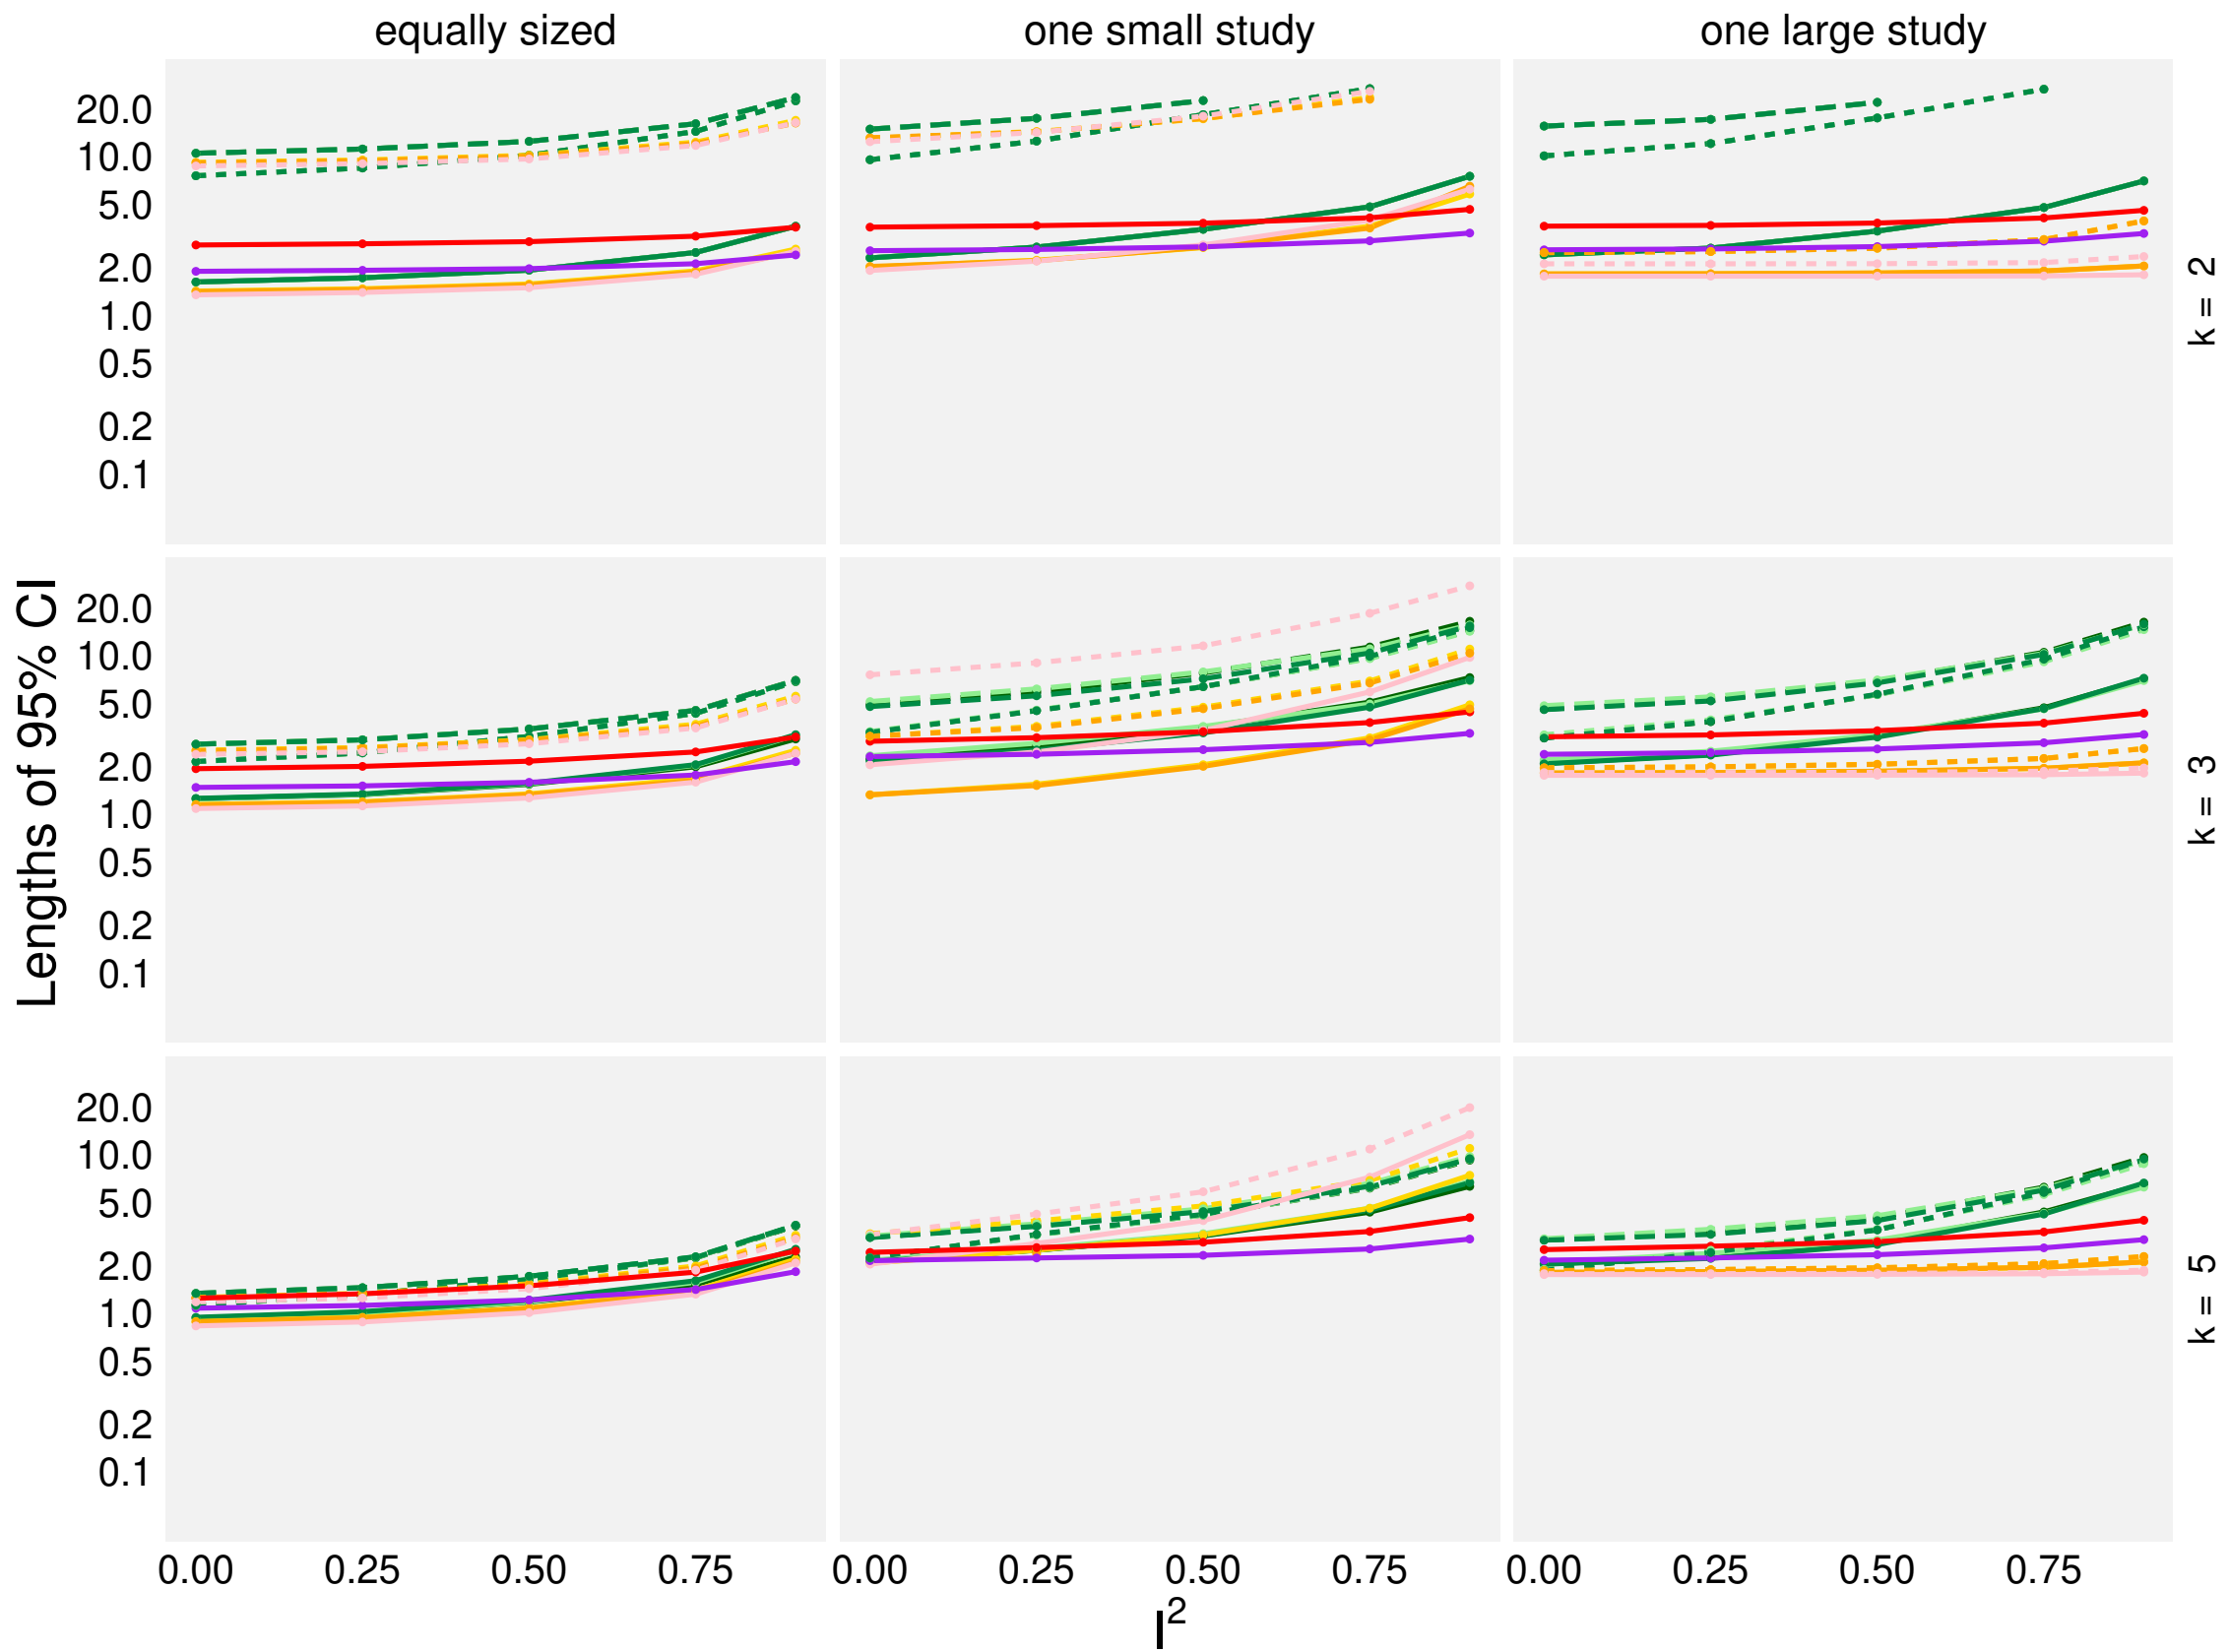

— NN — DL  
 — NN — REML  
 — NN — EB  
 — BN — UM.FS  
 — BN — UM.RS  
 — BN — CM.AL  
 — NN — Bayes HN(0.5)  
 — NN — Bayes HN(1)

— normal quantiles  
 -- HKSJ or Student's t  
 -·- mHKSJ

OR  
( $n_i=100, \pi_0=0.3$ )

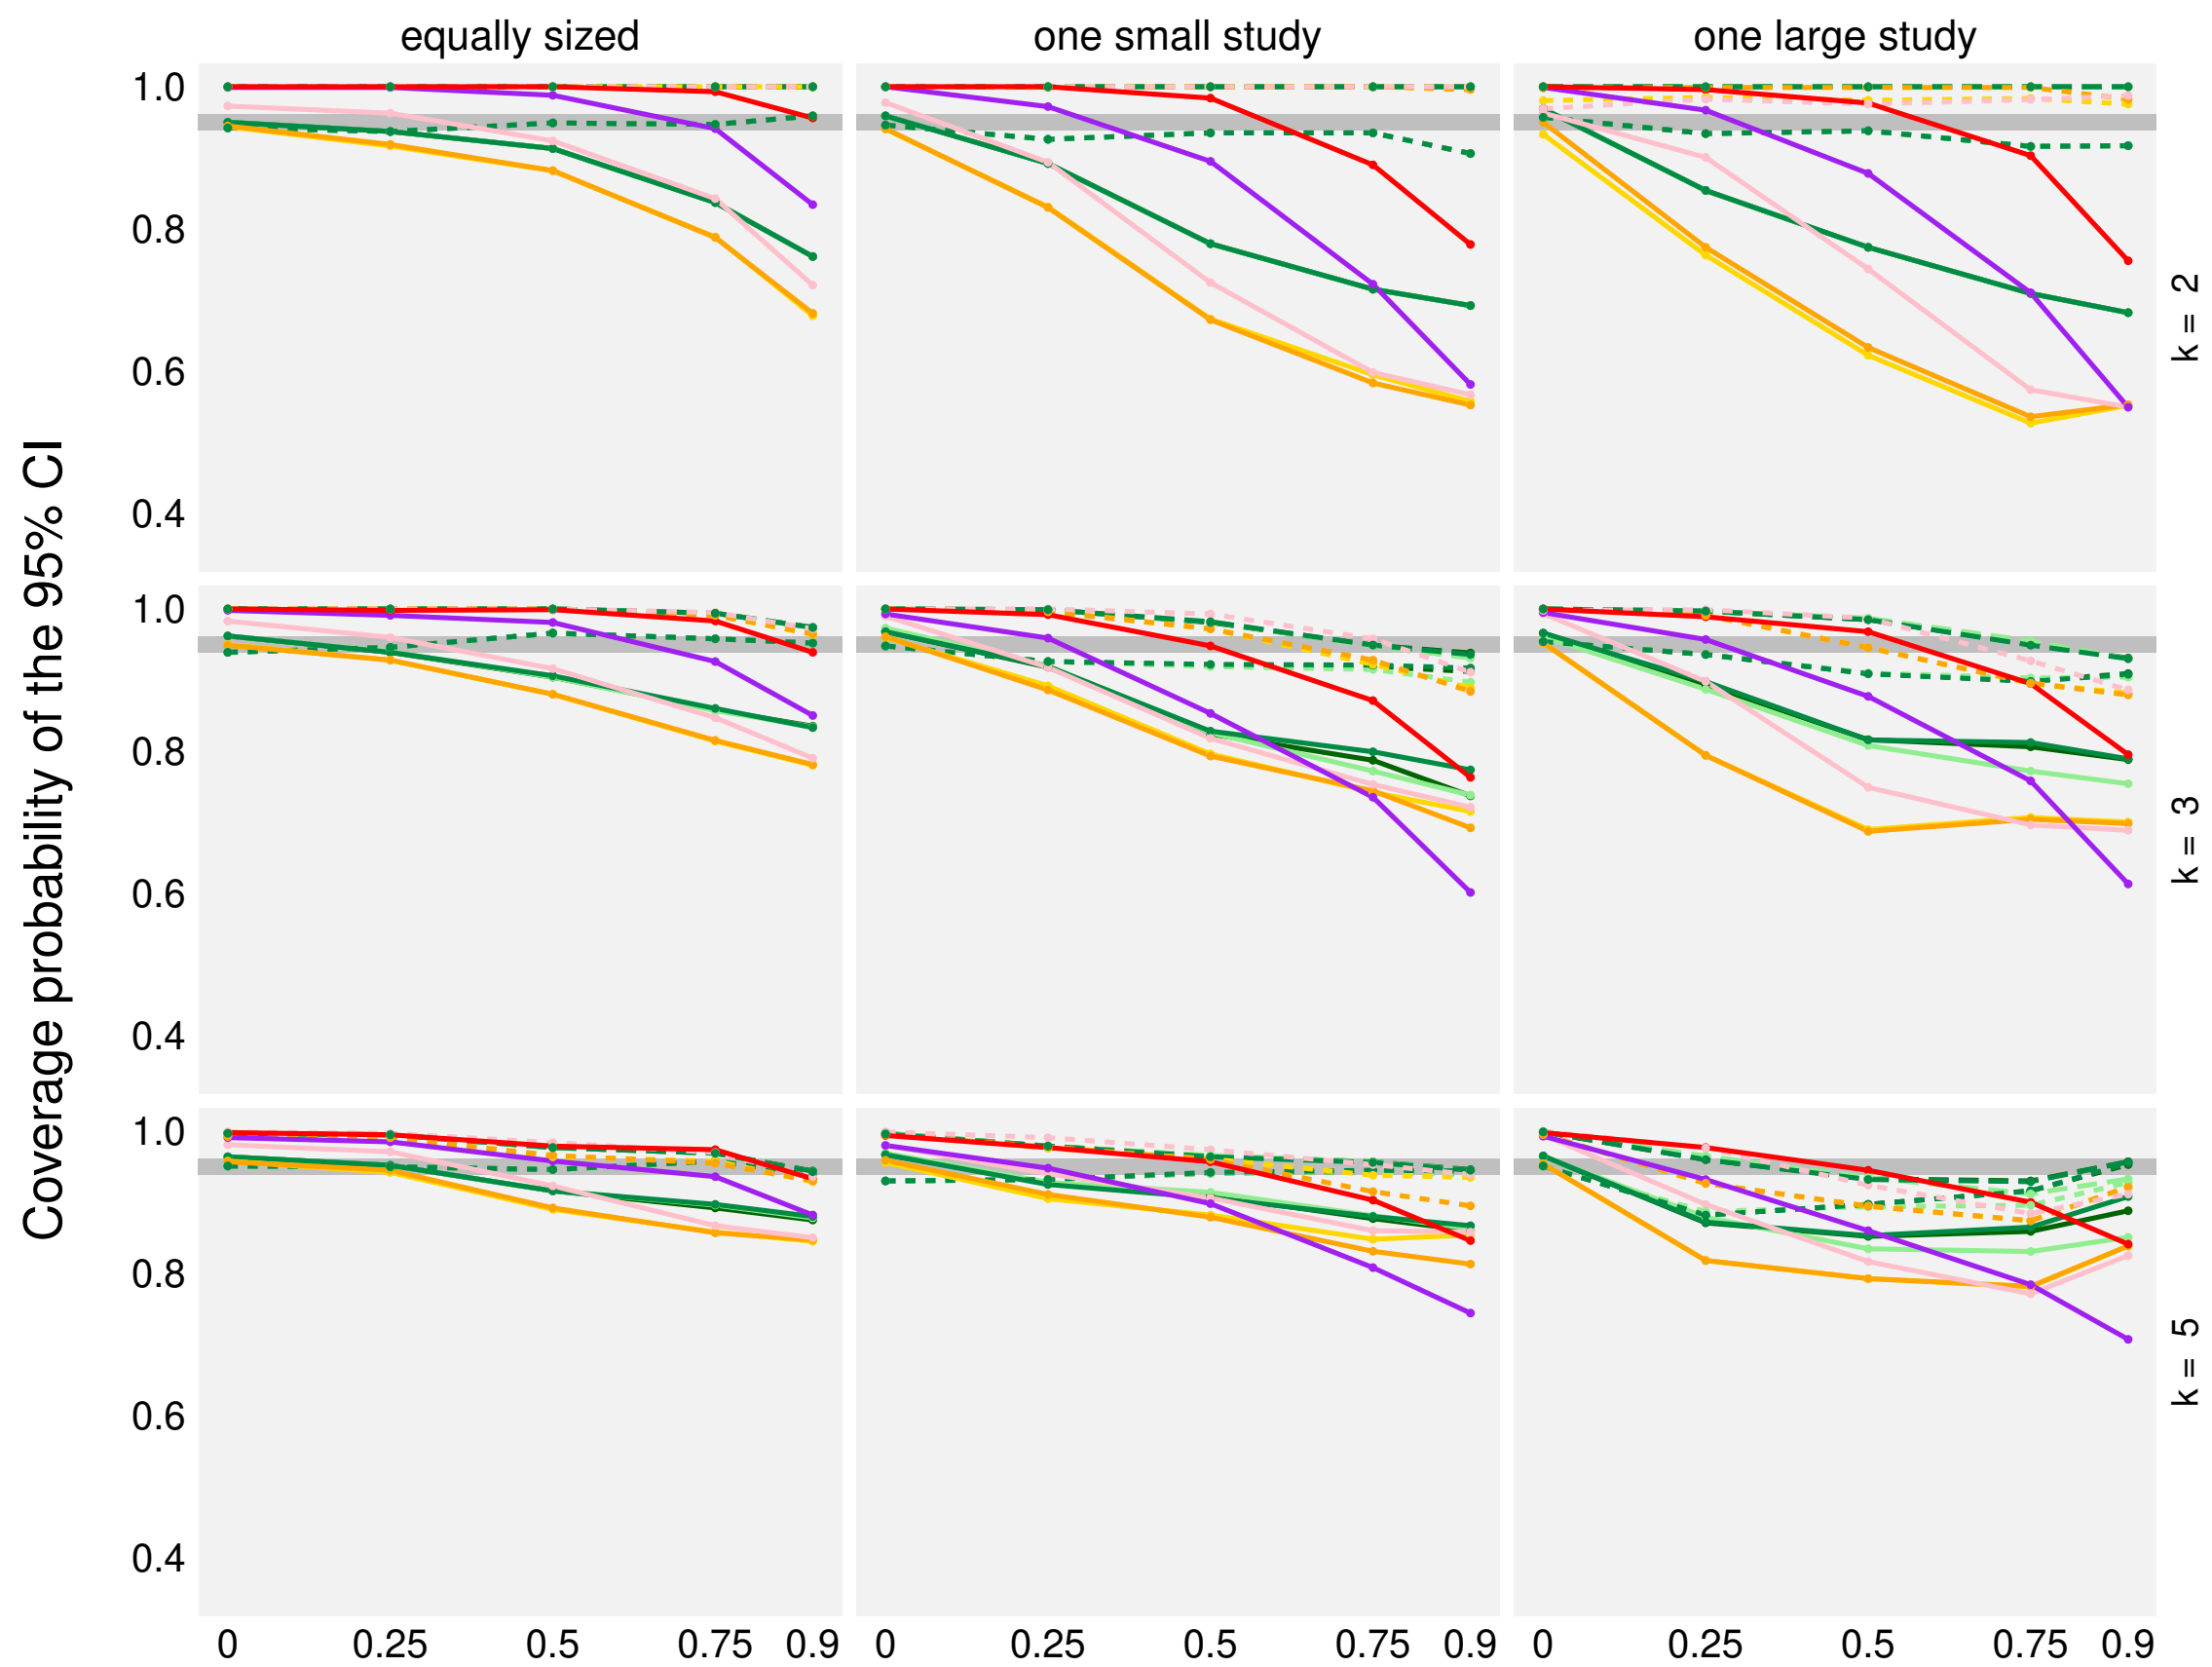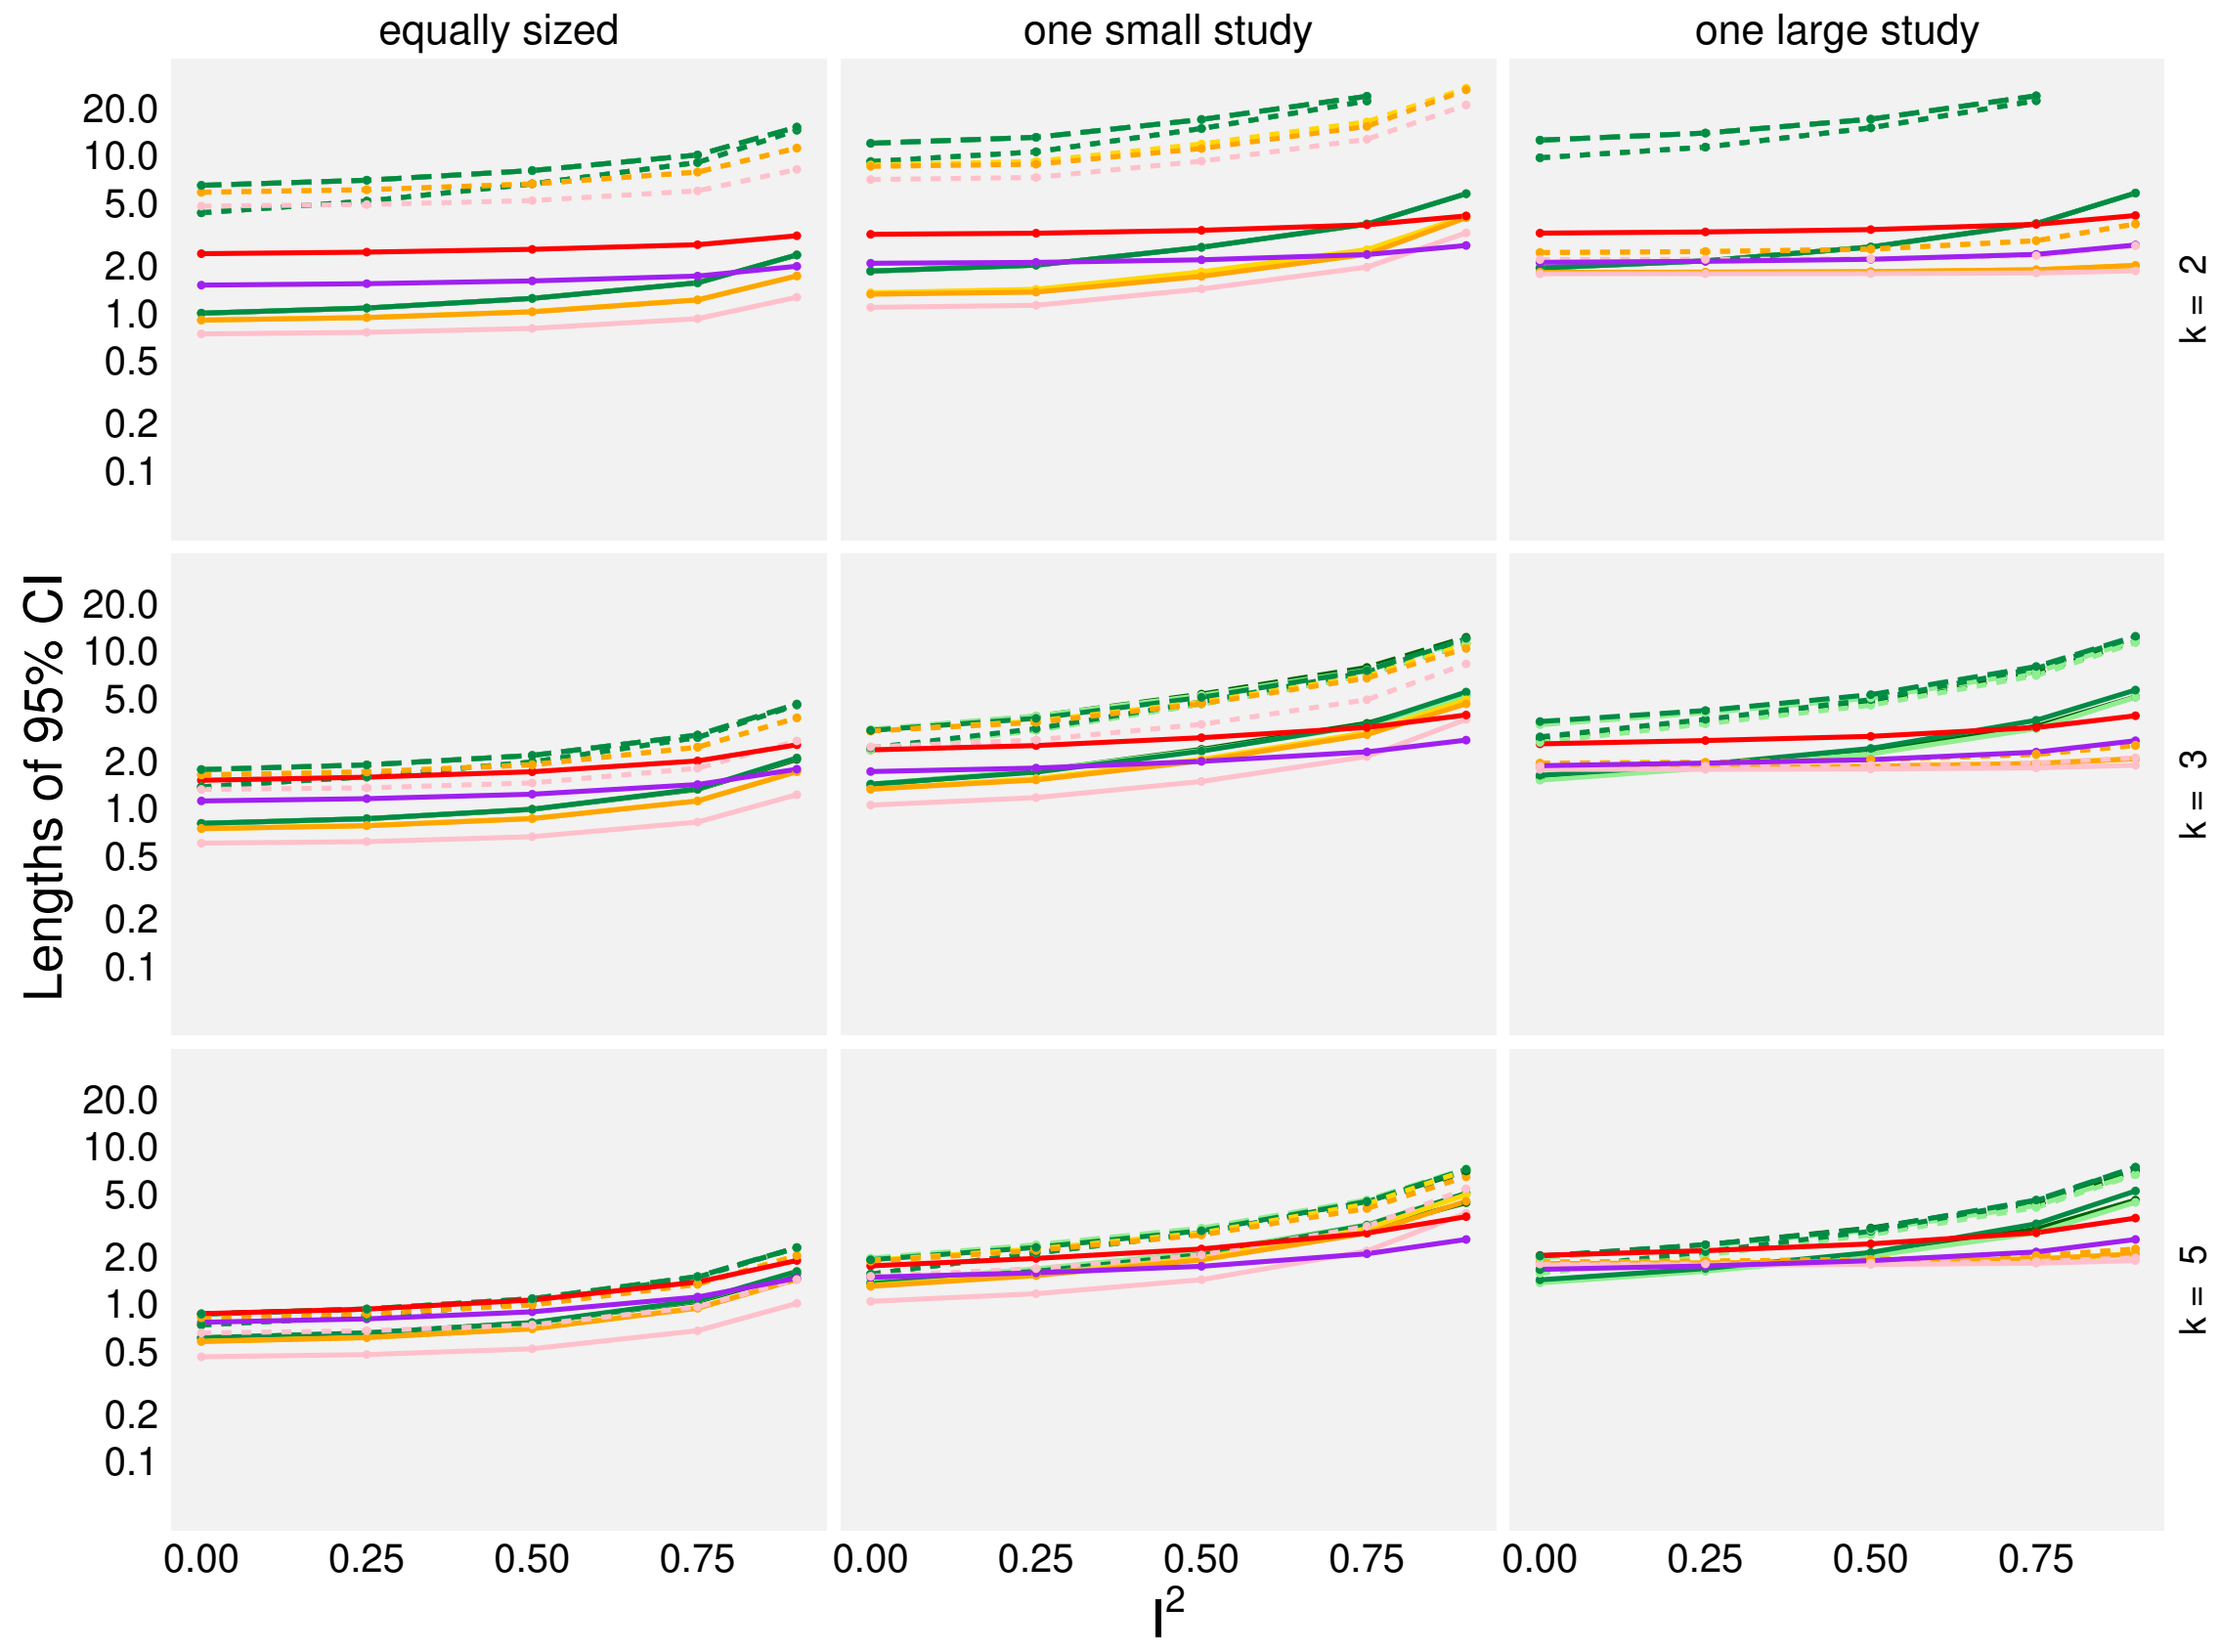

— NN – DL      — BN – UM.RS      — normal quantiles  
 — NN – REML      — BN – CM.AL      -- HKSJ or Student's t  
 — NN – EB      — NN – Bayes HN(0.5)      -- mHKSJ  
 — BN – UM.FS      — NN – Bayes HN(1)

OR  
( $n_i=100, \pi_0=0.5$ )

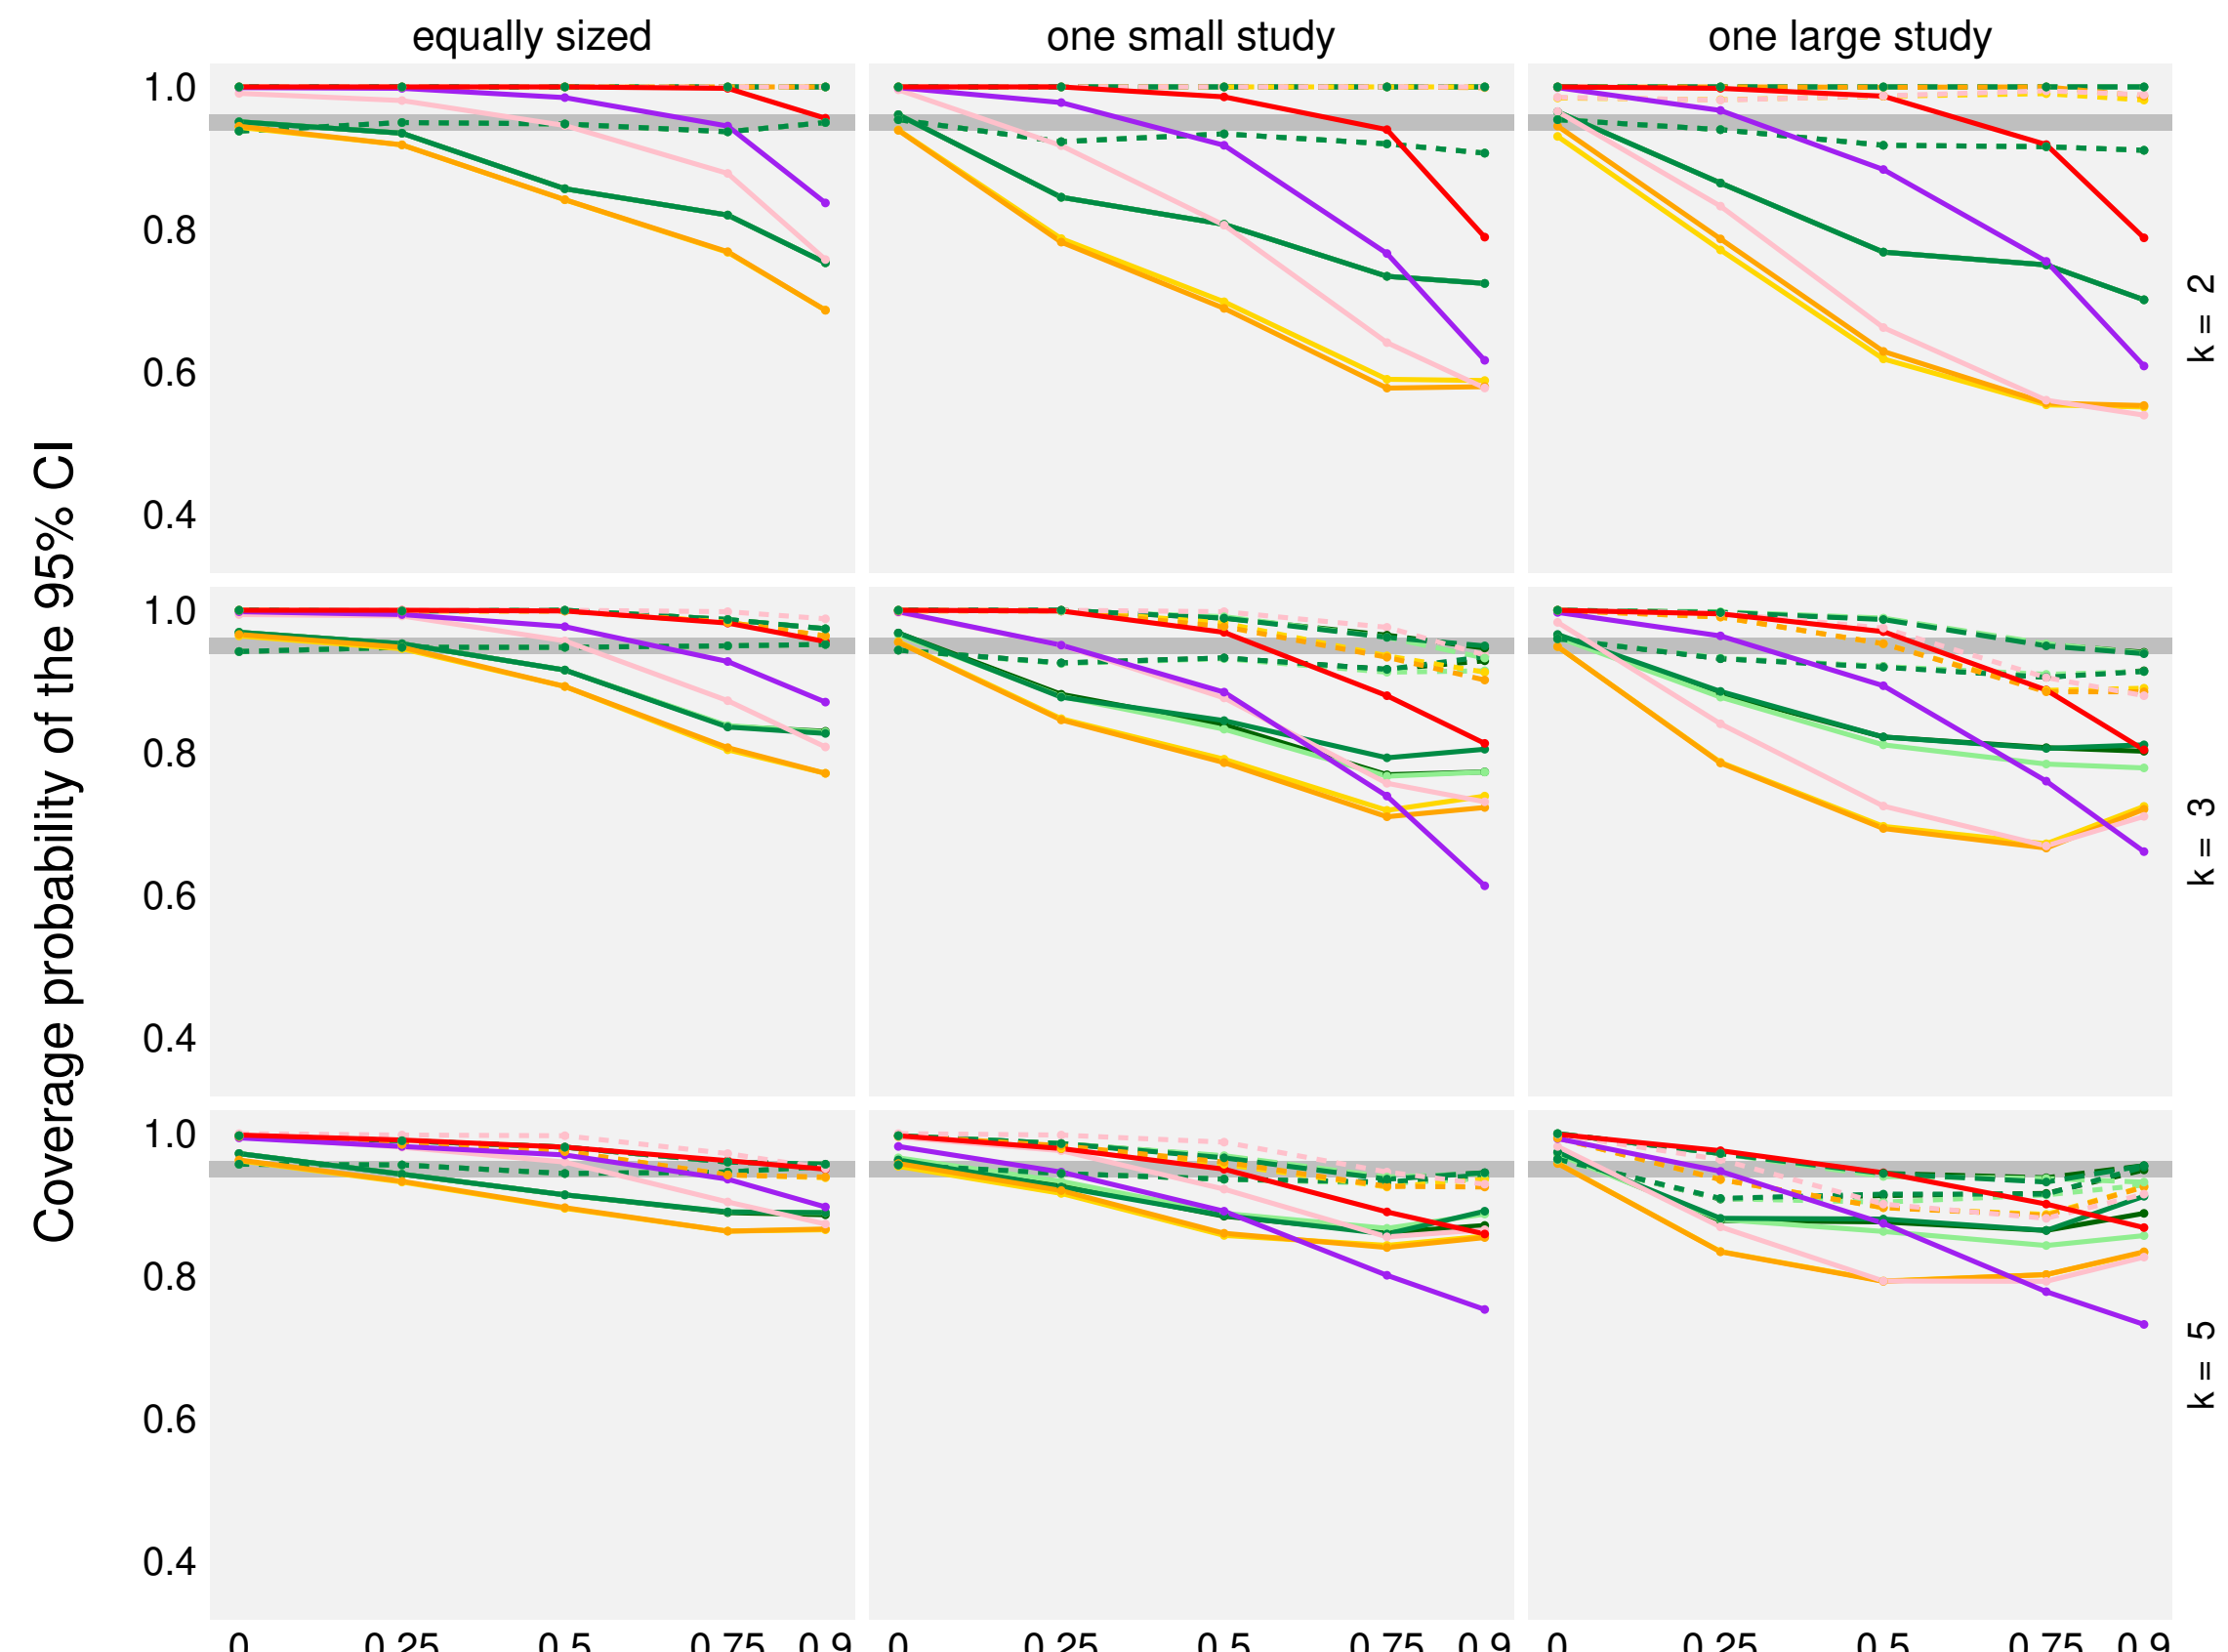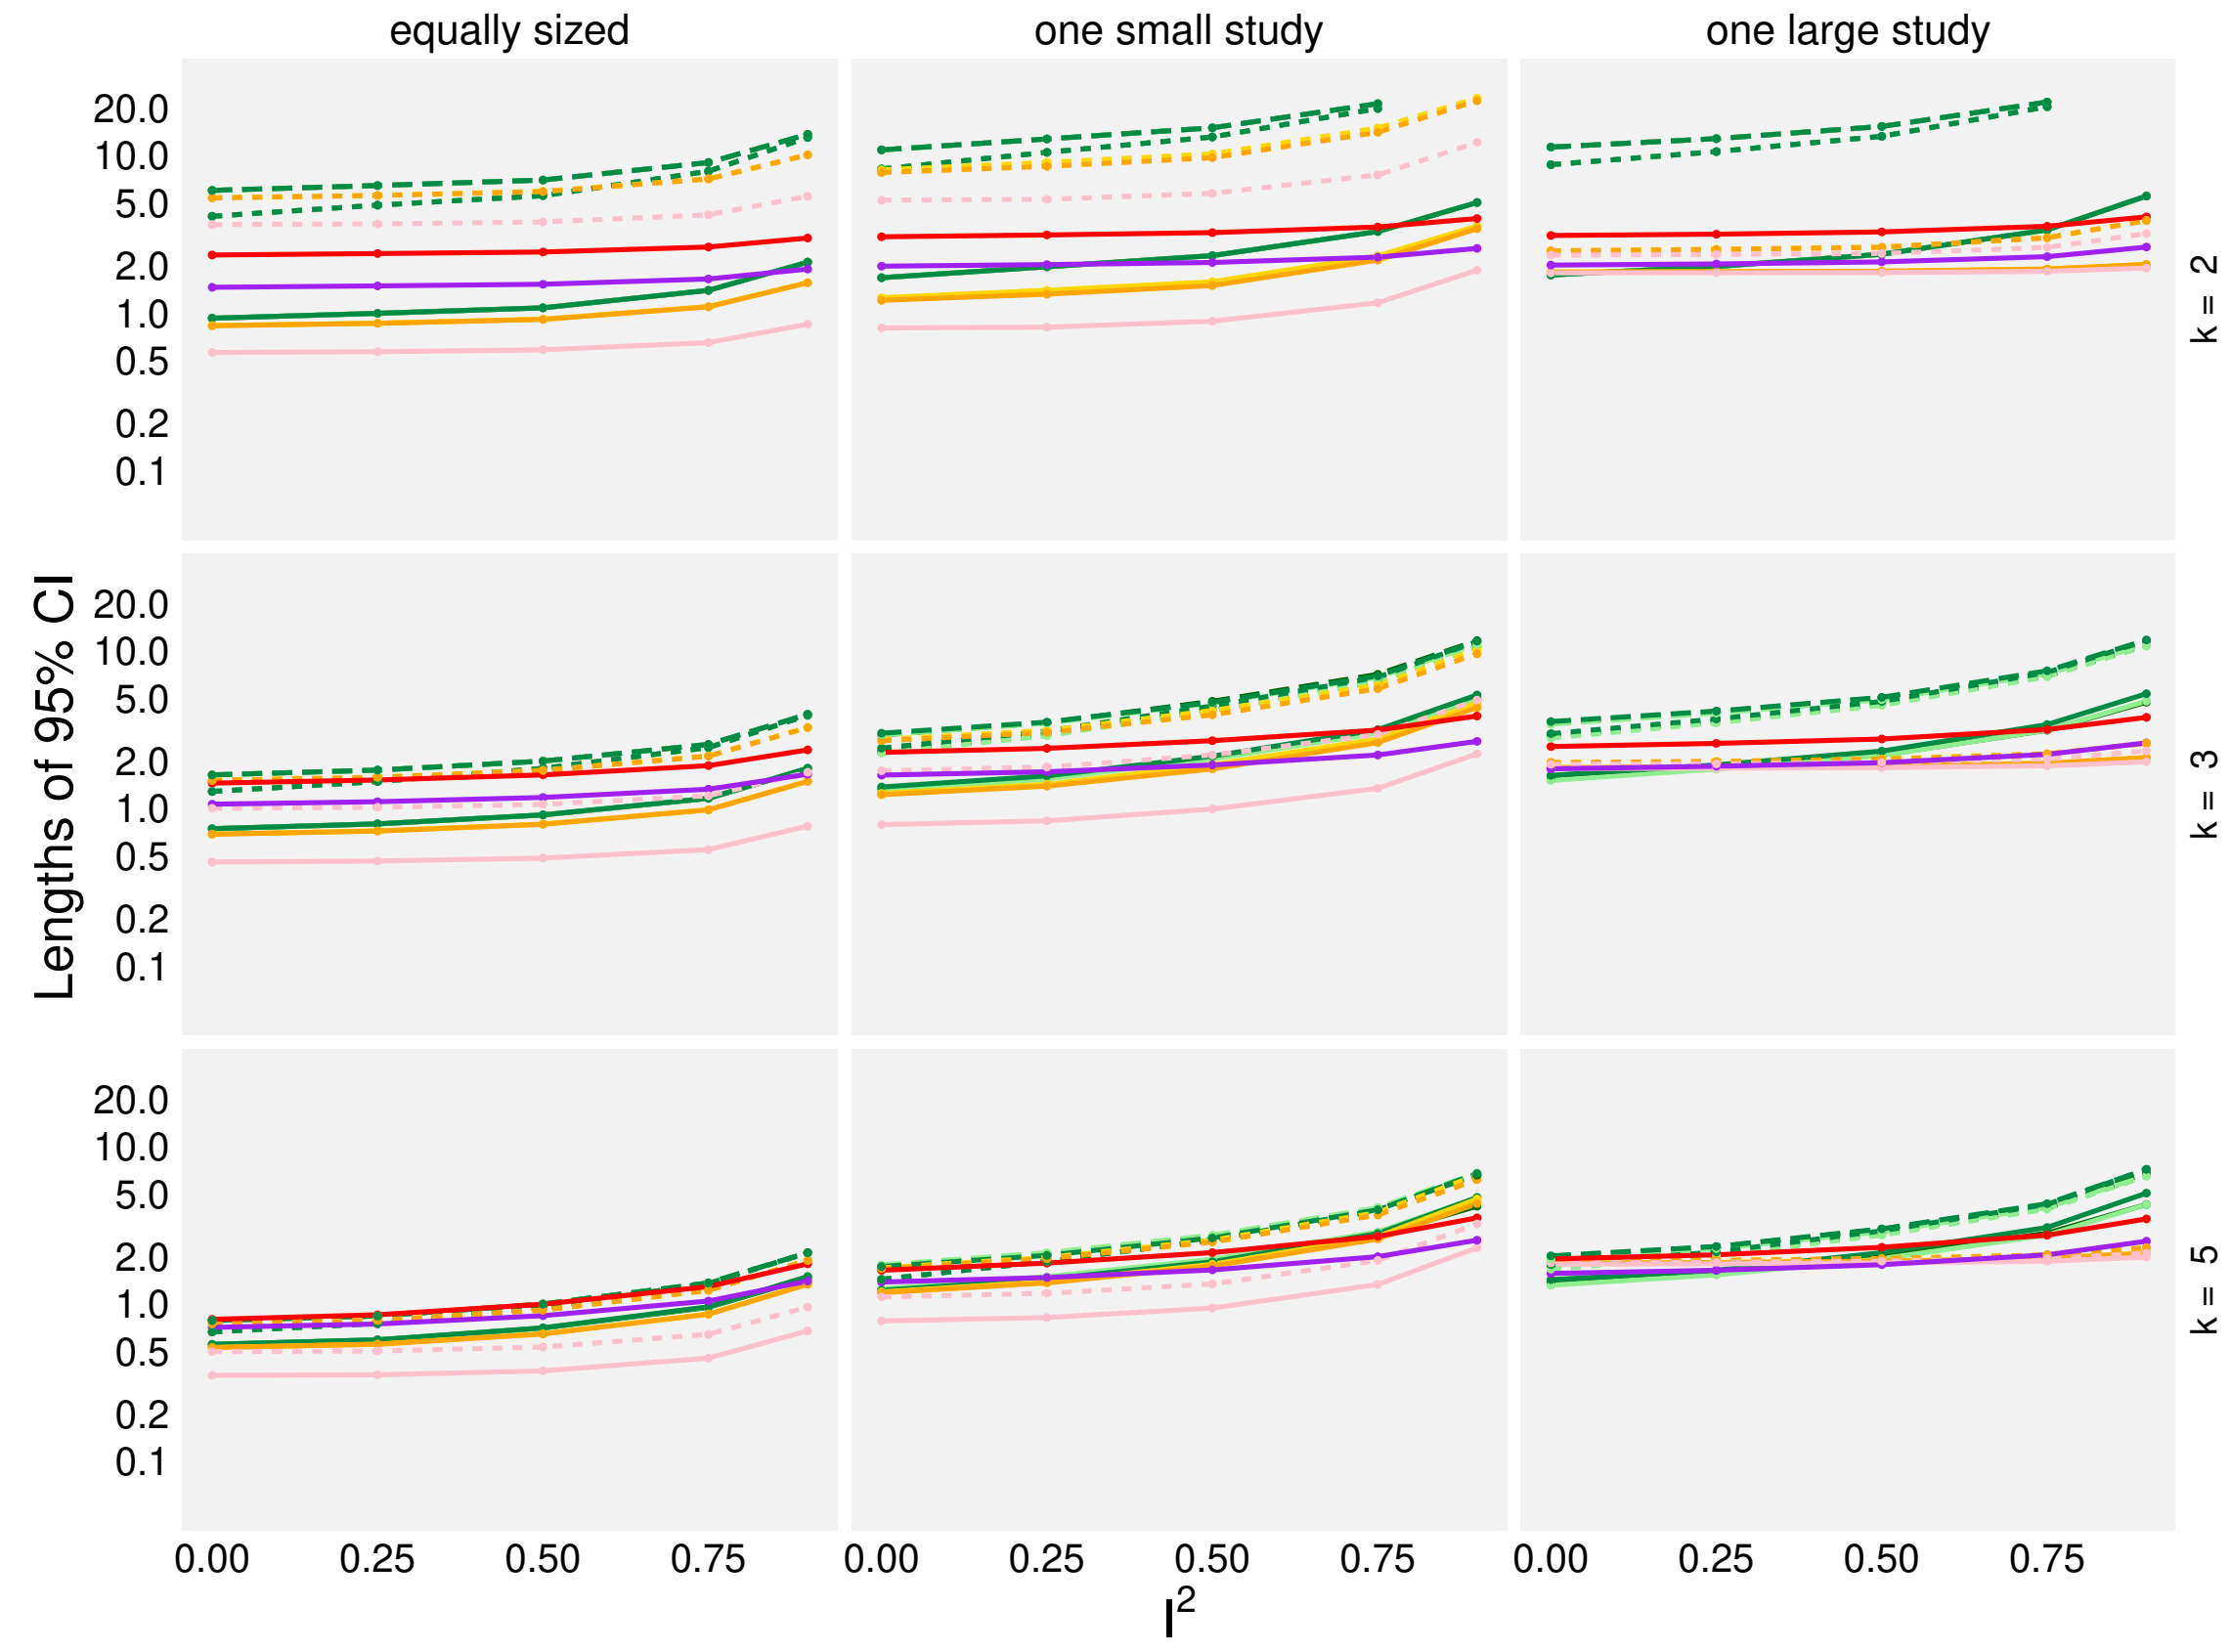

— NN — DL      — BN — UM.RS      — normal quantiles  
 — NN — REML      — BN — CM.AL      - - HKSJ or Student's t  
 — NN — EB      — NN — Bayes HN(0.5)      - · mHKSJ  
 — BN — UM.FS      — NN — Bayes HN(1)

OR  
( $n_i=100, \pi_0=0.7$ )

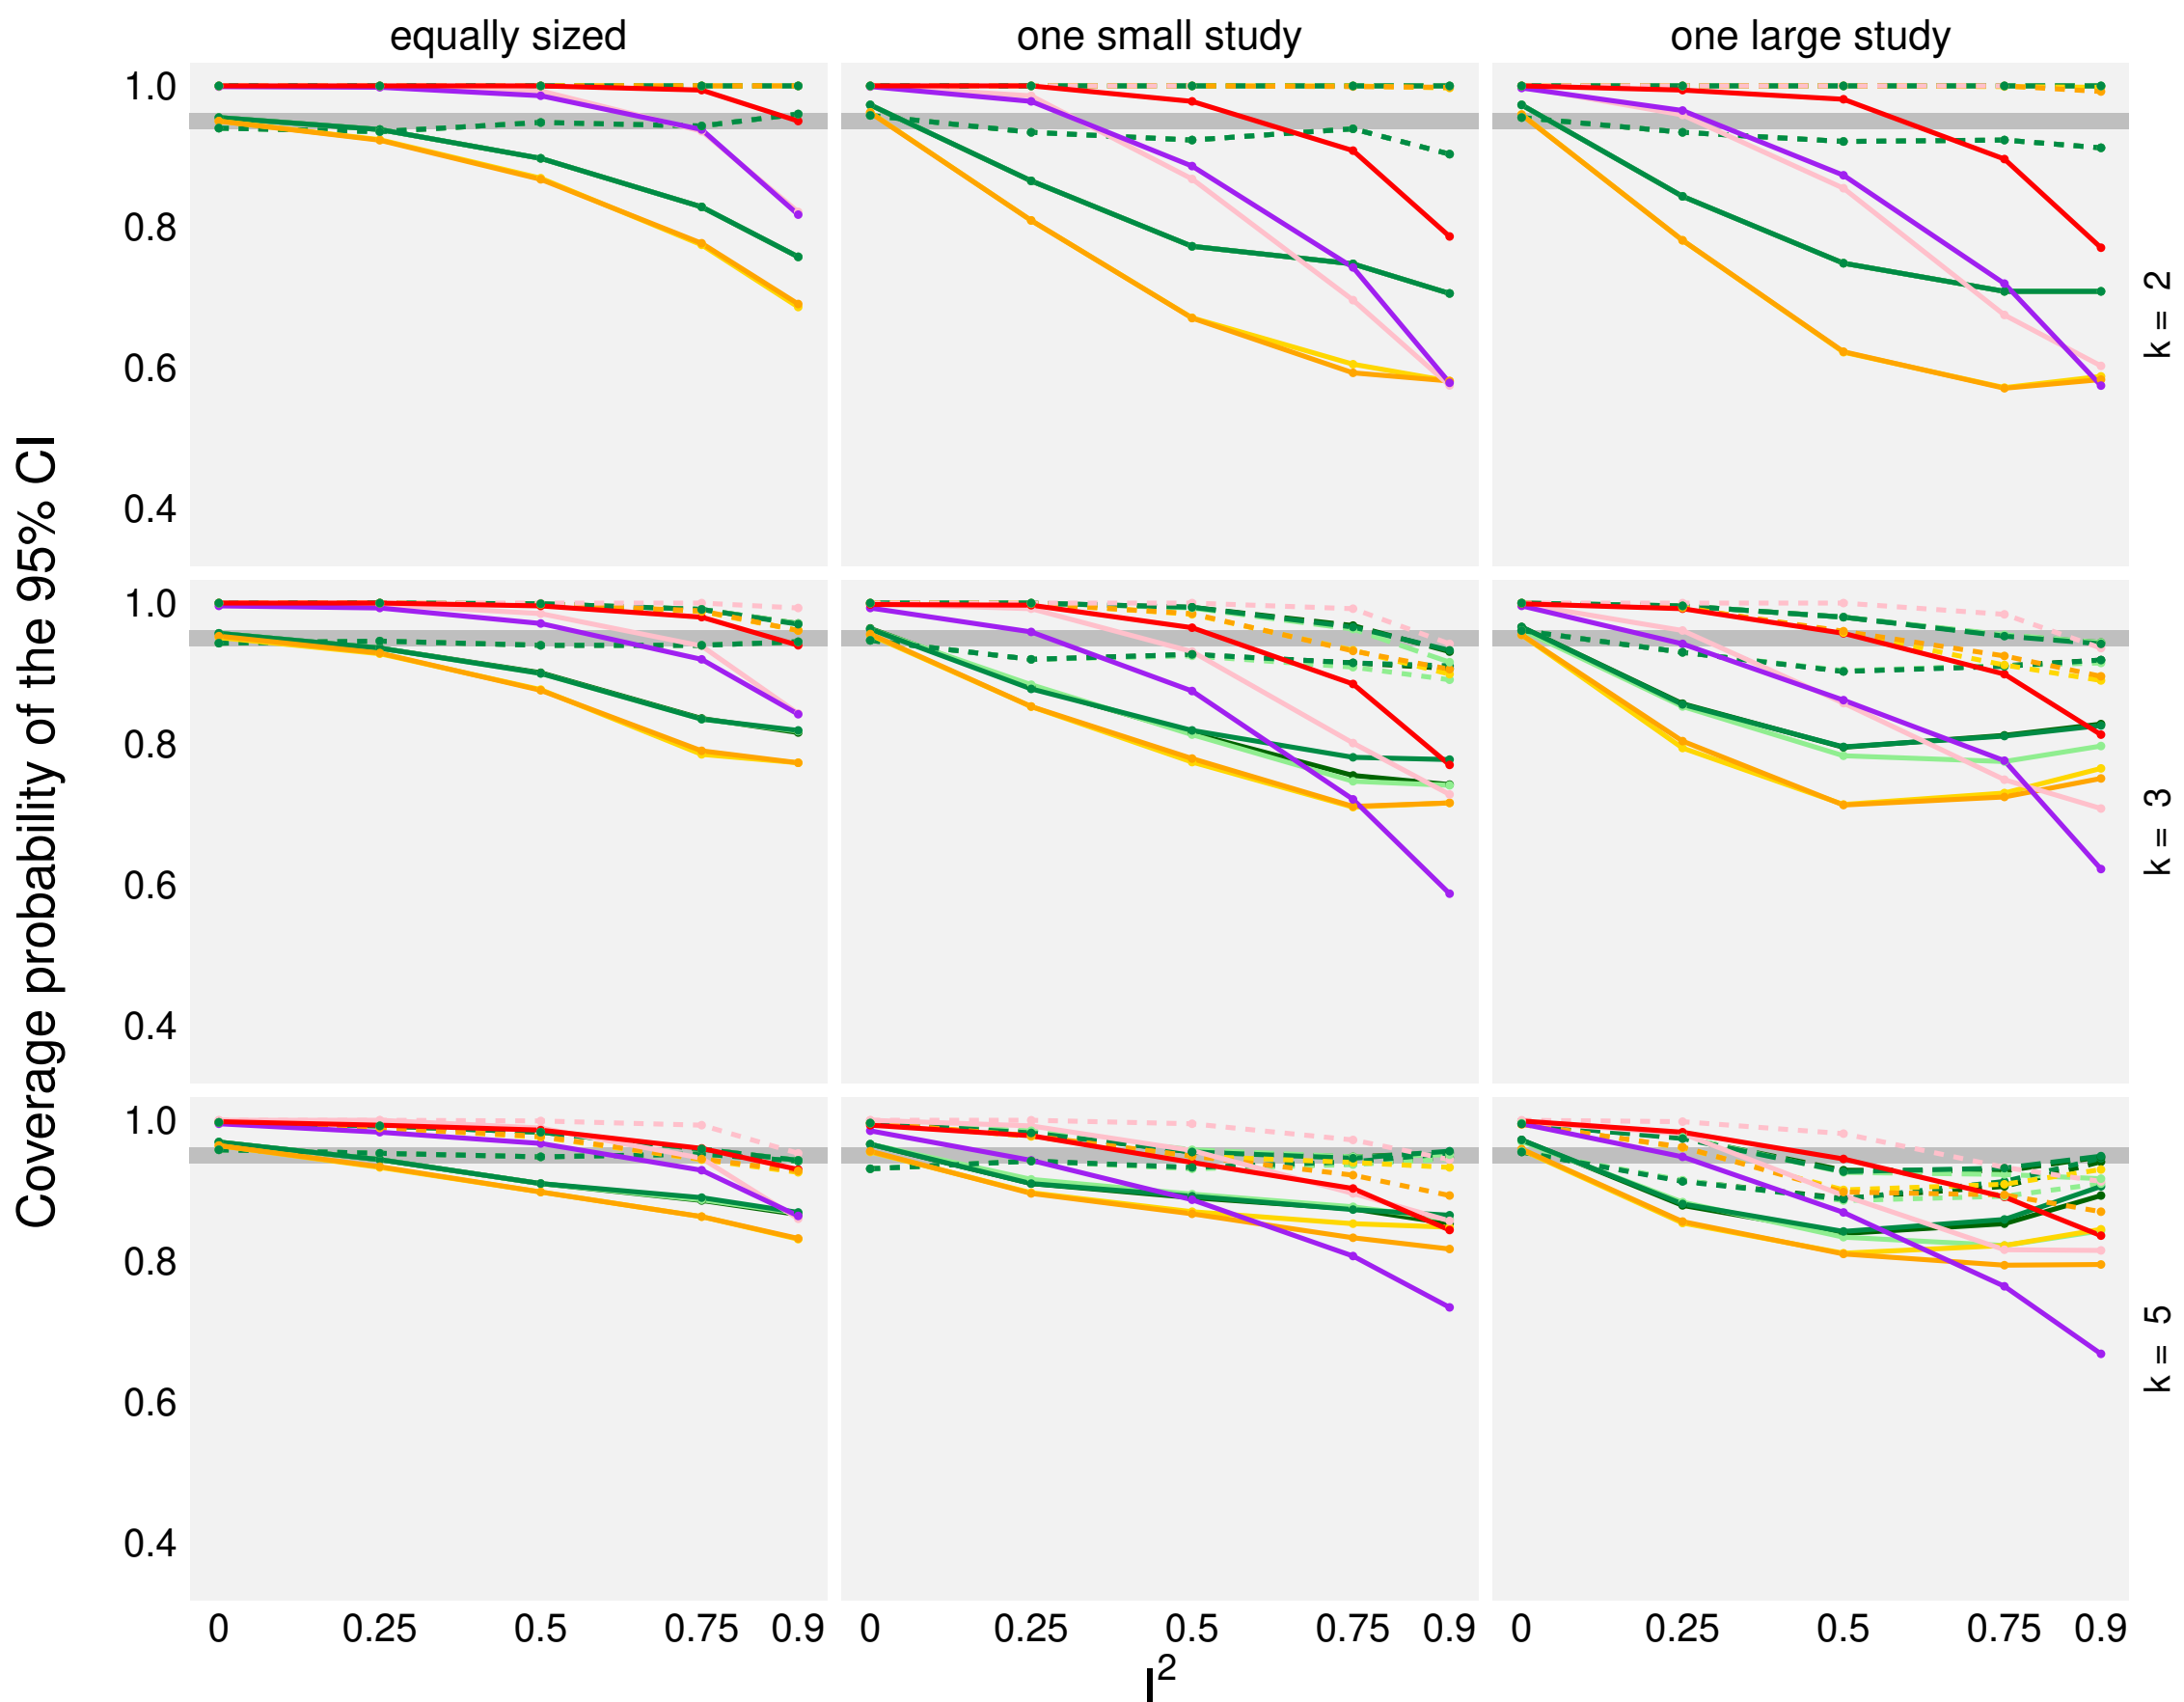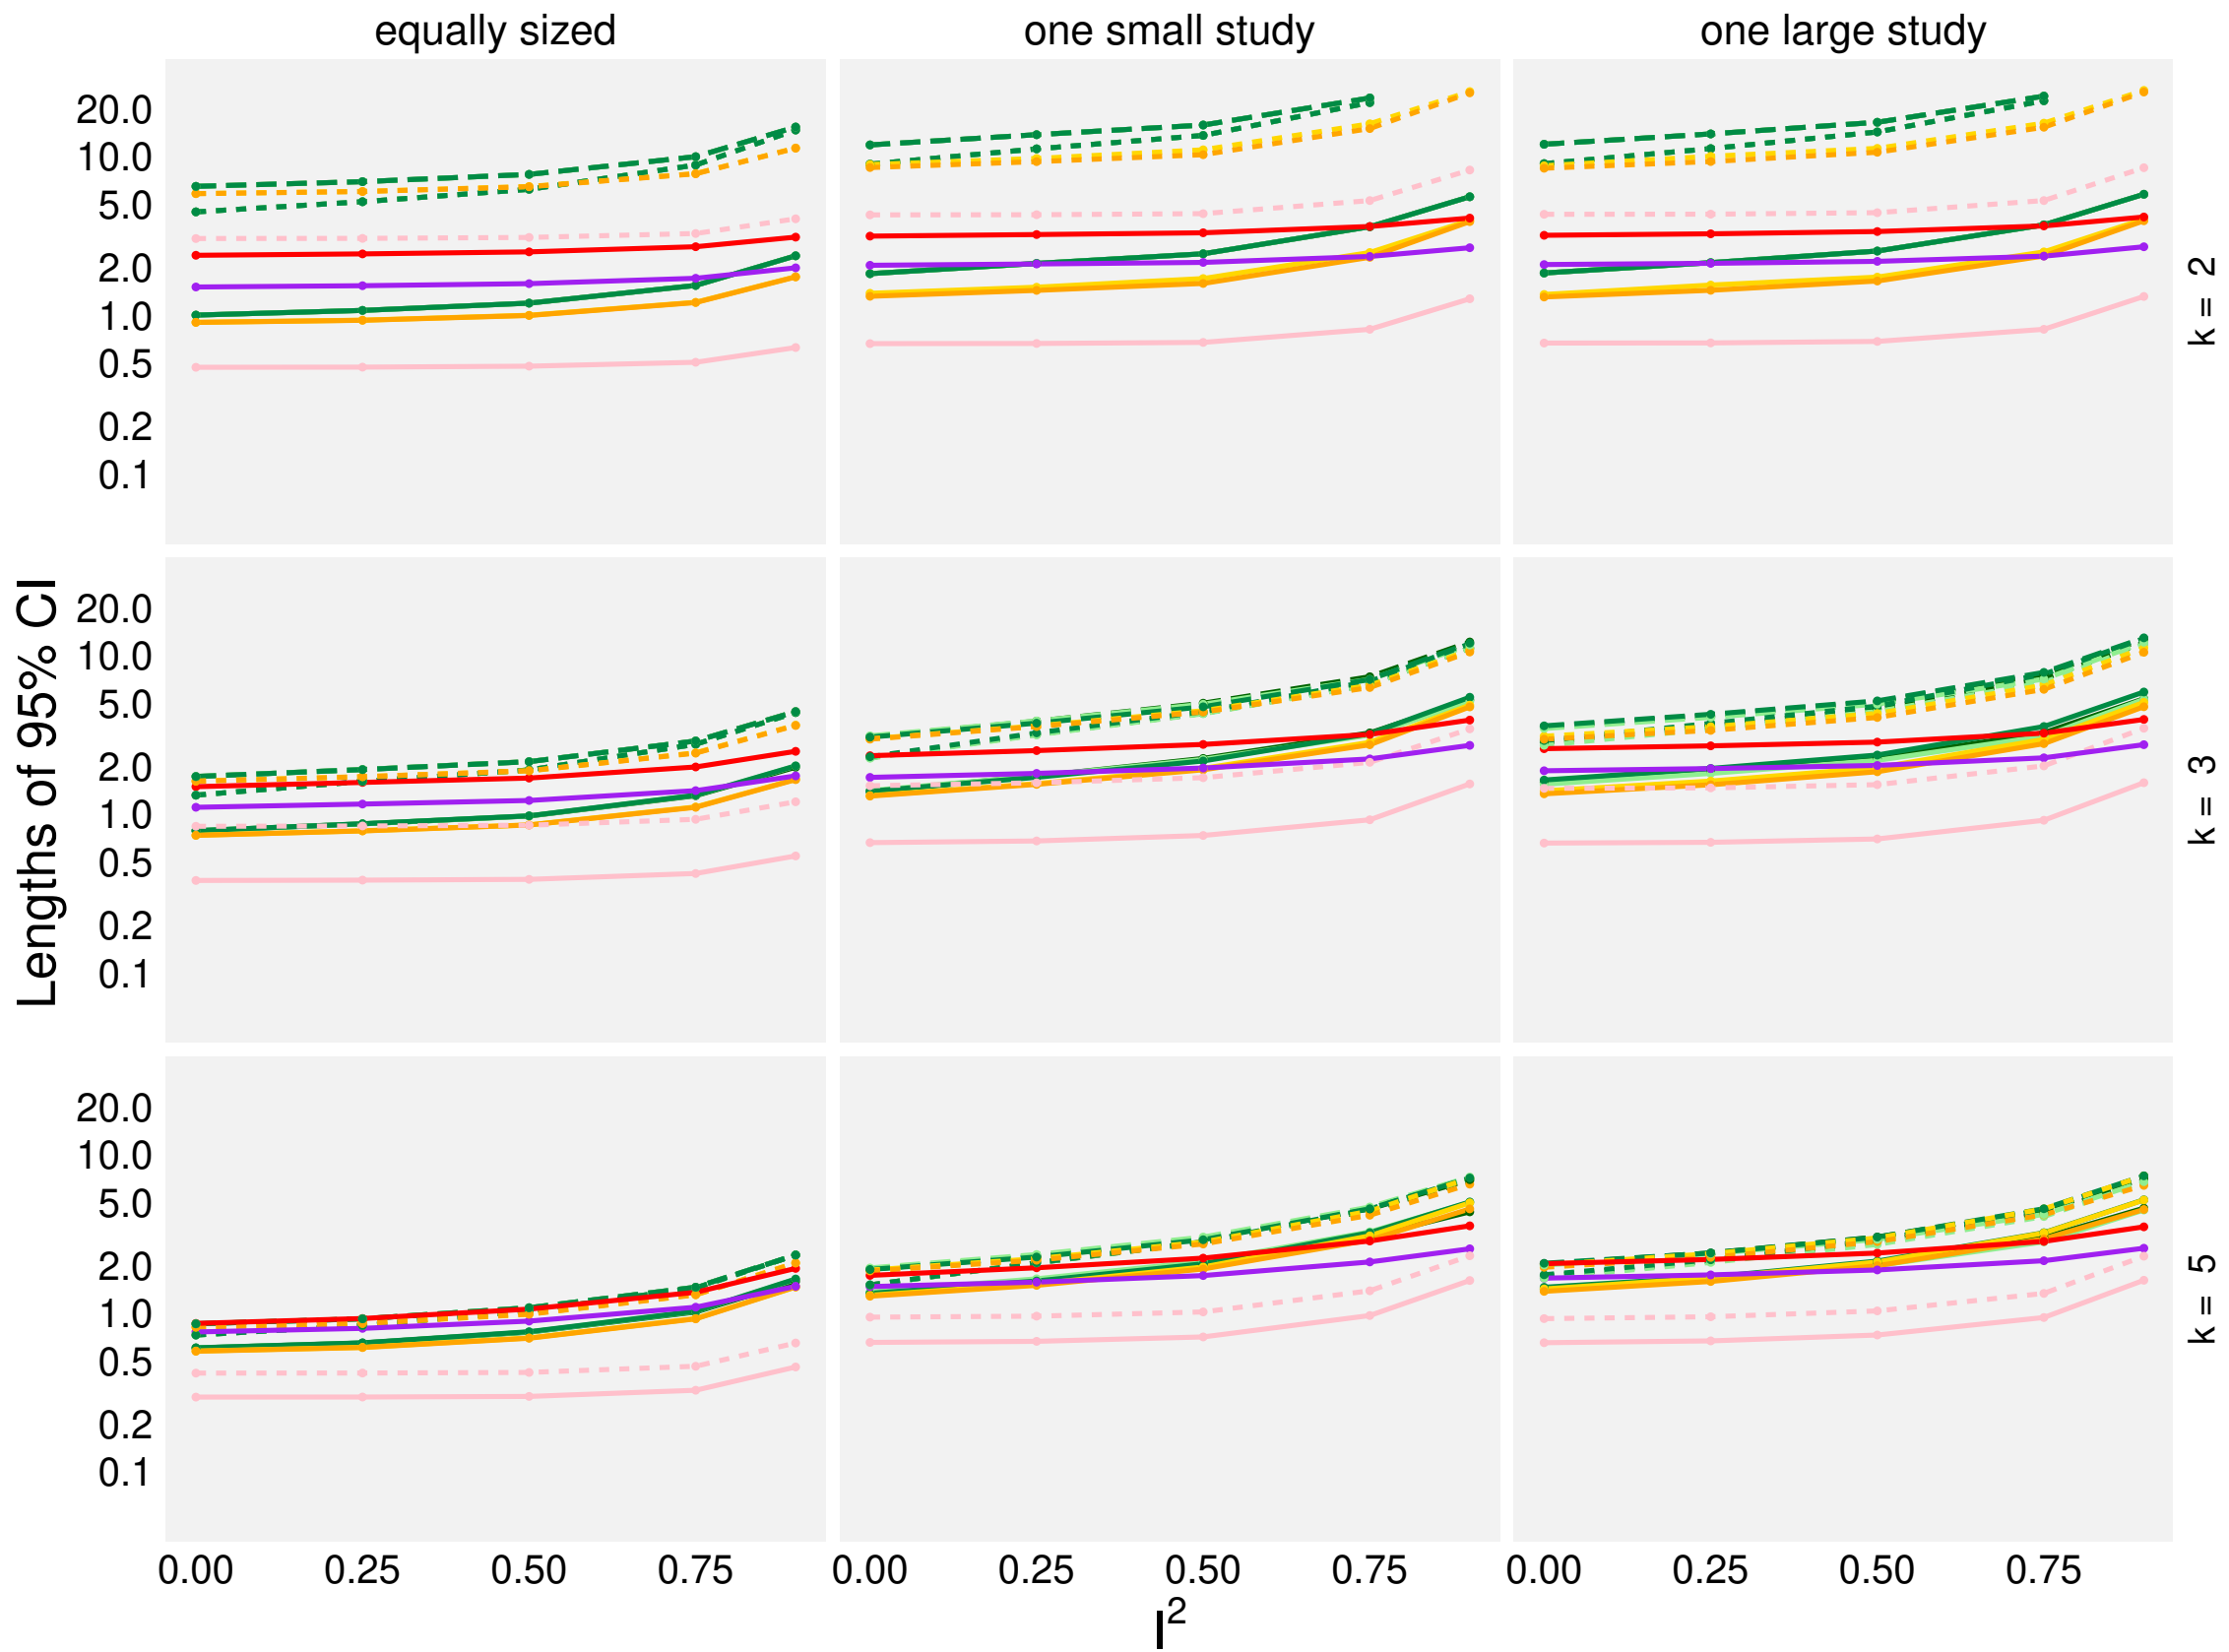

— NN — DL  
 — NN — REML  
 — NN — EB  
 — BN — UM.FS  
 — BN — UM.RS  
 — BN — CM.AL  
 — NN — Bayes HN(0.5)  
 — NN — Bayes HN(1)

— normal quantiles  
 -- HKSJ or Student's t  
 -·- mHKSJ

OR

( $n_i=100, \pi_0=0.9$ )

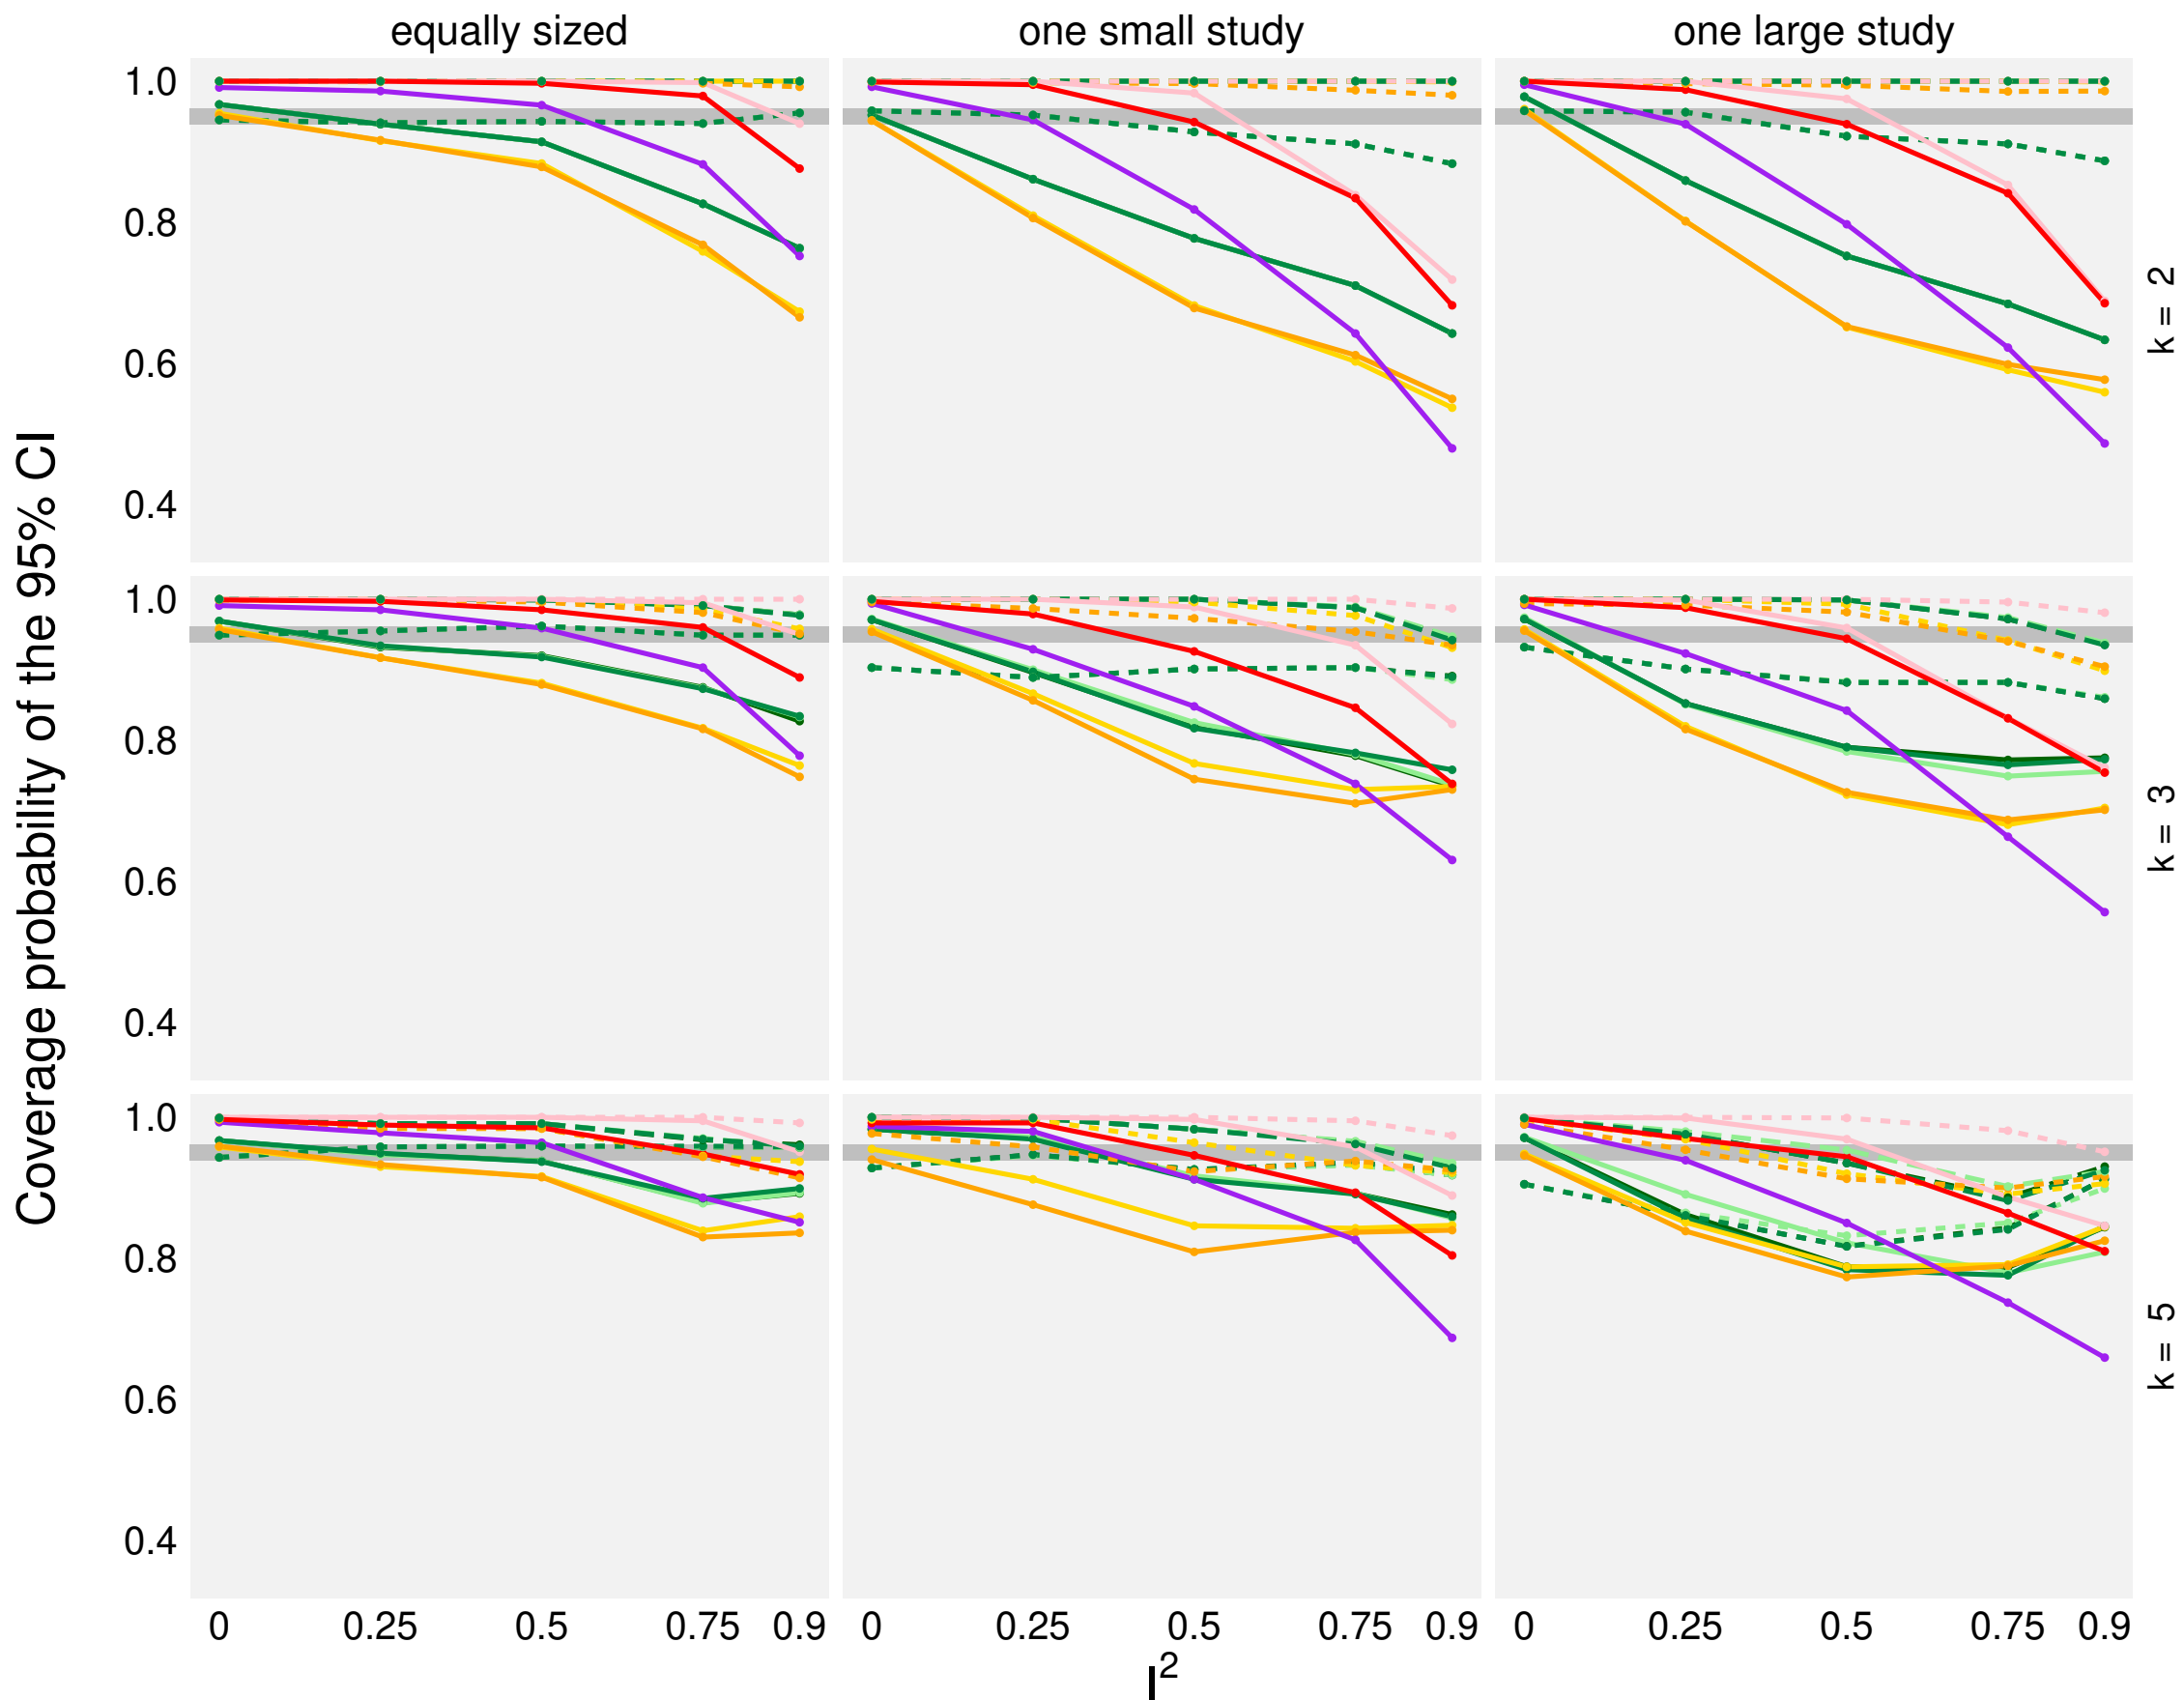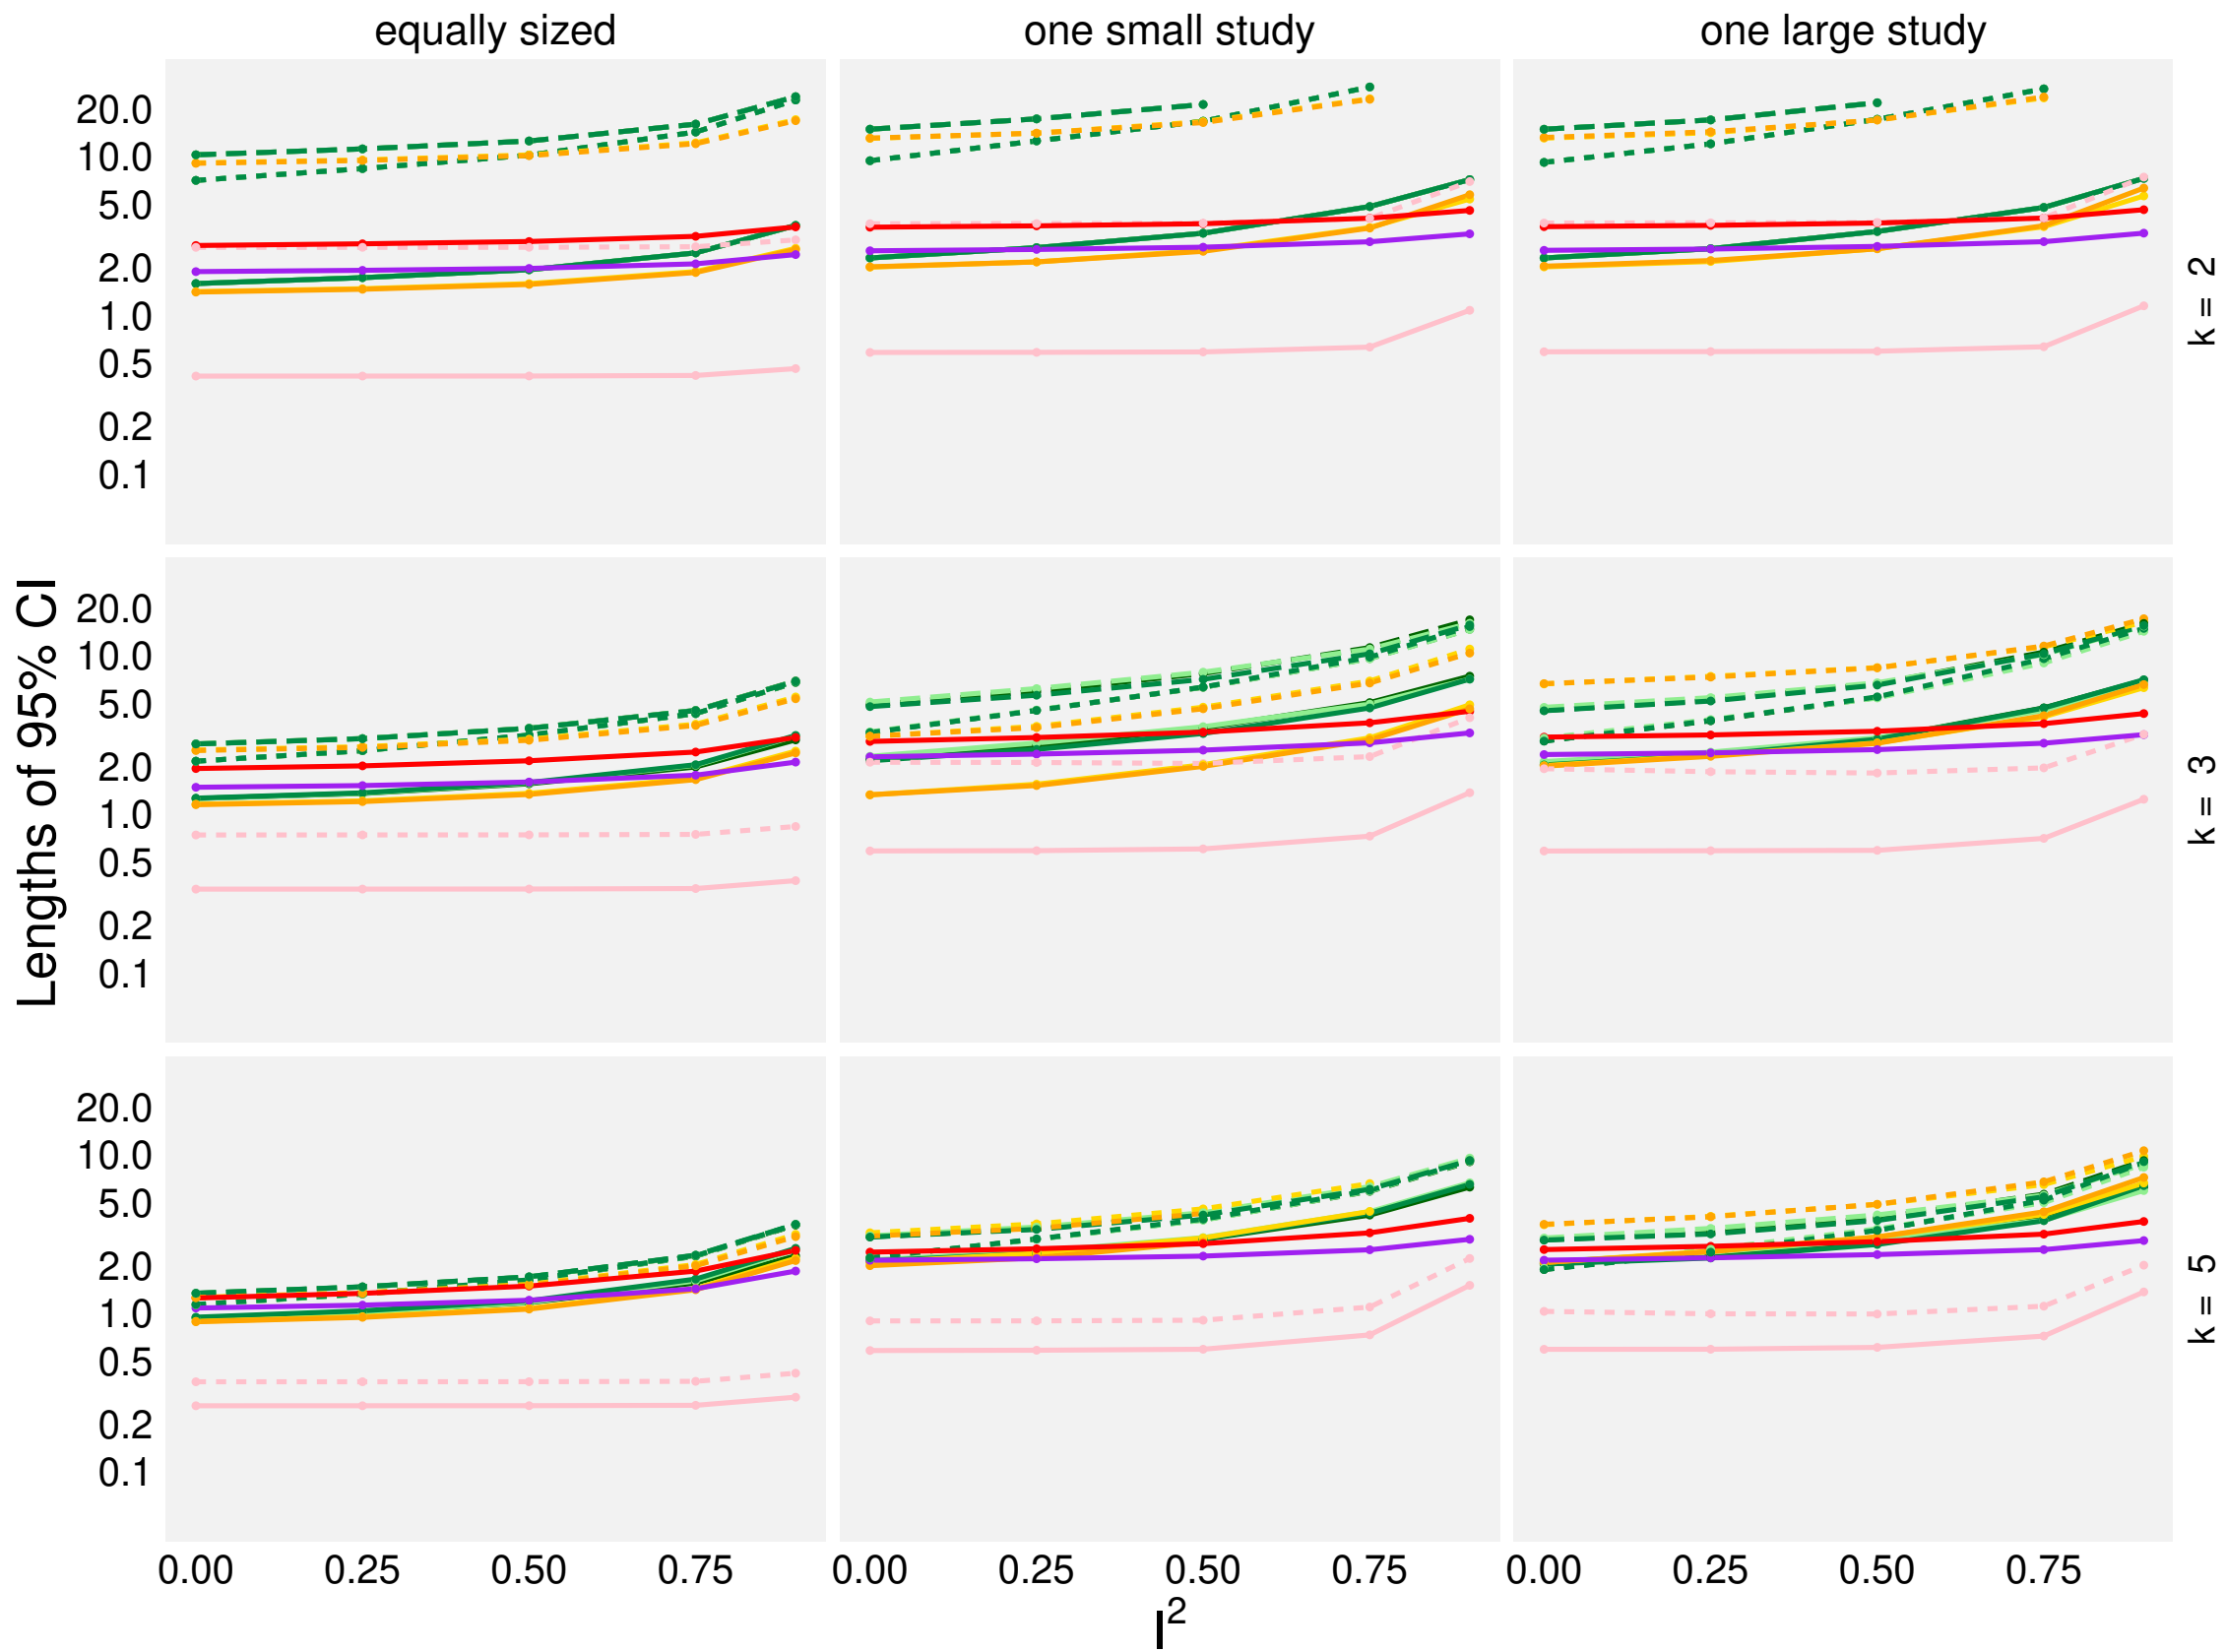

NN – DL  
 NN – REML  
 NN – EB  
 BN – UM.FS  
 BN – UM.RS  
 BN – CM.AL  
 NN – Bayes HN(0.5)  
 NN – Bayes HN(1)  
 — normal quantiles  
 - - HKSJ or Student's t  
 . . mHKSJ

OR  
( $n_i=250, \pi_0=0.1$ )

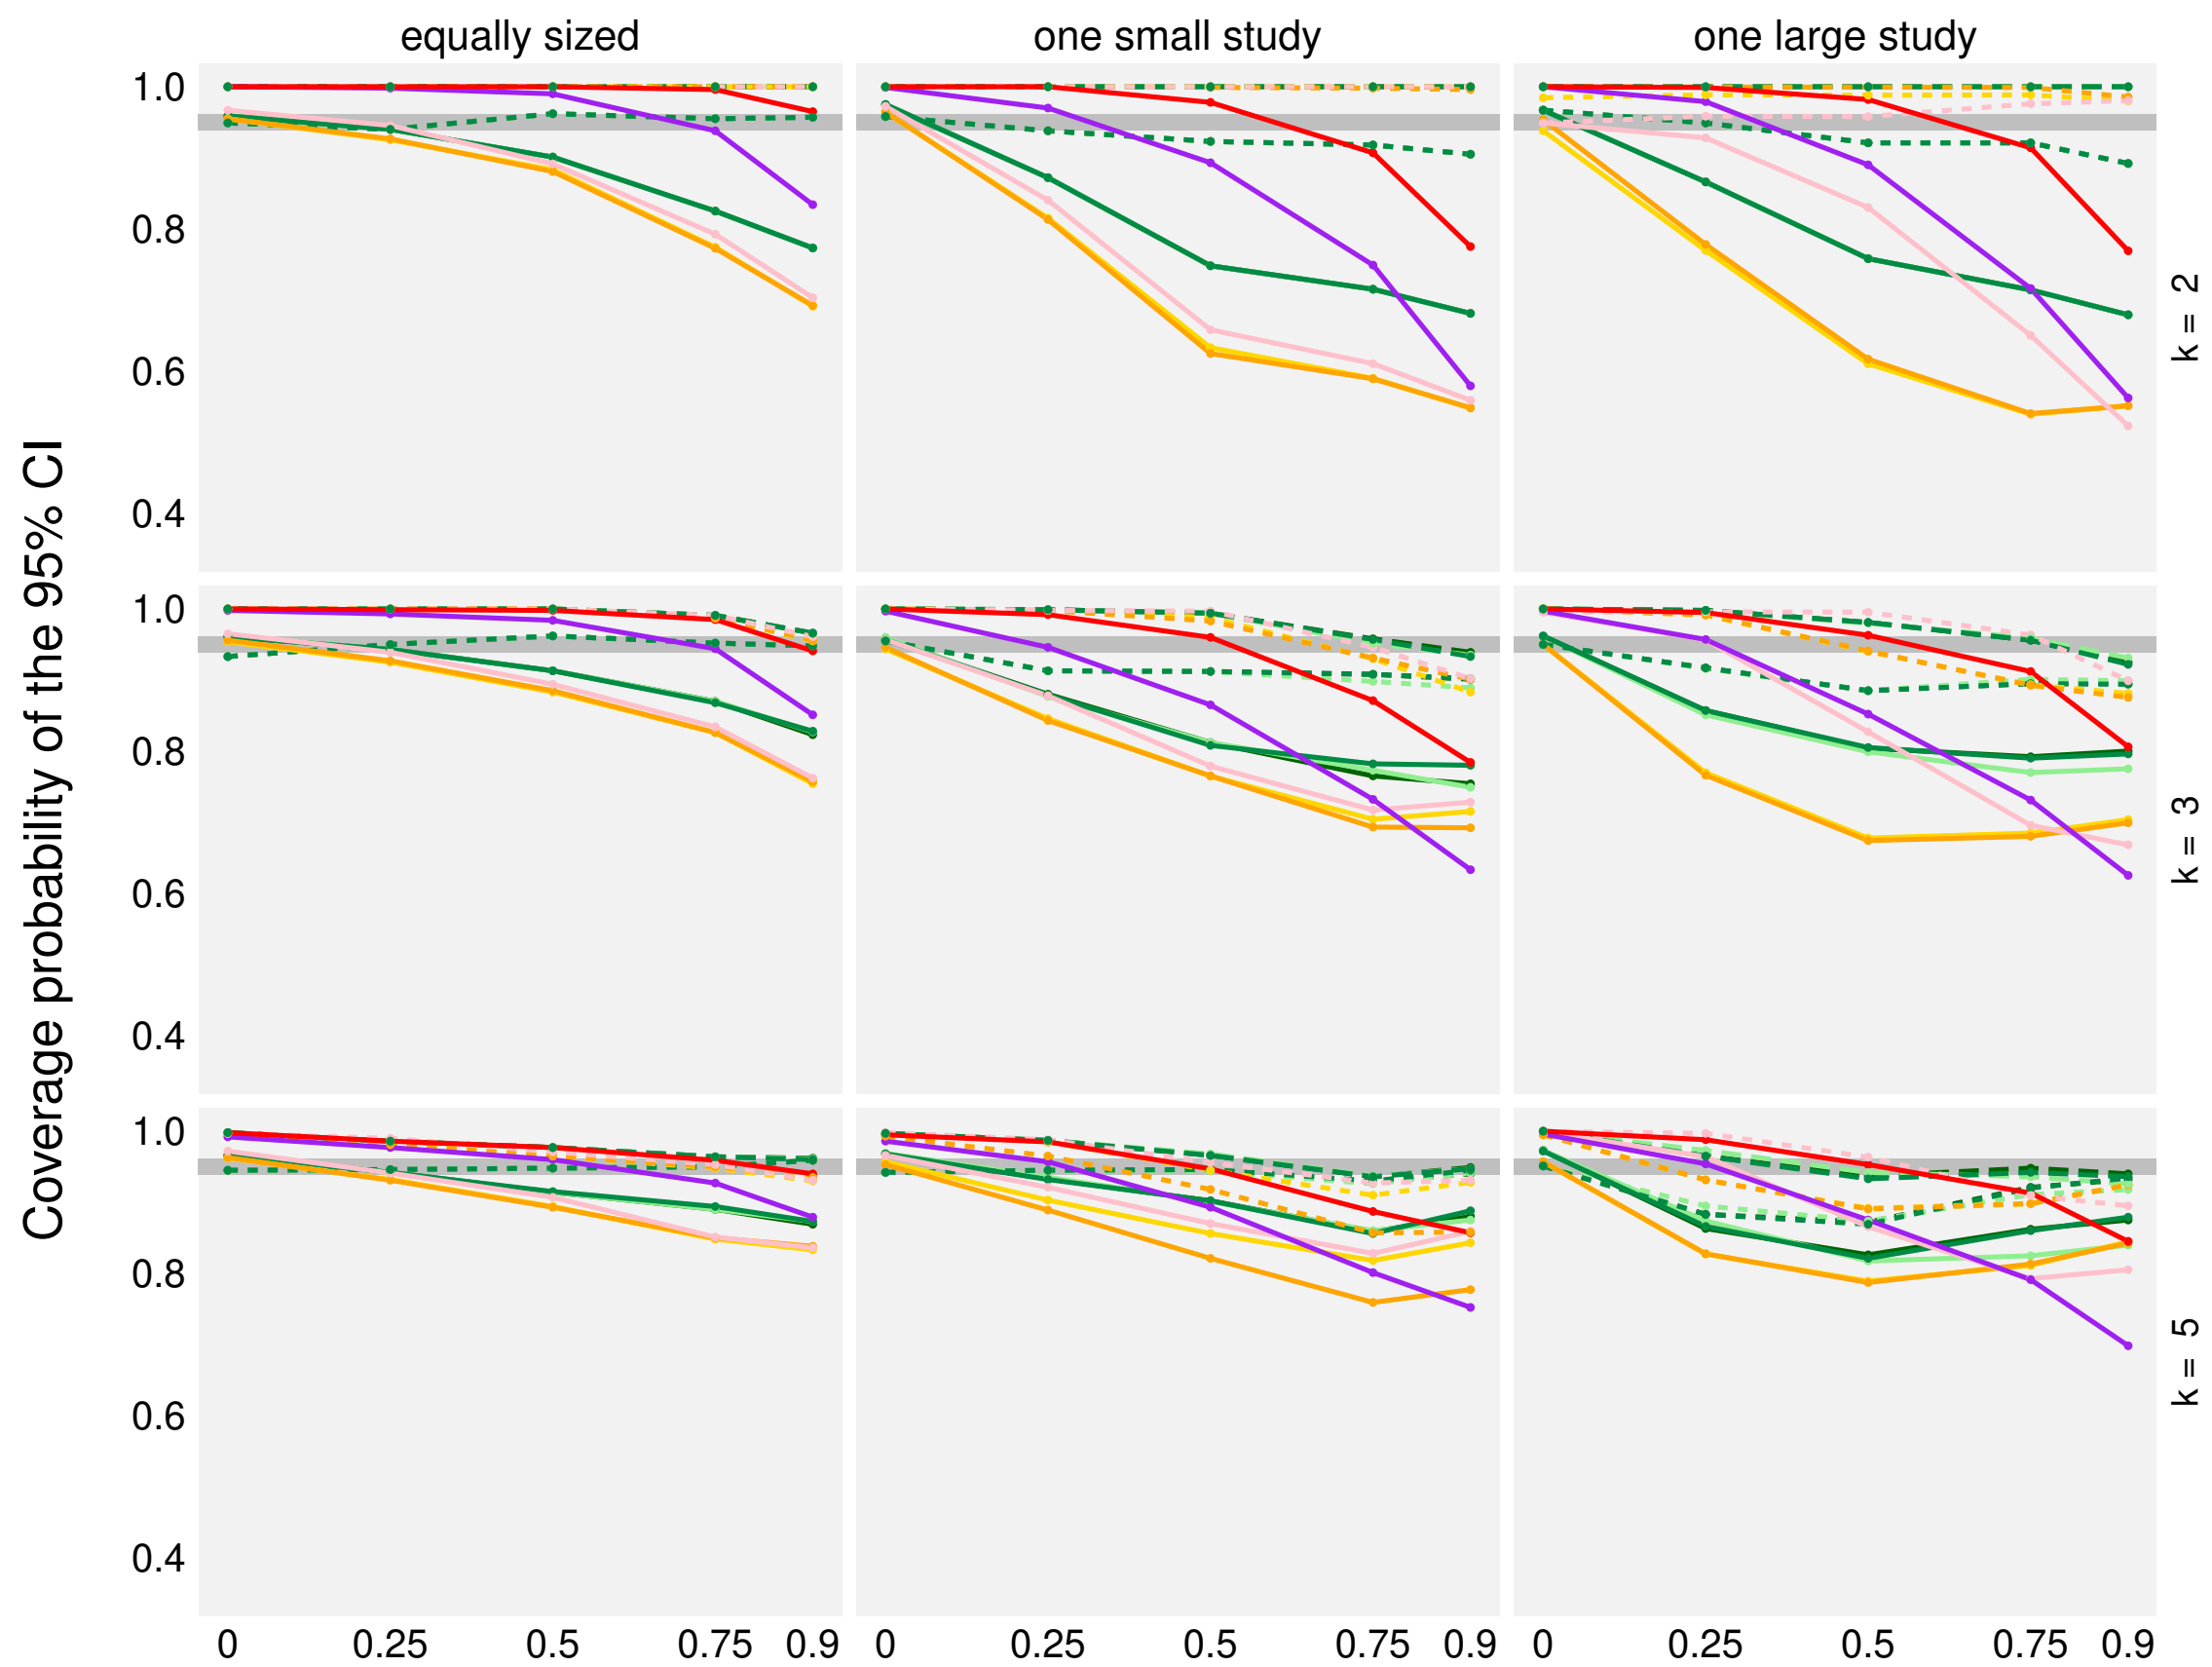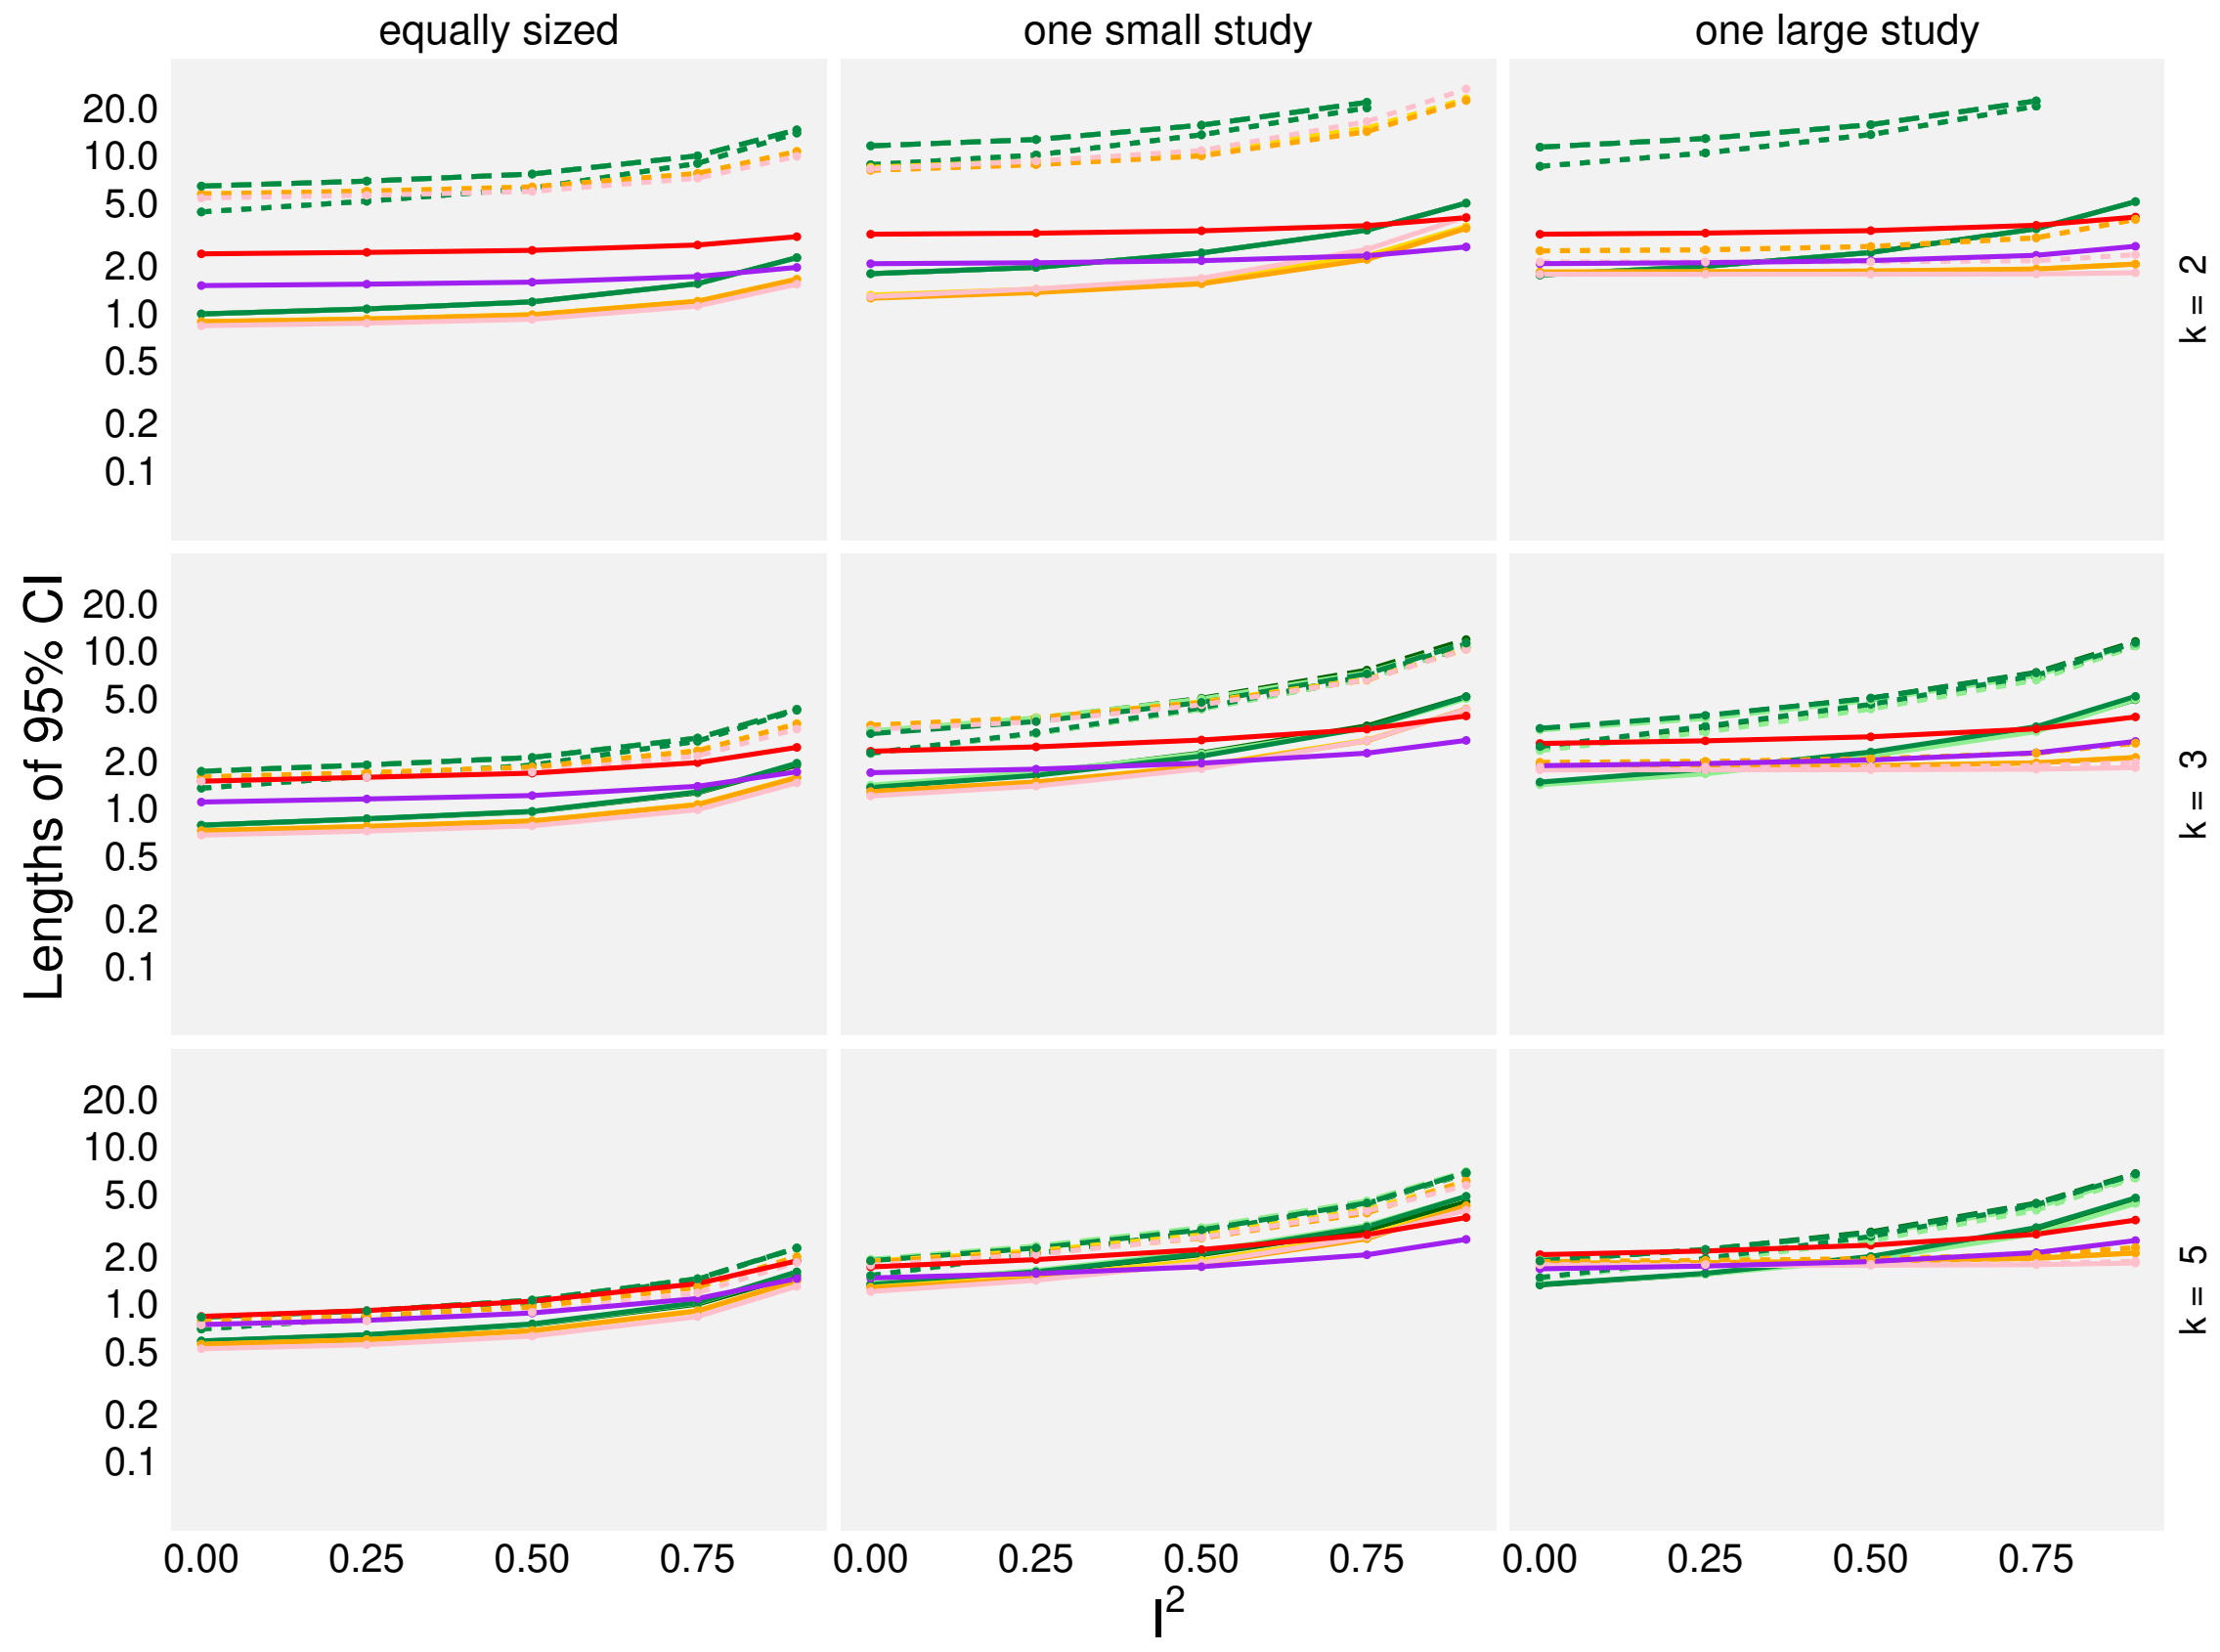

— NN — DL  
 — NN — REML  
 — NN — EB  
 — BN — UM.FS  
 — BN — UM.RS  
 — BN — CM.AL  
 — NN — Bayes HN(0.5)  
 — NN — Bayes HN(1)

— normal quantiles  
 - - HKSJ or Student's t  
 - - mHKSJ

OR  
( $n_i=250, \pi_0=0.3$ )

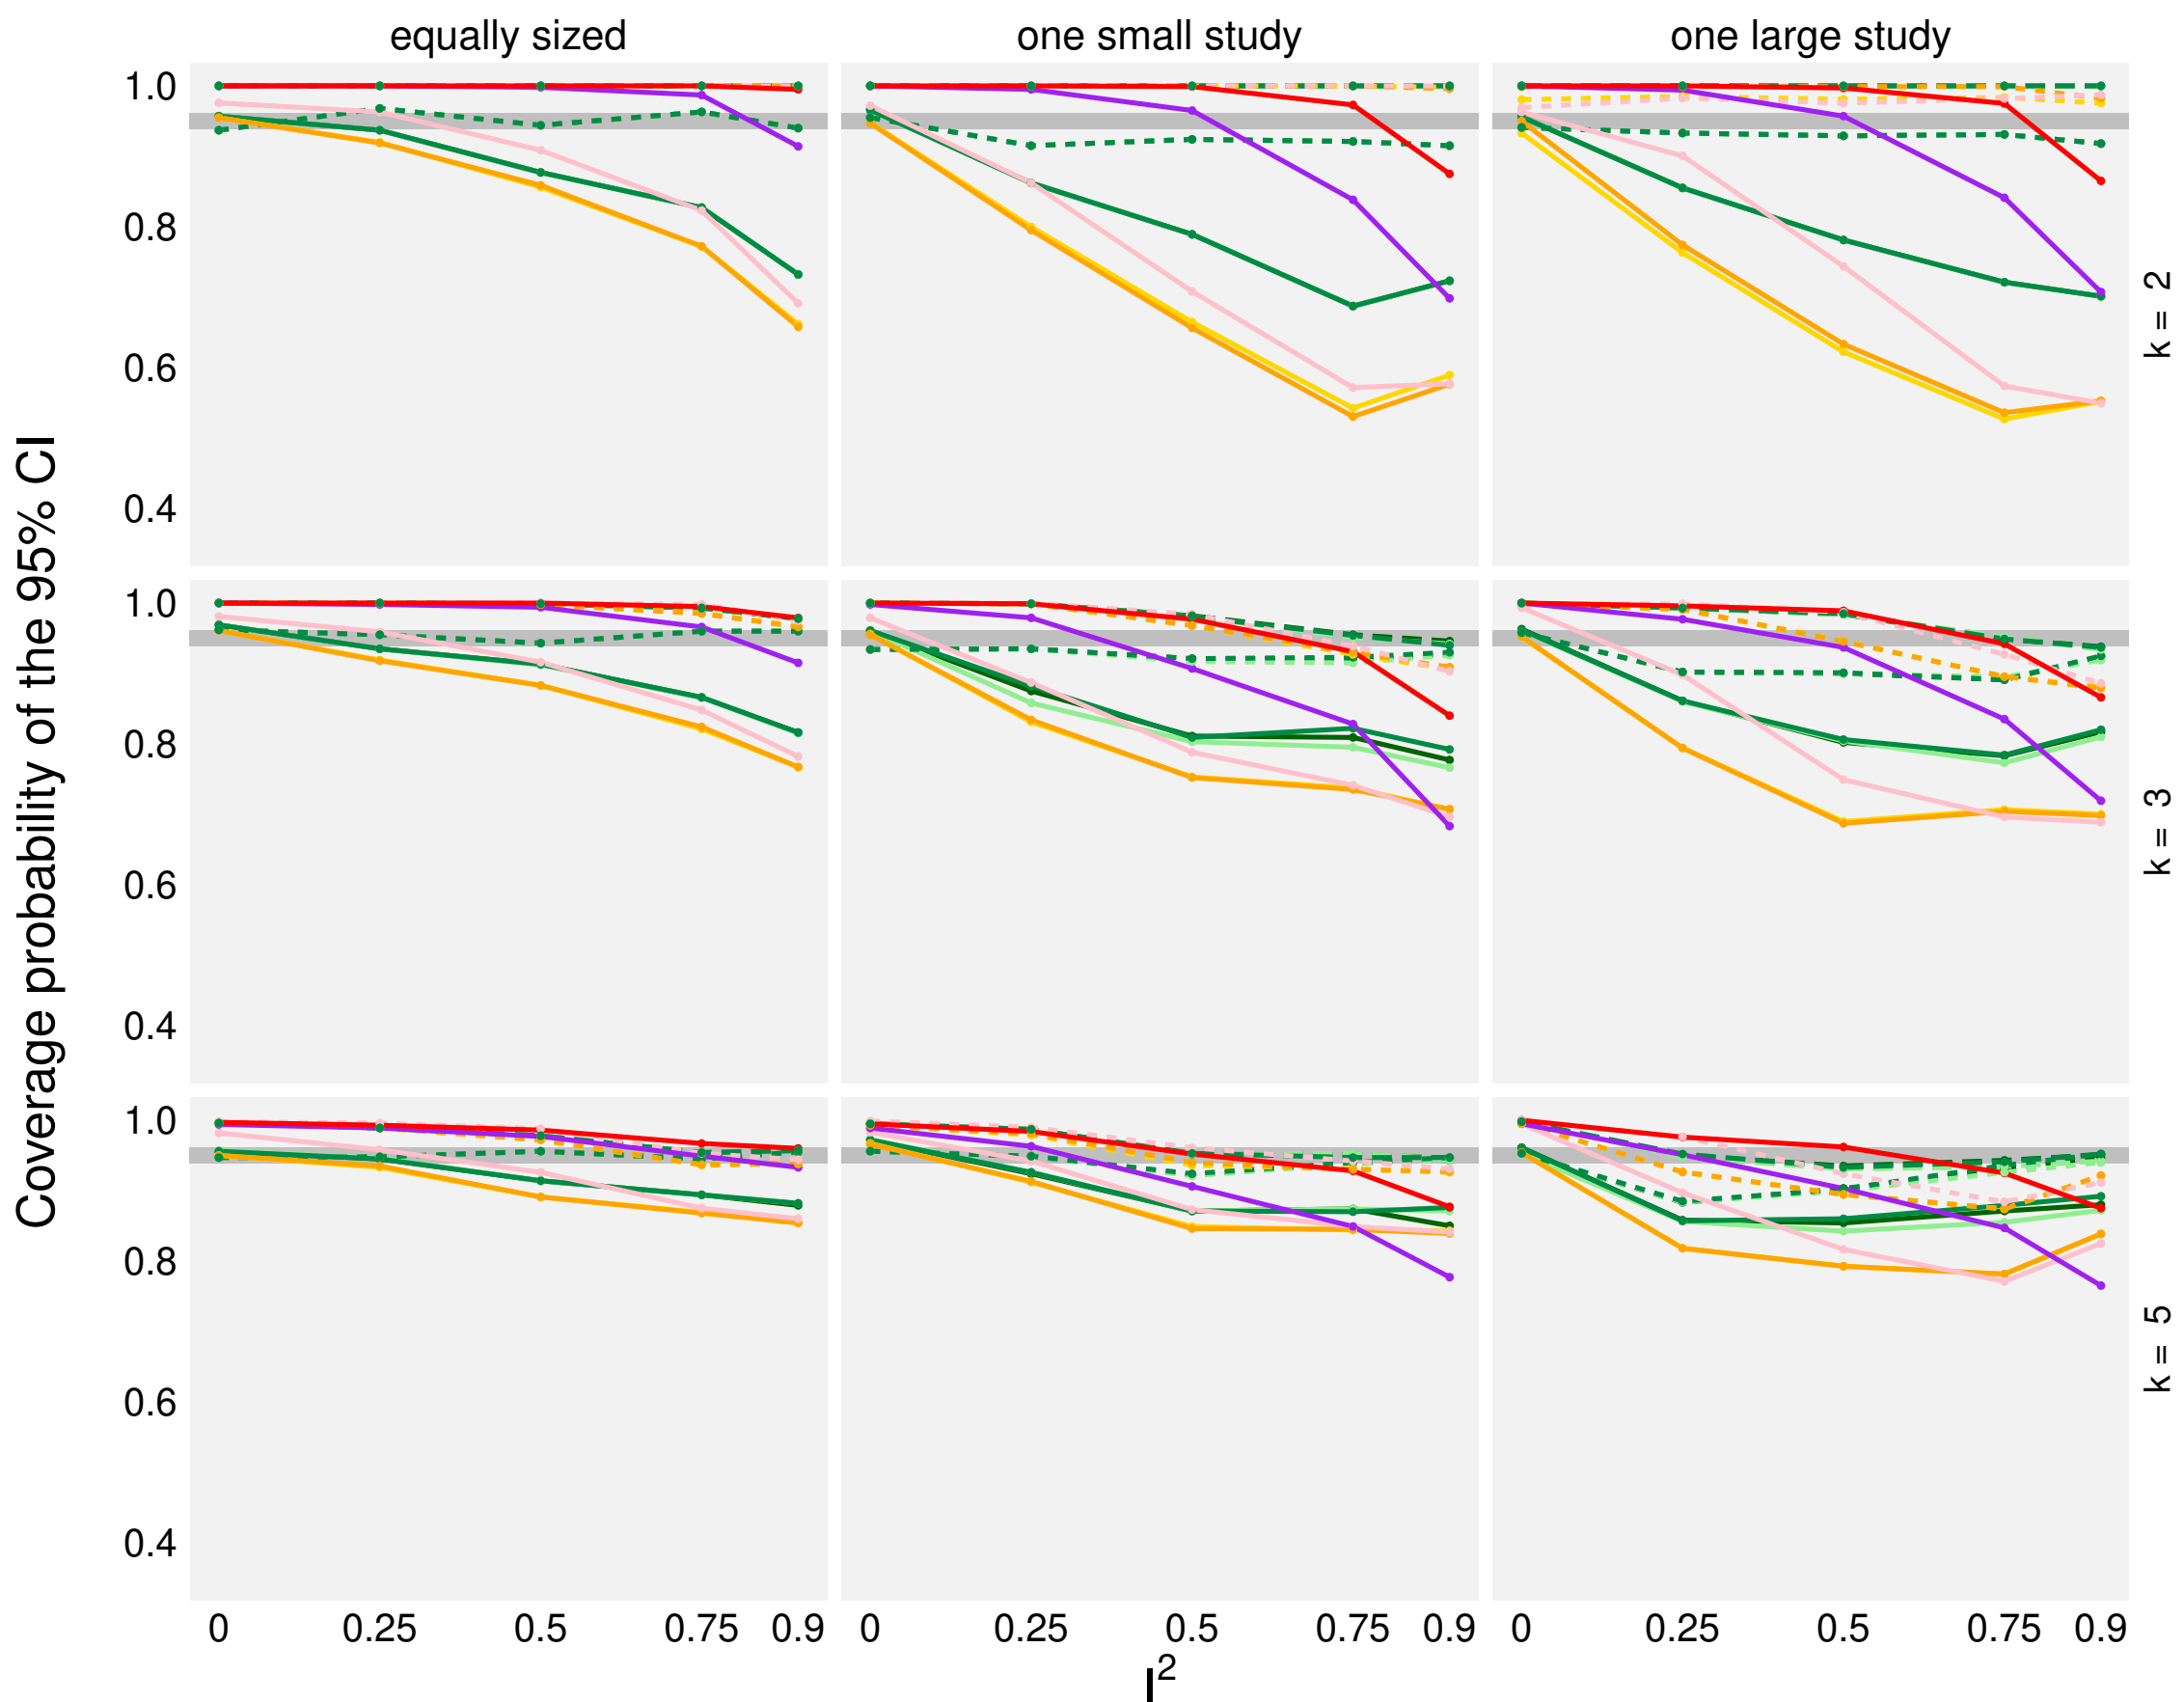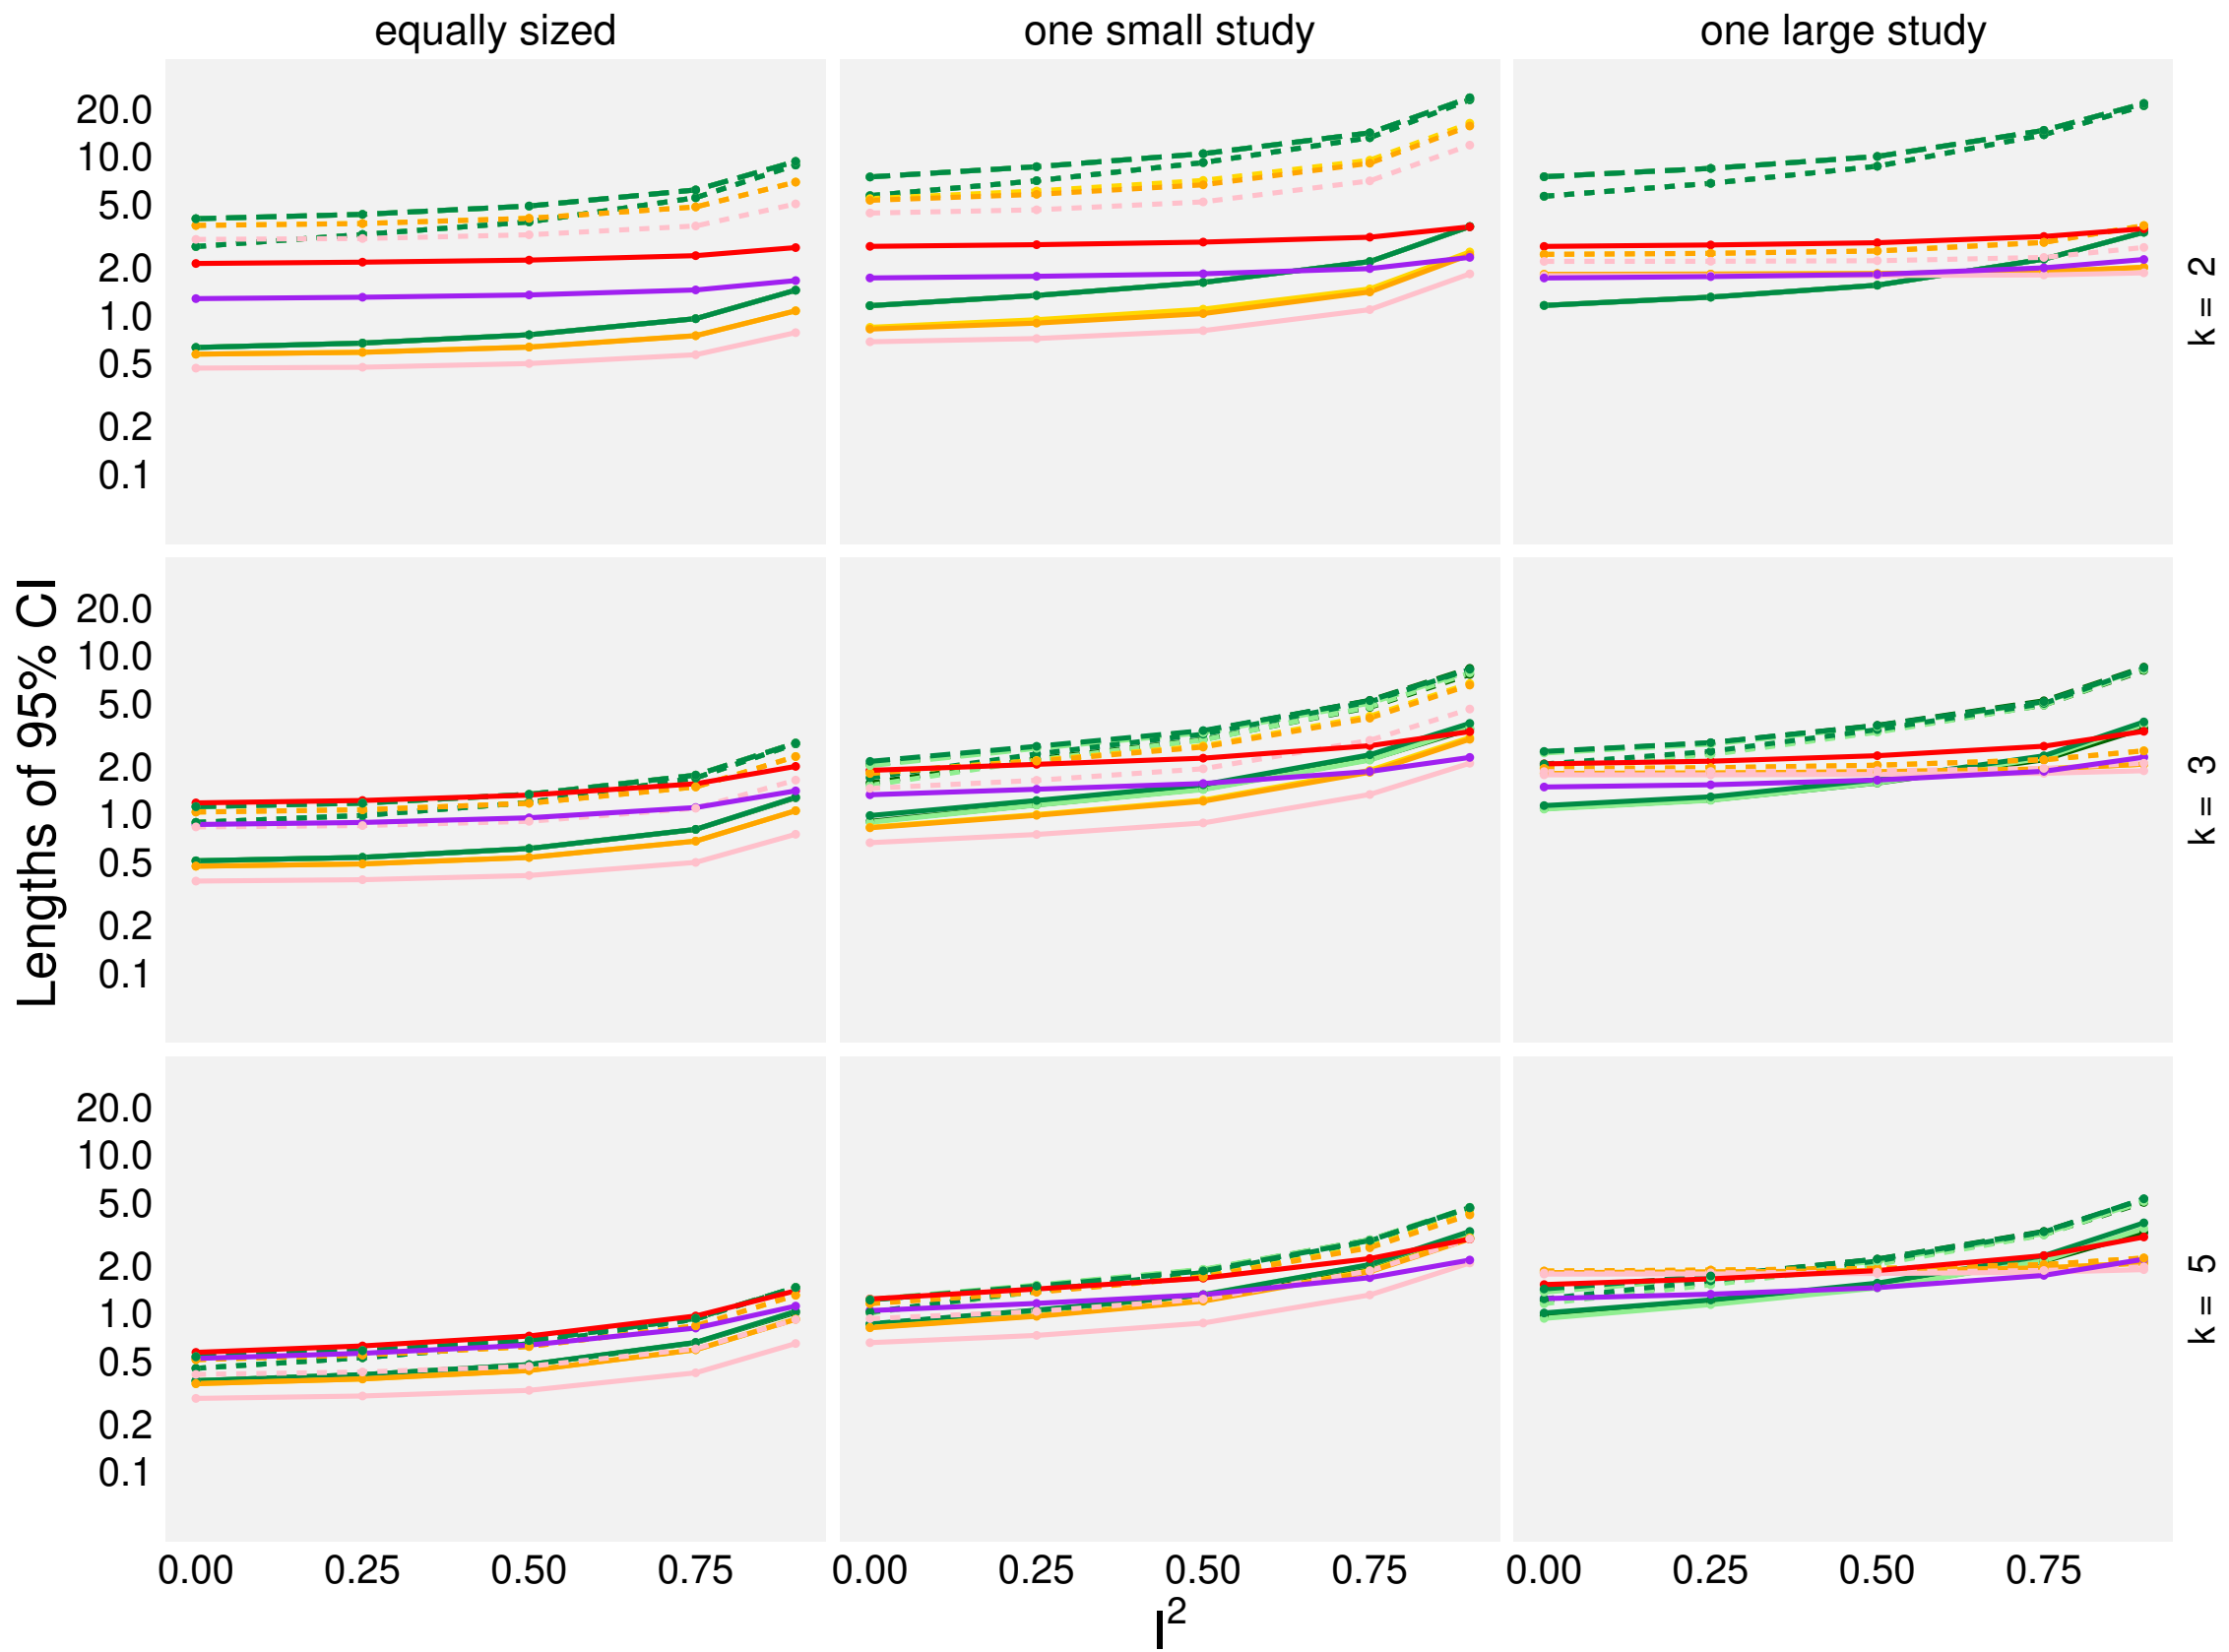

— NN — DL  
 — NN — REML  
 — NN — EB  
 — BN — UM.FS  
 — BN — UM.RS  
 — BN — CM.AL  
 — NN — Bayes HN(0.5)  
 — NN — Bayes HN(1)

— normal quantiles  
 - - HKSJ or Student's t  
 - - mHKSJ

OR  
( $n_i=250, \pi_0=0.5$ )

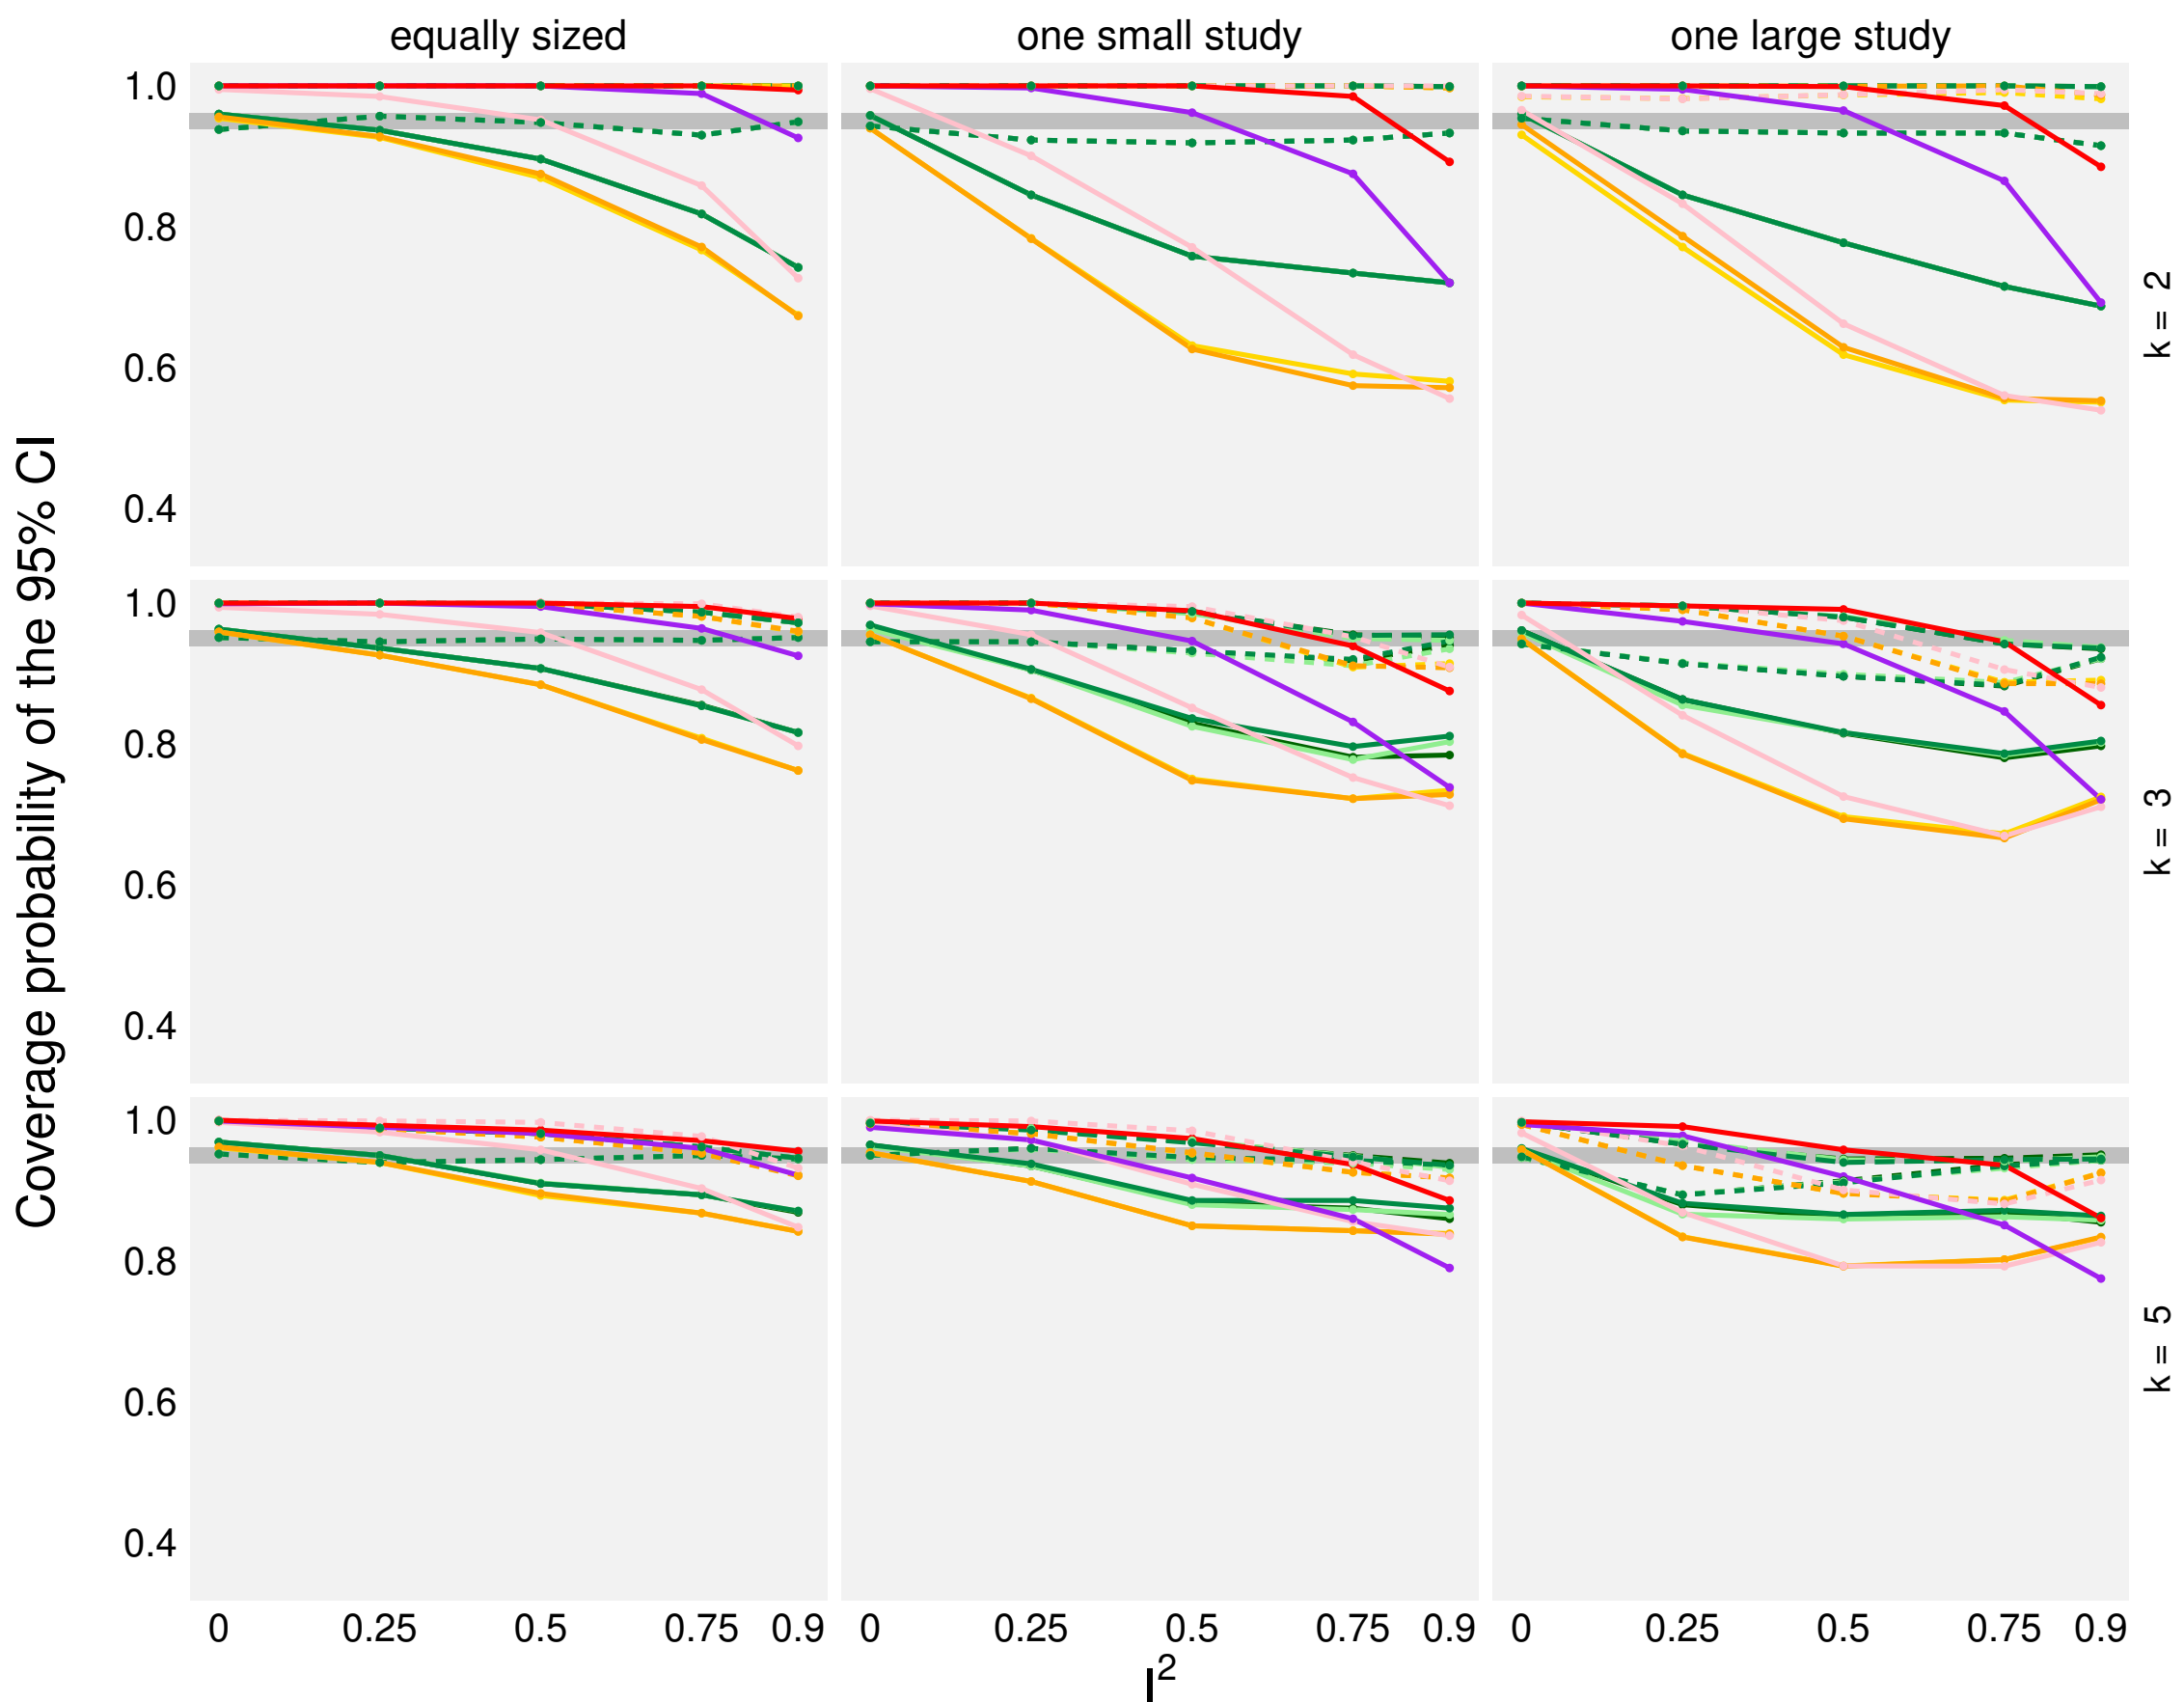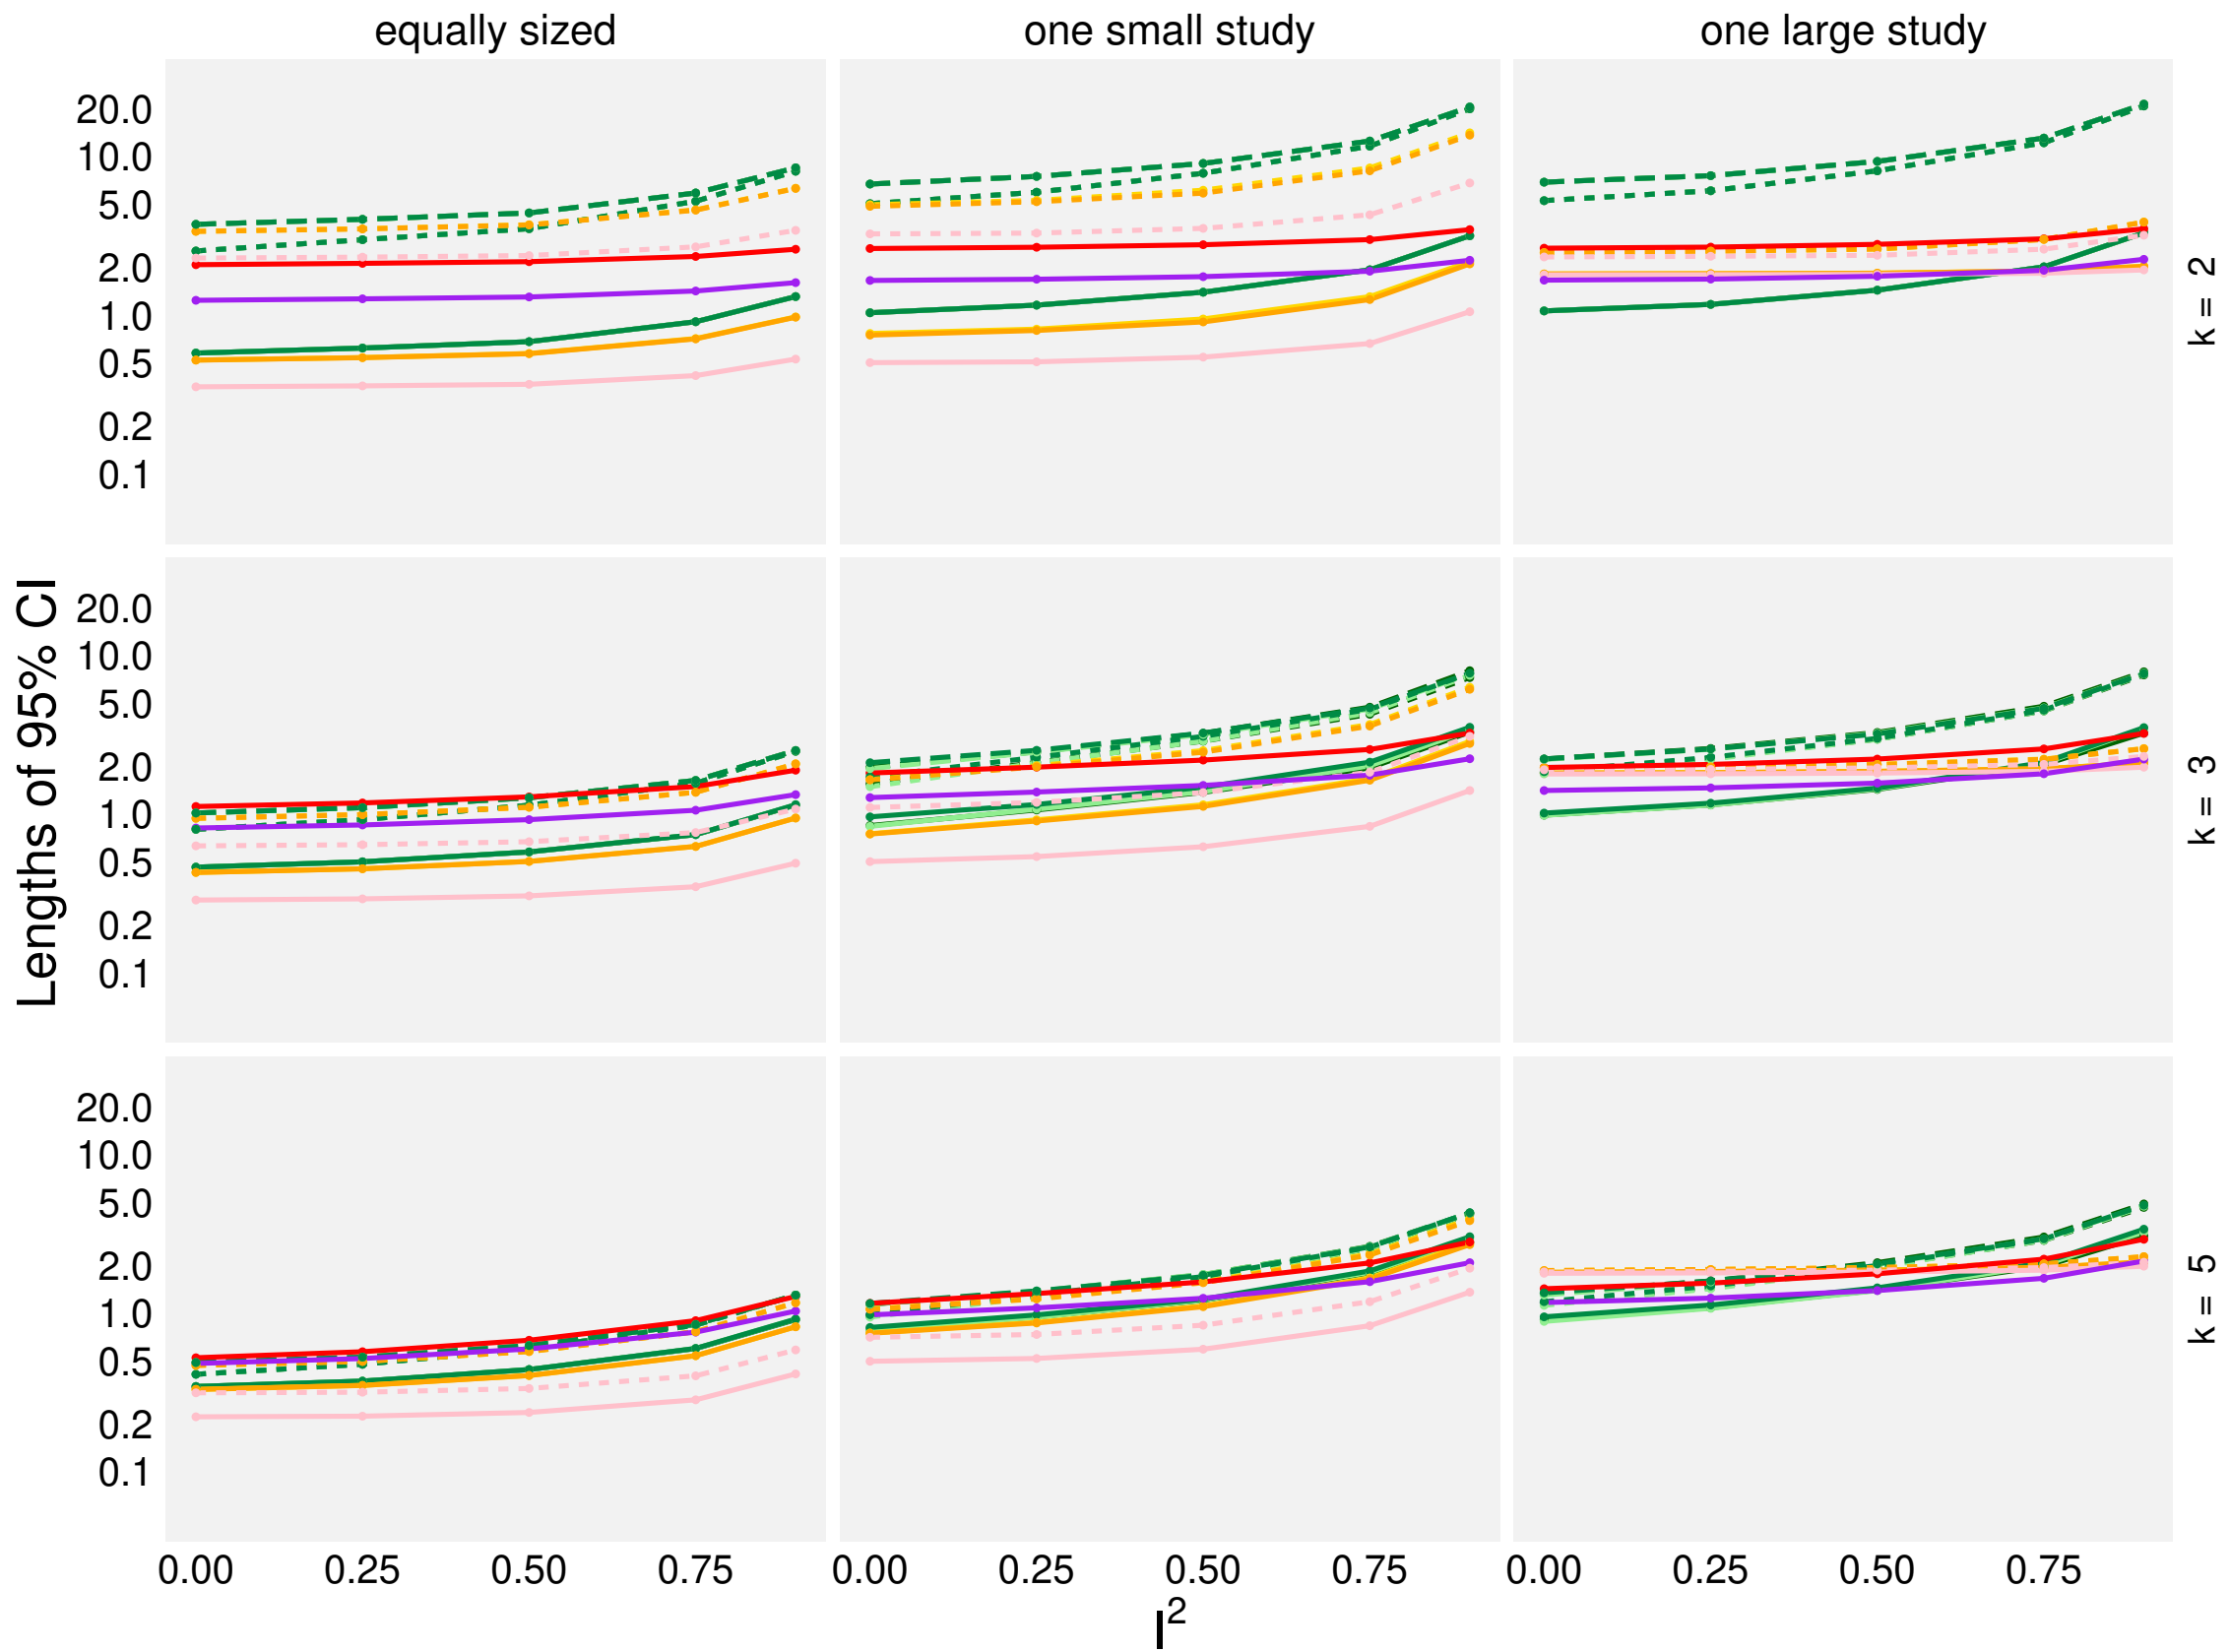

— NN — DL  
 — NN — REML  
 — NN — EB  
 — BN — UM.FS  
 — BN — UM.RS  
 — BN — CM.AL  
 — NN — Bayes HN(0.5)  
 — NN — Bayes HN(1)

— normal quantiles  
 - - HKSJ or Student's t  
 - - mHKSJ

OR  
( $n_i=250, \pi_0=0.7$ )

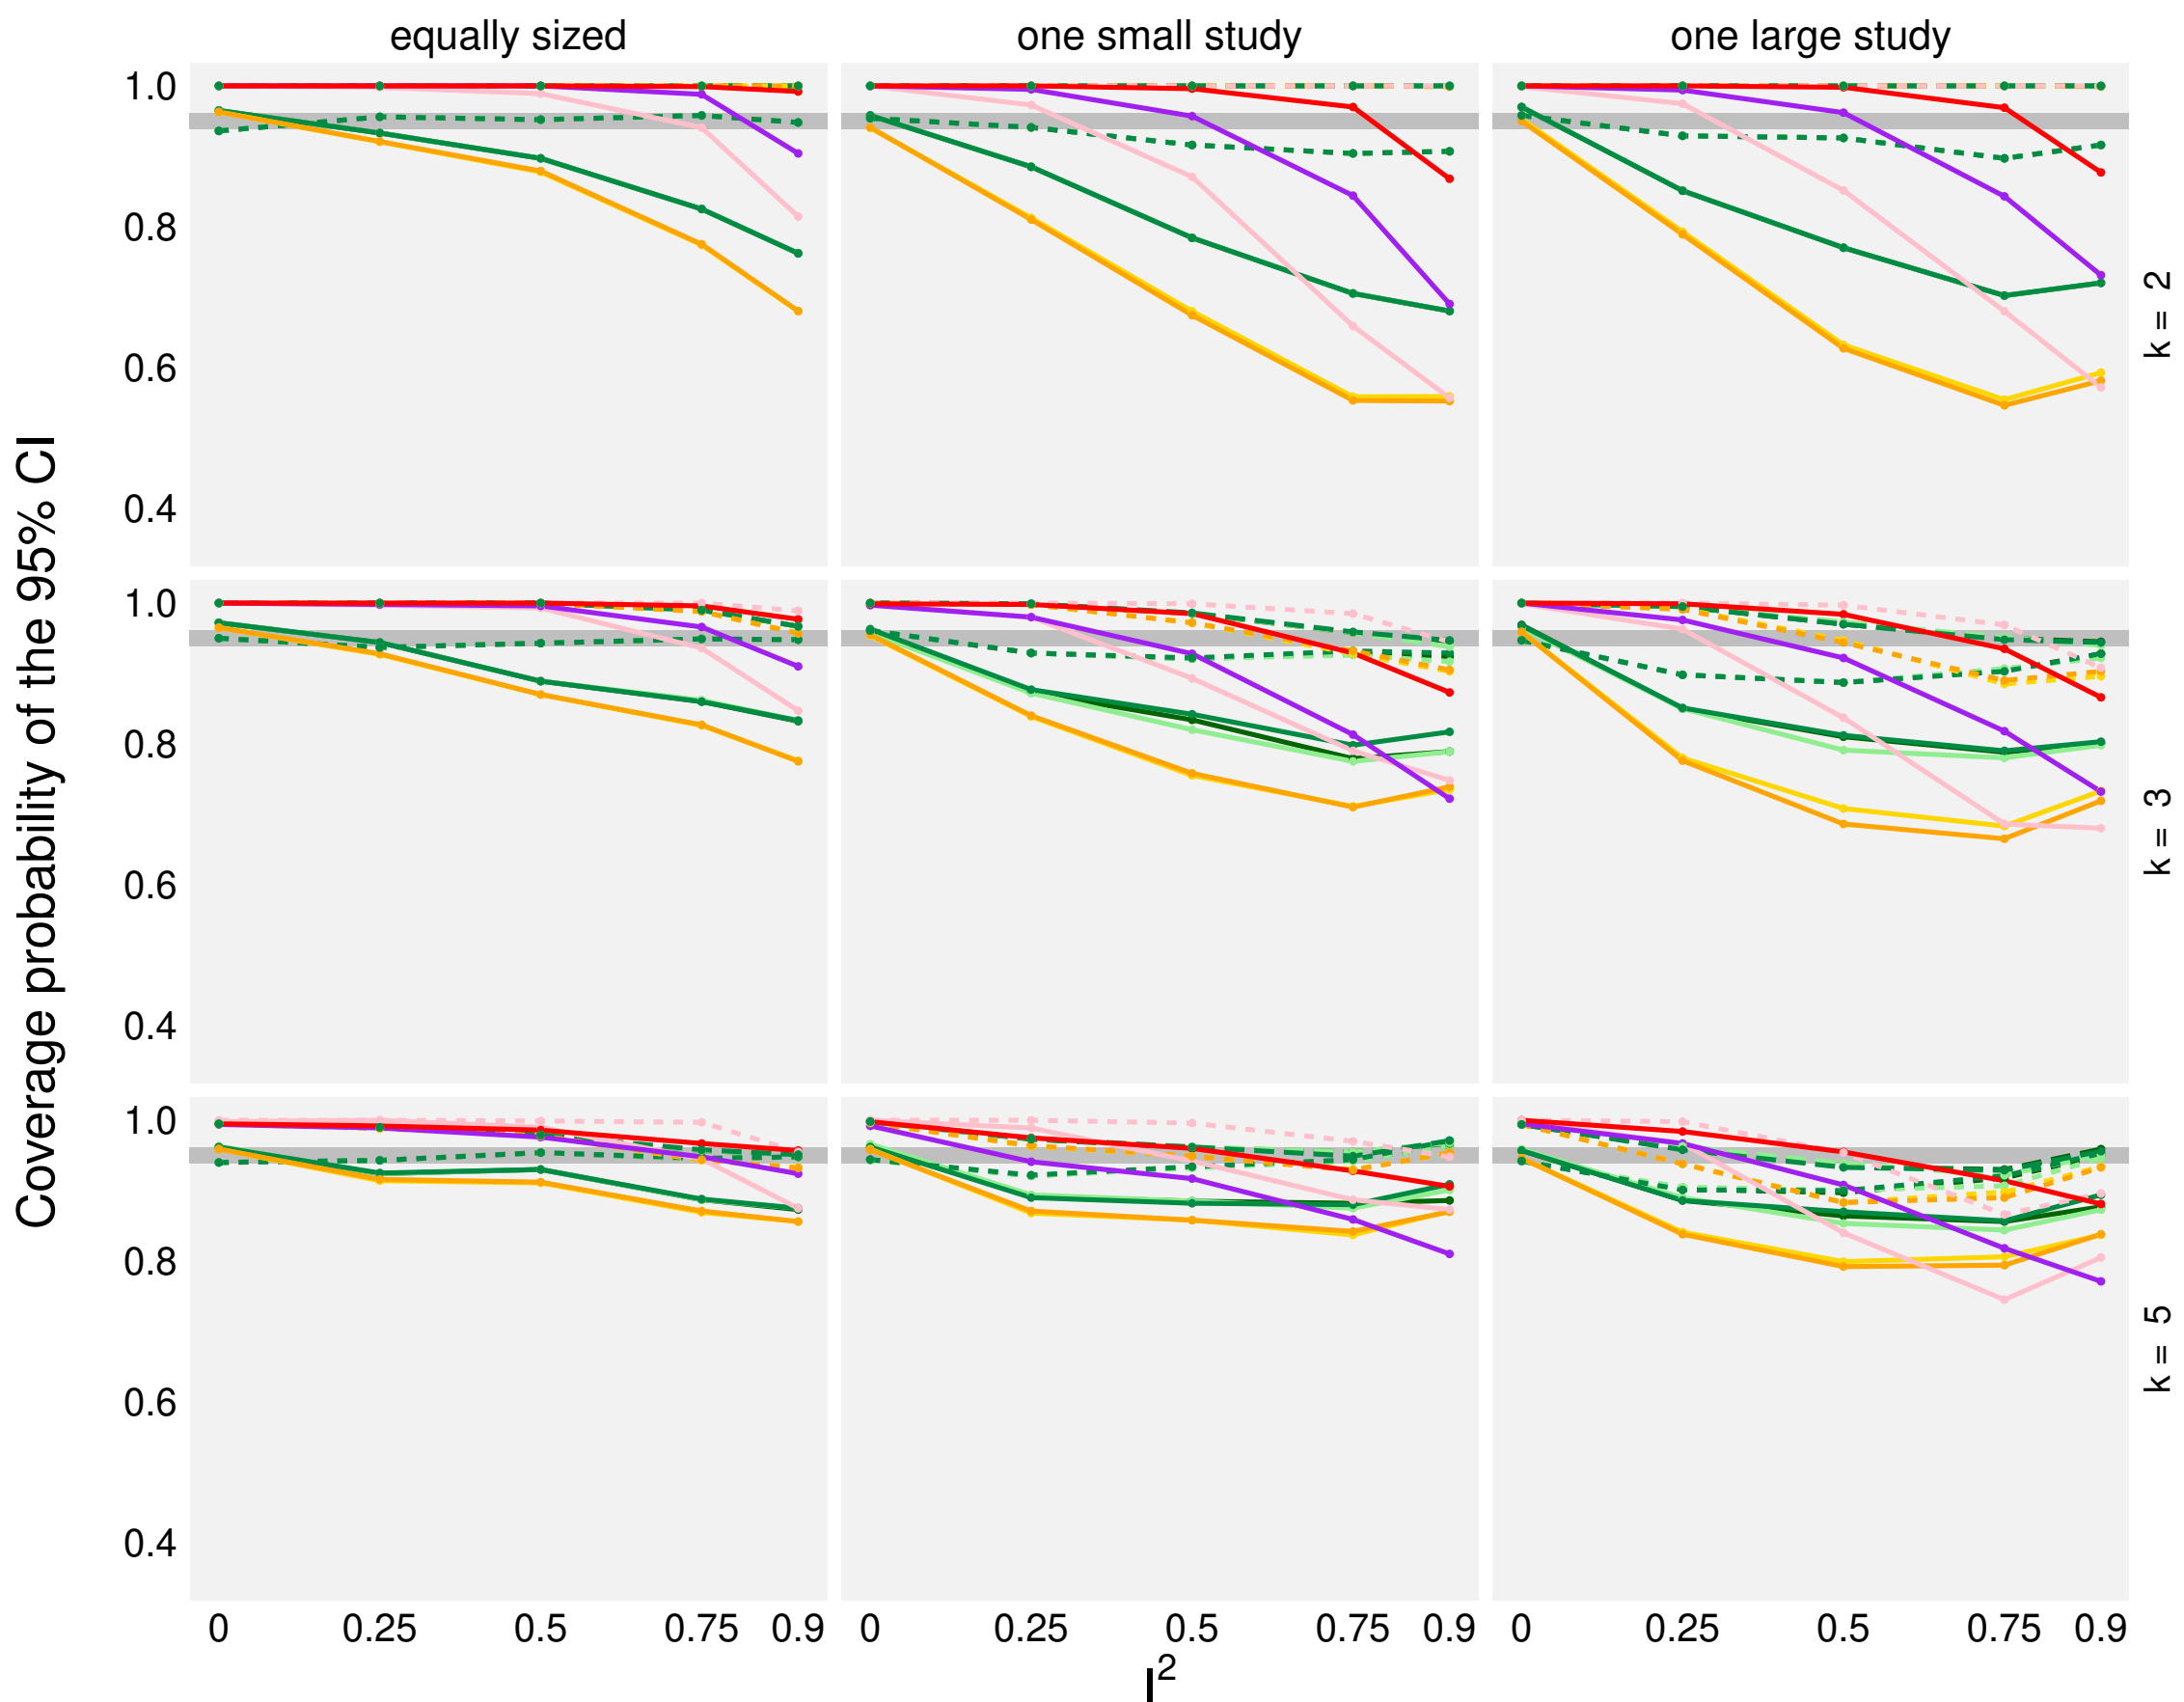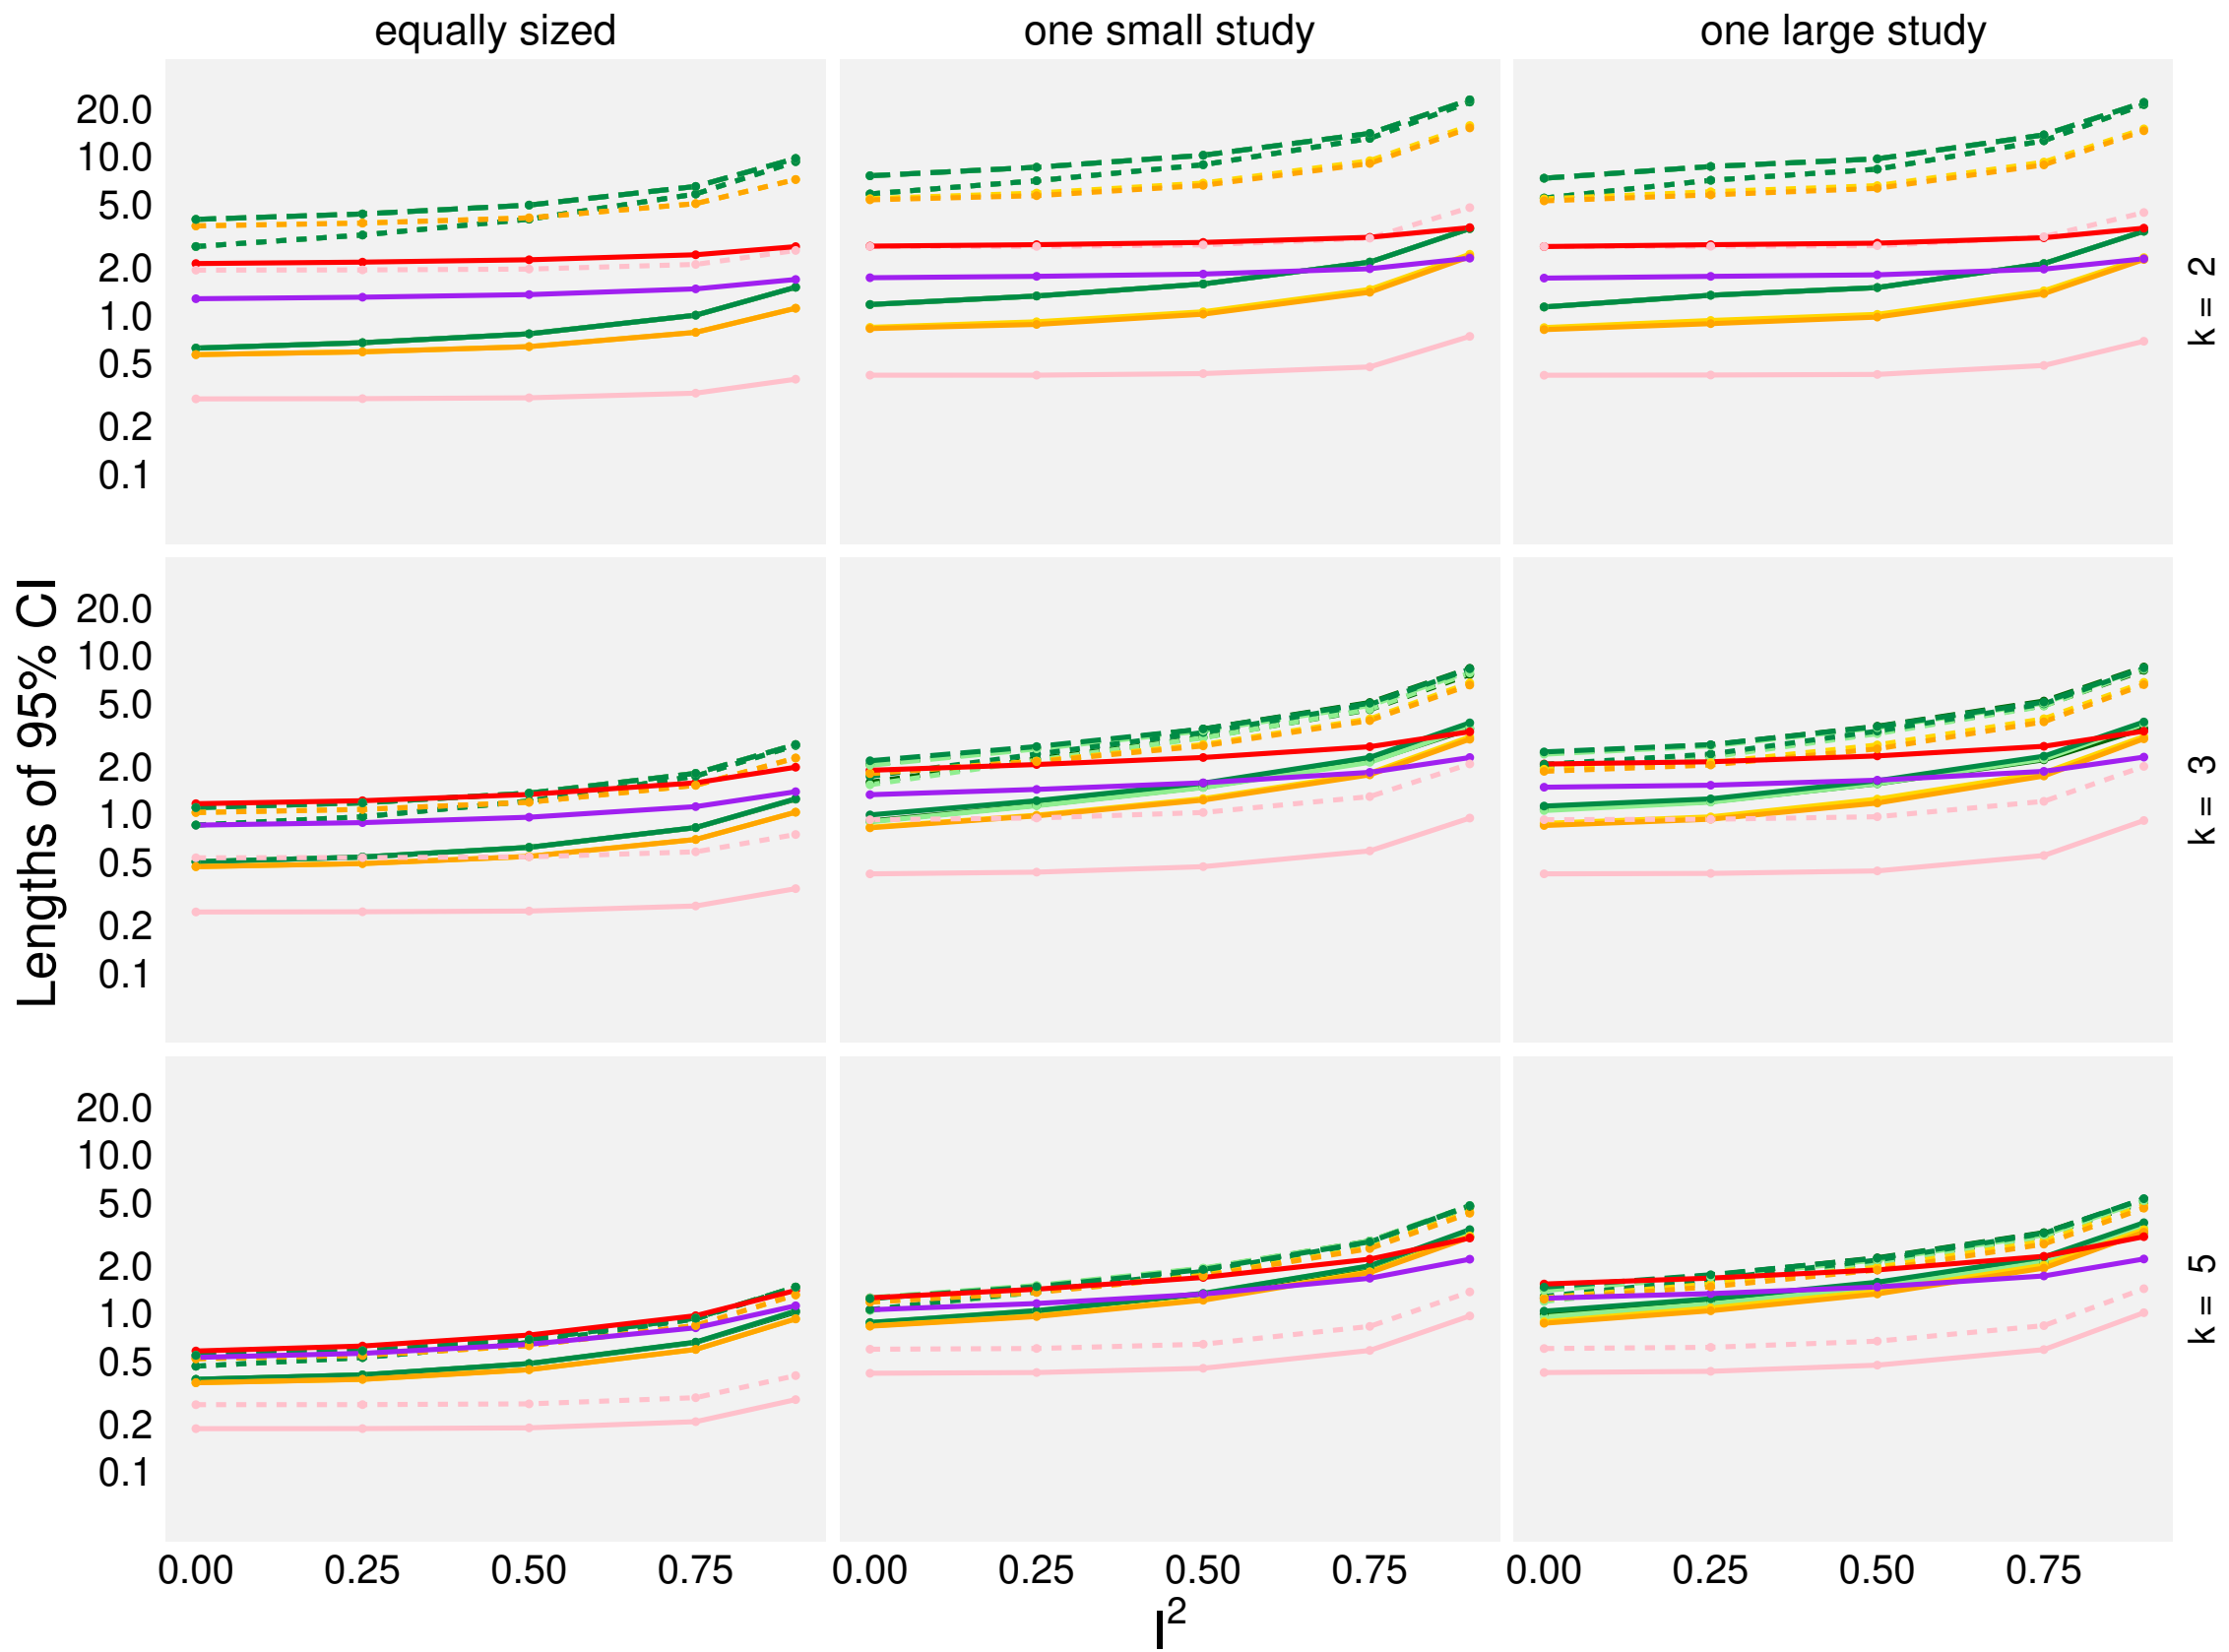

— NN — DL  
 — NN — REML  
 — NN — EB  
 — BN — UM.FS  
 — BN — UM.RS  
 — BN — CM.AL  
 — NN — Bayes HN(0.5)  
 — NN — Bayes HN(1)

— normal quantiles  
 - - HKSJ or Student's t  
 - - mHKSJ

OR  
( $n_i=250, \pi_0=0.9$ )

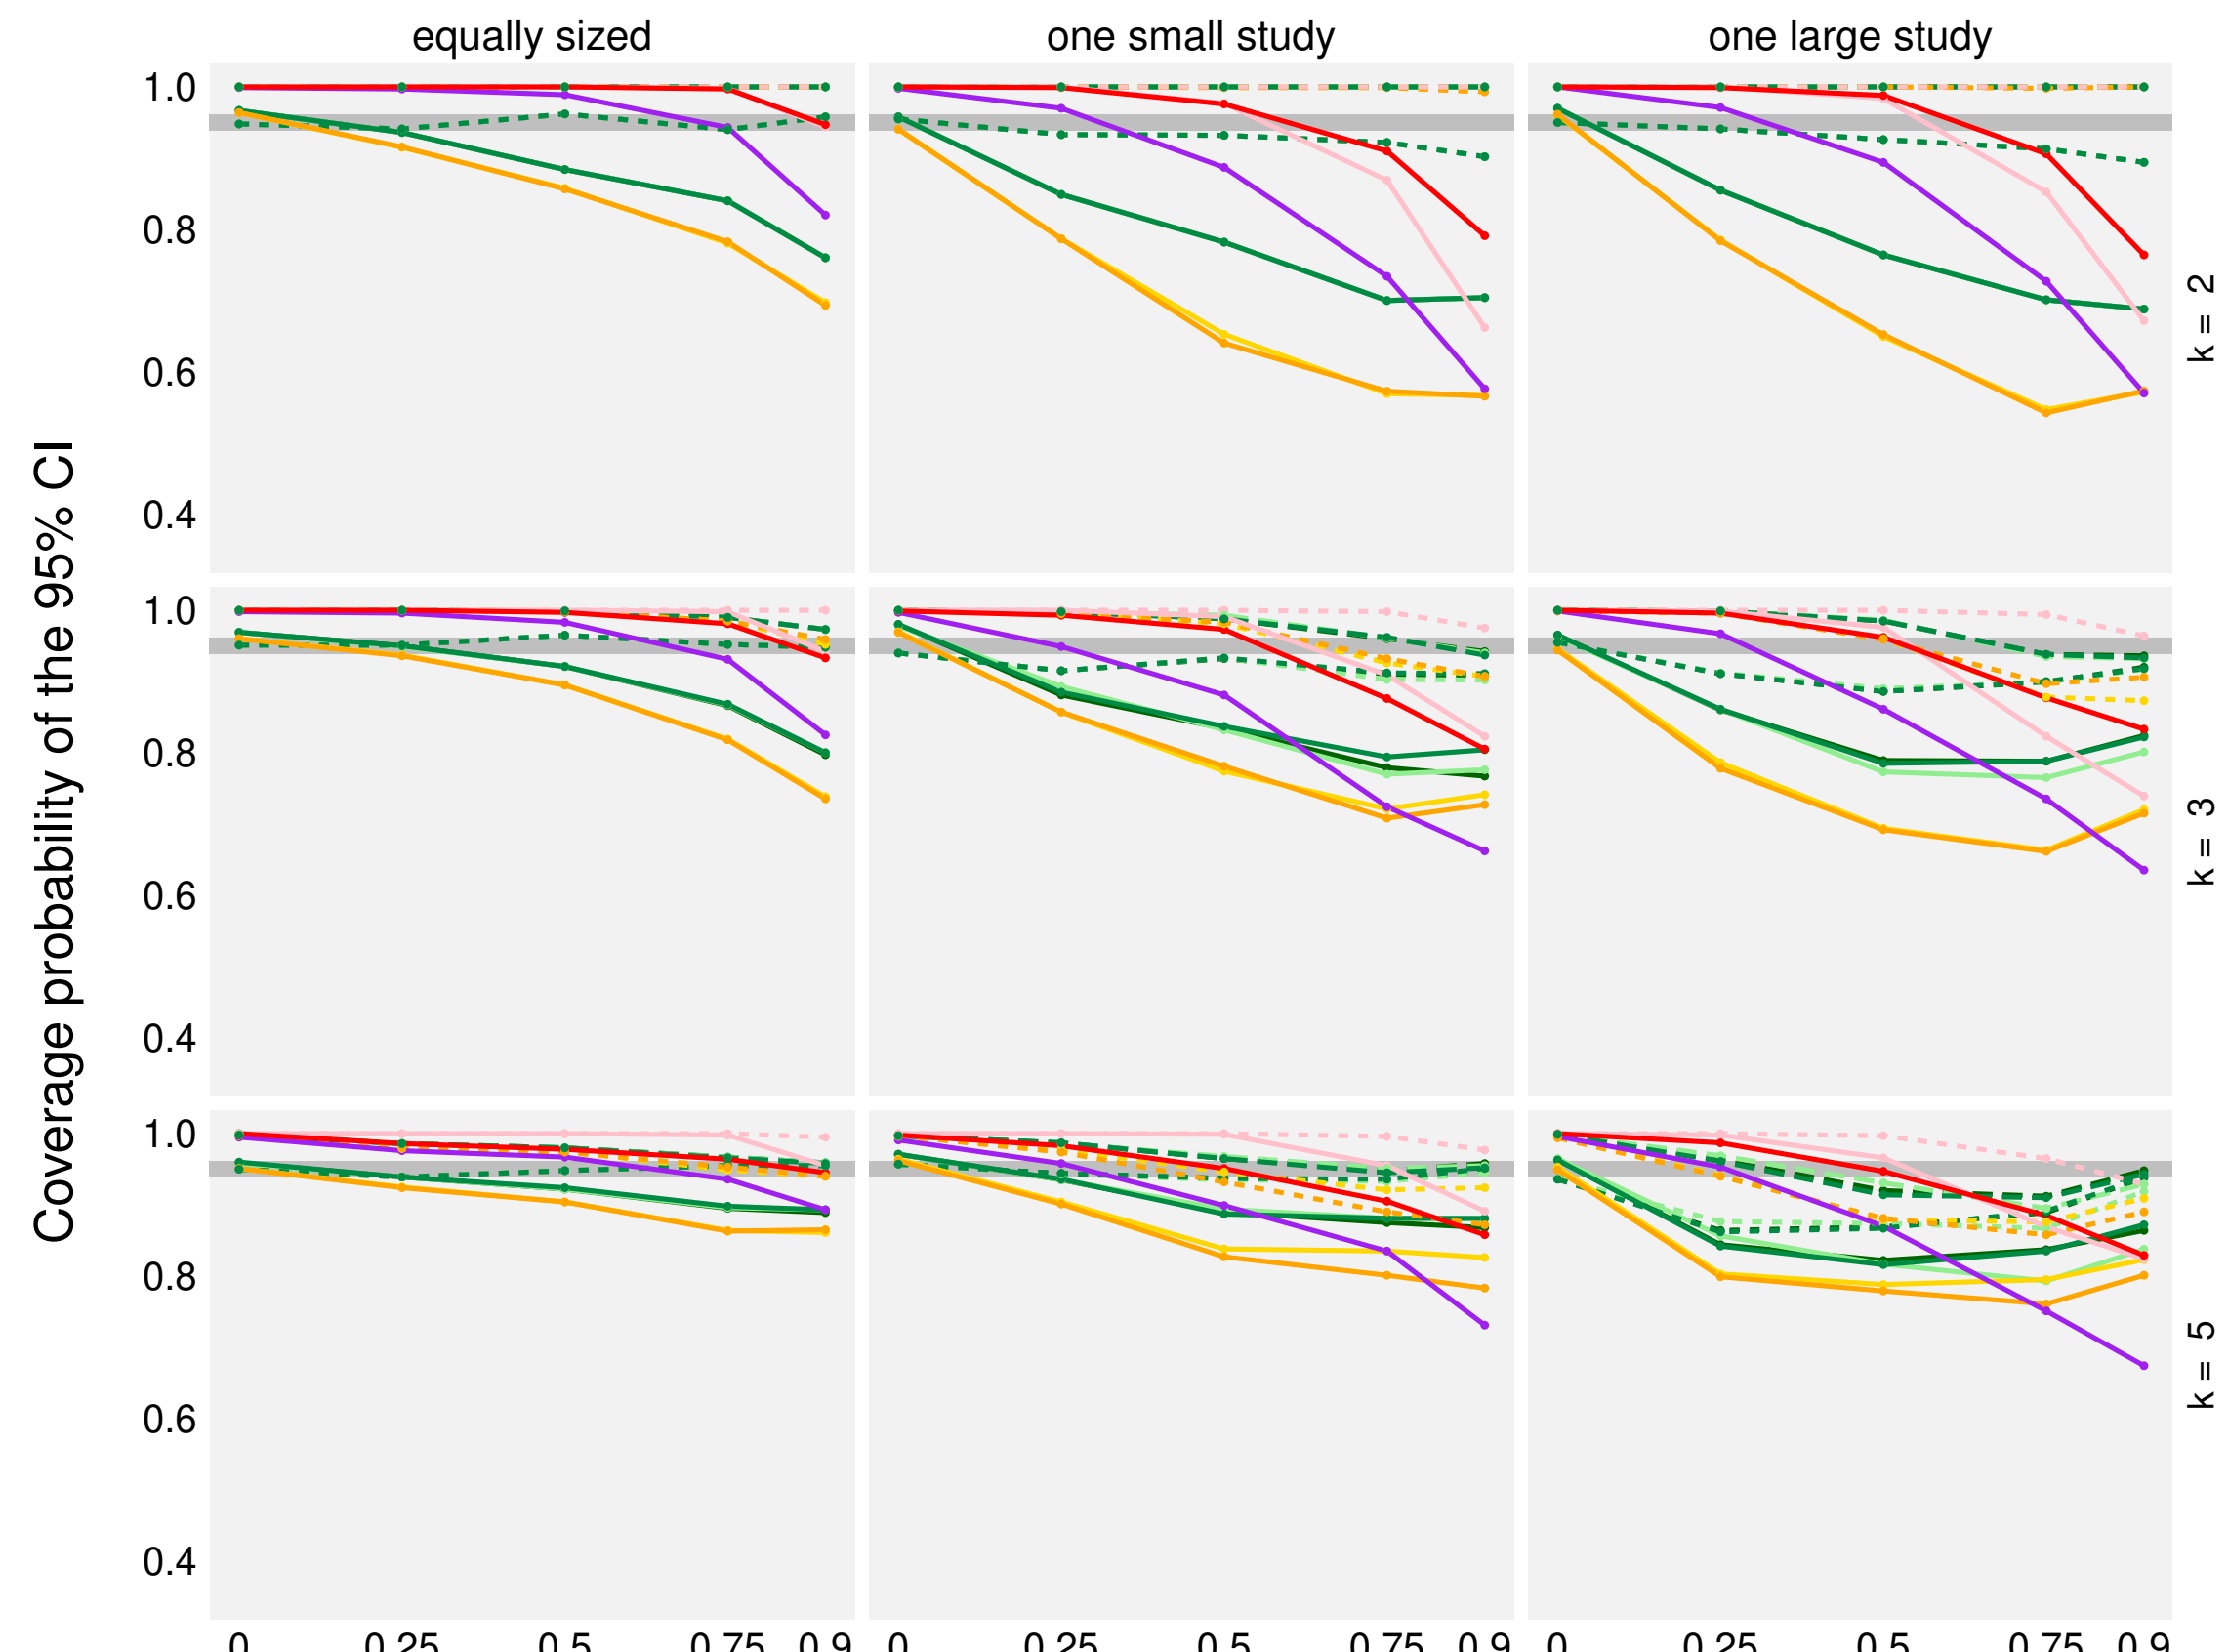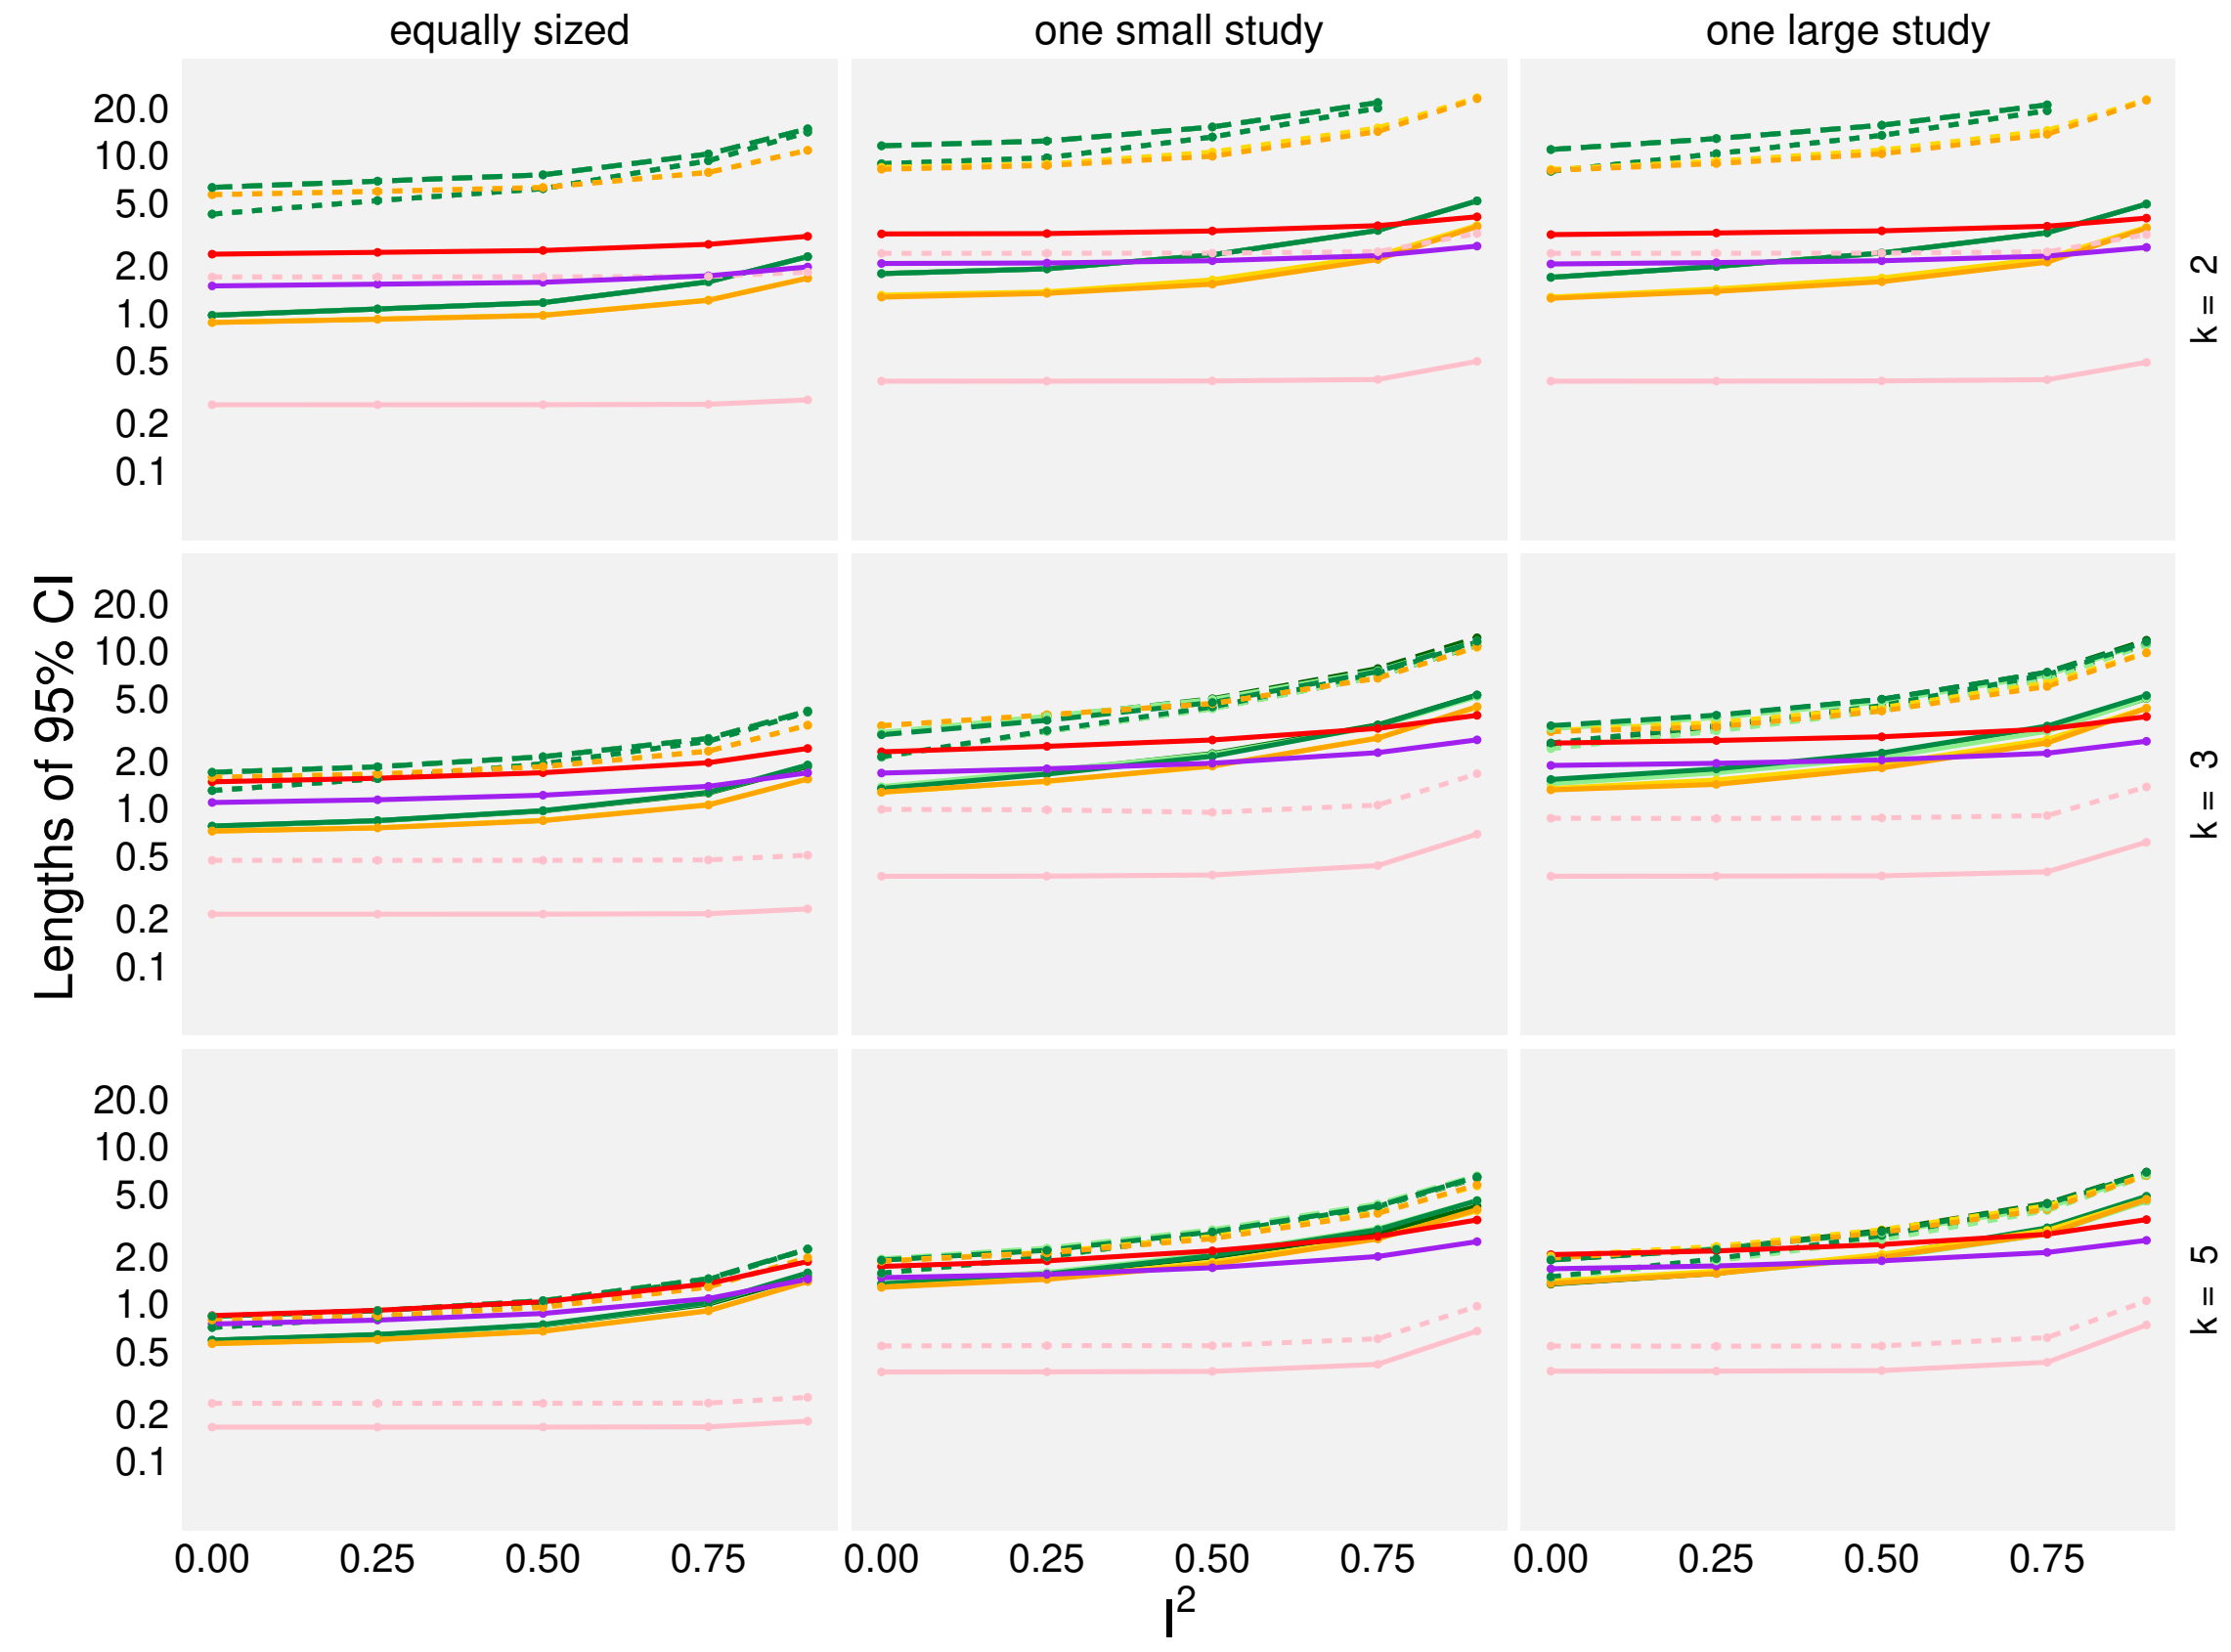

— NN — DL      — BN — UM.RS      — normal quantiles  
 — NN — REML      — BN — CM.AL      -- HKSJ or Student's t  
 — NN — EB      — NN — Bayes HN(0.5)      -- mHKSJ  
 — BN — UM.FS      — NN — Bayes HN(1)

OR  
( $n_i=500, \pi_0=0.1$ )

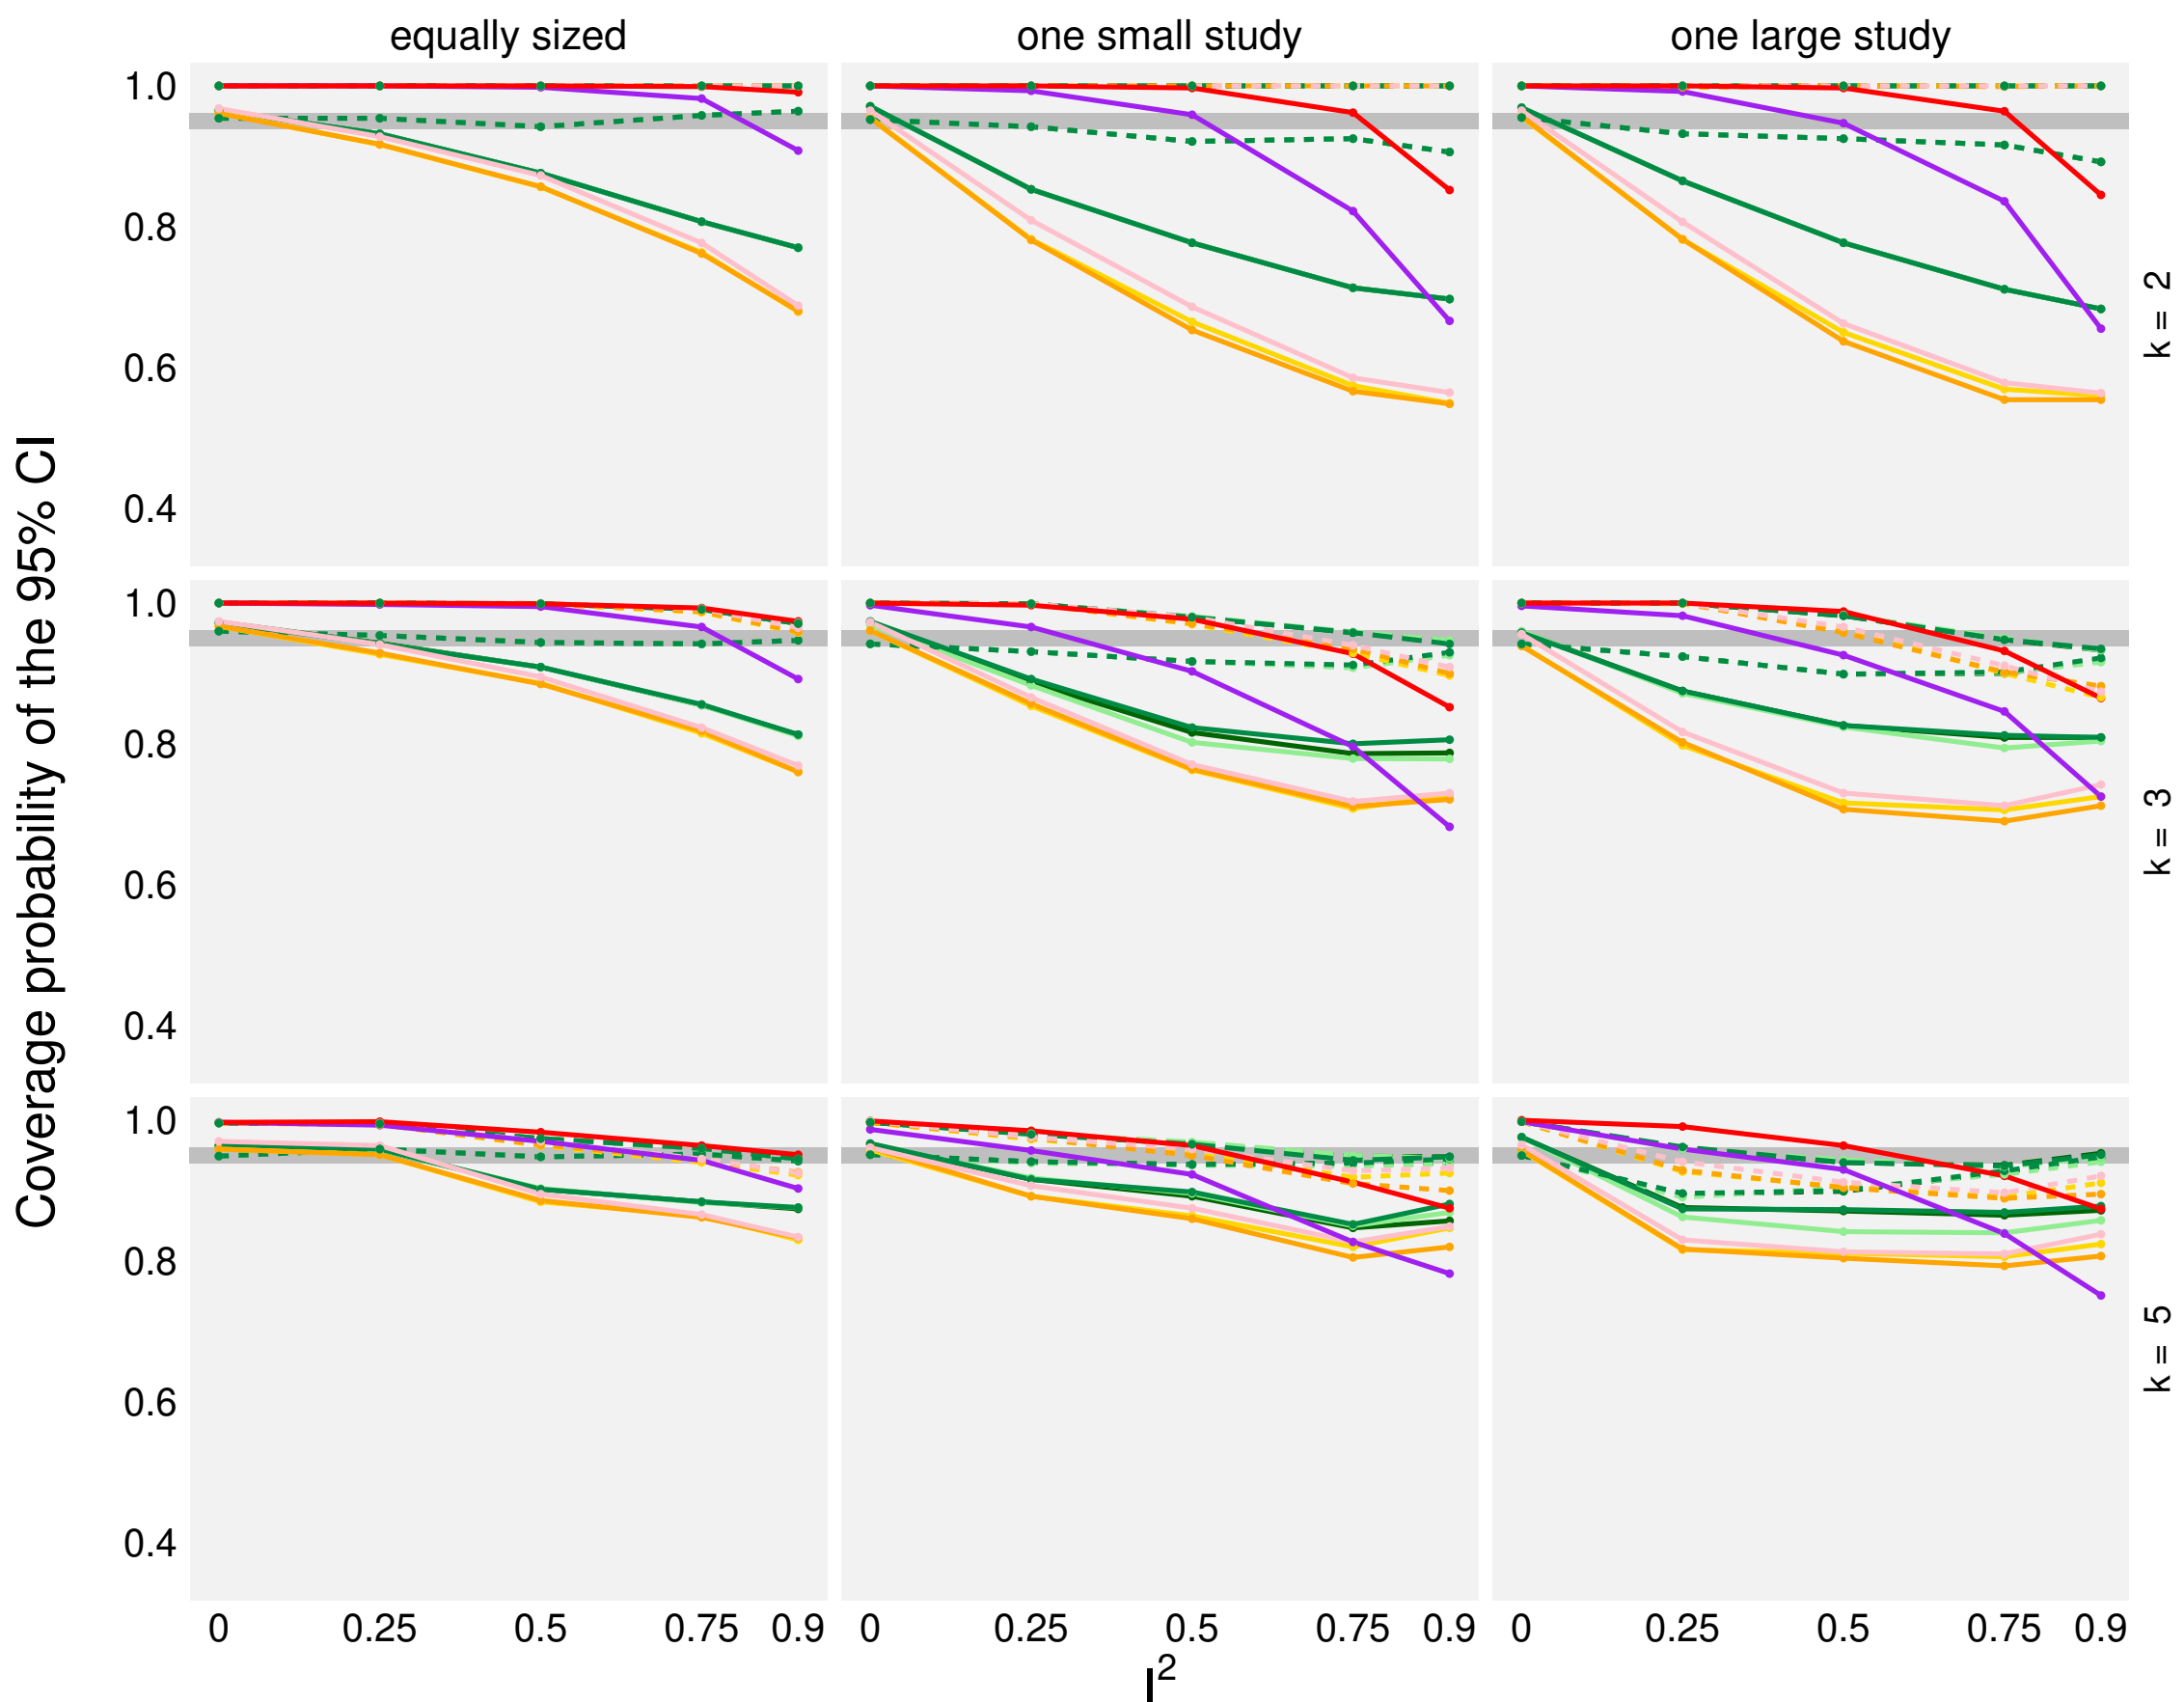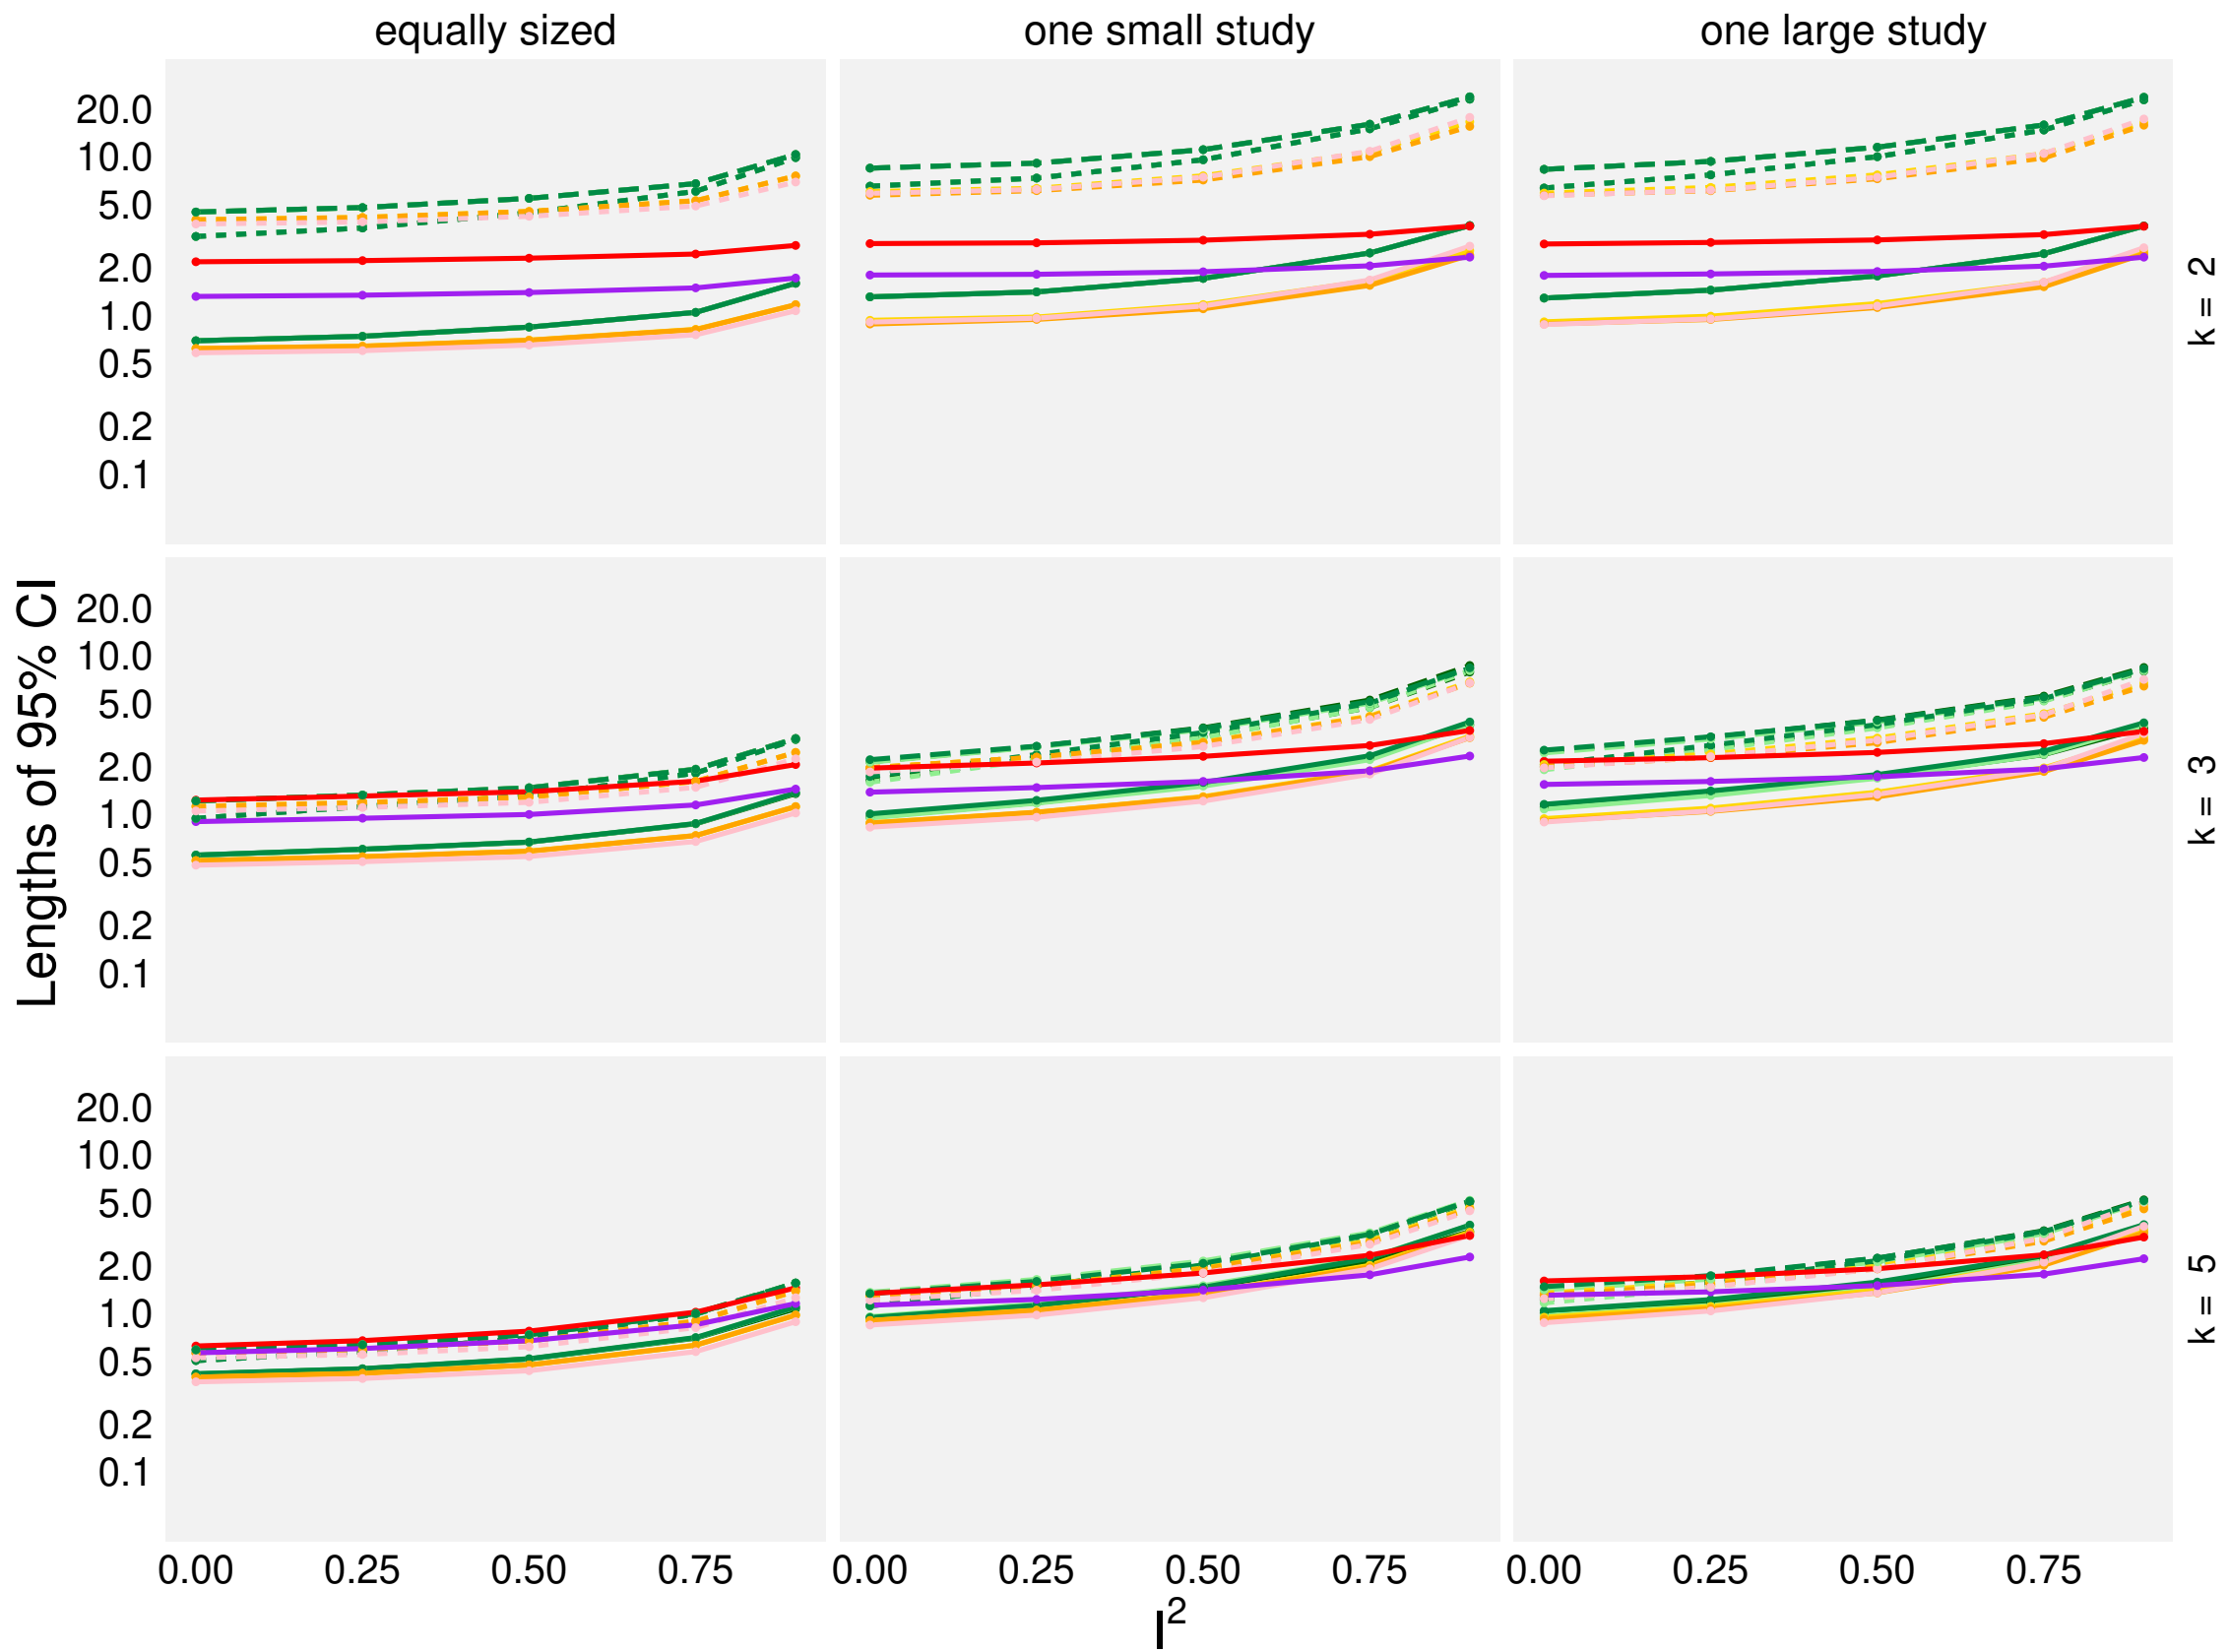

NN – DL  
 NN – REML  
 NN – EB  
 BN – UM.FS  
 BN – UM.RS  
 BN – CM.AL  
 NN – Bayes HN(0.5)  
 NN – Bayes HN(1)  
 — normal quantiles  
 -- HKSJ or Student's t  
 ··· mHKSJ

OR  
( $n_i=500, \pi_0=0.3$ )

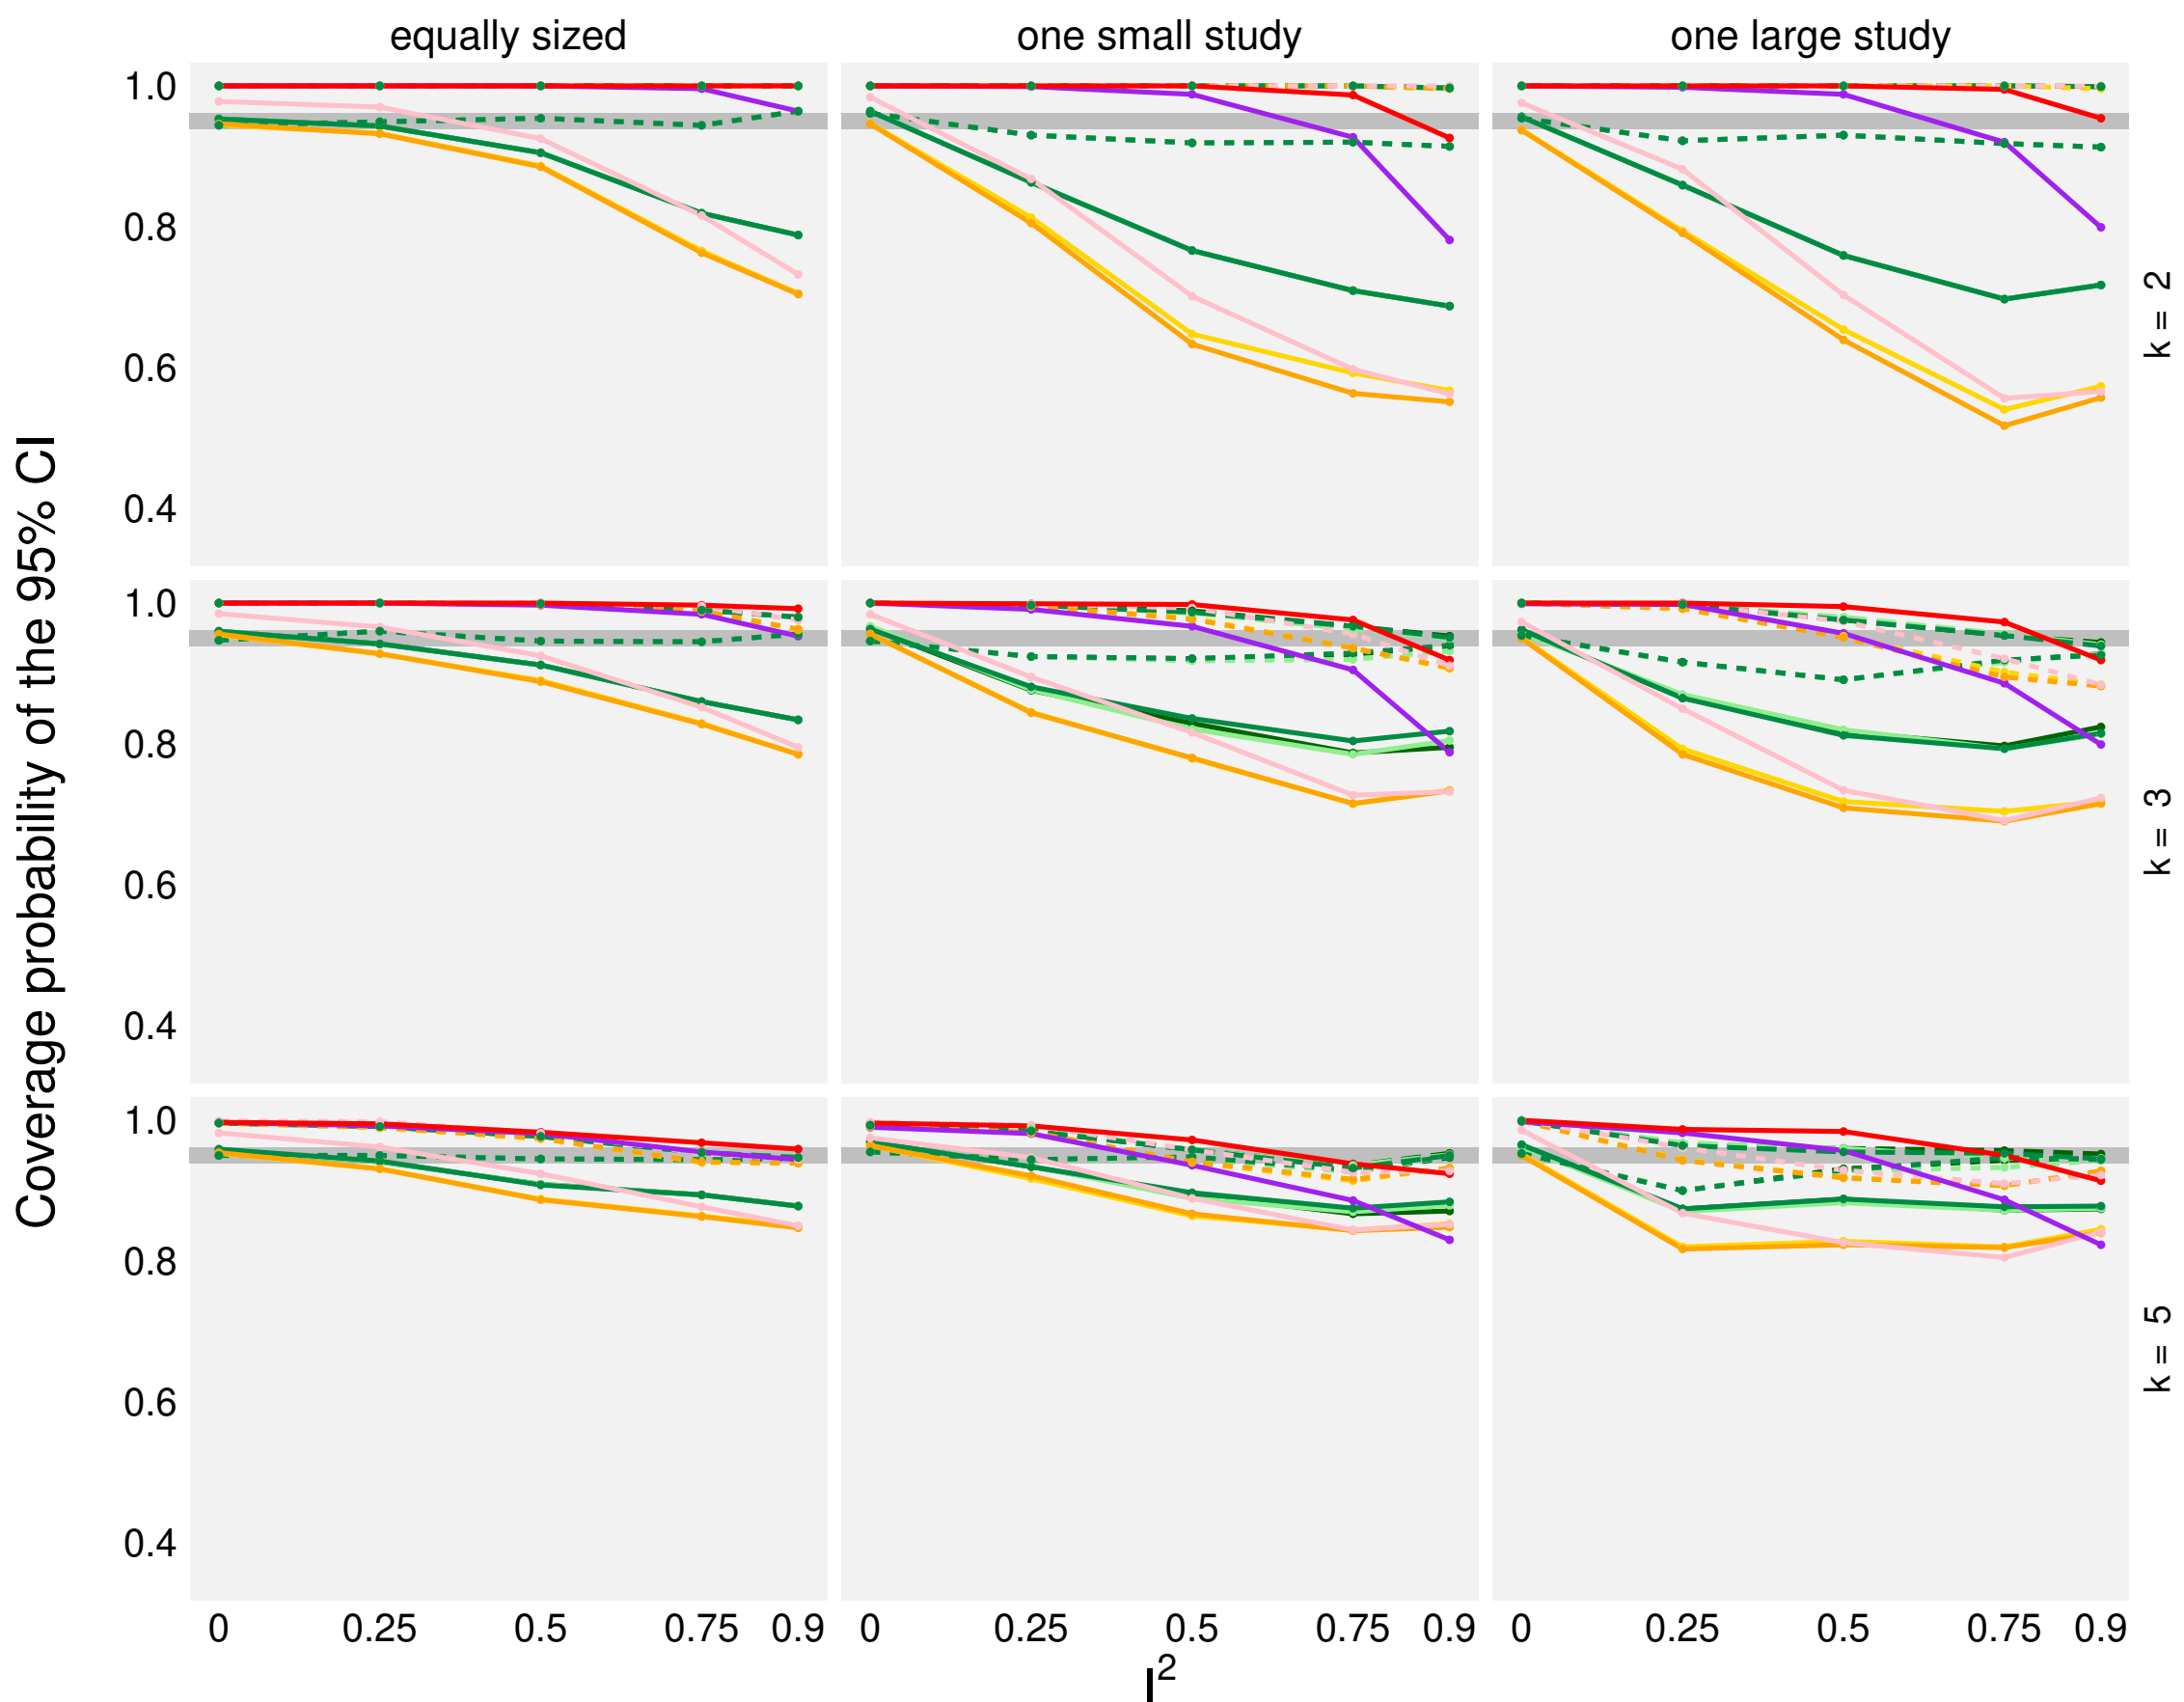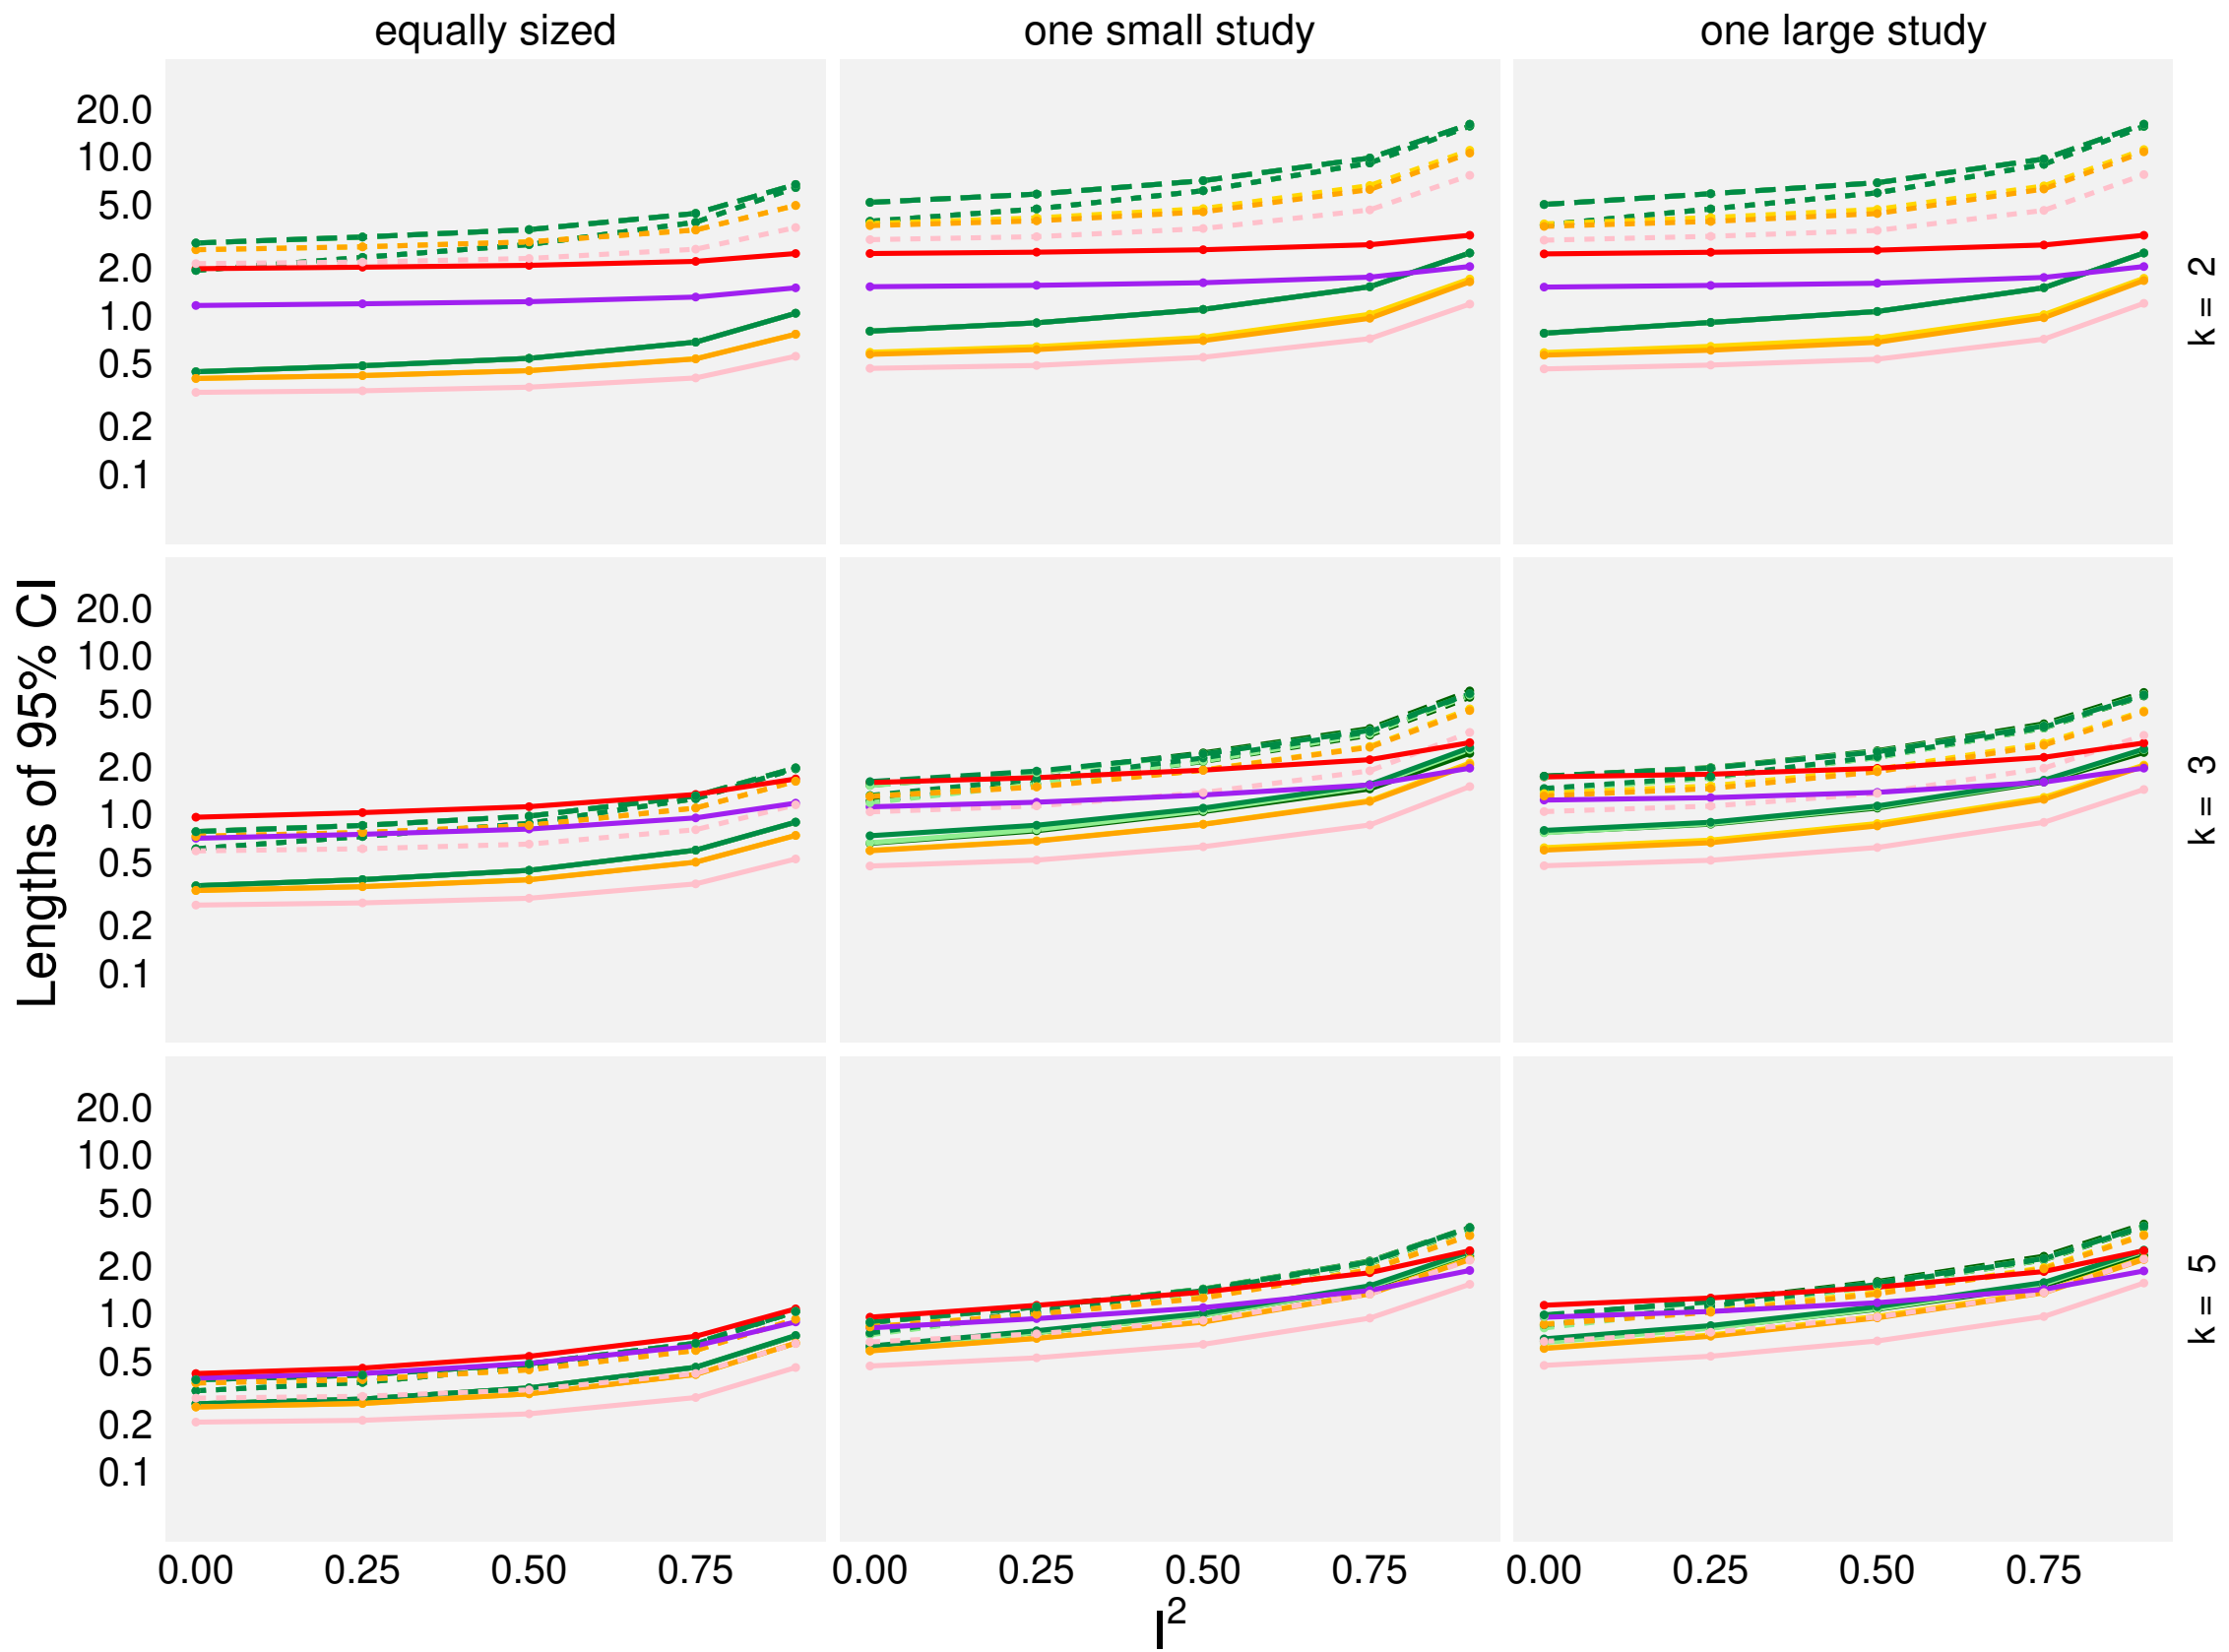

— NN — DL  
 — NN — REML  
 — NN — EB  
 — BN — UM.FS  
 — BN — UM.RS  
 — BN — CM.AL  
 — NN — Bayes HN(0.5)  
 — NN — Bayes HN(1)

— normal quantiles  
 - - HKSJ or Student's t  
 - - mHKSJ

OR  
( $n_i=500, \pi_0=0.5$ )

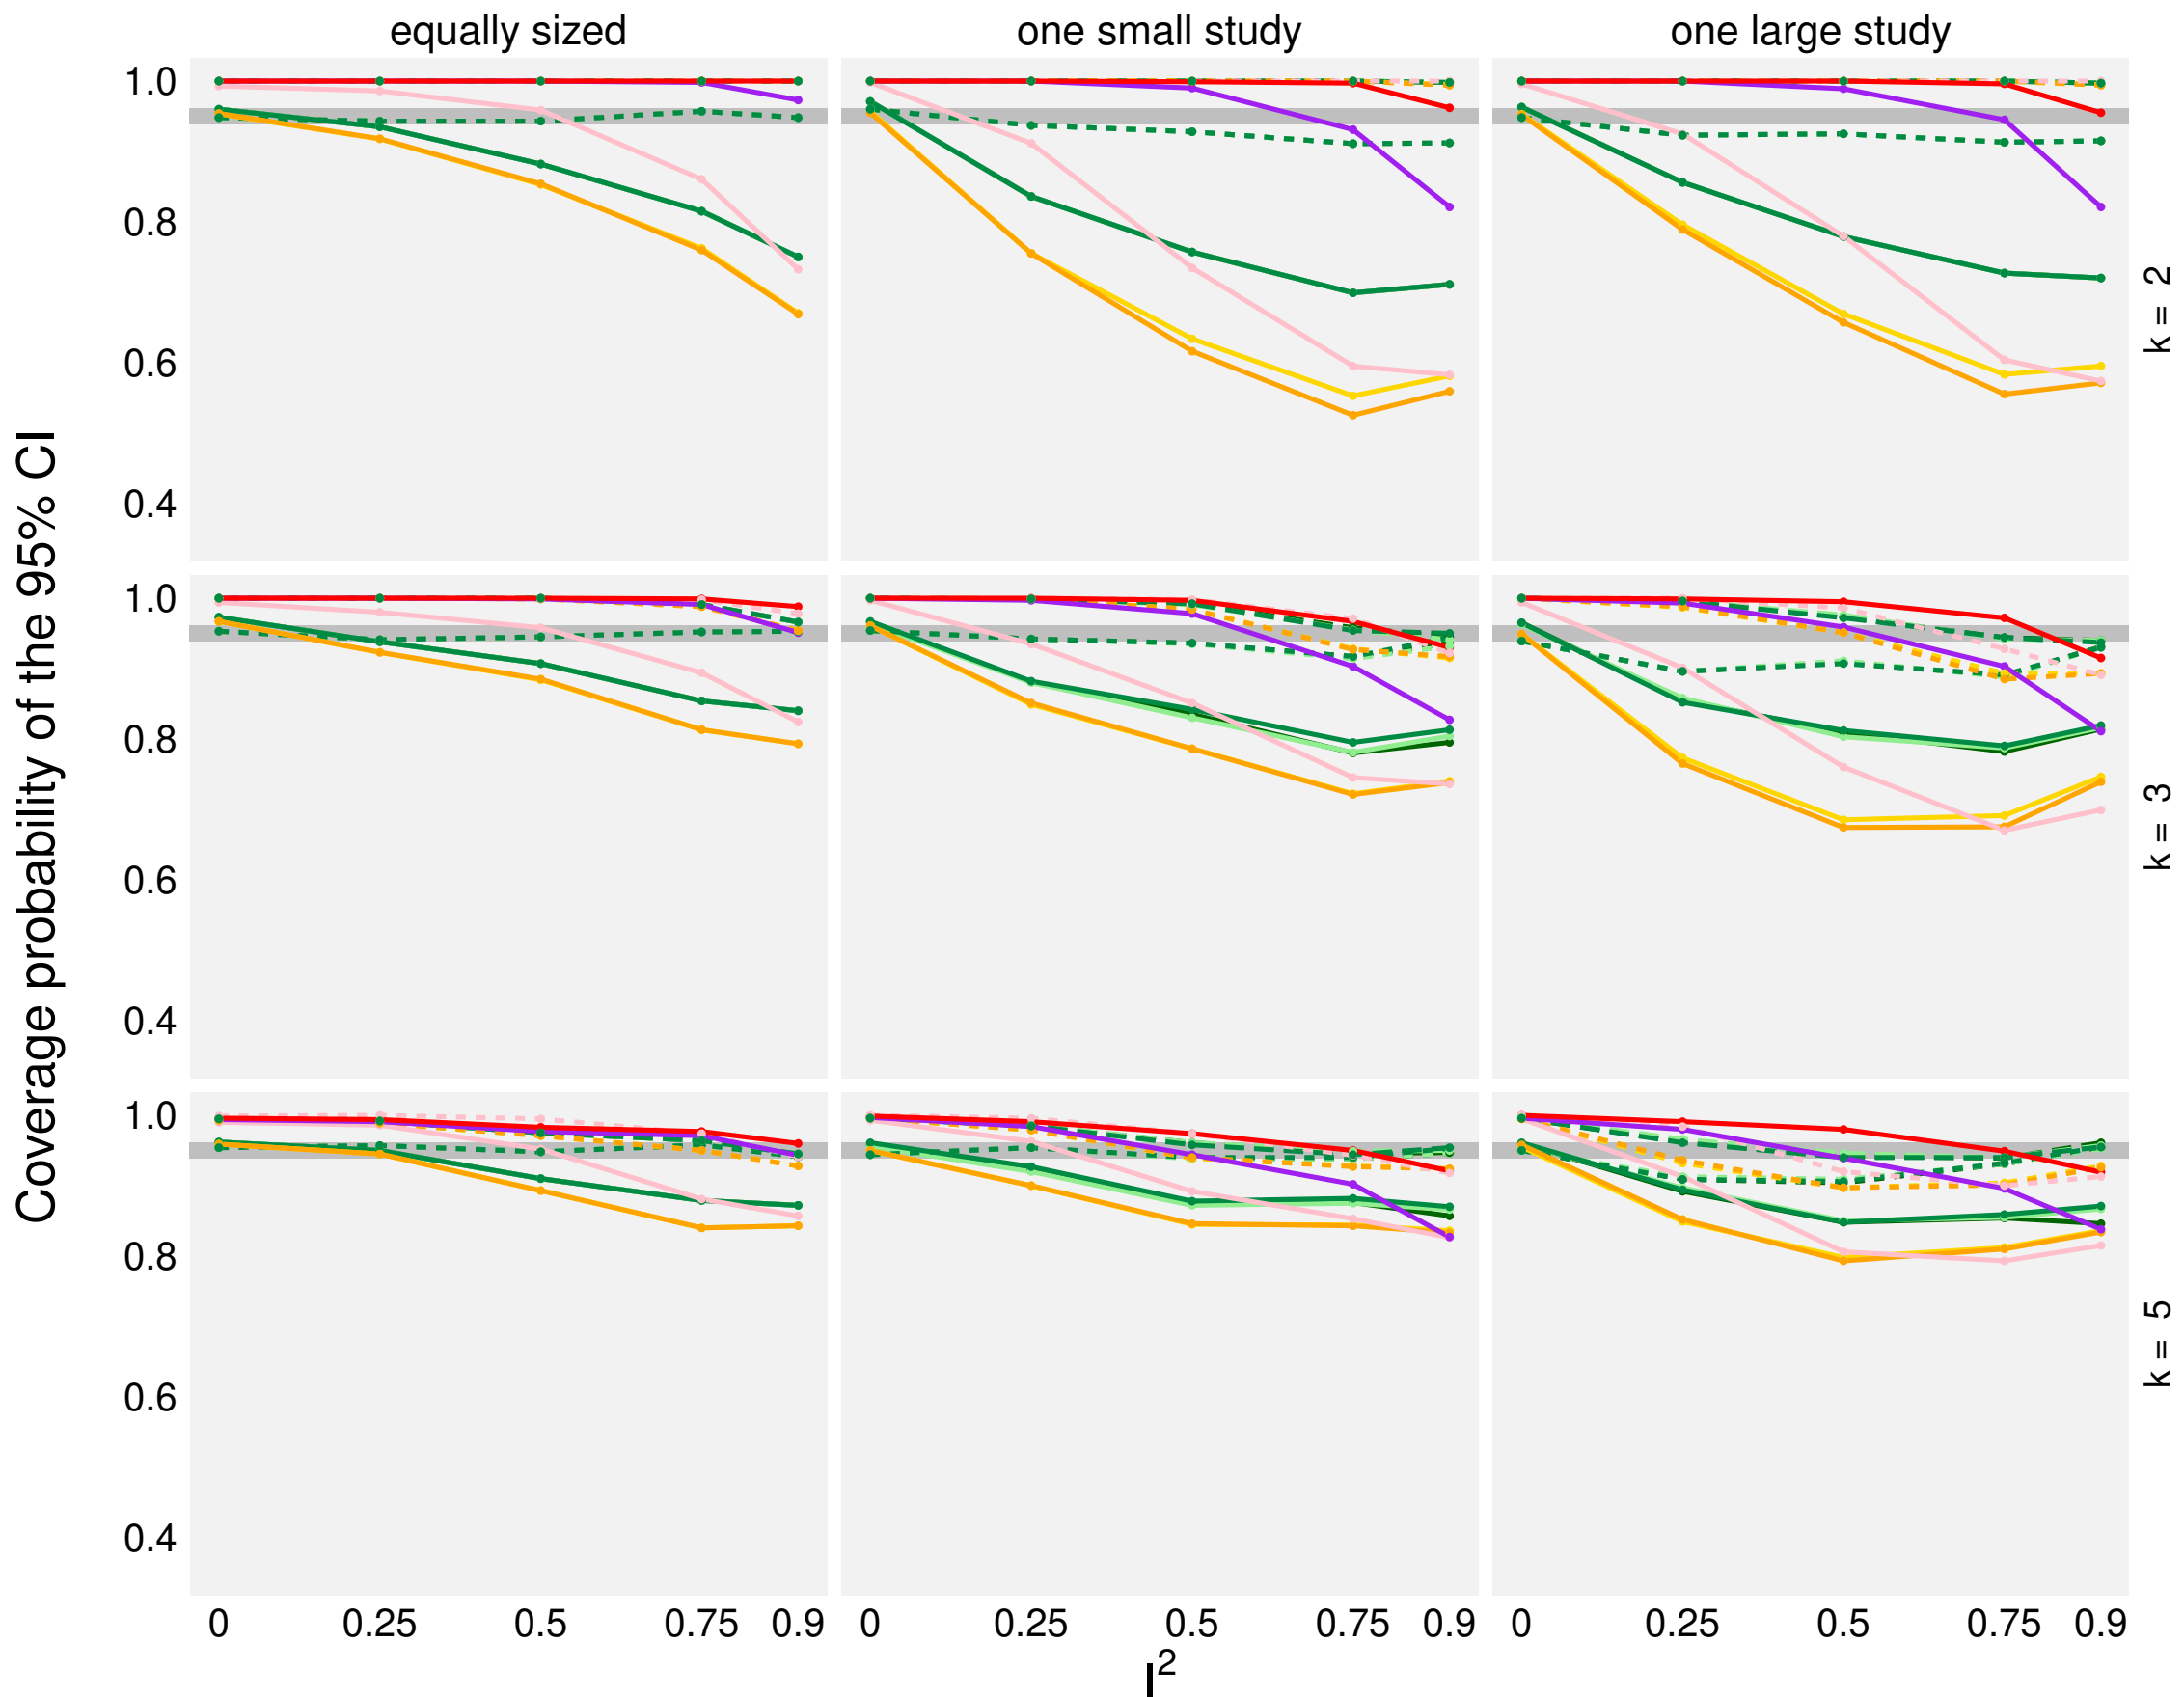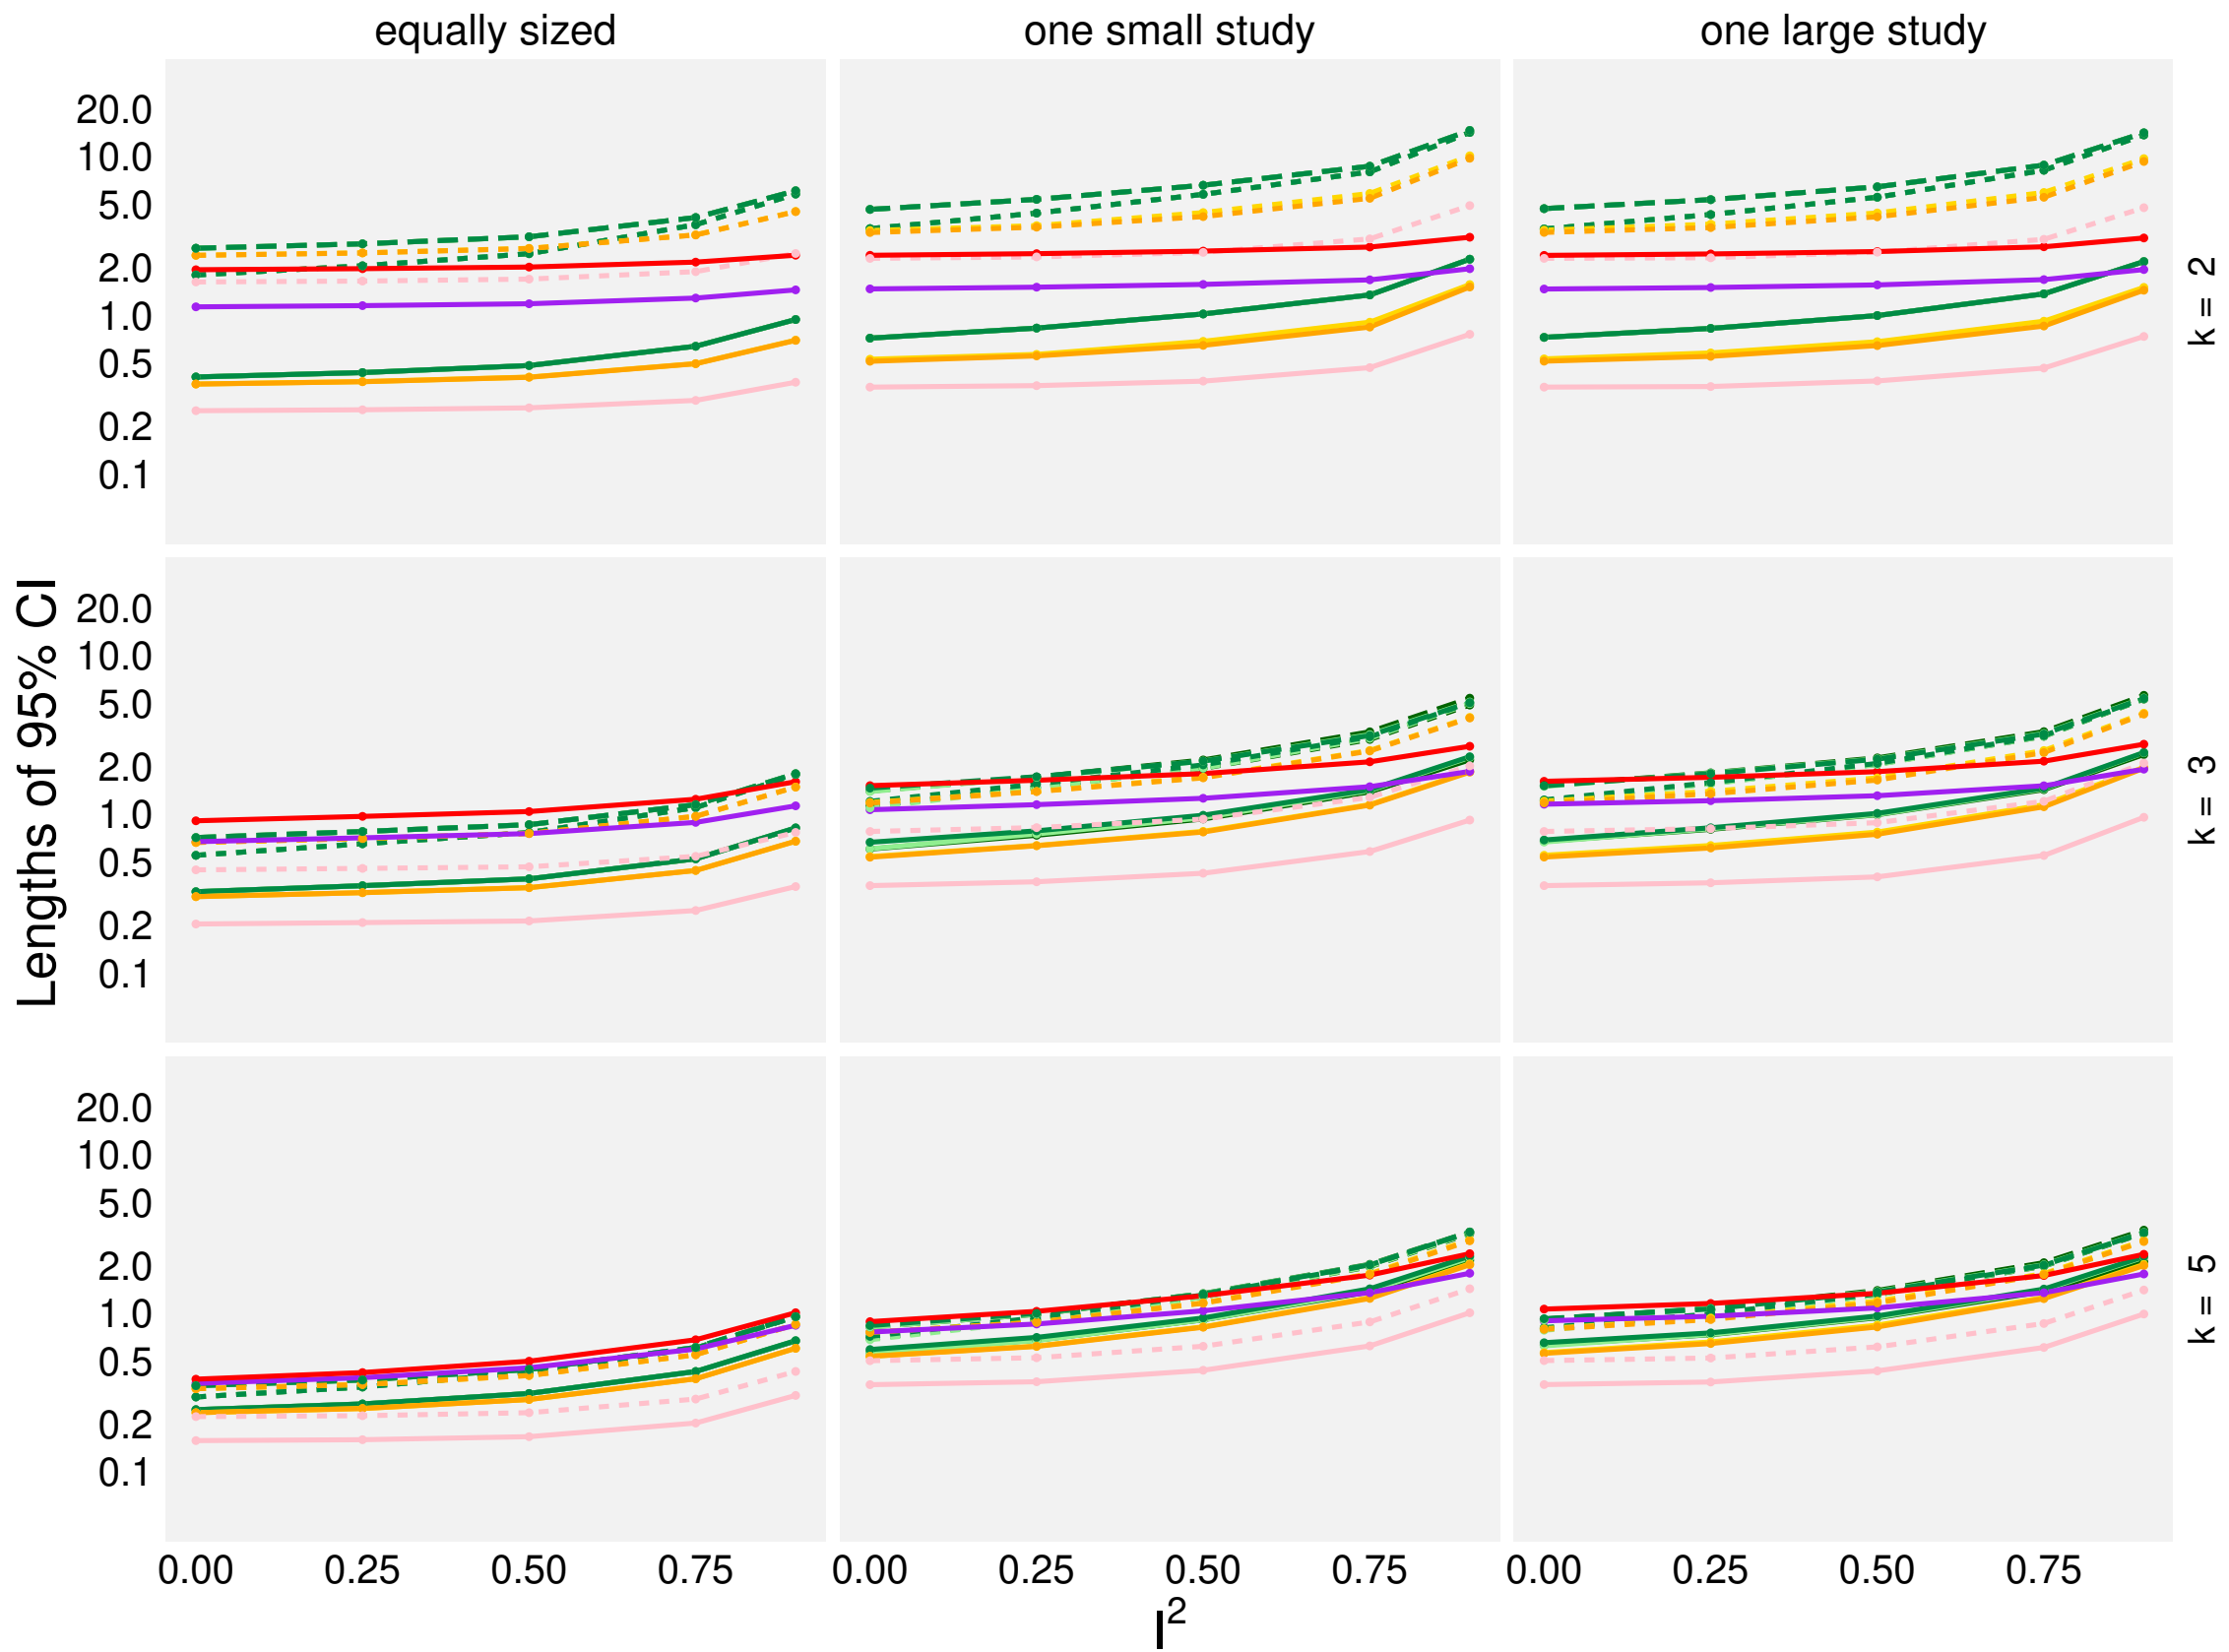

— NN — DL  
 — NN — REML  
 — NN — EB  
 — BN — UM.FS  
 — BN — UM.RS  
 — BN — CM.AL  
 — NN — Bayes HN(0.5)  
 — NN — Bayes HN(1)

— normal quantiles  
 - - HKSJ or Student's t  
 - - mHKSJ

OR  
( $n_i=500, \pi_0=0.7$ )

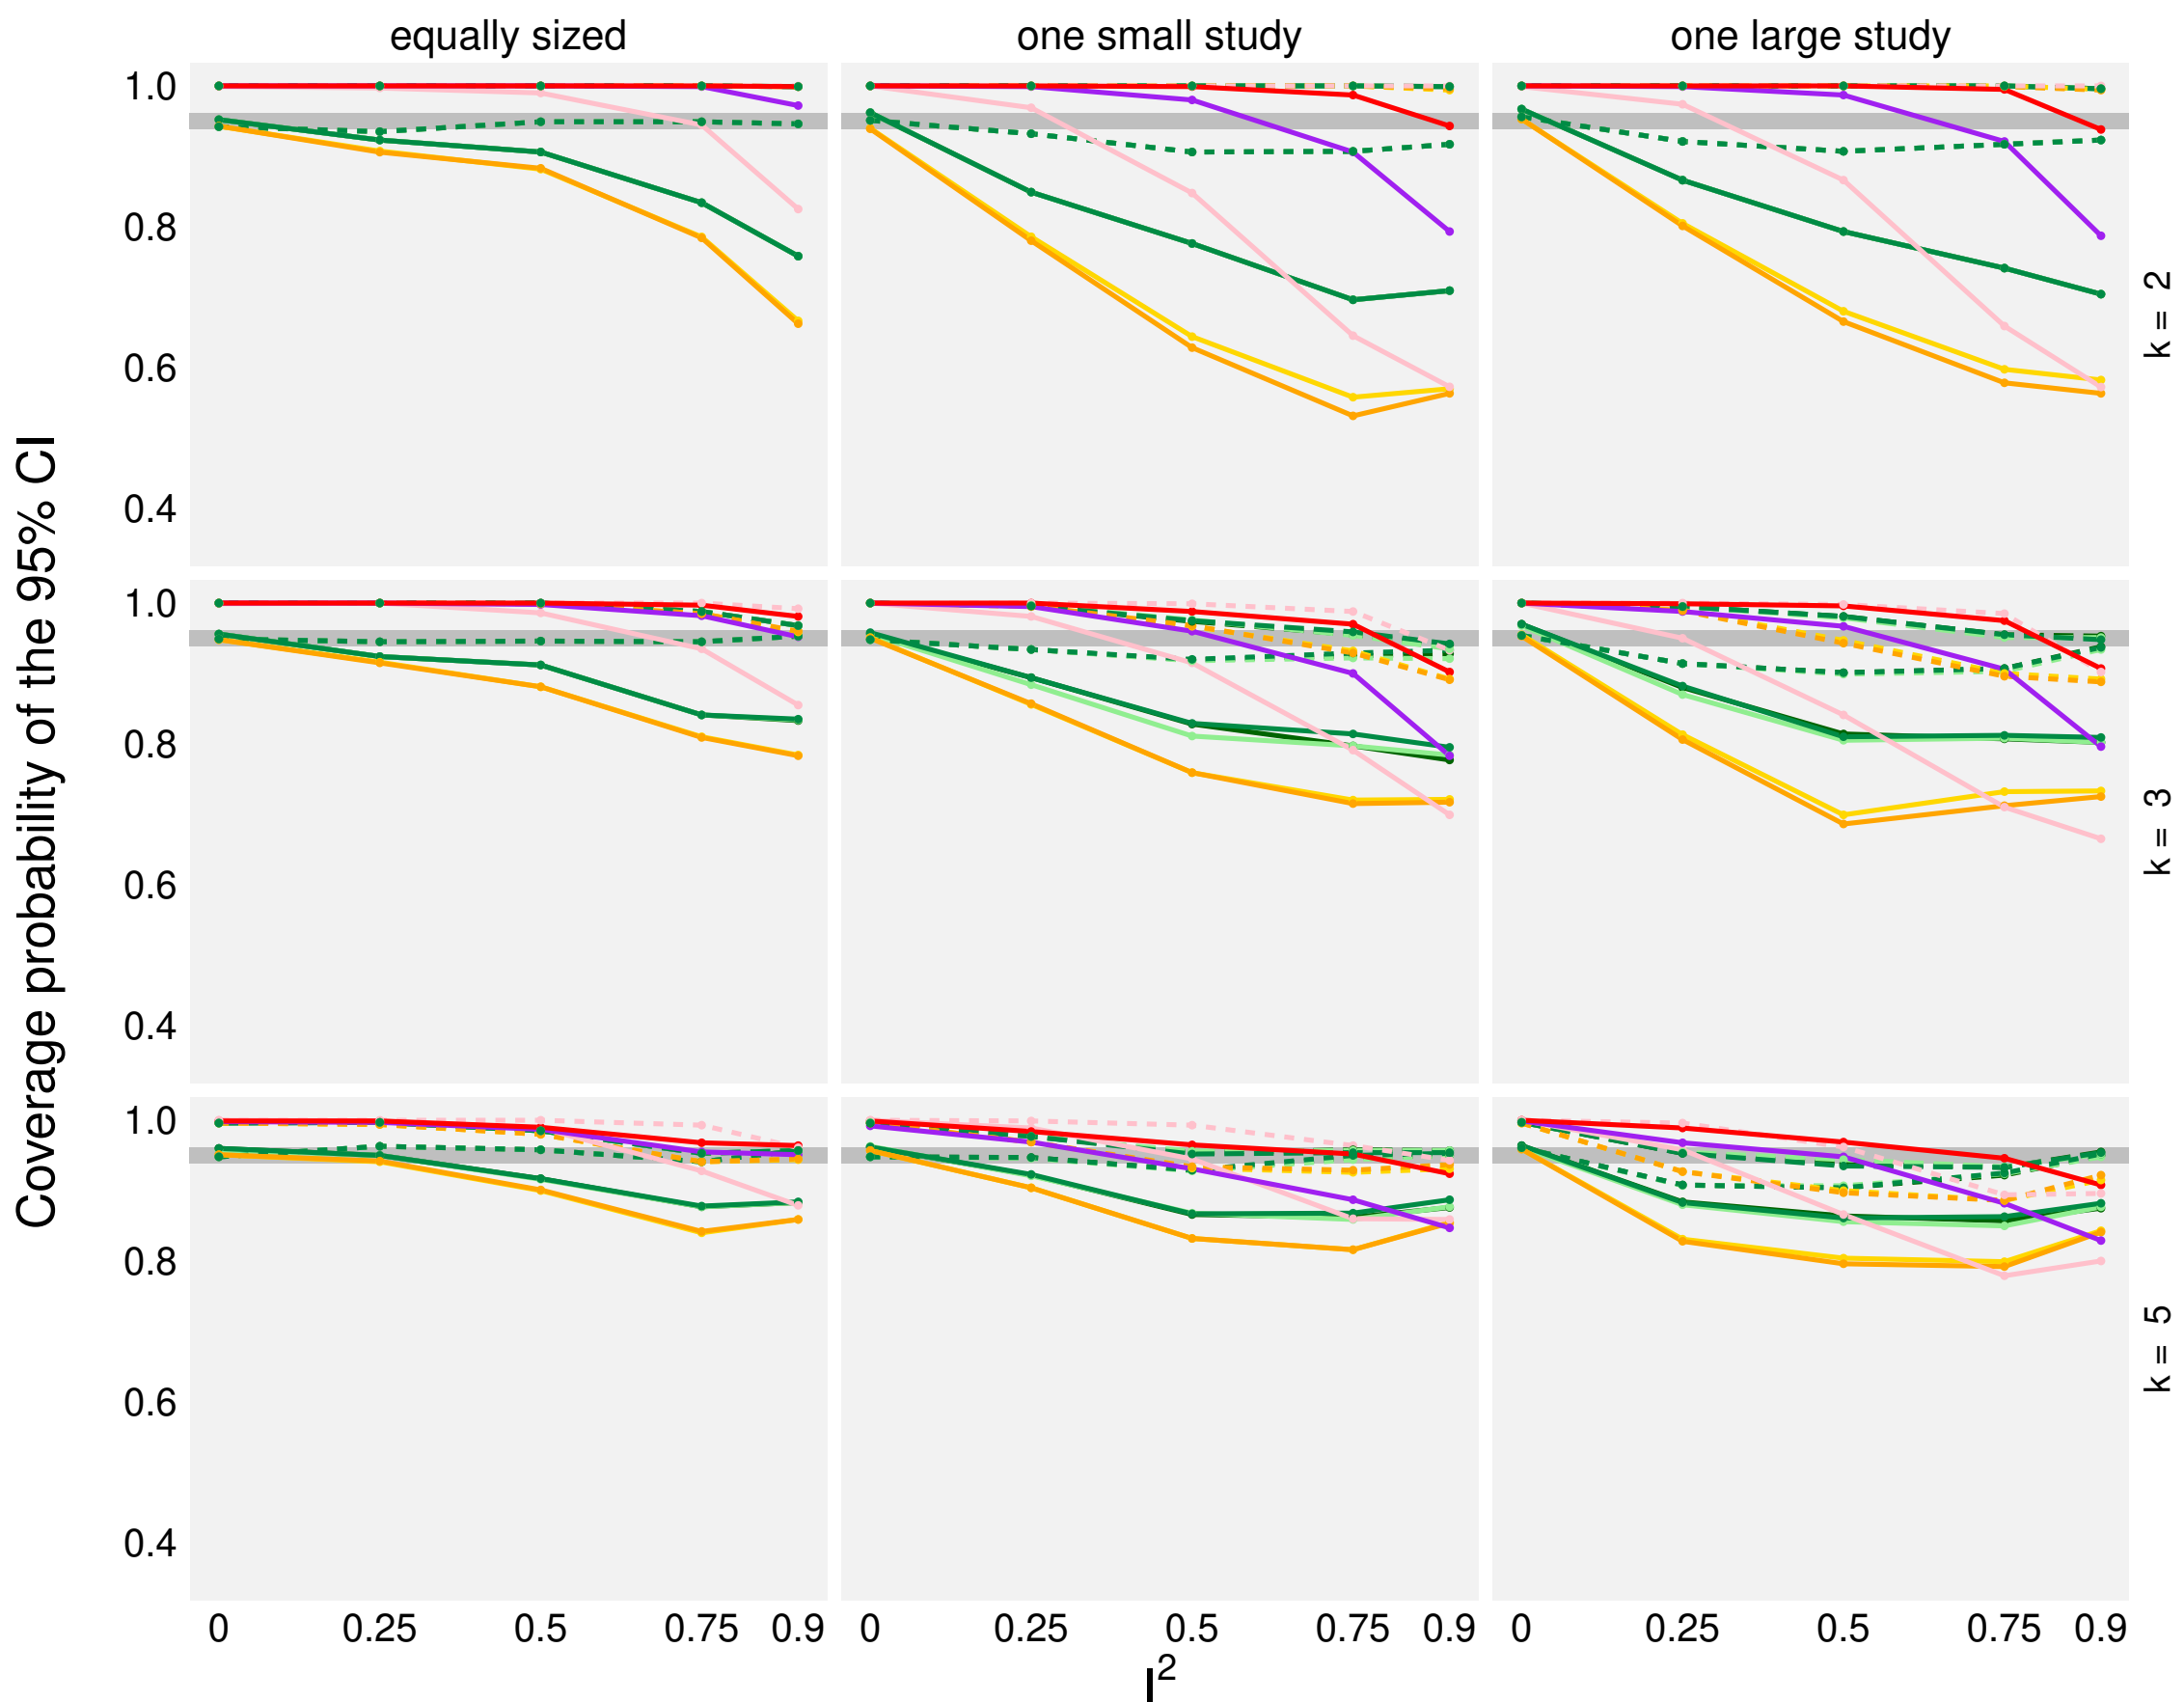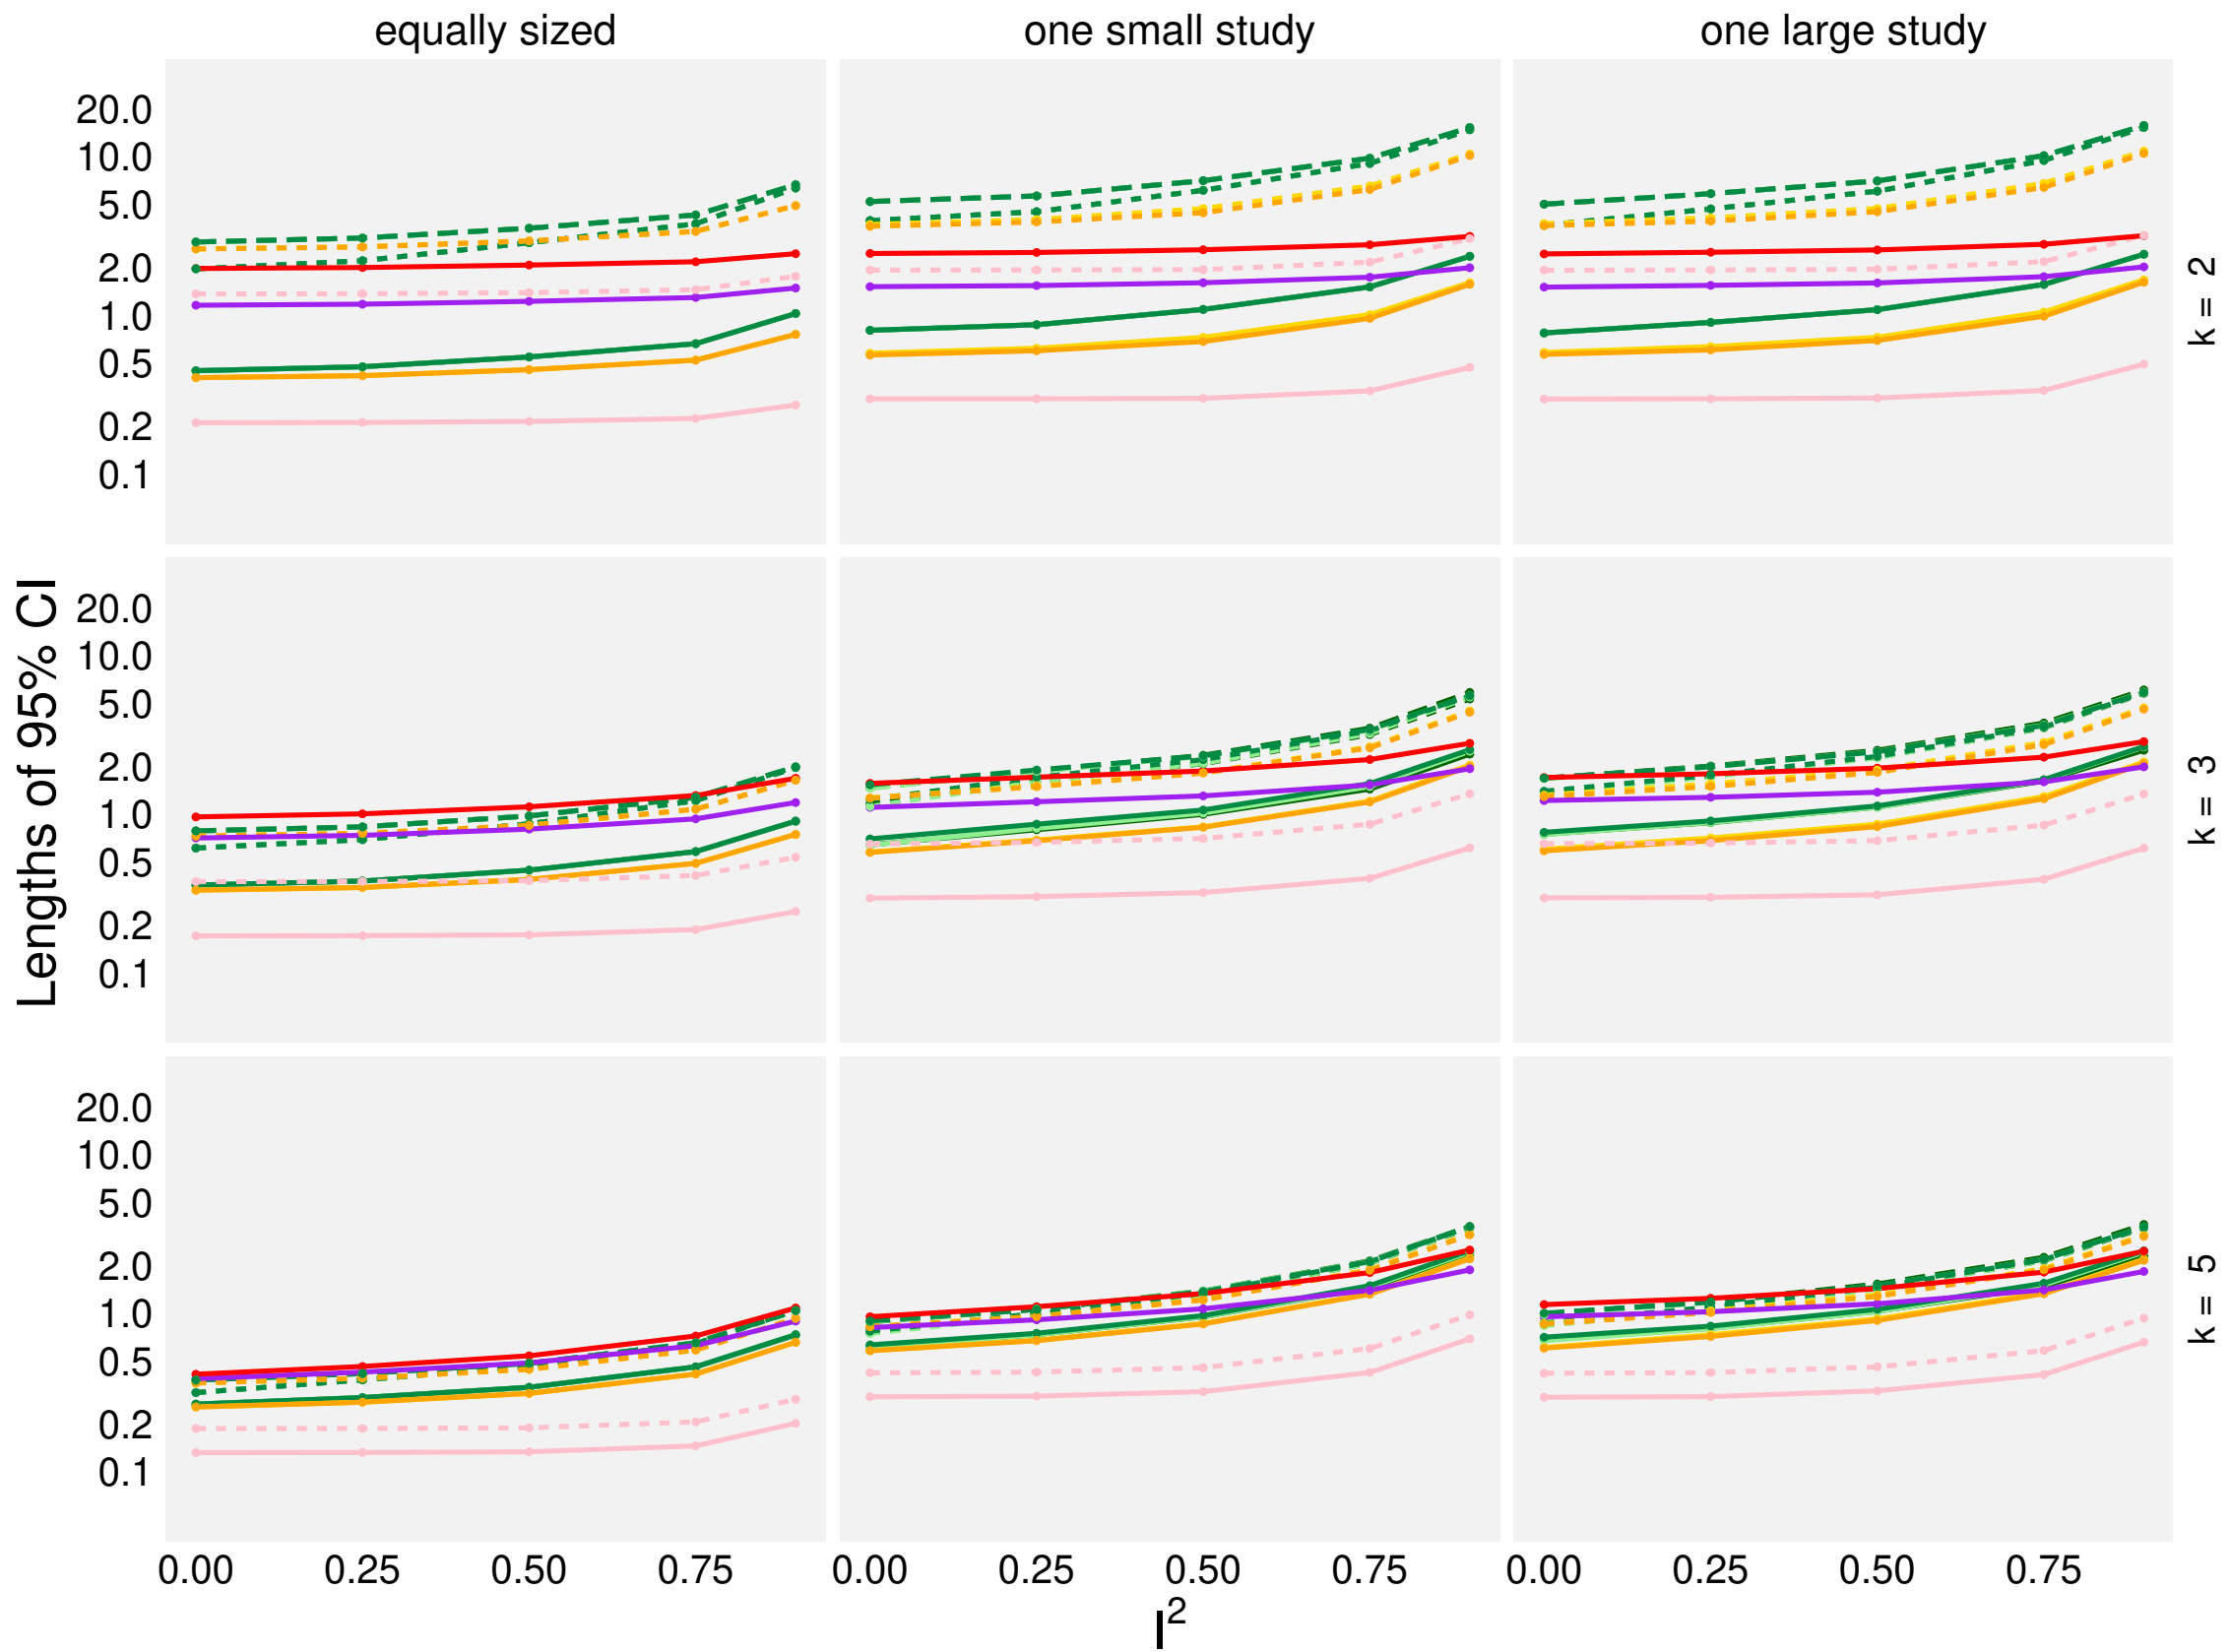

NN – DL  
 NN – REML  
 NN – EB  
 BN – UM.FS  
 BN – UM.RS  
 BN – CM.AL  
 NN – Bayes HN(0.5)  
 NN – Bayes HN(1)  
 — normal quantiles  
 - - HKSJ or Student's t  
 - · mHKSJ

OR  
( $n_i=500, \pi_0=0.9$ )

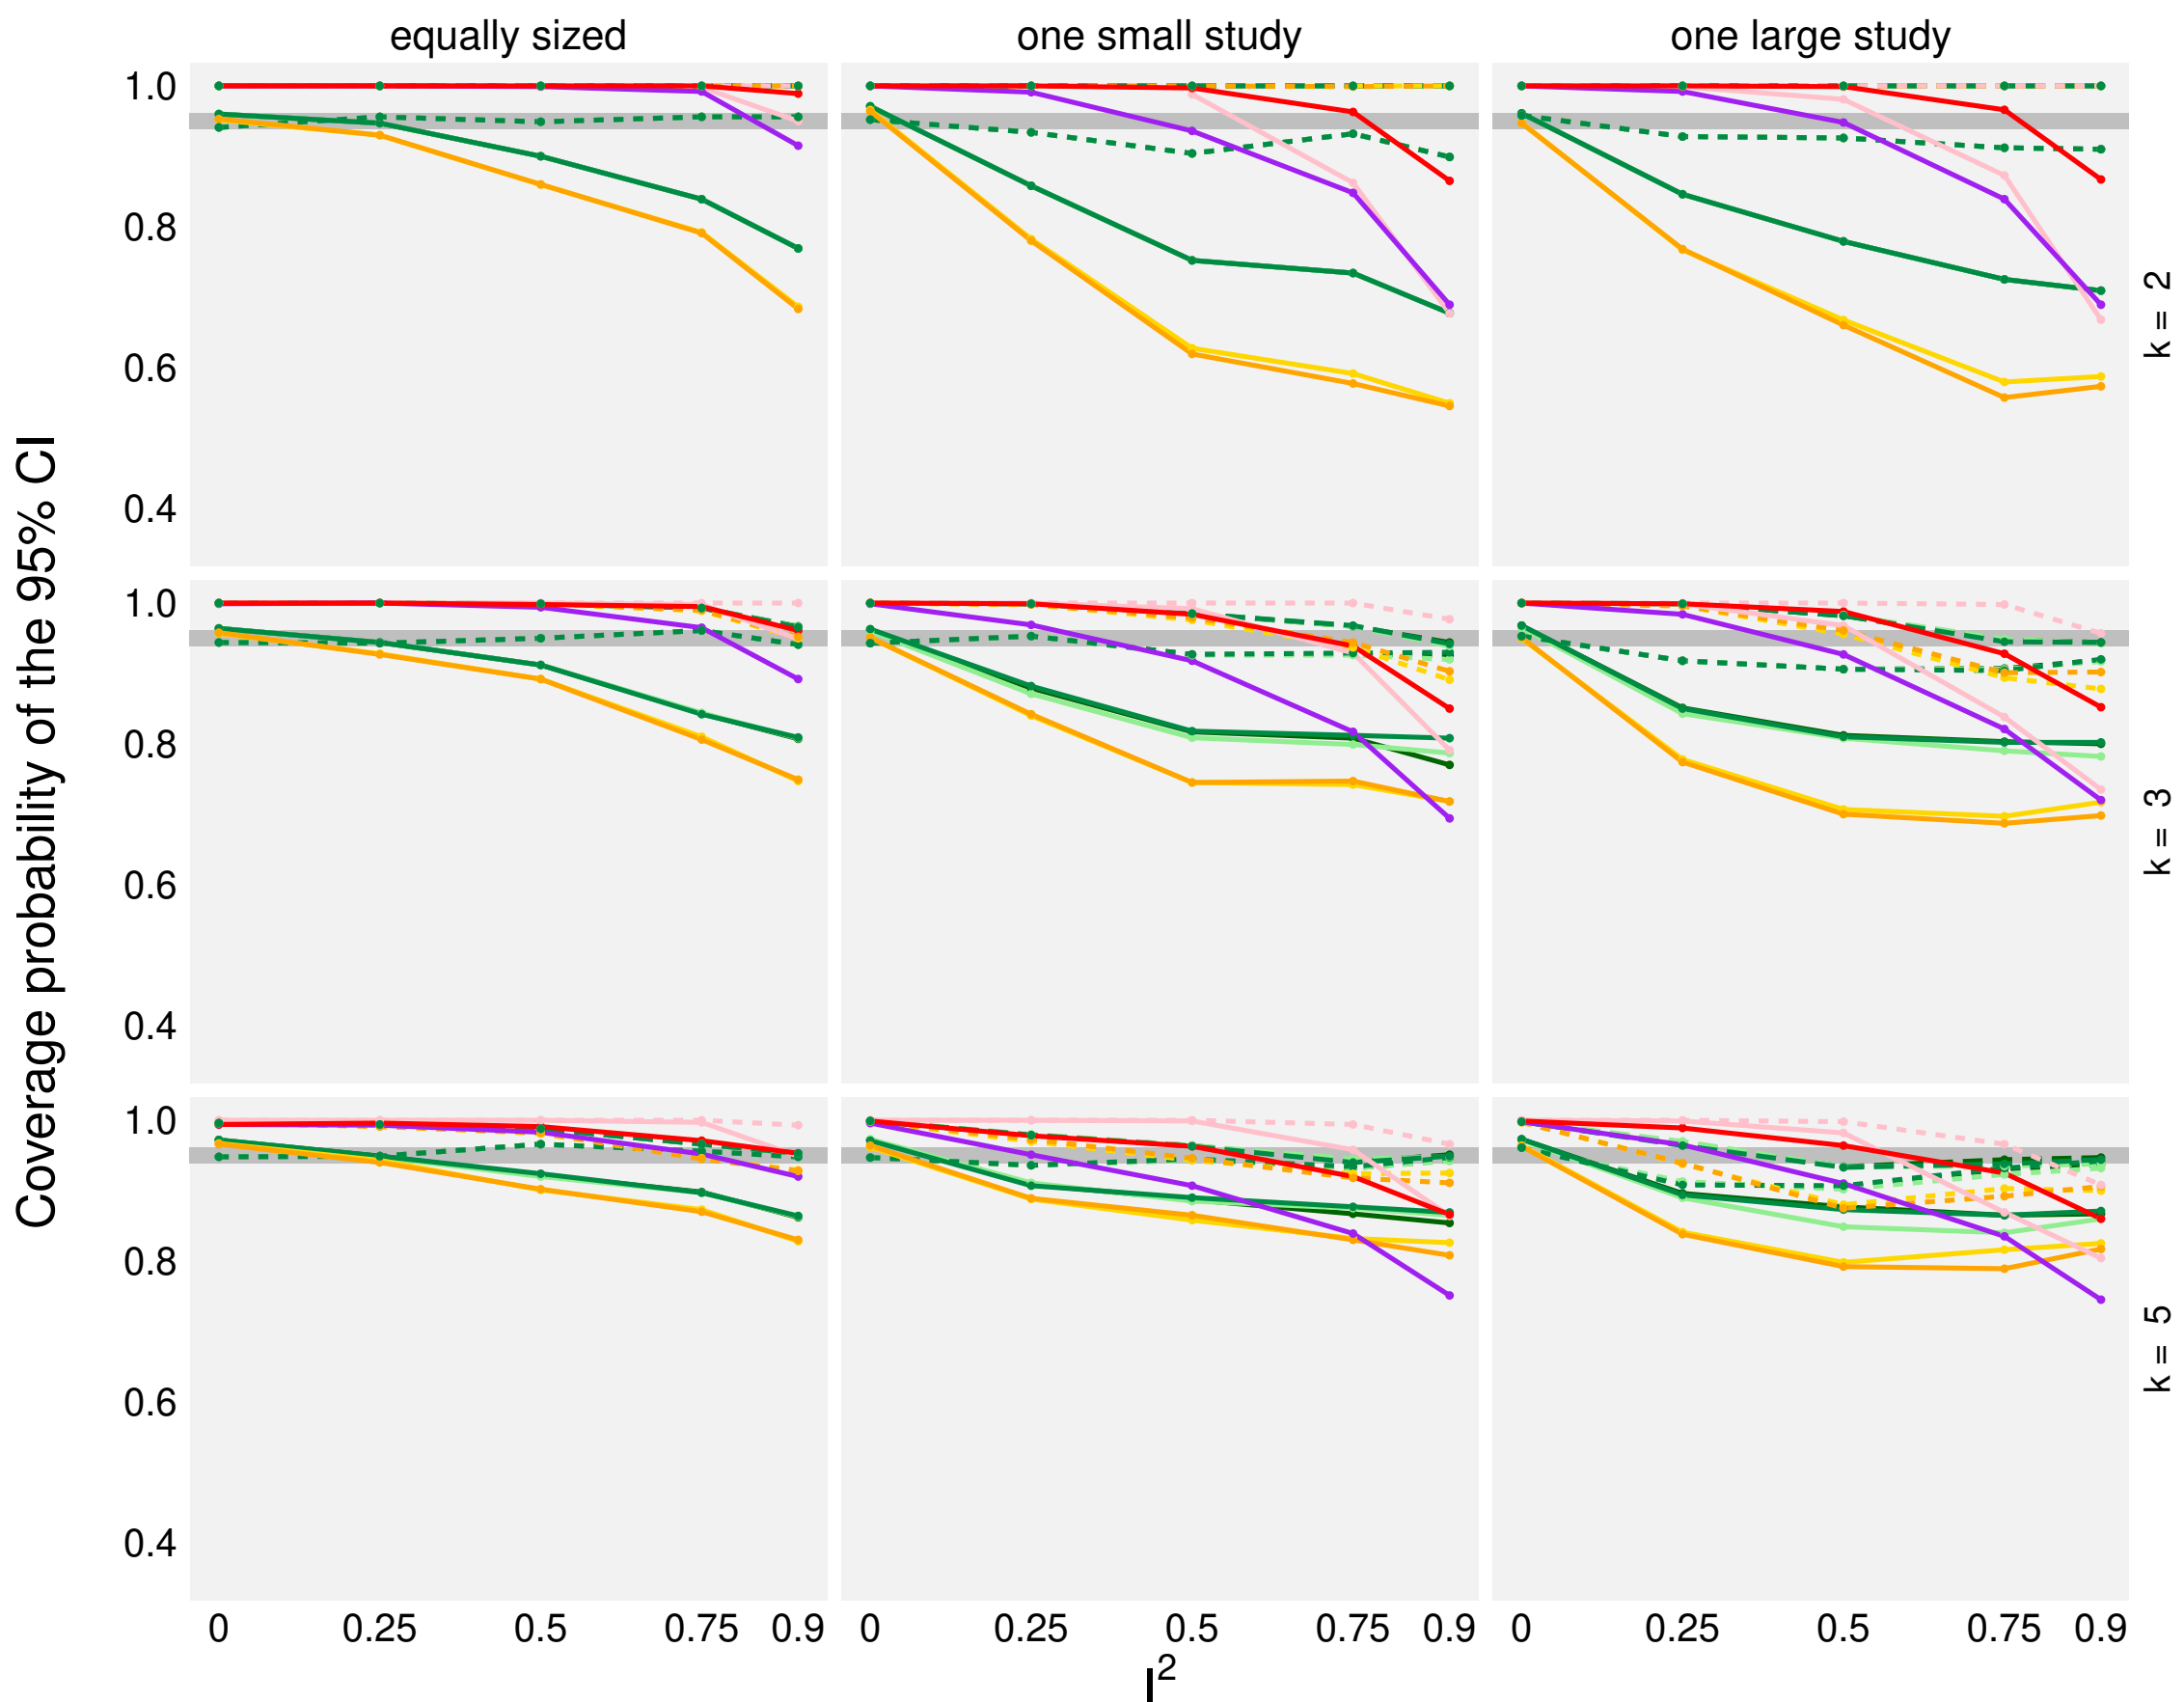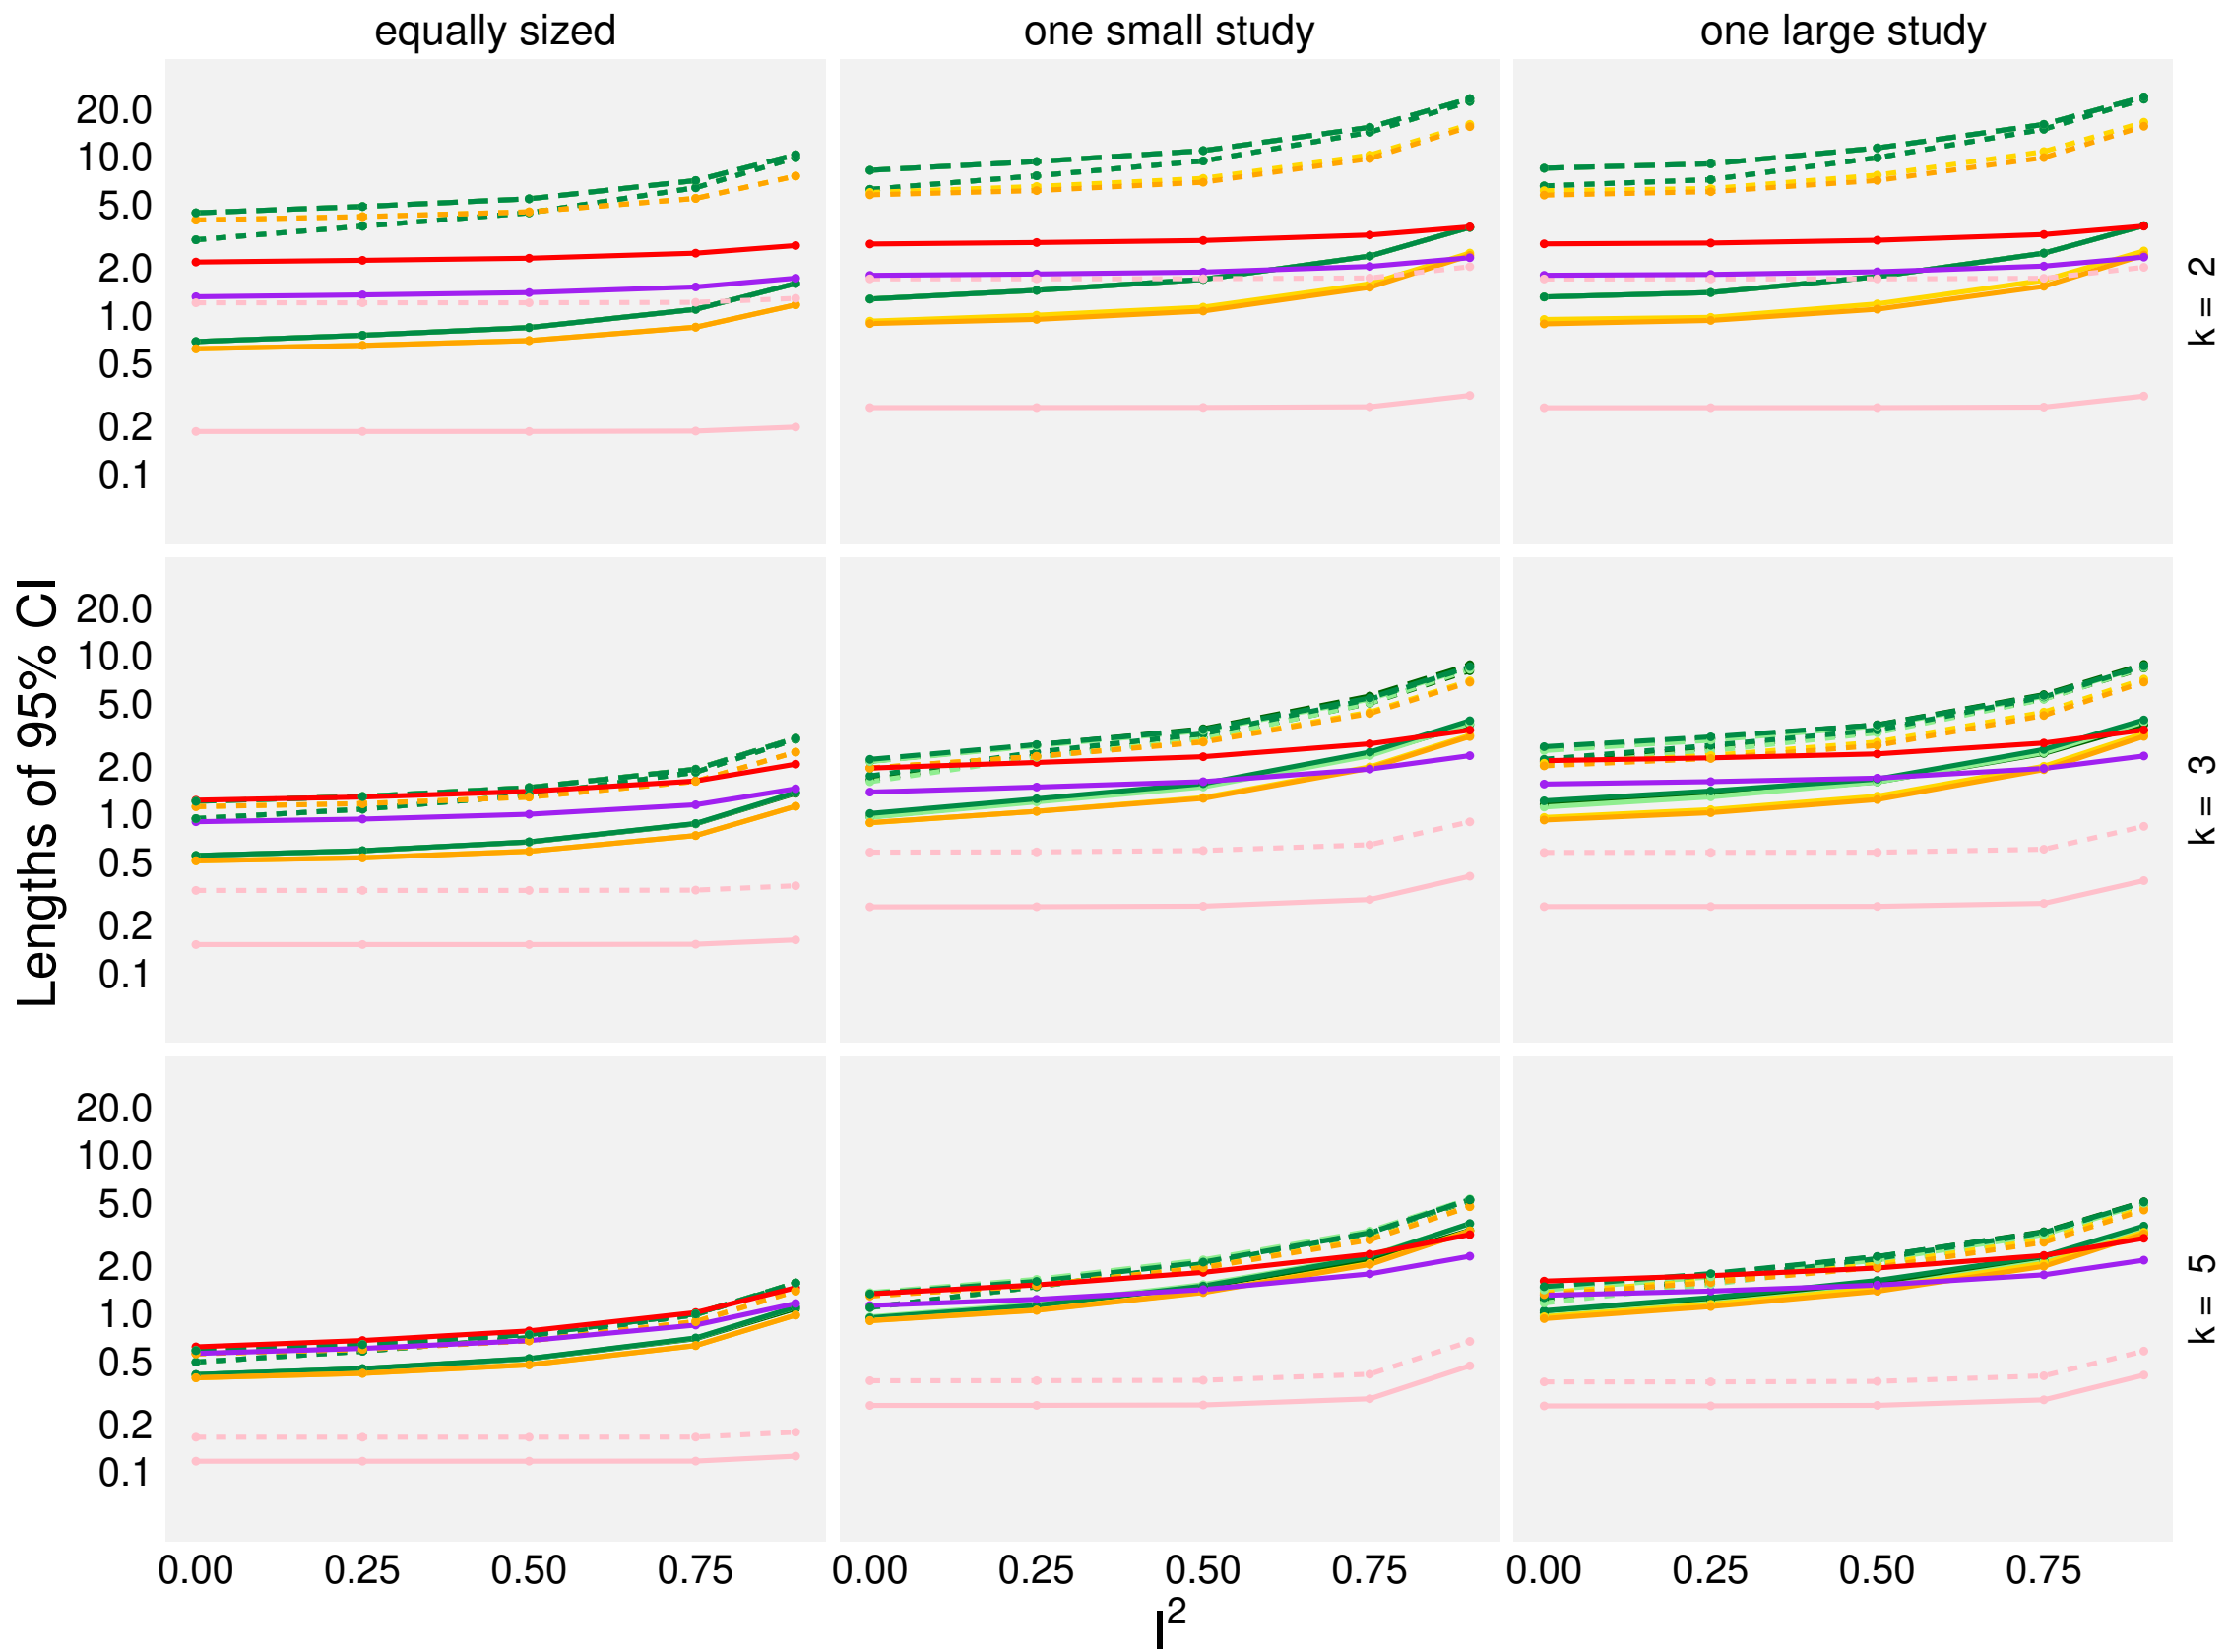

— NN — DL  
 — NN — REML  
 — NN — EB  
 — BN — UM.FS  
 — BN — UM.RS  
 — BN — CM.AL  
 — NN — Bayes HN(0.5)  
 — NN — Bayes HN(1)

— normal quantiles  
 - - HKSJ or Student's t  
 - - mHKSJ

OR  
( $n_i=1000, \pi_0=0.1$ )

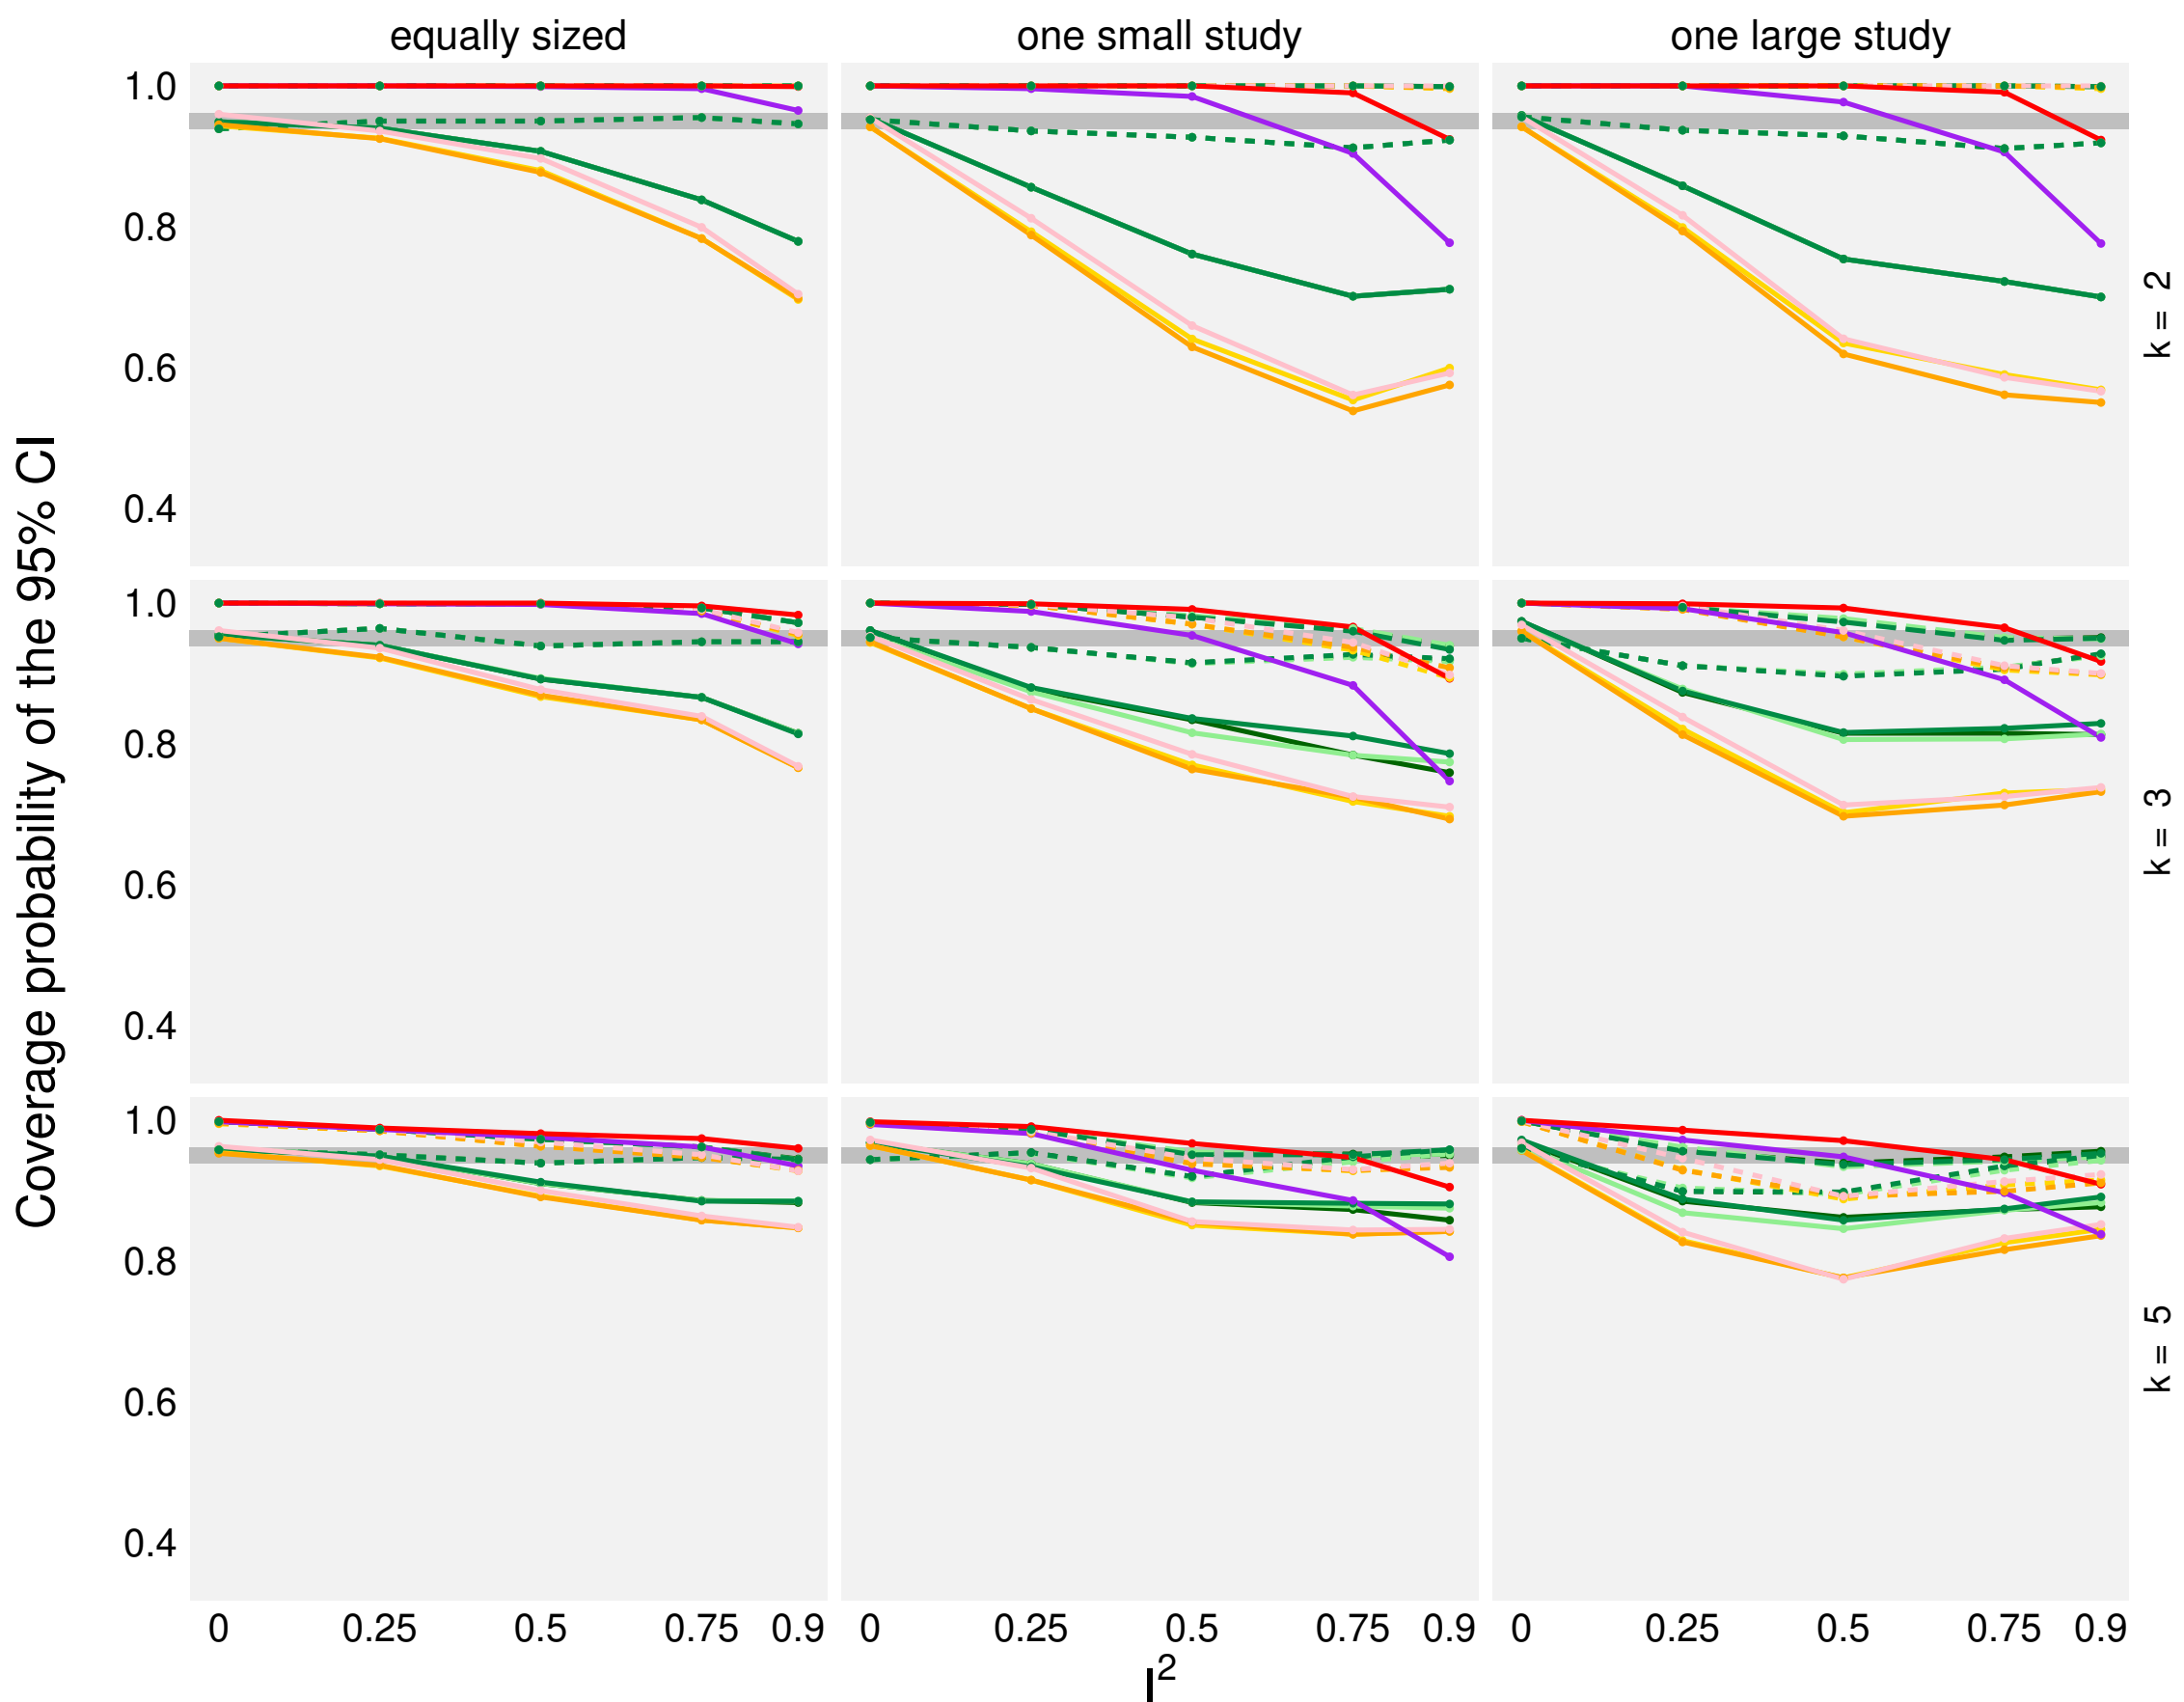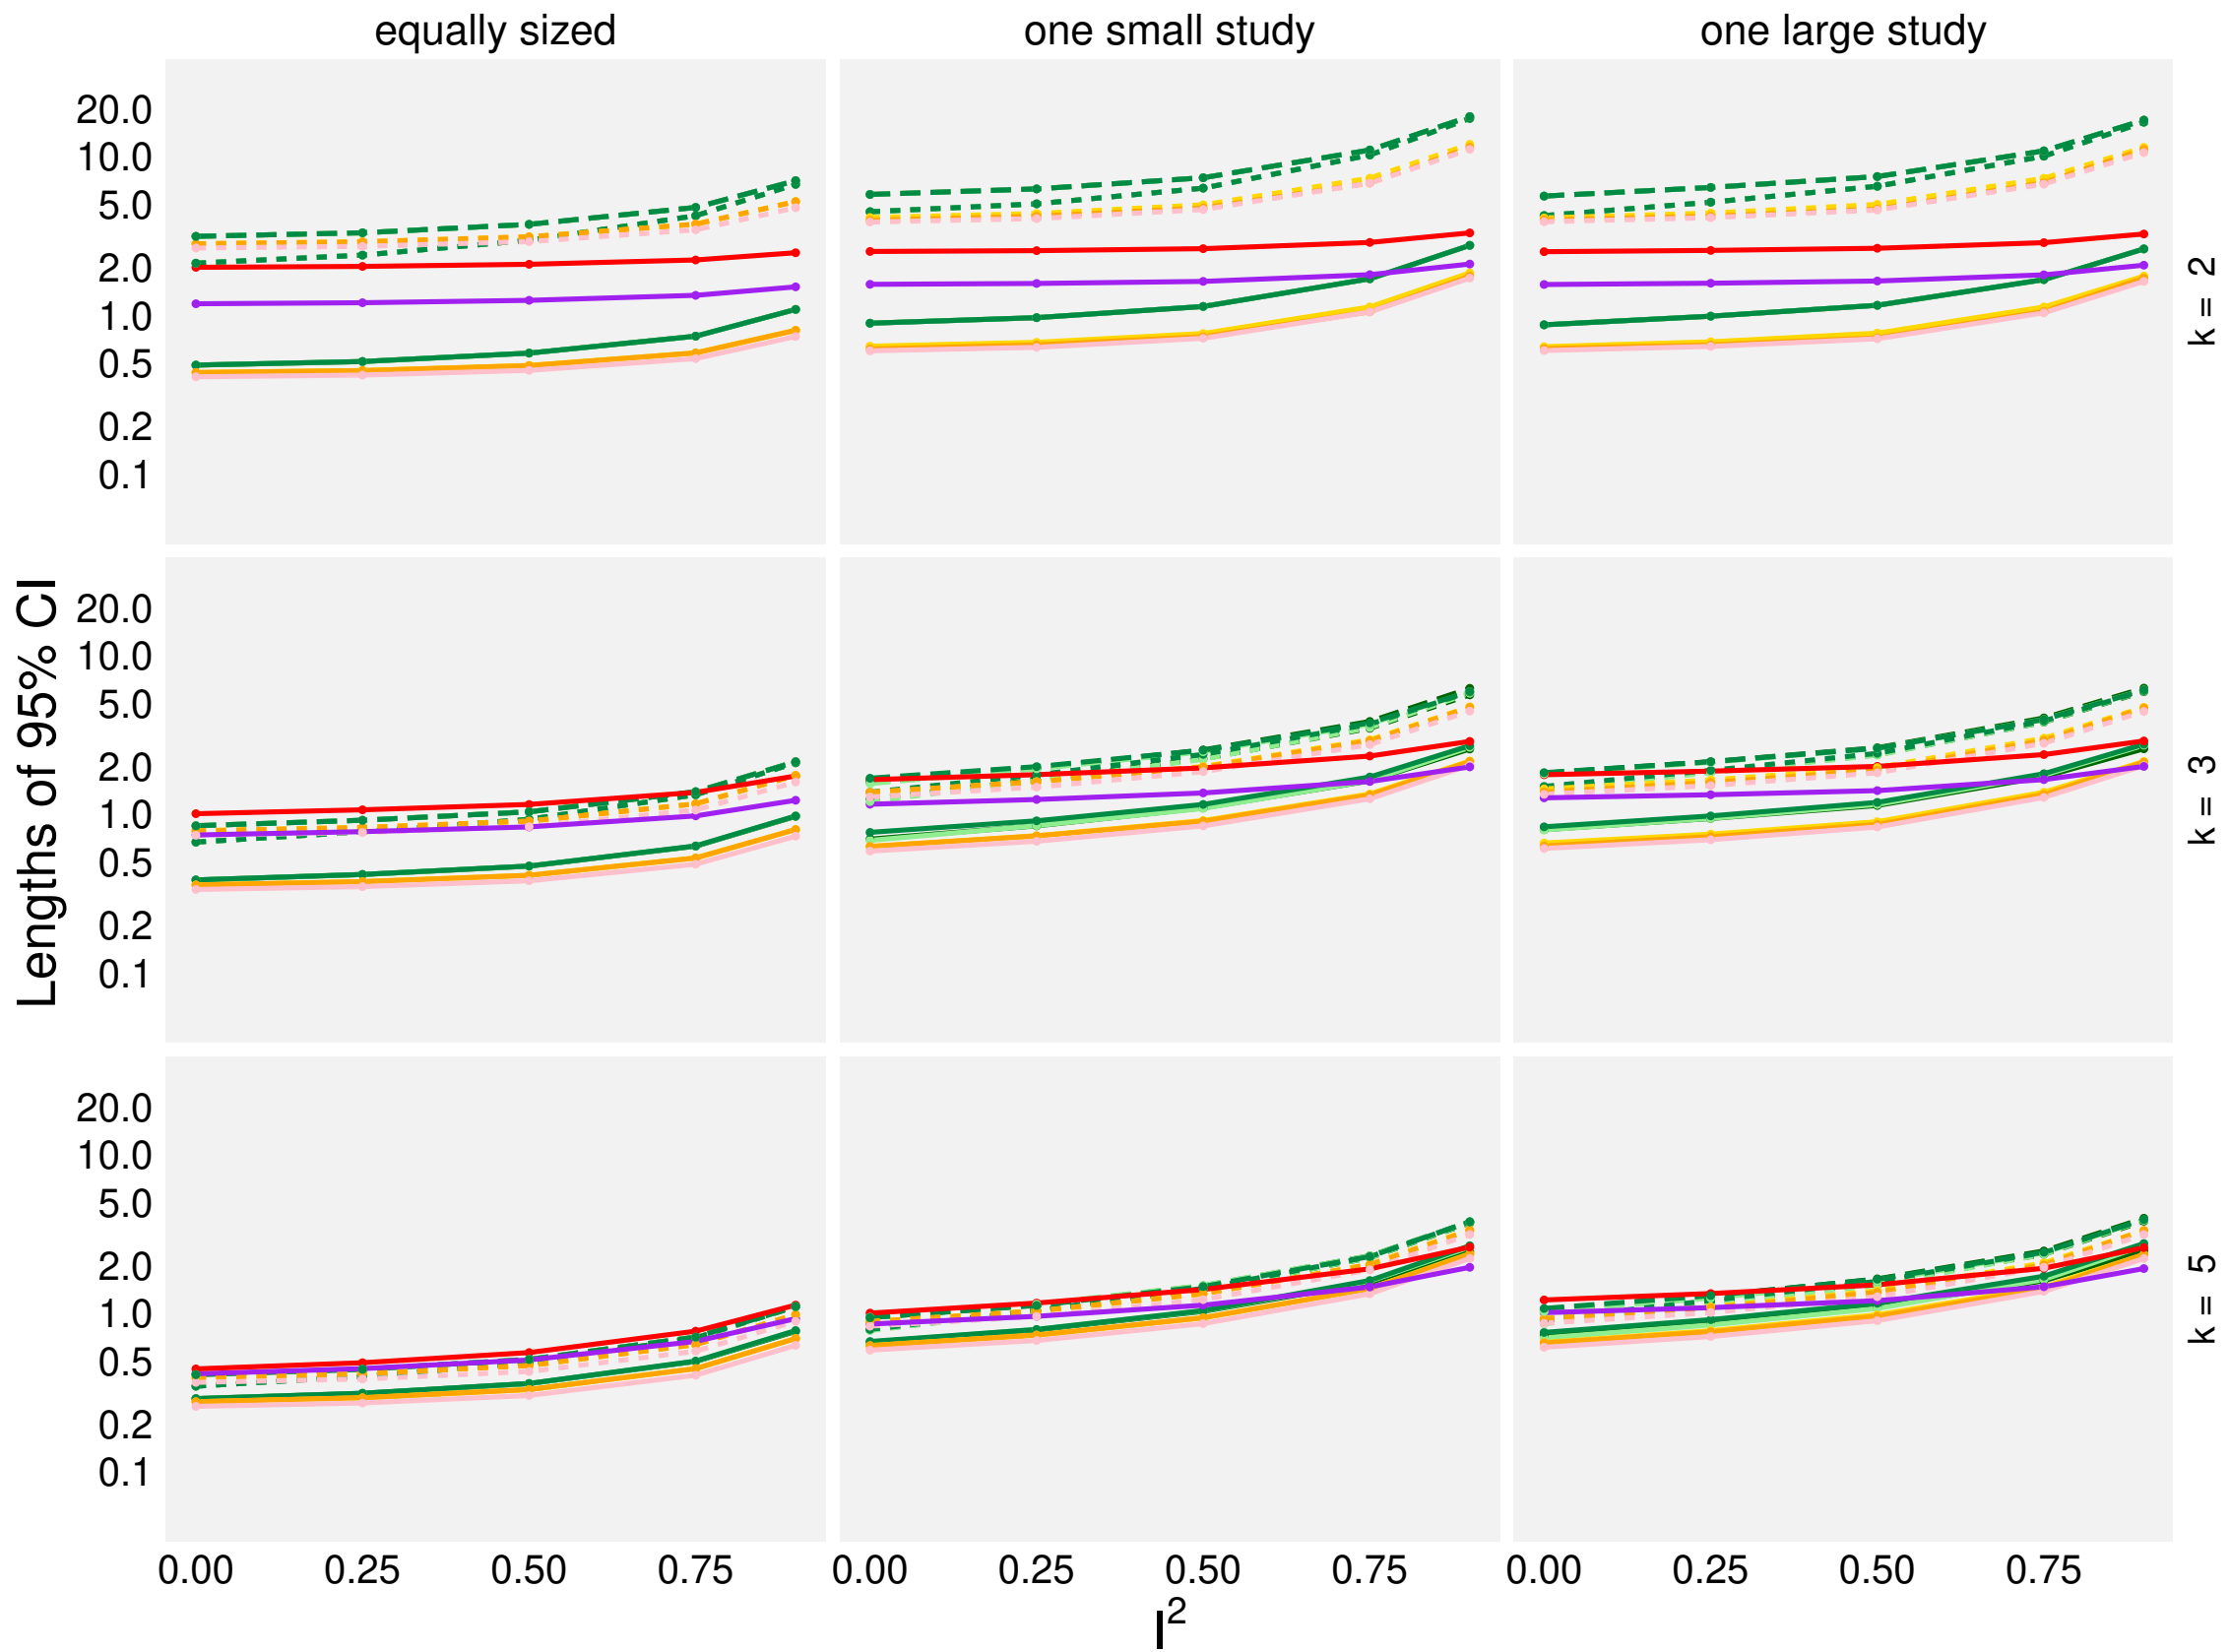

— NN — DL      — BN — UM.RS      — normal quantiles  
 — NN — REML      — BN — CM.AL      -- HKSJ or Student's t  
 — NN — EB      — NN — Bayes HN(0.5)      -·- mHKSJ  
 — BN — UM.FS      — NN — Bayes HN(1)

OR  
( $n_i=1000, \pi_0=0.3$ )

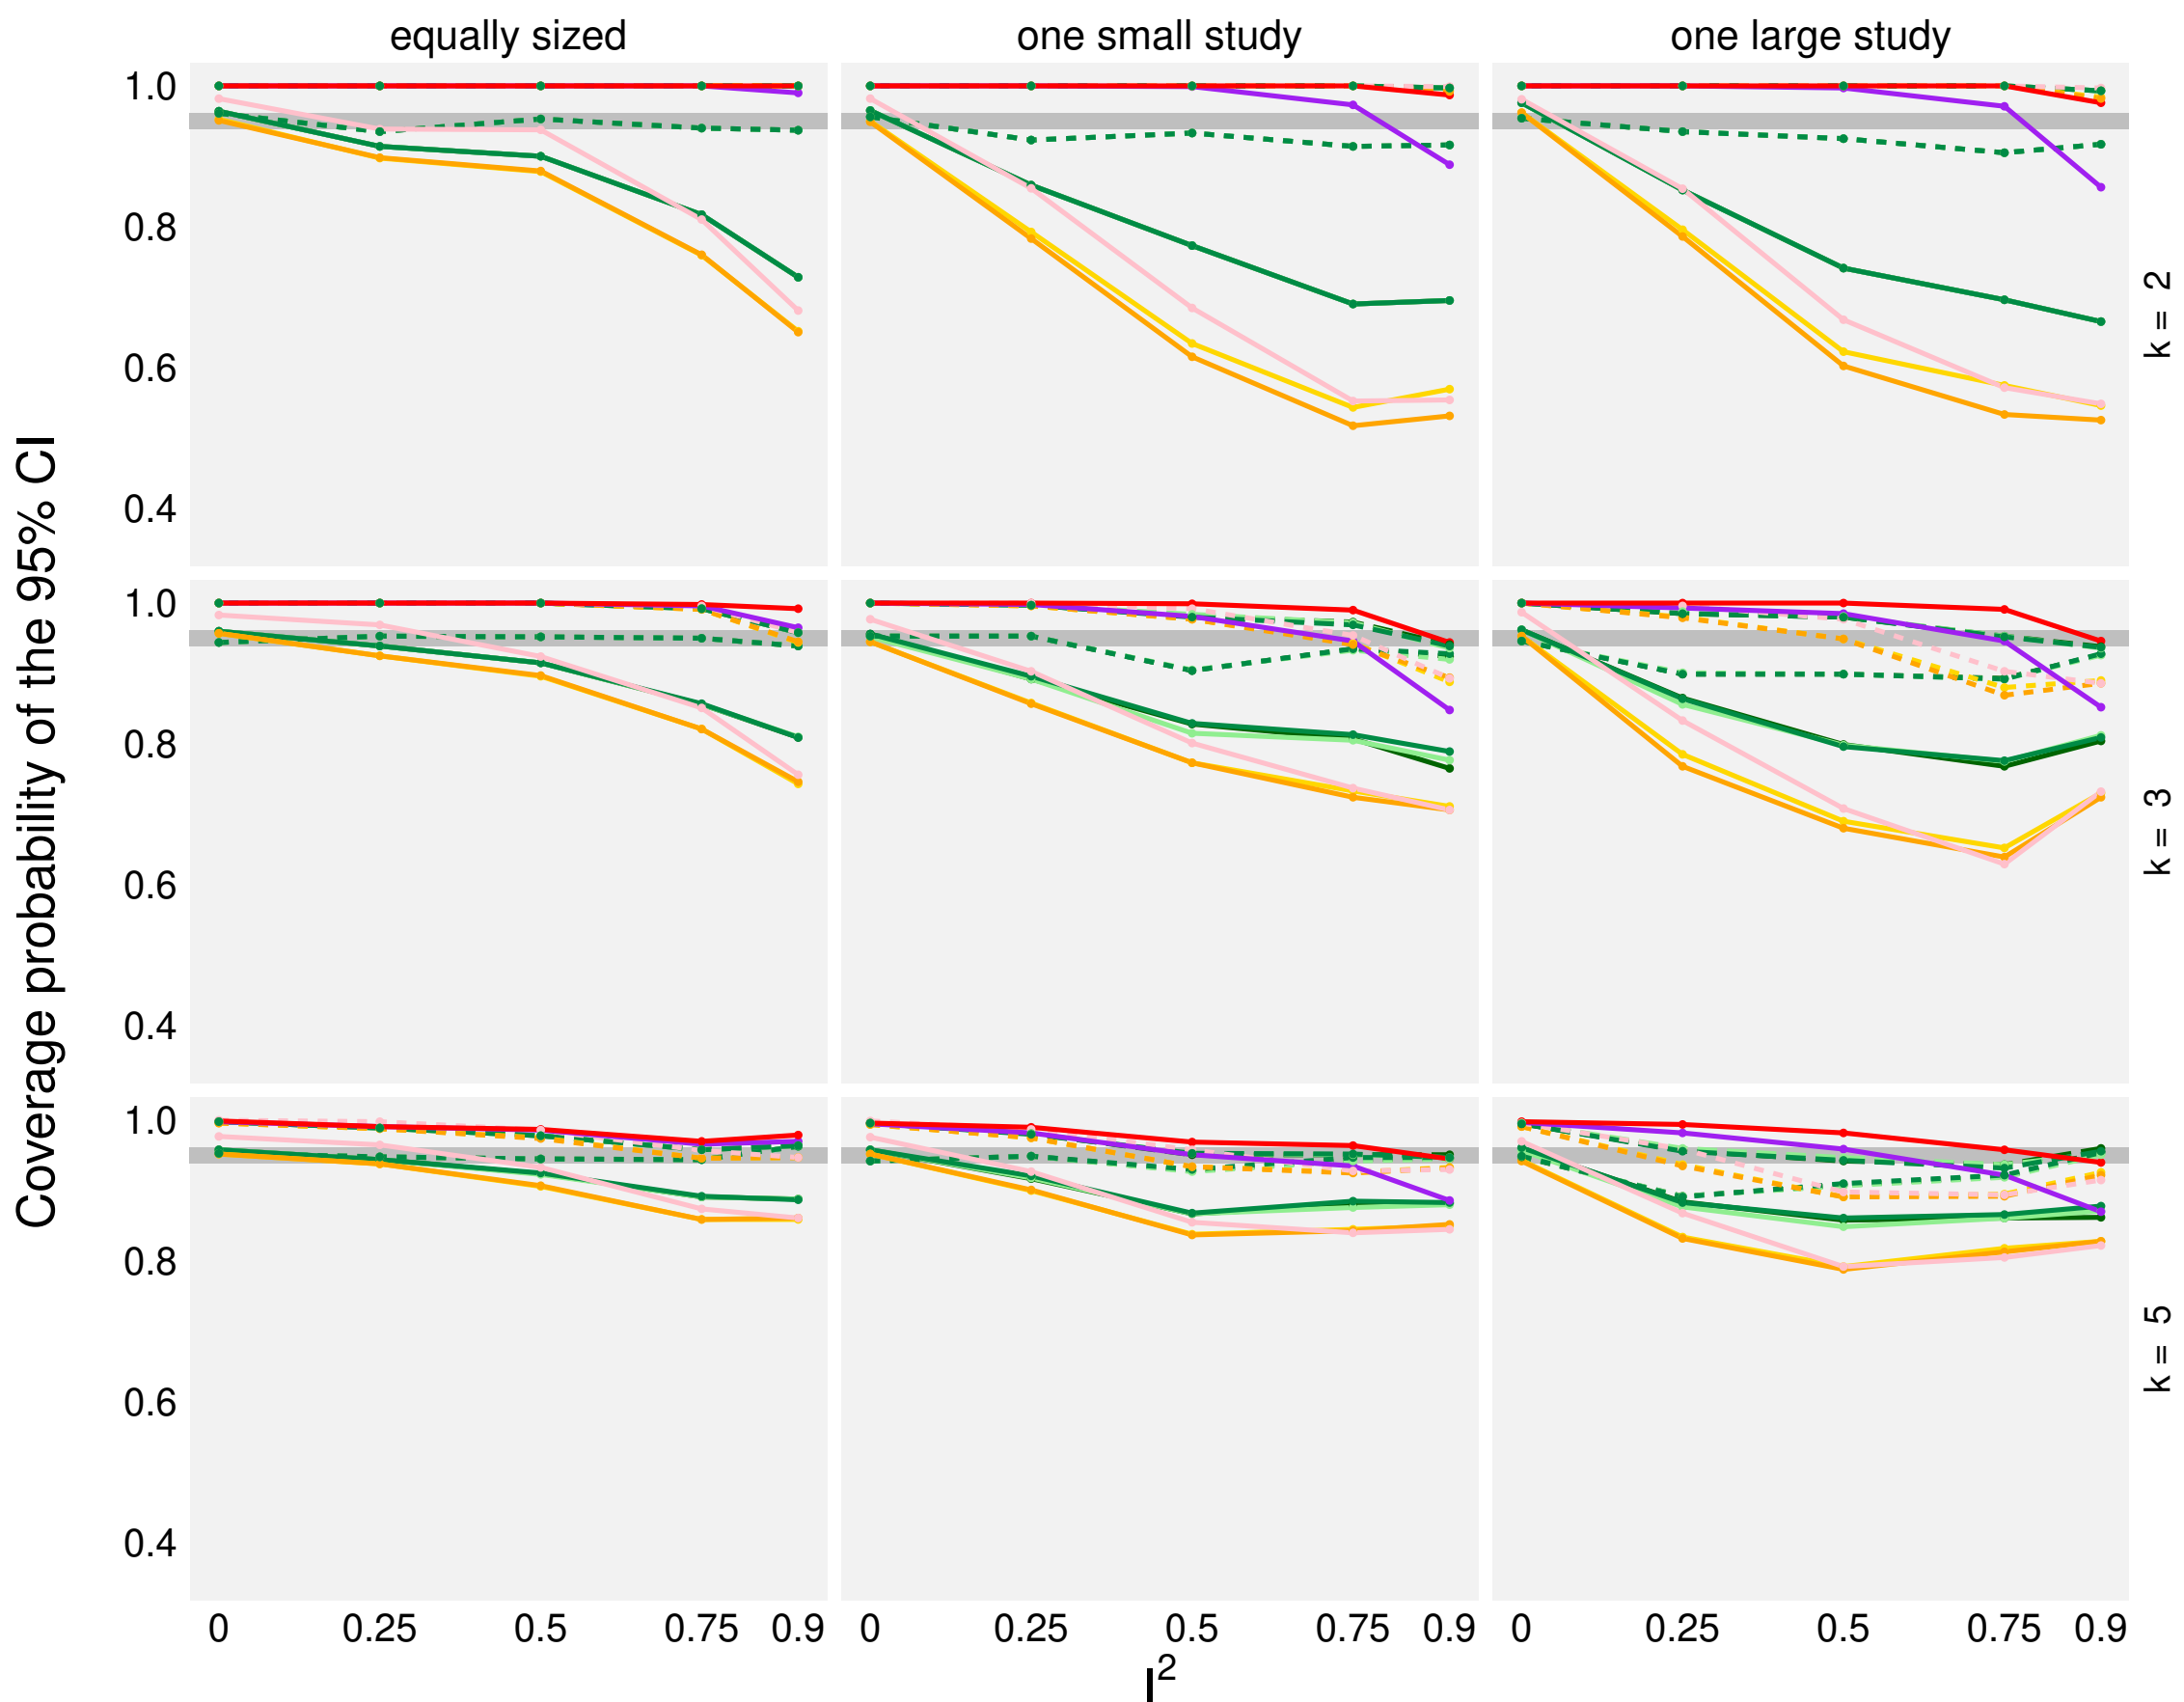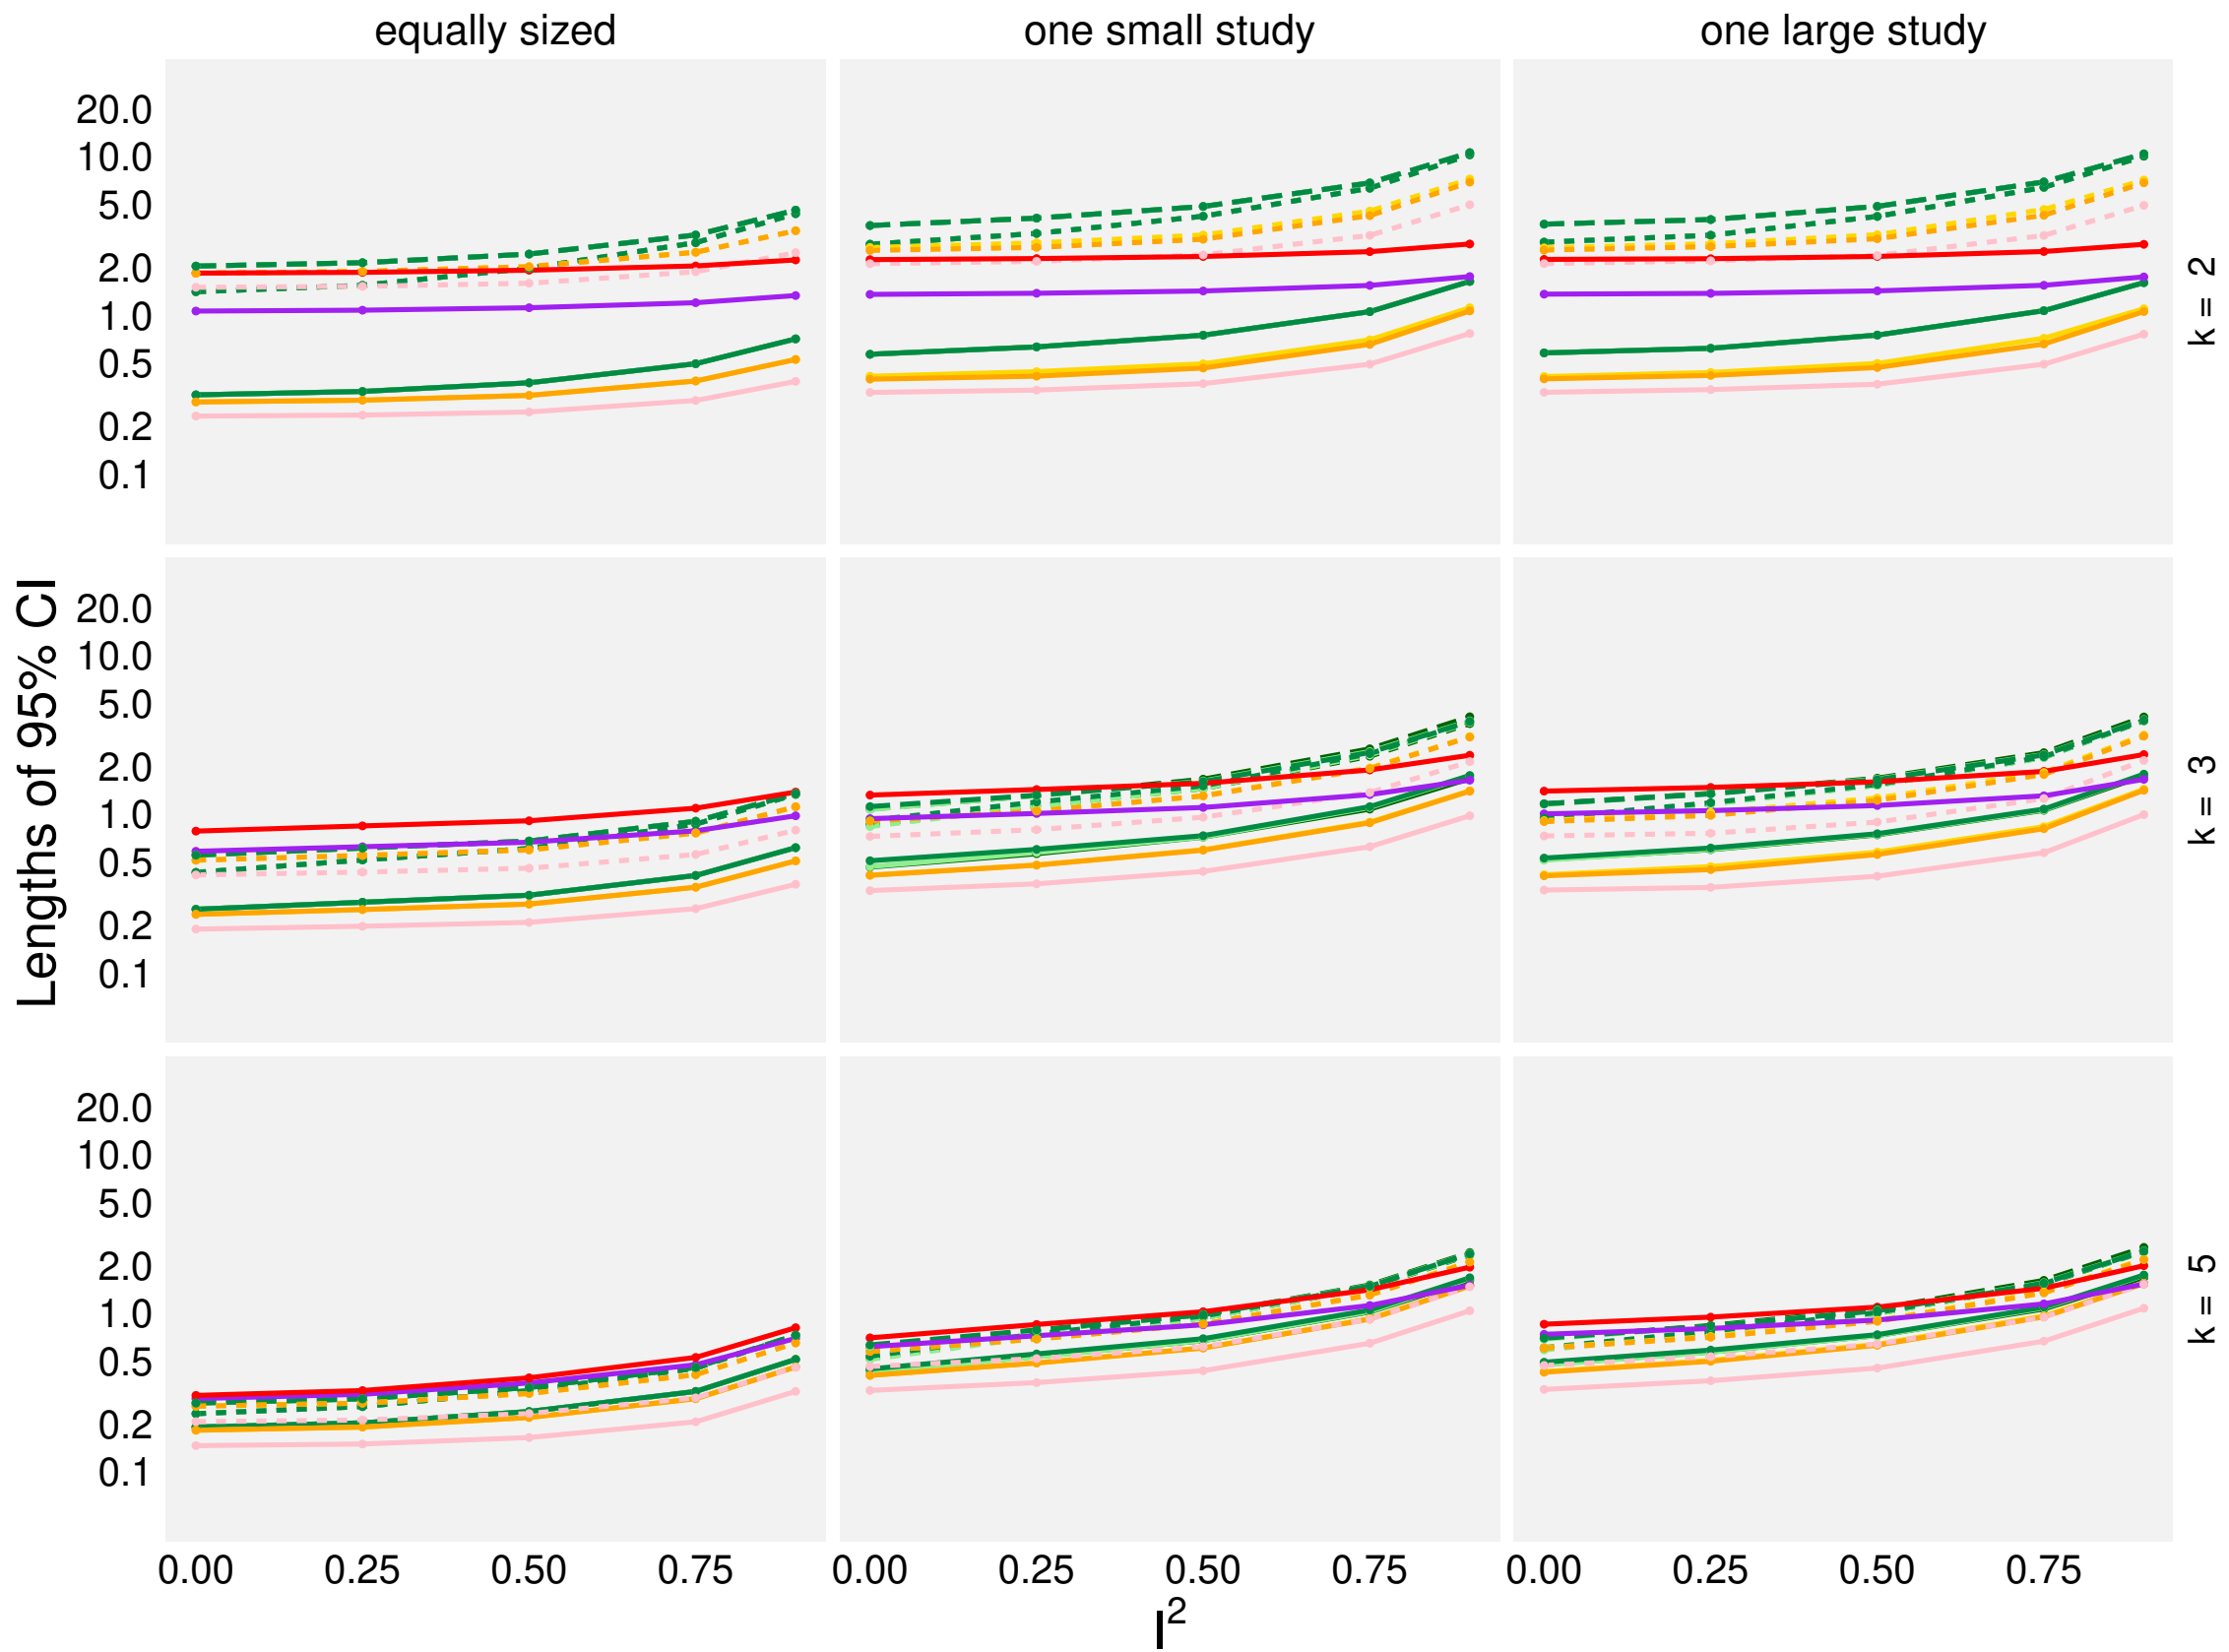

— NN — DL  
 — NN — REML  
 — NN — EB  
 — BN — UM.FS  
 — BN — UM.RS  
 — BN — CM.AL  
 — NN — Bayes HN(0.5)  
 — NN — Bayes HN(1)

— normal quantiles  
 - - HKSJ or Student's t  
 - · mHKSJ

OR  
( $n_i=1000, \pi_0=0.5$ )

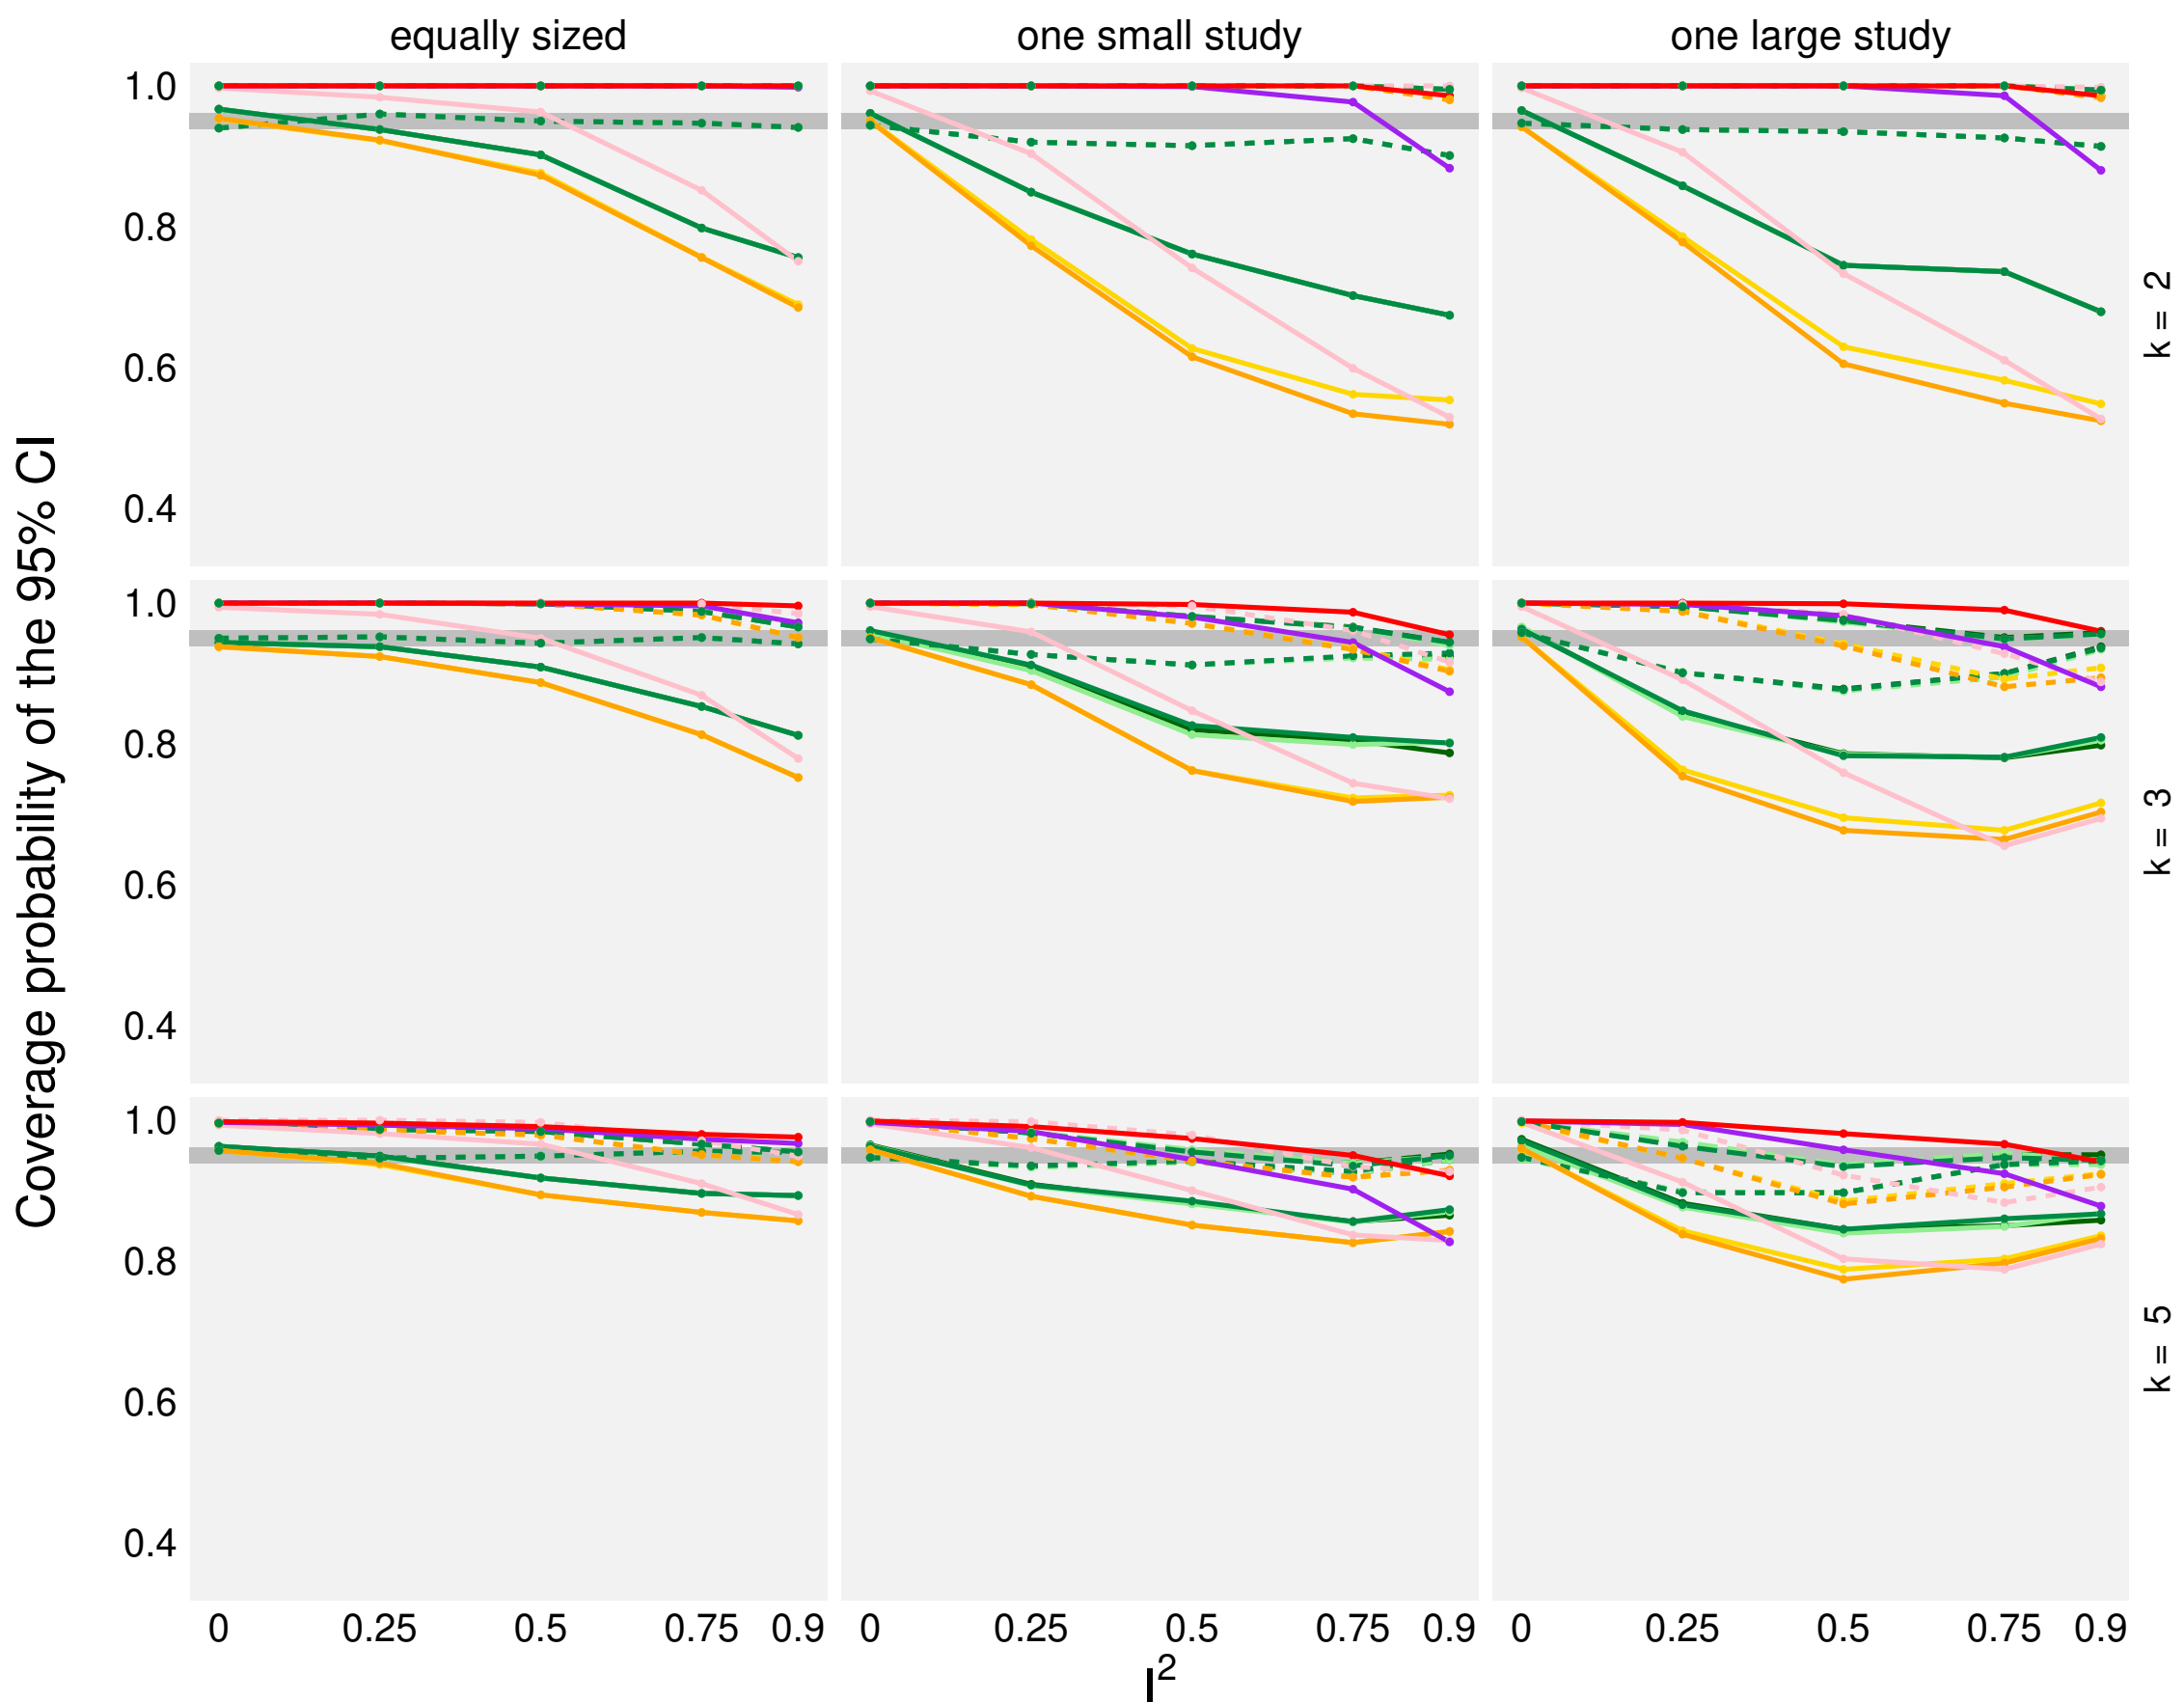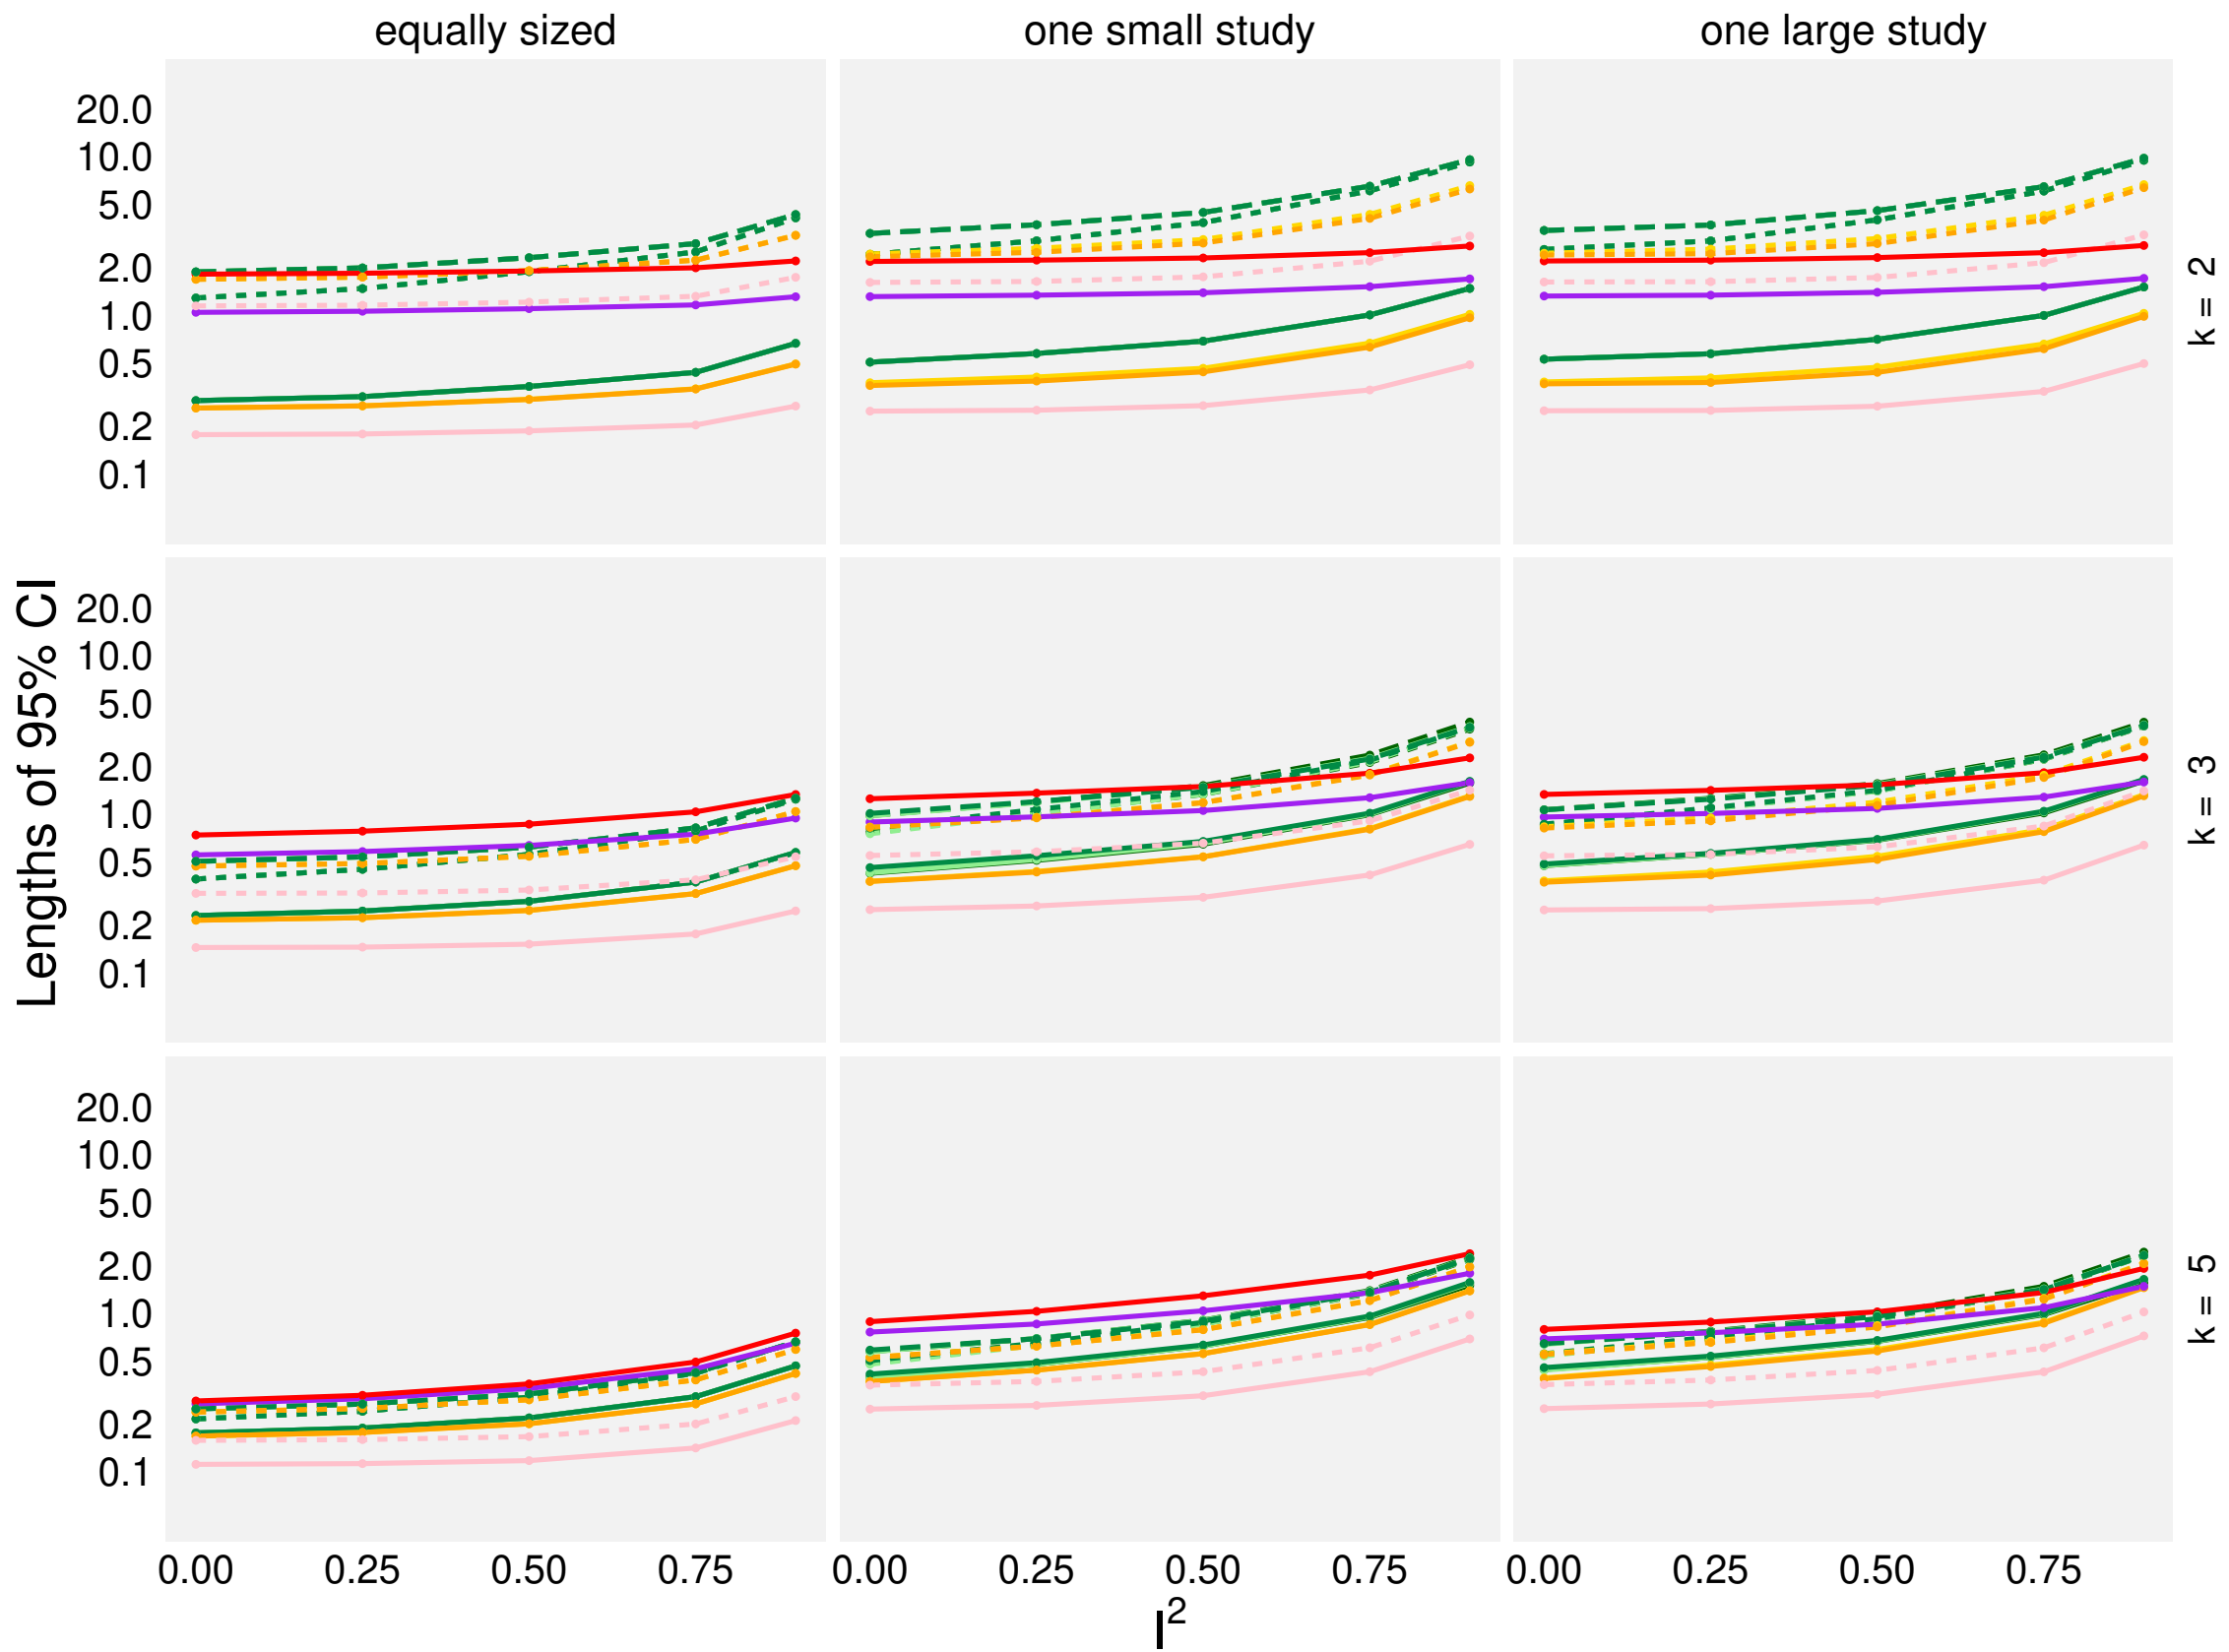

— NN — DL      — BN — UM.RS      — normal quantiles  
 — NN — REML      — BN — CM.AL      -- HKSJ or Student's t  
 — NN — EB      — NN — Bayes HN(0.5)      -- mHKSJ  
 — BN — UM.FS      — NN — Bayes HN(1)

OR  
( $n_i=1000, \pi_0=0.7$ )

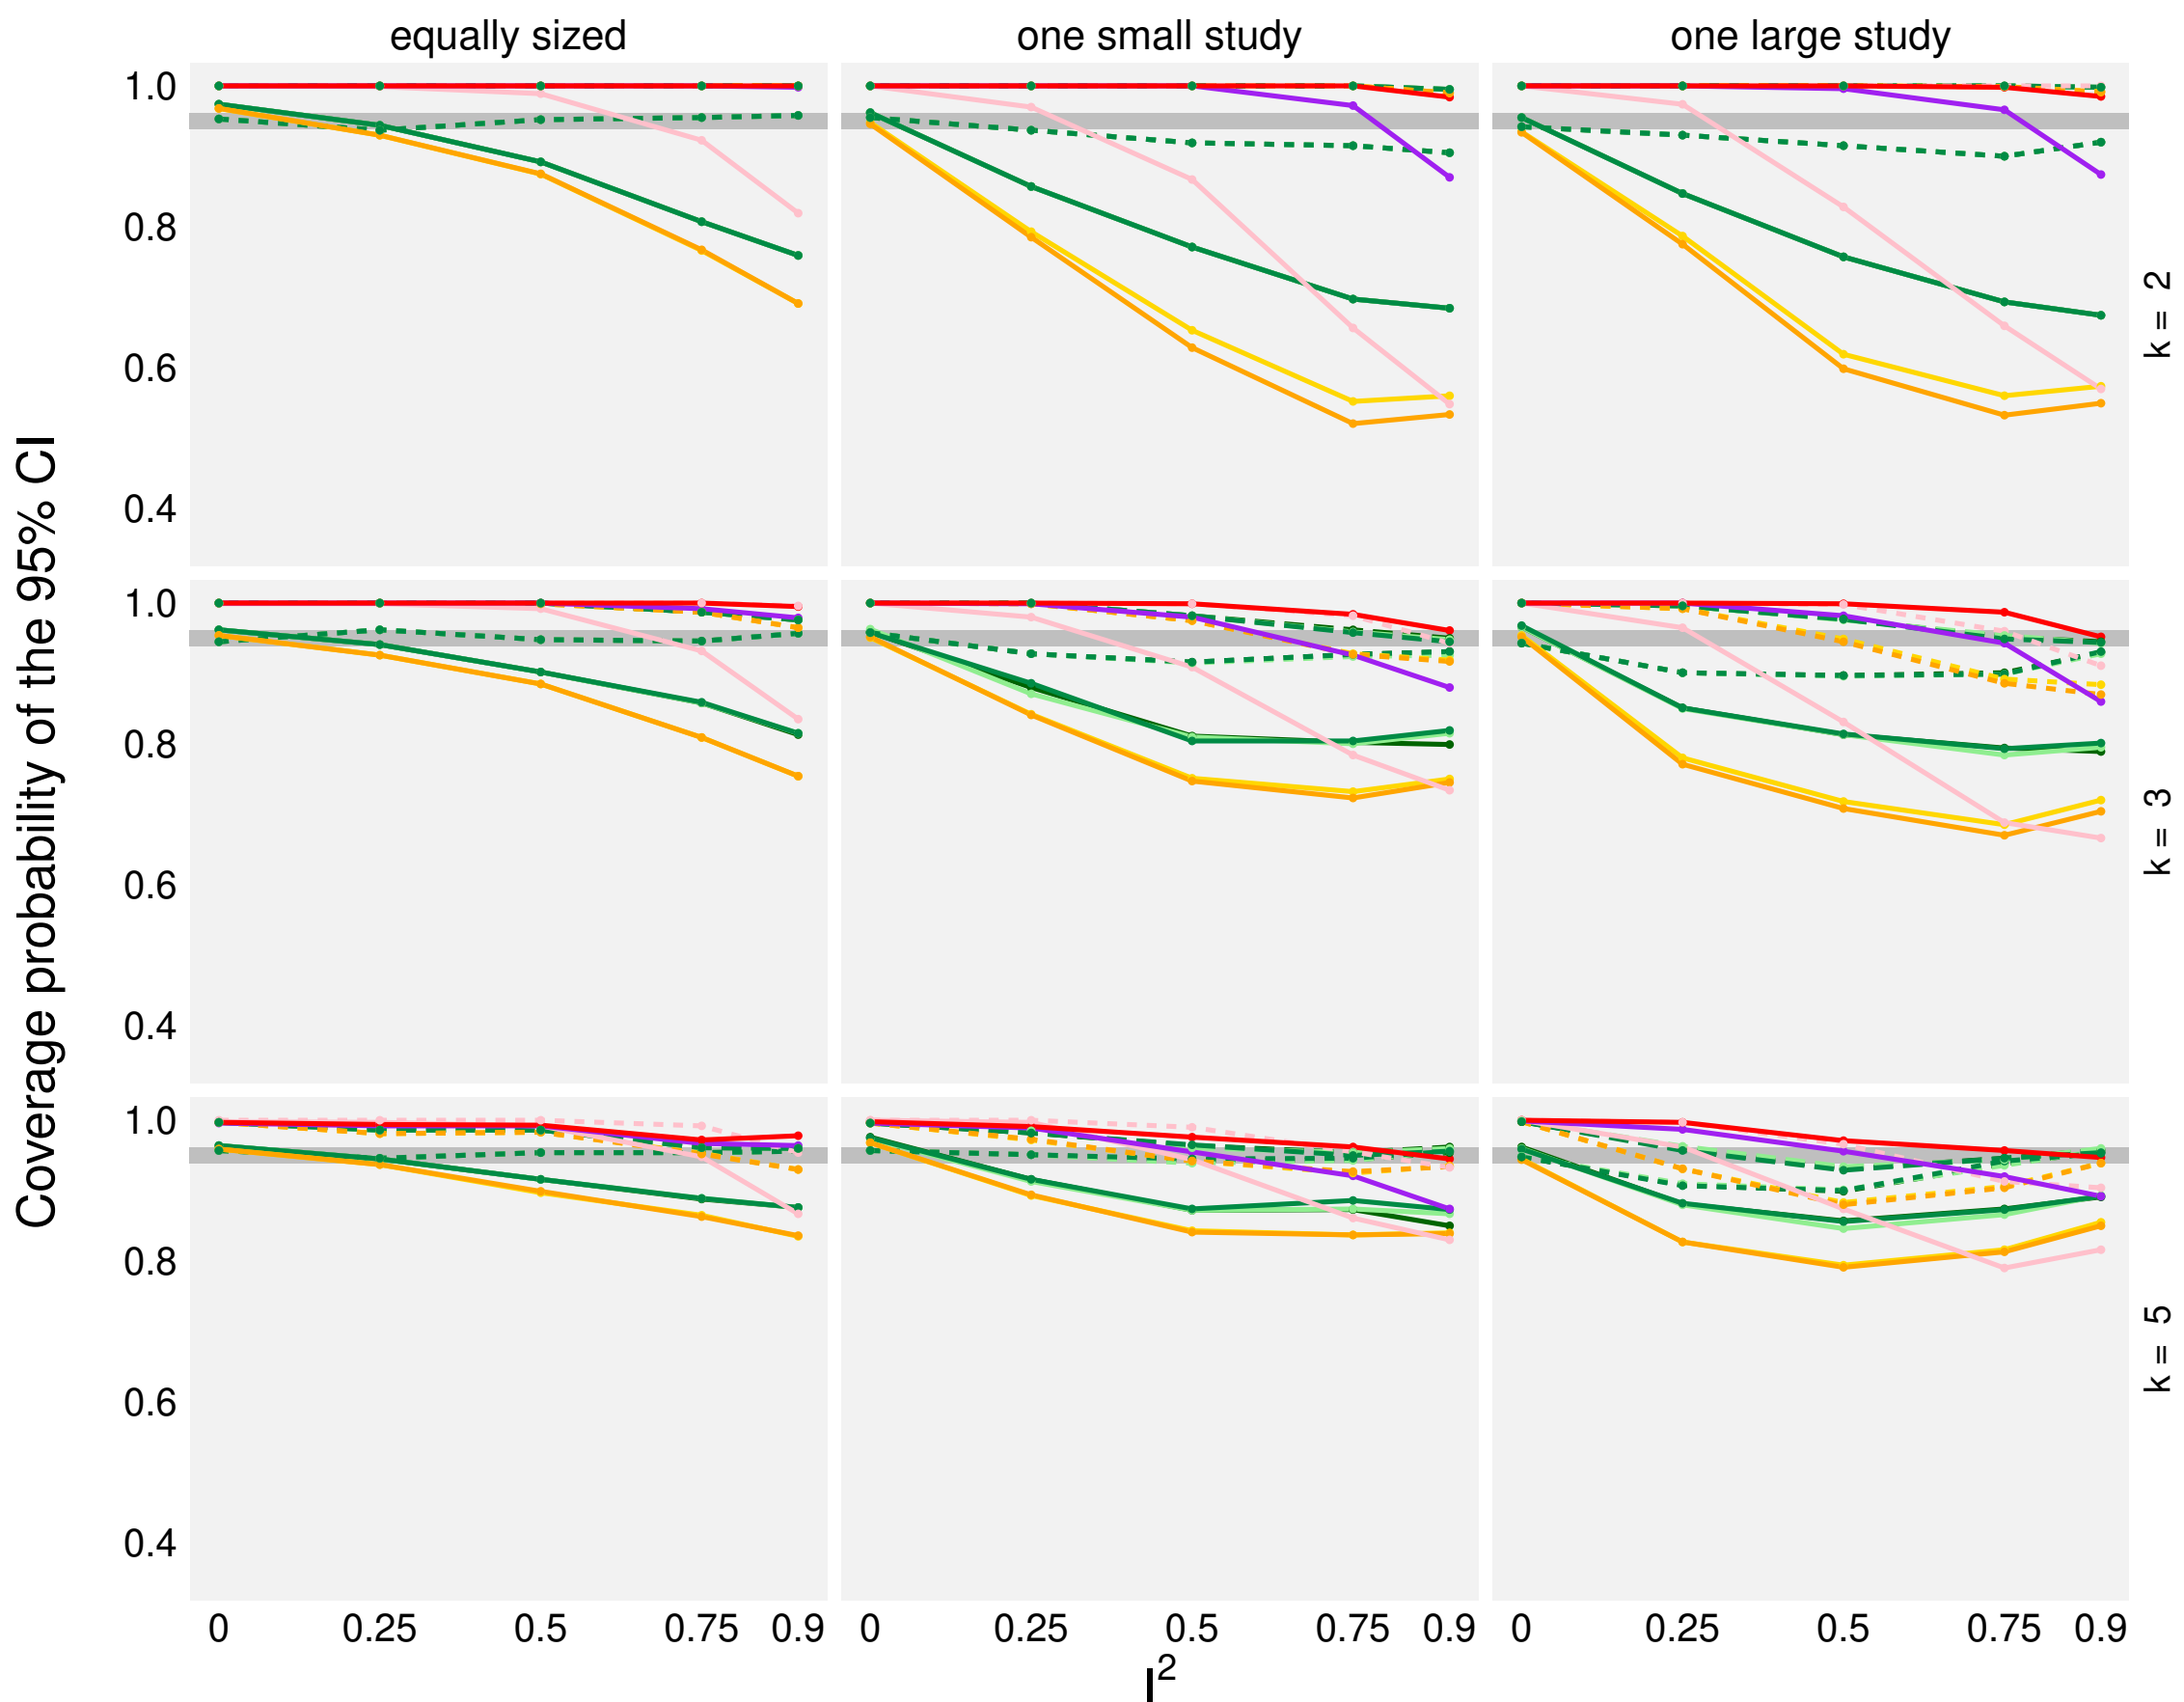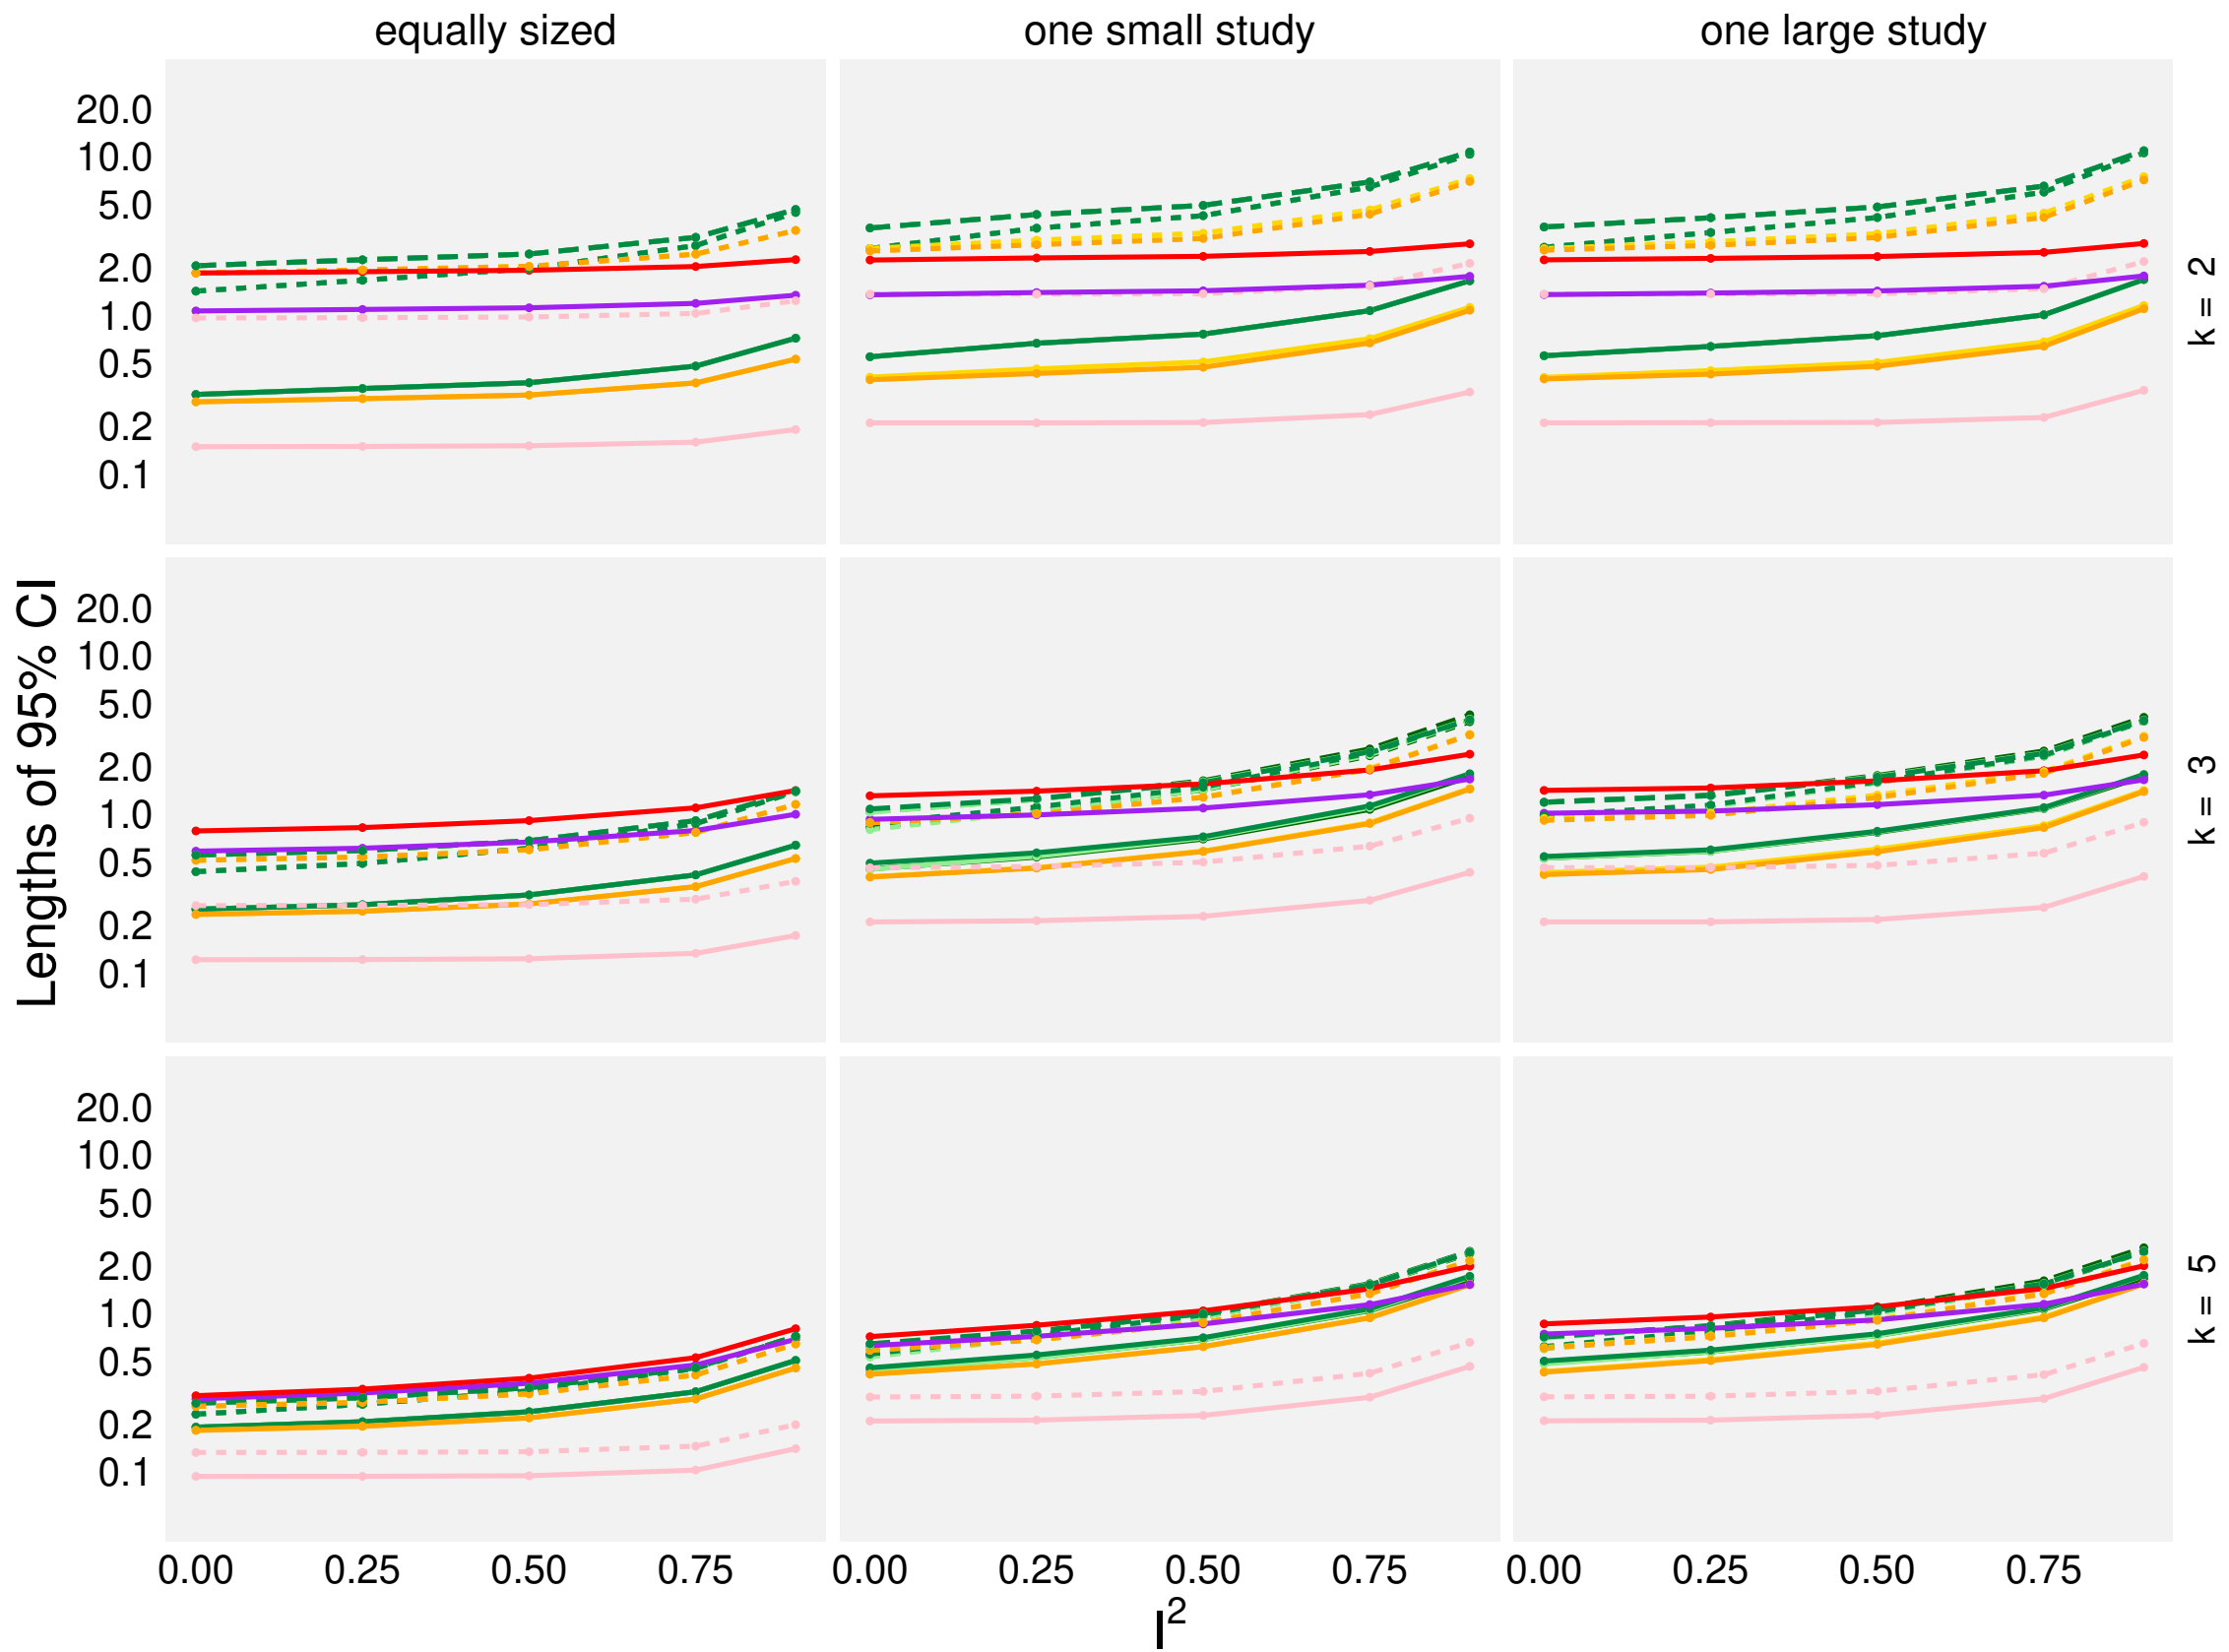

— NN — DL  
 — NN — REML  
 — NN — EB  
 — BN — UM.FS  
 — BN — UM.RS  
 — BN — CM.AL  
 — NN — Bayes HN(0.5)  
 — NN — Bayes HN(1)

— normal quantiles  
 - - HKSJ or Student's t  
 - · mHKSJ

OR  
( $n_i=1000, \pi_0=0.9$ )

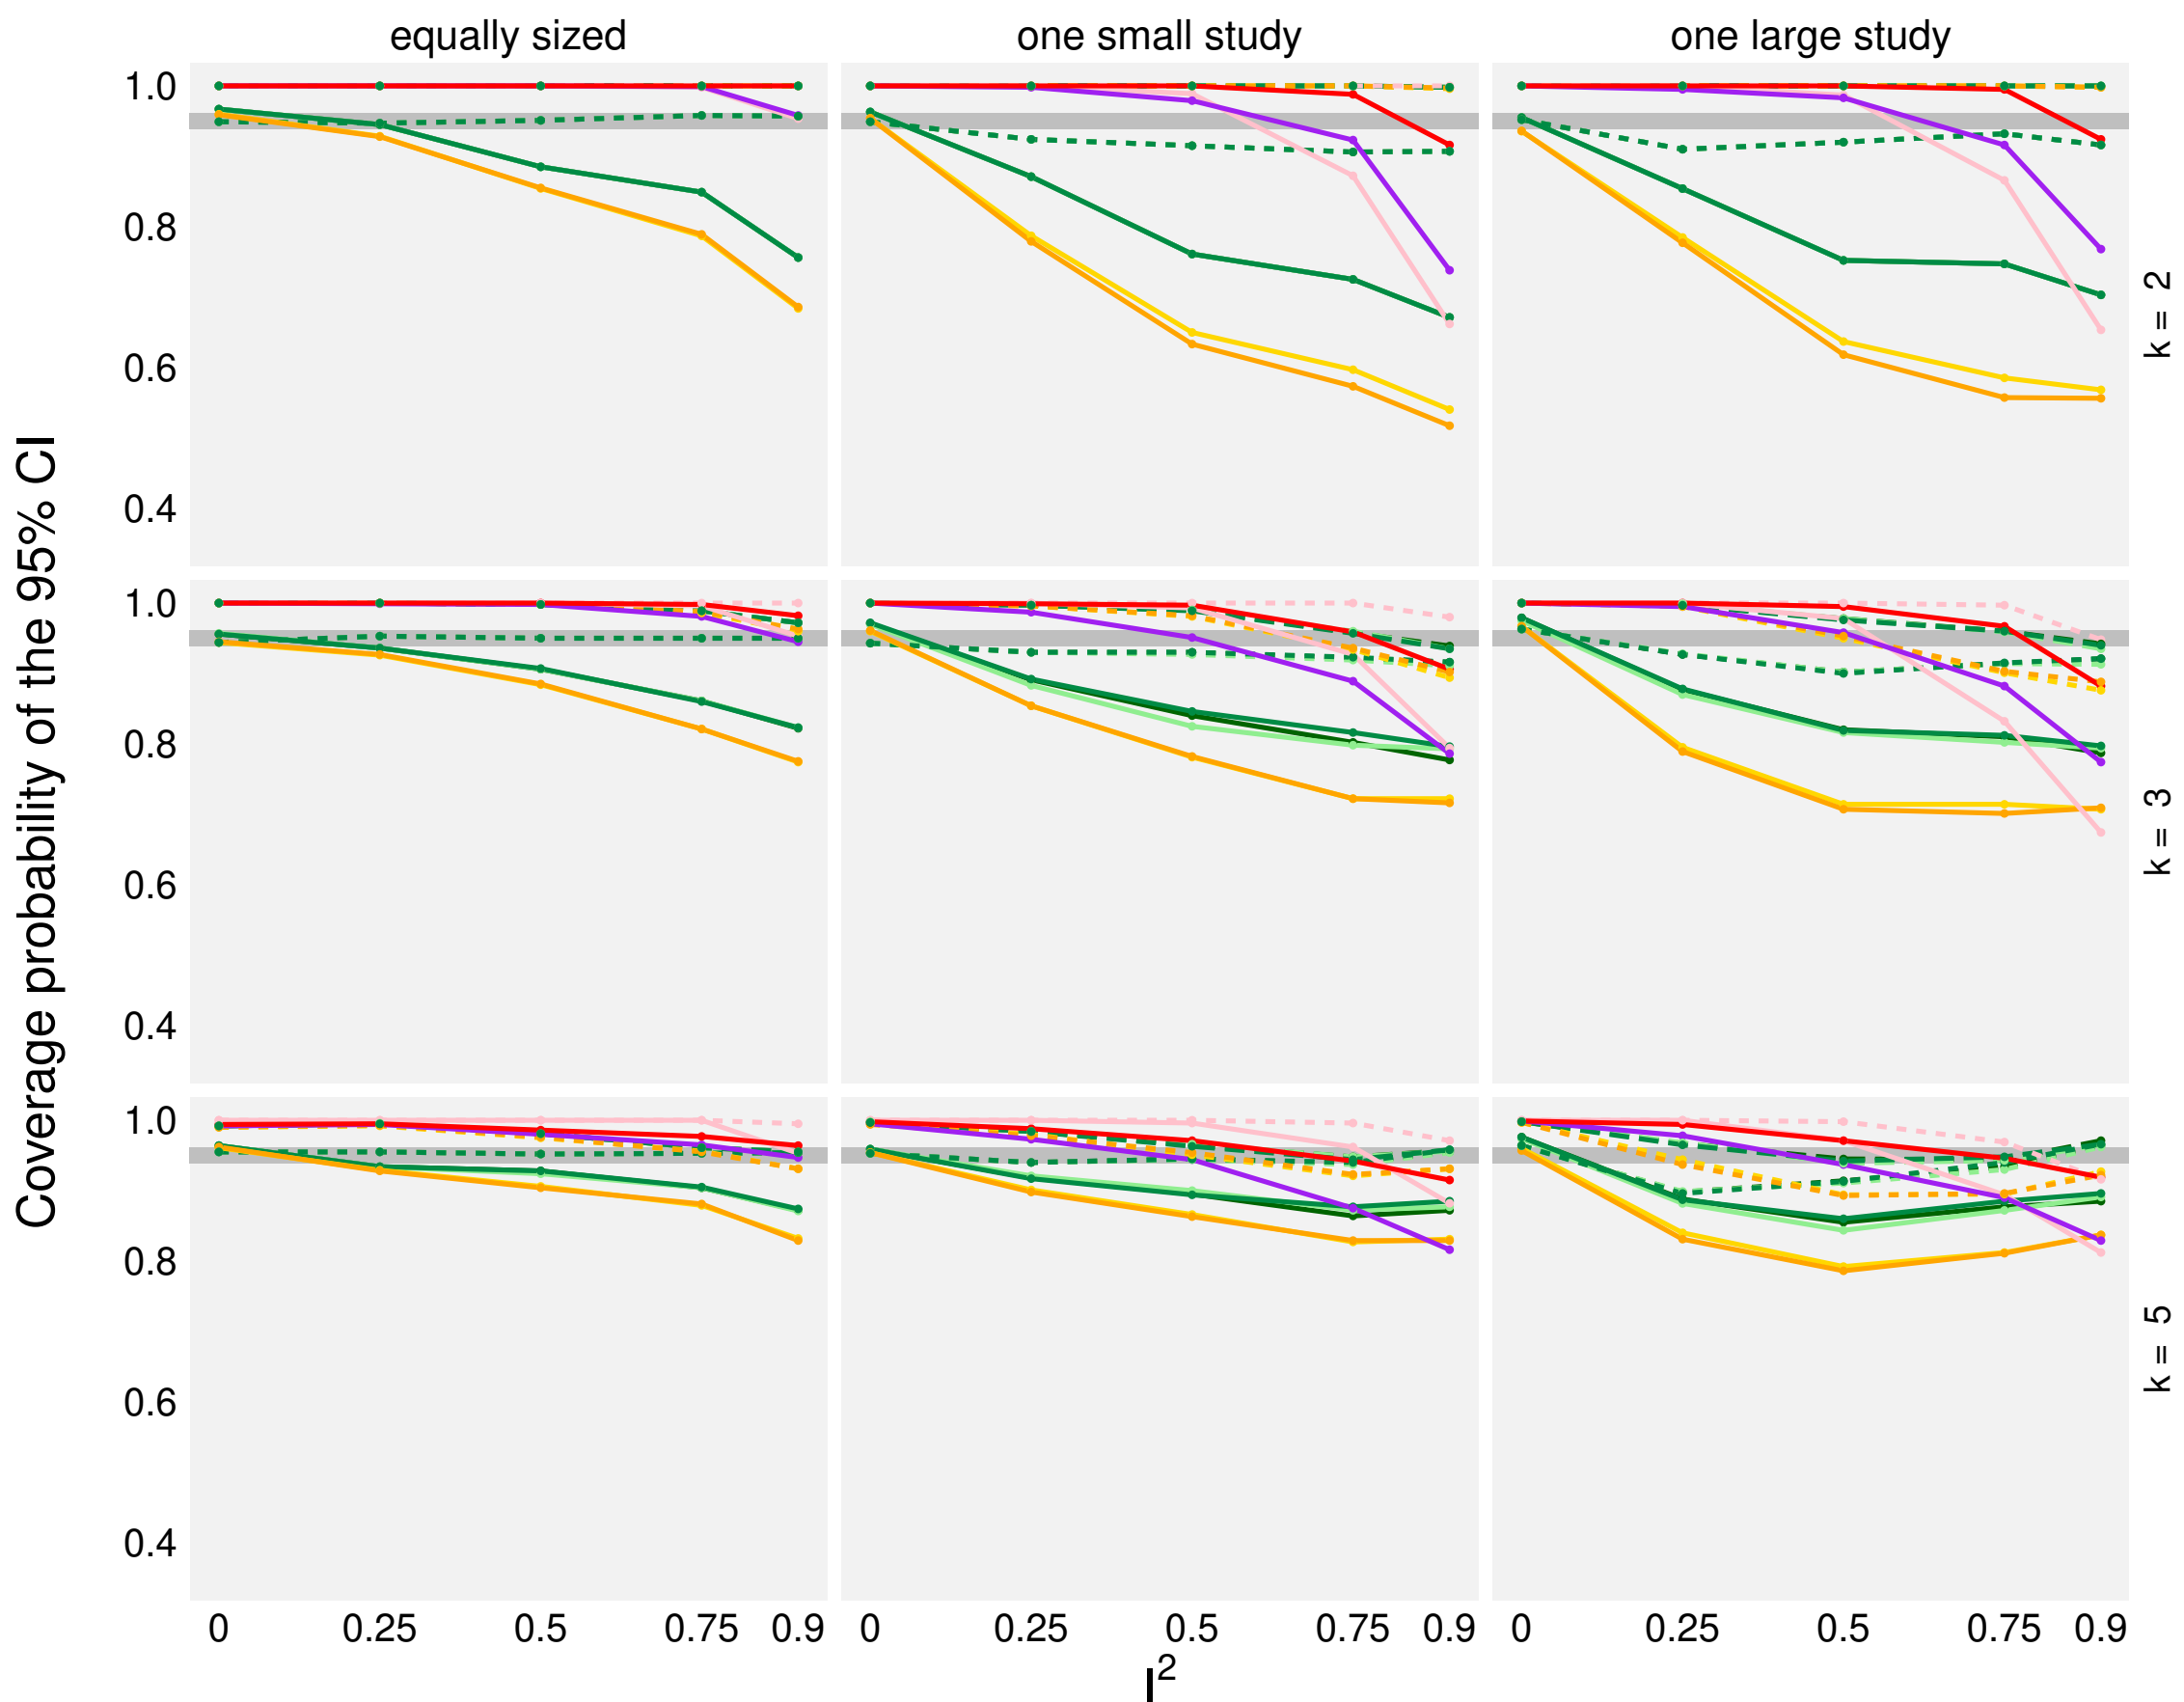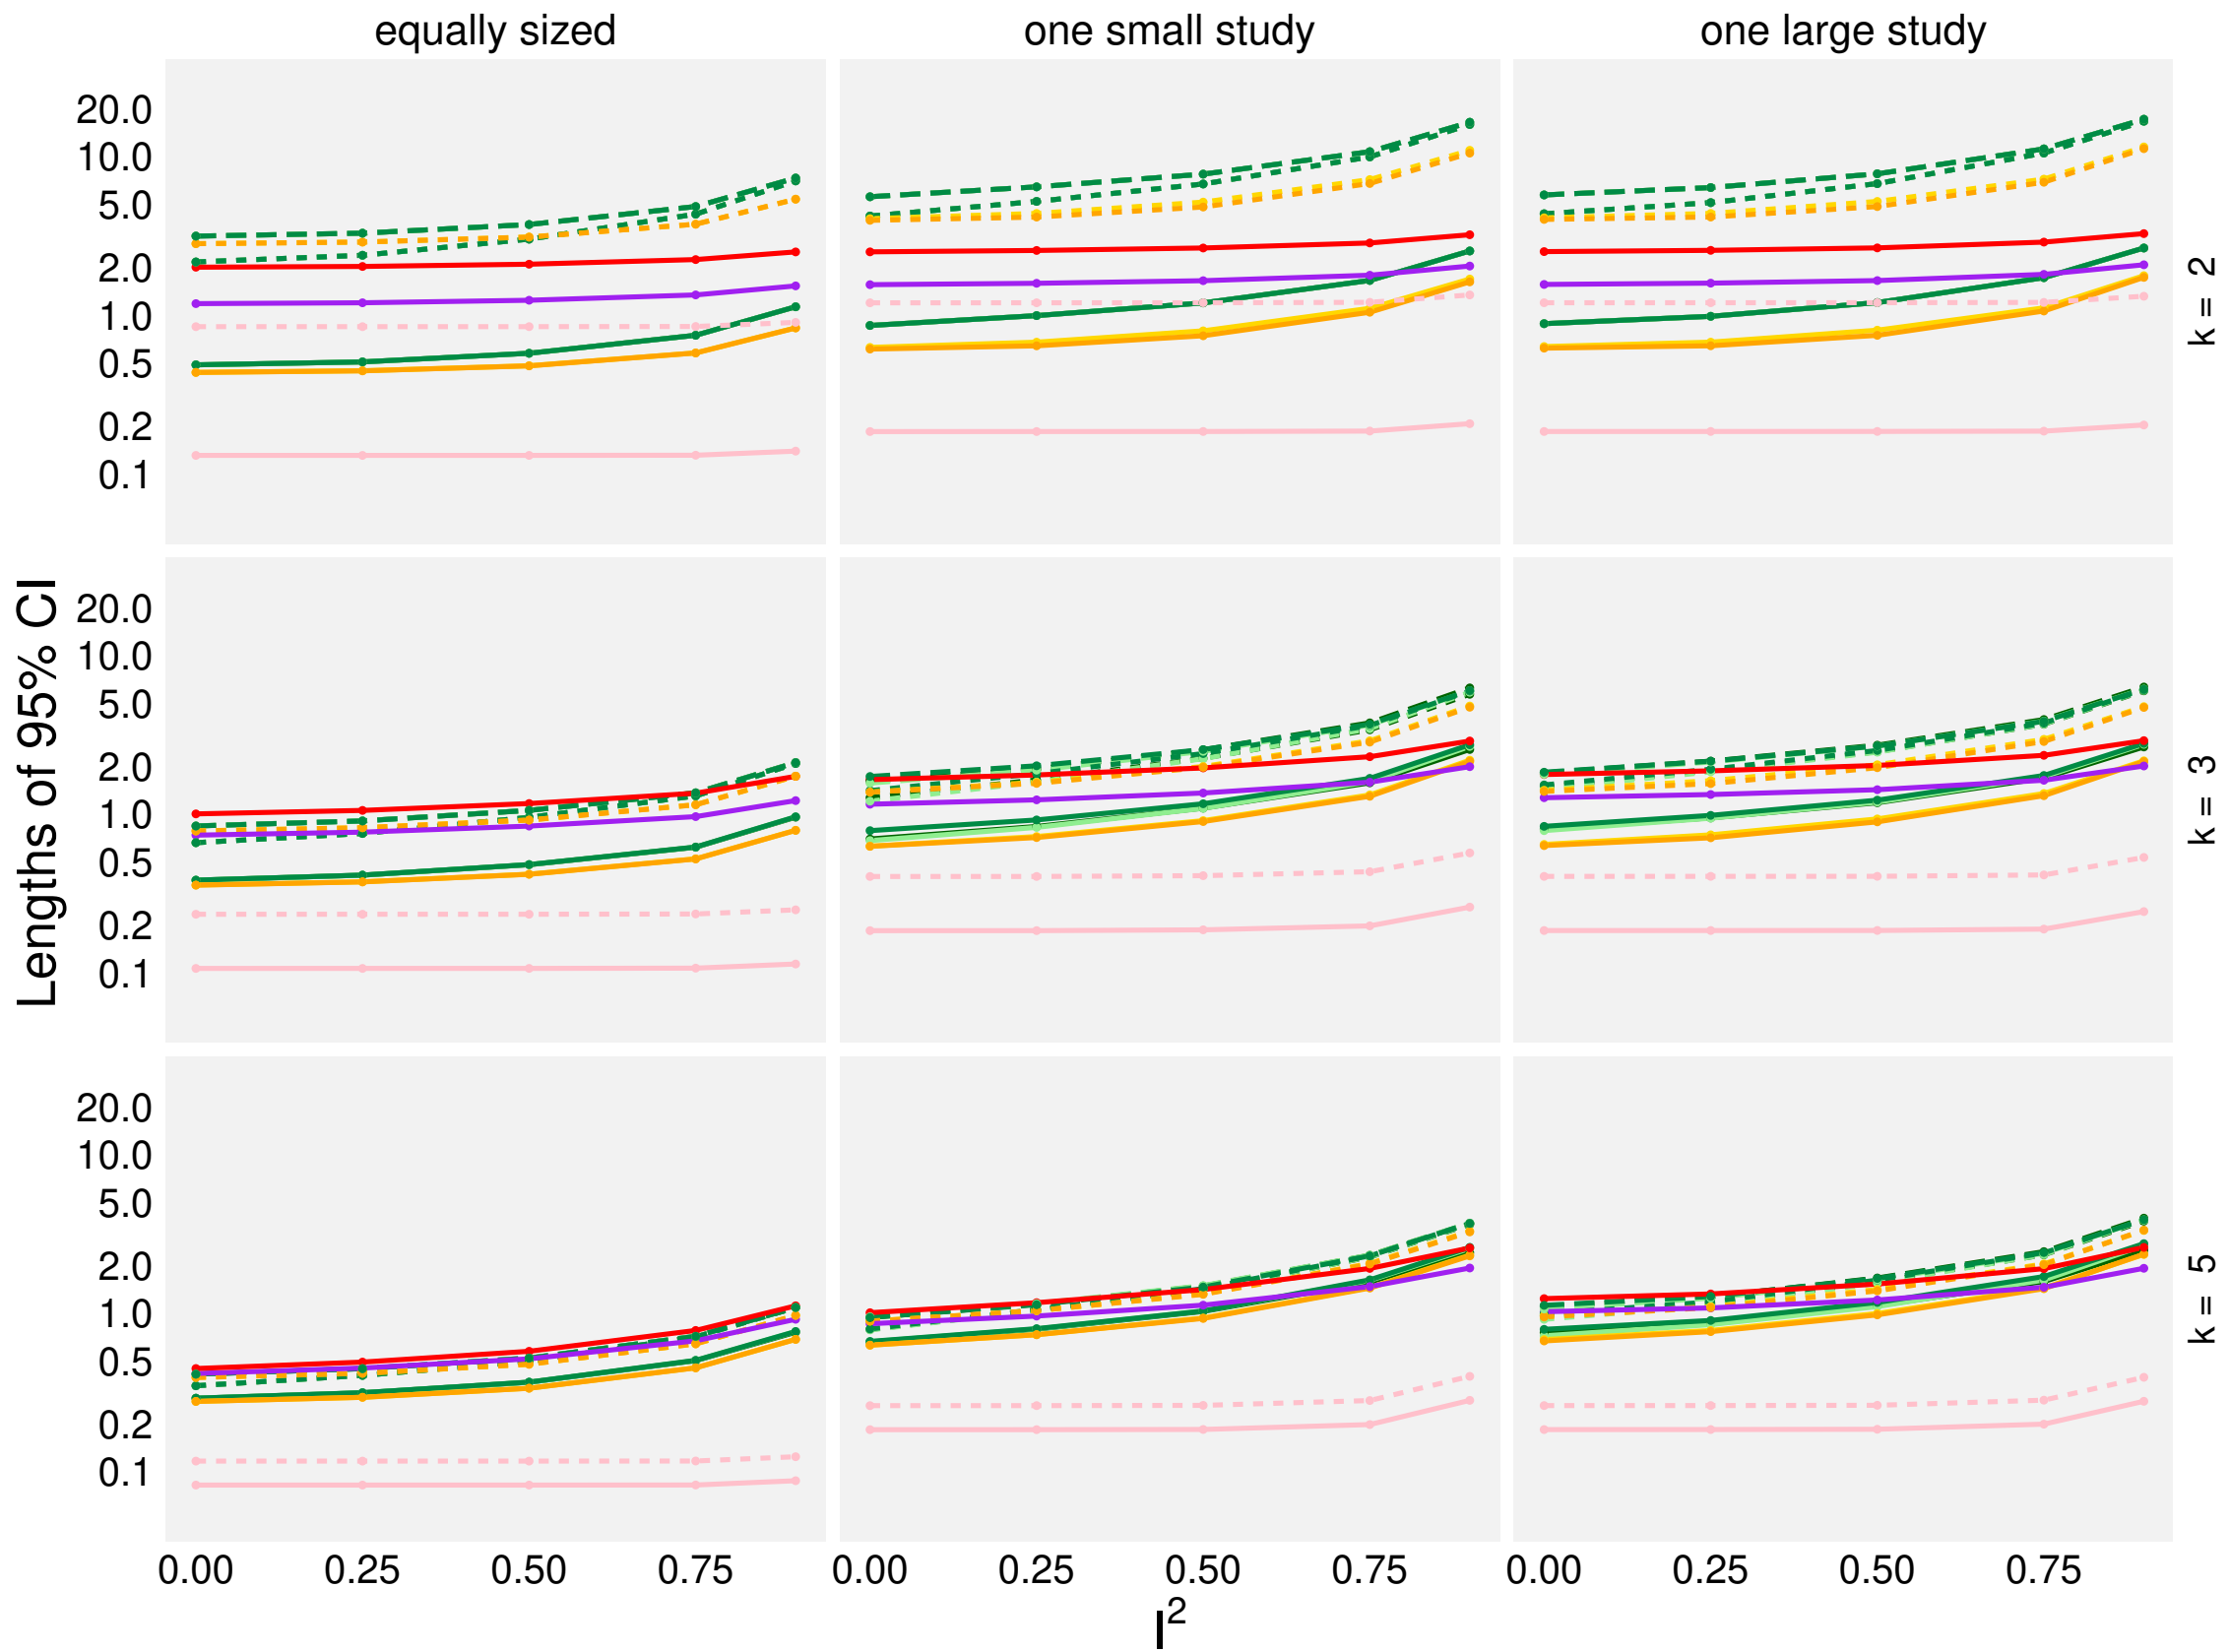

— NN — DL      — BN — UM.RS      — normal quantiles  
 — NN — REML      — BN — CM.AL      -- HKSJ or Student's t  
 — NN — EB      — NN — Bayes HN(0.5)      -- mHKSJ  
 — BN — UM.FS      — NN — Bayes HN(1)
